# Supplementary material for: A Complete Axiomatisation for Quantifier-Free Separation Logic
Source: arXiv:2006.05156 source file (2021-08-09)
Supplement: Supplementary file 1 [file appendix-dag-formula.tex]

\newpage 

\section{Derivation of the formula $\aformula_{\dag}$}
\label{appendix-dag-formula}

\noindent 
In this appendix, we explain how to derive the formula $\aformula_{\dag}$
introduced in the proof of Lemma~\ref{lemma:starPSLelim}. As the derivation is rather
complex, we provide it in the appendix with intermediate derivations. However, it mainly follows
the developments of a similar derivation in~\cite{Demri&Fervari&Mansutti19} with minor adjustments
as the axiom schemas related to the core formulae involving $\size$ are a bit different. 

We recall that the formula $\aformula_{\dag}$ is of the following form:

   $$
   \size \geq \inbound_1 \land \neg (\size \geq \inbound_2)
   \implies
   $$ 
   $$
   (\size \geq \inbound_1^1 \wedge \neg (\size \geq \inbound_2^1))
   \separate
    (\size \geq \inbound_1^2 \wedge \neg (\size \geq \inbound_2^2))   
   $$ 
   with the following provisos:
\begin{itemize}
\item $\inbound_2 > \inbound_1$, 
\item    $\inbound_1^1 < \inbound_2^1$ and  $\inbound_1^2 < \inbound_2^2$, 
\item $\inbound_1^1 + \inbound_1^2  \leq \inbound_1$, 
\item $\inbound_2^1 + \inbound_2^2 \dotminus 1 \geq \inbound_2$. 
\end{itemize}
Thanks to the presence of the intermediate axiom ~\ref{coreAx:Size}, we can restrict ourselves 
to the case $\inbound_1^1 + \inbound_1^2  = \inbound_1$ and $\inbound_2^1 + \inbound_2^2 \dotminus 1 = 
\inbound_2$.
Consequently, we just need to show the derivation of 
$$
\size \geq \inbound_1{+}\inbound_2 \land \lnot \size \geq (\inbound_1' {+} \inbound_2') {\dotminus} 1 \implies (\size \geq \inbound_1 \land \lnot \size \geq \inbound_1') \separate (\size \geq \inbound_2 \land \lnot \size \geq \inbound_2')
$$
with $0 \leq \inbound_1 < \inbound_1'$ and $0 \leq \inbound_2 < \inbound_2'$.

Below, we use the following admissible axiom schemas and inference rules from 
the propositional calculus (some of them have been already implicitly used in the body of the 
paper, some others have been explicitly introduced). 

\begin{multicols}{3}
\begin{enumerate}[align=left]
\item[\absaxlab{$\land$E}{pcax:andelim}] $\aformula \land \aformulabis \implies \aformula$
\item[\absaxlab{$\true$I}{pcax:trueintro}] $\aformula \iff \aformula \land \true$
\item[\absaxlab{$\true$S}{pcax:truesub}] $\true \iff \aformula \lor \lnot \aformula$
\item[\absaxlab{$\false$I}{pcax:falseintro}] $\false \implies \aformula$
\item[\absaxlab{$\land$C}{pcax:command}] $\aformula \land \aformulabis \implies \aformulabis \land \aformula$
\item[\absaxlab{$\land\lor$}{pcax:distand}]
  $\begin{aligned}[t]
    &\aformula \land (\aformulabis \lor \aformulater) \implies\\ &
    (\aformula \land \aformulabis) \lor (\aformula \land \aformulater)
  \end{aligned}$
\item[\absaxlab{${\land}$I}{pcrule:andWR}] $\inference{\aformulabis \implies \aformulater}{\aformula \land \aformulabis \implies \aformula \land \aformulater}$
\item[\absaxlab{$\Rightarrow$T}{pcrule:imptrans}] $\inference{\aformula \implies \aformulabis \quad \aformulabis \implies \aformulater }{\aformula \implies \aformulater}$
\item[\absaxlab{${\land}$R}{pcrule:andR}] $\inference{\aformula \implies \aformulabis \quad \aformula \implies \aformulater}{\aformula \implies \aformulabis \land \aformulater}$
\end{enumerate}
\end{multicols}

Before deriving $\aformula_{\dag}$, we shall establish the admissibility of the following axiom schemas
and inference rules. Some of them are easy to show or have been already considered but for the sake of being
rather self-contained in the appendix, we provide a bit more details here.

\begin{lem}\label{lemma:auxiliary-lemmas} \ 
\begin{enumerate}[label=\textbf{R\arabic*}]
\setcounter{enumi}{-1}
\item\label{SC-auxlemmaR0bis} Let $\aformula, \aformula'$ and $\aformulabis$ be
formulae built from core formulae, and using Boolean connectives and the separating conjunction $\separate$ such that
$\prove_{\starsys} \aformula \iff \aformula'$. Then,
$\prove_{\starsys}  \aformulabis[\aformula]_{\rho} \iff
\aformulabis[\aformula']_{\rho}$.
\end{enumerate}
The following formulae are derivable in  $\starsys$.
\begin{enumerate}[label=\textbf{L\arabic*}]
\setcounter{enumi}{-1}
\item\label{SC-auxlemmareal0}  $(\aformula \land \aformula') \separate (\aformulabis \land \aformulabis') \implies \aformula \separate \aformulabis$.
\item\label{SC-auxlemma0} $\size \geq \inbound_1 \separate \size \geq \inbound_2 \iff \size \geq \inbound_1 + \inbound_2$.
\item\label{SC-auxS5} $\size \geq \inbound_1 + \inbound_2 \implies (\size = \inbound_1) \separate \size \geq
\inbound_2$. 
\item\label{SC-auxlemma2} $((\aformula \land \size \geq \inbound ) \separate \aformulabis) \land \lnot \size \geq \inbound' \implies (\aformula \land \size \geq \inbound) \separate(\aformulabis \land \lnot \size \geq \inbound'{\dotminus}\inbound)$.
\item\label{SC-auxlemma3} $((\aformula \land \lnot \size \geq \inbound{+}1) \separate \aformulabis) \land \size \geq \inbound' \implies (\aformula \land \lnot \size \geq \inbound{+}1) \separate(\aformulabis \land \size \geq \inbound'{\dotminus}\inbound)$.
\end{enumerate}

\end{lem}

\begin{proof} \
\begin{itemize}
\item Proof of \ref{SC-auxlemmaR0bis}. This is exactly~\ref{SC-auxlemmaR0}
from the proof of Theorem~\ref{theo:starCompleteness}.
\item Proof of~\ref{SC-auxlemmareal0}. This is a direct consequence of the admissibility
of the inference rule~\ref{rule:starintroLR} (see Section~\ref{section:PSL}) and the axiom~\ref{pcax:andelim}. 
\item Proof of~\ref{SC-auxlemma0}. When $\inbound_1, \inbound_2 \geq 1$, this is a direct consequence
of the definition of the core formulae of the form $\size \geq \inbound$. 
Otherwise, $\size \geq 0$ is equal to $\top$, and 
we get the derivation thanks to the axiom~\ref{starAx:MonoCore}, and possibly the axiom~\ref{starAx:Commute}
for commutativity of the separating conjunction $\separate$. 
\item Proof of \ref{SC-auxS5}. Let us prove it by induction on $\inbound_1$. 
Here is the derivation for $\inbound_1 = 0$.
$$
\begin{array}{l|ll}
1 & (\size \geq \inbound_2) \implies \emp \separate (\size \geq \inbound_2)
& \mbox{\ref{starAx:Emp}} \\
2 & \emp \implies \lnot (\size \geq 1) \land \size \geq 0
& \mbox{Def. $\size$} \\
3 & \emp \separate (\size \geq \inbound_2)
    \implies
    (\size = 0) \separate  (\size \geq \inbound_2)
& \mbox{\ref{rule:starintroLR}, 2 + Def. $\size = 0$} \\
4 &  (\size \geq \inbound_2) \implies  (\size = 0) \separate  (\size \geq \inbound_2)
& \mbox{\ref{rule:imptr}, 1, 3}
\end{array}
$$
For the induction step, let us suppose that the property holds for $\inbound_1$ and let us
prove that it holds also for $\inbound_1+1$. 
$$
\begin{array}{l|ll}
1 & (\size \geq \inbound_1 + 1) \separate (\size \geq \inbound_2)
    \implies \\
&  (\size \geq 1) \separate ((\size \geq \inbound_1) \separate (\size \geq \inbound_2))
& \mbox{Def. $\size$, \ref{starAx:Commute}, \ref{starAx:Assoc}} \\
2 &   (\size \geq \inbound_1) \separate (\size \geq \inbound_2) \implies
      (\size \geq \inbound_1 + \inbound_2)
& \mbox{\ref{SC-auxlemma0}} \\
3 &  (\size \geq 1) \implies (\size = 1) \separate \top
& \mbox{\ref{starAx:SizeOne} + Def. $\size$} \\
4 & (\size \geq \inbound_1 + 1) \separate (\size \geq \inbound_2)
     \implies \\
& ((\size = 1) \separate \top) \separate (\size \geq \inbound_1 + \inbound_2)
& \mbox{\ref{rule:starintroLR}, 2, 3 + \ref{rule:imptr}} \\ 
%% 4 & (\size = 1) \separate \top \implies \size \geq 1 \separate \top
%% & \mbox{\ref{rule:starintroLR} + Def. $\size = 1$} \\
%% 5 & \size \geq 1 \separate \top \implies \size \geq 1  
%% & \mbox{\ref{starAx:MonoCore} + Def. $\size \geq 1$} \\
5 & \top \separate (\size \geq \inbound_1 + \inbound_2)
    \implies  (\size \geq \inbound_1 + \inbound_2) 
& \mbox{\ref{SC-auxlemma0}} \\
6 &  (\size \geq \inbound_1 + 1) \separate (\size \geq \inbound_2)
     \implies \\
& (\size = 1) \separate (\size \geq \inbound_1 + \inbound_2)
& \mbox{\ref{starAx:Commute}, \ref{starAx:Assoc} + \ref{rule:imptr}, 4 + \ref{rule:starintroLR}}\\
7 & (\size \geq \inbound_1 + 1) \separate (\size \geq \inbound_2) \implies\\
&    (\size = 1) \separate (\size = \inbound_1) \separate (\size \geq \inbound_2)
& \mbox{Ind. hypothesis, \ref{rule:starintroLR}, 6} \\
8 & (\size = 1) \separate (\size = \inbound_1) \implies \size \geq \inbound_1 +1 
& \mbox{Def. $\size$,  \ref{rule:starintroLR}} \\
9 & (\size = 1) \separate (\size = \inbound_1) \implies \neg (\size \geq \inbound_1 +2) 
& \mbox{Def. $\size$, \ref{rule:starintroLR} 8,  \ref{starAx:SizeNeg}} \\
10 &  (\size = 1) \separate (\size = \inbound_1) \implies  (\size = \inbound_1 +1)
& \mbox{Def. $\size$, prop. reasoning} \\
11 &   (\size \geq \inbound_1 + 1) \separate (\size \geq \inbound_2) \implies
    (\size = \inbound_1 +1) \separate (\size \geq \inbound_2)
& \mbox{\ref{rule:starintroLR}, 10 + \ref{rule:imptr}, 7} 
\end{array} 
$$
\item Proof of~\ref{SC-auxlemma2}.  Below, we write $\widehat{\aformulater}$ to denote
the following formula:
$$
  ((\aformula \land \size \geq \inbound) \separate (\aformulabis \land \size \geq \inbound'{\dotminus}\inbound) )
\lor ((\aformula \land \size \geq \inbound) \separate (\aformulabis \land \lnot \size \geq 
\inbound'{\dotminus}\inbound)).
$$
Here is the first part of the derivation:
$$
\begin{array}{l|ll}
1 &  \aformulabis \implies \aformulabis \land (\size \geq \inbound'{\dotminus}\inbound \lor \lnot 
      \size \geq \inbound'{\dotminus}\inbound)
& \mbox{\ref{pcax:trueintro} and \ref{pcax:truesub}} \\ 
2 & (\aformula \land \size \geq \inbound) \separate \aformulabis \implies\\
&  (\aformula \land \size \geq \inbound) \separate (\aformulabis \land (\size \geq \inbound'{\dotminus}
    \inbound \lor \lnot \size \geq \inbound'{\dotminus}\inbound))
& \mbox{\ref{rule:starinference} and \ref{starAx:Commute}, 1} \\
3 & (\aformula \land \size \geq \inbound) \separate (\aformulabis \land (\size \geq \inbound'{\dotminus}
     \inbound \lor \lnot \size \geq \inbound'{\dotminus}\inbound)) \implies \widehat{\aformulater}
& \mbox{\ref{pcax:distand} and \ref{starAx:DistrOr}} \\ 
4 & (\aformula \land \size \geq \inbound) \separate \aformulabis \implies \widehat{\aformulater}
& \mbox{\ref{pcrule:imptrans}, 2, 3} \\
5 & ((\aformula \land \size \geq \inbound) \separate \aformulabis) \land \lnot \size \geq \inbound' \implies \widehat{\aformulater} \land \lnot \size \geq \inbound'
& \mbox{\ref{pcrule:andWR} and \ref{pcax:command}, 4} \\
6 & \widehat{\aformulater} \land \lnot \size \geq \inbound' \implies\\
& (((\aformula \land \size \geq \inbound) \separate (\aformulabis \land \size \geq 
\inbound'{\dotminus}\inbound)) \land \lnot \size \geq \inbound') \lor\\
&          (((\aformula \land \size \geq \inbound) \separate (\aformulabis \land \lnot \size \geq 
\inbound'{\dotminus}\inbound)) \land \lnot \size \geq \inbound')
& \mbox{\ref{pcax:distand} and \ref{pcax:command}}
\end{array}
$$ 
Below, we write $\widetilde{\aformulater}$ to denote the following formula:
$$
(((\aformula \land \size \geq \inbound) \separate (\aformulabis \land \size \geq \inbound'{\dotminus}\inbound)) \land \lnot \size \geq \inbound') \lor
(((\aformula \land \size \geq \inbound) \separate (\aformulabis \land \lnot \size \geq \inbound'{\dotminus}\inbound)) \land \lnot \size \geq \inbound').
$$
Here is the remaining part of the derivation.
$$
\begin{array}{l|ll}
7 & ((\aformula \land \size \geq \inbound) \separate \aformulabis) \land \lnot \size \geq \inbound' \implies \widetilde{\aformulater}
& \mbox{\ref{pcrule:imptrans}, 5, 6} \\
8 & ((\aformula \land \size \geq \inbound) \separate (\aformulabis \land \size \geq 
\inbound'{\dotminus}\inbound)) \implies \size \geq \inbound \separate \size \geq 
\inbound'{\dotminus}\inbound 
& \mbox{\ref{SC-auxlemmareal0}} \\
9 & \size \geq \inbound \separate \size \geq \inbound'{\dotminus}\inbound \implies 
  \size \geq \max(\inbound,\inbound')
& \mbox{\ref{SC-auxlemma0}} \\
10 & ((\aformula \land \size \geq \inbound) \separate (\aformulabis \land \size \geq 
     \inbound'{\dotminus}\inbound)) \implies
          \size \geq \max(\inbound,\inbound')
& \mbox{\ref{pcrule:imptrans}, 8, 9} \\
11 & \size \geq \max(\inbound,\inbound') \implies \size \geq \inbound' 
& \mbox{repeated \ref{coreAx:Size} + \ref{pcrule:imptrans}} \\
12 & ((\aformula \land \size \geq \inbound) \separate (\aformulabis \land \size \geq 
\inbound'{\dotminus}\inbound)) \implies \size \geq \inbound' 
& \mbox{\ref{pcrule:imptrans}, 10, 11} \\
13 & ((\aformula \land \size \geq \inbound) \separate (\aformulabis \land \size \geq
 \inbound'{\dotminus}\inbound)) \land \lnot \size \geq \inbound' \implies\\
& \size \geq \inbound' \land \lnot \size \geq \inbound'
& \mbox{\ref{pcrule:andWR} and \ref{pcax:command}, 12} \\ 
14 & \size \geq \inbound' \land \lnot \size \geq \inbound' \iff \false
& \mbox{\ref{pcax:truesub} and Def. $\true$} \\
15 & ((\aformula \land \size \geq \inbound) \separate (\aformulabis \land \size 
\geq \inbound'{\dotminus}\inbound)) \land \lnot \size \geq \inbound' \iff \false
& \mbox{\ref{pcrule:imptrans} and~\ref{pcax:falseintro}, 14, 15} \\ 
16 & ((\aformula \land \size \geq \inbound) \separate \aformulabis) \land \lnot \size 
\geq \inbound' \implies\\
& \false \lor ((\aformula \land \size \geq \inbound) \separate (\aformulabis \land \lnot \size 
\geq \inbound'{\dotminus}\inbound) \land \lnot \size \geq \inbound')
& \mbox{\ref{SC-auxlemmaR0}, 7, 15} \\ 
17 &  \false \lor ((\aformula \land \size \geq \inbound) \separate (\aformulabis \land \lnot \size \geq 
\inbound'{\dotminus}\inbound) \land \lnot \size \geq \inbound')
    \implies\\ 
& (\aformula \land \size \geq \inbound) \separate (\aformulabis \land \lnot \size \geq
 \inbound'{\dotminus}\inbound)
& \mbox{Prop. reasoning} \\ 
18 & ((\aformula \land \size \geq \inbound) \separate \aformulabis) \land \lnot \size \geq 
\inbound' \implies\\
& (\aformula \land \size \geq \inbound) \separate (\aformulabis \land \lnot \size 
\geq \inbound'{\dotminus}\inbound)
& \mbox{\ref{pcrule:imptrans}, 16, 17}
\end{array}
$$ 

\item Proof of~\ref{SC-auxlemma3}. 
The proof is similar to the previous one. Let $\widehat{\aformulater}$ be the formula
below:
$$
  ((\aformula \land \lnot \size \geq \inbound{+}1) \separate (\aformulabis \land \size \geq \inbound'{\dotminus}\inbound) )
\lor ((\aformula \land \lnot \size \geq \inbound{+}1) \separate (\aformulabis \land \lnot \size \geq \inbound'{\dotminus}\inbound)).
$$
Here is the beginning of the derivation.
$$
\begin{array}{l|ll}
1 & \aformulabis \implies \aformulabis \land (\size \geq \inbound'{\dotminus}\inbound \lor \lnot \size \geq \inbound'{\dotminus}\inbound)
& \mbox{\ref{pcax:trueintro} and \ref{pcax:truesub}} \\
2 & (\aformula \land \lnot \size \geq \inbound{+}1) \separate \aformulabis \implies\\
&          (\aformula \land \lnot \size \geq \inbound{+}1) \separate (\aformulabis \land 
(\size \geq \inbound'{\dotminus}\inbound \lor \lnot \size \geq \inbound'{\dotminus}\inbound))
& \mbox{\ref{rule:starinference} and \ref{starAx:Commute}, 1} \\ 
3 &  (\aformula \land \lnot \size \geq \inbound{+}1) \separate (\aformulabis \land 
(\size \geq \inbound'{\dotminus}\inbound \lor \lnot \size \geq \inbound'{\dotminus}\inbound)) \implies 
\widehat{\aformulater}
& \mbox{\ref{pcax:distand} and \ref{starAx:DistrOr}} \\ 
4 & (\aformula \land \lnot\size \geq \inbound{+}1) \separate \aformulabis \implies \widehat{\aformulater}
& \mbox{\ref{pcrule:imptrans}, 2, 3} \\
5 & ((\aformula \land \lnot \size \geq \inbound{+}1) \separate \aformulabis) \land \size \geq \inbound' \implies \widehat{\aformulater} \land \size \geq \inbound'
& \mbox{\ref{pcrule:andWR} and \ref{pcax:command}, 4} \\
6 & \widehat{\aformulater} \land \size \geq \inbound' \implies\\
& (((\aformula \land \lnot \size \geq \inbound{+}1) \separate (\aformulabis \land \size \geq 
\inbound'{\dotminus}\inbound)) \land \size \geq \inbound') \lor\\
& (((\aformula \land \lnot \size \geq \inbound{+}1) \separate (\aformulabis \land \lnot \size \geq 
\inbound'{\dotminus}\inbound)) \land \size \geq \inbound')
& \mbox{\ref{pcax:distand} and \ref{pcax:command}}
\end{array}
$$
Below, we write $\widetilde{\aformulater}$ to denote the following formula: 
$$
  (((\aformula \land \lnot \size \geq \inbound{+}1) \separate (\aformulabis \land \size \geq
 \inbound'{\dotminus}\inbound)) \land \size \geq \inbound') \lor
$$
$$
  (((\aformula \land \lnot \size \geq \inbound{+}1) \separate (\aformulabis \land \lnot 
\size \geq \inbound'{\dotminus}\inbound)) \land \size \geq \inbound')
$$
Here is the continuation of the derivation.
$$
\begin{array}{l|ll}
7 & ((\aformula \land \lnot \size \geq \inbound{+}1) \separate \aformulabis) \land \size \geq \inbound' \implies \widetilde{\aformulater} 
& \mbox{\ref{pcrule:imptrans}, 5, 6} \\
8 & ((\aformula \land \lnot \size \geq \inbound{+}1) \separate (\aformulabis \land \lnot \size \geq \inbound'{\dotminus}\inbound)) \implies \\
&  \lnot \size \geq \inbound{+}1 \separate \lnot \size \geq \inbound'{\dotminus}\inbound
& \mbox{\ref{SC-auxlemmareal0}} 
\end{array}
$$
We now prove that $\prove_{\starsys} \lnot \size \geq \inbound{+}1 \separate \lnot \size \geq \inbound'{\dotminus}\inbound \implies \lnot \size \geq \inbound'$ by performing a case analysis depending on
the satisfaction of the condition  $\inbound' \leq \inbound$. If $\inbound' \leq \inbound$ then
$\inbound'{\dotminus}\inbound = 0$ and therefore we get the following derivation. 
$$
\begin{array}{l|ll}
9 & \lnot \size \geq 0 \iff \false
& \mbox{Def. of $\size$ + prop. reasoning} \\
10 &  \lnot \size \geq \inbound{+}1 \separate \lnot \size \geq 0 \implies \lnot \size \geq \inbound{+}1 
\separate \false
& \mbox{\ref{rule:starinference} and \ref{starAx:Commute}, 9} \\
11 & \lnot \size \geq \inbound{+}1 \separate \false \implies \false
& \mbox{\ref{starAx:False}} \\
12 &  \lnot \size \geq \inbound{+}1 \separate \lnot \size \geq 0 \implies \false
& \mbox{\ref{pcrule:imptrans} 10, 11} \\
13 & \false \implies \lnot \size \geq \inbound'
& \mbox{\ref{pcax:falseintro}} \\
14 & \lnot \size \geq \inbound{+}1 \separate \lnot \size \geq \inbound'{\dotminus}\inbound \implies 
\lnot \size \geq \inbound'
& \mbox{\ref{pcrule:imptrans}, 12, 13}
\end{array}
$$

If instead $\inbound' {>} \inbound$ then $\inbound' {\dotminus} \inbound = \inbound' {-} \inbound$ and
$\prove_{\starsys} \lnot \size \geq \inbound{+}1 \separate \lnot \size \geq \inbound' {-} \inbound \implies \lnot \size 
\geq \inbound'$ follows from the axiom~\ref{starAx:SizeNeg}. We are now ready to conclude the proof 
of~\ref{SC-auxlemma3}.
$$
\begin{array}{l|ll}
15 &  \lnot \size \geq \inbound{+}1 \separate \lnot \size \geq \inbound'{\dotminus}\inbound \implies \lnot \size \geq \inbound'
& \mbox{See above} \\ 
16 & ((\aformula \land \lnot \size \geq \inbound{+}{1}) \separate (\aformulabis \land \lnot \size \geq \inbound'{\dotminus}\inbound)) \implies
          \lnot \size \geq \inbound'
& \mbox{\ref{pcrule:imptrans} 8, 15} \\
17 & ((\aformula \land \lnot \size \geq \inbound{+}1) {\separate} (\aformulabis \land 
\lnot\size \geq \inbound'{\dotminus}\inbound)) \land \size \geq \inbound' \implies \\
& \lnot \size \geq \inbound' {\land} \size \geq \inbound'
& \mbox{\ref{pcrule:andWR} and \ref{pcax:command}, 16} \\
18 & \lnot \size \geq \inbound' \land \size \geq \inbound' \iff \false
& \mbox{\ref{pcax:truesub} +  Def. $\true$} \\
19 & ((\aformula \land \lnot \size \geq \inbound{+}1) \separate (\aformulabis \land \lnot\size \geq \inbound'{\dotminus}\inbound)) \land \size \geq \inbound' \iff \false
& \mbox{\ref{pcrule:imptrans} and \ref{pcax:falseintro} 17, 18} \\
20 & ((\aformula \land \lnot \size \geq \inbound{+}1) \separate \aformulabis) \land \size \geq \inbound' \implies\\
&  ((\aformula \land \lnot \size \geq \inbound{+}1) \separate (\aformulabis \land \size \geq 
\inbound'{\dotminus}\inbound) \land \size \geq \inbound') \lor \false
& \mbox{\ref{SC-auxlemmaR0}, 7, 19} \\
21 &  ((\aformula \land \lnot \size \geq \inbound{+}1) \separate (\aformulabis \land \size \geq 
\inbound'{\dotminus}\inbound) \land \size \geq \inbound') \lor \false
    \implies\\
& (\aformula \land \lnot \size \geq \inbound{+}1) \separate (\aformulabis \land \size \geq 
\inbound'{\dotminus}\inbound)
& \mbox{\ref{pcax:trueintro}} \\ 
22 & ((\aformula \land \lnot \size \geq \inbound{+}1) \separate \aformulabis) \land \size 
\geq \inbound' \implies\\
& (\aformula \land \lnot \size \geq \inbound{+}1) \separate (\aformulabis \land \size \geq 
\inbound'{\dotminus}\inbound)
& \mbox{\ref{pcrule:imptrans} 20, 21}
\end{array}
$$
\end{itemize}

\end{proof}

Let us conclude by deriving the formula below:  
$$
\size \geq \inbound_1{+}\inbound_2 \land \lnot \size \geq (\inbound_1' {+} \inbound_2') {\dotminus} 1 \implies (\size \geq \inbound_1 \land \lnot \size \geq \inbound_1') \separate (\size \geq \inbound_2 \land \lnot \size \geq \inbound_2')
$$

We start this case by first proving that for every $\inbound,\inbound'\geq1$
$$
  \prove_{\starsys}\lnot \size \geq (\inbound + \inbound'){\dotminus}1 \implies \lnot \size \geq \inbound \separate \lnot \size \geq \inbound'.
$$

$$
\begin{array}{l|ll}
1  & \lnot \size \geq (\inbound + \inbound'){\dotminus}1 \implies\\
&  \lnot \size \geq (\inbound + \inbound'){\dotminus}1 \land \bigwedge_{k \in \interval{0}{(\inbound +
 \inbound'){\dotminus}2}} (\size \geq k \lor \lnot \size \geq k)
& \mbox{PC} \\ 
2 & \lnot \size \geq (\inbound + \inbound'){\dotminus}1 \land \bigwedge_{k \in \interval{0}{(\inbound + 
\inbound'){\dotminus}2}} (\size \geq k \lor \lnot \size \geq k)
  \implies\\
&  \bigvee_{k \in \interval{0}{(\inbound + \inbound'){\dotminus}2}} \size = k
& \mbox{repeated \ref{pcax:distand}} \\
3 & \lnot \size \geq (\inbound + \inbound'){\dotminus}1 \implies \bigvee_{k \in 
\interval{0}{(\inbound + \inbound'){\dotminus}2}} \size = k
& \mbox{\ref{pcrule:imptrans}, 1, 2} \\
4 & \size \geq k \implies \size = \min(k,\inbound-1) \separate \size \geq k \dotminus (\inbound-1)
&  \mbox{\ref{SC-auxS5}} \\
5 & \size = k \implies (\size = \min(k,\inbound-1) \separate \size \geq k \dotminus (\inbound-1)) 
\land \lnot \size \geq k{+}1
& \mbox{\ref{pcrule:andWR} and \ref{pcax:command}, 4} \\ 
6 &  (\size = \min(k,(\inbound-1)) \separate \size \geq k \dotminus (\inbound-1)) \land \lnot \size \geq k{+}1
          \implies\\
& \size = \min(k,\inbound-1) \separate (\size \geq k \dotminus (\inbound-1) \land \lnot \size 
\geq (k{+}1){\dotminus}\min(k,(\inbound-1)))
& \mbox{\ref{SC-auxlemma2}} \\ 
7 & \size = k \implies\\
&            \size = \min(k,\inbound-1) \separate (\size \geq k \dotminus (\inbound-1) \land \lnot \size \geq (k{+}1){\dotminus}\min(k,(\inbound-1)))
& \mbox{\ref{pcrule:imptrans}, 5, 6} \\ 
8 & \size = \min(k,\inbound-1) \separate (\size \geq k \dotminus (\inbound-1) \land \lnot \size \geq (k{+}1){\dotminus}\min(k,(\inbound-1))) \implies\\
& \lnot \size \geq \min(k+1,\inbound) \separate \lnot \size \geq (k{+}1){\dotminus}\min(k,(\inbound-1))
& \mbox{\ref{SC-auxlemmareal0}} \\           
9 &  \size = k \implies
            \lnot \size \geq \min(k+1,\inbound) \separate \lnot \size \geq 
    (k{+}1){\dotminus}\min(k,(\inbound-1))
& \mbox{\ref{pcrule:imptrans}, 7, 8}
\end{array}
$$
We continue the proof by showing that for every $k \in \interval{0}{(\inbound + \inbound'){\dotminus}2}$,
$$
  \prove_{\starsys} \lnot \size \geq \min(k+1,\inbound) \separate \lnot \size \geq (k{+}1){\dotminus}\min(k,(\inbound-1))
  \implies \lnot \size \geq \inbound \separate \lnot \size \geq \inbound'.
$$
Indeed, for $k < \inbound$ the antecedent of this implication, i.e.
$\lnot \size \geq \min(k+1,\inbound) \separate \lnot \size \geq (k{+}1){\dotminus}\min(k,(\inbound-1))$, simplifies to
$\lnot \size \geq k \separate \lnot \size \geq 1$. Then, recalling that
$1 \leq \inbound'$,
by iterating the axiom \ref{coreAx:Size} together with the rule~\ref{rule:starinference} we conclude
$\prove_{\starsys} \lnot \size \geq k \separate \lnot \size \geq 1 \implies \lnot \size \geq \inbound \separate \lnot \size \geq \inbound'$.
If instead
$k \geq \inbound$,
then the antecedent becomes
$\lnot \size \geq \inbound \separate \lnot \size \geq (k+1){\dotminus}(\inbound-1)$.
Since $k \in \interval{0}{(\inbound + \inbound'){\dotminus}2}$
and
$\inbound,\inbound'\geq1$,
we have
$(k+1){\dotminus}(\inbound-1) \leq (((\inbound + \inbound'){\dotminus}2)+1){\dotminus}(\inbound-1) \leq \inbound'$.
Hence,
$\lnot \size \geq \inbound \separate \lnot \size \geq (k+1){\dotminus}(\inbound-1)$
simplifies to
$\lnot \size \geq \inbound \separate \lnot \size \geq j$ for some $j \leq \inbound'$.
Then,
$\prove_{\starsys}  \lnot \size \geq \inbound \separate \lnot \size \geq j \implies \lnot \size \geq \inbound \separate \lnot \size \geq \inbound'$
again by iterating the axiom \ref{coreAx:Size} together with the rule~\ref{rule:starinference}. We can now conclude the proof of
$\prove_{\starsys}\lnot \size \geq (\inbound + \inbound'){\dotminus}1 \implies \lnot \size \geq \inbound \separate \lnot \size \geq \inbound'.$

$$
\begin{array}{l|ll}
10 & \lnot \size \geq \min(k+1,\inbound) \separate \lnot \size \geq (k{+}1){\dotminus}\min(k,(\inbound-1))
\implies\\ 
& \lnot \size \geq \inbound \separate \lnot \size \geq \inbound'
& \mbox{$\forall k \in \interval{0}{(\inbound + \inbound'){\dotminus}2}$ -- just shown}\\
11 & \size = k \implies
          \lnot \size \geq \inbound \separate \lnot \size \geq \inbound'
& \mbox{$\forall k \in \interval{0}{(\inbound + \inbound'){\dotminus}2}$ -- \ref{pcrule:imptrans}, 9, 10} \\
12 & \lnot \size \geq (\inbound + \inbound'){\dotminus}1 \implies \lnot \size \geq 
\inbound \separate \lnot \size \geq \inbound'
& \mbox{Prop. reasoning, 3, 11}
\end{array}
$$

Here is the final steps of the derivation. 
Recall that $0 \leq \inbound_1 < \inbound_1'$ and $0 \leq \inbound_2 < \inbound_2'$.

$$
\begin{array}{l|ll}
1 & \size \geq \inbound_1 + \inbound_2 \implies \size = \inbound_1 \separate \size \geq \inbound_2
&  \mbox{\ref{SC-auxS5}} \\
2 & \size \geq \inbound_1 + \inbound_2 \land \lnot \size \geq (\inbound_1'+\inbound_2'){\dotminus}1
          \implies\\ 
& (\size = \inbound_1 \separate \size \geq \inbound_2) \land \lnot \size \geq 
(\inbound_1'+\inbound_2'){\dotminus}1
& \mbox{\ref{pcrule:andWR} and \ref{pcax:command}, 1} \\
3 & (\size = \inbound_1 \separate \size \geq \inbound_2)
          \land \lnot \size \geq (\inbound_1'+\inbound_2'){\dotminus}1 \implies\\
&          \size = \inbound_1 \separate (\size \geq \inbound_2 \land \lnot \size \geq 
((\inbound_1'-\inbound_1)+\inbound_2'){\dotminus}1)
& \mbox{\ref{SC-auxlemma2} and $\inbound_1 < \inbound_1'$} \\
4 & \size \geq \inbound_1 + \inbound_2 \land \lnot \size \geq (\inbound_1'+\inbound_2'){\dotminus}1
          \implies\\
&          \size = \inbound_1 \separate (\size \geq \inbound_2 \land \lnot 
\size \geq ((\inbound_1'-\inbound_1)+\inbound_2'){\dotminus}1)
& \mbox{\ref{pcrule:imptrans}, 2, 3} \\
5 & \size \geq \inbound_2 \implies \size = \inbound_2 \separate \size \geq 0
&  \mbox{\ref{SC-auxS5}} \\
6 & \size \geq \inbound_2 \land  \lnot \size \geq ((\inbound_1'-\inbound_1)+\inbound_2'){\dotminus}1
            \implies\\
& ( \size = \inbound_2 \separate \size \geq 0) \land  \lnot \size
 \geq ((\inbound_1'-\inbound_1)+\inbound_2'){\dotminus}1
& \mbox{\ref{pcrule:andWR} and \ref{pcax:command}, 5} \\
7 & (\size = \inbound_2 \separate \size \geq 0) \land
          \lnot \size \geq ((\inbound_1'-\inbound_1)+\inbound_2){\dotminus}1
          \implies\\
& \size = \inbound_2 \separate (\size \geq 0 \land
                    \lnot \size \geq ((\inbound_1'-\inbound_1)+(\inbound_2'-\inbound_2)){\dotminus}1)
& \mbox{\ref{SC-auxlemma2} and $\inbound_1 < \inbound_1'$}\\
8 & \size \geq \inbound_2 \land  \lnot \size \geq ((\inbound_1'-\inbound_1)+\inbound_2'){\dotminus}1
            \implies\\
&            \size = \inbound_2 \separate (\size \geq 0 \land
                      \lnot \size \geq ((\inbound_1'-\inbound_1)+(\inbound_2'-\inbound_2)){\dotminus}1)
& \mbox{\ref{pcrule:imptrans}, 6, 7}\\
9 & \size \geq 0 \land
          \lnot \size \geq ((\inbound_1'-\inbound_1)+(\inbound_2'-\inbound_2)){\dotminus}1
          \implies\\
& \lnot \size \geq ((\inbound_1'-\inbound_1)+(\inbound_2'-\inbound_2)){\dotminus}1
& \mbox{\ref{pcax:andelim}} \\ 
10 & \size = \inbound_2 \separate (\size \geq 0 \land
            \lnot \size \geq ((\inbound_1'-\inbound_1)+(\inbound_2'-\inbound_2)){\dotminus}1)
            \implies\\
& \size = \inbound_2 \separate \lnot \size \geq ((\inbound_1'-\inbound_1)+(\inbound_2'-\inbound_2)){\dotminus}1
& \mbox{\ref{rule:starinference} and \ref{starAx:Commute}, 9} \\ 
11 & \size \geq \inbound_2 \land  \lnot \size \geq ((\inbound_1'-\inbound_1)+\inbound_2'){\dotminus}1 \implies\\
& \size = \inbound_2 \separate \lnot \size \geq ((\inbound_1'-\inbound_1)+(\inbound_2'-\inbound_2)){\dotminus}1
& \mbox{\ref{pcrule:imptrans}, 8, 10} \\ 
12 & \lnot \size \geq ((\inbound_1'-\inbound_1)+(\inbound_2'-\inbound_2)){\dotminus}1 \implies\\
& \lnot \size \geq \inbound_1'-\inbound_1 \separate \lnot \size \geq \inbound_2'-\inbound_2
%% & \mbox{previous result, as $\inbound_1 < \inbound_1'$ and $\inbound_2 < \inbound_2'$} \\
 & \mbox{See above} \\
13 & \size = \inbound_2 \separate \lnot \size \geq ((\inbound_1'-\inbound_1)+(\inbound_2'-\inbound_2)){\dotminus}1 \implies\\
& \size = \inbound_2 \separate (\lnot \size \geq \inbound_1'-\inbound_1 \separate \lnot \size \geq \inbound_2'-\inbound_2)
& \mbox{\ref{rule:starinference} and \ref{starAx:Commute}, 12} \\ 
14 & \size \geq \inbound_2 \land  \lnot \size \geq ((\inbound_1'-\inbound_1)+\inbound_2'){\dotminus}1 \implies\\
&  \size = \inbound_2 \separate (\lnot \size \geq \inbound_1'-\inbound_1 \separate \lnot \size \geq 
\inbound_2'-\inbound_2)
& \mbox{\ref{pcrule:imptrans}, 12, 13} 
\end{array}
$$

$$
\begin{array}{l|ll}
15 & \size = \inbound_2 \separate (\lnot \size \geq \inbound_1'-\inbound_1 \separate \lnot \size \geq 
\inbound_2'-\inbound_2) \implies\\ 
& \lnot \size \geq \inbound_1'-\inbound_1 \separate (\size = \inbound_2 \separate \lnot  \size \geq \inbound_2'-\inbound_2) 
& \mbox{\ref{starAx:Commute} and \ref{starAx:Assoc}} \\ 
16 & \size \geq \inbound_2 \land  \lnot \size \geq ((\inbound_1'-\inbound_1)+\inbound_2'){\dotminus}1 \implies\\
& \lnot \size \geq \inbound_1'-\inbound_1 \separate (\size = \inbound_2 \separate \lnot  \size \geq \inbound_2'-\inbound_2) 
& \mbox{\ref{pcrule:imptrans}, 14, 15} \\ 
17 & \size = \inbound_2 \separate \lnot \size \geq \inbound_2' - \inbound_2 \implies
            \size \geq \inbound_2 \separate \size \geq 0
& \mbox{\ref{SC-auxlemmareal0} + $\size \geq 0 \egdef \top$, \ref{rule:starintroLR}} \\
18 &  \size \geq \inbound_2 \separate \size \geq 0 \implies \size \geq \inbound_2
& \mbox{\ref{SC-auxlemma0}} \\ 
19 &   \size = \inbound_2 \separate \lnot \size \geq \inbound_2' - \inbound_2 \implies \size \geq \inbound_2
& \mbox{\ref{pcrule:imptrans}, 17, 18} \\ 
20 & \size = \inbound_2 \separate \lnot \size \geq \inbound_2' - \inbound_2 \implies
            \lnot \size \geq \inbound_2{+}1 \separate \lnot \size \geq \inbound_2'-\inbound_2
& \mbox{\ref{SC-auxlemmareal0}}\\
21 & \lnot \size \geq \inbound_2{+}1 \separate \lnot \size \geq \inbound_2'-\inbound_2 \implies
            \lnot \size \geq \inbound_2'
& \mbox{\ref{starAx:SizeNeg}} \\
22 &      \size = \inbound_2 \separate \lnot \size \geq \inbound_2' - \inbound_2 \implies
          \lnot \size \geq \inbound_2'
& \mbox{\ref{pcrule:imptrans}, 20, 21} \\
23 &  \size = \inbound_2 \separate \lnot \size \geq \inbound_2' - \inbound_2 \implies
          \size \geq \inbound_2 \land \lnot \size \geq \inbound_2'
& \mbox{\ref{pcrule:andR}, 19, 22} \\
24 & \lnot \size \geq \inbound_1'-\inbound_1 \separate (\size = \inbound_2 \separate \lnot  \size \geq \inbound_2'-\inbound_2) \implies\\
& \lnot \size \geq \inbound_1'-\inbound_1 \separate (\size \geq \inbound_2 \land \lnot \size \geq \inbound_2')
& \mbox{\ref{rule:starinference} and \ref{starAx:Commute}, 23} \\ 
25 & \size \geq \inbound_2 \land  \lnot \size \geq ((\inbound_1'-\inbound_1)+\inbound_2'){\dotminus}1 \implies\\
& \lnot \size \geq \inbound_1'-\inbound_1 \separate (\size \geq \inbound_2 \land \lnot \size \geq 
\inbound_2')
& \mbox{\ref{pcrule:imptrans}, 16, 24} \\
26 & \size = \inbound_1 \separate (\size \geq \inbound_2 \land \lnot \size \geq ((\inbound_1'-\inbound_1)+\inbound_2'){\dotminus}1) \\
&  \size = \inbound_1 \separate (\lnot \size \geq \inbound_1'-\inbound_1 \separate (\size \geq \inbound_2 \land \lnot \size \geq \inbound_2'))
& \mbox{\ref{rule:starinference} and \ref{starAx:Commute}, 25} \\ 
27 &  \size \geq \inbound_1 + \inbound_2 \land \lnot \size \geq (\inbound_1'+\inbound_2'){\dotminus}1
          \implies\\
& \size = \inbound_1 \separate (\lnot \size \geq \inbound_1'-\inbound_1 \separate 
(\size \geq \inbound_2 \land \lnot \size \geq \inbound_2'))
& \mbox{\ref{pcrule:imptrans}, 4, 26} \\ 
28 & \size = \inbound_1 \separate (\lnot \size \geq \inbound_1'-\inbound_1 \separate 
(\size \geq \inbound_2 \land \lnot \size \geq \inbound_2'))
          \implies\\
&          (\size = \inbound_1 \separate \lnot \size \geq \inbound_1'-\inbound_1) \separate (\size \geq \inbound_2 \land \lnot \size \geq \inbound_2')
& \mbox{\ref{starAx:Assoc}} \\ 
29 & \size \geq \inbound_1 + \inbound_2 \land \lnot \size \geq (\inbound_1'+\inbound_2'){\dotminus}1
          \implies\\
&          (\size = \inbound_1 \separate \lnot \size \geq \inbound_1'-\inbound_1) \separate 
(\size \geq \inbound_2 \land \lnot \size \geq \inbound_2')
& \mbox{\ref{pcrule:imptrans}, 27, 28} \\ 
30 &  \size = \inbound_1 \separate \lnot \size \geq \inbound_1'-\inbound_1 \implies \size \geq \inbound_1 \land \lnot \size \geq \inbound_1'
& \mbox{analogous to 23} \\ 
31 & 
          (\size = \inbound_1 \separate \lnot \size \geq \inbound_1'-\inbound_1) \separate (\size \geq \inbound_2 \land \lnot \size \geq \inbound_2') \implies\\
& (\size \geq \inbound_1 \land \lnot \size \geq \inbound_1') \separate (\size \geq \inbound_2 \land \lnot \size \geq \inbound_2')
& \mbox{\ref{rule:starinference}, 30} \\ 
32 & \size \geq \inbound_1 + \inbound_2 \land \lnot \size \geq (\inbound_1'+\inbound_2'){\dotminus}1
          \implies\\
&          (\size \geq \inbound_1 \land \lnot \size \geq \inbound_1') \separate 
(\size \geq \inbound_2 \land \lnot \size \geq \inbound_2')
& \mbox{\ref{pcrule:imptrans}, 29, 31}
\end{array}
$$
