# Supplementary material for: A Complete Axiomatisation for Quantifier-Free Separation Logic
Source: arXiv:2006.05156 source file (2021-08-09)
Supplement: Supplementary file 2 [file appendix.tex]

\newpage
\section{A derivation in the proof system for \slSW}
\label{appendix-paragraphe-an-example}
We develop the proof of $\emp \implies (\alloc{\avariable} \magicwand \size = 1)$ as a more complete example with respect to the one shown in the body of the paper.
We use the following theorem and rules, which can be shown admissible in the calculus:
\begin{nscenter}
  \scalebox{0.9}{
  \lemmalab{\textbf{($\magicwand\land$-DistrL)}}{axiom:magicsep}\,
  $
  (\aformula \magicwand \aformulabis) \land (\aformula \magicwand \aformulater) \implies (\aformula \magicwand \aformulabis \land \aformulater)
  $}%
  \hfill
  \scalebox{0.9}{
  \lemmalab{\textbf{($\land\true$IL)}}{axiom:andtrue}\,
  $
  \aformula \implies \true \land \aformula
  $}%
  \hfill
  \scalebox{0.9}{
  \rulelab{\textbf{$\land$-InfL}}{rule:andinf}
  $
  \inference{\aformula \implies \aformulater}{\aformula \land \aformulabis \implies \aformulater \land \aformulabis}
  $}%
\end{nscenter}
Recall that $\size = \inbound$ is a shortcut for $\size \geq \inbound \land \lnot \size \geq \inbound{+}1$.\\
\scalebox{0.9}{
$
\begin{nd}
\have {5} {\true \separate (\alloc{\avariable} \land \size = 1) \implies (\alloc{\avariable} \land \size = 1) \separate \true} \by{\ref{starAx:Commute}}{}
\have {1} {\alloc{\avariable} \land \size = 1 \implies \size \geq 1} \by{\ref{axiom:andelim}}{}
\have {2} {\alloc{\avariable} \land \size = 1 \separate \true \implies \size \geq 1 \separate \true} \by{\ref{rule:starinference} rule}{1}
\have {3} {\size \geq 1 \separate \true \implies \size \geq 1} \by{\ref{starAx:MonoCore} ($\size \geq 1 \egdef \lnot \emp$)}{}
\have {6} {\true \separate (\alloc{\avariable} \land \size = 1) \implies \size \geq 1} \by{\ref{rule:imptr} twice}{5,2,3}
\have {7} {\true \implies (\alloc{\avariable} \land \size = 1 \magicwand \size \geq 1)} \by{\ref{rule:staradj} rule}{6}
\have {12} {\emp \implies (\alloc{\avariable} \land \size = 1 \magicwand \lnot \size \geq 2)} \by{\small{derived in the body of the paper}}{}
\have {14} {(\alloc{\avariable} \land \size = 1 \magicwand \lnot \size \geq 2) \implies\\
 \true \land (\alloc{\avariable} \land \size = 1 \magicwand \lnot \size \geq 2)} \by{\ref{axiom:andtrue}}{}
\have {15} { \true \land (\alloc{\avariable} \land \size = 1 \magicwand \lnot \size \geq 2) \implies\\
\big((\alloc{\avariable} \land \size = 1 \magicwand \size \geq 1) \land\\ (\alloc{\avariable} \land \size = 1 \magicwand \lnot \size \geq 2)\big)} \by{\ref{rule:andinf}}{7}
\have {16} {\big((\alloc{\avariable} \land \size = 1 \magicwand \size \geq 1) \land\\ (\alloc{\avariable} \land \size = 1 \magicwand \lnot \size \geq 2)\big) \implies\\
(\alloc{\avariable} \land \size = 1 \magicwand \size = 1)
} \by{\ref{axiom:magicsep}}{}
\have {17} {(\alloc{\avariable} \land \size = 1 \magicwand \lnot \size \geq 2) \implies\\ (\alloc{\avariable} \land \size = 1 \magicwand \size = 1)} \by{\ref{rule:imptr} twice}{14,15,16}
\have {18} {\emp \implies
(\alloc{\avariable} \land \size = 1 \magicwand \size = 1)
} \by{\ref{rule:imptr}}{12,17}
\end{nd}
$}

\newpage
{\em Below, you will find the table of contents as well as technical appendices containing the proofs of the statements
from the body of the paper.
%% Initially, we did not expect that the proofs would be so lengthy but we have included it in the
%% document so that this can be read at the discretion of the reviewers.
It should also be noted that Appendix~\ref{appendix:DerivedTautologies} solely contains syntactic derivations in the calculus presented in Section~\ref{section:IntervalSL}, which are by nature lenghty.
}

\tableofcontents

\section{Proofs of Section~\ref{section:PSL}}\label{appendix:Section3}

We recall that, given $\aliteral_1 \land \dots \land \aliteral_n \in \conjcomb{\coreformulae{\asetvar}{\bound}}$, we write $\literals{\aformula}$ to denote
$\{\aliteral_1,\dots,\aliteral_n\}$.
The notation $\aformulabis \inside \aformula$ is a shortcut for $\literals{\aformulabis} \subseteq \literals{\aformula}$.
Moreover, we write $\aformulater \inside \orliterals{\aformula}{\aformulabis}$ for
``$\aformulater \inside \aformula$ or $\aformulater \inside \aformulabis$'' and $\aformulater \inside \andliterals{\aformula}{\aformulabis}$ for ``$\aformulater \inside \aformula$ and $\aformulater \inside \aformulabis$''.
Similarly, $\orliterals{\aformula}{\aformulabis} \inside \aformulater$ (resp. $\andliterals{\aformula}{\aformulabis} \inside \aformulater$) stands for
``$\aformula \inside \aformulater$ or $\aformulabis \inside \aformulater$'' (resp. ``$\aformula \inside \aformulater$ and $\aformulabis \inside \aformulater$'').
Notice that the notation $\andliterals{\aformula}{\aformulabis} \inside \aformulater$ is not used nor defined in the body of the paper. However, it is (rarely) used in these appendices.

%% EL : uncomment if want to transfer the proof from core of the paper to the appendix
%% \subsection{Proof of Proposition~\ref{lemma:corePSLvalid}}
%% \lemmacorePSLvalid*
%% \begin{proof}
%% \input{appendixproofs/lemma-corePSLvalid}
%% \end{proof}

%% \subsection{Proof of Lemma~\ref{prop:corePSLone}}
%% \propcorePSLone*
%% \begin{proof}
%% \input{appendixproofs/property-corePSLone}
%% \end{proof}

%% \subsection{Proof of Lemma~\ref{prop:corePSLtwo}}
%% \propcorePSLtwo*
%% \begin{proof}
%% \input{appendixproofs/property-corePSLtwo}
%% \end{proof}

%% EL : a priori plus besoin de cette propriete
%% \subsection{Proof of Property~\ref{prop:corePSLthree}}
%% \propcorePSLthree*
%% \begin{proof}
%% \input{appendixproofs/property-corePSLthree}
%% \end{proof}

%% \subsection{Proof of Theorem~\ref{theo:corePSLcompl}}
%% \theocorePSLcompl*
%% \begin{proof}
%% \input{appendixproofs/theo-corePSLcompl}
%% \end{proof}

%% \subsection{Proof of Lemma~\ref{lemma:starPSLvalid}}
%% \lemmastarPSLvalid*
%% \begin{proof}
%% \input{appendixproofs/lemma-starPSLvalid}
%% \end{proof}

\subsection{Proof of Lemma~\ref{prop:corePSLtwo}}
\propcorePSLtwo*

\begin{proof}
We show that $\aformula$ is unsatisfiable if and only if $\vdash_{\coresys}\aformula\implies\bot$.
The ``only if'' part follows from the soundness of $\coresys$, so we just sketch the proof of the ``if'' part.
Let $\aformula\in \coretype{\asetvar}{\bound}$ be fixed such that $\not\vdash_{\coresys}\aformula\Rightarrow \bot$, and let us prove that
$\aformula$ is satisfiable.
By the axioms~\ref{coreAx:EqRef}
%,$\ref{coreAx:EqSymm}$,
and~\ref{coreAx:EqSub},
there is an equivalence relation $\approx$ on $\asetvar$ such that
$\avariable\approx\avariablebis$ iff $\avariable=\avariablebis$ occurs positively
in $\aformula$. We write $[\avariable]$ to denote the equivalence class of $\avariable$
with respect to $\approx$.
By the axioms $\ref{coreAx:EqSub}$, $\ref{coreAx:PointInj}$,
there is a partial map $f: (\asetvar/\approx)\to(\asetvar/\approx)$ on equivalence classes such
that $\avariable\Ipto \avariablebis$ occurs positively iff $f([x])$ is defined and $f([x])=[y]$.
Let $D=\{[\avariable]\mid \alloc{\avariable}\mbox{ occurs positively in }\aformula\}$.
By the axiom $\ref{coreAx:PointAlloc}$, $\mathsf{dom}(f)\subseteq D$.
Let $n$ be the greatest $\beta$ such that $\size\geq\beta$ occurs positively in $\aformula$.
By the axiom~\ref{coreAx:AllocSize}, $n\geq \card{D}$.
Let $\alocation_0,\alocation_1,\dots,\alocation_n\in\LOC$ be $n+1$ distinct locations, and let
us fix an enumeration $C_1,\dots,C_{\card{D}}$ on the equivalence classes of $\approx$.
Let $(\astore,\aheap)$ be defined by
\begin{itemize}
\item $\astore(\avariable)=\alocation_i$ if $[x]$ is the $i$th equivalence class,
\item $\aheap(\alocation_i)=\alocation_j$ if $0<i\leq \card{D}$ and the $i$th equivalence class is mapped to the $j$th
one by $f$,
\item $\aheap(\alocation_i)=\alocation_0$ if either $0<i\leq \card{D}$ and the $i$th equivalence class is not in the domain of $f$, or $i> \card{D}$.
\end{itemize}
Then, by construction, $\pair{\astore}{\aheap}$ satisfies all positive literals of the form $\avariable=\avariablebis$ or $\avariable\Ipto\avariablebis$ or $\alloc{\avariable}$
that occur positively in $\aformula$, and all negative literals of the same form that occur negatively in $\aformula$. It also
satisfies $\size\geq n$, falsifies $\size\geq n+1$ (assuming $n+1 \leq \bound$), and by thr axiom~\ref{coreAx:Size}, it satisfies all size literals
in $\aformula$.
\end{proof}

\subsection{Proof of Theorem~\ref{theo:corePSLcompl}}
\theocorePSLcompl*

In order to prove Theorem~\ref{theo:corePSLcompl}, let us first establish the following lemma.

\begin{restatable}{lemma}{propcorePSLone}
\stmtdesc{Core Types Lemma}
\label{prop:corePSLone}
Let $\aformula \in \boolcomb{\coreformulae{\asetvar}{\bound}}$. There is a disjunction
$\aformulabis=\aformulabis_1\vee\ldots\vee\aformulabis_n$ with
$\aformulabis_i\in\coretype{\asetvar}{\bound}$ for all $i$
such that $\prove_{\coresys} \aformula \iff \aformulabis$.
\end{restatable}

\begin{proof}
Let $\aformulabis_1\vee\ldots\vee\aformulabis_n$ be a formula in disjunctive normal form equivalent to $\aformula$. If $\aformulabis_i$ is not a core type, there is a core formula $\aformulater\in\coreformulae{\asetvar}{\bound}$ that occurs neither positively nor negatively in $\aformula_i$.
Replacing $\aformula_i$ with $(\aformula_i\wedge\aformulater)\vee(\aformula_i\wedge\neg\aformulater)$, and repeating this for all missing core types and for all $i$, we obtain a
disjunction of core types of the expected form. Since all equivalences follow from reasoning in classical logic, the equivalence between $\aformula$ and the obtained formula can be proved
in $\coresys$.
\end{proof}

\begin{proof} (Theorem~\ref{theo:corePSLcompl})
Let $\aformula$ be a Boolean combination of core formulae.
As all the axioms are valid (the proof can be found in Appendix~\ref{appendix:PSLSoundness}), $\prove_{\coresys} \aformula$ implies that $\aformula$ is
valid.
Now, let us assume that $\aformula$ is valid, and let us prove that $\prove_{\coresys}\aformula$.
By Lemma~\ref{prop:corePSLone}, there is a disjunction $\aformulabis=\aformula_1\vee\ldots\vee\aformula_n$ of core types
such that $\prove_{\coresys}(\neg \aformula)\Leftrightarrow\aformulabis$.
Since $\aformula$ is valid, the formulae
$\neg\aformula$, $\aformulabis$ and all the $\aformulabis_i$'s are unsatisfiable.
By Lemma~\ref{prop:corePSLtwo}, $\prove_{\coresys}\aformulabis_i\Rightarrow\bot$, for all $i$.
Therefore, by classical reasoning, $\prove_{\coresys}\neg\aformula\Rightarrow\bot$.
\end{proof}

\subsection{Proof of Proposition~\ref{prop:admissible-axioms-1}}
\label{appendix-proof-proposition-admissible-axioms-1}

%% \propadmissibleaxiomsone*

\begin{restatable}{proposition}{propadmissibleaxiomsone}\label{prop:admissible-axioms-1}
Axioms $\ref{coreAx:Size}$ and $\ref{coreAx:AllocSize}$ are derivable
in $\coresys(*)$.
\end{restatable}

\begin{proof}
\input{appendixproofs/proposition-admissible-axioms-1}
\end{proof}

\subsection{Proof of Lemma~\ref{lemma:starPSLelim}}
\lemmastarPSLelim*
\begin{proof}
 Let $\aformula$ and $\aformulabis$ in $\coretype{\asetvar}{\bound}$. 
Let us first treat the case where one of the two formulas is unsatisfiable.
Assume for instance that
$\aformula$ is not satisfiable. Then $\prove_{\coresys} \aformula\implies \bot$ by completeness of $\coresys$ (Lemma~\ref{prop:corePSLtwo}). By 
the rule~\ref{rule:starinference} and by the axiom~\ref{starAx:False}, we get  $\prove_{\starsys}\aformula*\aformulabis\implies\bot$.

Let us now assume that both $\aformula$ and $\aformulabis$ are satisfiable. Let $\aformulater$
be defined as
  $$
  \begin{array}{llll}
  &\bigwedge \formulasubset{\avariable \sim \avariablebis \inside \orliterals{\aformula}{\aformulabis}}{\bmat[\sim \in \{=,\neq\}]}
  & \land &
  \bigwedge \aformulasubset{\alloc{\avariable}\inside \orliterals{\aformula}{\aformulabis}}
  \\ \land &
  \bigwedge \aformulasubset{\lnot\alloc{\avariable} \inside\andliterals{\aformula}{\aformulabis}}
  & \land &
  \bigwedge \formulasubset{\lnot \avariable \Ipto \avariablebis}{\bmat[\alloc{\avariable}\land\lnot\avariable\Ipto\avariablebis\inside \orliterals{\aformula}{\aformulabis}]}
  \\ \land &
  \bigwedge \formulasubset{\avariable \neq \avariable}{\bmat[\alloc{\avariable}\inside\andliterals{\aformula}{\aformulabis}]}
  & \land & \bigwedge \formulasubset{\size\geq\inbound_1{+}\inbound_2}{\bmat[\size\geq\inbound_1\inside\aformula\\\size\geq\inbound_2\inside\aformulabis]}
  \\ \land &
  \bigwedge \aformulasubset{\avariable \Ipto \avariablebis \inside \orliterals{\aformula}{\aformulabis}}
  &\land &
  \bigwedge \formulasubset{\lnot\size\geq\inbound_1{+}\inbound_2{\dotminus}1}{\bmat[\lnot\size\geq\inbound_1\inside\aformula\\\lnot\size\geq\inbound_2\inside\aformulabis]}
  \end{array}
  $$

and let us show that $\prove_{\starsys}\aformula \separate \aformulabis\iff\aformulater$.
\begin{itemize}
\item Let us first show that $\prove_{\starsys}\aformula \separate \aformulabis\implies\aformulater$.
  We show that for any literal $\aliteral$ of $\aformulater$, $\prove_{\starsys}\aformula \separate \aformulabis\implies \aliteral$. We reason by a case analysis on $\aliteral$.

  \begin{itemize}
  \item
    All equalities and inequalities that occur in $\aformula$ or $\aformulabis$,
    and all literals of the
  form $\avariable\Ipto\avariablebis$ that occur in $\aformulater$ follow from the
rule~\ref{rule:starinference} and
  the axiom~\ref{starAx:MonoCore}.
   \item Assume there is a literal $\avariable\neq\avariable$ that occurs in $\aformulater$.
     This is necessarily due to $\alloc{\avariable}$ occurring both in $\aformula$ and
     $\aformulabis$. Then $\bot$ follows from the rule~\ref{rule:starinference}
     and the axiom~\ref{starAx:DoubleAlloc}.
  \item
  All literals of the form $\alloc{\avariable}$ follow from
  the rule~\ref{rule:starinference} and the axiom~\ref{starAx:StarAlloc}.
  \item
  All literals of the form $\neg\alloc{\avariable}$ 
  follow from the rule~\ref{rule:starinference} and the axiom~\ref{starAx:AllocNeg}.
  \item
    Let $\neg\avariable\Ipto\avariablebis$ be a literal occurring in $\aformulater$
    be fixed. Then $\alloc{\avariable}\wedge\neg\avariable\Ipto\avariablebis$ occurs either in
    $\aformula$ or $\aformulabis$. By the rule~\ref{rule:starinference} (and possibly by $\separate$-commutativity, see the axiom~\ref{starAx:Commute}), we get
    $
    \prove_{\starsys} \aformula \separate \aformulabis\implies (\alloc{\avariable}\wedge\neg\avariable\Ipto\avariablebis) \separate \top
    $
    and by the axiom~\ref{starAx:PointsNeg} and classical reasoning we finally get
    $
    \prove_{\starsys} \aformula \separate \aformulabis\implies \neg\avariable\Ipto\avariablebis
    $.
  \item
    Let a literal of the form $\size\geq \inbound_1+\inbound_2$
    occurring in $\aformulater$
    be fixed. Then $\size\geq\inbound_1'$ occurs in $\aformula$ and
    $\size\geq\inbound_2'$ occurs in $\aformulabis$ with $\inbound_1+\inbound_2 = \inbound_1'+\inbound_2'$. 
     By the rule~\ref{rule:starinference}
    $
    \prove_{\starsys} \aformula * \aformulabis\implies \size\geq \inbound_1' \separate \size\geq\inbound_2' 
    $;
    but then, by definition of
    $\size\geq \inbound$, we get 
    $
    \prove_{\starsys} \aformula*\aformulabis\implies \size\geq \inbound_1+\inbound_2    
    $
    
  \item
    Let a literal of the form $\neg (\size\geq \inbound_1+\inbound_2 \dotminus 1)$
    occurring in $\aformulater$
    be fixed. Then
    $\neg(\size\geq\inbound_1')$ occurs in $\aformula$ and
    $\neg(\size\geq\inbound_2')$ occurs in $\aformulabis$ with $\inbound_1+\inbound_2 = \inbound_1'+\inbound_2'$.
    By rule~\ref{rule:starinference},
    $
    \prove_{\starsys} \aformula*\aformulabis\implies \big(\neg (\size\geq \inbound_1')\big)*\big(\neg(\size\geq\inbound_2')\big)    
    $ ;
    but then by the axiom~\ref{starAx:SizeNeg}, 
    $
    \prove_{\starsys} \aformula*\aformulabis\implies \neg (\size\geq \inbound_1+\inbound_2 \dotminus 1).    
    $
    \end{itemize}
  
\item
   Let us now show that $\prove_{\starsys}\aformulater\implies\aformula*\aformulabis$.
   If there is an equality literal $\avariable=\avariablebis$
   that occurs positively in $\aformula$ and negatively in $\aformulabis$, then both
   occur in $\aformulater$, therefore $\prove_{\starsys}\aformulater\implies\bot$
   and $\prove_{\starsys}\aformulater\implies\aformula*\aformulabis$ by classical reasoning.
   Let us therefore assume that $\aformula$ and $\aformulabis$ contain exactly
   the same (in)equalities. Since $\aformula$ is satisfiable, these equalities
   define an equivalence relation.
   Let $\avariable_1,\ldots\avariable_n,\avariablebis_1,\ldots\avariablebis_m$ be an enumeration of representatives of the
   equivalence classes (one per equivalence class) such that $\alloc{\avariable_i}$ occurs in $\aformulater$.
   Applying the same reasoning as in the proof of Proposition~\ref{prop:admissible-axioms-1},
   we deduce from $\aformulater$
   $$
   \big(\alloc{\avariable_1}\wedge\size=1\big)*\cdots *
   \big(\alloc{\avariable_n}\wedge\size=1\big)*\top
   $$
   The rest of the proof is split in three big steps : (1) isolating allocated cells and garbage, (2) splitting them according to the goal $\aformula*\aformulabis$,
   (3) adding missing literals.
   \begin{enumerate}

   \item
   Let $\mathsf{ALLOC} = \big(\alloc{\avariable_1}\wedge\size=1\big) \separate \cdots \separate \big(\alloc{\avariable_n}\wedge\size=1\big)$
   and let $\mathsf{GARB} = \bigwedge\{\size\geq \inbound -n\mid\size\geq\inbound\in\literals{\aformulater}\}\wedge\bigwedge\{\neg (\size\geq \inbound -n)\mid\neg(\size\geq\inbound)\in\literals{\aformulater}\}$.
   We want to show that $\prove_{\starsys}\aformulater\implies\mathsf{ALLOC} * \mathsf{GARB}$.
   We proceed by showing that 
   $$
   \prove_{\starsys}\big(\aformulater \wedge (\mathsf{ALLOC}*\aformula_{g})\big)\implies \big(\mathsf{ALLOC}*(\aformula_{g}\wedge\aliteral)\big)
   $$
   where
   $\aliteral$ is any literal of $\mathsf{GARB}$, and $\aformula_{g}$ is any formula. Applying this reasoning
   iteratively on all $\aliteral$ of $\mathsf{GARB}$, we will reach our goal.
   There are two cases:
   \begin{itemize}
   \item $\aliteral$ is a literal $\size\geq \inbound-n$.
   From $\mathsf{ALLOC}*\aformula_{g}$, the rule~\ref{rule:starinference} and the axiom~\ref{starAx:DistrOr} we get
   $\big(\mathsf{ALLOC}*(\aformula_{g}\wedge \aliteral)\big)\vee\big(\mathsf{ALLOC}*(\aformula_{g}\wedge \neg\aliteral)\big)$. So by classical reasoning
   we resume to show that 
   $\mathsf{ALLOC} * \neg (\size\geq \inbound - n)$ implies $\bot$. By $*$ introduction and \ref{starAx:SizeNeg}
   we get $\neg \size\geq \inbound$. By definition of $\mathsf{GARB}$, $\size\geq\inbound$ occurs in $\aformulater$, so
   we get a contradiction.
   \item
   $\aliteral$ is a literal $\neg \size\geq \inbound-n$. Similarly,
   let us derive a contradiction from $\mathsf{ALLOC} \separate \size\geq \inbound - n$. By $*$ introduction and by definition of $\size\geq \inbound$,
   we get $\size\geq \inbound$, which contradicts $\neg \size\geq\inbound$ occurring in $\aformulater$.
   \end{itemize}

   \item Therefore, we  proved that $\prove_{\starsys}\aformulater\implies\mathsf{ALLOC} * \mathsf{GARB}$.
   If there is a formula $\alloc{\avariable_i}$ ocurring both in $\aformula$ and $\aformulabis$, then
   $\avariable_i\neq\avariable_i$ occurs in $\aformulater$ by definition of $\aformulater$, therefore $\aformulater\implies\aformula*\aformulabis$.
   We can thus assume that the set of variables $\avariable_1,\dots,\avariable_n$ can be split into two subsets, the one ``allocated''
   in $\aformula$, and the others in $\aformulabis$. Let $n_\aformula$ denote the number
   of equivalence classes allocated in $\aformula$, and let
   $$
   \begin{array}{lcl}
    \mathsf{ALLOC}(\aformula) & = &\circledast\{\alloc{\avariable_i}\wedge\size=1\mid\alloc{\avariable_i}\in\literals{\aformula}\}\\
    \mathsf{GARB}(\aformula) & = & \bigwedge\{\size\geq \inbound -n_\aformula\mid\size\geq\inbound\in\literals{\aformula}\}\\ & \wedge & \bigwedge\{\neg (\size\geq \inbound -n_\aformula)\mid\neg(\size\geq\inbound)\in\literals{\aformula}\}
    \end{array}               
    $$
    and let  $\mathsf{ALLOC}(\aformulabis)$ and $\mathsf{GARB}(\aformulabis)$ be defined accordingly.
   By definition of $\aformulater$, $\mathsf{GARB}\implies\mathsf{GARB}(\aformula) * \mathsf{GARB}(\aformulabis)$, and therefore
   $$
   \prove_{\starsys}\aformulater\implies \mathsf{ALLOC}(\aformula) *\mathsf{ALLOC}(\aformulabis) * \mathsf{GARB}(\aformula) * \mathsf{GARB}(\aformulabis)
   $$
   Let 
    $$
    \aformula^{(1)} =   \bigwedge_{\alloc{\avariable_i}\in\literals{\aformula}} \alloc{\avariable_i}\wedge
   \bigwedge_{\size\geq \inbound\in\literals{\aformula}}\size\geq\inbound\wedge
   \bigwedge_{\neg\size\geq \inbound\in\literals{\aformula}}\neg\size\geq\inbound
   $$
    and let $\aformulabis^{(1)}$ be defined accordingly.

   By the axioms~\ref{starAx:StarAlloc},~\ref{starAx:MonoCore},~\ref{starAx:SizeOne},~\ref{starAx:SizeNeg},~\ref{starAx:SizeTwo}, and the 
   rule~\ref{rule:starinference},
   we get
   $$
   \prove_{\starsys} \aformulater\implies\aformula^{(1)}*\aformulabis^{(1)}.
   $$

   \item We now need to add to the conjunct $\aformula^{(1)}$ all missing literals from $\aformula$, and similarly for
   $\aformulabis^{(1)}$. We add these literals iteratively, changing progressively $\aformula^{(1)}$ into $\aformula$.
   So at the $n$th step of the completion, we proved that $\prove_{\starsys}\aformulater \implies\aformula^{(n)}*\aformulabis^{(n)}$
   where $\aformula^{(n)}$ is of the form $\aformula^{(1)}\wedge\aliteral_1\wedge\ldots\wedge\aliteral_{s_n}$ and similarly for $\aformulabis^{(n)}$.
   Let $\aliteral$ be literal of $\aformula$ that does not occur yet in $\aformula^{(n)}$. We reason by a case analysis on $\aliteral$
   \begin{itemize}

   \item $\aliteral$ is an (in)equality : assuming by absurd $(\aformula^{(n)}\wedge\neg\aliteral)*\aformulabis^{(n)}$ we get by the axiom~\ref{starAx:MonoCore}
   and the rule~\ref{rule:starinference},  $\neg \aliteral$; by definition of $\aformulater$, $\aliteral$ occurs in $\aformulater$, whence the contradiction.

   \item $\aliteral$ is of the form $\alloc{\avariable}$ : then by construction of $\aformula^{(1)}$
   there is a variable $\avariable_i$ such that $\alloc{\avariable_i}$ occurs
   in $\aformula^{(n)}$ and $\avariable=\avariable_i$ occurs in $\aformulater$. We can therefore apply the axiom~\ref{coreAx:EqSub}.

   \item $\aliteral$ is of the form $\neg\alloc{\avariable}$. There are two subcases :
       \begin{itemize}
       \item
       $\alloc{\avariable}$ is a literal of $\aformulabis$. Then we derive a contradiction from
       $(\aformula^{(n)}\wedge\alloc{\avariable}) \separate \aformulabis$ by the axiom~\ref{starAx:DoubleAlloc}.
       \item
       $\neg \alloc{\avariable}$ is a literal of $\aformulabis$. Then by definition of $\aformulater$,
       $\neg \alloc{\avariable}$ is a literal of $\aformulater$.  We derive a contradiction from
       $(\aformula^{(n)}\wedge\alloc{\avariable}) \separate \aformulabis$ by the axiom~\ref{starAx:MonoCore}.
       \end{itemize}
   \item $\aliteral$ is of the form $\avariable\Ipto\avariablebis$.
   Then $\avariable\Ipto\avariablebis$ is a literal of
   $\aformulater$. Since $\aformula$ is satisfiable, $\alloc{\avariable}$ is a literal of $\aformula$.
   By construction of $\aformula^{(1)}$, there is $\avariable_i$ such that $\alloc{\avariable_i}$ occurs in $\aformula^{(1)}$ and
   $\avariable=\avariable_i$ is a literal of $\aformulater$. So $\aformulater\implies(\aformula^{(n)}\wedge\alloc{\avariable})*\aformulabis^{(n)}$.
   Assuming by absurd $\aformula^{(n)}\wedge\alloc{\avariable}\wedge\neg\avariable\Ipto\avariablebis)*\aformulabis^{(n)}$, we get
   by the axiom~\ref{starAx:PointsNeg} $\neg\avariable\Ipto\avariablebis$, and a contradiction with $\avariable\Ipto\avariablebis$ occuring in $\aformulater$.

   \item $\aliteral$ is of the form $\neg \avariable\Ipto\avariablebis$. There are three subcases:
         \begin{itemize}
         \item $\neg\alloc{\avariable}$ occurs in $\aformula$. Following the same argument as above, we can assume that $\neg\alloc{\avariable}$ occurs
         in $\aformula^{(n)}$. Assuming by absurd $(\aformula^{(n)}\wedge\avariable\Ipto\avariablebis)*\aformulabis^{(n)}$, we get a contradiction 
         by
         the axioms~\ref{coreAx:PointAlloc} and~\ref{starAx:False}.
         \item $\alloc{\avariable}$ occurs both in $\aformula$ and $\aformulabis$. Then $\avariable\neq\avariable$ occurs in $\aformulater$, so
         $\aformulater\implies\aformula*\aformulabis$
         \item $\alloc{\avariable}$ occurs in $\aformula$ but not in $\aformulabis$. Since $\aformulabis$ is satisfiable, $\neg\avariable\Ipto\avariablebis$
         occurs in $\aformulabis$, therefore $\neg\avariable\Ipto\avariablebis$ is a literal of $\aformulater$.
         Assuming by absurd $(\aformula^{(n)}\wedge\avariable\Ipto\avariablebis)*\aformulabis^{(n)}$, we get $\avariable\Ipto\avariablebis$ 
         by
         the axiom~\ref{starAx:MonoCore}, and the contradiction with $\aformulater$.
         \end{itemize}        
   \end{itemize}
\end{enumerate}       
\end{itemize}

\end{proof}

\subsection{Proof of Theorem~\ref{theo:starCompleteness}}
\theostarCompleteness*

\begin{proof}
\input{appendixproofs/theo-starPSLelim}
\end{proof}

\subsection{Proof of Soundness of $\coresys(\separate,\magicwand)$}\label{appendix:PSLSoundness}
We prove Lemma~\ref{lemma:magicwandPSLvalid}.
By showing Lemma~\ref{lemma:magicwandPSLvalid}, we also show
soundness of the restriction of the proof system.
%% Propositions~\ref{lemma:corePSLvalid} and~\ref{lemma:starPSLvalid}.

\begin{restatable}{lemma}{lemmamagicwandPSLvalid}\label{lemma:magicwandPSLvalid}
$\magicwandsys$ is sound.
\end{restatable}
\begin{proof}
Recall that intermediate axioms, such as \ref{coreAx:AllocSize}, do not need to be proved semantically as they are provable tautologies in $\coresys(\separate,\magicwand)$.
The axioms~\ref{coreAx:EqRef},
%\ref{coreAx:EqSymm},
\ref{coreAx:PointAlloc} and \ref{coreAx:PointInj} were already discussed in the body of the paper and their validity should be straightforward.
Moreover, the validity of the axioms~\ref{starAx:Commute},~\ref{starAx:Assoc} and~\ref{starAx:False}
and the three rules (\ref{rule:starinference},~\ref{rule:staradj} and~\ref{rule:magicwandadj}) is inherited from Boolean BI 
(see~\cite{Brotherston&Villard14} and~\cite[Section 2]{Galmiche&Larchey06}).

\begin{itemize}
\item The proof of every instantiation of \ref{starAx:MonoCore} is similar (and quite easy), therefore we show just the case of $\avariable \Ipto \avariablebis \separate \true \implies \avariable \Ipto \avariablebis$.
Suppose $\pair{\astore}{\aheap} \models \avariable \Ipto \avariablebis \separate \true$. Then there is a subheap $\aheap_1 \sqsubseteq \aheap$ such that $\pair{\astore}{\aheap_1} \models \avariable \Ipto \avariablebis$.
Hence, $\aheap_1(\astore(\avariable)) = \astore(\avariablebis)$.
As $\aheap_1 \sqsubseteq \aheap$, we obtain  $\aheap(\astore(\avariable)) = \astore(\avariablebis)$ which by definition implies $\pair{\astore}{\aheap} \models \avariable \Ipto \avariablebis$.
\item \ref{starAx:AllocNeg}.
Suppose $\pair{\astore}{\aheap} \models \lnot \alloc{\avariable} \separate \lnot \alloc{\avariable}$. Then there are
two disjoint heaps $\aheap_1,\aheap_2$ such that $\aheap = \aheap_1 + \aheap_2$, $\pair{\astore}{\aheap_1} \models \lnot \alloc{\avariable}$ and $\pair{\astore}{\aheap_2} \models \lnot \alloc{\avariable}$.
Then $\astore(\avariable) \not \in \domain{\aheap_1}$ and $\astore(\avariable) \not \in \domain{\aheap_2}$.
Since $\aheap = \aheap_1 + \aheap_2$, $\domain{\aheap} = \domain{\aheap_1}\cup\domain{\aheap_2}$ and therefore
$\astore(\avariable) \not \in \domain{\aheap}$.
We conclude that $\pair{\astore}{\aheap} \models \lnot \alloc{\avariable}$.
\item \ref{starAx:PointsNeg}.
Suppose $\pair{\astore}{\aheap} \models (\alloc{\avariable} \land \lnot \avariable \Ipto \avariablebis) \separate \true$.
Then there is a subheap $\aheap_1 \sqsubseteq \aheap$ such that $\pair{\astore}{\aheap_1} \models \alloc{\avariable} \land \lnot \avariable \Ipto \avariablebis$.
Hence, $\astore(\avariable) \in \domain{\aheap_1}$ and $\aheap_1(\astore(\avariable)) \neq \astore(\avariablebis)$.
As $\aheap_1 \sqsubseteq \aheap$, we obtain  $\astore(\avariable) \in \domain{\aheap}$ and $\aheap(\astore(\avariable)) \neq \astore(\avariablebis)$ which by definition implies $\pair{\astore}{\aheap} \models \lnot \avariable \Ipto \avariablebis$.
\item \ref{starAx:AllocSizeOne}. Suppose $\pair{\astore}{\aheap} \models \alloc{\avariable}$.
Then $\astore(\avariable) \in \domain{\aheap}$. Let $\aheap_1 \egdef \{\astore(\avariable)\pto\aheap(\astore(\avariable))\}$. Trivially, $\aheap_1 \sqsubseteq \aheap$ and
$\pair{\astore}{\aheap_1} \models \alloc{\avariable} \land \size = 1$.
We define $\aheap_2$ as the heap such that $\aheap_2 + \aheap_1 = \aheap$.
Trivially, $\pair{\astore}{\aheap_2} \models \true$.
Hence, $\pair{\astore}{\aheap} \models (\alloc{\avariable} \land \size = 1) \separate \true$.

The proof of validity of \ref{starAx:SizeOne} is similar.
\item \ref{starAx:SizeNeg}.
We suppose that $\inbound_1,\inbound_2\geq 1$, as the formula $\lnot \size \geq 0$ is by definition $\lnot \true$ and therefore is unsatisfiable.
Hence, the axiom~\ref{starAx:SizeNeg} is trivially valid by the axiom~\ref{starAx:False} for $\inbound_1$ and $\inbound_2$ equal to $0$.
Suppose $\pair{\astore}{\aheap} \models \lnot \size \geq \inbound_1 \separate \lnot \size \geq \inbound_2$.
Then there are two disjoint heaps $\aheap_1,\aheap_2$ such that $\aheap_1 + \aheap_2 = \aheap$, $\pair{\astore}{\aheap_1} \models \lnot \size \geq \inbound_1$ and $\pair{\astore}{\aheap_2} \models \lnot \size \geq \inbound_2$.
Then, by definition of $\size$, $\card{\domain{\aheap_1}} \leq \inbound_1-1$ and $\card{\domain{\aheap_2}} \leq \inbound_2-1$.
Then, as $\domain{\aheap} = \domain{\aheap_1}\cup\domain{\aheap_2}$, we obtain $\card{\domain{\aheap}} \leq \inbound_1+\inbound_2-2$, which implies
$\pair{\astore}{\aheap} \models \lnot \size \geq \inbound_1+\inbound_2 \dotminus 1$.
\item \ref{starAx:SizeTwo}. Suppose $\pair{\astore}{\aheap} \models \alloc{\avariable} \land \alloc{\avariablebis} \land \avariable \neq \avariablebis$. Then 
by definition,
$\astore(\avariable) \neq \astore(\avariablebis)$ and both $\astore(\avariable)$ and $\astore(\avariablebis)$ are in $\domain{\aheap}$. Hence $\card{\domain{\aheap}} \geq 2$, which implies $\pair{\astore}{\aheap} \models \size \geq 2$.
%%
%% SD 17/02/19
%% The axioms do not seem to be there anymore.
%% 
\cut{
\item \ref{wandAx:Emp}. Suppose $\pair{\astore}{\aheap} \models \emp \magicwand \aformula$.
Then for every $\aheap'\perp\aheap$ such that $\domain{\aheap'} = \emptyset$, $\pair{\astore}{\aheap+\aheap'} \models \aformula$.
However $\aheap + \aheap' = \aheap$ as $\aheap'$ is empty and therefore $\pair{\astore}{\aheap} \models \aformula$.
\item \ref{wandAx:GroundAlloc}.
Suppose $\pair{\astore}{\aheap} \models (\alloc{\avariable} \magicwand \bottom)$. Then for every $\aheap_1\perp\aheap$ such that $\astore(\avariable) \in \domain{\aheap_1}$, $\pair{\astore}{\aheap+\aheap'} \models \bottom$.
$\bottom$ is unsatisfiable, we then deduce that the set of heaps that is dijoint from $\aheap$ and have $\astore(\avariable)$ in their domain must be empty. We then conclude that $\astore(\avariable) \in \domain{\aheap}$ and therefore $\pair{\astore}{\aheap} \models \alloc{\avariable}$.
}
\item \ref{wandAx:Size}. Let $\asetvar\subseteq_\fin\PVAR$ and  $\pair{\astore}{\aheap}$ be a memory state.
Let $\aheap_1$ be a heap of size one such that $\aheap_1(\alocation) = \alocation$ for some $\alocation \not \in \domain{\aheap}\cup\astore(\asetvar)$.
Trivially $\pair{\astore}{\aheap_1}\models \size = 1 \land \bigwedge_{\avariable \in \asetvar} \lnot \alloc{\avariable}$.
Moreover $\aheap_1\perp\aheap$ holds, hence $\aheap_1+\aheap_2$ is defined and $\pair{\astore}{\aheap+\aheap_1} \models \true$.
Then, $\pair{\astore}{\aheap} \models (\size = 1 \land \bigwedge_{\avariable \in \asetvar} \lnot \alloc{\avariable}) \septraction \true$.
\item \ref{wandAx:PointsTo}. Suppose $\pair{\astore}{\aheap} \models \lnot \alloc{\avariable}$.
Let $\aheap_1$ be the heap of size one such that $\aheap_1(\astore(\avariable)) = \astore(\avariablebis)$.
Trivially, $\pair{\astore}{\aheap} \models \avariable \Ipto \avariablebis \land \size = 1$. Moreover, as $\astore(\avariable) \not\in\domain{\aheap}$, $\aheap_1\perp\aheap$ holds, hence $\aheap_1+\aheap_2$ is defined and $\pair{\astore}{\aheap+\aheap_1} \models \true$.
Then, $\pair{\astore}{\aheap} \models (\avariable \Ipto \avariablebis \land \size=1) \septraction \true$.
\item \ref{wandAx:Alloc}. Let $\asetvar \subseteq_\fin \PVAR$ and
suppose $\pair{\astore}{\aheap} \models \lnot \alloc{\avariable}$.
Let $\aheap_1$ be the heap of size one such that $\aheap_1(\astore(\avariable)) = \alocation$ where $\alocation \not \in \astore(\asetvar)$.
Trivially, $\pair{\astore}{\aheap_1} \models \alloc{\avariable} \land \size = 1 \land \bigwedge_{\avariablebis \in \asetvar} \lnot \avariable \Ipto \avariablebis$.
Moreover, as $\astore(\avariable) \not\in\domain{\aheap}$, $\aheap_1\perp\aheap$ holds, hence $\aheap+\aheap_1$ is defined and $\pair{\astore}{\aheap+\aheap_1} \models \true$.
Then, $\pair{\astore}{\aheap} \models (\alloc{\avariable} \land \size = 1 \land \bigwedge_{\avariablebis \in \asetvar} \lnot \avariable \Ipto \avariablebis) \septraction \true$.\qedhere
\end{itemize}

\end{proof}

\subsection{Proof of Proposition~\ref{prop:admissible-axioms-2}}
\label{appendix-proposition-admissible-axioms-2}
%% \propadmissibleaxiomstwo*

\begin{restatable}{proposition}{propadmissibleaxiomstwo}\label{prop:admissible-axioms-2}
The axioms~\ref{starAx:DistrOr},~\ref{starAx:False},~\ref{starAx:StarAlloc} and~\ref{starAx:DoubleAlloc} are derivable
in $\coresys(\separate,\magicwand)$.
\end{restatable}

\begin{proof}
\input{appendixproofs/proposition-admissible-axioms-2}
\end{proof}

%% \subsection{Proof of Lemma~\ref{lemma:septractioncongruence}}
%% \lemmaseptractioncongruence*
%%

\subsection{Proof of Lemma~\ref{lemma:magicwandPSLelim}}
\label{appendix-proof-lemma-magicwandPSLelim}

\begin{proof}(of Lemma~\ref{lemma:magicwandPSLelim})

SD: This proof needs to be significantly polished and completed to be able to be followed
smoothly (existence of Lemma~\ref{lemma:septractionadmissiblebis}  could contribute to this).

If either $\aformula$ or $\aformulabis$ is unsatisfiable, then $\prove_{\magicwandsys}
\aformula\septraction\aformulabis \implies \bot$ by using Lemma~\ref{lemma:corePSLtwo}
and the admissible axioms~\ref{mwAx:ImpL} and~\ref{mwAx:ImpR} from Lemma~\ref{lemma:septractionadmissible}.
So, in that case, it is enough  to take $\aformulater$ equal to $\lnot \avariable = \avariable$. Otherwise,
let $\aformulater$ be the formula introduced in Lemma~\ref{lemma:coreformulaseptraction}.
  \begin{itemize}
  \item Let us first show that $\prove_{\magicwandsys} \aformula\septraction\aformulabis\implies\aformulater$.
   $$
   \begin{array}{l|ll}
   1 & \neg \aformulater \separate \aformula \implies \neg \aformulabis 
   & \mbox{Completeness of $\starsys$} \\
   2 & \neg \aformulater \implies (\aformula \magicwand \neg \aformulabis)
   & \mbox{\ref{rule:staradj}, 1} \\
   3 & \neg (\aformula \magicwand \neg \aformulabis) \implies \aformulater
   & \mbox{Prop. reasoning, 2} \\
   4 & (\aformula \septraction \aformulabis) \implies \aformulater
   & \mbox{Def. $\septraction$, 3} 
   \end{array}
   $$
%% SD 06/05/20 -- previous version
\cut{
    By definition of $\septraction$, 
    the formula $\aformula\septraction\aformulabis\implies\aformulater$
    is propositionnally equivalent to $\neg\aformulater\implies\aformula\magicwand\neg\aformulabis$. By the rule~\ref{rule:staradj},
    this
    formula derives from $\aformula*\neg\aformulater\implies\neg\aformulabis$,
    which is valid by Lemma~\ref{lemma:coreformulaseptraction}. 
    So $\prove_{\starsys}\aformula*\neg\aformulater\implies\neg\aformulabis$
    by Theorem~\ref{theo:starCompleteness}. Finally, by Lemma~\ref{lemma:admissible-axioms-2}, 
    $\prove_{\magicwandsys}\aformula \separate \neg\aformulater\implies\neg\aformulabis$.
}
  \item Let us now show that $\prove_{\magicwandsys} \aformulater\implies \aformula\septraction\aformulabis$.
    First, let us  note that, since $\aformulater \separate \aformula \implies \aformulabis$
    is valid (Lemma~\ref{lemma:coreformulaseptraction}),
    it is derivable in $\starsys{}$ (due to its completeness), and therefore, by the rule~\ref{rule:staradj},
    $\prove_{\magicwandsys}\aformulater\implies\aformula\magicwand\aformulabis$. From that, it follows that it is enough to show that
    $\aformulater\implies\aformula\septraction\top$ is derivable in $\magicwandsys$. Indeed,
    from $\aformulater\implies \aformula\septraction\top$ and $\aformulater\implies\aformula\magicwand\aformulabis$, we get by \ref{mwAx:Mix}
    that $\aformulater\implies\aformula\septraction\aformulabis$ is derivable too.

    Let us therefore prove that $\aformulater\implies\aformula\septraction\top$ is derivable.
    Without loss of generality, we assume that $\aformulater$ is satisfiable (otherwise, by completeness of $\starsys$, 
    $\aformulater\implies \aformula\septraction\top$ is derivable).
    This implies that $\aformula$, $\aformulabis$ and $\aformulater$ have exactly the same equalities and
    inequalities. 
    We reason by induction on the number of positive literals of the form $\alloc{\avariable}$
    occurring in $\aformula$.
    \begin{itemize}

    \item
      Assume no $\alloc{\avariable}$ occurs positively in $\aformula$. 
      The satisfiable formula $\aformula$ can be decomposed as follows
      $
      \aformula = \mathsf{UNALLOC}(\asetvar) \wedge \aformula_{\size} \wedge \aformula_{eq} \wedge \aformula_{\Ipto}
      $, 
      where
      \begin{itemize}
      \item $\mathsf{UNALLOC}(\asetvar) \egdef \bigwedge\{\neg\alloc{\avariable}\mid\avariable\in\asetvar\}$.
      \item $\aformula_{\size}$ is a satisfiable conjunction of size literals and therefore by 
       Lemma~\ref{lemma:septractionadmissiblebis}, 
        $$
        \prove_{\magicwandsys} (\mathsf{UNALLOC}(\asetvar) \land \aformula_{\size}) \septraction \true
        $$
       \item $\aformula_{eq}$ is a (satisfiable) conjunction of equalities and inequalities that occurs also
       in $\aformulabis$ and $\aformulater$. Since $\prove_{\magicwandsys} \aformulater \implies \aformula_{eq}$,
       using the admissible axioms~\ref{mwAx:SeptEq} and~\ref{mwAx:SeptIneq} as many times as 
       the number of literals in  $\aformula_{eq}$ (as well as the admissible rule~\ref{rule:imptr}), 
       we can conclude that
       $$
       \prove_{\magicwandsys} \aformulater \implies  (\mathsf{UNALLOC}(\asetvar) \land \aformula_{\size} \land \aformula_{eq}) 
       \septraction \true.
       $$
       It is worth noting that in the remaining cases below, we shall use this type of argument to deal with
       equalities and inequalities. 
       \item  $\aformula_{\Ipto}$ is a conjunction of negated literals of the form
              $\neg (\avariable \Ipto \avariable')$ with $\avariable, \avariable' \in \asetvar$. 
              By using the axiom~\ref{coreAx:PointAlloc} and propositional reasoning, we obtain
              $$
              \prove_{\magicwandsys} \mathsf{UNALLOC}(\asetvar) \implies \aformula_{\Ipto}.
              $$ 
              Using the admissible rule~\ref{mwAx:ImpL} with the above implication, we can conclude that 
       $$
       \prove_{\magicwandsys} \aformulater \implies  (\mathsf{UNALLOC}(\asetvar) \land \aformula_{\size} \land \aformula_{eq} \land
        \aformula_{\Ipto}) \septraction \true.
       $$
      \end{itemize}
%% SD 07/05/20 -- previous version. Part of the reasoning is now to be done in the proof
%% of Lemma~\label{lemma:septractionadmissiblebis}. 
\cut{
      Then, since $\aformula$ is satisfiable,
      $\aformula$ is either equivalent to $\mathsf{UNALLOC}(\asetvar)\wedge \size\geq\inbound_1$ or
      equivalent to $\mathsf{UNALLOC}(\asetvar)\wedge \size=\inbound_2$
      where $\mathsf{UNALLOC}(\asetvar) \egdef \bigwedge\{\neg\alloc{\avariable}\mid\avariable\in\asetvar\}$.
      Let $\inbound$ be either $\inbound_1+1$ or $\inbound_2$.
      Applying \ref{wandAx:Size} $\inbound$ times in conjunction with \ref{mwAx:ImpR},
      we get
      $$
      \underbrace{(\mathsf{UNALLOC}(\asetvar)\wedge\size=1) \septraction (\mathsf{UNALLOC}(\asetvar)\wedge\size=1) \septraction\ldots\septraction}_{\inbound\mbox{ times}}  \top.
      $$
      Applying~\ref{mwAx:Curry}, \ref{mwAx:ImpL} and reasoning in $\starsys{}$, we get
      $\prove_{\magicwandsys} (\mathsf{UNALLOC}(\asetvar)\wedge\size=\inbound)\septraction\top$, and finally 
      by~\ref{mwAx:ImpL} we get $\prove_{\magicwandsys} \aformula\septraction\top$.
}
      
    \item
      Assume $\alloc{\avariable}$ occurs positively in $\aformula$ together with $\avariable\Ipto\avariablebis$.
      Then, there is $\aformula'$ in $\coretype{\asetvar}{\bound}$ such that $\aformula\iff(\avariable\Ipto\avariablebis\wedge\size=1) \separate \aformula'$
      is valid (and therefore derivable in $\starsys$) and $\aformula'$ has at least one less 
      positive occurrences of literals of the form $\alloc{\avariableter}$.
      {\bf SD: If $\aformula$ contains $\size \geq \bound$, then how to guarantee that
      $\aformula'$ is a core type, as it may contain either $\size \geq \bound$ or $\size \geq \bound-1$?}
      Since $\aformulater\implies\aformula\septraction\top$ is valid ({\bf SD: why?}), so is 
      $\aformulater \separate (\avariable\Ipto\avariablebis\wedge\size=1)\implies\aformula'\septraction\top$.
      By the induction hypothesis ({\bf SD: What does it mean here? I stop updating the rest of the proof before solving 
      this.}), 
      $\aformulater \separate (\avariable\Ipto\avariablebis\wedge\size=1)\implies\aformula'\septraction\top$ is derivable.
      By definition of $\aformulater$, $\neg\alloc{\avariable}$ occurs in $\aformulater$.
      By using the axiom~\ref{wandAx:PointsTo}, we conclude
      $\prove_{\magicwandsys} \aformulater\implies(\avariable \Ipto \avariablebis \land \size = 1) \septraction \true$.
      On the other hand,
      $\aformulater\implies (\avariable \Ipto \avariablebis \land \size = 1) \magicwand \big((\avariable \Ipto \avariablebis \land \size = 1) * \aformulater\big)$
      is derivable by adjunction rule, so by \ref{mwAx:Mix},
      $$
      \aformulater\implies(\avariable \Ipto \avariablebis \land \size = 1) \septraction \big((\avariable \Ipto \avariablebis \land \size = 1) * \aformulater\big)
      $$
      is derivable. From this and $\prove_{\magicwandsys} 
      \aformulater \separate (\avariable\Ipto\avariablebis\wedge\size=1)\implies\aformula'\septraction\top$, we get by using the
      intermediate axiom~\ref{mwAx:ImpR}
      $$
      \prove_{\magicwandsys}  \aformulater\implies(\avariable \Ipto \avariablebis \land \size = 1) \septraction (\aformula'\septraction\top).
      $$
       Then, by~\ref{mwAx:Curry} and~\ref{mwAx:ImpL},  $\prove_{\magicwandsys} \aformulater\implies\aformula\septraction\top$.

    \item
      (SD: to present this derivation in the Hilberty-style)
      Assume $\alloc{\avariable}$ occurs positively in $\aformula$ but without any literal of the form $\avariable\Ipto\avariablebis$.
      Then there is $\aformula'$ in $\coretype{\asetvar}{\bound}$ such that $\aformula\iff(\alloc{\avariable}\wedge\mathsf{UNDEF}\wedge\size=1) \separate \aformula'$ is valid
      (and therefore derivable in $\starsys$),
      where $\mathsf{UNDEF}$ is $\bigwedge\{\neg\avariable\Ipto\avariablebis\mid\avariablebis\in \asetvar\}$
      and $\aformula'$ has at least one less positive occurrence of literals of the form $\alloc{\avariableter}$.
      Since $\aformulater\implies\aformula\septraction\top$ is valid ({\bf SD: why?}), so is
      $\aformulater*(\alloc{\avariable}\wedge\mathsf{UNDEF} \wedge\size=1)\implies\aformula'\septraction\top$.
      By induction hypothesis ({\bf SD: see above}), $\aformulater*(\alloc{\avariable}\wedge\mathsf{UNDEF}\wedge\size=1)\implies\aformula'\septraction\top$ is derivable.
      By definition of $\aformulater$, $\neg\alloc{\avariable}$ occurs in $\aformulater$.
      By using the axiom~\ref{wandAx:Alloc}, $\prove_{\magicwandsys} 
      \aformulater\implies(\alloc{\avariable}\wedge\mathsf{UNDEF}\land \size = 1) \septraction \true$.
      With the same reasoning as in previous item, we get
      $$
      \prove_{\magicwandsys}  \aformulater\implies(\alloc{\avariable}\wedge\mathsf{UNDEF} \land \size = 1) \septraction (\aformula'\septraction\top)
      $$
      Finally, by using the intermediate axioms~\ref{mwAx:Curry} and~\ref{mwAx:ImpL} $\prove_{\magicwandsys} 
      \aformulater\implies\aformula\septraction\top$. \qedhere
    \end{itemize}
  \end{itemize}
\end{proof}

%% \subsection{Proof of Theorem~\ref{theo:magicwandPSLelim}}
%% \theomagicwandPSLelim*
%% \begin{proof}
%% \input{appendixproofs/theo-magicwandPSLelim}
%% \end{proof}

 \subsection{Proof of Theorem~\ref{theo:PSLcompleteAx}}
 \theoPSLcompleteAx*
 \begin{proof}
 \input{appendixproofs/theo-PSLcompleteAx}

 \end{proof}
