# Supplementary material for: A Complete Axiomatisation for Quantifier-Free Separation Logic
Source: arXiv:2006.05156 source file (2021-08-09)
Supplement: Supplementary file 3 [file apdxsection-int-taut-eq.tex]

\subsubsection{\ref{axiom2:auxlemma1} and \ref{axiom2:beforelemma1}}
\begin{enumerate}[align=left]
\item[\lemmalab{Eq{$\Rightarrow\!$}Def}{axiom2:auxlemma1}] $\boxed{\aterm = \aterm' \implies \defined{\aterm}}$ Notice that then $\aterm = \aterm' \implies \defined{\aterm'}$ by symmetry axiom~\ref{core2Ax:EqSymm}.
\[
\begin{nd}
\hypo {1} {\aterm = \aterm'}
\have {2} {\aterm = \aterm' \land \aterm = \aterm'} \by{\landtwo}{1,1}
\have {3} {\aterm' = \aterm'\quad (\text{i.e. } \defined{\aterm'})} \by{\ref{core2Ax:Substitute}}{2}
\end{nd}
\]
\item[\lemmalab{BeforeIrref}{axiom2:beforelemma1}]
$\boxed{\lnot \before{\aterm}{\aterm}}$

Again, we consider the case of $\aterm$ meet-point expression.
\[
\begin{nd}
\hypo {1} {\before{\ameetvar{\avariable}{\avariablebis}{\avariableter}}{\ameetvar{\avariable}{\avariablebis}{\avariableter}}}
\have {2} {\defined{\ameetvar{\avariable}{\avariablebis}{\avariableter}}} \ae{1}
\have {3} {\ameetvar{\avariable}{\avariablebis}{\avariableter} \neq \ameetvar{\avariable}{\avariablebis}{\avariableter}} \ae{1}
\have {4} {\bottom} \by{\landcontr}{2,3}
\end{nd}
\]
\end{enumerate}
\subsubsection{Some auxiliary lemmata}
The following are auxiliary lemmata, used to prove more general results (provided below).
We reserve the prefix \textbf{Aux} for lemmata of this kind.
\begin{enumerate}[label=\textbf{Aux\arabic*},align=left]
\item\label{axiom2:auxlemma13}
$
\boxed{
\ameetvar{\avariable}{\avariablebis}{\avariableter} = \ameetvar{\avariablefour}{\avariablefifth}{\avariablesix} \land \defined{\ameetvar{\avariable}{\avariablebis}{\avariablesept}} \implies \ameetvar{\avariable}{\avariablebis}{\avariablesept} = \ameetvar{\avariablefour}{\avariablefifth}{\avariablesix}
}
$
\[
\begin{nd}
\hypo {1} {\ameetvar{\avariable}{\avariablebis}{\avariableter} = \ameetvar{\avariablefour}{\avariablefifth}{\avariablesix}}
\hypo {2} {\defined{\ameetvar{\avariable}{\avariablebis}{\avariablesept}}}
\have {3} {\defined{\ameetvar{\avariable}{\avariablebis}{\avariableter}}} \by{\ref{axiom2:auxlemma1}}{1}
\have {4} {\ameetvar{\avariable}{\avariablebis}{\avariablesept} = \ameetvar{\avariable}{\avariablebis}{\avariableter}} \by{\ref{core2Ax:EqDef}}{2,3}
\have {5} {\ameetvar{\avariable}{\avariablebis}{\avariablesept} = \ameetvar{\avariablefour}{\avariablefifth}{\avariablesix}} \by{\ref{core2Ax:Substitute}}{1,4}
\end{nd}
\]

\item\label{axiom2:auxlemmaPedDef}
$
\boxed{\defined{\ameetvar{\avariable}{\avariablebis}{\avariableter}} \implies \defined{\ameetvar{\avariableter}{\avariable}{\avariableter}}}
$
\[
\begin{nd}
\hypo {1} {\defined{\ameetvar{\avariable}{\avariablebis}{\avariableter}}}
\have {2} {\avariableter = \ameetvar{\avariableter}{\avariableter}{\avariableter}} \by{\ref{core2Ax:Self}}{}
\have {3} {\defined{\ameetvar{\avariableter}{\avariableter}{\avariableter}}} \by{\ref{axiom2:auxlemma1}}{2}
\have {4} {\defined{\ameetvar{\avariableter}{\avariable}{\avariableter}}} \by{\ref{core2Ax:PedDefines}}{1,3}
\end{nd}
\]

\item\label{axiom2:auxlemma11}
$
\boxed{
\ameetvar{\avariable}{\avariablebis}{\avariableter} = \ameetvar{\avariablefour}{\avariablefifth}{\avariablesix} \implies \ameetvar{\avariable}{\avariablebis}{\avariablesix} = \ameetvar{\avariablefour}{\avariablefifth}{\avariablesix}
}
$

By symmetry (axiom~\ref{core2Ax:EqSymm}) then $\ameetvar{\avariable}{\avariablebis}{\avariableter} = \ameetvar{\avariablefour}{\avariablefifth}{\avariablesix} \Rightarrow \ameetvar{\avariable}{\avariablebis}{\avariableter} = \ameetvar{\avariablefour}{\avariablefifth}{\avariableter}$ is a tautology.
\[
\begin{nd}
\hypo {1} {\ameetvar{\avariable}{\avariablebis}{\avariableter} = \ameetvar{\avariablefour}{\avariablefifth}{\avariablesix}}
\have {3} {\defined{\ameetvar{\avariable}{\avariablebis}{\avariablesix}}} \by{\ref{core2Ax:PedInv}}{1}
\have {5} {\ameetvar{\avariable}{\avariablebis}{\avariablesix} = \ameetvar{\avariablefour}{\avariablefifth}{\avariablesix}} \by{\ref{axiom2:auxlemma13}}{1,3}
\end{nd}
\]

\item\label{axiom2:auxlemma6}
$
\boxed{
\symmetric{\ameetvar{\avariable}{\avariablebis}{\avariableter}} \land \symmetric{\ameetvar{\avariable}{\avariablefour}{\avariableter}} \implies \symmetric{\ameetvar{\avariablebis}{\avariablefour}{\avariableter}}
}
$
\[
\begin{nd}
\hypo {1} {\symmetric{\ameetvar{\avariable}{\avariablebis}{\avariableter}}}
\hypo {2} {\symmetric{\ameetvar{\avariable}{\avariablefour}{\avariableter}}}
\have {3} {\defined{\ameetvar{\avariablebis}{\avariable}{\avariableter}}} \by{\ref{axiom2:auxlemma1}}{1}
\have {4} {\defined{\ameetvar{\avariablefour}{\avariable}{\avariableter}}} \by{\ref{axiom2:auxlemma1}}{2}
\have {5} {\defined{\ameetvar{\avariablebis}{\avariablefour}{\avariableter}}} \by{\ref{core2Ax:PedDefines}}{3,4}
\open
\hypo {6} {\asymmetric{\ameetvar{\avariablebis}{\avariablefour}{\avariableter}}}
\have {7} {\ameetvar{\avariablebis}{\avariablefour}{\avariableter} \neq \ameetvar{\avariablefour}{\avariablebis}{\avariableter}} \ae{6}
\have {8} {\ameetvar{\avariable}{\avariablefour}{\avariableter} = \ameetvar{\avariablebis}{\avariablefour}{\avariableter} \land \ameetvar{\avariablefour}{\avariable}{\avariableter} = \ameetvar{\avariablefour}{\avariablebis}{\avariableter}} \by{\ref{core2Ax:OneAsym}}{2,6}
\have {9} {\ameetvar{\avariable}{\avariablefour}{\avariableter} = \ameetvar{\avariablebis}{\avariablefour}{\avariableter}} \ae{8}
\have {10}
{\ameetvar{\avariablefour}{\avariable}{\avariableter} = \ameetvar{\avariablefour}{\avariablebis}{\avariableter}} \ae{8}
\have {11} {\ameetvar{\avariablebis}{\avariablefour}{\avariableter} \neq \ameetvar{\avariablefour}{\avariable}{\avariableter}} \by{\ref{core2Ax:Substitute}}{7,10}
\have {12} {\ameetvar{\avariable}{\avariablefour}{\avariableter} \neq \ameetvar{\avariablefour}{\avariable}{\avariableter}} \by{\ref{core2Ax:Substitute}}{9,11}
\have {13} {\bottom} \by{\landcontr}{2,12}
\close
\have {14} {\lnot\asymmetric{\ameetvar{\avariablebis}{\avariablefour}{\avariableter}}} \ni{6-13}
\have {15} {\symmetric{\ameetvar{\avariablebis}{\avariablefour}{\avariableter}}} \by{\modusponens}{5,14}
\end{nd}
\]

\item\label{axiom2:auxlemma100}
$\boxed{\symmetric{\ameetvar{\avariable}{\avariablebis}{\avariableter}} \land \defined{\ameetvar{\avariable}{\avariablebis}{\avariablefour}} \implies \symmetric{\ameetvar{\avariable}{\avariablebis}{\avariablefour}}}$
\[
\begin{nd}
\hypo {1} {\symmetric{\ameetvar{\avariable}{\avariablebis}{\avariableter}}}
\hypo {2} {\defined{\ameetvar{\avariable}{\avariablebis}{\avariablefour}}}
\have {3} {\defined{\ameetvar{\avariablebis}{\avariable}{\avariableter}}} \by{\ref{core2Ax:Bothdef}}{2}
\have {4} {\ameetvar{\avariable}{\avariablebis}{\avariablefour} = \ameetvar{\avariablebis}{\avariable}{\avariableter}} \by{\ref{axiom2:auxlemma13}}{1,2}
\have {5} {\ameetvar{\avariable}{\avariablebis}{\avariablefour} = \ameetvar{\avariablebis}{\avariable}{\avariablefour}} \by{\ref{axiom2:auxlemma13}}{3,4}
\end{nd}
\]
\item\label{axiom2:auxlemma2}
$
\boxed{
\begin{aligned}[t]
\ameetvar{\avariable}{\avariablefour}{\avariableter} = \ameetvar{\avariablebis}{\avariablefour}{\avariableter}
\implies &
\symmetric{\ameetvar{\avariable}{\avariablebis}{\avariableter}} \land (\ameetvar{\avariable}{\avariablebis}{\avariableter}=\ameetvar{\avariable}{\avariablefour}{\avariableter} \lor\\
&
\before{\ameetvar{\avariable}{\avariablebis}{\avariableter}}{\ameetvar{\avariable}{\avariablefour}{\avariableter}})
\end{aligned}}
$
\[
\begin{nd}
\hypo {1} {\ameetvar{\avariable}{\avariablefour}{\avariableter} = \ameetvar{\avariablebis}{\avariablefour}{\avariableter}}
\have {2} {\symmetric{\ameetvar{\avariable}{\avariablebis}{\avariableter}}} \by{\ref{core2Ax:Symmetric}}{1}
\have {3} {\ameetvar{\avariable}{\avariablebis}{\avariableter} = \ameetvar{\avariable}{\avariablefour}{\avariableter} \lor\\ \ameetvar{\avariable}{\avariablebis}{\avariableter} \neq \ameetvar{\avariable}{\avariablefour}{\avariableter}}
\by{\trivialtrue}{}
\open
\hypo {A4} {\ameetvar{\avariable}{\avariablebis}{\avariableter} = \ameetvar{\avariable}{\avariablefour}{\avariableter}}
\have {A5} {\ameetvar{\avariable}{\avariablebis}{\avariableter} = \ameetvar{\avariable}{\avariablefour}{\avariableter} \lor\\ \before{\ameetvar{\avariable}{\avariablebis}{\avariableter}}{\ameetvar{\avariable}{\avariablefour}{\avariableter}}} \oi{A4}
\close
\end{nd}
\]
\[
\begin{ndresume}
\open
\hypo {B4} {\ameetvar{\avariable}{\avariablebis}{\avariableter} \neq \ameetvar{\avariable}{\avariablefour}{\avariableter}}
\have {B5} {\ameetvar{\avariable}{\avariablebis}{\avariableter} \neq \ameetvar{\avariablebis}{\avariablefour}{\avariableter}} \by{\ref{core2Ax:Substitute}}{1,B4}
\have {B7} {\defined{\ameetvar{\avariablebis}{\avariablefour}{\avariableter}}} \by{\ref{axiom2:auxlemma1}}{1}
\have {B8} {\before{\ameetvar{\avariable}{\avariablebis}{\avariableter}}{\ameetvar{\avariable}{\avariablefour}{\avariableter}}} \by{\defofbefore}{2,B7,B4,B5}
\have {B9} {\ameetvar{\avariable}{\avariablebis}{\avariableter} = \ameetvar{\avariable}{\avariablefour}{\avariableter} \lor\\ \before{\ameetvar{\avariable}{\avariablebis}{\avariableter}}{\ameetvar{\avariable}{\avariablefour}{\avariableter}}} \oi{B8}
\close
\have {4} {\ameetvar{\avariable}{\avariablebis}{\avariableter} = \ameetvar{\avariable}{\avariablefour}{\avariableter} \lor\\ \before{\ameetvar{\avariable}{\avariablebis}{\avariableter}}{\ameetvar{\avariable}{\avariablefour}{\avariableter}}}
  \oe{3,A4-A5,B4-B9}
\have {5} {\symmetric{\ameetvar{\avariable}{\avariablebis}{\avariableter}} \land (\ameetvar{\avariable}{\avariablebis}{\avariableter}=\ameetvar{\avariable}{\avariablefour}{\avariableter} \lor\\
\before{\ameetvar{\avariable}{\avariablebis}{\avariableter}}{\ameetvar{\avariable}{\avariablefour}{\avariableter}})} \by{\ndref{2} $\land$ \ndref{4}}{}
\end{ndresume}
\]
% \item\label{axiom2:auxlemma4}
% $
% \boxed{
% \before{\ameetvar{\avariable}{\avariablebis}{\avariableter}}{\ameetvar{\avariable}{\avariablefour}{\avariablefifth}}
% \implies
% \defined{\ameetvar{\avariable}{\avariablebis}{\avariablefifth}}}
% $
% \[
% \begin{nd}
% \hypo {1} {\before{\ameetvar{\avariable}{\avariablebis}{\avariableter}}{\ameetvar{\avariable}{\avariablefour}{\avariablefifth}}}
% \have {2} {\defined{\ameetvar{\avariable}{\avariablebis}{\avariablefifth}}} \ae{1}
% \end{nd}
% \]
\item\label{axiom2:auxlemma9}
$\boxed{
\begin{aligned}[t]
&\before{\ameetvar{\avariable}{\avariablebis}{\avariableter}}{\ameetvar{\avariable}{\avariablefour}{\avariablefifth}} \land \defined{\ameetvar{\avariable}{\avariablebis}{\avariablesix}}
\implies\\
&\before{\ameetvar{\avariable}{\avariablebis}{\avariablesix}}{\ameetvar{\avariable}{\avariablefour}{\avariablefifth}}
\end{aligned}}$
\[
\begin{nd}
\hypo {1} {\before{\ameetvar{\avariable}{\avariablebis}{\avariableter}}{\ameetvar{\avariable}{\avariablefour}{\avariablefifth}}}
\hypo {2} {\defined{\ameetvar{\avariable}{\avariablebis}{\avariablesix}}}
\have {3} {\symmetric{\ameetvar{\avariable}{\avariablebis}{\avariableter}}}
\ae{1}
\have {3b} {\defined{\ameetvar{\avariable}{\avariablebis}{\avariablefifth}}}
\ae{1}
\have {3c} {\defined{\ameetvar{\avariable}{\avariablefour}{\avariablefifth}}}
\ae{1}
\have {4}
{\ameetvar{\avariable}{\avariablebis}{\avariableter} \neq \ameetvar{\avariable}{\avariablefour}{\avariablefifth}
\land \ameetvar{\avariable}{\avariablebis}{\avariableter} \neq \ameetvar{\avariablebis}{\avariablefour}{\avariablefifth}}
\ae{1}
\have {4b} {\defined{\ameetvar{\avariablebis}{\avariable}{\avariablesix}}} \by{\ref{core2Ax:Bothdef}}{2}
\have {4c} {\ameetvar{\avariablebis}{\avariable}{\avariablesix} = \ameetvar{\avariablebis}{\avariable}{\avariableter}} \by{\ref{core2Ax:EqDef}}{3,4b}
\have {5} {\ameetvar{\avariable}{\avariablebis}{\avariablesix} = \ameetvar{\avariablebis}{\avariable}{\avariableter}}
\by{\ref{core2Ax:Substitute}}{2,3}
\have {5b} {\symmetric{\ameetvar{\avariable}{\avariablebis}{\avariablesix}}}
\by{\ref{core2Ax:Substitute}}{4c,5}
\have {5c} {\ameetvar{\avariable}{\avariablebis}{\avariableter} = \ameetvar{\avariable}{\avariablebis}{\avariablesix} } \by{\ref{core2Ax:EqDef}}{2,3}
\have {6} {\ameetvar{\avariable}{\avariablebis}{\avariablesix} \neq \ameetvar{\avariable}{\avariablefour}{\avariablefifth}
\land \ameetvar{\avariable}{\avariablebis}{\avariablesix} \neq \ameetvar{\avariablebis}{\avariablefour}{\avariablefifth}}
\by{\ref{core2Ax:Substitute}}{4,5c}
\have {7} {\before{\ameetvar{\avariable}{\avariablebis}{\avariablesix}}{\ameetvar{\avariable}{\avariablefour}{\avariablefifth}}} \by{\defofbefore}{3b,3c,5b,6}
\end{nd}
\]

\end{enumerate}
\subsubsection{\ref{axiom2:auxlemma7}}
\begin{enumerate}[align=left]
\item[\lemmalab{AsymIsBot}{axiom2:auxlemma7}]
$
\boxed{
\begin{aligned}[t]
\defined{\ameetvar{\avariable}{\avariablebis}{\avariableter}} \land \asymmetric{\ameetvar{\avariable}{\avariablefour}{\avariableter}} \land \ameetvar{\avariable}{\avariablebis}{\avariableter} \neq \ameetvar{\avariable}{\avariablefour}{\avariableter}
\implies\\
\before{\ameetvar{\avariable}{\avariablebis}{\avariableter}}{\ameetvar{\avariable}{\avariablefour}{\avariableter}}
\end{aligned}}
$
\[
\begin{nd}
\hypo {1} {\defined{\ameetvar{\avariable}{\avariablebis}{\avariableter}}}
\hypo {2} {\asymmetric{\ameetvar{\avariable}{\avariablefour}{\avariableter}}}
\hypo {3} {\ameetvar{\avariable}{\avariablebis}{\avariableter} \neq \ameetvar{\avariable}{\avariablefour}{\avariableter}}
\open
\hypo {A5} {\ameetvar{\avariable}{\avariablebis}{\avariableter} \neq \ameetvar{\avariablebis}{\avariable}{\avariableter}}
\have {A6} {\asymmetric{\ameetvar{\avariable}{\avariablebis}{\avariableter}}} \by{\ndref{1} $\land$ \ndref{A5}}{}
\have {A7} {\ameetvar{\avariable}{\avariablebis}{\avariableter} = \ameetvar{\avariable}{\avariablefour}{\avariableter}} \by{\ref{core2Ax:BothAsym}}{2,A6}
\have {A8} {\bottom} \by{\landcontr}{3,A7}
\close
\end{nd}
\]
\[
\begin{ndresume}
\have {B5} {\ameetvar{\avariable}{\avariablebis}{\avariableter} = \ameetvar{\avariablebis}{\avariable}{\avariableter}} \ni{A5-A8}
\have {B6} {\symmetric{\ameetvar{\avariable}{\avariablebis}{\avariableter}}}  \by{1 $\land$ 5}{}
\have {B7} {\ameetvar{\avariable}{\avariablefour}{\avariableter} = \ameetvar{\avariablebis}{\avariablefour}{\avariableter}} \by{\ref{core2Ax:OneAsym}}{2,B6}
\have {B8} {\defined{\ameetvar{\avariable}{\avariablefour}{\avariableter}}} \ae{2}
\have {B10} {\ameetvar{\avariable}{\avariablebis}{\avariableter} \neq \ameetvar{\avariablebis}{\avariablefour}{\avariableter}} \by{\ref{core2Ax:Substitute}}{3,B7}
\have {B11} {\before{\ameetvar{\avariable}{\avariablebis}{\avariableter}}{\ameetvar{\avariable}{\avariablefour}{\avariableter}}}
\by{\ndref{3} $\land$ \ndref{B6} $\land$ \ndref{B8} $\land$ \ndref{B10}}{}
\end{ndresume}
\]
\end{enumerate}

\subsubsection{\ref{axiom2:auxlemma3}}
\begin{enumerate}[align=left]
\item[\lemmalab{Var$\leq$Meet}{axiom2:auxlemma3}]
$
\boxed{
\begin{aligned}[t]
&\defined{\ameetvar{\avariable}{\avariablebis}{\avariableter}}
\implies\\
&\avariable = \ameetvar{\avariable}{\avariablebis}{\avariableter} \lor \before{\avariable}{\ameetvar{\avariable}{\avariablebis}{\avariableter}}
\end{aligned}}
$
\[
\begin{nd}
\hypo {1} {\defined{\ameetvar{\avariable}{\avariablebis}{\avariableter}}}
\have {2} {\avariable = \ameetvar{\avariable}{\avariable}{\avariable}} \by{\ref{core2Ax:Self}}{}
\have {3} {\defined{\ameetvar{\avariable}{\avariable}{\avariable}}} \by{\ref{axiom2:auxlemma1}}{2}
\have {mm} {\defined{\ameetvar{\avariable}{\avariablebis}{\avariableter}} \land \defined{\ameetvar{\avariable}{\avariablebis}{\avariableter}}} \by{\landtwo}{1}
\have {5} {\defined{\ameetvar{\avariable}{\avariable}{\avariableter}}} \by{\ref{core2Ax:PedDefines}}{mm}
\have {6} {\ameetvar{\avariable}{\avariable}{\avariableter} = \ameetvar{\avariable}{\avariable}{\avariable}} \by{\ref{core2Ax:EqDef}}{3,5}
\have {4}
{\symmetric{\ameetvar{\avariable}{\avariable}{\avariableter}} \land (\ameetvar{\avariable}{\avariable}{\avariableter}=\ameetvar{\avariable}{\avariablebis}{\avariableter} \lor\\
\before{\ameetvar{\avariable}{\avariable}{\avariableter}}{\ameetvar{\avariable}{\avariablebis}{\avariableter}})
} \by{\ref{axiom2:auxlemma2}}{1}
\have {8}
{\ameetvar{\avariable}{\avariable}{\avariableter}=\ameetvar{\avariable}{\avariablebis}{\avariableter} \lor\\
\before{\ameetvar{\avariable}{\avariable}{\avariableter}}{\ameetvar{\avariable}{\avariablebis}{\avariableter}}
} \ae{4}
\have {9}
{\ameetvar{\avariable}{\avariable}{\avariable}=\ameetvar{\avariable}{\avariablebis}{\avariableter} \lor\\
\before{\ameetvar{\avariable}{\avariable}{\avariable}}{\ameetvar{\avariable}{\avariablebis}{\avariableter}}
} \by{\ref{core2Ax:Substitute}}{6,8}
\have {10b} {\avariable = \ameetvar{\avariable}{\avariablebis}{\avariableter} \lor\\ \before{\ameetvar{\avariable}{\avariable}{\avariable}}{\ameetvar{\avariable}{\avariablebis}{\avariableter}}} \by{\ref{core2Ax:Substitute} and \lorimpL}{2,9}
\have {10} {\avariable = \ameetvar{\avariable}{\avariablebis}{\avariableter} \lor\\ \before{\avariable}{\ameetvar{\avariable}{\avariablebis}{\avariableter}}} \by{\defofbefore and \lorimpR}{2,10b}
\end{nd}
\]
\end{enumerate}

\subsubsection{\ref{axiom2:auxlemma5}}
\begin{enumerate}[align=left]
\item[\lemmalab{MeetOrder}{axiom2:auxlemma5}]
$
\boxed{
\begin{aligned}[t]
&\before{\ameetvar{\avariable}{\avariablebis}{\avariableter}}{\ameetvar{\avariable}{\avariablefour}{\avariablefifth}}
\implies\\
&\before{\ameetvar{\avariablebis}{\avariable}{\avariableter}}{\ameetvar{\avariablebis}{\avariablefour}{\avariablefifth}} \land \ameetvar{\avariable}{\avariablefour}{\avariablefifth} = \ameetvar{\avariablebis}{\avariablefour}{\avariablefifth}
\end{aligned}}
$
\[
\begin{nd}
\hypo {1} {\before{\ameetvar{\avariable}{\avariablebis}{\avariableter}}{\ameetvar{\avariable}{\avariablefour}{\avariablefifth}}}
\have {2a} {\defined{\ameetvar{\avariable}{\avariablebis}{\avariablefifth}}} \ae{1}
\have {2} {\before{\ameetvar{\avariable}{\avariablebis}{\avariablefifth}}{\ameetvar{\avariable}{\avariablefour}{\avariablefifth}}} \by{\ref{axiom2:auxlemma9}}{1,2a}
\have {2b} {\defined{\ameetvar{\avariablebis}{\avariable}{\avariablefifth}}} \by{\ref{core2Ax:Bothdef}}{2a}
\have {A1} {\symmetric{\ameetvar{\avariable}{\avariablebis}{\avariablefifth}}} \ae{2}
\have {A2} {\defined{\ameetvar{\avariable}{\avariablefour}{\avariablefifth}}} \ae{2}
\end{nd}
\]
\[
\begin{ndresume}
\have {A3} {\ameetvar{\avariable}{\avariablebis}{\avariablefifth} \neq \ameetvar{\avariable}{\avariablefour}{\avariablefifth}} \ae{2}
\have {A4} {\ameetvar{\avariable}{\avariablebis}{\avariablefifth} \neq \ameetvar{\avariablebis}{\avariablefour}{\avariablefifth}} \ae{2}
\open
  \hypo {H1} {\ameetvar{\avariable}{\avariablefour}{\avariablefifth} \neq \ameetvar{\avariablebis}{\avariablefour}{\avariablefifth}}
  \have {zz} {\ameetvar{\avariable}{\avariablebis}{\avariablefifth} = \ameetvar{\avariable}{\avariablefour}{\avariablefifth} \lor\\ \ameetvar{\avariable}{\avariablebis}{\avariablefifth} = \ameetvar{\avariablebis}{\avariablefour}{\avariablefifth}} \by{\ref{core2Ax:Before}}{A1,A2,H1}
  \have {zz1} {\ameetvar{\avariable}{\avariablebis}{\avariablefifth} = \ameetvar{\avariablebis}{\avariablefour}{\avariablefifth}} \by{\modusponens}{A3,zz}
  \have {zz2} {\bottom} \by{\landcontr}{A4,zz1}
\close
\have {6} {\ameetvar{\avariable}{\avariablefour}{\avariablefifth} = \ameetvar{\avariablebis}{\avariablefour}{\avariablefifth}}
\ni{H1-zz2}
\have {6b} {\ameetvar{\avariablebis}{\avariable}{\avariablefifth} \neq \ameetvar{\avariable}{\avariablefour}{\avariablefifth}} \by{\ref{core2Ax:Substitute}}{A1,A3}
\have {6c} {\ameetvar{\avariablebis}{\avariable}{\avariablefifth} \neq \ameetvar{\avariablebis}{\avariablefour}{\avariablefifth}} \by{\ref{core2Ax:Substitute}}{A1,A4}
\have {7} {\before{\ameetvar{\avariablebis}{\avariable}{\avariablefifth}}{\ameetvar{\avariablebis}{\avariablefour}{\avariablefifth}}} \by{\defofbefore}{A1,A2,6b,6c}
\have {7b} {\defined{\ameetvar{\avariable}{\avariablebis}{\avariableter}}} \ae{1}
\have {7c} {\defined{\ameetvar{\avariablebis}{\avariable}{\avariableter}}} \by{\ref{core2Ax:Bothdef}}{7b}
\have {8} {\before{\ameetvar{\avariablebis}{\avariable}{\avariableter}}{\ameetvar{\avariablebis}{\avariablefour}{\avariablefifth}}} \by{\ref{axiom2:auxlemma9}}{1,7c}
\have {9} {\before{\ameetvar{\avariablebis}{\avariable}{\avariableter}}{\ameetvar{\avariablebis}{\avariablefour}{\avariablefifth}} \land\\ \ameetvar{\avariable}{\avariablefour}{\avariablefifth} = \ameetvar{\avariablebis}{\avariablefour}{\avariablefifth}} \by{\ndref{6} $\land$ \ndref{8}}{}
\end{ndresume}
\]
\end{enumerate}
\subsubsection{\ref{axiom2:beforelemma0two}}
We want to prove that the following formula is a tautology:
\begin{nscenter}
$\before{\aterm_1}{\aterm_2} \land \aterm_2 = \aterm_3 \implies \before{\aterm_1}{\aterm_3}\qquad$ (\ref{axiom2:beforelemma0two})
\end{nscenter}
To simplify the proof, we first prove three intermediate results (\ref{axiom2:auxlemma12}, \ref{axiom2:auxlemma14} and \ref{axiom2:auxlemma15}).
\begin{enumerate}[label=\textbf{Aux\arabic*},align=left]
\setcounter{enumi}{7}
\item\label{axiom2:auxlemma12}
$\boxed{
\before{\ameetvar{\avariable}{\avariablebis}{\avariableter}}{\ameetvar{\avariable}{\avariablefour}{\avariablefifth}} \land \defined{\ameetvar{\avariable}{\avariablefour}{\avariablesix}}
\implies \before{\ameetvar{\avariable}{\avariablebis}{\avariableter}}{\ameetvar{\avariable}{\avariablefour}{\avariablesix}}}$
\[
\begin{nd}
\hypo {1}
{\before{\ameetvar{\avariable}{\avariablebis}{\avariableter}}{\ameetvar{\avariable}{\avariablefour}{\avariablefifth}}}
\hypo {2}
{\defined{\ameetvar{\avariable}{\avariablefour}{\avariablesix}}}
\have {3} {\symmetric{\ameetvar{\avariable}{\avariablebis}{\avariableter}}} \ae{1}
\have {4} {\ameetvar{\avariable}{\avariablebis}{\avariableter} \neq \ameetvar{\avariable}{\avariablefour}{\avariablefifth}} \ae{1}
\have {5} {\ameetvar{\avariable}{\avariablefour}{\avariablefifth} = \ameetvar{\avariablebis}{\avariablefour}{\avariablefifth}} \by{\ref{axiom2:auxlemma5}}{1}
\have {6} {\ameetvar{\avariable}{\avariablefour}{\avariablesix} = \ameetvar{\avariablebis}{\avariablefour}{\avariablefifth}} \by{\ref{core2Ax:Substitute}}{2,5}
\have {7} {\ameetvar{\avariable}{\avariablefour}{\avariablesix} = \ameetvar{\avariablebis}{\avariablefour}{\avariablesix}} \by{\ref{axiom2:auxlemma11}}{2,5}
\have {8a} {\defined{\ameetvar{\avariablebis}{\avariablefour}{\avariablesix}}} \by{\ref{axiom2:auxlemma1}}{7}
\have {8} {\defined{\ameetvar{\avariable}{\avariablebis}{\avariablesix}}} \by{\ref{core2Ax:PedDefines}}{2,8a}
\have {9} {\ameetvar{\avariable}{\avariablebis}{\avariableter} \neq \ameetvar{\avariablebis}{\avariablefour}{\avariablefifth}} \by{\ref{core2Ax:Substitute}}{4,5}
\have {10} {\ameetvar{\avariable}{\avariablebis}{\avariableter} \neq \ameetvar{\avariable}{\avariablefour}{\avariablesix}} \by{\ref{core2Ax:Substitute}}{6,9}
\have {11} {\ameetvar{\avariable}{\avariablebis}{\avariableter} \neq \ameetvar{\avariablebis}{\avariablefour}{\avariablesix}} \by{\ref{core2Ax:Substitute}}{7,10}
\have {12}
{\before{\ameetvar{\avariable}{\avariablebis}{\avariableter}}{\ameetvar{\avariable}{\avariablefour}{\avariablesix}}}
\by{\defofbefore}{2,3,8,10,11}
\end{nd}
\]
\item\label{axiom2:auxlemma14}
$\boxed{
\begin{aligned}[t]
&\before{\ameetvar{\avariable}{\avariablebis}{\avariableter}}{\ameetvar{\avariable}{\avariablefour}{\avariablefifth}} \land \ameetvar{\avariable}{\avariablefour}{\avariablefifth} = \ameetvar{\avariable}{\avariablesix}{\avariablesept}
\implies\\
&\before{\ameetvar{\avariable}{\avariablebis}{\avariableter}}{\ameetvar{\avariable}{\avariablesix}{\avariablesept}}
\end{aligned}}$
\[
\begin{nd}
\hypo {1}
{\before{\ameetvar{\avariable}{\avariablebis}{\avariableter}}{\ameetvar{\avariable}{\avariablefour}{\avariablefifth}}}
\hypo {2}
{\ameetvar{\avariable}{\avariablefour}{\avariablefifth} = \ameetvar{\avariable}{\avariablesix}{\avariablesept}}
\have {5} {\symmetric{\ameetvar{\avariable}{\avariablebis}{\avariableter}}} \ae{1}
\have {3}
{\defined{\ameetvar{\avariable}{\avariablefour}{\avariablesept}}} \by{\ref{axiom2:auxlemma1}}{2}
\have {4}
 {\before{\ameetvar{\avariable}{\avariablebis}{\avariableter}}{\ameetvar{\avariable}{\avariablefour}{\avariablesept}}} \by{\ref{axiom2:auxlemma12}}{1,3}
\have {6} {\defined{\ameetvar{\avariable}{\avariablebis}{\avariablesept}}} \ae{4}
\have {7} {\ameetvar{\avariable}{\avariablebis}{\avariableter} \neq \ameetvar{\avariable}{\avariablefour}{\avariablefifth}} \ae{1}
\have {8} {\ameetvar{\avariable}{\avariablefour}{\avariablefifth} = \ameetvar{\avariablebis}{\avariablefour}{\avariablefifth}} \by{\ref{axiom2:auxlemma5}}{1}
\have {9} {\ameetvar{\avariable}{\avariablebis}{\avariableter} \neq \ameetvar{\avariable}{\avariablesix}{\avariablesept}} \by{\ref{core2Ax:Substitute}}{2,7}
\have {10} {\ameetvar{\avariable}{\avariablesix}{\avariablesept} = \ameetvar{\avariablebis}{\avariablefour}{\avariablefifth}} \by{\ref{core2Ax:Substitute}}{2,8}
\have {11} {\ameetvar{\avariable}{\avariablesix}{\avariablefifth} = \ameetvar{\avariablebis}{\avariablefour}{\avariablefifth}} \by{\ref{axiom2:auxlemma11}}{10}
\have {12} {\ameetvar{\avariablebis}{\avariablefour}{\avariablefifth} = \ameetvar{\avariable}{\avariablesix}{\avariablefifth}} \by{\ref{core2Ax:EqSymm}}{11}
\have {13} {\ameetvar{\avariablebis}{\avariablefour}{\avariablefifth} = \ameetvar{\avariablebis}{\avariable}{\avariablefifth} \lor\\ \ameetvar{\avariablebis}{\avariablefour}{\avariablefifth} = \ameetvar{\avariablebis}{\avariablesix}{\avariablefifth}} \by{\ref{core2Ax:Symmetric}}{12}
\open
\hypo {A1} {\ameetvar{\avariablebis}{\avariablefour}{\avariablefifth} = \ameetvar{\avariablebis}{\avariable}{\avariablefifth}}
\have {A2} {\ameetvar{\avariablebis}{\avariablefour}{\avariablefifth} = \ameetvar{\avariable}{\avariablebis}{\avariablefifth}} \by{\ref{core2Ax:Substitute}}{5,A1}
\have {A3} {\ameetvar{\avariable}{\avariablebis}{\avariablefifth} = \ameetvar{\avariablebis}{\avariablefour}{\avariablefifth}} \by{\ref{core2Ax:EqSymm}}{A2}
\have {A3b} {\defined{\ameetvar{\avariable}{\avariablebis}{\avariableter}}} \by{\ref{axiom2:auxlemma1}}{5}
\have {A3c} {\ameetvar{\avariable}{\avariablebis}{\avariableter} = \ameetvar{\avariablebis}{\avariablefour}{\avariablefifth}} \by{\ref{axiom2:auxlemma13}}{A3,A3b}
\have {A4}
{\ameetvar{\avariable}{\avariablebis}{\avariableter} = \ameetvar{\avariable}{\avariablefour}{\avariablefifth}} \by{\ref{core2Ax:Substitute}}{8,A3c}
\have {A5} {\bottom} \by{\landcontr}{7,A4}
\close
\have {14} {\ameetvar{\avariablebis}{\avariablefour}{\avariablefifth} \neq \ameetvar{\avariablebis}{\avariable}{\avariablefifth}} \ni{A1-A5}
\have {15} {\ameetvar{\avariablebis}{\avariablefour}{\avariablefifth} = \ameetvar{\avariablebis}{\avariablesix}{\avariablefifth}} \by{\modusponens}{13,14}
\have {16} {\ameetvar{\avariable}{\avariablesix}{\avariablesept} = \ameetvar{\avariablebis}{\avariablesix}{\avariablefifth}} \by{\ref{core2Ax:Substitute}}{10,16}
\have {17} {\ameetvar{\avariable}{\avariablesix}{\avariablesept} = \ameetvar{\avariablebis}{\avariablesix}{\avariablesept}} \by{\ref{axiom2:auxlemma11}}{17}
\have {18} {\ameetvar{\avariable}{\avariablebis}{\avariableter} \neq \ameetvar{\avariablebis}{\avariablesix}{\avariablesept}} \by{\ref{core2Ax:Substitute}}{9,17}
\have {19} {\defined{\ameetvar{\avariable}{\avariablesix}{\avariablesept}}} \by{\ref{axiom2:auxlemma1}}{2}
\have {20}
{\before{\ameetvar{\avariable}{\avariablebis}{\avariableter}}{\ameetvar{\avariable}{\avariablesix}{\avariablesept}}}
\by{\defofbefore}{5,3,9,18,19}
\end{nd}
\]
\item\label{axiom2:auxlemma15}
$\boxed{
\begin{aligned}[t]
&\before{\ameetvar{\avariable}{\avariablebis}{\avariableter}}{\ameetvar{\avariable}{\avariablefour}{\avariablefifth}} \land \ameetvar{\avariable}{\avariablefour}{\avariablefifth} = \ameetvar{\avariablesix}{\avariablesept}{\avariableoct}
\implies\\
&\before{\ameetvar{\avariable}{\avariablebis}{\avariableter}}{\ameetvar{\avariablesix}{\avariablesept}{\avariableoct}}
\end{aligned}}$
\[
\begin{nd}
\hypo {1} {\before{\ameetvar{\avariable}{\avariablebis}{\avariableter}}{\ameetvar{\avariable}{\avariablefour}{\avariablefifth}}}
\hypo {2}
{\ameetvar{\avariable}{\avariablefour}{\avariablefifth} = \ameetvar{\avariablesix}{\avariablesept}{\avariableoct}}
\have {3} {\defined{\ameetvar{\avariable}{\avariablefour}{\avariableoct}}} \by{\ref{axiom2:auxlemma1}}{2}
\have {4} {\before{\ameetvar{\avariable}{\avariablebis}{\avariableter}}{\ameetvar{\avariable}{\avariablefour}{\avariableoct}}} \by{\ref{axiom2:auxlemma12}}{1,3}
\have {5} {\defined{\ameetvar{\avariable}{\avariablebis}{\avariableoct}}} \ae{4}
\have {6} {\ameetvar{\avariable}{\avariablefour}{\avariableoct} = \ameetvar{\avariablesix}{\avariablesept}{\avariableoct}} \by{\ref{axiom2:auxlemma11}}{2}
\have {7} {\ameetvar{\avariable}{\avariablefour}{\avariableoct} = \ameetvar{\avariable}{\avariablesix}{\avariableoct} \lor\\ \ameetvar{\avariable}{\avariablefour}{\avariableoct} = \ameetvar{\avariable}{\avariablesept}{\avariableoct}} \by{\ref{core2Ax:Symmetric}}{6}
\end{nd}
\]
\[
\begin{ndresume}
\open
\hypo {8} {\ameetvar{\avariable}{\avariablefour}{\avariableoct} = \ameetvar{\avariable}{\avariablesix}{\avariableoct}}
\have {9} {\ameetvar{\avariable}{\avariablesix}{\avariableoct} = \ameetvar{\avariablesix}{\avariablesept}{\avariableoct}} \by{\ref{core2Ax:Substitute}}{6,8}
\have {10}
{\before{\ameetvar{\avariable}{\avariablebis}{\avariableter}}{\ameetvar{\avariable}{\avariablesix}{\avariableoct}}}
\by{\ref{axiom2:auxlemma14}}{4,9}
\have {11} {\before{\ameetvar{\avariable}{\avariablebis}{\avariableter}}{\ameetvar{\avariable}{\avariablesix}{\avariableoct}} \land\\ \ameetvar{\avariable}{\avariablesix}{\avariableoct} = \ameetvar{\avariablesix}{\avariablesept}{\avariableoct}} \by{\ndref{9} $\land$ \ndref{10}}{}
\have {12}
{\bigvee_{a \in \{\avariablesix,\avariablesept\}} \big( \before{\ameetvar{\avariable}{\avariablebis}{\avariableter}}{\ameetvar{\avariable}{a}{\avariableoct}} \land\\ \ameetvar{\avariable}{a}{\avariableoct} = \ameetvar{\avariablesix}{\avariablesept}{\avariableoct} \big)}
\oi{11}
\have {13}
{\before{\ameetvar{\avariable}{\avariablebis}{\avariableter}}{\ameetvar{\avariablesix}{\avariablesept}{\avariableoct}}}
\by{\defofbefore}{12}
\close
\open
\hypo {A8} {\ameetvar{\avariable}{\avariablefour}{\avariableoct} = \ameetvar{\avariable}{\avariablesept}{\avariableoct}}
\have {A9} {\ameetvar{\avariable}{\avariablesept}{\avariableoct} = \ameetvar{\avariablesix}{\avariablesept}{\avariableoct}} \by{\ref{core2Ax:Substitute}}{6,A8}
\have {A10}
{\before{\ameetvar{\avariable}{\avariablebis}{\avariableter}}{\ameetvar{\avariable}{\avariablesept}{\avariableoct}}}
\by{\ref{axiom2:auxlemma14}}{4,A9}
\have {A11} {\before{\ameetvar{\avariable}{\avariablebis}{\avariableter}}{\ameetvar{\avariable}{\avariablesept}{\avariableoct}} \land\\ \ameetvar{\avariable}{\avariablesept}{\avariableoct} = \ameetvar{\avariablesix}{\avariablesept}{\avariableoct}} \by{\ndref{A9} $\land$ \ndref{A10}}{}
\have {A12}
{\bigvee_{a \in \{\avariablesix,\avariablesept\}} \big( \before{\ameetvar{\avariable}{\avariablebis}{\avariableter}}{\ameetvar{\avariable}{a}{\avariableoct}} \land\\ \ameetvar{\avariable}{a}{\avariableoct} = \ameetvar{\avariablesix}{\avariablesept}{\avariableoct} \big)}
\oi{A11}
\have {A13}
{\before{\ameetvar{\avariable}{\avariablebis}{\avariableter}}{\ameetvar{\avariablesix}{\avariablesept}{\avariableoct}}}
\by{\defofbefore}{A12}
\close
\have {C}
{\before{\ameetvar{\avariable}{\avariablebis}{\avariableter}}{\ameetvar{\avariablesix}{\avariablesept}{\avariableoct}}}
\oe{7,8-13,A8-A13}
\end{ndresume}
\]
\end{enumerate}
\begin{enumerate}[align=left]
\item[\lemmalab{BeforeSubR}{axiom2:beforelemma0two}]
$
\boxed{ \before{\aterm_1}{\aterm_2} \land \aterm_2 = \aterm_3 \implies \before{\aterm_1}{\aterm_3}}
$\\
We are now ready to deal with the general case.
It is sufficient to prove the result for $\aterm_1$, $\aterm_2$ and $\aterm_3$ meet-point expressions,
as $\avariable = \ameetvar{\avariable}{\avariable}{\avariable}$ by axiom~\ref{core2Ax:Self} and
by definition $\before{\avariable}{\aterm} = \before{\ameetvar{\avariable}{\avariable}{\avariable}}{\aterm}$ and $\before{\aterm}{\avariable} = \before{\aterm}{\ameetvar{\avariable}{\avariable}{\avariable}}$.
Hence, we prove that
\begin{nscenter}
$\before{\ameetvar{\avariable}{\avariablebis}{\avariableter}}{\ameetvar{\avariablefour}{\avariablefifth}{\avariablesix}}
\land \ameetvar{\avariablefour}{\avariablefifth}{\avariablesix} = \ameetvar{\avariablesept}{\avariableoct}{\avariablenine}
\implies \before{\ameetvar{\avariable}{\avariablebis}{\avariableter}}{\ameetvar{\avariablesept}{\avariableoct}{\avariablenine}}$
\end{nscenter}
\[
\begin{nd}
\hypo {1} {\before{\ameetvar{\avariable}{\avariablebis}{\avariableter}}{\ameetvar{\avariablefour}{\avariablefifth}{\avariablesix}}}
\hypo {2} {\ameetvar{\avariablefour}{\avariablefifth}{\avariablesix} = \ameetvar{\avariablesept}{\avariableoct}{\avariablenine}}
\have {3} {\bigvee_{a \in \{\avariablefour,\avariablefifth\}} \big( \before{\ameetvar{\avariable}{\avariablebis}{\avariableter}}{\ameetvar{\avariable}{a}{\avariablesix}}
\land\\ \ameetvar{\avariable}{a}{\avariablesix} = \ameetvar{\avariablefour}{\avariablefifth}{\avariablesix} \big)}
\by{\defofbefore}{1}
\open
\hypo {A1}
  {\before{\ameetvar{\avariable}{\avariablebis}{\avariableter}}{\ameetvar{\avariable}{\avariablefour}{\avariablesix}}}
\hypo {A2}
  {\ameetvar{\avariable}{\avariablefour}{\avariablesix} = \ameetvar{\avariablefour}{\avariablefifth}{\avariablesix}}
\have {A3}
  {\ameetvar{\avariable}{\avariablefour}{\avariablesix} = \ameetvar{\avariablesept}{\avariableoct}{\avariablenine}}
  \by{\ref{core2Ax:Substitute}}{2,A2}
\have {A4} {\before{\ameetvar{\avariable}{\avariablebis}{\avariableter}}{\ameetvar{\avariablesept}{\avariableoct}{\avariablenine}}}
  \by{\ref{axiom2:auxlemma15}}{A1,A3}
\close
\open
\hypo {B1}
  {\before{\ameetvar{\avariable}{\avariablebis}{\avariableter}}{\ameetvar{\avariable}{\avariablefifth}{\avariablesix}}}
\hypo {B2}
  {\ameetvar{\avariable}{\avariablefifth}{\avariablesix} = \ameetvar{\avariablefour}{\avariablefifth}{\avariablesix}}
\have {B3}
  {\ameetvar{\avariable}{\avariablefifth}{\avariablesix} = \ameetvar{\avariablesept}{\avariableoct}{\avariablenine}}
  \by{\ref{core2Ax:Substitute}}{2,B2}
\have {B4} {\before{\ameetvar{\avariable}{\avariablebis}{\avariableter}}{\ameetvar{\avariablesept}{\avariableoct}{\avariablenine}}}
  \by{\ref{axiom2:auxlemma15}}{B1,B3}
\close
\have {4} {\before{\ameetvar{\avariable}{\avariablebis}{\avariableter}}{\ameetvar{\avariablesept}{\avariableoct}{\avariablenine}}}
\oe{3,A1-A4,B1-B4}
\end{nd}
\]
\end{enumerate}
\subsubsection{\ref{axiom2:beforelemma0}}
We now want to prove that the following formula is a tautology:
\begin{nscenter}
$\before{\aterm_1}{\aterm_2} \land \aterm_1 = \aterm_3 \implies \before{\aterm_3}{\aterm_2}\qquad$ (\ref{axiom2:beforelemma0})
\end{nscenter}
As done for the previous tautology, to simplify the proof we first prove two intermediate results (\ref{axiom2:auxlemma10} and \ref{axiom2:auxlemma16}).
\begin{enumerate}[label=\textbf{Aux\arabic*},align=left]
\setcounter{enumi}{10}
\item\label{axiom2:auxlemma10}
$\boxed{
\begin{aligned}[t]
&\before{\ameetvar{\avariable}{\avariablebis}{\avariableter}}{\ameetvar{\avariable}{\avariablefour}{\avariablefifth}} \land \ameetvar{\avariable}{\avariablebis}{\avariableter} = \ameetvar{\avariable}{\avariablesix}{\avariablesept}
\implies\\
&\before{\ameetvar{\avariable}{\avariablesix}{\avariablesept}}{\ameetvar{\avariable}{\avariablefour}{\avariablefifth}}
\end{aligned}}$\\
We first show that
\begin{nscenter}
\lemmalab{($\separate$)}{axiom2:auxauxlemma10}:\qquad $\before{\ameetvar{\avariable}{\avariablebis}{\avariableter}}{\ameetvar{\avariable}{\avariablefour}{\avariableter}} \land \ameetvar{\avariable}{\avariablebis}{\avariableter} = \ameetvar{\avariable}{\avariablesix}{\avariableter}
\implies \before{\ameetvar{\avariable}{\avariablesix}{\avariableter}}{\ameetvar{\avariable}{\avariablefour}{\avariableter}}
\qquad$
\end{nscenter}
And then use this result to prove the \ref{axiom2:auxlemma10} formula.
\[
\begin{nd}
\hypo {1} {\before{\ameetvar{\avariable}{\avariablebis}{\avariableter}}{\ameetvar{\avariable}{\avariablefour}{\avariableter}}}
\hypo {2} {\ameetvar{\avariable}{\avariablebis}{\avariableter} = \ameetvar{\avariable}{\avariablesix}{\avariableter}}
\have {3} {\symmetric{\ameetvar{\avariable}{\avariablebis}{\avariableter}}} \ae{1}
\have {4} {\defined{\ameetvar{\avariable}{\avariablefour}{\avariableter}}} \ae{1}
\have {5} {\ameetvar{\avariable}{\avariablebis}{\avariableter} \neq \ameetvar{\avariable}{\avariablefour}{\avariableter}} \ae{1}
\have {6} {\ameetvar{\avariable}{\avariablefour}{\avariableter} = \ameetvar{\avariablebis}{\avariablefour}{\avariableter}} \by{\ref{axiom2:auxlemma5}}{1}
\have {6b} {\defined{\ameetvar{\avariablebis}{\avariablefour}{\avariableter}}} \by{\ref{axiom2:auxlemma1}}{6}
\have {8} {\ameetvar{\avariable}{\avariablesix}{\avariableter} \neq \ameetvar{\avariable}{\avariablefour}{\avariableter}} \by{\ref{core2Ax:Substitute}}{5,2}
\have {9} {\ameetvar{\avariable}{\avariablesix}{\avariableter} \neq \ameetvar{\avariablebis}{\avariablefour}{\avariableter}} \by{\ref{core2Ax:Substitute}}{6,8}
\open
\hypo {A1} {\asymmetric{\ameetvar{\avariable}{\avariablesix}{\avariableter}}}
\have {A2} {\before{\ameetvar{\avariable}{\avariablefour}{\avariableter}}{\ameetvar{\avariable}{\avariablesix}{\avariableter}}} \by{\ref{axiom2:auxlemma6}}{4,8,A1}
\have {A3} {\before{\ameetvar{\avariablebis}{\avariablefour}{\avariableter}}{\ameetvar{\avariable}{\avariablesix}{\avariableter}}} \by{\ref{axiom2:auxlemma6}}{6b,9,A1}
\have {A4} {\symmetric{\ameetvar{\avariable}{\avariablefour}{\avariableter}}} \ae{A2}
\have {A4b} {\symmetric{\ameetvar{\avariablebis}{\avariablefour}{\avariableter}}} \ae{A3}
\have {A2} {\ameetvar{\avariablefour}{\avariablesix}{\avariableter} = \ameetvar{\avariable}{\avariablesix}{\avariableter}} \by{\ref{axiom2:auxlemma5}}{A4}
\have {A6} {\ameetvar{\avariablefour}{\avariablesix}{\avariableter} = \ameetvar{\avariable}{\avariablebis}{\avariableter}} \by{\ref{core2Ax:Substitute}}{2,A5}
\have {A7} {\ameetvar{\avariablefour}{\avariablesix}{\avariableter} = \ameetvar{\avariablefour}{\avariable}{\avariableter} \lor\\ \ameetvar{\avariablefour}{\avariablesix}{\avariableter} = \ameetvar{\avariablefour}{\avariablebis}{\avariableter}} \by{\ref{core2Ax:Symmetric}}{A6}
\have {A8} {\ameetvar{\avariable}{\avariablebis}{\avariableter} = \ameetvar{\avariablefour}{\avariable}{\avariableter} \lor\\ \ameetvar{\avariable}{\avariablebis}{\avariableter} = \ameetvar{\avariablefour}{\avariablebis}{\avariableter}} \by{\ref{core2Ax:Substitute}}{A6,A7}
\open
\hypo {B1} {\ameetvar{\avariable}{\avariablebis}{\avariableter} = \ameetvar{\avariablefour}{\avariable}{\avariableter}}
 \have {B2} {\ameetvar{\avariable}{\avariablebis}{\avariableter} = \ameetvar{\avariable}{\avariablefour}{\avariableter}} \by{\ref{core2Ax:Substitute}}{A4,B1}
 \have {B3} {\bottom} \by{\landcontr}{5,B2}
\close
\open
\hypo {C1} {\ameetvar{\avariable}{\avariablebis}{\avariableter} = \ameetvar{\avariablefour}{\avariablebis}{\avariableter}}
 \have {C2} {\ameetvar{\avariable}{\avariablebis}{\avariableter} = \ameetvar{\avariablebis}{\avariablefour}{\avariableter}} \by{\ref{core2Ax:Substitute}}{A4b,C1}
 \have {C2b} {\ameetvar{\avariable}{\avariablebis}{\avariableter} = \ameetvar{\avariable}{\avariablefour}{\avariableter}} \by{\ref{core2Ax:Substitute}}{6,C2}
 \have {C3} {\bottom} \by{\landcontr}{5,C2b}
\close
\have {A9} {\bottom} \oe{A8,B1-B3,C1-C3}
\close
\have {10} {\lnot \asymmetric{\ameetvar{\avariable}{\avariablesix}{\avariableter}}} \ni{A1-A9}
\have {11} {\defined{\ameetvar{\avariable}{\avariablesix}{\avariableter}}} \by{\ref{axiom2:auxlemma1}}{2}
\have {12} {\symmetric{\ameetvar{\avariable}{\avariablesix}{\avariableter}}} \by{\modusponens}{10,11}
\have {13} {\asymmetric{\ameetvar{\avariable}{\avariablefour}{\avariableter}} \lor\\ \lnot \asymmetric{\ameetvar{\avariable}{\avariablefour}{\avariableter}}} \by{\trivialtrue}{}
\open
\hypo {D1} {\asymmetric{\ameetvar{\avariable}{\avariablefour}{\avariableter}}}
\have {D2} {\before{\ameetvar{\avariable}{\avariablesix}{\avariableter}}{\ameetvar{\avariable}{\avariablefour}{\avariableter}}} \by{\ref{axiom2:auxlemma6}}{8,12,D1}
\close
\end{nd}
\]
\[
\begin{ndresume}
\open
\hypo {E1} {\lnot \asymmetric{\ameetvar{\avariable}{\avariablefour}{\avariableter}}}
\have {E2} {\symmetric{\ameetvar{\avariable}{\avariablefour}{\avariableter}}} \by{\modusponens}{4,E1}
\have {E3} {\symmetric{\ameetvar{\avariablesix}{\avariablefour}{\avariableter}}} \by{\ref{axiom2:auxlemma6}}{12,E2}
\open
\hypo {E4} {\ameetvar{\avariable}{\avariablesix}{\avariableter} = \ameetvar{\avariablesix}{\avariablefour}{\avariableter}}
\have {E5} {\ameetvar{\avariable}{\avariablesix}{\avariableter} = \ameetvar{\avariablefour}{\avariablesix}{\avariableter}} \by{\ref{core2Ax:Substitute}}{E3,E4}
\have {E6} {\ameetvar{\avariable}{\avariablebis}{\avariableter} = \ameetvar{\avariablefour}{\avariablesix}{\avariableter}} \by{\ref{core2Ax:Substitute}}{2,E5}
\have {E7} {\ameetvar{\avariablefour}{\avariablesix}{\avariableter} = \ameetvar{\avariable}{\avariablebis}{\avariableter}} \by{\ref{core2Ax:EqSymm}}{E6}
\have {E8} {\ameetvar{\avariablefour}{\avariablesix}{\avariableter} = \ameetvar{\avariablefour}{\avariable}{\avariableter} \lor\\ \ameetvar{\avariablefour}{\avariablesix}{\avariableter} = \ameetvar{\avariablefour}{\avariablebis}{\avariableter}} \by{\ref{core2Ax:Symmetric}}{E7}
\have {E9} {\ameetvar{\avariable}{\avariablebis}{\avariableter} = \ameetvar{\avariablefour}{\avariable}{\avariableter} \lor\\ \ameetvar{\avariable}{\avariablebis}{\avariableter} = \ameetvar{\avariablefour}{\avariablebis}{\avariableter}} \by{\ref{core2Ax:Substitute}}{E7,E8}
\open
\hypo {F1} {\ameetvar{\avariable}{\avariablebis}{\avariableter} = \ameetvar{\avariablefour}{\avariable}{\avariableter}}
 \have {F2} {\ameetvar{\avariable}{\avariablebis}{\avariableter} = \ameetvar{\avariable}{\avariablefour}{\avariableter}} \by{\ref{core2Ax:Substitute}}{E2,F1}
 \have {F3} {\bottom} \by{\landcontr}{5,F2}
\close
\open
\hypo {G1} {\ameetvar{\avariable}{\avariablebis}{\avariableter} = \ameetvar{\avariablefour}{\avariablebis}{\avariableter}}
\have {G2} {\symmetric{\ameetvar{\avariablefour}{\avariablebis}{\avariableter}}} \by{\ref{axiom2:auxlemma6}}{3,E2}
 \have {G3} {\ameetvar{\avariable}{\avariablebis}{\avariableter} = \ameetvar{\avariablebis}{\avariablefour}{\avariableter}} \by{\ref{core2Ax:Substitute}}{G1,G2}
 \have {G4} {\ameetvar{\avariable}{\avariablebis}{\avariableter} = \ameetvar{\avariable}{\avariablefour}{\avariableter}} \by{\ref{core2Ax:Substitute}}{6,G3}
 \have {G5} {\bottom} \by{\landcontr}{5,G4}
\close
\have {E10} {\bottom} \oe{E9,F1-F3,G1-G5}
\close
\have {E11} {\ameetvar{\avariable}{\avariablesix}{\avariableter} \neq \ameetvar{\avariablesix}{\avariablefour}{\avariableter}} \ni{E4-E10}
\have {E12} {
\symmetric{\ameetvar{\avariable}{\avariablesix}{\avariableter}}
\land \defined{\ameetvar{\avariable}{\avariablefour}{\avariableter}}
}
\by{\ndref{4} $\land$ \ndref{13}}{}
\have {E13} {
\ameetvar{\avariable}{\avariablesix}{\avariableter} \neq \ameetvar{\avariable}{\avariablefour}{\avariableter}
\land \ameetvar{\avariable}{\avariablesix}{\avariableter} \neq \ameetvar{\avariablesix}{\avariablefour}{\avariableter}
}
\by{\ndref{9} $\land$ \ndref{E11}}{}
\have {E14} {\before{\ameetvar{\avariable}{\avariablesix}{\avariableter}}{\ameetvar{\avariable}{\avariablefour}{\avariableter}}} \by{\defofbefore}{E12,E14}
\close
\have {14}
{\before{\ameetvar{\avariable}{\avariablesix}{\avariableter}}{\ameetvar{\avariable}{\avariablefour}{\avariableter}}}
\oe{13,D1-D2,E1-E14}
\end{ndresume}
\]
Let us now tackle the proof of~\ref{axiom2:auxlemma10}.
\[
\begin{nd}
\hypo {1} {\before{\ameetvar{\avariable}{\avariablebis}{\avariableter}}{\ameetvar{\avariable}{\avariablefour}{\avariablefifth}}}
\hypo {2} {\ameetvar{\avariable}{\avariablebis}{\avariableter} = \ameetvar{\avariable}{\avariablesix}{\avariablesept}}
\have {3} {\defined{\ameetvar{\avariable}{\avariablebis}{\avariablefifth}}} \ae{1}
\have {4} {\before{\ameetvar{\avariable}{\avariablebis}{\avariablefifth}}{\ameetvar{\avariable}{\avariablefour}{\avariablefifth}}} \by{\ref{axiom2:auxlemma9}}{1,3}
\have {5} {\defined{\ameetvar{\avariable}{\avariablebis}{\avariableter}}}  \by{\ref{axiom2:auxlemma1}}{2}
\have {6} {\ameetvar{\avariable}{\avariablebis}{\avariableter} = \ameetvar{\avariable}{\avariablebis}{\avariablefifth}} \by{\ref{core2Ax:EqDef}}{3,5}
\have {7} {\ameetvar{\avariable}{\avariablebis}{\avariablefifth} = \ameetvar{\avariable}{\avariablesix}{\avariablesept}} \by{\ref{core2Ax:Substitute}}{2,6}
\have {8} {\defined{\ameetvar{\avariable}{\avariablesix}{\avariablesept}}} \by{\ref{axiom2:auxlemma1}}{2}
\have {11} {\ameetvar{\avariable}{\avariablebis}{\avariablefifth} = \ameetvar{\avariable}{\avariablesix}{\avariablefifth}} \by{\ref{axiom2:auxlemma11}}{7}
\have {12} {\before{\ameetvar{\avariable}{\avariablesix}{\avariablefifth}}{\ameetvar{\avariable}{\avariablefour}{\avariablefifth}}} \by{\ref{axiom2:auxauxlemma10}}{4,11}
\have {13} {\before{\ameetvar{\avariable}{\avariablesix}{\avariablesept}}{\ameetvar{\avariable}{\avariablefour}{\avariablefifth}}} \by{\ref{axiom2:auxlemma9}}{8,12}
\end{nd}
\]
\item\label{axiom2:auxlemma16}
$\boxed{
\begin{aligned}[t]
&\before{\ameetvar{\avariable}{\avariablebis}{\avariableter}}{\ameetvar{\avariable}{\avariablefour}{\avariablefifth}} \land \ameetvar{\avariable}{\avariablebis}{\avariableter} = \ameetvar{\avariablesix}{\avariablesept}{\avariableoct}
\implies\\ &\before{\ameetvar{\avariablesix}{\avariablesept}{\avariableoct}}{\ameetvar{\avariable}{\avariablefour}{\avariablefifth}}
\end{aligned}}$
\[
\begin{nd}
\hypo {1} {\before{\ameetvar{\avariable}{\avariablebis}{\avariableter}}{\ameetvar{\avariable}{\avariablefour}{\avariablefifth}}}
\hypo {2} {\ameetvar{\avariable}{\avariablebis}{\avariableter} = \ameetvar{\avariablesix}{\avariablesept}{\avariableoct}}
\have {2b} {\defined{\ameetvar{\avariablesix}{\avariablesept}{\avariableoct}}} \by{\ref{axiom2:auxlemma1}}{2}
\have {3} {\ameetvar{\avariable}{\avariablebis}{\avariableter} = \ameetvar{\avariablesix}{\avariablesept}{\avariableter}}
\by{\ref{axiom2:auxlemma11}}{2}
\have {3b} {\symmetric{\ameetvar{\avariable}{\avariablesix}{\avariableter}}} \by{\ref{core2Ax:Symmetric}}{3}
\have {4}
{\ameetvar{\avariable}{\avariablebis}{\avariableter} = \ameetvar{\avariable}{\avariablesix}{\avariableter} \lor\\ \ameetvar{\avariable}{\avariablebis}{\avariableter} = \ameetvar{\avariable}{\avariablesept}{\avariableter}}
\by{\ref{core2Ax:Symmetric}}{3}
\open
\hypo {5} {\ameetvar{\avariable}{\avariablebis}{\avariableter} = \ameetvar{\avariable}{\avariablesix}{\avariableter}}
\have {6} {\before{\ameetvar{\avariable}{\avariablesix}{\avariableter}}{\ameetvar{\avariable}{\avariablefour}{\avariablefifth}}}
\by{\ref{axiom2:auxlemma10}}{1,5}
\have {7}
{\before{\ameetvar{\avariablesix}{\avariable}{\avariableter}}{\ameetvar{\avariablesix}{\avariablefour}{\avariablefifth}}}
\by{\ref{axiom2:auxlemma5}}{6}
\have {7b}
{\ameetvar{\avariable}{\avariablefour}{\avariablefifth} = \ameetvar{\avariablesix}{\avariablefour}{\avariablefifth}}
\by{\ref{axiom2:auxlemma5}}{6}
\have {8} {\ameetvar{\avariable}{\avariablebis}{\avariableter} = \ameetvar{\avariablesix}{\avariable}{\avariableter}}
\by {\ref{core2Ax:Substitute}}{3b,5}
\have {9} {\ameetvar{\avariablesix}{\avariablesept}{\avariableoct} = \ameetvar{\avariablesix}{\avariable}{\avariableter}}
\by {\ref{core2Ax:Substitute}}{2,8}
\have {10} {\before{\ameetvar{\avariablesix}{\avariablesept}{\avariableoct}}{\ameetvar{\avariablesix}{\avariablefour}{\avariablefifth}}}
\by {\ref{axiom2:auxlemma10}}{7,9}
\have {11} {\before{\ameetvar{\avariablesix}{\avariablesept}{\avariableoct}}{\ameetvar{\avariable}{\avariablefour}{\avariablefifth}}}
\by {\ref{axiom2:beforelemma0two}}{7b,10}
\close
\open
\hypo {A1} {\ameetvar{\avariable}{\avariablebis}{\avariableter} = \ameetvar{\avariable}{\avariablesept}{\avariableter}}
\have {A2} {\before{\ameetvar{\avariable}{\avariablesept}{\avariableter}}{\ameetvar{\avariable}{\avariablefour}{\avariablefifth}}}
\by{\ref{axiom2:auxlemma10}}{1,A1}
\have {A3} {\symmetric{\ameetvar{\avariable}{\avariablesept}{\avariableter}}} \ae{A2}
\have {A4} {\symmetric{\ameetvar{\avariablesix}{\avariablesept}{\avariableter}}} \by{\ref{axiom2:auxlemma6}}{3b,A3}
\have {A5} {\before{\ameetvar{\avariablesept}{\avariable}{\avariableter}}{\ameetvar{\avariablesept}{\avariablefour}{\avariablefifth}} \land\\ \ameetvar{\avariable}{\avariablefour}{\avariablefifth} = \ameetvar{\avariablesept}{\avariablefour}{\avariablefifth}}
\by{\ref{axiom2:auxlemma5}}{A4}
\have {A6} {\ameetvar{\avariablesept}{\avariable}{\avariableter} = \ameetvar{\avariable}{\avariablebis}{\avariableter}}
\by{\ref{core2Ax:Substitute}}{A1,A3}
\have {A7} {\ameetvar{\avariablesept}{\avariable}{\avariableter} = \ameetvar{\avariablesix}{\avariablesept}{\avariableoct}}
\by{\ref{core2Ax:Substitute}}{2,A6}
\have {A8} {\ameetvar{\avariablesept}{\avariable}{\avariableter} = \ameetvar{\avariablesept}{\avariablesix}{\avariableoct}}
\by{\ref{core2Ax:Substitute}}{A4,A7}
\have {A9}
{\before{\ameetvar{\avariablesept}{\avariablesix}{\avariableter}}{\ameetvar{\avariablesept}{\avariablefour}{\avariablefifth}}}
\by{\ref{axiom2:auxlemma10}}{A2,A8}
\have {A10}
{\before{\ameetvar{\avariablesix}{\avariablesept}{\avariableter}}{\ameetvar{\avariablesix}{\avariablefour}{\avariablefifth}}}
\by{\ref{axiom2:auxlemma5}}{A9}
\have {A10b}
{\before{\ameetvar{\avariablesix}{\avariablesept}{\avariableoct}}{\ameetvar{\avariablesix}{\avariablefour}{\avariablefifth}}}
\by{\ref{axiom2:auxlemma9}}{2b,A10}
\have {A11}
{\ameetvar{\avariablesix}{\avariablefour}{\avariablefifth} = \ameetvar{\avariablesept}{\avariablefour}{\avariablefifth}}
\by{\ref{axiom2:auxlemma5}}{A9}
\have {A12}
{\ameetvar{\avariablesix}{\avariablefour}{\avariablefifth} = \ameetvar{\avariable}{\avariablefour}{\avariablefifth}}
\by{\ref{core2Ax:Substitute}}{A5,A11}
\have {A13} {\before{\ameetvar{\avariablesix}{\avariablesept}{\avariableoct}}{\ameetvar{\avariable}{\avariablefour}{\avariablefifth}}}
\by {\ref{axiom2:beforelemma0two}}{A10b,A12}
\close
\have {F} {\before{\ameetvar{\avariablesix}{\avariablesept}{\avariableoct}}{\ameetvar{\avariable}{\avariablefour}{\avariablefifth}}}
\oe{4,5-11,A1-A13}
\end{nd}
\]
\end{enumerate}
\begin{enumerate}[align=left]
\item[\lemmalab{BeforeSubL}{axiom2:beforelemma0}]
$
\boxed{ \before{\aterm_1}{\aterm_2} \land \aterm_1 = \aterm_3 \implies \before{\aterm_3}{\aterm_2}}
$\\
We are now ready to deal with the general case.
It is sufficient to prove the result for $\aterm_1$, $\aterm_2$ and $\aterm_3$ meet-point expressions,
as $\avariable = \ameetvar{\avariable}{\avariable}{\avariable}$ by axiom~\ref{core2Ax:Self} and
by definition $\before{\avariable}{\aterm} = \before{\ameetvar{\avariable}{\avariable}{\avariable}}{\aterm}$ and $\before{\aterm}{\avariable} = \before{\aterm}{\ameetvar{\avariable}{\avariable}{\avariable}}$.
Hence, we prove that
\begin{nscenter}
$\before{\ameetvar{\avariable}{\avariablebis}{\avariableter}}{\ameetvar{\avariablefour}{\avariablefifth}{\avariablesix}}
\land \ameetvar{\avariable}{\avariablebis}{\avariablesix} = \ameetvar{\avariablesept}{\avariableoct}{\avariablenine}
\implies \before{\ameetvar{\avariablesept}{\avariableoct}{\avariablenine}}{\ameetvar{\avariablefour}{\avariablefifth}{\avariablesix}}$
\end{nscenter}
\[
\begin{nd}
\hypo {1} {\before{\ameetvar{\avariable}{\avariablebis}{\avariableter}}{\ameetvar{\avariablefour}{\avariablefifth}{\avariablesix}}}
\hypo {2} {\ameetvar{\avariable}{\avariablebis}{\avariableter} = \ameetvar{\avariablesept}{\avariableoct}{\avariablenine}}
\have {3}
{
\bigvee_{a \in \{\avariablefour,\avariablefifth\}} \big(
\before{\ameetvar{\avariable}{\avariablebis}{\avariableter}}{\ameetvar{\avariable}{a}{\avariablesix}}
\land\\ \ameetvar{\avariable}{a}{\avariablesix} = \ameetvar{\avariablefour}{\avariablefifth}{\avariablesix}
\big)
}
\by{\defofbefore}{1}
\open
\hypo {A1} {\before{\ameetvar{\avariable}{\avariablebis}{\avariableter}}{\ameetvar{\avariable}{\avariablefour}{\avariablesix}}}
\hypo {A2} {\ameetvar{\avariable}{\avariablefour}{\avariablesix} = \ameetvar{\avariablefour}{\avariablefifth}{\avariablesix}}
\have {A3}
{\before{\ameetvar{\avariablesept}{\avariableoct}{\avariablenine}}{\ameetvar{\avariable}{\avariablefour}{\avariablesix}}}
\by{\ref{axiom2:auxlemma16}}{2,A1}
\have {A4} {\before{\ameetvar{\avariablesept}{\avariableoct}{\avariablenine}}{\ameetvar{\avariablefour}{\avariablefifth}{\avariablesix}}}
\by{\ref{axiom2:beforelemma0two}}{A2,A3}
\close
\open
\hypo {B1} {\before{\ameetvar{\avariable}{\avariablebis}{\avariableter}}{\ameetvar{\avariable}{\avariablefifth}{\avariablesix}}}
\hypo {B2} {\ameetvar{\avariable}{\avariablefifth}{\avariablesix} = \ameetvar{\avariablefour}{\avariablefifth}{\avariablesix}}
\have {B3}
{\before{\ameetvar{\avariablesept}{\avariableoct}{\avariablenine}}{\ameetvar{\avariable}{\avariablefifth}{\avariablesix}}}
\by{\ref{axiom2:auxlemma16}}{2,B1}
\have {B4} {\before{\ameetvar{\avariablesept}{\avariableoct}{\avariablenine}}{\ameetvar{\avariablefour}{\avariablefifth}{\avariablesix}}}
\by{\ref{axiom2:beforelemma0two}}{B2,B3}
\close
\have{F} {\before{\ameetvar{\avariablesept}{\avariableoct}{\avariablenine}}{\ameetvar{\avariablefour}{\avariablefifth}{\avariablesix}}}
\oe{3,A1-A4,B1-B4}
\end{nd}
\]
\end{enumerate}
\subsubsection{\ref{axiom2:beforelemma2}}
We now want to prove that the following formula is a tautology:
\begin{nscenter}
$\before{\aterm_1}{\aterm_2} \implies \lnot \before{\aterm_2}{\aterm_1}\qquad$ (\ref{axiom2:beforelemma2})
\end{nscenter}
As done for the previous tautology, to simplify the proof we first prove an intermediate result.
\begin{enumerate}[label=\textbf{Aux\arabic*},align=left]
\setcounter{enumi}{12}
\item\label{axiom2:auxlemma8}
$\boxed{
\begin{aligned}[t]
&\before{\ameetvar{\avariable}{\avariablebis}{\avariableter}}{\ameetvar{\avariable}{\avariablefour}{\avariableter}} \implies\\
&\lnot \before{\ameetvar{\avariable}{\avariablefour}{\avariableter}}{\ameetvar{\avariable}{\avariablebis}{\avariableter}}
\end{aligned}}$
\[
\begin{nd}
\hypo {1} {\before{\ameetvar{\avariable}{\avariablebis}{\avariableter}}{\ameetvar{\avariable}{\avariablefour}{\avariableter}}}
\have {2} {\ameetvar{\avariable}{\avariablebis}{\avariableter} \neq \ameetvar{\avariable}{\avariablefour}{\avariableter}} \ae{1}
\have {3} {\ameetvar{\avariable}{\avariablefour}{\avariableter} = \ameetvar{\avariablebis}{\avariablefour}{\avariableter}}
\by{\ref{axiom2:auxlemma5}}{1}
\have {4} {\symmetric{\ameetvar{\avariable}{\avariablebis}{\avariableter}}} \ae{1}
\open
\hypo {A1} {\before{\ameetvar{\avariable}{\avariablefour}{\avariableter}}{\ameetvar{\avariable}{\avariablebis}{\avariableter}}}
\have {A2} {\ameetvar{\avariable}{\avariablebis}{\avariableter} = \ameetvar{\avariablefour}{\avariablebis}{\avariableter}} \by{\ref{axiom2:auxlemma5}}{A1}
\have {A3} {\symmetric{\ameetvar{\avariable}{\avariablefour}{\avariableter}}} \ae{A1}
\have {A4} {\symmetric{\ameetvar{\avariablebis}{\avariablefour}{\avariableter}}} \by{\ref{axiom2:auxlemma6}}{4,A3}
\have {A5} {\ameetvar{\avariable}{\avariablebis}{\avariableter} = \ameetvar{\avariablebis}{\avariablefour}{\avariableter}} \by{\ref{core2Ax:Substitute}}{A2,A4}
\have {A6} {\ameetvar{\avariable}{\avariablebis}{\avariableter} = \ameetvar{\avariable}{\avariablefour}{\avariableter}} \by{\ref{core2Ax:Substitute}}{3,A5}
\have {A7} {\bottom} \by{\landcontr}{2,A6}
\close
\have {5} {\lnot\before{\ameetvar{\avariable}{\avariablefour}{\avariableter}}{\ameetvar{\avariable}{\avariablebis}{\avariableter}}}
\ni{A1-A7}
\end{nd}
\]
\end{enumerate}
\begin{enumerate}[align=left]
\item[\lemmalab{BeforeAsym}{axiom2:beforelemma2}]
$\boxed{\before{\aterm_1}{\aterm_2} \implies \lnot \before{\aterm_2}{\aterm_1}}$\\
We are now ready to deal with the general case.
Again, it is sufficient to prove the result for $\aterm_1$ and $\aterm_2$ meet-point expressions.
Hence, we prove that
\begin{nscenter}
$\before{\ameetvar{\avariable}{\avariablebis}{\avariableter}}{\ameetvar{\avariablefour}{\avariablefifth}{\avariablesix}} \implies \lnot \before{\ameetvar{\avariablefour}{\avariablefifth}{\avariablesix}}{\ameetvar{\avariable}{\avariablebis}{\avariableter}}$
\end{nscenter}
\[
\begin{nd}
\hypo {1} {\before{\ameetvar{\avariable}{\avariablebis}{\avariableter}}{\ameetvar{\avariablefour}{\avariablefifth}{\avariablesix}}}
\have {2} {
\bigvee_{a \in \{\avariablefour,\avariablefifth\}} \big( \before{\ameetvar{\avariable}{\avariablebis}{\avariableter}}{\ameetvar{\avariable}{a}{\avariablesix}} \land\\
    \ameetvar{\avariable}{a}{\avariablesix} = \ameetvar{\avariablefour}{\avariablefifth}{\avariablesix}
    \big)
}
\by{\defofbefore}{1}
\open
\hypo {A1}
{
  \before{\ameetvar{\avariable}{\avariablebis}{\avariableter}}{\ameetvar{\avariable}{\avariablefour}{\avariablesix}}
}
\hypo {A2}
{
  \ameetvar{\avariable}{\avariablefour}{\avariablesix} = \ameetvar{\avariablefour}{\avariablefifth}{\avariablesix}
}
\have {A3}
{\lnot \before{\ameetvar{\avariable}{\avariablefour}{\avariablesix}}{\ameetvar{\avariable}{\avariablebis}{\avariableter}}}
\by{\ref{axiom2:auxlemma8}}{A1}
\open
\hypo {B1} {\before{\ameetvar{\avariablefour}{\avariablefifth}{\avariablesix}}{\ameetvar{\avariable}{\avariablebis}{\avariableter}}}
\have {B2}
{\before{\ameetvar{\avariable}{\avariablefour}{\avariablesix}}{\ameetvar{\avariable}{\avariablebis}{\avariableter}}}
\by{\ref{axiom2:beforelemma0two}}{A2,B1}
\have {B3} {\bottom} \by{\landcontr}{A3,B2}
\close
\have {A4} {\lnot \before{\ameetvar{\avariablefour}{\avariablefifth}{\avariablesix}}{\ameetvar{\avariable}{\avariablebis}{\avariableter}}}
\ni{B1-B3}
\close
\open
\hypo {C1}
{
  \before{\ameetvar{\avariable}{\avariablebis}{\avariableter}}{\ameetvar{\avariable}{\avariablefifth}{\avariablesix}}
}
\hypo {C2}
{
  \ameetvar{\avariable}{\avariablefifth}{\avariablesix} = \ameetvar{\avariablefour}{\avariablefifth}{\avariablesix}
}
\have {C3}
{\lnot \before{\ameetvar{\avariable}{\avariablefifth}{\avariablesix}}{\ameetvar{\avariable}{\avariablebis}{\avariableter}}}
\by{\ref{axiom2:auxlemma8}}{C1}
\open
\hypo {D1} {\before{\ameetvar{\avariablefour}{\avariablefifth}{\avariablesix}}{\ameetvar{\avariable}{\avariablebis}{\avariableter}}}
\have {D2}
{\before{\ameetvar{\avariable}{\avariablefifth}{\avariablesix}}{\ameetvar{\avariable}{\avariablebis}{\avariableter}}}
\by{\ref{axiom2:beforelemma0two}}{C2,D1}
\have {D3} {\bottom} \by{\landcontr}{C3,D2}
\close
\have {C4} {\lnot \before{\ameetvar{\avariablefour}{\avariablefifth}{\avariablesix}}{\ameetvar{\avariable}{\avariablebis}{\avariableter}}}
\ni{D1-D3}
\close
\have {E} {\lnot \before{\ameetvar{\avariablefour}{\avariablefifth}{\avariablesix}}{\ameetvar{\avariable}{\avariablebis}{\avariableter}}}
\oe{2,A1-A4,C1-C4}
\end{nd}
\]
\end{enumerate}
\subsubsection{\ref{axiom2:beforelemma3}}
We now want to prove that the following formula is a tautology:
\begin{nscenter}
$\before{\aterm_1}{\aterm_2} \land \before{\aterm_2}{\aterm_3} \implies \before{\aterm_1}{\aterm_3}\qquad$ (\ref{axiom2:beforelemma3})
\end{nscenter}
As done for the previous tautology, to simplify the proof we first prove an intermediate result.
\begin{enumerate}[label=\textbf{Aux\arabic*},align=left]
\setcounter{enumi}{13}
\item\label{axiom2:auxlemma17}
$
\boxed{
\begin{aligned}[t]
&\before{\ameetvar{\avariable}{\avariablebis}{\avariableter}}{\ameetvar{\avariable}{\avariablefour}{\avariablefifth}} \land
\before{\ameetvar{\avariable}{\avariablefour}{\avariablefifth}}{\ameetvar{\avariable}{\avariablesix}{\avariablesept}} \implies\\
&
\before{\ameetvar{\avariable}{\avariablebis}{\avariableter}}{\ameetvar{\avariable}{\avariablesix}{\avariablesept}}
\end{aligned}
}
$
\[
\begin{nd}
\hypo {1} {\before{\ameetvar{\avariable}{\avariablebis}{\avariableter}}{\ameetvar{\avariable}{\avariablefour}{\avariablefifth}}}
\hypo {2} {\before{\ameetvar{\avariable}{\avariablefour}{\avariablefifth}}{\ameetvar{\avariable}{\avariablesix}{\avariablesept}}}
\have {3}
{\symmetric{\ameetvar{\avariable}{\avariablebis}{\avariableter}}} \ae{1}
\have {4}
{\defined{\ameetvar{\avariable}{\avariablefour}{\avariablesept}}} \ae{2}
\have {5}
{\before{\ameetvar{\avariable}{\avariablebis}{\avariableter}}{\ameetvar{\avariable}{\avariablefour}{\avariablesept}}} \by{\ref{axiom2:beforelemma0two}}{1,4}
\have {6}
{\defined{\ameetvar{\avariable}{\avariablebis}{\avariablesept}}}
\ae {5}
\have {8}
{\ameetvar{\avariable}{\avariablefour}{\avariablefifth} = \ameetvar{\avariablebis}{\avariablefour}{\avariablefifth}}
\by{\ref{axiom2:auxlemma5}}{1}
\have {26b} {\defined{\ameetvar{\avariable}{\avariablefour}{\avariablefifth}}}
\by{\ref{axiom2:auxlemma1}}{8}
\have {9}
{\ameetvar{\avariable}{\avariablefour}{\avariablefifth} \neq \ameetvar{\avariable}{\avariablesix}{\avariablesept}} \ae{2}
\have {10}
{\ameetvar{\avariable}{\avariablesix}{\avariablesept} = \ameetvar{\avariablefour}{\avariablesix}{\avariablesept}}
\by{\ref{axiom2:auxlemma5}}{2}
\have {11}
{\before{\ameetvar{\avariablebis}{\avariablefour}{\avariablefifth}}{\ameetvar{\avariable}{\avariablesix}{\avariablesept}}}
\by{\ref{axiom2:beforelemma0two}}{2,8}
\end{nd}
\]
\[
\begin{ndresume}
\have {12}
{
\bigvee_{a \in \{\avariable,\avariablesix\}} \big(
\before{\ameetvar{\avariablebis}{\avariablefour}{\avariablefifth}}{\ameetvar{\avariablebis}{a}{\avariablesept}}
\\ \land\ameetvar{\avariablebis}{a}{\avariablesept} = \ameetvar{\avariable}{\avariablesix}{\avariablesept}
\big)
}
\by{\defofbefore}{11}
\open
\hypo {13} {\before{\ameetvar{\avariablebis}{\avariablefour}{\avariablefifth}}{\ameetvar{\avariablebis}{\avariable}{\avariablesept}}}
\hypo {14} {\ameetvar{\avariablebis}{\avariable}{\avariablesept} = \ameetvar{\avariable}{\avariablesix}{\avariablesept}}
\have {15}
{\before{\ameetvar{\avariable}{\avariablefour}{\avariablefifth}}{\ameetvar{\avariablebis}{\avariable}{\avariablesept}}}
\by{\ref{axiom2:beforelemma0}}{8,13}
\have {15a} {\ameetvar{\avariable}{\avariablebis}{\avariablesept} = \ameetvar{\avariablebis}{\avariable}{\avariableter}}
\by{\ref{core2Ax:Substitute}}{3,6}
\have {15ab} {\ameetvar{\avariable}{\avariablebis}{\avariablesept} = \ameetvar{\avariablebis}{\avariable}{\avariablesept}}
\by{\ref{axiom2:auxlemma11}}{15a}
\have {15ac} {\defined{\ameetvar{\avariable}{\avariablebis}{\avariableter}}} \by{\ref{axiom2:auxlemma1}}{3}
\have {15b} {\before{\ameetvar{\avariable}{\avariablefour}{\avariablefifth}}{\ameetvar{\avariable}{\avariablebis}{\avariablesept}}}
\by{\ref{axiom2:beforelemma0two}}{14,15ab}
\have {15c} {\before{\ameetvar{\avariable}{\avariablefour}{\avariablefifth}}{\ameetvar{\avariable}{\avariablebis}{\avariableter}}}
\by{\ref{axiom2:beforelemma0two}}{15ac,15b}
\have {16} {\bottom} \by{\landcontr}{1,15b}
\close
\have {17}
{\before{\ameetvar{\avariablebis}{\avariablefour}{\avariablefifth}}{\ameetvar{\avariablebis}{\avariablesix}{\avariablesept}}
\land\\ \ameetvar{\avariablebis}{\avariablesix}{\avariablesept} = \ameetvar{\avariable}{\avariablesix}{\avariablesept}}
\by{\modusponens}{12,13-16}
\have {18}
{\ameetvar{\avariablebis}{\avariablesix}{\avariablesept} = \ameetvar{\avariable}{\avariablesix}{\avariablesept}}
\ae{17}
\open
\hypo {19} {\ameetvar{\avariable}{\avariablebis}{\avariableter} = \ameetvar{\avariable}{\avariablesix}{\avariablesept}}
\have {20} {\ameetvar{\avariable}{\avariablebis}{\avariableter} = \ameetvar{\avariablefour}{\avariablesix}{\avariablesept}}
\by{\ref{core2Ax:Substitute}}{10,19}
\have {21} {\ameetvar{\avariablefour}{\avariablesix}{\avariablesept} = \ameetvar{\avariable}{\avariablebis}{\avariableter}}
\by{\ref{core2Ax:EqSymm}}{20}
\have {21b}  {\ameetvar{\avariablefour}{\avariablesix}{\avariablesept} = \ameetvar{\avariable}{\avariablebis}{\avariablesept}}
\by{\ref{axiom2:auxlemma11}}{21}
\have {22} {\ameetvar{\avariablefour}{\avariablesix}{\avariablesept} = \ameetvar{\avariablefour}{\avariable}{\avariablesept} \lor\\ \ameetvar{\avariablefour}{\avariablesix}{\avariablesept} = \ameetvar{\avariablefour}{\avariablebis}{\avariablesept}}
\by{\ref{core2Ax:Symmetric}}{21b}
\open
\hypo {23} {\ameetvar{\avariablefour}{\avariablesix}{\avariablesept} = \ameetvar{\avariablefour}{\avariable}{\avariablesept}}
\have {24} {\ameetvar{\avariable}{\avariablesix}{\avariablesept} = \ameetvar{\avariablefour}{\avariable}{\avariablesept}}
\by{\ref{core2Ax:Substitute}}{10,23}
\have {25} {\symmetric{\ameetvar{\avariablefour}{\avariable}{\avariablesept}}}
\by{\ref{core2Ax:Symmetric}}{24}
\have {26} {\ameetvar{\avariable}{\avariablesix}{\avariablesept} = \ameetvar{\avariable}{\avariablefour}{\avariablesept}}
\by{\ref{core2Ax:Substitute}}{24,25}
\have {26c} {\ameetvar{\avariable}{\avariablesix}{\avariablesept} = \ameetvar{\avariable}{\avariablefour}{\avariablefifth}}
\by{\ref{axiom2:auxlemma13}}{26,26b}
\have {27} {\bottom} \by{\landcontr}{9,26c}
\close
\have {28} {\ameetvar{\avariablefour}{\avariablesix}{\avariablesept} = \ameetvar{\avariablefour}{\avariablebis}{\avariablesept}} \by{\modusponens}{22,23-27}
\have {29} {\ameetvar{\avariable}{\avariablesix}{\avariablesept} = \ameetvar{\avariablefour}{\avariablebis}{\avariablesept}}
\by{\ref{core2Ax:Substitute}}{10,28}
\have {29a} {\ameetvar{\avariablebis}{\avariablesix}{\avariablesept} = \ameetvar{\avariablefour}{\avariablebis}{\avariablesept}}
\by{\ref{core2Ax:Substitute}}{18,29}
\have {29b} {\symmetric{\ameetvar{\avariablebis}{\avariablefour}{\avariablesept}}}
\by{\ref{core2Ax:Symmetric}}{29a}
\have {29c} {\ameetvar{\avariable}{\avariablesix}{\avariablesept} = \ameetvar{\avariablebis}{\avariablefour}{\avariablesept}}
\by{\ref{core2Ax:Substitute}}{29,29b}
\have {29d} {\defined{\ameetvar{\avariablebis}{\avariablefour}{\avariablefifth}}}
\by{\ref{axiom2:auxlemma1}}{8}
\have {29e} {\ameetvar{\avariable}{\avariablesix}{\avariablesept} = \ameetvar{\avariablebis}{\avariablefour}{\avariablefifth}}
\by{\ref{axiom2:auxlemma13}}{29c,29d}
\have {30} {\ameetvar{\avariable}{\avariablesix}{\avariablesept} = \ameetvar{\avariable}{\avariablefour}{\avariablefifth}}
\by{\ref{core2Ax:Substitute}}{8,29e}
\have {31} {\bottom} \by{\landcontr}{9,29e}
\close
\have {32} {\ameetvar{\avariable}{\avariablebis}{\avariableter} \neq \ameetvar{\avariable}{\avariablesix}{\avariablesept}}
\ni{19-31}
\have {33} {\ameetvar{\avariable}{\avariablebis}{\avariableter} \neq \ameetvar{\avariablebis}{\avariablesix}{\avariablesept}}
\by{\ref{core2Ax:Substitute}}{18,32}
\have {33b} {\defined{\ameetvar{\avariable}{\avariablesix}{\avariablesept}}} \ae{2}
\have {34} {\before{\ameetvar{\avariable}{\avariablebis}{\avariableter}}{\ameetvar{\avariable}{\avariablesix}{\avariablesept}}}
\by{\defofbefore}{3,6,32,33,33b}
\end{ndresume}
\]
\end{enumerate}
\begin{enumerate}[align=left]
\item[\lemmalab{BeforeTrans}{axiom2:beforelemma3}]
$\boxed{\before{\aterm_1}{\aterm_2} \land \before{\aterm_2}{\aterm_3} \implies \before{\aterm_1}{\aterm_3}}$\\
We are now ready to deal with the general case.
Again, it is sufficient to prove the result for $\aterm_1$, $\aterm_2$ and $\aterm_3$ meet-point expressions.
Hence, we prove that
\begin{nscenter}
$\before{\ameetvar{\avariable}{\avariablebis}{\avariableter}}{\ameetvar{\avariablefour}{\avariablefifth}{\avariablesix}} \land
\before{\ameetvar{\avariablefour}{\avariablefifth}{\avariablesix}}{\ameetvar{\avariablesept}{\avariableoct}{\avariablenine}} \implies
\before{\ameetvar{\avariable}{\avariablebis}{\avariableter}}{\ameetvar{\avariablesept}{\avariableoct}{\avariablenine}}$
\end{nscenter}
\[
\begin{nd}
\hypo {1}
{\before{\ameetvar{\avariable}{\avariablebis}{\avariableter}}{\ameetvar{\avariablefour}{\avariablefifth}{\avariablesix}}}
\hypo {2}
{\before{\ameetvar{\avariablefour}{\avariablefifth}{\avariablesix}}{\ameetvar{\avariablesept}{\avariableoct}{\avariablenine}}}
\have {3}
{\bigvee_{a \in \{\avariablefour,\avariablefifth\}} \big(
\before{\ameetvar{\avariable}{\avariablebis}{\avariableter}}{\ameetvar{\avariable}{a}{\avariablesix}} \land\\ \ameetvar{\avariable}{a}{\avariablesix} = \ameetvar{\avariablefour}{\avariablefifth}{\avariablesix}
\big)
}
\by{\defofbefore}{1}
\open
\hypo {4}
{\before{\ameetvar{\avariable}{\avariablebis}{\avariableter}}{\ameetvar{\avariable}{\avariablefour}{\avariablesix}}}
\hypo {5}
{\ameetvar{\avariable}{\avariablefour}{\avariablesix} = \ameetvar{\avariablefour}{\avariablefifth}{\avariablesix}}
\have {6}
{\before{\ameetvar{\avariable}{\avariablefour}{\avariablesix}}{\ameetvar{\avariablesept}{\avariableoct}{\avariablenine}}}
\by{\ref{axiom2:beforelemma0}}{2,5}
\have {7}
{\bigvee_{b \in \{\avariablesept,\avariableoct\}} \big(
\before{\ameetvar{\avariable}{\avariablefour}{\avariablesix}}{\ameetvar{\avariable}{b}{\avariablenine}} \land\\ \ameetvar{\avariable}{b}{\avariablenine} = \ameetvar{\avariablesept}{\avariableoct}{\avariablenine}
\big)
}
\by{\defofbefore}{6}
\open
\hypo {8}
{\before{\ameetvar{\avariable}{\avariablefour}{\avariablesix}}{\ameetvar{\avariable}{\avariablesept}{\avariablenine}}}
\hypo {9} {\ameetvar{\avariable}{\avariablesept}{\avariablenine} = \ameetvar{\avariablesept}{\avariableoct}{\avariablenine}}
\have {10} {\before{\ameetvar{\avariable}{\avariablebis}{\avariableter}}{\ameetvar{\avariable}{\avariablesept}{\avariablenine}}}
\by{\ref{axiom2:auxlemma17}}{4,8}
\have {11} {\before{\ameetvar{\avariable}{\avariablebis}{\avariableter}}{\ameetvar{\avariablesept}{\avariableoct}{\avariablenine}}}
\by{\ref{axiom2:beforelemma0two}}{9,10}
\close
\open
\hypo {A8}
{\before{\ameetvar{\avariable}{\avariablefour}{\avariablesix}}{\ameetvar{\avariable}{\avariableoct}{\avariablenine}}}
\hypo {A9} {\ameetvar{\avariable}{\avariableoct}{\avariablenine} = \ameetvar{\avariablesept}{\avariableoct}{\avariablenine}}
\have {A10} {\before{\ameetvar{\avariable}{\avariablebis}{\avariableter}}{\ameetvar{\avariable}{\avariableoct}{\avariablenine}}}
\by{\ref{axiom2:auxlemma17}}{4,A8}
\have {A11} {\before{\ameetvar{\avariable}{\avariablebis}{\avariableter}}{\ameetvar{\avariablesept}{\avariableoct}{\avariablenine}}}
\by{\ref{axiom2:beforelemma0two}}{A9,A10}
\close
\have {12} {\before{\ameetvar{\avariable}{\avariablebis}{\avariableter}}{\ameetvar{\avariablesept}{\avariableoct}{\avariablenine}}}
\oe{7,8-11,A8-A11}
\close
%Second part
\open
\hypo {B4}
{\before{\ameetvar{\avariable}{\avariablebis}{\avariableter}}{\ameetvar{\avariable}{\avariablefifth}{\avariablesix}}}
\hypo {B5}
{\ameetvar{\avariable}{\avariablefifth}{\avariablesix} = \ameetvar{\avariablefour}{\avariablefifth}{\avariablesix}}
\have {B6}
{\before{\ameetvar{\avariable}{\avariablefifth}{\avariablesix}}{\ameetvar{\avariablesept}{\avariableoct}{\avariablenine}}}
\by{\ref{axiom2:beforelemma0}}{2,B5}
\have {B7}
{\bigvee_{b \in \{\avariablesept,\avariableoct\}} \big(
\before{\ameetvar{\avariable}{\avariablefifth}{\avariablesix}}{\ameetvar{\avariable}{b}{\avariablenine}} \land\\ \ameetvar{\avariable}{b}{\avariablenine} = \ameetvar{\avariablesept}{\avariableoct}{\avariablenine}
\big)
}
\by{\defofbefore}{B6}
\open
\hypo {B8}
{\before{\ameetvar{\avariable}{\avariablefifth}{\avariablesix}}{\ameetvar{\avariable}{\avariablesept}{\avariablenine}}}
\hypo {B9} {\ameetvar{\avariable}{\avariablesept}{\avariablenine} = \ameetvar{\avariablesept}{\avariableoct}{\avariablenine}}
\have {B10} {\before{\ameetvar{\avariable}{\avariablebis}{\avariableter}}{\ameetvar{\avariable}{\avariablesept}{\avariablenine}}}
\by{\ref{axiom2:auxlemma17}}{B4,B8}
\have {B11} {\before{\ameetvar{\avariable}{\avariablebis}{\avariableter}}{\ameetvar{\avariablesept}{\avariableoct}{\avariablenine}}}
\by{\ref{axiom2:beforelemma0two}}{B9,B10}
\close
\open
\hypo {BA8}
{\before{\ameetvar{\avariable}{\avariablefifth}{\avariablesix}}{\ameetvar{\avariable}{\avariableoct}{\avariablenine}}}
\hypo {BA9} {\ameetvar{\avariable}{\avariableoct}{\avariablenine} = \ameetvar{\avariablesept}{\avariableoct}{\avariablenine}}
\have {BA10} {\before{\ameetvar{\avariable}{\avariablebis}{\avariableter}}{\ameetvar{\avariable}{\avariableoct}{\avariablenine}}}
\by{\ref{axiom2:auxlemma17}}{B4,A8}
\have {BA11} {\before{\ameetvar{\avariable}{\avariablebis}{\avariableter}}{\ameetvar{\avariablesept}{\avariableoct}{\avariablenine}}}
\by{\ref{axiom2:beforelemma0two}}{BA9,BA10}
\close
\have {B12} {\before{\ameetvar{\avariable}{\avariablebis}{\avariableter}}{\ameetvar{\avariablesept}{\avariableoct}{\avariablenine}}}
\oe{B7,B8-B11,BA8-BA11}
\close
\have {F}
{\before{\ameetvar{\avariable}{\avariablebis}{\avariableter}}{\ameetvar{\avariablesept}{\avariableoct}{\avariablenine}}}
\oe{3,4-12,B4-B12}
\end{nd}
\]
\end{enumerate}

\subsubsection{\ref{axiom2:definetobefore}}
We want to prove that the following formula is a tautology:
\begin{nscenter}
$\begin{aligned}
&\defined{\ameetvar{\avariable}{\avariablebis}{\avariableter}} \land \defined{\ameetvar{\avariable}{\avariablefour}{\avariablefifth}} \land \ameetvar{\avariable}{\avariablebis}{\avariableter} \neq \ameetvar{\avariable}{\avariablefour}{\avariablefifth}\implies\\
&\before{\ameetvar{\avariable}{\avariablebis}{\avariableter}}{\ameetvar{\avariable}{\avariablefour}{\avariablefifth}}
\lor \before{\ameetvar{\avariable}{\avariablefour}{\avariablefifth}}{\ameetvar{\avariable}{\avariablebis}{\avariableter}}
\end{aligned}$\qquad
(\ref{axiom2:definetobefore})
\end{nscenter}
We first prove two intermediate results.\\
\begin{enumerate}[label=\textbf{Aux\arabic*},align=left]
\setcounter{enumi}{14}
\item\label{axiom2:auxlemmajune1}
$
\boxed{
\begin{aligned}[t]
&\symmetric{\ameetvar{\avariable}{\avariablebis}{\avariableter}}
\land \symmetric{\ameetvar{\avariable}{\avariablefour}{\avariableter}}
\land \ameetvar{\avariable}{\avariablebis}{\avariableter} \neq \ameetvar{\avariable}{\avariablefour}{\avariableter}\\
&\implies \before{\ameetvar{\avariable}{\avariablebis}{\avariableter}}{\ameetvar{\avariable}{\avariablefour}{\avariableter}}
\lor \before{\ameetvar{\avariable}{\avariablefour}{\avariableter}}{\ameetvar{\avariable}{\avariablebis}{\avariableter}}
\end{aligned}
}
$

\[
  \begin{nd}
  \hypo {1} {\symmetric{\ameetvar{\avariable}{\avariablebis}{\avariableter}}}
  \hypo {2} {\symmetric{\ameetvar{\avariable}{\avariablefour}{\avariableter}}}
  \hypo {3} {\ameetvar{\avariable}{\avariablebis}{\avariableter} \neq \ameetvar{\avariable}{\avariablefour}{\avariableter}}
  \have {4} {\defined{\ameetvar{\avariable}{\avariablebis}{\avariableter}}} \ae{1}
  \have {5} {\defined{\ameetvar{\avariable}{\avariablefour}{\avariableter}}} \ae{2}
  \have {6} {\ameetvar{\avariable}{\avariablefour}{\avariableter} = \ameetvar{\avariablebis}{\avariablefour}{\avariableter}
  \lor\\ \ameetvar{\avariable}{\avariablefour}{\avariableter} \neq \ameetvar{\avariablebis}{\avariablefour}{\avariableter}} \by{\trivialtrue}{}
  \open
  \hypo {7} {\ameetvar{\avariable}{\avariablefour}{\avariableter} = \ameetvar{\avariablebis}{\avariablefour}{\avariableter}}
  \have {8} {\ameetvar{\avariable}{\avariablebis}{\avariableter} \neq \ameetvar{\avariablebis}{\avariablefour}{\avariableter}} \by{\ref{core2Ax:Substitute}}{3,7}
  \have {9} {\before{\ameetvar{\avariable}{\avariablebis}{\avariableter}}{\ameetvar{\avariable}{\avariablefour}{\avariableter}}} \by{\defofbefore}{1,3,4,5,8}
  \have {10} {\before{\ameetvar{\avariable}{\avariablebis}{\avariableter}}{\ameetvar{\avariable}{\avariablefour}{\avariableter}}
  \lor\\ \before{\ameetvar{\avariable}{\avariablefour}{\avariableter}}{\ameetvar{\avariable}{\avariablebis}{\avariableter}}}
  \oi{9}
  \close
  \open
  \hypo {11} {\ameetvar{\avariable}{\avariablefour}{\avariableter} \neq \ameetvar{\avariablebis}{\avariablefour}{\avariableter}}
  \have {12} {\ameetvar{\avariable}{\avariablebis}{\avariableter} = \ameetvar{\avariable}{\avariablefour}{\avariableter} \lor\\ \ameetvar{\avariable}{\avariablebis}{\avariableter} = \ameetvar{\avariablebis}{\avariablefour}{\avariableter}} \by{\ref{core2Ax:Before}}{1,5,11}
  \have {13} {\ameetvar{\avariable}{\avariablebis}{\avariableter} = \ameetvar{\avariablebis}{\avariablefour}{\avariableter}} \by{\modusponens}{3,12}
  \have {14} {\symmetric{\ameetvar{\avariablebis}{\avariablefour}{\avariableter}}} \by{\ref{axiom2:auxlemma6}}{1,2}
  \have {15} {\ameetvar{\avariable}{\avariablebis}{\avariableter} = \ameetvar{\avariablefour}{\avariablebis}{\avariableter}} \by{\ref{core2Ax:Substitute}}{13,14}
  \have {16} {\ameetvar{\avariablefour}{\avariablebis}{\avariableter} = \ameetvar{\avariable}{\avariablefour}{\avariableter}} \by{\ref{core2Ax:Substitute}}{3,15}
  \have {17} {\before{\ameetvar{\avariable}{\avariablefour}{\avariableter}}{\ameetvar{\avariable}{\avariablebis}{\avariableter}}} \by{\defofbefore}{2,3,4,5,16}
  \have {18} {\before{\ameetvar{\avariable}{\avariablebis}{\avariableter}}{\ameetvar{\avariable}{\avariablefour}{\avariableter}}
  \lor\\ \before{\ameetvar{\avariable}{\avariablefour}{\avariableter}}{\ameetvar{\avariable}{\avariablebis}{\avariableter}}}
  \oi{17}
  \close
  \have {19} {\before{\ameetvar{\avariable}{\avariablebis}{\avariableter}}{\ameetvar{\avariable}{\avariablefour}{\avariableter}}
  \lor\\ \before{\ameetvar{\avariable}{\avariablefour}{\avariableter}}{\ameetvar{\avariable}{\avariablebis}{\avariableter}}}
  \oe{6,7-10,11-19}
  \end{nd}
\]

\item\label{axiom2:auxlemma18}
$
\boxed{
\begin{aligned}[t]
&\symmetric{\ameetvar{\avariable}{\avariablebis}{\avariableter}}
\land \symmetric{\ameetvar{\avariable}{\avariablefour}{\avariablefifth}}
\land \ameetvar{\avariable}{\avariablebis}{\avariableter} \neq \ameetvar{\avariable}{\avariablefour}{\avariablefifth}\\
&\implies \before{\ameetvar{\avariable}{\avariablebis}{\avariableter}}{\ameetvar{\avariable}{\avariablefour}{\avariablefifth}}
\lor \before{\ameetvar{\avariable}{\avariablefour}{\avariablefifth}}{\ameetvar{\avariable}{\avariablebis}{\avariableter}}
\end{aligned}
}
$
\[
\begin{nd}
\hypo {1} {\symmetric{\ameetvar{\avariable}{\avariablebis}{\avariableter}}}
\hypo {2} {\symmetric{\ameetvar{\avariable}{\avariablefour}{\avariablefifth}}}
\hypo {3} {\ameetvar{\avariable}{\avariablebis}{\avariableter} \neq \ameetvar{\avariable}{\avariablefour}{\avariablefifth}}
\have {4} {\defined{\ameetvar{\avariable}{\avariablebis}{\avariableter}}} \ae{1}
\have {5} {\defined{\ameetvar{\avariable}{\avariablefour}{\avariablefifth}}} \ae{2}
\have {6} {\defined{\ameetvar{\avariableter}{\avariableter}{\avariablefifth}} \lor \defined{\ameetvar{\avariablefifth}{\avariablefifth}{\avariableter}}} \by{\ref{core2Ax:PedLinear}}{4,5}
\open
  \hypo {A1} {\defined{\ameetvar{\avariableter}{\avariableter}{\avariablefifth}}}
  \have {A2} {\defined{\ameetvar{\avariable}{\avariablebis}{\avariablefifth}}} \by{\ref{core2Ax:Pedix}}{4,A1}
  \end{nd}
  \]
  \[
  \begin{ndresume}
  \have {A6b} {\ameetvar{\avariable}{\avariablebis}{\avariableter} = \ameetvar{\avariable}{\avariablebis}{\avariablefifth}} \by{\ref{core2Ax:EqDef}}{4,A2}
  \have {A2b} {\ameetvar{\avariable}{\avariablebis}{\avariablefifth} = \ameetvar{\avariablebis}{\avariable}{\avariableter}} \by{\ref{core2Ax:Substitute} and \ref{core2Ax:EqSymm}}{1,A6b}
  \have {A2c} {\symmetric{\ameetvar{\avariable}{\avariablebis}{\avariablefifth}}} \by{\ref{axiom2:auxlemma11}}{A2b}
  \have {zz1} {\ameetvar{\avariable}{\avariablebis}{\avariablefifth} \neq \ameetvar{\avariable}{\avariablefour}{\avariablefifth}} \by{\ref{core2Ax:Substitute}}{3,A6b}
  \have {zz2} {
  \before{\ameetvar{\avariable}{\avariablebis}{\avariablefifth}}{\ameetvar{\avariable}{\avariablefour}{\avariablefifth}}
  \lor\\ \before{\ameetvar{\avariable}{\avariablefour}{\avariablefifth}}{\ameetvar{\avariable}{\avariablebis}{\avariablefifth}}
  } \by{\ref{axiom2:auxlemmajune1}}{2,A2c,zz1}
  \have {zz3} {
  \before{\ameetvar{\avariable}{\avariablebis}{\avariableter}}{\ameetvar{\avariable}{\avariablefour}{\avariablefifth}}
  \lor\\ \before{\ameetvar{\avariable}{\avariablefour}{\avariablefifth}}{\ameetvar{\avariable}{\avariablebis}{\avariablefifth}}
  }
  \by{\ref{axiom2:beforelemma0} and \lorimpL}{A6b,zz2}
  \have {zz4} {
  \before{\ameetvar{\avariable}{\avariablebis}{\avariableter}}{\ameetvar{\avariable}{\avariablefour}{\avariablefifth}}
  \lor\\ \before{\ameetvar{\avariable}{\avariablefour}{\avariablefifth}}{\ameetvar{\avariable}{\avariablebis}{\avariableter}}
  }
  \by{\ref{axiom2:beforelemma0two} and \lorimpR}{A6b,zz3}
\close
\open
  \hypo {C1} {\defined{\ameetvar{\avariablefifth}{\avariablefifth}{\avariableter}}}
  \have {C2} {\defined{\ameetvar{\avariable}{\avariablefour}{\avariableter}}} \by{\ref{core2Ax:Pedix}}{5,C1}
  \have {C6b} {\ameetvar{\avariable}{\avariablefour}{\avariablefifth} = \ameetvar{\avariable}{\avariablefour}{\avariableter}} \by{\ref{core2Ax:EqDef}}{5,C2}
  \have {C2b} {\ameetvar{\avariable}{\avariablefour}{\avariableter} = \ameetvar{\avariablefour}{\avariable}{\avariablefifth}} \by{\ref{core2Ax:Substitute} and \ref{core2Ax:EqSymm}}{2,C6b}
  \have {C2c} {\symmetric{\ameetvar{\avariable}{\avariablefour}{\avariableter}}} \by{\ref{axiom2:auxlemma11}}{C2b}
  \have {yy1} {\ameetvar{\avariable}{\avariablebis}{\avariableter} \neq \ameetvar{\avariable}{\avariablefour}{\avariableter}} \by{\ref{core2Ax:Substitute}}{3,C6b}
  \have {yy2} {
  \before{\ameetvar{\avariable}{\avariablebis}{\avariableter}}{\ameetvar{\avariable}{\avariablefour}{\avariableter}}
  \lor\\ \before{\ameetvar{\avariable}{\avariablefour}{\avariableter}}{\ameetvar{\avariable}{\avariablebis}{\avariableter}}
  } \by{\ref{axiom2:auxlemmajune1}}{2,C2c,yy1}
  \have {yy3} {
  \before{\ameetvar{\avariable}{\avariablebis}{\avariableter}}{\ameetvar{\avariable}{\avariablefour}{\avariablefifth}}
  \lor\\ \before{\ameetvar{\avariable}{\avariablefour}{\avariableter}}{\ameetvar{\avariable}{\avariablebis}{\avariableter}}
  }
  \by{\ref{axiom2:beforelemma0two} and \lorimpL}{C6b,yy2}
  \have {yy4} {
  \before{\ameetvar{\avariable}{\avariablebis}{\avariableter}}{\ameetvar{\avariable}{\avariablefour}{\avariablefifth}}
  \lor\\ \before{\ameetvar{\avariable}{\avariablefour}{\avariablefifth}}{\ameetvar{\avariable}{\avariablebis}{\avariableter}}
  }
  \by{\ref{axiom2:beforelemma0} and \lorimpR}{C6b,yy3}
\close
\have {40} {\before{\ameetvar{\avariable}{\avariablebis}{\avariableter}}{\ameetvar{\avariable}{\avariablefour}{\avariablefifth}}
\lor\\ \before{\ameetvar{\avariable}{\avariablefour}{\avariablefifth}}{\ameetvar{\avariable}{\avariablebis}{\avariableter}}} \oe{6,A1-zz4,C1-yy4}
\end{ndresume}
\]
\end{enumerate}

\begin{enumerate}[align=left]
\item[\lemmalab{DefNeq{$\Rightarrow\!$}Before}{axiom2:definetobefore}]
$
\boxed{
\begin{aligned}[t]
&\defined{\ameetvar{\avariable}{\avariablebis}{\avariableter}} \land \defined{\ameetvar{\avariable}{\avariablefour}{\avariablefifth}} \land \ameetvar{\avariable}{\avariablebis}{\avariableter} \neq \ameetvar{\avariable}{\avariablefour}{\avariablefifth} \implies\\
&\before{\ameetvar{\avariable}{\avariablebis}{\avariableter}}{\ameetvar{\avariable}{\avariablefour}{\avariablefifth}}
\lor \before{\ameetvar{\avariable}{\avariablefour}{\avariablefifth}}{\ameetvar{\avariable}{\avariablebis}{\avariableter}}
\end{aligned}
}
$
\[
\begin{nd}
\hypo {1} {\defined{\ameetvar{\avariable}{\avariablebis}{\avariableter}}}
\hypo {2} {\defined{\ameetvar{\avariable}{\avariablefour}{\avariablefifth}}}
\hypo {3} {\ameetvar{\avariable}{\avariablebis}{\avariableter} \neq \ameetvar{\avariable}{\avariablefour}{\avariablefifth}}
\have {4} {\asymmetric{\ameetvar{\avariable}{\avariablebis}{\avariableter}} \lor\\ \lnot \asymmetric{\ameetvar{\avariable}{\avariablebis}{\avariableter}}} \by{\trivialtrue}{}
\open
\hypo {5} {\asymmetric{\ameetvar{\avariable}{\avariablebis}{\avariableter}}}
\have {6} {\before{\ameetvar{\avariable}{\avariablefour}{\avariablefifth}}{\ameetvar{\avariable}{\avariablebis}{\avariableter}}} \by{\ref{axiom2:auxlemma7}}{2,3,6}
\have {7}  {\before{\ameetvar{\avariable}{\avariablebis}{\avariableter}}{\ameetvar{\avariable}{\avariablefour}{\avariablefifth}}
\lor\\ \before{\ameetvar{\avariable}{\avariablefour}{\avariablefifth}}{\ameetvar{\avariable}{\avariablebis}{\avariableter}}}
\oi{6}
\close
\open
\hypo {8} {\lnot \asymmetric{\ameetvar{\avariable}{\avariablebis}{\avariableter}}}
\have {9} {\symmetric{\ameetvar{\avariable}{\avariablebis}{\avariableter}}} \by{\modusponens}{1,8}
\have {10} {\asymmetric{\ameetvar{\avariable}{\avariablefour}{\avariablefifth}} \lor \lnot \asymmetric{\ameetvar{\avariable}{\avariablefour}{\avariablefifth}}} \by{\trivialtrue}{}
\end{nd}
\]
\[
\begin{ndresume}
\open
\hypo {11} {\asymmetric{\ameetvar{\avariable}{\avariablefour}{\avariablefifth}}}
\have {12} {\before{\ameetvar{\avariable}{\avariablebis}{\avariableter}}{\ameetvar{\avariable}{\avariablefour}{\avariablefifth}}} \by{\ref{axiom2:auxlemma7}}{1,3,11}
\have {13} {\before{\ameetvar{\avariable}{\avariablebis}{\avariableter}}{\ameetvar{\avariable}{\avariablefour}{\avariablefifth}}
\lor\\ \before{\ameetvar{\avariable}{\avariablefour}{\avariablefifth}}{\ameetvar{\avariable}{\avariablebis}{\avariableter}}}
\oi{11}
\close
\open
\hypo {14} {\lnot \asymmetric{\ameetvar{\avariable}{\avariablefour}{\avariablefifth}}}
\have {15} {\symmetric{\ameetvar{\avariable}{\avariablefour}{\avariablefifth}}} \by{\modusponens}{2,14}
\have {16} {\before{\ameetvar{\avariable}{\avariablebis}{\avariableter}}{\ameetvar{\avariable}{\avariablefour}{\avariablefifth}}
\lor\\ \before{\ameetvar{\avariable}{\avariablefour}{\avariablefifth}}{\ameetvar{\avariable}{\avariablebis}{\avariableter}}} \by{\ref{axiom2:auxlemma18}}{3,9,15}
\close
\have {17} {\before{\ameetvar{\avariable}{\avariablebis}{\avariableter}}{\ameetvar{\avariable}{\avariablefour}{\avariablefifth}}
\lor\\ \before{\ameetvar{\avariable}{\avariablefour}{\avariablefifth}}{\ameetvar{\avariable}{\avariablebis}{\avariableter}}}
\oe{10,11-13,14-16}
\close
\have {18} {\before{\ameetvar{\avariable}{\avariablebis}{\avariableter}}{\ameetvar{\avariable}{\avariablefour}{\avariablefifth}}
\lor\\ \before{\ameetvar{\avariable}{\avariablefour}{\avariablefifth}}{\ameetvar{\avariable}{\avariablebis}{\avariableter}}}
\oe{4,5-7,8-17}
\end{ndresume}
\]

\end{enumerate}

\subsubsection{\ref{axiom2:beforefunc}}
\begin{enumerate}[align=left]
\item[\lemmalab{BeforeLinear}{axiom2:beforefunc}]
$\boxed{
\begin{aligned}[t]
&\before{\aterm_1}{\aterm_2} \land \before{\aterm_1}{\aterm_3} \land \aterm_2 \neq \aterm_3 \implies\\ &\before{\aterm_2}{\aterm_3} \lor \before{\aterm_3}{\aterm_2}
\end{aligned}}
$\\
As usual, we prove the result for $\aterm_1$, $\aterm_2$ and $\aterm_3$ meet-point expressions.
\[
\begin{nd}
\hypo {1} {\before{\ameetvar{\avariable}{\avariablebis}{\avariableter}}{\ameetvar{\avariablefour}{\avariablefifth}{\avariablesix}}}
\hypo {2} {\before{\ameetvar{\avariable}{\avariablebis}{\avariableter}}{\ameetvar{\avariablesept}{\avariableoct}{\avariablenine}}}
\hypo {3} {\ameetvar{\avariablefour}{\avariablefifth}{\avariablesix} \neq \ameetvar{\avariablesept}{\avariableoct}{\avariablenine}}
\have {4} {\bigvee_{b \in \{\avariablefour,\avariablefifth\}} \big(
\before{\ameetvar{\avariable}{\avariablebis}{\avariableter}}{\ameetvar{\avariable}{b}{\avariablesix}} \land\\ \ameetvar{\avariable}{b}{\avariablesix} = \ameetvar{\avariablefour}{\avariablefifth}{\avariablesix}
\big)}
\by{\defofbefore}{1}
\open
\hypo {5} {\before{\ameetvar{\avariable}{\avariablebis}{\avariableter}}{\ameetvar{\avariable}{b}{\avariablesix}}} \by{where $b$ is $\avariablefour$ or $\avariablefifth$}{}
\hypo {6} {\ameetvar{\avariable}{b}{\avariablesix} = \ameetvar{\avariablefour}{\avariablefifth}{\avariablesix}}
\have {7} {\bigvee_{a \in \{\avariablesept,\avariableoct\}} \big(
\before{\ameetvar{\avariable}{\avariablebis}{\avariableter}}{\ameetvar{\avariable}{a}{\avariablenine}} \land\\ \ameetvar{\avariable}{a}{\avariablenine} = \ameetvar{\avariablesept}{\avariableoct}{\avariablesix}
\big)} \by{\defofbefore}{2}
\open
\hypo {8} {\before{\ameetvar{\avariable}{\avariablebis}{\avariableter}}{\ameetvar{\avariable}{a}{\avariablenine}}} \by{where $a$ is $\avariablesept$ or $\avariableoct$}{}
\hypo {9} {\ameetvar{\avariable}{a}{\avariablenine} = \ameetvar{\avariablesept}{\avariableoct}{\avariablesix}}
\have {10} {\ameetvar{\avariablefour}{\avariablefifth}{\avariablesix} \neq \ameetvar{\avariable}{a}{\avariablenine}} \by{\ref{core2Ax:Substitute}}{4,9}
\have {12} {\ameetvar{\avariable}{b}{\avariablesix} \neq \ameetvar{\avariable}{a}{\avariablenine}} \by{\ref{core2Ax:Substitute}}{6,10}
\have {13} {\defined{\ameetvar{\avariable}{b}{\avariablesix}}} \by{\ref{axiom2:auxlemma1}}{6}
\have {14} {\defined{\ameetvar{\avariable}{a}{\avariablenine}}} \by{\ref{axiom2:auxlemma1}}{9}
\have  {15} {\before{\ameetvar{\avariable}{b}{\avariablesix}}{\ameetvar{\avariable}{a}{\avariablenine}} \lor\\ \before{\ameetvar{\avariable}{a}{\avariablenine}}{\ameetvar{\avariable}{b}{\avariablesix}}}
\by{\ref{axiom2:definetobefore}}{12,13,14}
\have {17} {\before{\ameetvar{\avariablefour}{\avariablefifth}{\avariablesix}}{ \ameetvar{\avariablesept}{\avariableoct}{\avariablesix}} \lor\\
\before{\ameetvar{\avariablesept}{\avariableoct}{\avariablesix}}{\ameetvar{\avariablefour}{\avariablefifth}{\avariablesix}}}
\by{
$
\begin{aligned}[t]
&\ref{axiom2:beforelemma0}\\
&\ref{axiom2:beforelemma0two}\\
&\text{and prop. calc.}
\end{aligned}
$
}{6,9,15}
\close
\end{nd}
\]
\[
\begin{ndresume}
\have {18} {\before{\ameetvar{\avariablefour}{\avariablefifth}{\avariablesix}}{ \ameetvar{\avariablesept}{\avariableoct}{\avariablesix}} \lor\\
\before{\ameetvar{\avariablesept}{\avariableoct}{\avariablesix}}{\ameetvar{\avariablefour}{\avariablefifth}{\avariablesix}}}
\oe{7,8-17}
\close
\have {19} {\before{\ameetvar{\avariablefour}{\avariablefifth}{\avariablesix}}{ \ameetvar{\avariablesept}{\avariableoct}{\avariablesix}} \lor\\
\before{\ameetvar{\avariablesept}{\avariableoct}{\avariablesix}}{\ameetvar{\avariablefour}{\avariablefifth}{\avariablesix}}}
\oe{4,5-18}
\end{ndresume}
\]
\end{enumerate}

\subsubsection{\ref{axiom2:diffbeforemeet}}
\begin{enumerate}[align=left]
\item[\lemmalab{DiffBeforeMeet}{axiom2:diffbeforemeet}]
$
\boxed{
\begin{aligned}[t]
&\before{\ameetvar{\avariable}{\avariablefour}{\avariablefifth}}{\ameetvar{\avariable}{\avariablebis}{\avariableter}}
\land
\before{\ameetvar{\avariablebis}{\avariablesix}{\avariablesept}}{\ameetvar{\avariable}{\avariablebis}{\avariableter}}
\implies\\
&\ameetvar{\avariable}{\avariablefour}{\avariablefifth} \neq
\ameetvar{\avariablebis}{\avariablesix}{\avariablesept}
\end{aligned}
}
$
\[
\begin{nd}
\hypo {1} {\before{\ameetvar{\avariable}{\avariablefour}{\avariablefifth}}{\ameetvar{\avariable}{\avariablebis}{\avariableter}}}
\hypo {2} {\before{\ameetvar{\avariablebis}{\avariablesix}{\avariablesept}}{\ameetvar{\avariable}{\avariablebis}{\avariableter}}}
\have {3} {\ameetvar{\avariable}{\avariablefour}{\avariablefifth} \neq \ameetvar{\avariable}{\avariablebis}{\avariableter}} \ae{1}
\have {3a} {\defined{\ameetvar{\avariable}{\avariablebis}{\avariableter}}} \ae{1}
\have {3b} {\symmetric{\ameetvar{\avariablebis}{\avariablesix}{\avariablesept}}} \ae{2}
\have {3c} {\defined{\ameetvar{\avariablebis}{\avariablesix}{\avariableter}}} \ae{2}
\have {3d} {\symmetric{\ameetvar{\avariablebis}{\avariablesix}{\avariableter}}} \by{\ref{axiom2:auxlemma100}}{3b,3c}
\have {4} {\ameetvar{\avariablebis}{\avariable}{\avariableter} = \ameetvar{\avariablesix}{\avariable}{\avariableter}} \by{\ref{axiom2:auxlemma5}}{2}
\open
\hypo {5} {\ameetvar{\avariable}{\avariablefour}{\avariablefifth} =
\ameetvar{\avariablebis}{\avariablesix}{\avariablesept}}
\have {6} {\symmetric{\ameetvar{\avariable}{\avariablebis}{\avariablefifth}}} \by{\ref{core2Ax:Symmetric}}{5}
\have {6b} {\symmetric{\ameetvar{\avariable}{\avariablebis}{\avariableter}}} \by{\ref{axiom2:auxlemma100}}{3a,6}
\have {6c} {\symmetric{\ameetvar{\avariable}{\avariablesix}{\avariableter}}} \by{\ref{axiom2:auxlemma6}}{3b,6b}
\have {7} {\ameetvar{\avariable}{\avariablefour}{\avariablefifth} = \ameetvar{\avariable}{\avariablebis}{\avariablefifth} \lor\\ \ameetvar{\avariable}{\avariablefour}{\avariablefifth} = \ameetvar{\avariable}{\avariablesix}{\avariablefifth}}  \by{\ref{core2Ax:Symmetric}}{5}
\open
\hypo {8} {\ameetvar{\avariable}{\avariablefour}{\avariablefifth} = \ameetvar{\avariable}{\avariablebis}{\avariablefifth}}
\have {9} {\defined{\ameetvar{\avariable}{\avariablebis}{\avariablefifth}}} \by{\ref{axiom2:auxlemma1}}{8}
\have {10} {\ameetvar{\avariable}{\avariablefour}{\avariablefifth} \neq \ameetvar{\avariable}{\avariablebis}{\avariablefifth}} \by{\ref{core2Ax:Substitute}}{3,9}
\have {11} {\bottom} \by{\landcontr}{8,10}
\close
\open
\hypo {12} {\ameetvar{\avariable}{\avariablefour}{\avariablefifth} = \ameetvar{\avariable}{\avariablesix}{\avariablefifth}}
\have {13} {\ameetvar{\avariable}{\avariablebis}{\avariableter} = \ameetvar{\avariablesix}{\avariable}{\avariableter}} \by{\ref{core2Ax:Substitute}}{4,6}
\have {14} {\ameetvar{\avariable}{\avariablebis}{\avariableter} = \ameetvar{\avariable}{\avariablesix}{\avariableter}} \by{\ref{core2Ax:Substitute}}{6b,13}
\have {15} {\defined{\ameetvar{\avariable}{\avariablesix}{\avariableter}}} \by{\ref{axiom2:auxlemma1}}{14}
\have {16} {\ameetvar{\avariable}{\avariablefour}{\avariablefifth} = \ameetvar{\avariable}{\avariablesix}{\avariableter}} \by{\ref{axiom2:auxlemma13}}{12,15}
\have {17} {\ameetvar{\avariable}{\avariablebis}{\avariableter} = \ameetvar{\avariable}{\avariablefour}{\avariablefifth}} \by{\ref{core2Ax:Substitute}}{14,16}
\have {18} {\bottom} \by{\landcontr}{3,17}
\close
\have {19} {\bottom} \oe{7,8-11.12-18}
\close
\have {20} {\ameetvar{\avariable}{\avariablefour}{\avariablefifth} \neq
\ameetvar{\avariablebis}{\avariablesix}{\avariablesept}} \ni{5-19}
\end{nd}
\]
\end{enumerate}

\subsubsection{\ref{axiom2:samelooplemma0}}
\begin{enumerate}[align=left]
\item[\lemmalab{SameloopIrref}{axiom2:samelooplemma0}]
$
\boxed{\lnot\sameloop{\aterm}{\aterm}}
$\\
As usual, it is sufficient to prove the result for $\aterm$ meet-point expression.
\[
\begin{nd}
\hypo {1} {\sameloop{\ameetvar{\avariable}{\avariablebis}{\avariableter}}{\ameetvar{\avariable}{\avariablebis}{\avariableter}}}
\have {2}
{\asymmetric{\ameetvar{\avariable}{\avariable}{\avariableter}}}
\ae{1}
\have {3}
{\ameetvar{\avariable}{\avariable}{\avariableter} = \ameetvar{\avariable}{\avariable}{\avariableter}
\land \ameetvar{\avariable}{\avariable}{\avariableter} \neq \ameetvar{\avariable}{\avariable}{\avariableter}}
\by{\defofasym}{2}
\have {4} {\bottom} \by{\landcontr}{3}
\end{nd}
\]
\end{enumerate}

\subsubsection{\ref{axiom2:samelooplemma1}}
\begin{enumerate}[align=left]
\item[\lemmalab{SameloopSym}{axiom2:samelooplemma1}]
$
\boxed{\sameloop{\aterm_1}{\aterm_2} \implies \sameloop{\aterm_2}{\aterm_1}}
$\\
As usual, it is sufficient to prove the result for $\aterm_1$ and $\aterm_2$ meet-point expressions.
\[
\begin{nd}
\hypo {1} {\sameloop{\ameetvar{\avariable}{\avariablebis}{\avariableter}}{\ameetvar{\avariablefour}{\avariablefifth}{\avariablesix}}}
\have {2}
{\ameetvar{\avariable}{\avariablebis}{\avariableter} = \ameetvar{\avariable}{\avariablefour}{\avariablesix}}
 \ae{1}
\have {3}
{\ameetvar{\avariablefour}{\avariablefifth}{\avariablesix} = \ameetvar{\avariablefour}{\avariable}{\avariableter}} \ae{1}
\have {4}
{\asymmetric{\ameetvar{\avariable}{\avariablefour}{\avariableter}}} \ae{1}
\have {5} {\defined{\ameetvar{\avariable}{\avariablefour}{\avariablesix}}} \by{\ref{axiom2:auxlemma1}}{2}
\have {6} {\defined{\ameetvar{\avariablefour}{\avariable}{\avariablesix}}} \by{\ref{core2Ax:Bothdef}}{5}
\have {7} {\ameetvar{\avariable}{\avariablefour}{\avariableter} \neq  \ameetvar{\avariablefour}{\avariable}{\avariableter}} \ae{4}
\have {8} {\ameetvar{\avariable}{\avariablefour}{\avariablesix} \neq  \ameetvar{\avariablefour}{\avariable}{\avariableter}} \by{\ref{core2Ax:Substitute}}{5,7}
\have {9} {\ameetvar{\avariable}{\avariablefour}{\avariablesix} \neq  \ameetvar{\avariablefour}{\avariable}{\avariablesix}} \by{\ref{core2Ax:Substitute}}{6,8}
\have {10} {\asymmetric{\ameetvar{\avariablefour}{\avariable}{\avariablesix}}} \by{\ndref{6} $\land$ \ndref{9}}{}
\have {11} {\sameloop{\ameetvar{\avariablefour}{\avariablefifth}{\avariablesix}}{\ameetvar{\avariable}{\avariablebis}{\avariableter}}} \by{\defofsameloop}{2,3,10}
\end{nd}
\]
\end{enumerate}

\subsubsection{\ref{axiom2:samelooplemma2}}
\begin{enumerate}[align=left]
\item[\lemmalab{SameloopAlioTrans}{axiom2:samelooplemma2}]
$
\boxed{
\begin{aligned}[t]
&\sameloop{\aterm_1}{\aterm_2} \land \sameloop{\aterm_2}{\aterm_3} \land \aterm_1 \neq \aterm_3 \implies\\ &\sameloop{\aterm_1}{\aterm_3}
\end{aligned}}
$\\
As usual, it is sufficient to prove the result for $\aterm_1$, $\aterm_2$ and $\aterm_3$ meet-point expressions.
\[
\begin{nd}
\hypo {1} {\sameloop{\ameetvar{\avariable}{\avariablebis}{\avariableter}}{\ameetvar{\avariablefour}{\avariablefifth}{\avariablesix}}}
\hypo {2}
{\sameloop{\ameetvar{\avariablefour}{\avariablefifth}{\avariablesix}}{\ameetvar{\avariablesept}{\avariableoct}{\avariablenine}}}
\hypo {3}
{\ameetvar{\avariable}{\avariablebis}{\avariableter} \neq \ameetvar{\avariablesept}{\avariableoct}{\avariablenine}}
\have {4}
{\ameetvar{\avariable}{\avariablebis}{\avariableter} = \ameetvar{\avariable}{\avariablefour}{\avariablesix}}
\ae{1}
\end{nd}
\]
\[
\begin{ndresume}
\have {5}
{\ameetvar{\avariablefour}{\avariablefifth}{\avariablesix} = \ameetvar{\avariablefour}{\avariable}{\avariableter}} \ae{1}
\have {6}
{\asymmetric{\ameetvar{\avariable}{\avariablefour}{\avariableter}}} \ae{1}
\have {4B}
{\ameetvar{\avariablefour}{\avariablefifth}{\avariablesix} = \ameetvar{\avariablefour}{\avariablesept}{\avariablenine}}
\ae{2}
\have {5B}
{\ameetvar{\avariablesept}{\avariableoct}{\avariablenine} = \ameetvar{\avariablesept}{\avariablefour}{\avariablesix}} \ae{2}
\have {6B}
{\asymmetric{\ameetvar{\avariablefour}{\avariablesept}{\avariablesix}}} \ae{2}
\have {7} {\defined{\ameetvar{\avariablefour}{\avariablefifth}{\avariableter}}}
\by{\ref{core2Ax:PedInv}}{5}
\have {8} {\ameetvar{\avariablefour}{\avariablefifth}{\avariableter} = \ameetvar{\avariablefour}{\avariablesept}{\avariablenine}}
\by{\ref{core2Ax:Substitute}}{4B,7}
\have {9}
{\defined{\ameetvar{\avariablefour}{\avariablesept}{\avariableter}}}
\by{\ref{core2Ax:PedInv}}{8}
\have {10}
{\defined{\ameetvar{\avariablesept}{\avariablefour}{\avariableter}}}
\by{\ref{core2Ax:Bothdef}}{9}
\have {11}
{\defined{\ameetvar{\avariable}{\avariablebis}{\avariableter}}}
\by{\ref{axiom2:auxlemma1}}{4}
\have {12}
{\defined{\ameetvar{\avariable}{\avariablesept}{\avariableter}}}
\by{\ref{core2Ax:PedDefines}}{10,11}
\open
\hypo {S1} {\symmetric{\ameetvar{\avariable}{\avariablesept}{\avariableter}}}
\have {S2} {\ameetvar{\avariable}{\avariablefour}{\avariableter} = \ameetvar{\avariablesept}{\avariablefour}{\avariableter}}
\by{\ref{core2Ax:OneAsym}}{6,S1}
\have {S3} {\defined{\ameetvar{\avariablesept}{\avariablefour}{\avariablesix}}}
\by{\ref{axiom2:auxlemma1}}{5B}
\have {S4} {\ameetvar{\avariable}{\avariablefour}{\avariableter} = \ameetvar{\avariablesept}{\avariablefour}{\avariablesix}}
\by{\ref{axiom2:auxlemma13}}{S2,S3}
\have {S5} {\ameetvar{\avariable}{\avariablebis}{\avariableter} = \ameetvar{\avariablesept}{\avariablefour}{\avariablesix}}
\by{\ref{core2Ax:Substitute}}{4,S4}
\have {S6} {\ameetvar{\avariable}{\avariablebis}{\avariableter} = \ameetvar{\avariablesept}{\avariableoct}{\avariablenine}}
\by{\ref{core2Ax:Substitute}}{5B,S5}
\have {S7} {\bottom} \by{\landcontr}{3,S6}
\close
\have {13} {\lnot \symmetric{\ameetvar{\avariable}{\avariablesept}{\avariableter}}}
\ni{S1-S7}
\have {14} {\asymmetric{\ameetvar{\avariable}{\avariablesept}{\avariableter}}} \by{\modusponens}{12,13}
\have {15} {\ameetvar{\avariable}{\avariablefour}{\avariableter} = \ameetvar{\avariable}{\avariablesept}{\avariableter}}
\by{\ref{core2Ax:BothAsym}}{5,14}
\have {16} {\ameetvar{\avariable}{\avariablebis}{\avariableter} = \ameetvar{\avariable}{\avariablesept}{\avariableter}}
\by{\ref{core2Ax:Substitute}}{4,15}
\have {17} {\asymmetric{\ameetvar{\avariablesept}{\avariable}{\avariableter}}}
\by{\defofasym}{14}
\have {18} {\asymmetric{\ameetvar{\avariablesept}{\avariablefour}{\avariablesix}}}
\by{\defofasym}{6B}
\have {19} {\ameetvar{\avariablesept}{\avariable}{\avariableter} = \ameetvar{\avariablesept}{\avariablefour}{\avariablesix}} \by{\ref{core2Ax:BothAsym}}{17,18}
\have {20} {\ameetvar{\avariablesept}{\avariable}{\avariableter} = \ameetvar{\avariablesept}{\avariableoct}{\avariablenine}} \by{\ref{core2Ax:Substitute}}{5B,19}
\have {21} {\defined{\ameetvar{\avariablesept}{\avariable}{\avariablenine}}} \by{\ref{axiom2:auxlemma1}}{20}
\have {22} {\defined{\ameetvar{\avariable}{\avariablesept}{\avariablenine}}} \by{\ref{core2Ax:Bothdef}}{21}
\have {23} {\ameetvar{\avariable}{\avariablebis}{\avariableter} = \ameetvar{\avariable}{\avariablesept}{\avariablenine}} \by{\ref{core2Ax:Substitute}}{16,22}
\have {24} {\sameloop{\ameetvar{\avariable}{\avariablebis}{\avariableter}}{\ameetvar{\avariablesept}{\avariableoct}{\avariablenine}}} \by{\defofsameloop}{14,20,23}
\end{ndresume}
\]
\end{enumerate}

\subsubsection{\ref{axiom2:samelooplemma0two}}
\begin{enumerate}[align=left]
\item[\lemmalab{Asym{$\Rightarrow\!$}Sameloop}{axiom2:samelooplemma0two}]
$
\boxed{\asymmetric{\ameetvar{\avariable}{\avariablebis}{\avariableter}}\implies \sameloop{\ameetvar{\avariable}{\avariablebis}{\avariableter}}{\ameetvar{\avariablebis}{\avariable}{\avariableter}}}
$\\
\[
\begin{nd}
\hypo {1} {\asymmetric{\ameetvar{\avariable}{\avariablebis}{\avariableter}}}
\have {2} {\defined{\ameetvar{\avariable}{\avariablebis}{\avariableter}}} \ae{1}
\have {3} {\defined{\ameetvar{\avariablebis}{\avariable}{\avariableter}}} \by{\ref{core2Ax:Bothdef}}{2}
\have {4} {\sameloop{\ameetvar{\avariable}{\avariablebis}{\avariableter}}{\ameetvar{\avariablebis}{\avariable}{\avariableter}}}
\by{\defofsameloop}{1,2,3}
\end{nd}
\]
\end{enumerate}

\subsubsection{\ref{axiom2:sameloopsubr}}

\begin{enumerate}[align=left]
\item[\lemmalab{SameloopSubR}{axiom2:sameloopsubr}]
$
\boxed{\sameloop{\aterm_1}{\aterm_2} \land \aterm_2 = \aterm_3 \implies \sameloop{\aterm_1}{\aterm_3}}
$\\
As usual, it is sufficient to show the case for $\aterm_1$, $\aterm_2$ and $\aterm_3$ meet-points expressions.
\[
\begin{nd}
\hypo {1} {\sameloop{\ameetvar{\avariable}{\avariablebis}{\avariableter}}{\ameetvar{\avariablefour}{\avariablefifth}{\avariablesix}}}
\hypo {2} {\ameetvar{\avariablefour}{\avariablefifth}{\avariablesix} = \ameetvar{\avariablesept}{\avariableoct}{\avariablenine}}
\have {3} {\ameetvar{\avariable}{\avariablebis}{\avariableter} = \ameetvar{\avariable}{\avariablefour}{\avariablesix}} \ae{1}
\have {4} {\ameetvar{\avariablefour}{\avariablefifth}{\avariablesix} = \ameetvar{\avariablefour}{\avariable}{\avariableter}} \ae{1}
\have {5} {\asymmetric{\ameetvar{\avariable}{\avariablefour}{\avariableter}}} \ae{1}
\have {6} {\ameetvar{\avariablefour}{\avariablefifth}{\avariablesix} = \ameetvar{\avariablesept}{\avariableoct}{\avariablesix}} \by{\ref{axiom2:auxlemma13}}{2}
\have {7} {\symmetric{\ameetvar{\avariablefour}{\avariablesept}{\avariablesix}}} \by{\ref{core2Ax:Symmetric}}{6}
\have {8} {\defined{\ameetvar{\avariable}{\avariablefour}{\avariablesix}}} \by{\ref{core2Ax:PedInv}}{3}
\have {9} {\defined{\ameetvar{\avariablefour}{\avariable}{\avariablesix}}} \by{\ref{core2Ax:Bothdef}}{8}
\have {10} {\ameetvar{\avariable}{\avariablefour}{\avariablesix}=\ameetvar{\avariable}{\avariablefour}{\avariablesix} \land \ameetvar{\avariable}{\avariablefour}{\avariablesix}\neq\ameetvar{\avariablefour}{\avariable}{\avariableter}} \by{\ref{core2Ax:Substitute}}{5,8}
\have {12} {\asymmetric{\ameetvar{\avariable}{\avariablefour}{\avariablesix}}}
\by{\ref{core2Ax:Substitute}}{9,10}
\have {13} {\ameetvar{\avariablesept}{\avariable}{\avariablesix} = \ameetvar{\avariablefour}{\avariable}{\avariablesix} \land \ameetvar{\avariable}{\avariablesept}{\avariablesix} = \ameetvar{\avariable}{\avariablefour}{\avariablesix}}
\by{\ref{core2Ax:OneAsym}}{7,12}
\have {14} {\ameetvar{\avariablefour}{\avariablefifth}{\avariablesix} = \ameetvar{\avariablefour}{\avariable}{\avariablesix}} \by{\ref{axiom2:auxlemma11}}{4}
\have {15} {\ameetvar{\avariablefour}{\avariablefifth}{\avariablesix} = \ameetvar{\avariablesept}{\avariable}{\avariablesix}}
\by{\ref{core2Ax:Substitute}}{13,14}
\have {16} {\ameetvar{\avariable}{\avariablebis}{\avariableter} = \ameetvar{\avariable}{\avariablesept}{\avariablesix}}
\by{\ref{core2Ax:Substitute}}{3,13}
\have {17} {\defined{\ameetvar{\avariable}{\avariablesept}{\avariableter}}} \by{\ref{core2Ax:PedInv}}{16}
\have {18} {\defined{\ameetvar{\avariablesept}{\avariable}{\avariableter}}} \by{\ref{core2Ax:Bothdef}}{17}
\have {19} {\ameetvar{\avariablefour}{\avariablefifth}{\avariablesix} = \ameetvar{\avariablesept}{\avariable}{\avariableter}}
\by{\ref{core2Ax:Substitute}}{15,18}
\have {20} {\ameetvar{\avariablesept}{\avariableoct}{\avariablenine} = \ameetvar{\avariablesept}{\avariable}{\avariableter}}
\by{\ref{core2Ax:Substitute}}{2,19}
\have {21} {\defined{\ameetvar{\avariablesept}{\avariable}{\avariablenine}}} \by{\ref{core2Ax:PedInv}}{20}
\have {22} {\defined{\ameetvar{\avariable}{\avariablesept}{\avariablenine}}} \by{\ref{core2Ax:Bothdef}}{21}
\have {23} {\ameetvar{\avariable}{\avariablebis}{\avariableter} = \ameetvar{\avariable}{\avariablesept}{\avariablenine}} \by{\ref{axiom2:auxlemma1}}{16,22}
\open
\hypo {24} {\symmetric{\ameetvar{\avariablesept}{\avariable}{\avariableter}}}
\have {25} {\ameetvar{\avariablesept}{\avariable}{\avariableter} = \ameetvar{\avariablefour}{\avariable}{\avariablesix}} \by{\ref{axiom2:auxlemma13}}{13,18}
\have {26} {\ameetvar{\avariable}{\avariablesept}{\avariableter} = \ameetvar{\avariable}{\avariablefour}{\avariablesix}} \by{\ref{axiom2:auxlemma13}}{13,17}
\have {27} {\ameetvar{\avariablesept}{\avariable}{\avariableter} = \ameetvar{\avariable}{\avariablefour}{\avariablesix}} \by{\ref{core2Ax:Substitute}}{24,26}
\have {28} {\symmetric{\ameetvar{\avariable}{\avariablefour}{\avariablesix}}} \by{\ref{core2Ax:Substitute}}{25,27}
\have {29} {\ameetvar{\avariable}{\avariablefour}{\avariablesix} \neq \ameetvar{\avariablefour}{\avariable}{\avariablesix}}
\ae{12}
\have {30} {\bottom} \by{\landcontr}{28,29}
\close
\have {31} {\lnot \symmetric{\ameetvar{\avariablesept}{\avariable}{\avariableter}}} \ni{24-30}
\have {32} {\asymmetric{\ameetvar{\avariablesept}{\avariable}{\avariableter}}} \by{\ndref{18} $\land$ \ndref{31}}{}
\have {33} {\sameloop{\ameetvar{\avariable}{\avariablebis}{\avariableter}}{\ameetvar{\avariablesept}{\avariableoct}{\avariablenine}}}
\by{\defofsameloop}{20,23,32}
\end{nd}
\]
\end{enumerate}

\subsubsection{\ref{axiom2:sameloopsubl}}

\begin{enumerate}[align=left]
\item[\lemmalab{SameloopSubL}{axiom2:sameloopsubl}]
$
\boxed{\sameloop{\aterm_1}{\aterm_2} \land \aterm_1 = \aterm_3 \implies \sameloop{\aterm_3}{\aterm_2}}
$
\[
\begin{nd}
\hypo {1} {\sameloop{\aterm_1}{\aterm_2}}
\hypo {2} {\aterm_1 = \aterm_3}
\have {3} {\sameloop{\aterm_2}{\aterm_1}} \by{\ref{axiom2:samelooplemma1}}{1}
\have {4} {\sameloop{\aterm_2}{\aterm_3}} \by{\ref{axiom2:sameloopsubr}}{2,3}
\have {5} {\sameloop{\aterm_3}{\aterm_2}} \by{\ref{axiom2:samelooplemma1}}{4}
\end{nd}
\]
\end{enumerate}

\subsubsection{\ref{axiom2:subscriptforward}}

\begin{enumerate}[align=left]
\item[\lemmalab{SubscriptForward}{axiom2:subscriptforward}]
$
\boxed{
\begin{aligned}[t]
\defined{\ameetvar{\avariable}{\avariablebis}{\avariableter}} \land \avariableter \neq \ameetvar{\avariable}{\avariablebis}{\avariableter} \implies\\
\before{\ameetvar{\avariable}{\avariablebis}{\avariableter}}{\avariableter} \lor \sameloop{\ameetvar{\avariable}{\avariableter}{\avariableter}}{\avariableter}
\end{aligned}
}
$
\[
\begin{nd}
\hypo {1} {\defined{\ameetvar{\avariable}{\avariablebis}{\avariableter}}}
\hypo {2} {\avariableter \neq \ameetvar{\avariable}{\avariablebis}{\avariableter}}
\have {3} {\defined{\ameetvar{\avariableter}{\avariable}{\avariableter}}} \by{\ref{axiom2:auxlemmaPedDef}}{1}
\have {3b} {\defined{\ameetvar{\avariable}{\avariableter}{\avariableter}}} \by{\ref{core2Ax:Bothdef}}{3}
\have {4} {\avariableter = \ameetvar{\avariableter}{\avariable}{\avariableter}} \by{\ref{core2Ax:Self2}}{3}
\have {5} {\defined{\ameetvar{\avariablebis}{\avariable}{\avariableter}}} \by{\ref{core2Ax:Bothdef}}{1}
\have {6} {\defined{\ameetvar{\avariableter}{\avariablebis}{\avariableter}}} \by{\ref{core2Ax:PedDefines}}{3,5}
\have {6b} {\avariableter = \ameetvar{\avariableter}{\avariablebis}{\avariableter}} \by{\ref{core2Ax:Self2}}{6}
\have {6c} {\ameetvar{\avariableter}{\avariable}{\avariableter} = \ameetvar{\avariableter}{\avariablebis}{\avariableter}} \by{\ref{core2Ax:Substitute}}{4,6b}
\have {7} {\avariableter = \ameetvar{\avariable}{\avariableter}{\avariableter} \lor \avariableter \neq \ameetvar{\avariable}{\avariableter}{\avariableter} } \by{\trivialtrue}{}
\open
\hypo {8} {\avariableter = \ameetvar{\avariable}{\avariableter}{\avariableter}}
\have {9} {\ameetvar{\avariable}{\avariablebis}{\avariableter} \neq \ameetvar{\avariable}{\avariableter}{\avariableter}} \by{\ref{core2Ax:Substitute}}{2,8}
\have {10} {\before{\ameetvar{\avariable}{\avariableter}{\avariableter}}{\ameetvar{\avariable}{\avariablebis}{\avariableter}} \lor\\ \before{\ameetvar{\avariable}{\avariablebis}{\avariableter}}{\ameetvar{\avariable}{\avariableter}{\avariableter}}}
\by{\ref{axiom2:definetobefore}}{1,3b,9}
\open
\hypo {11} {\before{\ameetvar{\avariable}{\avariableter}{\avariableter}}{\ameetvar{\avariable}{\avariablebis}{\avariableter}}}
\have {12} {\symmetric{\ameetvar{\avariable}{\avariableter}{\avariableter}}} \ae{11}
\have {13} {\ameetvar{\avariable}{\avariableter}{\avariableter} \neq \ameetvar{\avariableter}{\avariablebis}{\avariableter}} \ae{11}
\have {14} {\ameetvar{\avariableter}{\avariable}{\avariableter} \neq \ameetvar{\avariableter}{\avariablebis}{\avariableter}} \by{\ref{core2Ax:Substitute}}{12,13}
\have {15} {\bottom} \by{\landcontr}{6c,14}
\close
\have {16} {\before{\ameetvar{\avariable}{\avariableter}{\avariableter}}{\ameetvar{\avariable}{\avariablebis}{\avariableter}}} \ni{11-15}
\have {17} {\before{\ameetvar{\avariable}{\avariablebis}{\avariableter}}{\ameetvar{\avariable}{\avariableter}{\avariableter}}} \by{\modusponens}{7,16}
\have {18} {\before{\ameetvar{\avariable}{\avariablebis}{\avariableter}}{\avariableter} \lor\\ \sameloop{\ameetvar{\avariable}{\avariableter}{\avariableter}}{\avariableter}} \oi{17}
\close
\open
\hypo {19} {\avariableter \neq \ameetvar{\avariable}{\avariableter}{\avariableter}}
\have {20} {\ameetvar{\avariableter}{\avariable}{\avariableter} \neq \ameetvar{\avariable}{\avariableter}{\avariableter}} \by{\ref{core2Ax:Substitute}}{4}
\have {21} {\asymmetric{\ameetvar{\avariable}{\avariableter}{\avariableter}}} \by{\ndref{3b} $\land$ \ndref{20}}{}
\have {22} {\sameloop{\ameetvar{\avariable}{\avariableter}{\avariableter}}{\ameetvar{\avariableter}{\avariable}{\avariableter}}} \by{\ref{axiom2:samelooplemma0two}}{19,21}
\have {23} {\sameloop{\ameetvar{\avariable}{\avariableter}{\avariableter}}{\avariableter}} \by{\ref{axiom2:sameloopsubr}}{4,22}
\have {24} {\before{\ameetvar{\avariable}{\avariablebis}{\avariableter}}{\avariableter} \lor\\ \sameloop{\ameetvar{\avariable}{\avariableter}{\avariableter}}{\avariableter}} \oi{23}
\close
\have {25} {\before{\ameetvar{\avariable}{\avariablebis}{\avariableter}}{\avariableter} \lor\\ \sameloop{\ameetvar{\avariable}{\avariableter}{\avariableter}}{\avariableter}} \oe{7,8-18,19-24}
\end{nd}
\]
\end{enumerate}
