# Supplementary material for: A Complete Axiomatisation for Quantifier-Free Separation Logic
Source: arXiv:2006.05156 source file (2021-08-09)
Supplement: Supplementary file 4 [file apdxsection-int-taut-sees.tex]

\subsubsection{\ref{axiom2:notseeseq}}
\begin{enumerate}[align=left]
\item[\lemmalab{NotSeesEq}{axiom2:notseeseq}]
$
\boxed{
\aterm_3 \in \asetmeetvar \implies (\lnot \sees{\aterm_1}{\aterm_2}{\asetmeetvar\cup\{\aterm_3\}} \iff \lnot\sees{\aterm_1}{\aterm_2}{\asetmeetvar})}
$\\
We show one direction of the double implication, the other is analogous.
\[
\begin{nd}
\hypo {1} {\lnot \sees{\aterm_1}{\aterm_2}{\asetmeetvar\cup\{\aterm_3\}}}
\hypo {2} {\aterm_3 \in \asetmeetvar}
\open
\hypo {3} {\sees{\aterm_1}{\aterm_2}{\asetmeetvar}}
\have {4} {\sees{\aterm_1}{\aterm_2}{\{\aterm_3\} \cup \asetmeetvar}} \by{\ref{core2Ax:SeesTermEq}}{2,3}
\have {5} {\bottom} \by{\landcontr}{1,4}
\close
\have {6} {\lnot\sees{\aterm_1}{\aterm_2}{\asetmeetvar}} \ni{3-5}
\end{nd}
\]
\end{enumerate}

\subsubsection{\ref{axiom2:notseespreservedL}}
\begin{enumerate}[align=left]
\item[\lemmalab{NotSeesPreservedL}{axiom2:notseespreservedL}]
$
\boxed{
\begin{aligned}[t]
&
\lnot \sees{\aterm_1}{\aterm_2}{\asetmeetvar\cup\{\aterm_3\}} \land \lnot \sees{\aterm_1}{\aterm_3}{\asetmeetvar\cup\{\aterm_3\}}
\implies\\
&\lnot\sees{\aterm_1}{\aterm_2}{\asetmeetvar}
\end{aligned}}
$
\[
\begin{nd}
\hypo {1} {\lnot \sees{\aterm_1}{\aterm_2}{\asetmeetvar\cup\{\aterm_3\}}}
\hypo {2} {\lnot \sees{\aterm_1}{\aterm_3}{\asetmeetvar\cup\{\aterm_3\}}}
\open
\hypo {2b} {\sees{\aterm_1}{\aterm_3}{\asetmeetvar}}
\have {2c} {\sees{\aterm_1}{\aterm_3}{\asetmeetvar \cup \{\aterm_3\}}} \by{\ref{core2Ax:SeesRef}\ \text{and}\ \ref{core2Ax:SeesMono1}}{2b}
\have {2d} {\bottom} \by{\landcontr}{2,2c}
\close
\have {2e} {\lnot \sees{\aterm_1}{\aterm_3}{\asetmeetvar}} \ni{2b-2d}
\open
\hypo {3} {\sees{\aterm_1}{\aterm_2}{\asetmeetvar}}
\open
\hypo {4} {\sees{\aterm_1}{\aterm_2}{\{\aterm_3\}}}
\have {5} {\sees{\aterm_1}{\aterm_2}{\asetmeetvar\cup\{\aterm_3\}}} \by{\ref{core2Ax:SeesSum}}{3,4}
\have {6} {\bottom} \by{\landcontr}{1,5}
\close
\have {7} {\lnot\sees{\aterm_1}{\aterm_2}{\{\aterm_3\}}} \ni{4-6}
\have {8} {\sees{\aterm_1}{\aterm_3}{\asetmeetvar}} \by{\ref{core2Ax:SeesNegSum}}{3,7}
\have {9} {\bottom} \by{\landcontr}{2e,8}
\close
\have {10} {\lnot\sees{\aterm_1}{\aterm_2}{\asetmeetvar}} \ni{3-9}
\end{nd}
\]
\end{enumerate}

\subsubsection{\ref{axiom2:notseespreservedR}}
\begin{enumerate}[align=left]
\item[\lemmalab{NotSeesPreservedR}{axiom2:notseespreservedR}]
$
\boxed{
\begin{aligned}[t]
&
\lnot \sees{\aterm_1}{\aterm_2}{\asetmeetvar\cup\{\aterm_3\}} \land \lnot \sees{\aterm_3}{\aterm_2}{\asetmeetvar\cup\{\aterm_3\}}
\implies\\
&\lnot\sees{\aterm_1}{\aterm_2}{\asetmeetvar}
\end{aligned}}
$
\[
\begin{nd}
\hypo {1} {\lnot \sees{\aterm_1}{\aterm_2}{\asetmeetvar\cup\{\aterm_3\}}}
\hypo {2} {\lnot \sees{\aterm_3}{\aterm_2}{\asetmeetvar\cup\{\aterm_3\}}}
\open
\hypo {2b} {\sees{\aterm_3}{\aterm_2}{\asetmeetvar}}
\have {2c} {\sees{\aterm_3}{\aterm_2}{\asetmeetvar \cup \{\aterm_3\}}} \by{\ref{core2Ax:SeesRef}\ \text{and}\ \ref{core2Ax:SeesMono1}}{2b}
\have {2d} {\bottom} \by{\landcontr}{2,2c}
\close
\have {2e} {\lnot \sees{\aterm_3}{\aterm_2}{\asetmeetvar}} \ni{2b-2d}
\end{nd}
\]
\[
\begin{ndresume}
\open
\hypo {3} {\sees{\aterm_1}{\aterm_2}{\asetmeetvar}}
\open
\hypo {4} {\sees{\aterm_1}{\aterm_2}{\{\aterm_3\}}}
\have {5} {\sees{\aterm_1}{\aterm_2}{\asetmeetvar\cup\{\aterm_3\}}} \by{\ref{core2Ax:SeesSum}}{3,4}
\have {6} {\bottom} \by{\landcontr}{1,5}
\close
\have {7} {\lnot\sees{\aterm_1}{\aterm_2}{\{\aterm_3\}}} \ni{4-6}
\have {8} {\sees{\aterm_3}{\aterm_2}{\asetmeetvar}} \by{\ref{core2Ax:SeesNegSum}}{3,7}
\have {9} {\bottom} \by{\landcontr}{2e,8}
\close
\have {10} {\lnot\sees{\aterm_1}{\aterm_2}{\asetmeetvar}} \ni{3-9}
\end{ndresume}
\]
\end{enumerate}

\subsubsection{\ref{axiom2:seeslengthpreserved}}
\begin{enumerate}[align=left]
\item[\lemmalab{SeesLength}{axiom2:seeslengthpreserved}]
$
\boxed{\sees{\aterm_1}{\aterm_2}{\asetmeetvar\cup\{\aterm_3\}}{=}{\inbound} \implies \sees{\aterm_1}{\aterm_2}{\asetmeetvar}{=}{\inbound}}
$
\[
\begin{nd}
\hypo {1} {\seesgeq{\aterm_1}{\aterm_2}{\asetmeetvar\cup\{\aterm_3\}}{\inbound}}
\hypo {2} {\lnot \seesgeq{\aterm_1}{\aterm_2}{\asetmeetvar\cup\{\aterm_3\}}{\inbound{+}1}}
\have {3} {\seesgeq{\aterm_1}{\aterm_2}{\asetmeetvar}{\inbound}} \by{\ref{core2Ax:SeesMono1}}{1}
\open
\hypo {4} {\seesgeq{\aterm_1}{\aterm_2}{\asetmeetvar}{\inbound{+}1}}
\have {5} {\seesgeq{\aterm_1}{\aterm_2}{\asetmeetvar\cup\{\aterm_3\}}{\inbound{+}1}} \by{\ref{core2Ax:SeesMax}}{1,4}
\have {6} {\bottom} \by{\landcontr}{2,5}
\close
\have {7} {\lnot \seesgeq{\aterm_1}{\aterm_2}{\asetmeetvar}{\inbound{+}1}} \ni{4-6}
\have {8} {\sees{\aterm_1}{\aterm_2}{\asetmeetvar}{=}{\inbound}} \by{\ndref{3} $\land$ \ndref{7}}{}
\end{nd}
\]
\end{enumerate}

\subsubsection{\ref{axiom2:seeslengthsum}}
\begin{enumerate}[align=left]
\item[\lemmalab{SeesLengthSum}{axiom2:seeslengthsum}]
$
\boxed{
\begin{aligned}[t]
&(\sees{\aterm_1}{\aterm_2}{\asetmeetvar}{=}{\inbound_1} \land  \sees{\aterm_2}{\aterm_3}{\asetmeetvar}{=}{\inbound_2}\\
&\land \aterm_2 \not\in\asetmeetvar \land \aterm_3 \in \asetmeetvar) \implies\\
&\sees{\aterm_1}{\aterm_3}{\asetmeetvar}{=}{\inbound_1+\inbound_2} \land
\lnot \sees{\aterm_1}{\aterm_2}{\{\aterm_3\}}
\end{aligned}}
$
\[
\begin{nd}
\hypo {1} {\seesgeq{\aterm_1}{\aterm_2}{\asetmeetvar}{\inbound_1}}
\hypo {2} {\lnot \seesgeq{\aterm_1}{\aterm_2}{\asetmeetvar}{\inbound_1+1}}
\hypo {3} {\seesgeq{\aterm_2}{\aterm_3}{\asetmeetvar}{\inbound_2+1}}
\hypo {4} {\lnot \seesgeq{\aterm_2}{\aterm_3}{\asetmeetvar}{\inbound_2+1}}
\hypo {5} {\aterm_2 \not\in\asetmeetvar}
\hypo {6} {\aterm_3 \in \asetmeetvar}
\have {7} {\seesgeq{\aterm_1}{\aterm_3}{\asetmeetvar}{\inbound_1{+}\inbound_2}} \by{\ref{core2Ax:SeesSum}}{1,3,5,6}
\have {8} {\lnot \sees{\aterm_1}{\aterm_2}{\{\aterm_3\}}} \by{\ref{core2Ax:SeesSum}}{1,3,5,6}
\open
\hypo {9} {\seesgeq{\aterm_1}{\aterm_3}{\asetmeetvar}{\inbound_1{+}\inbound_2{+}1}}
\have {10} {{\bigvee_{\mathrlap{
  \raisebox{-0.2cm}[0pt][0pt]{$\kern-1em\scriptstyle{\inbound_3+\inbound_4=\inbound_1{+}\inbound_2{-}1}$}}}
}
(\seesgeq{\aterm_1}{\aterm_2}{\asetmeetvar}{\inbound_3{+}1} \land\\ \seesgeq{\aterm_2}{\aterm_3}{\asetmeetvar}{\inbound_4{+}1})}
\by{\ref{core2Ax:SeesNegSum}}{9}
\end{nd}
\]
\[
\begin{ndresume}
\open
\hypo {11} {\seesgeq{\aterm_1}{\aterm_2}{\asetmeetvar}{\inbound_3{+}1}} \by{for $\inbound_3,\inbound_4$ s.t.}{}
\hypo {12} {\seesgeq{\aterm_2}{\aterm_3}{\asetmeetvar}{\inbound_4{+}1}} \by{ $\inbound_3{+}\inbound_4=\inbound_1{+}\inbound_2{-}1$}{}
\have {15} {\bottom, \text{ as }(\inbound_3{+}1\leq\inbound_1\ \text{iff}\ \inbound_4{+}1>\inbound_2)} \by{and \landcontr
}{2,4,11,12}
\close
\have {16} {\bottom} \oe{10,11-15}
\close
\have {17} {\lnot\seesgeq{\aterm_1}{\aterm_3}{\asetmeetvar}{\inbound_1{+}\inbound_2{+}1}} \ni{9-16}
\have {18} {\sees{\aterm_1}{\aterm_3}{\asetmeetvar}{=}{\inbound_1+\inbound_2} \land\\
\lnot \sees{\aterm_1}{\aterm_2}{\{\aterm_3\}}} \by{\ndref{7} $\land$ \ndref{8} $\land$ \ndref{17}}{}
\end{ndresume}
\]
\end{enumerate}

\subsubsection{\ref{axiom2:beforesees}}
\begin{enumerate}[align=left]
\item[\lemmalab{BeforeSees}{axiom2:beforesees}]
$
\boxed{
\begin{aligned}[t]
&\before{\aterm_1}{\aterm_2} \land \before{\aterm_2}{\aterm_3} \implies\\
&\sees{\aterm_1}{\aterm_3}{\emptyset} \land \lnot \sees{\aterm_1}{\aterm_3}{\{\aterm_2\}}
\end{aligned}}
$
\[
\begin{nd}
\hypo {1} {\before{\aterm_1}{\aterm_2}}
\hypo {2} {\before{\aterm_2}{\aterm_3}}
\have {3} {\before{\aterm_1}{\aterm_3}} \by{\ref{axiom2:beforelemma3}}{1,2}
\have {4} {\sees{\aterm_1}{\aterm_3}{\emptyset}} \by{\ref{core2Ax:SeesBefore}}{3}
\have {5} {\aterm_2 \neq \aterm_3} \ae{2}
\have {6} {\sees{\aterm_2}{\aterm_3}{\emptyset}} \by{\ref{core2Ax:SeesBefore}}{2}
\open
\hypo {7} {\lnot \sees{\aterm_1}{\aterm_2}{\{\aterm_3\}}}
\have {8} {\lnot \sees{\aterm_2}{\aterm_3}{\emptyset}} \by{\ref{core2Ax:SeesElsewhere}}{1,7}
\have {9} {\bottom} \by{\landcontr}{6,8}
\close
\have {10} {\sees{\aterm_1}{\aterm_2}{\{\aterm_3\}}} \ni{7-9}
\have {11} {\sees{\aterm_2}{\aterm_3}{\{\aterm_2,\aterm_3\}}} \by{\ref{core2Ax:SeesRef}}{6}
\have {12} {\sees{\aterm_2}{\aterm_3}{\{\aterm_3\}}} \by{\ref{core2Ax:SeesMono1}}{11}
\have {13} {\lnot\sees{\aterm_1}{\aterm_3}{\{\aterm_2\}}} \by{\ref{core2Ax:SeesSum}}{10,12}
\have {14} {\sees{\aterm_1}{\aterm_3}{\emptyset} \land \lnot \sees{\aterm_1}{\aterm_3}{\{\aterm_2\}}} \by{\ndref{4} $\land$ \ndref{13}}{}
\end{nd}
\]
\end{enumerate}

\subsubsection{\ref{axiom2:seessameloop}}

\begin{enumerate}[align=left]
\item[\lemmalab{SeesSameloop}{axiom2:seessameloop}]
$
\boxed{
\begin{aligned}[t]
&(\asymmetric{\ameetvar{\avariable}{\avariablebis}{\avariableter}} \land
{\sees{\ameetvar{\avariable}{\avariablebis}{\avariableter}}{\ameetvar{\avariablefour}{\avariablefifth}{\avariablesix}}{\asetmeetvar}}
\land\\
&
{\ameetvar{\avariable}{\avariablebis}{\avariableter} \neq \ameetvar{\avariablefour}{\avariablefifth}{\avariablesix}})
\implies\\
&{\sameloop{\ameetvar{\avariable}{\avariablebis}{\avariableter}}{\ameetvar{\avariablefour}{\avariablefifth}{\avariablesix}}}
\end{aligned}
}
$
\[
\begin{nd}
\hypo {6b} {\asymmetric{\ameetvar{\avariable}{\avariablebis}{\avariableter}}}
\hypo {2} {\sees{\ameetvar{\avariable}{\avariablebis}{\avariableter}}{\ameetvar{\avariablefour}{\avariablefifth}{\avariablesix}}{\asetmeetvar}}
\hypo {3} {\ameetvar{\avariable}{\avariablebis}{\avariableter} \neq \ameetvar{\avariablefour}{\avariablefifth}{\avariablesix}}
\have {4} {\defined{\ameetvar{\avariable}{\avariablebis}{\avariablesix}}} \by{\ref{core2Ax:SeesSubscript}}{2}
\have {5} {\defined{\ameetvar{\avariablefour}{\avariablefifth}{\avariablesix}}} \by{\ref{core2Ax:SeesDef}}{2}
\have {6} {\defined{\ameetvar{\avariable}{\avariablefour}{\avariablesix}}} \by{\ref{core2Ax:PedDefines}}{4,5}
\open
\hypo {8} {\symmetric{\ameetvar{\avariable}{\avariablefour}{\avariablesix}}}
\have {9} {\before{\ameetvar{\avariable}{\avariablebis}{\avariableter}}{\ameetvar{\avariablefour}{\avariablefifth}{\avariablesix}}} \by{\ref{core2Ax:SeesElsewhere}}{2,3,8}
\end{nd}
\]
\[
\begin{ndresume}
\have {10} {\symmetric{\ameetvar{\avariable}{\avariablebis}{\avariableter}}} \ae{9}
\have {11} {\bottom} \by{\landcontr}{6b,10}
\close
\have {13} {\lnot \symmetric{\ameetvar{\avariable}{\avariablefour}{\avariablesix}}} \ni{8-11}
\have {14} {\asymmetric{\ameetvar{\avariable}{\avariablefour}{\avariablesix}}} \by{ \ndref{6} $\land$ \ndref{13}}{}
\have {15} {\ameetvar{\avariablefour}{\avariablefifth}{\avariablesix} = \ameetvar{\avariablefour}{\avariable}{\avariablesix}} \by{\ref{core2Ax:SeesToLoop}}{2,14}
\have {16} {\ameetvar{\avariable}{\avariablebis}{\avariableter} = \ameetvar{\avariable}{\avariablefour}{\avariablesix}} \by{\ref{core2Ax:BothAsym}}{6b,14}
\have {17} {\sameloop{\ameetvar{\avariable}{\avariablefour}{\avariablesix}}{\ameetvar{\avariablefour}{\avariable}{\avariablesix}}} \by{\ref{axiom2:samelooplemma0two}}{14}
\have {18} {\sameloop{\ameetvar{\avariable}{\avariablebis}{\avariableter}}{\ameetvar{\avariablefour}{\avariable}{\avariablesix}}} \by{\ref{axiom2:sameloopsubl}}{16,17}
\have {19} {\sameloop{\ameetvar{\avariable}{\avariablebis}{\avariableter}}{\ameetvar{\avariablefour}{\avariablefifth}{\avariablesix}}} \by{\ref{axiom2:sameloopsubl}}{15,18}
\end{ndresume}
\]
\end{enumerate}

\subsubsection{\ref{axiom2:outsideloopsees}}
\begin{enumerate}[align=left]
\item[\lemmalab{OutsideLoopSees}{axiom2:outsideloopsees}]
$
\boxed{
\begin{aligned}[t]
&
\sameloop{\aterm_1}{\aterm_2} \land \lnot \sameloop{\aterm_1}{\aterm_3} \implies\\
&\sees{\aterm_1}{\aterm_2}{\{\aterm_3\}}
\end{aligned}}
$\\
we show the equivalent formula (and w.l.o.g., using meet-points) $\sameloop{\ameetvar{\avariable}{\avariablebis}{\avariableter}}{\ameetvar{\avariablefour}{\avariablefifth}{\avariablesix}} \land
\lnot \sees{\ameetvar{\avariable}{\avariablebis}{\avariableter}}{\ameetvar{\avariablefour}{\avariablefifth}{\avariablesix}}{\{\ameetvar{\avariablesept}{\avariableoct}{\avariablenine}\}}
{\implies}$\\
$\sameloop{\ameetvar{\avariable}{\avariablebis}{\avariableter}}{\ameetvar{\avariablesept}{\avariableoct}{\avariablenine}}$
\[
\begin{nd}
\hypo {1} {\sameloop{\ameetvar{\avariable}{\avariablebis}{\avariableter}}{\ameetvar{\avariablefour}{\avariablefifth}{\avariablesix}}}
\hypo {2} {\lnot \sees{\ameetvar{\avariable}{\avariablebis}{\avariableter}}{\ameetvar{\avariablefour}{\avariablefifth}{\avariablesix}}{\{\ameetvar{\avariablesept}{\avariableoct}{\avariablenine}\}}}
\have {3} {\asymmetric{\ameetvar{\avariable}{\avariablefour}{\avariableter}}} \ae{1}
%\have {4} {\ameetvar{\avariable}{\avariablebis}{\avariableter} = \ameetvar{\avariable}{\avariablefour}{\avaraibleter}} \ae{1}
\have {5} {\sees{\ameetvar{\avariable}{\avariablebis}{\avariableter}}{\ameetvar{\avariable}{\avariablebis}{\avariableter}}{\emptyset}} \by{\ref{core2Ax:SeesEWCycl}}{1}
\have {6} {\lnot \sees{\ameetvar{\avariable}{\avariablebis}{\avariableter}}{\ameetvar{\avariable}{\avariablebis}{\avariableter}}{\{\ameetvar{\avariablefour}{\avariablefifth}{\avariablesix}\}}} \by{\ref{core2Ax:SeesEWCycl}}{1}
\have {7} {\sees{\ameetvar{\avariable}{\avariablebis}{\avariableter}}{\ameetvar{\avariablefour}{\avariablefifth}{\avariablesix}}{\emptyset}} \by{\ref{core2Ax:SeesNegSum}}{5,6}
\have {8} {\sees{\ameetvar{\avariable}{\avariablebis}{\avariableter}}{\ameetvar{\avariablesept}{\avariableoct}{\avariablenine}}{\emptyset}} \by{\ref{core2Ax:SeesNegSum}}{2,7}
\open
\hypo {9} {\ameetvar{\avariable}{\avariablebis}{\avariableter} = {\ameetvar{\avariablesept}{\avariableoct}{\avariablenine}}}
\have {10} { \sees{\ameetvar{\avariable}{\avariablebis}{\avariableter}}{\ameetvar{\avariablefour}{\avariablefifth}{\avariablesix}}{\{\ameetvar{\avariablesept}{\avariableoct}{\avariablenine}\}}} \by{\ref{core2Ax:SeesTermEq}}{7,9}
\have {11} {\bottom} \by{\landcontr}{2,10}
\close
\have {12} {\ameetvar{\avariable}{\avariablebis}{\avariableter} \neq {\ameetvar{\avariablesept}{\avariableoct}{\avariablenine}}} \ni{9-11}
\have {13} {\sameloop{\ameetvar{\avariable}{\avariablebis}{\avariableter}}{\ameetvar{\avariablesept}{\avariableoct}{\avariablenine}}} \by{\ref{axiom2:seessameloop}}{3,8,12}
\end{nd}
\]
\end{enumerate}

\subsubsection{\ref{axiom2:beforesameloopsees}}
\begin{enumerate}[align=left]
\item[\lemmalab{$(<,\circlearrowleft)$-Sees}{axiom2:beforesameloopsees}]
$
\boxed{
\begin{aligned}[t]
&\before{\aterm_1}{\aterm_2} \land \sameloop{\aterm_2}{\aterm_3} \implies\\
&\sees{\aterm_1}{\aterm_3}{\emptyset} \land \lnot \sees{\aterm_1}{\aterm_3}{\{\aterm_2\}}
\end{aligned}}
$
\[
\begin{nd}
\hypo {1} {\before{\aterm_1}{\aterm_2}}
\hypo {2} {\sameloop{\aterm_2}{\aterm_3}}
\have {3} {\sees{\aterm_2}{\aterm_2}{\emptyset} \land \lnot \sees{\aterm_2}{\aterm_2}{\{\aterm_3\}}} \by{\ref{core2Ax:SeesEWCycl}}{2}
\have {4} {\sees{\aterm_2}{\aterm_3}{\emptyset}} \by{\ref{core2Ax:SeesNegSum}}{3}
\open
\hypo {5} {\lnot \sees{\aterm_1}{\aterm_2}{\{\aterm_3\}}}
\have {6} {\lnot \sees{\aterm_2}{\aterm_3}{\emptyset}} \by{\ref{core2Ax:SeesElsewhere}}{1,5}
\have {7} {\bottom} \by{\landcontr}{4,6}
\close
\end{nd}
\]
\[
\begin{ndresume}
\have {8} {\sees{\aterm_1}{\aterm_2}{\{\aterm_3\}}} \ni{5-7}
\have {11} {\sees{\aterm_2}{\aterm_3}{\{\aterm_2,\aterm_3\}}} \by{\ref{core2Ax:SeesRef}}{4}
\have {12} {\sees{\aterm_2}{\aterm_3}{\{\aterm_3\}}} \by{\ref{core2Ax:SeesMono1}}{11}
\have {13} {\lnot\sees{\aterm_1}{\aterm_3}{\{\aterm_2\}}} \by{\ref{core2Ax:SeesSum}}{8,12}
\have {14} {\seesgeq{\aterm_1}{\aterm_3}{\{\aterm_3\}}{2}} \by{\ref{core2Ax:SeesSum}}{8,12}
\have {15} {\sees{\aterm_1}{\aterm_3}{\emptyset}} \by{\ref{core2Ax:SeesMono1} and \ref{core2Ax:SeesMono2}}{14}
\have {16} {\sees{\aterm_1}{\aterm_3}{\emptyset} \land \lnot \sees{\aterm_1}{\aterm_3}{\{\aterm_2\}}} \by{\ndref{13} $\land$ \ndref{15}}{}
\end{ndresume}
\]
\end{enumerate}

\subsubsection{\ref{axiom2:meetneqsees}}
\begin{enumerate}[align=left]
\item[\lemmalab{MeetNeq{$\implies\!$}Sees}{axiom2:meetneqsees}]
$
\boxed{
\begin{aligned}[t]
&\defined{\ameetvar{\avariable}{\avariablebis}{\avariableter}} \land \avariable \neq \ameetvar{\avariable}{\avariablebis}{\avariableter} \land \avariableter \neq \ameetvar{\avariable}{\avariablebis}{\avariableter}
\implies\\
&\sees{\avariable}{\avariableter}{\emptyset} \land \lnot \sees{\avariable}{\avariableter}{\{\ameetvar{\avariable}{\avariablebis}{\avariableter}\}}
\end{aligned}
}
$
\[
\begin{nd}
\hypo {1} {\defined{\ameetvar{\avariable}{\avariablebis}{\avariableter}}}
\hypo {2} {\avariable \neq \ameetvar{\avariable}{\avariablebis}{\avariableter}}
\hypo {3} {\avariableter \neq \ameetvar{\avariable}{\avariablebis}{\avariableter}}
\have {4} {\avariable = \ameetvar{\avariable}{\avariablebis}{\avariableter} \lor\\ \before{\avariable}{\ameetvar{\avariable}{\avariablebis}{\avariableter}}}
\by{\ref{axiom2:auxlemma3}}{1}
\have {5} {\before{\avariable}{\ameetvar{\avariable}{\avariablebis}{\avariableter}}}
\by{\modusponens}{2,4}
\have {6} {\sees{\avariable}{\ameetvar{\avariable}{\avariablebis}{\avariableter}}{\emptyset}} \by{\ref{core2Ax:SeesBefore}}{5}
\have {7} {\before{\ameetvar{\avariable}{\avariablebis}{\avariableter}}{\avariableter} \lor\\ \sameloop{\ameetvar{\avariable}{\avariableter}{\avariableter}}{\avariableter}} \by{\ref{axiom2:subscriptforward}}{1,3}
\open
\hypo {8} {\before{\ameetvar{\avariable}{\avariablebis}{\avariableter}}{\avariableter}}
\have {9} {\sees{\avariable}{\avariableter}{\emptyset} \land\\ \lnot \sees{\avariable}{\avariableter}{\{\ameetvar{\avariable}{\avariablebis}{\avariableter}\}}} \by{\ref{axiom2:beforesees}}{5,8}
\close
\open
\hypo {10} {\sameloop{\ameetvar{\avariable}{\avariableter}{\avariableter}}{\avariableter}}
\have {11a} {\asymmetric{\ameetvar{\avariable}{\avariableter}{\avariableter}}} \ae{10}
\have {10b} {\ameetvar{\avariable}{\avariablebis}{\avariableter} = \ameetvar{\avariable}{\avariableter}{\avariableter} \lor\\ \ameetvar{\avariable}{\avariablebis}{\avariableter} \neq \ameetvar{\avariable}{\avariableter}{\avariableter}} \by{\trivialtrue}{}
\open
\hypo {11} {\ameetvar{\avariable}{\avariablebis}{\avariableter} = \ameetvar{\avariable}{\avariableter}{\avariableter}}
\have {12} {\sameloop{\ameetvar{\avariable}{\avariablebis}{\avariableter}}{\avariableter}} \by{\ref{axiom2:sameloopsubl}}{11}
\have {13} {\sees{\avariable}{\avariableter}{\emptyset} \land\\ \lnot \sees{\avariable}{\avariableter}{\{\ameetvar{\avariable}{\avariablebis}{\avariableter}\}}} \by{\ref{axiom2:beforesameloopsees}}{5,12}
\close
\open
\hypo {14} {\ameetvar{\avariable}{\avariablebis}{\avariableter} \neq \ameetvar{\avariable}{\avariableter}{\avariableter}}
\have {15} {\before{\ameetvar{\avariable}{\avariablebis}{\avariableter}}{\ameetvar{\avariable}{\avariableter}{\avariableter}}} \by{\ref{axiom2:auxlemma7}}{1,11a,14}
\have {17} {\lnot \sees{\avariable}{\ameetvar{\avariable}{\avariableter}{\avariableter}}{\{\ameetvar{\avariable}{\avariablebis}{\avariableter}
\}}} \by{\ref{axiom2:beforesees}}{5,15}
\have {18} {\before{\avariable}{\ameetvar{\avariable}{\avariableter}{\avariableter}}} \by{\ref{axiom2:beforelemma3}}{5,15}
\have {19} {\sees{\avariable}{\avariableter}{\emptyset}} \by{\ref{axiom2:beforesameloopsees}}{10,18}
\end{nd}
\]
\[
\begin{ndresume}
\have {20} {\lnot \sees{\avariable}{\avariableter}{\{\ameetvar{\avariable}{\avariableter}{\avariableter}\}}} \by{\ref{axiom2:beforesameloopsees}}{10,18}
\open
\hypo {21} {\sees{\avariable}{\avariableter}{\{\ameetvar{\avariable}{\avariablebis}{\avariableter}\}}}
\have {22} {\sees{\avariable}{\ameetvar{\avariable}{\avariableter}{\avariableter}}{\{\ameetvar{\avariable}{\avariablebis}{\avariableter}\}}} \by{\ref{core2Ax:SeesNegSum}}{20,21}
\have {23} {\bottom} \by{\landcontr}{17,22}
\close
\have {24} {\lnot\sees{\avariable}{\avariableter}{\{\ameetvar{\avariable}{\avariablebis}{\avariableter}\}}} \ni{21-23}
\have {25} {\sees{\avariable}{\avariableter}{\emptyset} \land\\ \lnot \sees{\avariable}{\avariableter}{\{\ameetvar{\avariable}{\avariablebis}{\avariableter}\}}} \by{\ndref{19} $\land$ \ndref{24}}{}
\end{ndresume}
\]
\end{enumerate}
