# Supplementary material for: A Complete Axiomatisation for Quantifier-Free Separation Logic
Source: arXiv:2006.05156 source file (2021-08-09)
Supplement: Supplementary file 5 [file definition-symbolic-composition.tex]

In this section we provide useful information on the symbolic composition $\asymbunion$ evoked in Section~\ref{section:axiom2starelim}.
\ifLongVersionWithAppendix
We refer the reader to this section for the definitions (central in this appendix) of symbolic memory state, abstraction
of a memory state and characteristic formula.
\fi
We denote with $\pi_i$ the projection map, so that
given a symbolic memory state $\triple{\symbterms}{\amap}{\symbrem}$ over $\pair{\asetvar}{\bound}$, the function
$\pi_1 \circ \amap$ goes from $\symbterms$ to $\symbterms$, whereas $\pi_2 \circ \amap$ goes from $\symbterms$ to  $\interval{1}{\bound}$
($\pi_i$ is the projection on the $i$th component).

We want to characterise the relation $\asymbunion \subseteq \sum_{\asetvar,\bound_1,\bound_2}
\symbdomain{\asetvar}{\bound_1}\times\symbdomain{\asetvar}{\bound_2}\times\symbdomain{\asetvar}{\bound_1+\bound_2}$, on symbolic memory states having satisfiable characteristic formulae, such that
\begin{description}
\item[\lemmalab{(+$_{\mathsf{sms}}$-adequacy)}{compositionproperty}] For all $\pair{\astore}{\aheap}$ and all
$\asms_1$ and $\asms_2$,
respectively over $\pair{\asetvar}{\bound_1}$ and $\pair{\asetvar}{\bound_2}$,
$\triple{\asms_1}{\asms_2}{\symbms{\astore}{\aheap}{\asetvar}{\bound_1+\bound_2}} \in \asymbunion$
iff
$\aheap_1 + \aheap_2 = \aheap$,
$\asms_1 = \symbms{\astore}{\aheap_1}{\asetvar}{\bound_1}$ and
$\asms_2 = \symbms{\astore}{\aheap_2}{\asetvar}{\bound_2}$ for some $\aheap_1$ and $\aheap_2$.
\end{description}
We write $\symbunion{\triple{\symbterms_1}{\amap_1}{\symbrem_1}}{\triple{\symbterms_2}{\amap_2}{\symbrem_2}}{\triple{\symbterms}{\amap}{\symbrem}}$ for
$\triple{\triple{\symbterms_1}{\amap_1}{\symbrem_1}}{\triple{\symbterms_2}{\amap_2}{\symbrem_2}}{\triple{\symbterms}{\amap}{\symbrem}} \in \asymbunion$.
By Lemma~\ref{lemma:msmodelsabs}, if $\asymbunion$ satisfies \ref{compositionproperty}, then it correctly behaves with respect to separating conjunction $\separate$, as follows:
\begin{nscenter}
$\symbunion{\triple{\symbterms_1}{\amap_1}{\symbrem_1}}{\triple{\symbterms_2}{\amap_2}{\symbrem_2}}{\triple{\symbterms}{\amap}{\symbrem}}\quad
\text{iff}\quad
\models \charsymbform{\triple{\symbterms}{\amap}{\symbrem}} \implies \charsymbform{\triple{\symbterms_1}{\amap_1}{\symbrem_1}} \separate \charsymbform{\triple{\symbterms_2}{\amap_2}{\symbrem_2}}$
\end{nscenter}
As shown in Section~\ref{section:axiom2starelim}, $\asymbunion$ cannot be functional in its first two components.
Moreover, in Section~\ref{section:axiom2starelim} we described the membership problem $\triple{\triple{\symbterms}{\amap_1}{\symbrem_1}}{\triple{\symbterms}{\amap_2}{\symbrem_2}}{\triple{\symbterms}{\amap}{\symbrem}} \in \asymbunion$ to be roughly equivalent to the problem of finding
two graph homomorphisms from the graphs $\pair{\symbterms_1}{\amap_1}$ and $\pair{\symbterms_2}{\amap_2}$ to $\pair{\symbterms}{\amap}$,
together with the existence of a partition that guarantees that paths that do not belong to the homomorphisms can be generated using the
%% additional
memory cells from the garbage (abstracted by $\symbrem_1$ and $\symbrem_2$) -- see the details below.
Now, we  define this problem and we give an informal explanation to its components.
\cut{
Notice that $\asymbunion$ cannot be functional on its first two components.
Take for example the symbolic memory state $\asms = (\{\avariable,\ameetvar{\avariable}{\avariable}{\avariable}\},\emptyset,1)$ and let us
ask ourselves for which symbolic memory states $\asms$,  it should hold that $\symbunion{\asms}{\asms}{\asms'}$
There are (at least) two possibilities.
\begin{enumerate}
\item As $\asms$ is the abstraction of the memory states $(\astore,\{\alocation_1\pto\alocation_2\})$ and $(\astore,\{\alocation_2\pto\alocation_1)\})$ where $\astore(\avariable) = \alocation_1 \neq \alocation_2$,
the abstraction of $(\astore,\{\alocation_1\pto\alocation_2,\alocation_2\pto\alocation_1\})$ must be a solution for $\asms'$.
More precisely, this abstraction is
$(\asymbterm,\{\asymbterm \pto (\asymbterm,2) \},0)$ where $\asymbterm = \{\avariable,\ameetvar{\avariable}{\avariable}{\avariable}\}$.
\item However, $\asms$ is  also the abstraction of $(\astore,\{\alocation_1\pto\alocation_2\})$ and $(\astore,\{\alocation_3\pto\alocation_4)\})$ such that $\astore(\avariable) \not\in \{\alocation_1,\alocation_3\}$.
Then, the abstraction $\triple{\{\avariable,\ameetvar{\avariable}{\avariable}{\avariable}\}}{\emptyset}{2}$ must also be a solution for $\asms'$.
\end{enumerate}
From the above example, it is clear what is the main challenge in defining
This possibility was depicted in the first case above.
}

Let $\asms_1 = {\triple{\symbterms_1}{\amap_1}{\symbrem_1}}$, $\asms_2 = {\triple{\symbterms_2}{\amap_2}{\symbrem_2}}$ and $\asms = {\triple{\symbterms}{\amap}{\symbrem}}$ be three symbolic memory states
respectively over $\pair{\asetvar}{\bound_1}$, $\pair{\asetvar}{\bound_2}$ and
$\pair{\asetvar}{\bound_1+\bound_2}$
% The characterisation of $\asymbunion$ that we are tring to achieve is reminiscent of the computation of graph homomorphisms, as paths between program variables in the heaps $\aheap_1$ and $\aheap_2$ are preserved in their composition, with additional conditions that model how paths can be introduced.
We have $\symbunion{\asms_1}{\asms_2}{\asms}$ $\equivdef$ \\

{
\small
\noindent $\charsymbform(\asms_1)$, $\charsymbform(\asms_2)$ and $\charsymbform(\asms)$ are satisfiable
and
there are injections $\ainj_1:\symbterms_1 \to \symbterms$ and $\ainj_2:\symbterms_2 \to \symbterms$
satisfying the following 4 conditions:

\begin{enumerate}
\item[\lemmalab{1}{C-functionality}.] for each $\asymbterm \in \domain{\amap}$ then it cannot be that
$\ainj_1^{-1}(\asymbterm) \in \domain{\amap_1}$ and $\ainj_2^{-1}(\asymbterm) \in \domain{\amap_2}$;
\end{enumerate}

\begin{enumerate}
\item[\lemmalab{2}{C-meet-points}.] for all $i \in \{1,2\}$, for each $\asymbterm \in \symbterms_i$,
  \begin{enumerate}[nosep]
  \item for each $\avariable \in \asetvar$, \ $\avariable \in \asymbterm \iff \avariable \in \ainj_i(\asymbterm)$;
  \item for each meet-point term $\ameetvar{\avariable}{\avariablebis}{\avariableter} \in \asymbterm$,
  if $\ameetvar{\avariablebis}{\avariable}{\avariableter} \not\in \asymbterm$ then
  $\ameetvar{\avariable}{\avariablebis}{\avariableter} \in \ainj_i(\asymbterm)$, otherwise
  $\ameetvar{\avariable}{\avariablebis}{\avariableter} \in \ainj_i(\asymbterm)$ or $\ameetvar{\avariablebis}{\avariable}{\avariableter} \in \ainj_i(\asymbterm)$.
  \end{enumerate}
\end{enumerate}

\begin{enumerate}
\item[\lemmalab{3}{C-homomorphism}.] for all $i \in \{1,2\}$, for all $\aterm_1,\aterm_2 \in \atermset{\asetvar}$ and all $\inbound \in \interval{1}{\bound_i}$, if $\amap_i(\equivclass{\aterm_1}{\symbterms_i}) = (\equivclass{\aterm_2}{\symbterms_i},\inbound)$ then
there is $n \in \Nat$ and a set $\{\asymbterm_0,\dots,\asymbterm_{n+1}\} \subseteq \symbterms$ such that
\begin{enumerate}[nosep]
\item $\asymbterm_0 {=} \ainj_i(\equivclass{\aterm_1}{\symbterms_i})$ and $\asymbterm_{n+1} {=} \ainj_i(\equivclass{\aterm_2}{\symbterms_i})$;
\item for each $j \in \interval{1}{n}$, $\asymbterm_j \not\in\range{\ainj_1} \cup \range{\ainj_2}$;
\item for each $j \in \interval{0}{n}$, $(\pi_1 \circ \amap)(\asymbterm_j) = \asymbterm_{j+1}$;
\item if $\inbound < \bound_i$ then $\sum_{j\in\interval{0}{n}} (\pi_2 \circ \amap)(\asymbterm_j) = \inbound$,
else $\sum_{j\in\interval{0}{n}} (\pi_2 \circ \amap)(\asymbterm_j) \geq \bound_i$.
\end{enumerate}
\end{enumerate}

\noindent Let $\symbsources{\asms_1}{\asms_2}{\asms}$, $\symbtargets{\asms_i}{\asms}$ ($i \in \{1,2\}$) and
$\symbinternal{\asms_1}{\asms_2}{\asms}$ be the sets defined below
\begin{itemize}[nosep]
\item $\symbsources{\asms_1}{\asms_2}{\asms}$ $\egdef$
$\{ \asymbterm \in \symbterms \mid$ $\asymbterm {\cap} \asetvar \neq \emptyset$ \& for every $\avariable \in \asymbterm {\cap} \asetvar$ and $i {\in} \{1,2\}$,
$\equivclass{\avariable}{\symbterms_i} {\not \in} \domain{\amap_i}\}$.
\item $\symbtargets{\asms_i}{\asms}$ is the set of $\asymbterm \in \symbterms$\ such that $\asymbterm \cap \asetvar \neq \emptyset$ or there are
$\aterm_1,\aterm_2 \in \atermset{\asetvar}$, $\alength_1,\alength_2 \geq 0$ such that
\begin{itemize}[nosep]
\item $(\pi_1\circ\amap_i)(\equivclass{\aterm_1}{\symbterms_i}) = \equivclass{\aterm_2}{\symbterms_i}$;
\item $(\pi_1 \circ \amap)^{\alength_1}(\ainj_i(\equivclass{\aterm_1}{\symbterms_i})) = \asymbterm$ and
$(\pi_1 \circ \amap)^{\alength_2}(\asymbterm) = \ainj_i(\equivclass{\aterm_2}{\symbterms_i})$;
\item for every $\alength < \alength_1+\alength_2$, $(\pi_2 \circ \amap)^{\alength}(\equivclass{\aterm_1}{\symbterms_i}) \neq \ainj_i(\equivclass{\aterm_2}{\symbterms_i})$.
\end{itemize}
\item
$\symbinternal{\asms_1}{\asms_2}{\asms} \egdef \domain{\amap} \setminus
((\cup_{i\in\{1,2\}}\symbtargets{\asms}{\asms_i}) \setminus \symbsources{\asms_1}{\asms_2}{\asms})$.
\end{itemize}

\cut{
\begin{enumerate}
\item[\lemmalab{4}{C-stillgarbage}.] If $\symbrem_1 < \bound_1$ and $\symbrem_2 < \bound_2$ then
$R \egdef \symbrem +
\sum_{\asymbterm \in \symbinternal{\asms_1}{\asms_2}{\asms}} (\pi_2 \circ \amap)(\asymbterm)$ equals $\symbrem_1 + \symbrem_2$,
else $R \geq \symbrem_1 + \symbrem_2$.
\end{enumerate}
}

\begin{enumerate}
\item[\lemmalab{4}{C-wasgarbage}.]
there are two functions $\amapbis_1,\amapbis_2: \symbinternal{\asms_1}{\asms_2}{\asms} \to \interval{1}{\bound_1+\bound_2}$ and $\symbrem_1',\symbrem_2' \in \Nat$ such that
\begin{enumerate}
\item $\symbrem = \symbrem_1' + \symbrem_2'$ and for every $\asymbterm \in \symbinternal{\asms_1}{\asms_2}{\asms}$, $(\pi_2 \circ \amap)(\asymbterm) = \amapbis_1(\asymbterm) + \amapbis_2(\asymbterm)$;
\item for all $i \in \{1,2\}$,
 $\min(\symbrem_i' + \sum_{\asymbterm \in \symbinternal{\asms_1}{\asms_2}{\asms}} \amapbis_i(\asymbterm), \bound_i) = \min(\symbrem_i, \bound_i)$;
\item for every $\asymbterm \in \symbsources{\asms_1}{\asms_2}{\asms} \cap \domain{\amap}$ there is
$\{\asymbterm_0 {=} \asymbterm, \asymbterm_1,\dots,\asymbterm_n\} \subseteq \symbinternal{\asms_1}{\asms_2}{\asms}$ such that
\begin{itemize}
\item for every
$j \in \interval{0}{n-1}$, $(\pi_1 \circ \amap)(\asymbterm_j) = \asymbterm_{j+1}$;
\item $(\pi_1 \circ \amap)(\asymbterm_n) \in \bigcup_{i \in \{1,2\}} \symbtargets{\asms_i}{\asms}$;
\item given $i \in \{1,2\}$, if $(\pi_1 \circ \amap)(\asymbterm_n) \in \symbtargets{\asms_i}{\asms}$ then
$\sum_{j \in \interval{0}{n}} \amapbis_{(3-i)}(\asymbterm_j) \geq 1$ .
\end{itemize}
\end{enumerate}
\end{enumerate}
\cut{
\begin{enumerate}

\item[\lemmalab{5}{C-wasgarbage}.]
there are two functions $\amapbis_1,\amapbis_2: \symbinternal{\asms_1}{\asms_2}{\asms} \to \interval{1}{\bound_1+\bound_2}$ such that
\begin{enumerate}
\item for all $i \in \{1,2\}$, the sum $\sum_{\asymbterm \in \symbinternal{\asms_1}{\asms_2}{\asms}} \amapbis_i(\asymbterm)$ is at most $\symbrem_i$ whenever $\symbrem_i < \bound_i$;
\item for every $\asymbterm \in \symbinternal{\asms_1}{\asms_2}{\asms}$, $(\pi_2 \circ \amap)(\asymbterm) = \amapbis_1(\asymbterm) + \amapbis_2(\asymbterm)$;
\item for every $\asymbterm \in \symbsources{\asms_1}{\asms_2}{\asms} \cap \domain{\amap}$ there is
$\{\asymbterm_0 {=} \asymbterm, \asymbterm_1,\dots,\asymbterm_n\} \subseteq \symbinternal{\asms_1}{\asms_2}{\asms}$ such that
\begin{itemize}
\item for every
$j \in \interval{0}{n-1}$, $(\pi_1 \circ \amap)(\asymbterm_j) = \asymbterm_{j+1}$;
\item $(\pi_1 \circ \amap)(\asymbterm_n) \in \bigcup_{i \in \{1,2\}} \symbtargets{\asms_i}{\asms}$;
\item given $i \in \{1,2\}$, if $(\pi_1 \circ \amap)(\asymbterm_n) \in \symbtargets{\asms_i}{\asms}$ then
$\sum_{j \in \interval{0}{n}} \amapbis_{(3-i)}(\asymbterm_j) \geq 1$ .
\end{itemize}
\end{enumerate}
\end{enumerate}
}
}

\noindent Let us dissect this involved definition.
First of, notice that we only consider symbolic memory states that correspond to concrete ones. This follows directly from the fact that we require $\charsymbform(\asms_1)$, $\charsymbform(\asms_2)$ and $\charsymbform(\asms)$ to be satisfiable (first line in the definition).
The main objects in this definition are the two injections $\ainj_1$ and $\ainj_2$.
Given $i \in \{1,2\}$, the injection $\ainj_i$ goes from elements of $\symbterms_i$ to elements of $\symbterms$. Recall that, by definition of symbolic memory states, members of these sets represent equivalence classes between terms.
Informally speaking, the role of $\ainj_1$ and $\ainj_2$ is then to explain how the terms in $\asms_1$ and $\asms_2$ are updated when the two symbolic memory states are combined into $\asms$.
For the remaining part of the section, let us fix three memory states
$\pair{\astore}{\aheap_1}$, $\pair{\astore}{\aheap_2}$ and $\pair{\astore}{\aheap}$, and let us assume $\asms_1 = \symbms{\astore}{\aheap_1}{\asetvar}{\bound_1} = {\triple{\symbterms_1}{\amap_1}{\symbrem_1}}$, $\asms_2 = \symbms{\astore}{\aheap_2}{\asetvar}{\bound_2} = {\triple{\symbterms_2}{\amap_2}{\symbrem_2}}$
and $\asms = \symbms{\astore}{\aheap}{\asetvar}{\bound_1+\bound_2} = {\triple{\symbterms}{\amap}{\symbrem}}$ to be their abstractions.
The key property of $\ainj_1$ and $\ainj_2$ is that, if $\triple{\asms_1}{\asms_2}{\asms} \in \asymbunion$ holds, then
for every equivalence class $\asymbterm \in \symbterms_i$ ($i \in \{1,2\}$),
the location $\alocation$ corresponding in $\pair{\astore}{\aheap_i}$ to the terms in $\asymbterm$ also corresponds
to the terms in $\ainj_i(\asymbterm)$ w.r.t. $\pair{\astore}{\aheap}$.
Essentially then, each pair in $\ainj_i$ (seen as a binary relation) uniquely corresponds to a location.
When this correspondence is understood, most of the conditions on these two injections are easy to follow.
When possible, we explain these conditions with easy ``small-step'' tautologies of \intervalSL (e.g.\ in \ref{C-meet-points}(a)).
\begin{enumerate}
\item Condition~\ref{C-functionality} essentially tells us that $\symbunion{\asms_1}{\asms_2}{\asms}$ cannot hold if the two symbolic memory states only correspond to concrete models that do not have a disjoint heap domain.
For example, let us consider the symbolic memory state $\asms' = (\asymbterm,\{\asymbterm \pto (\asymbterm,2) \},0)$ where $\asymbterm = \{ \avariable, \ameetvar{\avariable}{\avariable}{\avariable}\}$ and $\avariable \in \asetvar$.
Trivially, it cannot be that there is a symbolic memory state $\asms''$ such that $\symbunion{\asms'}{\asms'}{\asms''}$.
Indeed, every concrete memory state $\pair{\astore'}{\aheap'}$ having $\symbms{\astore'}{\aheap'}{\asetvar}{\bound} = \asms'$ must present a cycle involving the location corresponding to $\avariable$.
Hence, it cannot be that both $\pair{\astore}{\aheap_1}$ and $\pair{\astore}{\aheap_2}$ are abstracted by $\asms'$, as it implies that $\domain{\aheap_1} \cap \domain{\aheap_2} \neq \emptyset$ and therefore
$\aheap_1 + \aheap_2$ is not defined (which is required by \ref{compositionproperty}).
Alternatively, this condition can be easily explained with the formula $\lnot(\seesgeq{\aterm}{\aterm_1}{\asetmeetvar_1}{\inbound_1} \separate \seesgeq{\aterm}{\aterm_2}{\asetmeetvar_2}{\inbound_2})$, which is tautological in \intervalSL.
\item Let us now consider the Condition~\ref{C-meet-points}.
 \ref{C-meet-points}(a) essentially tells us that (dis)equivalences between program variables is preserved, and is better explained just by considering the tautology $\avariable = \avariablebis \iff (\avariable = \avariablebis \separate \true)$ (together with the commutativity of $\separate$).
To explain  \ref{C-meet-points}(b), consider $\pair{\astore}{\aheap_1}$ such that for a meet-point term $\ameetvar{\avariable}{\avariablebis}{\avariableter}$,
we have $\semantics{\ameetvar{\avariable}{\avariablebis}{\avariableter}}_{\astore,\aheap_1} = \alocation$.
Moreover, let $\aheap$
\begin{minipage}{0.8\linewidth}
be such that $\aheap_1 \subheap \aheap$.
The condition \ref{C-meet-points}(b) essentially
states the following:
\begin{itemize}[nosep]
  \item
  if $\ameetvar{\avariable}{\avariablebis}{\avariableter}$ is an asymmetric meet-point then the location $\alocation$ corresponds to $\ameetvar{\avariable}{\avariablebis}{\avariableter}$ also in $\pair{\astore}{\aheap}$. Formally,
  if $\pair{\astore}{\aheap_1} \models \ameetvar{\avariable}{\avariablebis}{\avariableter} \neq \ameetvar{\avariablebis}{\avariable}{\avariableter}$ then
  $\semantics{\ameetvar{\avariable}{\avariablebis}{\avariableter}}_{\astore,\aheap} = \semantics{\ameetvar{\avariable}{\avariablebis}{\avariableter}}_{\astore,\aheap_1}$.
  \item if instead $\ameetvar{\avariable}{\avariablebis}{\avariableter}$ is a symmetric meet-point, then the location $\alocation$ corresponds in $\pair{\astore}{\aheap}$ to at least one term between $\ameetvar{\avariable}{\avariablebis}{\avariableter}$ and $\ameetvar{\avariablebis}{\avariable}{\avariableter}$.
  Formally, if $\pair{\astore}{\aheap_1} \models \ameetvar{\avariable}{\avariablebis}{\avariableter} = \ameetvar{\avariablebis}{\avariable}{\avariableter}$ then
  $\semantics{\ameetvar{\avariable}{\avariablebis}{\avariableter}}_{\astore,\aheap} = \semantics{\ameetvar{\avariable}{\avariablebis}{\avariableter}}_{\astore,\aheap_1}$ or
  $\semantics{\ameetvar{\avariable}{\avariablebis}{\avariableter}}_{\astore,\aheap} = \semantics{\ameetvar{\avariablebis}{\avariable}{\avariableter}}_{\astore,\aheap_1}$.
\end{itemize}
The validity of this condition is pretty straightforward. If $\ameetvar{\avariable}{\avariablebis}{\avariableter}$ is an
asymmetric meet-point, it must be that $\alocation$ belongs to a cycle, as depicted on the first figure on the right.
Then, in every extension of this heap, $\alocation$ must still be the first location reachable from $\avariable$ that belongs to~the~cycle.%
\parfillskip=0pt
\end{minipage}%
\begin{minipage}{0.2\linewidth}
  \begin{flushright}
    \begin{minipage}{0.9\linewidth}
    \begin{tikzpicture}
      \coordinate (cir) at (0,0);
      \def\radius{0.45cm}
      %\draw (cir) circle[radius=\radius];

      \draw (cir) ++(90:\radius) node[highlightnode,label={[xshift=-15pt,yshift=-6pt]{$\scriptstyle{\ameetvar{\avariable}{\avariablebis}{\avariableter}}$}}] (k) {};

      \draw (cir) ++(270:\radius) node[dot,label={[yshift=-15pt]{$\scriptstyle{{\avariableter}}$}}] (u) {};

      \node[dot,label={[xshift=0pt]$\scriptstyle{\avariable}$}] (m) [above = 0.5cm of k] {};

      \draw (cir) ++(180:\radius) node[highlightnode,label={[xshift=17pt,yshift=-10pt]$\scriptstyle{
      \ameetvar{\avariablebis}{\avariable}{\avariableter}}$}] (ze) {};

      \node[dot,label=below:{$\scriptstyle{\avariablebis}$}] (z) [left=0.6cm of u] {};

      \draw[pto] (m.center) -- (k);
      \draw[pto] (z.center) -- (ze);

      \draw[pto] (u) .. controls +(0:1) and +(0:1) .. (k);
      \draw[pto] (k) .. controls +(180:0.3) and +(90:0.3) .. (ze);
      \draw[pto] (ze) .. controls +(-90:0.3) and +(180:0.3) .. (u);
    \end{tikzpicture}

    \begin{tikzpicture}
      \coordinate (cir) at (0,0);
      \def\radius{0.45cm}
      %\draw (cir) circle[radius=\radius];

      \draw (cir) ++(90:\radius) node[dot] (k) {};

      \draw (cir) ++(270:\radius) node[dot,label={[yshift=-15pt]{$\scriptstyle{{\avariableter}}$}}] (u) {};

      \node[dot,label={[xshift=0pt]$\scriptstyle{\avariable}$}] (m) [above = 0.5cm of k] {};

      \draw (cir) ++(180:\radius) node[highlightnode,label={[xshift=32pt,yshift=-10pt]$\scriptstyle{
      \ameetvar{\avariable}{\avariablebis}{\avariableter}} = \ameetvar{\avariablebis}{\avariable}{\avariableter}$}] (ze) {};

      \node[dot,label=below:{$\scriptstyle{\avariablebis}$}] (z) [left=0.6cm of u] {};

      \draw[pto] (m.center) -- (k);
      \draw[pto] (z.center) -- (ze);

      \draw[pto] (k) .. controls +(180:0.3) and +(90:0.3) .. (ze);
      \draw[pto] (ze) .. controls +(-90:0.3) and +(180:0.3) .. (u);
    \end{tikzpicture}
    \end{minipage}
    \end{flushright}
\end{minipage}

\noindent
Hence, by definition of meet-points, $\alocation$ still corresponds to $\ameetvar{\avariable}{\avariablebis}{\avariableter}$.
If instead $\ameetvar{\avariable}{\avariablebis}{\avariableter}$ is a symmetric meet-point (as depicted on the second figure) then there are essentially three possibilities.
First, it could be that $\ameetvar{\avariable}{\avariablebis}{\avariableter}$ is still a symmetric meet-point in $\pair{\astore}{\aheap}$. Then, as shortest paths are preserved when taking extensions of a heap, this meet-point must correspond to $\alocation$.
If instead $\ameetvar{\avariable}{\avariablebis}{\avariableter}$ is no longer a symmetric meet-point, $\alocation$ now belongs to a cycle. There are essentially two distinct ways to introduce such a cycle:
\begin{itemize}
  \item It could be that the cycle is closed on a location in the path from $\astore(\avariable)$ to $\semantics{\ameetvar{\avariable}{\avariablebis}{\avariableter}}_{\astore,\aheap_1}$ (excluded). Essentially, this means moving from the memory state depicted in the second figure to the one depicted in the first one.
  Then, $\alocation$ corresponds to $\ameetvar{\avariablebis}{\avariable}{\avariableter}$.
  \item It could be that the cycle is closed on a location in the path from $\astore(\avariablebis)$ to $\semantics{\ameetvar{\avariable}{\avariablebis}{\avariableter}}_{\astore,\aheap_1}$ (excluded).
  For instance, in the memory state depicted in the second figure, this can be done by adding a path from $\astore(\avariableter)$ to $\astore(\avariablebis)$. This case is symmetrical to the previous one, and $\alocation$ corresponds to $\ameetvar{\avariable}{\avariablebis}{\avariableter}$.
\end{itemize}

\item
For Condition~\ref{C-homomorphism},
let us start by reasoning on the two concrete memory states $\pair{\astore}{\aheap_1}$ and $\pair{\astore}{\aheap_2}$, and suppose that $\aheap_1 + \aheap_2$ is defined as $\aheap$. By looking at $\aheap$, it could be that new paths between program variables are generated. An example of this is depicted in the following figure, where a non-empty path from $\astore(\avariablebis)$ to itself is introduced.

\noindent\hfill%
\begin{tikzpicture}[baseline]

\node[dot,label={[xshift=0pt]$\scriptstyle{\avariable}$}] (x) at (0,0) {};
\node[dot,label={[yshift=-15pt]{$\scriptstyle{{\alocation}}$}}] (l) [right = 0.7cm of x] {};
\node[dot,label={[yshift=-15pt]{$\scriptstyle{{\avariablebis}}$}}] (y) [right = 0.7cm of l] {};

\draw[pto] (x.center) -- (l);
\draw[pto] (l.center) -- (y);

\end{tikzpicture}
\qquad\heapsum\qquad
\begin{tikzpicture}[baseline]

\node[dot,label={[xshift=0pt]$\scriptstyle{\avariable}$}] (x) at (0,0) {};
\node[dot,label={[yshift=-15pt]{$\scriptstyle{{\alocation}}$}}] (l) [right = 0.7cm of x] {};
\node[dot,label={[yshift=-15pt]{$\scriptstyle{{\avariablebis}}$}}] (y) [right = 0.7cm of l] {};

\draw[pto] (y) .. controls +(90:0.6) and +(90:0.6) .. (l);
\end{tikzpicture}
\qquad=\qquad
\begin{tikzpicture}[baseline]

\node[dot,label={[xshift=0pt]$\scriptstyle{\avariable}$}] (x) at (0,0) {};
\node[highlightnode,label={[yshift=-15pt]{$\scriptstyle{{\alocation}}$}}] (l) [right = 0.7cm of x] {};
\node[dot,label={[yshift=-15pt]{$\scriptstyle{{\avariablebis}}$}}] (y) [right = 0.7cm of l] {};

\draw[pto] (x.center) -- (l);
\draw[pto] (l.center) -- (y);

\draw[pto] (y) .. controls +(90:0.6) and +(90:0.6) .. (l);
\end{tikzpicture}
\hfill\,

Because of this, the truth values of $\mathtt{sees}$ predicates change. Indeed, it is clear that the memory state on the left satisfies $\seesgeq{\avariable}{\avariablebis}{\atermset{\{\avariable,\avariablebis\}}}{2}$.
However, this core formula is  not satisfied in the memory state on the right (the disjoint union), as the location $\alocation$ corresponds to the meet-point term $\ameetvar{\avariable}{\avariablebis}{\avariablebis}$. However, this memory state still satisfies
$\seesgeq{\avariable}{\avariablebis}{\emptyset}{2}$.
Then, Condition~\ref{C-homomorphism} essentially states that paths between locations corresponding to terms are preserved when the heap is extended.
With respect to program variables, this condition can therefore be understood from the tautology
$\seesgeq{\avariable}{\avariablebis}{\asetmeetvar}{\inbound} \separate \true \implies \seesgeq{\avariable}{\avariablebis}{\emptyset}{\inbound}$.
\end{enumerate}
As we just saw, Condition~\ref{C-homomorphism} deals with existing paths between terms, and states that they still exist when a heap is extended. The last condition (Condition~\ref{C-wasgarbage}) mainly deals instead with the new paths, created by the union of two heaps.
This condition uses the sets $\symbsources{\asms_1}{\asms_2}{\asms}$, $\symbtargets{\asms_i}{\asms}$ ($i \in \{1,2\}$) and
$\symbinternal{\asms_1}{\asms_2}{\asms}$, whose role is explained below.
\begin{itemize}
\item The set $\symbsources{\asms_1}{\asms_2}{\asms}$ contains the set of equivalence classes of $\symbterms$ having variables from which it is possible to start new paths.
An example of such a variable is given by $\avariablebis$ in the three memory states introduced in order to explain Condition~\ref{C-homomorphism}.
The key property is that, when considering the two leftmost memory states, $\astore(\avariablebis)$ does not reach
(in at least one step) any location corresponding to terms (formally, for every $i \in \{1,2\}$, $\equivclass{\avariablebis}{\symbterms_i} {\not \in} \domain{\amap_i}\}$).
\item The definition of $\symbtargets{\asms_i}{\asms}$ is more involved. Essentially, it contains the set of equivalence classes in $\symbterms$ corresponding to locations where new paths end.
By considering the example in Condition~\ref{C-homomorphism}, these locations are $\astore(\avariable)$, $\astore(\avariablebis)$ or $\alocation$, where this last location is taken into account since it belongs to the path from $\astore(\avariable)$ to $\astore(\avariablebis)$ of the leftmost memory state.
\item Lastly, $\symbinternal{\asms_1}{\asms_2}{\asms}$ is the set of equivalence classes in $\symbterms$ that corresponds to locations inside new paths. In particular, a member $\asymbterm$ of $\symbinternal{\asms_1}{\asms_2}{\asms}$ satisfies two properties:
\begin{itemize}
  \item In the concrete memory state abstracted with $\asms$, $\asymbterm$ corresponds to a location $\alocation$ in the shortest path from a location corresponding to some element in $\symbsources{\asms_1}{\asms_2}{\asms}$ to a location corresponding to an element in $\symbtargets{\asms_i}{\asms}$ (this latter element excluded);
  \item In the concrete memory states abstracted with $\asms_1$ and $\asms_2$, $\alocation$ does not belong to any non-empty path between location corresponding to terms.
\end{itemize}
As an example, let us consider the following three memory states:

\noindent\hfill%
\begin{tikzpicture}[baseline]

\node[dot,label={[xshift=0pt,yshift=-15pt]$\scriptstyle{\alocation}$}] (l) at (0,0) {};
\node[dot,label={[yshift=0pt]{$\scriptstyle{{\avariable}}$}}] (x) [above left = 0.7cm of l] {};
\node[dot,label={[yshift=-15pt]{$\scriptstyle{{\avariablebis}}$}}] (y) [below left = 0.7cm of l] {};
\node[dot,label={[yshift=-15pt]{$\scriptstyle{{\avariableter}}$}}] (z) [right = 0.7cm of l] {};

\draw[pto] (x.center) -- (l);
\draw[pto] (y.center) -- (l);

\end{tikzpicture}
\qquad\heapsum\qquad
\begin{tikzpicture}[baseline]

\node[dot,label={[yshift=-15pt]{$\scriptstyle{{\alocation}}$}}] (l) at (0,0) {};
\node[dot,label={[yshift=0pt]{$\scriptstyle{{\avariable}}$}}] (x) [above left = 0.7cm of l] {};
\node[dot,label={[yshift=-15pt]{$\scriptstyle{{\avariablebis}}$}}] (y) [below left = 0.7cm of l] {};
\node[dot,label={[yshift=-15pt]{$\scriptstyle{{\avariableter}}$}}] (z) [right = 0.7cm of l] {};

\draw[pto] (l.center) -- (z);

\end{tikzpicture}
\qquad=\qquad
\begin{tikzpicture}[baseline]

\node[highlightnode,label={[xshift=0pt,yshift=-15pt]$\scriptstyle{\alocation}$}] (l) at (0,0) {};
\node[dot,label={[yshift=0pt]{$\scriptstyle{{\avariable}}$}}] (x) [above left = 0.7cm of l] {};
\node[dot,label={[yshift=-15pt]{$\scriptstyle{{\avariablebis}}$}}] (y) [below left = 0.7cm of l] {};
\node[dot,label={[yshift=-15pt]{$\scriptstyle{{\avariableter}}$}}] (z) [right = 0.7cm of l] {};

\draw[pto] (x.center) -- (l);
\draw[pto] (y.center) -- (l);
\draw[pto] (l.center) -- (z);
\end{tikzpicture}
\hfill\,

\noindent Suppose $\asms_1$, $\asms_2$ and $\asms$ to be the abstractions of these three memory states (from the left to the right).
By definition, $\symbsources{\asms_1}{\asms_2}{\asms}$ and $\symbtargets{\asms_i}{\asms}$ (for $i \in \{1,2\}$) all contains the equivalence classes
$\equivclass{\avariable}{\symbterms}$, $\equivclass{\avariablebis}{\symbterms}$ and $\equivclass{\avariableter}{\symbterms}$.
The equivalence class $\equivclass{\ameetvar{\avariable}{\avariablebis}{\avariableter}}{\symbterms}$ is instead in $\symbinternal{\asms_1}{\asms_2}{\asms}$ (together with $\equivclass{\avariable}{\symbterms}$ and $\equivclass{\avariablebis}{\symbterms}$), as the location $\alocation$ that corresponds to it does not belong to any path between terms in the two subheaps abstracted with $\asms_1$ and $\asms_2$, whereas it belongs to the path from $\equivclass{\avariable}{\symbterms}$ to $\equivclass{\avariableter}{\symbterms}$ in the memory state abstracted with $\asms$.
\end{itemize}
We are now ready to explain Condition~\ref{C-wasgarbage}, which mainly deal with quantitative aspects of the \emph{new paths} generated by the union of memory states.
More precisely, supposing that $\pair{\astore}{\aheap_1}$ and $\pair{\astore}{\aheap_2}$ are such that $\aheap_1 + \aheap_2$ is defined, these paths must be created solely from location in $\domain{\aheap_1}$ or $\domain{\aheap_2}$ that (in both memory states) are not inside paths between locations corresponding to program variables.
From the definition of the symbolic memory states $\asms_1 = {\triple{\symbterms_1}{\amap_1}{\symbrem_1}}$ and $\asms_2 = {\triple{\symbterms_2}{\amap_2}{\symbrem_2}}$, these locations are abstracted with the two quantities $\symbrem_1$ and $\symbrem_2$. These two quantities give precise bounds and constraints on the lengths and the types of paths that can occur in $\asms$. Condition~\ref{C-wasgarbage} faithfully reflects these constraints.
\begin{enumerate}[start=4]
\item  Condition~\ref{C-wasgarbage} makes use of two functions $\amapbis_1$ and $\amapbis_2$, and two quantities $\symbrem_1'$ and $\symbrem_2'$. The role of these objects is, roughly speaking, to explain how the quantities $\symbrem_1$ and $\symbrem_2$ are distributed in $\asms$. Let us be more precise.

Given $i \in \{1,2\}$ and an element $\asymbterm$ in $\symbinternal{\asms_1}{\asms_2}{\asms}$,
$\amapbis_i(\asymbterm)$ reflects the number of locations abstracted with $\symbrem_i$ that are in the path from the location corresponding to $\asymbterm$ to the one corresponding to $\pi_1 \circ \amap(\asymbterm)$ (see \ref{C-wasgarbage}(a)).
Similarly, $\symbrem_i'$ reflects the number of locations abstracted with $\symbrem_i$ that are still garbage locations in $\asms$ (i.e. they are abstracted by $\symbrem$).
Condition~\ref{C-wasgarbage} then distinguishes two cases (both treated by \ref{C-wasgarbage}(b)): $\symbrem_i < \bound_i$ and $\symbrem_i = \bound_i$.
\begin{itemize}
\item If $\symbrem_i < \bound_i$ then, by definition of symbolic memory state, it holds that $\pair{\astore}{\aheap_i}$ (which is abstracted by $\asms_i$) contains exactly $\symbrem_i$ memory cells that are not inside paths between locations corresponding to program variables. Hence, exactly this number of locations must be retrieved from $\symbrem$ and the paths generated by terms in $\symbinternal{\asms_1}{\asms_2}{\asms}$.
Here is where $\amapbis_i$ and $\symbrem_i$ come into play, as we require $\symbrem_i' {+} \sum_{\asymbterm \in \symbinternal{\asms_1}{\asms_2}{\asms}} \amapbis_i(\asymbterm)$ to be equal~to~$\symbrem_i$.
\item If instead $\symbrem_i = \bound_i$, by definition of symbolic memory states it holds that $\pair{\astore}{\aheap_i}$ contains at least $\symbrem_i$ memory cells that are not inside paths between locations corresponding to program variables.
Hence, we require $\symbrem_i' + \sum_{\asymbterm \in \symbinternal{\asms_1}{\asms_2}{\asms}} \amapbis_i(\asymbterm)$ to be at least $\symbrem_i$.
\end{itemize}
Lastly, let us briefly explain \ref{C-wasgarbage}(c).
Let us consider a non-empty \emph{new} shortest path from a location corresponding to an equivalence class of $\symbsources{\asms_1}{\asms_2}{\asms}$ to a location corresponding to an equivalence class of $\symbtargets{\asms_i}{\asms}$.
Essentially, as it reaches an element in $\symbtargets{\asms_i}{\asms}$, \ref{C-wasgarbage}(c) states that there must be at least one location in this path that belongs to $\domain{\aheap_{3-i}}$ (i.e. the other heap).
Indeed, if this was not the case, the whole path would belong to the heap $\aheap_i$, and hence it is not generated by the union of the two memory states.
\end{enumerate}
