# Supplementary material for: A Complete Axiomatisation for Quantifier-Free Separation Logic
Source: arXiv:2006.05156 source file (2021-08-09)
Supplement: Supplementary file 6 [file intervalSL-auxiliary-lemmata-and-proofs.tex]

% \begin{lemma}\label{lemma:between-set}
% Let $\astore$ be a store and let $\aheap \subheap \aheap'$ be two heaps.
% If $\minpath{\alocation_1}{\alocation_2}{\aheap} \neq \emptyset$ then
% $\minpath{\alocation_1}{\alocation_2}{\aheap} = \minpath{\alocation_1}{\alocation_2}{\aheap'}$.
% \end{lemma}
% \begin{proof}(sketch)
% This is trivial from the dfinition of $\minpath{\alocation_1}{\alocation_2}{\aheap}$ as the set of location in the minimal non-empty path between $\alocation_1$ and $\alocation_2$ in $\aheap$. Indeed, as $\aheap \subheap \aheap'$ holds, the location in the set $\minpath{\alocation_1}{\alocation_2}{\aheap}$ are still in a path from $\alocation_1$ to $\alocation_2$. This path is still minimal, as $\aheap$ is a functional relation. Therefore
% $\minpath{\alocation_1}{\alocation_2}{\aheap} = \minpath{\alocation_1}{\alocation_2}{\aheap'}$.
% \end{proof}

%%%%%%CALCULUS

During the appendix (and moreso in Appendix~\ref{appendix:DerivedTautologies}), we will often give proofs in the style of Fitch proofs for natural deduction.
A proof
\[
  \begin{nd}
  \hypo {1} {\aformula_1}
  \hypo [\vdots] {2} {\vdots}
  \hypo [n] {3} {\aformula_n}
  \have [n+1] {4} {\aformulabis_1}
  \have [\vdots] {5} {\vdots}
  \have [j] {6} {\aformulater} \by{A, $i_{1}$, \dots, $i_{k}$}{}
  \have [\vdots] {7} {\vdots}
  \have [n+m] {8} {\aformulabis_m}
  \end{nd}
\]
where $\aformula_1,\dots,\aformula_n$ are the premises whereas $\aformulabis_1,\dots,\aformulabis_m$ are derivations, can be seen as the formula $\bigwedge_{i \in \interval{1}{n}} \aformula_{i} \implies \bigwedge_{i \in \interval{1}{m}} \aformulabis_i$.
In the proof below, we are only interested in the last derivation, so that we obtain a proof of $\bigwedge_{i \in \interval{1}{n}} \aformula_{i} \implies \aformulabis_m$.
With the notation
\begin{nscenter}
$
  \begin{nd}
  \have [j] {6} {\aformulater} \by{A, $i_{1}$, \dots, $i_{k}$}{}
  \end{nd}
$
\end{nscenter}
we denote that $\aformulater$ is derivable from the hypothesis and derivations labeled in the proof with the indices $i_{1}$, \dots, $i_{k}$ (that are bound to be less than $j$) by applying the axiom or rule $A$.

Some trivial steps, as the use of the symmetry axiom~\ref{core2Ax:EqSymm} and proofs that are exclusively from propositional calculus (e.g. the proof of $(\aformula \lor \aformulabis) \land (\aformula \implies \aformulater) \implies \aformulater \lor \aformulabis$) are omitted to shorten the presentation.
It should be kept in mind that these are not natural deduction proofs, as our system uses axioms to express logical reasoning, whereas natural deduction focus on inference rules. In the proofs,
with $\lor\text{E}$ we denote the tautology
\begin{nscenter}
$(\Gamma \Rightarrow ((\aformula \lor \aformulabis) \land (\aformula \Rightarrow \aformulater)\land(\aformulabis \Rightarrow \aformulater))) \implies (\Gamma \Rightarrow \aformulater)$
\end{nscenter}
that corresponds to a proof by cases started with hypothesis $\Gamma$.
Similarly, by $\lnot\text{I}$ we instead denote the tautology
\begin{nscenter}
$(\Gamma \Rightarrow (\aformula \Rightarrow \bottom)) \implies (\Gamma \Rightarrow \lnot \aformula)$
\end{nscenter}
that corresponds to a proof by contradiction started with hypothesis $\Gamma$.
Other tautologies of propositional calculus are denoted as follows:\\
\begin{tabular}{lcl}
\landcontr & : & $\aformula \land \lnot \aformula \implies \bottom$\\
\landtwo & : & $\aformula \implies \aformula \land \aformula$\\
\modusponens & : & $(\aformula \implies \aformulabis) \land \aformula \implies \aformulabis$\\
$\lor\text{I}$ & : & $\aformula \implies \aformula \lor \aformulabis$\\
$\land\text{E}$ & : & $\aformula_1 \land \aformula_2 \land \dots \land \aformula_n \implies \aformulabis_1 \land \aformulabis_2 \land \dots \land \aformulabis_m$, where $\{\aformulabis_1,\dots,\aformulabis_n\}\subseteq\{\aformula_1,\dots,\aformula_m\}$
\\
\lorimpL & : & $(\aformula \lor \aformulabis) \land (\aformula \implies \aformulater) \implies \aformulater \lor \aformulabis$\\
\lorimpR & : & $(\aformula \lor \aformulabis) \land (\aformulabis \implies \aformulater) \implies (\aformula \lor \aformulater)$
\end{tabular}
