# Supplementary material for: A Complete Axiomatisation for Quantifier-Free Separation Logic
Source: arXiv:2006.05156 source file (2021-08-09)
Supplement: Supplementary file 7 [file proof-lemma-axioms-eliminate-exists.tex]

Before tackling the proof of Lemma~\ref{lemma:axiomseliminateexists}, we introduce the notion of ``symbolic quantification'' on symbolic memory states,
which is analogous to what is done in
Appendix~\ref{appendix:CompositionMemoryState}  with the composition of symbolic memory states. This notion will be later needed in order to conclude that the satisfiability problem of \intervalSL is \pspace-complete.

Given three variables $\avariable$, $\avariablebis$, $\avariableter$ so that $\avariableter \not \in \{\avariable,\avariablebis\}$, symbolic quantification is a relation
$$
\asymbexists{\avariable}{\avariablebis}{\avariableter} \subseteq \sum_{\mathclap{\substack{\asetvar,\bound \ {\rm and} \  b  \in \set{0,1}\\ \avariableter \not \in \asetvar \supseteq \{\avariable,\avariablebis\}}}}(
\symbdomain{\asetvar\cup\{\avariableter\}}{\bound}\times \symbdomain{\asetvar}{2\bound+b})
$$
such that,
for $\triple{\symbterms}{\amap}{\symbrem}$ over $\pair{\asetvar\cup\{\avariableter\}}{\bound}$
and $\triple{\symbterms'}{\amap'}{\symbrem'}$ over $\pair{\asetvar}{2\bound+b}$,
where $\avariableter \not\in\asetvar\supseteq\{\avariable,\avariablebis\}$,
\begin{nscenter}
$\symbexists{\triple{\symbterms}{\amap}{\symbrem}}{\triple{\symbterms'}{\amap'}{\symbrem'}}{\avariable}{\avariablebis}{\avariableter}$ holds $\equivdef$
\end{nscenter}
\begin{enumerate}[label=\textbf{E\arabic*}]
\itemsep 0 cm
\item\label{E-satisfiability} $\triple{\symbterms}{\amap}{\symbrem}$ and $\triple{\symbterms'}{\amap'}{\symbrem'}$ are satisfiable, i.e.
$\charsymbform \triple{\symbterms}{\amap}{\symbrem}$ and $\charsymbform  \triple{\symbterms'}{\amap'}{\symbrem'}$ are satisfiable, which can be checked in \ptime.
\item\label{E-placement} There is a set $\{\asymbterm_0 {=} \equivclass{\avariable}{\symbterms},\asymbterm_1,\dots,\asymbterm_{n},\asymbterm_{n+1} {=} \equivclass{\avariablebis}{\symbterms}\} \subseteq \symbterms$ such that
\begin{enumerate}
\item for every $j \in \interval{0}{n}$, $(\pi_1 \circ \amap)(\asymbterm_j) = \asymbterm_{j+1}$;
\item $\avariableter \in  \bigcup_{j \in \interval{0}{n+1}}\asymbterm_j$, and $\avariablebis \not \in \bigcup_{j \in \interval{1}{n}}\asymbterm_j$.
\end{enumerate}
%%
%% SD 16/02/19
%% Does not seem anymore needed.
%% \item
%% $\prove_{\coresys} \charsymbform{\triple{\symbterms}{\amap}{\symbrem}} \implies \sees{\avariable}{\avariablebis}{\emptyset} \land (\avariableter = \avariable \lor \avariablebis =
%% \avariable \lor \lnot\sees{\avariable}{\avariablebis}{\{\avariable,\avariablebis,\avariableter\}})$;
%%
\item\label{E-garbage} If $\symbrem < \bound$ then $\symbrem'=\symbrem$, otherwise $\symbrem' \geq \bound$.
\item\label{E-no-new-location} $\boxed{\text{If there is}\ \aterm \in \equivclass{\avariableter}{\symbterms}\ \text{such that}\ \avariableter \not \in \chars{\aterm}}$ then there is a bijection $\amapbis: \symbterms \to \symbterms'$ such that
\begin{enumerate}
\item for every $\asymbterm \in \symbterms$, $\amapbis(\asymbterm) \subseteq \asymbterm$;
\item for all $\asymbterm_1,\asymbterm_2 \in \symbterms$,  $\inbound \in \interval{1}{\bound}$,
we have $\amap(\asymbterm_1) = \pair{\asymbterm_2}{\inbound}$ iff $\amap'(\amapbis(\asymbterm_1)) = \pair{\amapbis(\asymbterm_2)}{\inbound'}$
 and $\inbound' \in \interval{\bound}{2 \bound +b}$
such that ($\inbound' = \inbound$ if $\inbound < \bound$, otherwise $\inbound' \in \interval{\bound}{2 \bound + b}$).
%% that is is equivalent to $\inbound$ whenever $\inbound < \bound$, otherwise $\inbound' \geq \bound$;
\end{enumerate}
Informally, these constraints model the case when $\equivclass{\avariableter}{\symbterms}$ contains a term $\aterm$ such that $\avariableter \not\in\chars{\aterm}$. Then,
$\symbterms'$ and $\amap'$ are exactly like $\symbterms$ and $\amap$, but where $\avariableter$ is forgotten,
but still  $\triple{\symbterms'}{\amap'}{\symbrem'}$ is over
$\pair{\asetvar}{2\bound+b}$ and $\avariableter \not \in \asetvar$.
\item\label{E-new-location} $\boxed{\text{Otherwise} \  (\text{for every}\ \aterm \in \equivclass{\avariableter}{\symbterms}, \avariableter \in \chars{\aterm})}$ there is a bijection
$\amapbis: (\symbterms \setminus \{ \equivclass{\avariableter}{\symbterms}\}) \to \symbterms'$ s.t.\
\begin{enumerate}
\item for every $\asymbterm \in \symbterms \setminus \{ \equivclass{\avariableter}{\symbterms}\}$, $\amapbis(\asymbterm) \subseteq \asymbterm$;
\item for all $\asymbterm_1,\asymbterm_2 \in \symbterms \setminus \{ \equivclass{\avariableter}{\symbterms}\}$,
      $\inbound \in \interval{1}{\bound}$,
if $\amap(\asymbterm_1) = \pair{\asymbterm_2}{\inbound}$ then
$\amap'(\amapbis(\asymbterm_1)) = \pair{\amapbis(\asymbterm_2)}{\inbound'}$ and $\inbound' \in \interval{1}{2 \bound + b}$ such that
($\inbound' = \inbound$ if $\inbound < \bound$, otherwise $\inbound' \in \interval{\bound}{2 \bound + b}$).
%% that is is equivalent to $\inbound$ whenever $\inbound < \bound$, otherwise $\inbound' \geq \bound$;
\item for every $\asymbterm_1,\asymbterm_2 \in \symbterms \setminus \{ \equivclass{\avariableter}{\symbterms}\}$ and
$\inbound_1,\inbound_2 \in \interval{1}{\bound}$,
if $\amap(\asymbterm_1) = \pair{\equivclass{\avariableter}{\symbterms}}{\inbound_1}$ and
$\amap(\equivclass{\avariableter}{\symbterms}) = \pair{\asymbterm_2}{\inbound_2}$
then
$\amap'(\amapbis(\asymbterm_1)) = \pair{\amapbis(\asymbterm_2)}{\inbound'}$
for some $\inbound'$
such that $\inbound' = \inbound_1+\inbound_2$ if $\inbound_1 < \bound$ and $\inbound_2 < \bound$, otherwise $\inbound' \in
\interval{\inbound_1+\inbound_2}{2 \bound+b}$.
%% that is  equivalent to $\inbound_1+\inbound_2$ whenever $\inbound_1+\inbound_2 < \bound$, otherwise $\inbound' \geq \bound$;
\item for every $\asymbterm_1',\asymbterm_2'\in \symbterms'$, if $(\pi_1 \circ \amap')(\asymbterm_1') = \asymbterm_2'$ then $(\pi_1 \circ \amap)(\amapbis^{-1}(\asymbterm_1')) = \amapbis^{-1}(\asymbterm_2')$ or it holds that
$(\pi_1 \circ \amap)(\amapbis^{-1}(\asymbterm_1')) = \equivclass{\avariableter}{\symbterms}$ and $ (\pi_1 \circ \amap)(\equivclass{\avariableter}{\symbterms}) = \amapbis^{-1}(\asymbterm_2')$.
\end{enumerate}
Informally, these constraints model the case when each term $\aterm$ in $\equivclass{\avariableter}{\symbterms}$ is such that $\avariableter \in \chars{\aterm}$. Hence, removing $\avariableter$ will make the equivalence class disappears and $\amap$ must be updated accordingly.
\end{enumerate}

Correctness of the abstraction is stated in Lemma~\ref{lemma:quantificationisok} below, similarly to
forthcoming Lemma~\ref{lemma:compositionisok} dedicated to the composition of symbolic memory states.

\begin{lemma}\label{lemma:quantificationisok}
Let $b \in \set{0,1}$, $\bound \in \Nat^+$ and $\asetvar \subseteq_\fin \PVAR$ be such that $\avariableter \not \in \asetvar \supseteq \{\avariable,\avariablebis\}$.
Let $\pair{\astore}{\aheap}$ be a memory state and  $\triple{\symbterms}{\amap}{\symbrem}$
be a symbolic memory state over $\pair{\asetvar\cup\{\avariableter\}}{\bound}$. It holds that,
$\symbexists{\triple{\symbterms}{\amap}{\symbrem}}{\symbms{\astore}{\aheap}{\asetvar}{2\bound+b}}{\avariable}{\avariablebis}{\avariableter}$
if and only if
$\minpath{\astore(\avariable)}{\astore(\avariablebis)}{\aheap} \neq \emptyset$ and
there is $\alocation \in \minpath{\astore(\avariable)}{\astore(\avariablebis)}{\aheap}\cup\{\astore(\avariablebis)\}$ such that
$\symbms{\astore[\avariableter \gets \alocation]}{\aheap}{\asetvar\cup\{\avariableter\}}{\bound} = \triple{\symbterms}{\amap}{\symbrem}$.
\end{lemma}

\begin{proof} 
First, assume that $\minpath{\astore(\avariable)}{\astore(\avariablebis)}{\aheap} \neq \emptyset$ and
there is $\alocation \in \minpath{\astore(\avariable)}{\astore(\avariablebis)}{\aheap}\cup\{\astore(\avariablebis)\}$ such that 
$\symbms{\astore[\avariableter \gets \alocation]}{\aheap}{\asetvar\cup\{\avariableter\}}{\bound} = \triple{\symbterms}{\amap}{\symbrem}$.
Let us show that $\symbexists{\triple{\symbterms}{\amap}{\symbrem}}{\symbms{\astore}{\aheap}{\asetvar}{2\bound+b}}{\avariable}{\avariablebis}{\avariableter}$.
Let us verify the satisfaction of the conditions \ref{E-satisfiability}--\ref{E-new-location}.

Before checking the satisfaction of \ref{E-satisfiability}--\ref{E-new-location}, let us recall what are
$\triple{\symbterms}{\amap}{\symbrem}$ and $\triple{\symbterms'}{\amap'}{\symbrem'} = \symbms{\astore}{\aheap}{\asetvar}{2\bound+b}$.
Let us start by the definition of  $\triple{\symbterms'}{\amap'}{\symbrem'}$.
\begin{itemize}
\item $\symbterms' = \{ \{ \aterm_1 \in \atermset{\asetvar} \mid \pair{\astore}{\aheap} \models \aterm_1 = \aterm_2 \} \mid \aterm_2 \in \atermset{\asetvar} \}$;
\item $\amap'(\asymbterm) = (\asymbterm',\inbound)$ $\equivdef$ there are $\aterm_1 {\in} \asymbterm$ and $\aterm_2 {\in} \asymbterm'$ such that $\pair{\astore}{\aheap} \models \seesgeq{\aterm_1}{\aterm_2}{\atermset{\asetvar}}{\inbound}$ and if $\inbound < 2\bound+b$ then
$\pair{\astore}{\aheap} \models \lnot \seesgeq{\aterm_1}{\aterm_2}{\atermset{\asetvar}}{\inbound{+}1}$;
\item $\symbrem' = \inbound$ $\equivdef$ $\pair{\astore}{\aheap} \models \remgeq{\atermset{\asetvar}\times\atermset{\asetvar}}{\inbound}$ and 
if $\inbound < 2\bound +b$ then
$\pair{\astore}{\aheap} \models \lnot\remgeq{\atermset{\asetvar}\times\atermset{\asetvar}}{\inbound{+}1}$.
\end{itemize}
Here is the definition for $\triple{\symbterms}{\amap}{\symbrem}$:
\begin{itemize}
\item $\symbterms \egdef \{ \{ \aterm_1 \in \atermset{\asetvar \cup\{\avariableter\}} \mid \pair{\astore[\avariableter \gets \alocation]}{\aheap} \models 
\aterm_1 = \aterm_2 \} \mid \aterm_2 \in \atermset{\asetvar \cup\{\avariableter\}} \}$;
\item $\amap(\asymbterm) = (\asymbterm',\inbound)$ $\equivdef$ there are $\aterm_1 {\in} \asymbterm$ and $\aterm_2 {\in} \asymbterm'$ such that 
$\pair{\astore[\avariableter \gets \alocation]}{\aheap} \models \seesgeq{\aterm_1}{\aterm_2}{\atermset{\asetvar\cup\set{\avariableter}}}{\inbound}$ and 
if $\inbound < \bound$ then
$\pair{\astore[\avariableter \gets \alocation]}{\aheap} \models \lnot \seesgeq{\aterm_1}{\aterm_2}{\atermset{\asetvar\cup\set{\avariableter}}}{\inbound{+}1}$;
\item $\symbrem = \inbound$ $\equivdef$ $\pair{\astore[\avariableter \gets \alocation]}{\aheap} \models 
\remgeq{\atermset{\asetvar \cup\set{\avariableter}}\times\atermset{\asetvar\cup\set{\avariableter}}}{\inbound}$ and if $\inbound < \bound$ then
$\pair{\astore[\avariableter \gets \alocation]}{\aheap} \models 
\lnot \remgeq{\atermset{\asetvar\cup\set{\avariableter}}\times\atermset{\asetvar\cup\set{\avariableter}}}{\inbound{+}1}$.
\end{itemize}
The satisfaction of \ref{E-satisfiability} is obvious whereas the satisfaction of~\ref{E-garbage}
follows from the fact that 
$$
\remset{\astore[\avariableter \gets \alocation],\aheap}{\atermset{\asetvar\cup\set{\avariableter}}\times\atermset{\asetvar\cup\set{\avariableter}}} = \remset{\astore,\aheap}{\atermset{\asetvar}\times\atermset{\asetvar}}.
$$
Indeed, as  $\minpath{\astore(\avariable)}{\astore(\avariablebis)}{\aheap} \neq \emptyset$
and $\alocation \in \minpath{\astore(\avariable)}{\astore(\avariablebis)}{\aheap}\cup\{\astore(\avariablebis)\}$, 
the new value of $\avariableter$ in $\pair{\astore[\avariableter \gets \alocation]}{\aheap}$ does not change the memory cells
in the garbage with respect to 
$\atermset{\asetvar\cup\set{\avariableter}}\times\atermset{\asetvar\cup\set{\avariableter}} \ni \pair{\avariable}{\avariablebis}$.
Let us check the remaining conditions.

\begin{description}
\itemsep 0 cm 
\item[\ref{E-placement}] As $\alocation \in \minpath{\astore(\avariable)}{\astore(\avariablebis)}{\aheap}\cup\{\astore(\avariablebis)\}$, there is a minimal
path of length at least one in $\pair{\astore[\avariableter \gets \alocation]}{\aheap}$ of the form below:
$$
\semantics{\avariable}_{\astore,\aheap} = \semantics{\avariable}_{\astore[\avariableter \gets \alocation],\aheap} = \alocation_0 \mapsto
\alocation_1 \mapsto \cdots \mapsto \alocation_N = \semantics{\avariablebis}_{\astore,\aheap} = \semantics{\avariablebis}_{\astore[\avariableter \gets \alocation],\aheap}
$$
such that:
\begin{enumerate}
\item There are $0 = n_1 < \cdots < n_{\gamma} = N$ ($\gamma \geq 2$) such that $\alocation_{n_1}, \ldots, \alocation_{n_{\gamma}}$
are the only locations in $\set{\alocation_0, \ldots, \alocation_N}$ belonging to 
$\semantics{\atermset{\asetvar\cup\set{\avariableter}}}_{\astore[\avariableter \gets \alocation],\aheap}$.
\item There is some $\gamma' \in \interval{1}{\gamma}$ such that $\alocation_{n_{\gamma'}} = \alocation$ (indeed $\avariableter \in \atermset{\asetvar\cup\set{\avariableter}}$). 
Consequently, 
$$\set{\semantics{\avariable}_{\astore[\avariableter \gets \alocation],\aheap}, \semantics{\avariablebis}_{\astore[\avariableter \gets \alocation],\aheap},
\semantics{\avariableter}_{\astore[\avariableter \gets \alocation],\aheap}} \subseteq \set{\alocation_0, \ldots, \alocation_N}.
$$
\end{enumerate}
For every $i \in \interval{1}{\gamma}$, let $\asymbterm_i = \set{\aterm \in \atermset{\asetvar\cup\set{\avariableter}} \mid 
\semantics{\aterm}_{\astore[\avariableter \gets \alocation],\aheap} = \alocation_{n_i}}$. By definition of $n_i$, $\asymbterm_i$ is non-empty. Therefore,
by definition of $\triple{\symbterms}{\amap}{\symbrem}$ above, 
the following conditions hold:
\begin{enumerate}
\item for every $j \in \interval{1}{\gamma-1}$, $(\pi_1 \circ \amap)(\asymbterm_j) = \asymbterm_{j+1}$;
\item $\avariableter \in  \bigcup_{j \in \interval{1}{\gamma}}\asymbterm_j$, and $\avariablebis \not \in \bigcup_{j \in \interval{1}{\gamma-1}}\asymbterm_j$.
\end{enumerate} 
This concludes the verification for the condition~\ref{E-placement}. 
\item[\ref{E-no-new-location}] Assume that there is $\aterm \in \equivclass{\avariableter}{\symbterms}$
such that $\avariableter \not \in \chars{\aterm}$. Hence $\aterm \in \atermset{\asetvar}$ and therefore
for every $\asymbterm' \in \symbterms'$, there is  some $\asymbterm \in \symbterms$ such that
$\semantics{\asymbterm'}_{\astore,\aheap} = \semantics{\asymbterm}_{\astore[\avariableter \gets \alocation],\aheap}$
(note that $\semantics{\asymbterm'}_{\astore,\aheap}$ is  a singleton set).
Typically, no new location in the memory state $\pair{\astore[\avariableter \gets \alocation]}{\aheap}$ is interpreted
by a term from $\atermset{\asetvar \cup \set{\avariableter}}  \setminus \atermset{\asetvar}$.
Similarly, for every $\asymbterm \in \symbterms$, there is $\asymbterm' \in \symbterms'$ such that
$\semantics{\asymbterm'}_{\astore,\aheap} = \semantics{\asymbterm}_{\astore[\avariableter \gets \alocation],\aheap}$.
Actually, $\asymbterm'$ can be simply defined as $\asymbterm \cap \atermset{\asetvar}$ 
and therefore $\asymbterm' \subseteq \asymbterm$.  Let $\amapbis: \symbterms \to \symbterms'$ be the map
such that $\amapbis(\asymbterm) \egdef \asymbterm \cap \atermset{\asetvar}$. From the above observations, we can make the following conclusions.
\begin{itemize}
\item $\amapbis$ is a bijection.
\item For every $\asymbterm \in \symbterms$, $\amapbis(\asymbterm) \subseteq \asymbterm$.
\item Suppose that $\amap(\asymbterm_1) = \pair{\asymbterm_2}{\inbound}$.
      As no new location in the memory state $\pair{\astore[\avariableter \gets \alocation]}{\aheap}$ is interpreted
by a term from $\atermset{\asetvar} \cup \set{\avariableter} \setminus \atermset{\asetvar}$,
      we have $\amap'(\amapbis(\asymbterm_1)) = \pair{\amapbis(\asymbterm_2)}{\inbound'}$ for some $\inbound' \in \interval{1}{2 \bound + b}$.
      When $\inbound' < \bound$, again, as there is no new location  interpreted
by a term from $\atermset{\asetvar \cup \set{\avariableter}}  \setminus \atermset{\asetvar}$,
      we can conclude that $\inbound = \inbound'$. 
\item Finally, suppose that $\amap'(\amapbis(\asymbterm_1)) = \pair{\amapbis(\asymbterm_2)}{\inbound'}$
      and $\inbound = \inbound'$ if $\inbound' < \bound$, otherwise $\inbound = \bound$. As above, 
      no new location in the memory state $\pair{\astore[\avariableter \gets \alocation]}{\aheap}$ is interpreted
by a term from $\atermset{\asetvar} \cup \set{\avariableter} \setminus \atermset{\asetvar}$ and therefore we have 
$\amap(\asymbterm_1) = \pair{\asymbterm_2}{\inbound}$.
\end{itemize}
\item[\ref{E-new-location}] Contrary to the previous condition, assume that there is no 
 $\aterm \in \equivclass{\avariableter}{\symbterms}$
such that $\avariableter \not \in \chars{\aterm}$. Consequently, $\asymbterm_{\gamma'-1} \cap \atermset{\asetvar} \neq \emptyset$,
$\asymbterm_{\gamma'+1} \cap \atermset{\asetvar} \neq \emptyset$ and $\avariableter \in \asymbterm_{\gamma'} = \equivclass{\avariableter}{\symbterms}$. 
Let $\amapbis: (\symbterms \setminus \set{\equivclass{\avariableter}{\symbterms}}) \rightarrow \symbterms'$ be the map
such that $\amapbis(\asymbterm) \egdef \asymbterm \cap \atermset{\asetvar}$. Observe that by assumption, $\equivclass{\avariableter}{\symbterms} \cap
\atermset{\asetvar} = \emptyset$. Hence, the only new location in $\pair{\astore[\avariableter \gets \alocation]}{\aheap}$  interpreted
by a term from $\atermset{\asetvar \cup \set{\avariableter}}  \setminus \atermset{\asetvar}$ is precisely $\alocation$.
From the above observations, we can make the following conclusions.
\begin{enumerate}
\item $\amapbis$ is a bijection and for every $\asymbterm \in \symbterms$, $\amapbis(\asymbterm) \subseteq \asymbterm$.
\item Suppose that $\amap(\asymbterm_1) = \pair{\asymbterm_2}{\inbound}$ with $\asymbterm_1, \asymbterm_2 \in 
\symbterms \setminus \set{\equivclass{\avariableter}{\symbterms}}$. As $\alocation$ is the only location
in $\semantics{\atermset{\asetvar} \cup \set{\avariableter}}_{\astore[\avariableter \gets \alocation],\aheap} \setminus 
\semantics{\atermset{\asetvar}}_{\astore,\aheap}$, 
 we have $\amap'(\amapbis(\asymbterm_1)) = \pair{\amapbis(\asymbterm_2)}{\inbound'}$ for some $\inbound' \in \interval{1}{2 \bound+b}$.
      When $\inbound' < \bound$, again, as there is no new location  interpreted
by a term from $\atermset{\asetvar \cup \set{\avariableter}} \setminus \atermset{\asetvar}$,
      we can conclude that $\inbound = \inbound'$. 
\item Suppose that $\amap(\asymbterm_1) = \pair{\equivclass{\avariableter}{\symbterms}}{\inbound_1}$ and
$\amap(\equivclass{\avariableter}{\symbterms}) = \pair{\asymbterm_2}{\inbound_2}$. Necessarily, $\asymbterm_1 = \asymbterm_{\gamma'-1}$
and $\asymbterm_2 = \asymbterm_{\gamma'+1}$. Again, as $\alocation$ is the only location in 
 $\semantics{\atermset{\asetvar \cup \set{\avariableter}} }_{\astore[\avariableter \gets \alocation],\aheap} \setminus 
\semantics{\atermset{\asetvar}}_{\astore,\aheap}$, we have $\amap'(\amapbis(\asymbterm_1)) = \pair{\amapbis(\asymbterm_2)}{\inbound'}$
for some $\inbound'$. By a simple analysis on the way $\inbound$ and $\inbound'$ are computed (by truncation up to $\bound$ and $2 \bound+b$ respectively),
we can conclude that 
$\inbound' = \inbound_1+\inbound_2$ if $\inbound_1 < \bound$ and $\inbound_2 < \bound$, otherwise $\inbound' \in 
\interval{\inbound_1+\inbound_2}{2 \bound+b}$. 
\item Using similar arguments, one can show that for all $\asymbterm_1',\asymbterm_2'\in \symbterms'$, if 
      $(\pi_1 \circ \amap')(\asymbterm_1') = \asymbterm_2'$ then either
      $(\pi_1 \circ \amap)(\amapbis^{-1}(\asymbterm_1')) = \amapbis^{-1}(\asymbterm_2')$ or we have
     $(\pi_1 \circ \amap)(\amapbis^{-1}(\asymbterm_1')) = \equivclass{\avariableter}{\symbterms}$ and 
     $(\pi_1 \circ \amap)(\equivclass{\avariableter}{\symbterms}) = \amapbis^{-1}(\asymbterm_2')$.
\end{enumerate}

\end{description}

For the proof of the other direction, let us assume that $\triple{\symbterms}{\amap}{\symbrem}$ is a symbolic memory state
over $\pair{\asetvar\cup\{\avariableter\}}{\bound}$ such that 
$\symbexists{\triple{\symbterms}{\amap}{\symbrem}}{\symbms{\astore}{\aheap}{\asetvar}{2\bound+b}}{\avariable}{\avariablebis}{\avariableter}$.
As previously, we write $\triple{\symbterms'}{\amap'}{\symbrem'}$ to denote $\symbms{\astore}{\aheap}{\asetvar}{2\bound+b}$. 
Let us show that 
$\minpath{\astore(\avariable)}{\astore(\avariablebis)}{\aheap} \neq \emptyset$ and
there is $\alocation \in \minpath{\astore(\avariable)}{\astore(\avariablebis)}{\aheap}\cup\{\astore(\avariablebis)\}$ such that 
$\symbms{\astore[\avariableter \gets \alocation]}{\aheap}{\asetvar\cup\{\avariableter\}}{\bound} = \triple{\symbterms}{\amap}{\symbrem}$.
Note that the condition~\ref{E-placement} combined with either the condition~\ref{E-no-new-location} or the condition~\ref{E-new-location}
leads to get  $\minpath{\astore(\avariable)}{\astore(\avariablebis)}{\aheap} \neq \emptyset$.
Let us start by defining $\alocation$.
\begin{enumerate}
\item In the case there is $\aterm \in \equivclass{\avariableter}{\symbterms}$ such that $\avariableter \not \in \chars{\aterm}$,
let $\alocation = \semantics{\aterm}_{\astore,\aheap}$. 
\item Otherwise, let $I$ be such that $\avariableter \in \asymbterm_{I}$ from the condition~\ref{E-placement}.
As $\amap(\asymbterm_{I-1}) = \pair{\equivclass{\avariableter}{\symbterms}}{\inbound_1}$ and
$\amap(\equivclass{\avariableter}{\symbterms}) = \pair{\asymbterm_{I+1}}{\inbound_2}$, by the condition~\ref{E-new-location}, 
 we have $\amap'(\amapbis(\asymbterm_{I-1})) = \pair{\amapbis(\asymbterm_{I+1})}{\inbound'}$
for some $\inbound'$. Moreover, $\inbound' = \inbound_1+\inbound_2$ if $\inbound_1 < \bound$ and $\inbound_2 < \bound$, otherwise 
$\inbound' \in \interval{\inbound_1 + \inbound_2}{2 \bound+b}$.
By definition of $\amap'$,  in $\pair{\astore}{\aheap}$, there is a path from the unique location in $\semantics{\amapbis(\asymbterm_{I-1})}_{\astore,\aheap}$ and
the unique location in $\semantics{\amapbis(\asymbterm_{I+1})}_{\astore,\aheap}$ of the form $\alocation_0 \mapsto \alocation_1 \mapsto \cdots \mapsto \alocation_N$
with $\inbound' = \min(N,2 \bound+b)$. If $\inbound_1 < \bound$, then $\alocation = \alocation_{\inbound_1}$ otherwise
$\alocation = \alocation_{N - \inbound_2}$.
\end{enumerate}
It remains to check that $\symbms{\astore[\avariableter \gets \alocation]}{\aheap}{\asetvar\cup\{\avariableter\}}{\bound} = \triple{\symbterms}{\amap}{\symbrem}$,
which follows essentially from the satisfaction of the conditions~\ref{E-satisfiability}--\ref{E-new-location}.
For instance, the value $\symbrem$ matches thanks to the condition~\ref{E-garbage} and the value $\amap$ matches by the 
conditions~\ref{E-no-new-location} and~\ref{E-new-location}. The condition~\ref{E-satisfiability} is helpful for having the right set $\symbterms$. 
\end{proof}

We then obtain the following result, which, in a sense, checks that Lemma~\ref{lemma:quantificationisok} is what we need for the developments of Section~\ref{subsection:PSpace}.
\begin{lemma}\label{lemma:AbsQuantVsQuant}
Let $\bound \in \Nat^+$ and $\asetvar \subseteq_\fin \PVAR$ such that $\avariableter \not \in \asetvar \supseteq \{\avariable,\avariablebis\}$.
Let ${\triple{\symbterms}{\amap}{\symbrem}}$ and ${\triple{\symbterms'}{\amap'}{\symbrem'}}$
symbolic memory states respectively over $\pair{\asetvar\cup\{\avariableter\}}{\bound}$ and $\pair{\asetvar}{2\bound+b}$ and s.t.\
$\charsymbform\triple{\symbterms'}{\amap'}{\symbrem'}$ is satisfiable.
Then,
$\symbexists{\triple{\symbterms}{\amap}{\symbrem}}{\triple{\symbterms'}{\amap'}{\symbrem'}}{\avariable}{\avariablebis}{\avariableter}$ iff
$\models \charsymbform\triple{\symbterms'}{\amap'}{\symbrem'} \implies \inpath{\avariable}{\avariablebis}{\avariableter}\charsymbform\triple{\symbterms}{\amap}{\symbrem}$.
\end{lemma}

\begin{proof}
For the left to right direction, suppose $\symbexists{\triple{\symbterms}{\amap}{\symbrem}}{\triple{\symbterms'}{\amap'}{\symbrem'}}{\avariable}{\avariablebis}{\avariableter}$ and
$\pair{\astore}{\aheap} \models \charsymbform\triple{\symbterms'}{\amap'}{\symbrem'}$.
Then by Lemma~\ref{lemma:msmodelsabs}, $\triple{\symbterms'}{\amap'}{\symbrem'} = \symbms{\astore}{\aheap}{\asetvar}{2\bound+b}$.
We now apply Lemma~\ref{lemma:quantificationisok} and obtain that then
$\minpath{\astore(\avariable)}{\astore(\avariablebis)}{\aheap} \neq \emptyset$ and
there is $\alocation \in \minpath{\astore(\avariable)}{\astore(\avariablebis)}{\aheap}\cup\{\astore(\avariablebis)\}$ s.t.\
$\symbms{\astore[\avariableter \gets \alocation]}{\aheap}{\asetvar\cup\{\avariableter\}}{\bound} = \triple{\symbterms}{\amap}{\symbrem}$.
Again by Lemma~\ref{lemma:msmodelsabs}, then
$\pair{\astore[\avariableter \gets \alocation]}{\aheap} \models \charsymbform\triple{\symbterms}{\amap}{\symbrem}$.
By the semantics of the quantifier $\weirdexists$, we conclude that
$\pair{\astore}{\aheap} \models \inpath{\avariable}{\avariablebis}{\avariableter} \charsymbform\triple{\symbterms}{\amap}{\symbrem}$.

We now prove the right to left direction. Suppose
$\models \charsymbform\triple{\symbterms'}{\amap'}{\symbrem'} \implies \charsymbform\inpath{\avariable}{\avariablebis}{\avariableter}\triple{\symbterms}{\amap}{\symbrem}$.
As $\charsymbform\triple{\symbterms'}{\amap'}{\symbrem'}$ is satisfiable by hypothesis, there is a memory state $\pair{\astore}{\aheap} \models \charsymbform\triple{\symbterms'}{\amap'}{\symbrem'}$.
From the tautology above, we then have
$\pair{\astore}{\aheap} \models \inpath{\avariable}{\avariablebis}{\avariableter}\charsymbform\triple{\symbterms}{\amap}{\symbrem}$.
Hence, by definition of $\weirdexists$, $\minpath{\astore(\avariable)}{\astore(\avariablebis)}{\aheap} \neq \emptyset$ and
there is $\alocation \in \minpath{\astore(\avariable)}{\astore(\avariablebis)}{\aheap}\cup\{\astore(\avariablebis)\}$ such that
$\pair{\astore[\avariableter \gets \alocation]}{\aheap} \models \charsymbform\triple{\symbterms}{\amap}{\symbrem}$.
by Lemma~\ref{lemma:msmodelsabs} we have:
\begin{itemize}
\item $\symbms{\astore[\avariableter \gets \alocation]}{\aheap}{\asetvar}{2\bound+b} = \triple{\symbterms'}{\amap'}{\symbrem'}$;
\item $\symbms{\astore[\avariableter \gets \alocation]}{\aheap}{\asetvar\cup\{\avariableter\}}{\bound} = \triple{\symbterms}{\amap}{\symbrem}$.
\end{itemize}
By Lemma~\ref{lemma:quantificationisok}, we conclude that $\symbexists{\triple{\symbterms}{\amap}{\symbrem}}{\triple{\symbterms'}{\amap'}{\symbrem'}}{\avariable}{\avariablebis}{\avariableter}$.
\end{proof}

 We prove three auxiliary results. In particular, the third one proves of the elimination of a quantification $\inpath{\avariable}{\avariablebis}{\avariableter} \aformula$ where $\aformula$ is a core type.
 The general case for an arbitrary Boolean combination  $\aformula$ of core formulae is instead treated in Lemma~\ref{lemma:axiomseliminateexists}.
 The first lemma is pretty straightforward.

 \begin{lemma}\label{lemma:firstseesterm}
 Let $\asetvar \subseteq \PVAR$. Let $\aterm_1,\aterm_2 \in \atermset{\asetvar}$ and $\asetmeetvar \subseteq \atermset{\asetvar}$.
 Let $\pair{\astore}{\aheap}$ be a memroy state such that $\pair{\astore}{\aheap} \models \sees{\aterm_1}{\aterm_2}{\asetmeetvar}$. There is $\aterm_3 \in \atermset{\asetvar}$ such that
 $\pair{\astore}{\aheap} \models \sees{\aterm_1}{\aterm_3}{\atermset{\asetvar}}$.
 \end{lemma}
 \begin{proof}
 By definition, from $\pair{\astore}{\aheap} \models \sees{\aterm_1}{\aterm_2}{\asetmeetvar}$ it holds that
 there is $\delta \geq 1$ such that (a) $\aheap^{\delta}(\semantics{\aterm_1}_{\astore,\aheap}) = \semantics{\aterm_2}_{\astore,\aheap}$
 and (b) for all $\delta' \in \interval{1}{\delta-1}$, $\aheap^{\delta'}(\semantics{\aterm_1}_{\astore,\aheap}) \not \in
 \set{\semantics{\aterm_2}_{\astore,\aheap}} \cup \set{\semantics{\aterm}_{\astore,\aheap} \mid \aterm \in \asetmeetvar}$.
 Trivially, let us consider then the first location $\alocation$ reachable from $\semantics{\aterm_1}_{\astore,\aheap}$ in at least one step and such that $\alocation = \semantics{\aterm_3}_{\astore,\aheap}$ fore some $\aterm_3 \in \atermset{\asetvar}$.
 Formally,
 $\alocation$ is such that there is $\delta'' \leq \delta$ such that $\aheap^{\delta''}(\semantics{\aterm_1}_{\astore,\aheap}) = \alocation$ and for every $\delta''' \in \interval{1}{\delta''-1}$, $\aheap^{\delta'''}(\semantics{\aterm_1}_{\astore,\aheap}) \not \in \atermset{\asetvar}$.
 Since $\alocation = \semantics{\aterm_3}_{\astore,\aheap}$, by definition we obtain
 $\pair{\astore}{\aheap} \models \sees{\aterm_1}{\aterm_3}{\atermset{\asetvar}}$.
 \end{proof}

 The next lemma is instead technically involved (an informal description is given after its statement)

 \begin{lemma}\label{lemma:deterministicexistentialcompletion}
Let $\bound \in \Nat^+$ and let $\asetvar \subseteq_\fin \PVAR$ such that $\avariableter \not \in \asetvar$.
Let $\aformula \in \coretype{\asetvar \cup \{\avariableter\}}{\bound}$ be a satisfiable formula such that
for two terms
$\aterm_1,\aterm_2 \in \atermset{\asetvar}$ we have
  \begin{itemize}
    \item $\sees{\aterm_1}{\aterm_2}{\atermset{\asetvar}} \inside \aformula$;
    \item $\threeorliterals{\aterm_1 = \avariableter}{\aterm_2 = \avariableter}{\lnot \sees{\aterm_1}{\aterm_2}{\{\avariableter\}}} \inside \aformula$.
  \end{itemize}
Let $\aformula' = \bigwedge\{ \aformulater \inside \aformula \mid \aformulater \in \coreformulae{\asetvar}{\bound}\}$.
It holds that,
\begin{enumerate}
\item if there is $\aterm \in \{\aterm_1,\aterm_2\}$ such that $\aterm = \avariableter \inside \aformula$ then
$\prove_{\coresys} (\aterm = \avariableter \land \aformula') \iff \aformula$;
\item otherwise, there are $\inbound_1,\inbound_2 \in \interval{1}{\bound}$ such that
\begin{itemize}
\item $\seesgeq{\aterm_1}{\avariableter}{\atermset{\asetvar}}{\inbound_1} \land \seesgeq{\avariableter}{\aterm_2}{\atermset{\asetvar}}{\inbound_2} \inside \aformula$;
\item $\seesgeq{\aterm_1}{\avariableter}{\atermset{\asetvar}}{\inbound_1+1} \not\inside \aformula$ and $\seesgeq{\avariableter}{\aterm_2}{\atermset{\asetvar}}{\inbound_2+1} \not\inside \aformula$.
\end{itemize}
Let $\sim_1,\sim_2\in\{\geq,=\}$ such that for every $i \in \{1,2\}$, $\sim_i$ is $=$ iff $\inbound_i < \bound$.
Then
\begin{nscenter}
$\prove_{\coresys} (\sees{\aterm_1}{\avariableter}{\atermset{\asetvar}}{\sim_1}{\inbound_1} \land \sees{\avariableter}{\aterm_2}{\atermset{\asetvar}}{\sim_2}{\inbound_2}  \land \avariableter \not\in\{\aterm_1,\aterm_2\} \land \aformula') \iff \aformula$.
\end{nscenter}
\end{enumerate}
\end{lemma}

Let us informally explain this lemma. As hypothesis, we consider a core type  $\aformula \in \coretype{\asetvar \cup \{\avariableter\}}{\bound}$ where the variable $\avariableter$ is in the path starting from the location corresponding to $\aterm_1$ and ending in the location corresponding to $\aterm_2$, for some $\aterm_1$ and $\aterm_2$ in $\atermset{\asetvar}$ such that $\sees{\aterm_1}{\aterm_2}{\atermset{\asetvar}} \inside \aformula$.
Then, the lemma states that given a literal $\aformulabis \inside \aformula$ such that $\aformulabis \in \coreformulae{\asetvar\cup\{\avariableter\}}{\inbound}$ and $\avariableter \in \chars{\aformulabis}$,
the formula obtained from $\aformula$ by eliminating $\aformulabis$ is equivalent to the original one, with
the following exceptions of formulae that must be kept:
\begin{itemize}
\item if $\avariableter = \aterm_1$ or $\avariableter = \aterm_2$ occurs positively in $\aformula$, then one of these two formulae must be kept.
\item otherwise
(notice that then we are in the case that ${\lnot \sees{\aterm_1}{\aterm_2}{\{\avariableter\}}} \inside \aformula$) it is sufficient to keep
 $\sees{\aterm_1}{\avariableter}{\atermset{\asetvar}}{\sim_1}{\inbound_1} \land \sees{\avariableter}{\aterm_2}{\atermset{\asetvar}}{\sim_2}{\inbound_2}  \land \avariableter \not\in\{\aterm_1,\aterm_2\}$
where $\sees{\aterm_1}{\avariableter}{\atermset{\asetvar}}{\sim_1}{\inbound_1} \land \sees{\avariableter}{\aterm_2}{\atermset{\asetvar}}{\sim_2}{\inbound_2}$ has the ``maximal amount of information'' among all the $\sees{\aterm_1}{\avariableter}{\atermset{\asetvar}}$ and $\sees{\avariableter}{\aterm_2}{\atermset{\asetvar}}$
formulae.
Informally (the formal definition is in the statement of the lemma)
$\sees{\aterm_1}{\avariableter}{\atermset{\asetvar}}{\sim_1}{\inbound_1} \land \sees{\avariableter}{\aterm_2}{\atermset{\asetvar}}{\sim_2}{\inbound_2}$ has the ``maximal amount of information'' if it is not a consequence of a formula of the same shape (conjunctions of sees formulae).
For example, if $\sees{\aterm_1}{\avariableter}{\atermset{\asetvar}}{\geq}{3}$, $\sees{\aterm_1}{\avariableter}{\atermset{\asetvar}}{\geq}{4}$, $\lnot\sees{\aterm_1}{\avariableter}{\atermset{\asetvar}}{\geq}{5}$ and
$\lnot\sees{\aterm_1}{\avariableter}{\atermset{\asetvar}}{\geq}{6}$ all occurs in $\literals{\aformula}$, it is sufficient to keep
$\sees{\aterm_1}{\avariableter}{\atermset{\asetvar}}{\geq}{4}$ and $\lnot\sees{\aterm_1}{\avariableter}{\atermset{\asetvar}}{\geq}{5}$,
as the two other literals can clearly be deduced from these two (see the axiom~\ref{core2Ax:SeesMono1}).
\end{itemize}

\begin{proof}(sketch)
Let us start the proof by reasoning independently on the two cases dividing the lemma, and define
$\aformulater$ to be $\aterm = \avariableter$ if we are in the first case, and otherwise, if we are in the second case, let $\aformulater$ to be
\begin{nscenter}
$\sees{\aterm_1}{\avariableter}{\atermset{\asetvar}}{\sim_1}{\inbound_1} \land \sees{\avariableter}{\aterm_2}{\atermset{\asetvar}}{\sim_2}{\inbound_2}  \land \avariableter \not\in\{\aterm_1,\aterm_2\}$
\end{nscenter}
w.r.t. $\sim_1$, $\sim_2$, $\inbound_1$ and $\inbound_2$ as in the statement (the existence of $\aformulater$ in this case is easy to prove, as all its conjuncts are in $\literals{\aformula}$).
We want to prove that $\prove_{\coresys} \aformulater \land \aformula' \iff \aformula$, where
$\aformula' = \bigwedge\{ \aformulater \inside \aformula \mid \aformulater \in \coreformulae{\asetvar}{\bound}\}$.
Notice that, since $\coresys$ is a sound and complete axiomatisation for Boolean combination of core formulae, we can reason semantically in order to deduce that the above double implication is provable in the system.
Hence we show that $\models \aformulater \land \aformula' \iff \aformula$.
The right-to-let direction
$\models \aformulater \land \aformula' \Leftarrow \aformula$ trivially holds from $\aformulater \land \aformula' \inside \aformula$. From the satisfiability of $\aformula$, we then conclude that $\aformulater \land \aformula'$ is satisfiable.

In order to show that $\models \aformulater \land \aformula' \Rightarrow \aformula$, we consider two memory states
$\pair{\astore}{\aheap}$ and $\pair{\astore'}{\aheap'}$ satisfying $\aformulater \land \aformula'$.
We then prove that $\charsymbform(\symbms{\astore}{\aheap}{\asetvar \cup \{\avariableter\}}{\bound}) \iff \charsymbform(\symbms{\astore'}{\aheap'}{\asetvar \cup \{\avariableter\}}{\bound})$.
This is enough to prove the left-to-right direction.
Indeed, by Lemma~\ref{lemma:coretypecharsms} we know that every characteristic formula $\charsymbform(\asms)$ of a symbolic memory state $\asms$  w.r.t. $\pair{\asetvar \cup \{\avariableter\}}{\bound}$ is equivalent to exactly one core type of $\coretype{\asetvar \cup \{\avariableter\}}{\bound}$.
Moreover, since $\aformulater$ and $\aformula'$ are formulae in $\coreformulae{\asetvar \cup \{\avariableter\}}{\bound}$, by standard arguments we then conclude that $\aformulater \land \aformula'$ is equivalent to the infinite disjunction
$\bigvee_{(\astore'',\aheap'') \models \aformulater \land \aformula'} \charsymbform(\symbms{\astore''}{\aheap''}{\asetvar \cup \{\avariableter\}}{\bound}$.
Then, by proving that for every two $\pair{\astore}{\aheap}$ and $\pair{\astore'}{\aheap'}$ satisfying $\aformulater \land \aformula'$ are such that
$\charsymbform(\symbms{\astore}{\aheap}{\asetvar \cup \{\avariableter\}}{\bound}) \iff \charsymbform(\symbms{\astore'}{\aheap'}{\asetvar \cup \{\avariableter\}}{\bound})$, we directly conclude that there is a symbolic memory state
$\asms \in \symbdomain{\asetvar \cup \{\avariableter\}}{\bound}$
such that $\aformulater \land \aformula' \iff \charsymbform(\asms)$.
Thus, again by Lemma~\ref{lemma:coretypecharsms}, there is exactly one core type $\aformulabis$ in $\coretype{\asetvar \cup \{\avariableter\}}{\bound}$ such that
$\charsymbform(\asms) \iff \aformulabis$.
From the left-to-right direction of this lemma (i.e. $\aformula \implies \aformula' \land \aformulater$) together with $\aformula' \land \aformulater \implies \charsymbform(\asms)$, by propositional calculus we then conclude that
$\aformula \implies \aformula \land \aformulabis$. As $\aformula$ is  satisfiable by hypothesis, 
by definition of core types this implies that $\aformula \iff \aformulabis$, ending the proof.

Therefore, we show that given two memory states
$\pair{\astore}{\aheap}$ and $\pair{\astore'}{\aheap'}$ satisfying $\aformulater \land \aformula'$,
it holds that
$\charsymbform(\symbms{\astore}{\aheap}{\asetvar \cup \{\avariableter\}}{\bound}) \iff \charsymbform(\symbms{\astore'}{\aheap'}{\asetvar \cup \{\avariableter\}}{\bound})$.
To do so, we reason on the structure of the symbolic memory state and prove the equivalent statement
$\symbms{\astore}{\aheap}{\asetvar \cup \{\avariableter\}}{\bound} = \symbms{\astore'}{\aheap'}{\asetvar \cup \{\avariableter\}}{\bound}$.
First of, notice that directly by definition of core types, the fact that $\aformula \in \coretype{\asetvar \cup \{\avariableter\}}{\bound}$ and $\aformula' \inside \aformula$, we conclude that $\aformula'$ is a core type of $\coretype{\asetvar}{\bound}$.
Hence from $\pair{\astore}{\aheap} \models \aformula'$ and $\pair{\astore'}{\aheap'} \models \aformula'$ we already conclude by Lemma~\ref{lemma:msmodelsabs} that
$\symbms{\astore}{\aheap}{\asetvar}{\bound} = \symbms{\astore'}{\aheap'}{\asetvar}{\bound}$.
We say that a location is $\atermset{\asetvar}$\emph{-labelled} if it corresponds to a term of $\atermset{\asetvar}$.
We now consider the formula $\aformulater$, and essentially prove the following two properties:
\begin{enumerate}
\item Let $\asetbis$ be the set of $\atermset{\asetvar}$-labelled locations of $\pair{\astore}{\aheap}$, and let $\asetbis'$ be the set of its $\atermset{\asetvar \cup \{\avariableter\}}$-labelled locations. Then $\asetbis' = \asetbis$ (when $\aformulater$ corresponds to the first case of the statement) or $\asetbis' = \asetbis \cup \{\astore(\avariableter)\}$ (when $\aformulater$ corresponds to the second case of the statement).
\item Given a $\atermset{\asetvar}$-labelled location $\alocation$ of $\pair{\astore}{\aheap}$, given $\aformulater$ we can deterministically compute the set of terms $\aterm \in \atermset{\asetvar \cup \{\avariableter\}}$ such that $\semantics{\aterm}_{\astore,\aheap} = \alocation$.
\end{enumerate}
The same two properties also hold for $\pair{\astore'}{\aheap'}$. By definition of $\aformulater$, from these two properties we will conclude that
$\symbms{\astore}{\aheap}{\asetvar \cup \{\avariableter\}}{\bound}) = \symbms{\astore'}{\aheap'}{\asetvar \cup \{\avariableter\}}{\bound}$.
Moreover, notice that we can prove (2) from the proof of (1) as soon as for a given term $\ameetvar{\avariable'}{\avariablebis'}{\avariablesix'}$ where at least one variable between
$\avariable'$, $\avariablebis'$ and $\avariablesix'$ equals $\avariableter$, we can deterministically conclude that $\semantics{\ameetvar{\avariable'}{\avariablebis'}{\avariablesix'}}_{\astore,\aheap} = \astore(\avariableter)$ or find a term $\ameetvar{\avariable''}{\avariablebis''}{\avariablesix''} \in \atermset{\asetvar}$ such that
$\semantics{\ameetvar{\avariable'}{\avariablebis'}{\avariablesix'}}_{\astore,\aheap} = \semantics{\ameetvar{\avariable''}{\avariablebis''}{\avariablesix''}}_{\astore,\aheap}$.
This is exactly what we do. Hence, we focus on the proof of (1), which is by cases depending on $\aformulater$.
\begin{description}
  \item[a. $\aformulater$ is $\aterm {=} \avariableter$ for some $\aterm \in \{\aterm_1,\aterm_2\}$.] W.l.o.g. let $\aterm$ be syntactically equal to $\ameetvar{\avariable}{\avariablebis}{\avariablesix}$
  (indeed, if $\aterm$ is $\avariable \in \asetvar$, then by axiom~\ref{core2Ax:Self} we can consider $\ameetvar{\avariable}{\avariable}{\avariable}$ instead).
  Let us prove that the set $\asetbis$ of $\atermset{\asetvar}$-labelled locations of $\pair{\astore}{\aheap}$, equals the set $\asetbis'$ of $\atermset{\asetvar \cup \{\avariableter\}}$-labelled locations of $\pair{\astore}{\aheap}$.
  By definition every $\atermset{\asetvar}$-labelled locations is also a $\atermset{\asetvar \cup \{\avariableter\}}$-labelled locations, so we simply need to prove that $\asetbis' \subseteq \asetbis$.
  Let $\alocation$ be a $\atermset{\asetvar \cup \{\avariableter\}}$-labelled locations corresponding to a term $\overline{\aterm}$. If $\avariableter$ does not appear (syntactically) in $\overline{\aterm}$, then trivially $\alocation$ is also a
  $\atermset{\asetvar}$-labelled location. Otherwise, w.l.o.g. (again, see the axiom~\ref{core2Ax:Self}), let $\ameetvar{\avariable'}{\avariablebis'}{\avariablesix'}$ be a term such that
  $\semantics{\ameetvar{\avariable'}{\avariablebis'}{\avariablesix'}}_{\astore,\aheap} = \alocation$ and
  at least one variable between
  $\avariable'$, $\avariablebis'$ and $\avariablesix'$ equals $\avariableter$.
  By definition of meet-point, $\alocation$ is the first location reachable from $\astore(\avariable')$ that reaches $\astore(\avariablesix')$ and is also reached by $\astore(\avariablebis')$.
  We show that then there is a term in $\widehat{\aterm} \in \atermset{\asetvar}$ such that $\semantics{\ameetvar{\avariable'}{\avariablebis'}{\avariablesix'}}_{\astore,\aheap} = \semantics{\widehat{\aterm}}_{\astore,\aheap}$.
  We proceed by cases:
  \begin{itemize}
  \item if (syntactically) $\avariablesix' = \avariableter$, then $\alocation$ is also the first location reachable from $\astore(\avariable')$ that reaches $\astore(\avariablesix)$ and is also reached by $\astore(\avariablebis')$.
  Hence $\semantics{\ameetvar{\avariable'}{\avariablebis'}{\avariablesix'}}_{\astore,\aheap} = \semantics{\ameetvar{\avariable'}{\avariablebis'}{\avariablesix}}_{\astore,\aheap}$.
  \item if (syntactically) $\avariable' = \avariableter$, then $\alocation$ is also the first location reachable from $\astore(\avariable)$ that reaches $\astore(\avariablesix')$ and is also reached by $\astore(\avariablebis')$.
  Hence $\semantics{\ameetvar{\avariable'}{\avariablebis'}{\avariablesix'}}_{\astore,\aheap} = \semantics{\ameetvar{\avariable}{\avariablebis'}{\avariablesix'}}_{\astore,\aheap}$.
  \item if (syntactically) $\avariablebis' = \avariableter$, then $\alocation$ is also the first location reachable from $\astore(\avariable')$ that reaches $\astore(\avariablesix')$ and is also reached by $\astore(\avariable)$.
  Hence $\semantics{\ameetvar{\avariable'}{\avariablebis'}{\avariablesix'}}_{\astore,\aheap} = \semantics{\ameetvar{\avariable'}{\avariable}{\avariablesix'}}_{\astore,\aheap}$.
  \end{itemize}
  Thus, it is easy to see that by iterating the three steps just above, given $\ameetvar{\avariable'}{\avariablebis'}{\avariablesix'}$ it is always possible to (deterministically, since $=$ is an equivalence relation) replace every occurrence of $\avariableter$ in order to find a term $\widehat{\aterm} \in \atermset{\asetvar}$ such that $\semantics{\widehat{\aterm}}_{\astore,\aheap} = \alocation$.
  Hence $\asetbis' = \asetbis$.
  \item[b. $\aformulater$ is $\sees{\aterm_1}{\avariableter}{\atermset{\asetvar}}{\sim_1}{\inbound_1} \land \sees{\avariableter}{\aterm_2}{\atermset{\asetvar}}{\sim_2}{\inbound_2}  \land \avariableter \not\in\{\aterm_1,\aterm_2\}$.]

  W.r.t. the sets $\asetbis$ and $\asetbis'$ in the statement of (1), we prove that $\asetbis' = \asetbis \cup \{\astore(\avariableter)\}$. As in the previous case, it is sufficient to show $\asetbis' \subseteq \asetbis \cup \{\astore(\avariableter)\}$.
  W.l.o.g. (see the axiom~\ref{core2Ax:Self})
  suppose
  $\aterm_1 = \ameetvar{\avariable}{\avariablebis}{\avariablesix}$ and
  $\aterm_2 = \ameetvar{\avariable'}{\avariablebis'}{\avariablesix'}$, syntactically.
  From $\aformulater$, we conclude that every location in the path from $\semantics{\aterm_1}_{\astore,\aheap}$ to $\semantics{\aterm_2}_{\astore,\aheap}$, both ends excluded, is not a $\atermset{\asetvar}$-labelled location.
  However, one of these locations corresponds to $\astore(\avariableter)$, hence $\astore(\avariableter) \in \asetbis'$ and moreover $\aheap$ must present exactly one of the following three patterns:
  \begin{center}
  \vspace{-0.7cm}
   \scalebox{0.85}{
       \begin{tikzpicture}[baseline]
         \node (i) at (0,0) {};
         \node[dot,label=below:{$\ameetvar{\avariable}{\avariablebis}{\avariablesix}$}] (m) [below = 1.5cm of i] {};
         \node[dot,label=above:{$\avariableter$}] (z) [right = 1cm of m] {};
         \node[dot,label=right:$\ameetvar{\avariable'}{\avariablebis'}{\avariablesix'}$] (j) [right= 1cm of z] {};
         \node[label=below:{does not loop}] (k) [below of=j] {};
         \node (kk) [above = 1.5cm of j] {};

         \draw[reach] (i) -- (m);
         \draw[pto] (m) to node [above] {$+$} (z);
         \draw[pto] (z) to node [above] {$+$} (j);
         \draw[reach] (kk) -- (j);
         \draw[reach] (j) -- (k);
       \end{tikzpicture}
       \quad
       \begin{tikzpicture}[baseline]
         \node (i) at (0,0) {};
         \node[dot,label=below:{$\ameetvar{\avariable}{\avariablebis}{\avariablesix}$}] (m) [below = 1.5cm of i] {};
         \node[dot,label=above:{$\avariableter$}] (z) [right = 1cm of m] {};
         \node[dot,label=right:$\ameetvar{\avariable'}{\avariablebis'}{\avariablesix'}$] (j) [right= 1cm of z] {};
         \node[dot,label=above right:{$\overline{\alocation}$}] (k) [below of=j] {};
         \node (kk) [above = 1.5cm of j] {};

         \draw[reach] (i) -- (m);
         \draw[pto] (m) to node [above] {$+$} (z);
         \draw[pto] (z) to node [above] {$+$} (j);
         \draw[reach] (j) -- (k);
         \draw[reach] (kk) -- (j);
         \draw[reach] (k) to [out=-20, in=-160
                , looseness=0.8, loop
                , distance=2cm, reach] node {} (k);
       \end{tikzpicture}
       \quad
       \begin{tikzpicture}[baseline]
         \node (i) at (0,0) {};
         \node[dot,label=left:{$\ameetvar{\avariable}{\avariablebis}{\avariablesix}$}] (m) [below = 1.5cm of i] {};
         \node[dot,label=above:{$\avariableter$}] (z) [right = 1cm of m] {};
         \node[dot,label=right:$\ameetvar{\avariable'}{\avariablebis'}{\avariablesix'}$] (j) [right= 1cm of z] {};
         \node (kk) [above = 1.5cm of j] {};

         \draw[reach] (i) -- (m);
         \draw[pto] (m) to node [above] {$+$} (z);
         \draw[pto] (z) to node [above] {$+$} (j);
         \draw[reach] (kk) -- (j);
         \draw[reach] (j) to [out=-90, in=-90
                , looseness=0.8, loop
                , distance=2cm, reach] node {} (m);
       \end{tikzpicture}
   }
  \end{center}
  Let $\alocation$ be a $\atermset{\asetvar \cup \{\avariableter\}}$-labelled locations corresponding to a term $\overline{\aterm}$. If $\avariableter$ does not appear (syntactically) in $\overline{\aterm}$, or $\alocation = \astore(\avariableter)$, then $\alocation \in \asetbis \cup \{\astore(\avariableter)\}$.
   Otherwise, w.l.o.g. (again, see the axiom~\ref{core2Ax:Self}), let us consider $\ameetvar{\widehat{\avariable}}{\widehat{\avariablebis}}{\widehat{\avariablesix}}$ be a term such that $\astore(\avariableter) \neq \alocation$,
  $\semantics{\ameetvar{\widehat{\avariable}}{\widehat{\avariablebis}}{\widehat{\avariablesix}}}_{\astore,\aheap} = \alocation$ and
  at least one variable between
  $\avariable'$, $\avariablebis'$ and $\avariablesix'$ equals $\avariableter$.
  By definition of meet-point, $\alocation$ is the first location reachable from $\astore(\avariable')$ that reaches $\astore(\avariablesix')$ and is also reached by $\astore(\avariablebis')$.
  We show that then there is a term in $\widehat{\aterm} \in \atermset{\asetvar}$ such that $\semantics{\ameetvar{\widehat{\avariable}}{\widehat{\avariablebis}}{\widehat{\avariablesix}}}_{\astore,\aheap} = \semantics{\widehat{\aterm}}_{\astore,\aheap}$.
  We proceed by cases:
  \begin{itemize}
  \item if (syntactically) $\widehat{\avariablesix} = \avariableter$, then $\alocation$ is also the first location reachable from $\astore(\widehat{\avariablebis})$ that reaches $\astore(\avariablesix')$ and is also reached by $\astore(\widehat{\avariablebis})$.
  Hence $\semantics{\ameetvar{\widehat{\avariable}}{\widehat{\avariablebis}}{\widehat{\avariablesix}}}_{\astore,\aheap} = \semantics{\ameetvar{\widehat{\avariable}}{\widehat{\avariablebis}}{\avariablesix'}}_{\astore,\aheap}$.
  \item Suppose (syntactically) $\widehat{\avariable} = \avariableter$.
  Then, the third pattern cannot occur in $\aheap$.
  Indeed, Suppose (ad absurdum) that the third pattern occurs in $\aheap$ and therefore that
   $\astore(\avariableter)$ belongs to a cycle.
   It is then easy to see that $\ameetvar{\avariableter}{\widehat{\avariablebis}}{\widehat{\avariablesix}}$ then corresponds to the location $\astore(\avariableter)$.
  Informally, this holds as by definition $\semantics{\ameetvar{\avariableter}{\widehat{\avariablebis}}{\widehat{\avariablesix}}}_{\astore,\aheap}$ must be the \emph{first location} that is reached by $\astore(\avariableter)$, reaches $\widehat{\avariablebis}$ and is reached by $\astore(\avariablesix)$.
  Since $\astore(\avariable)$ belongs to a cycle, the constraint of being the ``first location'' holds for $\astore(\avariableter)$.
  A more formal proof of this can be found inside Lemma~\ref{lemma:axiomstwoRCchars} (point 2, see also \ref{axiom2:auxlemma7}).
  Then, the third pattern leads to a contradiction with $\alocation \neq \astore(\avariableter)$.

  Therefore, the first or second pattern holds in $\aheap$. In each of these two cases, since $\alocation \neq \astore(\avariableter)$, we can easily prove that $\alocation$ is also the first location reachable from $\astore(\avariable)$ that reaches $\astore(\widehat{\avariablesix})$ and is reached by $\astore(\widehat{\avariablebis})$.
  Hence,
  $\ameetvar{\widehat{\avariable}}{\widehat{\avariablebis}}{\widehat{\avariablesix}} = \ameetvar{\avariable}{\widehat{\avariablebis}}{\widehat{\avariablesix}}$.
  \item Suppose (syntactically) $\widehat{\avariablebis} = \avariableter$.
  We then split the proof, depending on whether or not the third pattern occurs in $\aheap$.
  \begin{itemize}
  \item Similarly to the last point of the proof, if the first or second pattern occur in $\aheap$, then in both cases  $\alocation$ is also the first location reachable from $\astore(\avariable)$ that reaches $\astore(\widehat{\avariablesix})$ and is reached by $\astore(\widehat{\avariablebis})$.
  Hence,
  $\ameetvar{\widehat{\avariable}}{\widehat{\avariablebis}}{\widehat{\avariablesix}} = \ameetvar{\avariable}{\widehat{\avariablebis}}{\widehat{\avariablesix}}$.
  \item If instead we have that the third pattern occur in $\aheap$,
  then $\alocation$ that belongs to the same cycle as $\astore(\avariableter)$ (recall that $\alocation \neq \astore(\avariableter)$).
  Trivially, if $\semantics{\ameetvar{\widehat{\avariable}}{\widehat{\avariablebis}}{\widehat{\avariablesix}}}_{\astore,\aheap} = \semantics{\ameetvar{\avariable}{\avariablebis}{\avariablesix}}_{\astore,\aheap}$, we
  the term $\ameetvar{\avariable}{\avariablebis}{\avariablesix}$ is a solution for the term $\widehat{\aterm}$ we are searching.
  Otherwise, we have $\alocation = \semantics{\ameetvar{\widehat{\avariable}}{\widehat{\avariablebis}}{\widehat{\avariablesix}}}_{\astore,\aheap} \not \in \{ \astore(\avariableter), \semantics{\ameetvar{\avariable}{\avariablebis}{\avariablesix}}_{\astore,\aheap}\}$.
  Then, as shown in Lemma~\ref{lemma:axiomstwoRCchars} (points 5 and 6), from the fact that $\alocation$, $\astore(\avariableter)$ and $\semantics{\ameetvar{\avariable}{\avariablebis}{\avariablesix}}_{\astore,\aheap}$ are dfferent and belongs to the same loop, we conclude that
  $\semantics{\ameetvar{\widehat{\avariable}}{\widehat{\avariablebis}}{\widehat{\avariablesix}}}_{\astore,\aheap} = \semantics{\ameetvar{\widehat{\avariable}}{\avariableter}{\widehat{\avariablesix}}}_{\astore,\aheap}$.
  \end{itemize}
  \end{itemize}
  Again, it is easy to see that we can iterate these three steps and, given $\ameetvar{\widehat{\avariable}}{\widehat{\avariablebis}}{\widehat{\avariablesix}}$, always (deterministically) find a term $\widehat{\aterm} \in \atermset{\asetvar}$ such that $\semantics{\widehat{\aterm}}_{\astore,\aheap} = \alocation$.
  This concludes the proof of $\asetbis' = \asetbis \cup \{\astore(\avariableter)\}$.
\end{description}
This ends the proofs of (1) and (2).

We are now ready to show that $\symbms{\astore}{\aheap}{\asetvar \cup \{\avariableter\}}{\bound} = \symbms{\astore'}{\aheap'}{\asetvar \cup \{\avariableter\}}{\bound}$. We consider the following four objects:
\begin{itemize}
\item $\symbms{\astore}{\aheap}{\asetvar}{\bound} = \triple{\symbterms_{\asetvar}}{\amap_{\asetvar}}{\symbrem_{\asetvar}}$ and $\symbms{\astore}{\aheap}{\asetvar \cup \{\avariableter\}}{\bound} =
\triple{\symbterms_{\asetvar \cup \{\avariableter\}}}{\amap_{\asetvar \cup \{\avariableter\}}}{\symbrem_{\asetvar \cup \{\avariableter\}}}$;
\item $\symbms{\astore'}{\aheap'}{\asetvar}{\bound} = \triple{\symbterms_{\asetvar}'}{\amap_{\asetvar}'}{\symbrem_{\asetvar}'}$
and $\symbms{\astore'}{\aheap'}{\asetvar \cup \{\avariableter\}}{\bound} = \triple{\symbterms_{\asetvar \cup \{\avariableter\}}'}{\amap_{\asetvar \cup \{\avariableter\}}'}{\symbrem_{\asetvar \cup \{\avariableter\}}'}$.
\end{itemize}
Recall that $\symbms{\astore}{\aheap}{\asetvar}{\bound} = \symbms{\astore'}{\aheap'}{\asetvar}{\bound}$.
From this, together $\pair{\astore}{\aheap} \models \aformulater$, $\pair{\astore'}{\aheap'} \models \aformulater$ and
$\symbms{\astore}{\aheap}{\asetvar}{\bound}) = \symbms{\astore'}{\aheap'}{\asetvar}{\bound}$, by (1) and (2) we already conclude that $\symbterms_{\asetvar \cup \{\avariableter\}} = \symbterms_{\asetvar \cup \{\avariableter\}}'$.
Let us how show that $\symbrem_{\asetvar \cup \{\avariableter\}} = \symbrem_{\asetvar \cup \{\avariableter\}}'$.
First, by definition of symbolic memory state, given a memory state $\pair{\astore''}{\aheap''}$ and  $\symbms{\astore''}{\aheap''}{\asetvar}{\bound} = \triple{\symbterms}{\amap}{\symbrem}$ the natural number $\symbrem$ encoding the number of memory cells (up to $\bound$)
not in paths between terms of $\atermset{\asetvar}$. Formally, for $\inbound \in \interval{0}{\bound}$
\begin{nscenter}
$\symbrem = \inbound$ $\equivdef$ $\pair{\astore''}{\aheap''} \models \remgeq{\atermset{\asetvar}\times\atermset{\asetvar}}{\inbound}$ and if $\inbound < \bound$ then
$\pair{\astore''}{\aheap''} \models \lnot\remgeq{\atermset{\asetvar}\times\atermset{\asetvar}}{\inbound{+}1}$.
\end{nscenter}
Let us consider $\pair{\astore}{\aheap}$ (the same reasoning can be done for $\pair{\astore'}{\aheap'}$).
Since $\pair{\astore}{\aheap} \models \aformulater$, it is easy to see that the location $\astore(\avariableter)$ belongs to a (possibly empty) path between two terms in $\atermset{\asetvar}$. Hence, $\symbrem_{\asetvar \cup \{\avariableter\}} = \symbrem_{\asetvar}$.
Then, from $\symbms{\astore}{\aheap}{\asetvar}{\bound} = \symbms{\astore'}{\aheap'}{\asetvar}{\bound}$ (more precisely from $\symbrem_{\asetvar} = \symbrem_{\asetvar}'$), we conclude that
$\symbrem_{\asetvar \cup \{\avariableter\}} = \symbrem_{\asetvar \cup \{\avariableter\}}'$.
Lastly, let us show that $\amap_{\asetvar \cup \{\avariableter\}} = \amap_{\asetvar \cup \{\avariableter\}}'$.
We divide the proof into two cases, depending on whether $\aformulater$ corresponds to the first or second case in the statement of the lemma.
\begin{description}
\item[a. $\aformulater$ is $\aterm {=} \avariableter$ for some $\aterm \in \{\aterm_1,\aterm_2\}$.]
Then, from (1) and (2) we have that there is a bijection $\amapbis: \symbterms_{\asetvar \cup \{\avariableter\}} \to  \symbterms_{\asetvar}$ such that for every $\asetmeetvar \in \symbterms_{\asetvar \cup \{\avariableter\}}$,
$\amapbis(\asetmeetvar) \subseteq \asetmeetvar$.
Hence, by definition of symbolic memory state, for every $\aterm \in \atermset{\asetvar \cup \{\avariableter\}}$,
$\amap_{\asetvar \cup \{\avariable\}}(\equivclass{\aterm'}{\symbterms_{\asetvar\cup\{ \avariableter \}}}) = \amap_{\asetvar}(\equivclass{\aterm'}{\symbterms_{\asetvar}})$
where $\aterm' \in \amapbis(\equivclass{\aterm}{\symbterms_{\asetvar\cup\{ \avariableter \}}})$.
As $\symbterms_{\asetvar} = \symbterms_{\asetvar}'$ and $\symbterms_{\asetvar \cup \{\avariableter\}} = \symbterms_{\asetvar \cup \{\avariableter\}}'$, we can use the same $\amapbis$
and conclude a similar statement for $\pair{\astore'}{\aheap'}$, i.e. for every $\aterm \in \atermset{\asetvar \cup \{\avariableter\}}$,
$\amap_{\asetvar \cup \{\avariable\}}'(\equivclass{\aterm'}{\symbterms_{\asetvar\cup\{ \avariableter \}}'}) = \amap_{\asetvar}'(\equivclass{\aterm'}{\symbterms_{\asetvar}'})$
where $\aterm' \in \amapbis(\equivclass{\aterm}{\symbterms_{\asetvar\cup\{ \avariableter \}}})$.
Thus, from $\amap_{\asetvar} = \amap_{\asetvar}'$, we conclude that
$\amap_{\asetvar\cup\{ \avariableter \}} = \amap_{\asetvar\cup\{ \avariableter \}}'$.
\item[b. $\aformulater$ is $\sees{\aterm_1}{\avariableter}{\atermset{\asetvar}}{\sim_1}{\inbound_1} \land \sees{\avariableter}{\aterm_2}{\atermset{\asetvar}}{\sim_2}{\inbound_2}  \land \avariableter \not\in\{\aterm_1,\aterm_2\}$.]
Let us consider $\pair{\astore}{\aheap}$ (the same reasoning can be done for $\pair{\astore'}{\aheap'}$)
First, from (1) and (2) it holds that for every term $\aterm \in \atermset{\asetvar \cup \{\avariableter\}}$,
$\pair{\astore}{\aheap} \models \aterm = \avariableter$ or there is $\aterm' \in \atermset{\asetvar}$ such that
$\pair{\astore}{\aheap} \models \aterm = \aterm'$.
Hence, by axioms~\ref{core2Ax:SeesTermEq} and~\ref{core2Ax:SeesRef}
from $\pair{\astore}{\aheap} \models \aformulater$ we conclude that
\begin{nscenter}
$\pair{\astore}{\aheap} \models \sees{\aterm_1}{\avariableter}{\atermset{\asetvar \cup \{\avariableter\}}}{\sim_1}{\inbound_1} \land \sees{\avariableter}{\aterm_2}{\atermset{\asetvar \cup \{\avariableter\}}}{\sim_2}{\inbound_2}
\land \avariableter \not\in\{\aterm_1,\aterm_2\}$.
\end{nscenter}
Moreover, again from (1) and (2)
there is a bijection $\amapbis: \symbterms_{\asetvar \cup \{\avariableter\}} \setminus \{\equivclass{\avariableter}{\symbterms_{\asetvar \cup \{\avariableter\}}} \to  \symbterms_{\asetvar}$
such that for every $\asetmeetvar \in \symbterms_{\asetvar \cup \{\avariableter\}} \setminus \{\equivclass{\avariableter}{\symbterms_{\asetvar \cup \{\avariableter\}}}$,
$\amapbis(\asetmeetvar) \subseteq \asetmeetvar$.
Then, by definition of symbolic memory state, we can show that for every term $\aterm \in \atermset{\asetvar \cup \{\avariableter\}}$,
\begin{itemize}
\item if $\equivclass{\aterm}{\symbterms_{\asetvar \cup \{\avariableter\}}} \neq \equivclass{\aterm_1}{\symbterms_{\asetvar \cup \{\avariableter\}}}$ and
$\equivclass{\aterm}{\symbterms_{\asetvar \cup \{\avariableter\}}} \neq \equivclass{\avariableter}{\symbterms_{\asetvar \cup \{\avariableter\}}}$, then
$\amap_{\asetvar \cup \{\avariable\}}(\equivclass{\aterm'}{\symbterms_{\asetvar\cup\{ \avariableter \}}}) = \amap_{\asetvar}(\equivclass{\aterm'}{\symbterms_{\asetvar}})$
where $\aterm' \in \amapbis(\equivclass{\aterm}{\symbterms_{\asetvar\cup\{ \avariableter \}}})$;
\item if $\equivclass{\aterm}{\symbterms_{\asetvar \cup \{\avariableter\}}} = \equivclass{\aterm_1}{\symbterms_{\asetvar \cup \{\avariableter\}}}$ then
$\amap_{\asetvar \cup \{\avariable\}}(\equivclass{\aterm}{\symbterms_{\asetvar\cup\{ \avariableter \}}}) = \pair{\equivclass{\avariableter}{\symbterms_{\asetvar \cup \{\avariableter\}}}}{\inbound_1}$;
\item if $\equivclass{\aterm}{\symbterms_{\asetvar \cup \{\avariableter\}}} = \equivclass{\avariableter}{\symbterms_{\asetvar \cup \{\avariableter\}}}$,
$\amap_{\asetvar \cup \{\avariable\}}(\equivclass{\aterm}{\symbterms_{\asetvar\cup\{ \avariableter \}}}) = \pair{\equivclass{\aterm_2}{\symbterms_{\asetvar \cup \{\avariableter\}}}}{\inbound_2}$.
\end{itemize}
As $\symbterms_{\asetvar} = \symbterms_{\asetvar}'$ and $\symbterms_{\asetvar \cup \{\avariableter\}} = \symbterms_{\asetvar \cup \{\avariableter\}}'$, we can use the same $\amapbis$
and conclude a similar statement for $\pair{\astore'}{\aheap'}$.
Again from $\amap_{\asetvar} = \amap_{\asetvar}'$, we conclude that
$\amap_{\asetvar\cup\{ \avariableter \}} = \amap_{\asetvar\cup\{ \avariableter \}}'$. \qedhere
\end{description}
\end{proof}

\begin{lemma}\label{lemma:existscoretypeelim}
  Let $\bound \in \Nat^+$ and $\asetvar \subset_\fin \PVAR$ be such that $\avariableter \not\in \asetvar \supseteq \{\avariable,\avariablebis\}$.
  Let $\aformula \in \coretype{\asetvar\cup\{\avariableter\}}{\bound}$ be a satisfiable core type such that
  \begin{enumerate}[label=\textbf{\textsf{\alph*.}}]
  \item $\aformula$ is satisfiable;
  \item $\sees{\avariable}{\avariablebis}{\emptyset} \inside \aformula$;
  \item $\threeorliterals{\avariable = \avariableter}{\avariablebis = \avariableter}{\lnot \sees{\avariable}{\avariablebis}{\{\avariable,\avariableter,\avariablebis\}}} \inside \aformula$.
  \end{enumerate}
  Then,
  \begin{enumerate}
  \item if there is $\aterm \in \atermset{\asetvar}$ such that $\avariableter = \aterm \inside \aformula$ then there is $\aformulabis \in \conjcomb{\coreformulae{\asetvar}{\bound}}$ such that
  $\prove_{\coresys(\weirdexists)}   \inpath{\avariable}{\avariablebis}{\avariableter} \aformula \iff
   \aformulabis$.
  \item Otherwise (i.e.\ for every  $\aterm \in \atermset{\asetvar}$,
  $\avariableter \neq \aterm \inside \aformula$), there is $\aformulabis \in  \conjcomb{\coreformulae{\asetvar}{2\bound}}$
  such that
  $\prove_{\coresys(\weirdexists)}   \inpath{\avariable}{\avariablebis}{\avariableter} \aformula \iff
     \aformulabis$.
  \end{enumerate}
\end{lemma}

\begin{proof}
Recall that $\coresys$ is sound and complete for Boolean combinations of core formulae (Theorem~\ref{theo:core2PSLcompl}).
We start by the following property, which allows us to apply Lemma~\ref{lemma:deterministicexistentialcompletion} during the construction:
there are two terms
$\aterm_1,\aterm_2 \in \atermset{\asetvar}$ such that
  \begin{enumerate}[label=\textbf{\textsf{\Roman*.}}]
    \item $\sees{\aterm_1}{\aterm_2}{\atermset{\asetvar}} \inside \aformula$;
    \item $\threeorliterals{\aterm_1 = \avariableter}{\aterm_2 = \avariableter}{\lnot \sees{\aterm_1}{\aterm_2}{\{\avariableter\}}} \inside \aformula$.
  \end{enumerate}
This holds from the hypothesis (b)--(c).
We reason semantically, knowing that then the result holds syntactically from Theorem~\ref{theo:core2PSLcompl} and the fact that $\aformula$ is a satisfiable core type.
Suppose $\pair{\astore}{\aheap} \models \aformula$.
Then, from (b) there is a path of length at least one from $\astore(\avariable)$ to $\astore(\avariablebis)$.
From (c), $\astore(\avariableter)$ is a location inside this path.
If $\astore(\avariable) = \astore(\avariableter)$, then (I) and (II) hold for $\aterm_1 = \avariable$ and $\aterm_2$ be such that $\pair{\astore}{\aheap} \models \sees{\aterm_1}{\aterm_2}{\atermset{\asetvar}}$ , which exists by Lemma~\ref{lemma:firstseesterm}.
Otherwise ($\astore(\avariable) \neq \astore(\avariableter)$),
let us consider $\aterm_1$ as the term in $\atermset{\asetvar}$ corresponding to the closest location reaching in at least one step $\astore(\avariableter)$ that is also reached by $\astore(\avariable)$ (it can be that this location is $\astore(\avariable)$).
Similarly, let $\aterm_2$ be the term in $\atermset{\asetvar}$ corresponding to the closest location reachable from $\astore(\avariableter)$, that reaches $\astore(\avariablebis)$ (it can be that this location is $\astore(\avariableter)$ or $\astore(\avariablebis)$).
It is easy to show that both (I) and (II) holds, where the first property again is from Lemma~\ref{lemma:firstseesterm}.

We split the proof into two cases (1) and (2), as in the statement of the lemma.
\begin{enumerate}
\item Suppose $\aformula$ as in the hypothesis, and moreover that there is $\aterm \in \atermset{\asetvar}$ such that $\avariableter = \aterm \inside \aformula$.
Then by (I), (II) and Lemma~\ref{lemma:deterministicexistentialcompletion}, the formula $\aformulabis \egdef \bigwedge\{ \aformulater \inside \aformula \mid \aformulater \in \coreformulae{\asetvar}{\bound}\}$ is such that
\begin{nscenter}
$\prove_{\coresys} (\avariableter = \aterm \land \aformulabis) \iff \aformula$
\end{nscenter}
Hence by \ref{rule:wierdexistsinference},
\begin{nscenter}
$\prove_{\coresys(\weirdexists)} \inpath{\avariable}{\avariablebis}{\avariableter} \aformula \iff \inpath{\avariable}{\avariablebis}{\avariableter} (\avariableter = \aterm \land \aformulabis)$.
\end{nscenter}
By definition the variable $\avariableter$ does not appear in $\aformulabis$ and by using axiom~\ref{existsAx:Conjunction},
we obtain the following proof:
\begin{nscenter}
$\prove_{\coresys(\weirdexists)}  \inpath{\avariable}{\avariablebis}{\avariableter} (\avariableter = \aterm \land \aformulabis) \iff (\aformulabis \land \inpath{\avariable}{\avariablebis}{\avariableter} \avariableter = \aterm)$
\end{nscenter}
To conclude the proof, we then just need to show that $\prove_{\coresys} \aformulabis \implies \inpath{\avariable}{\avariablebis}{\avariableter} \avariableter = \aterm$.
Indeed, if this is the case, then by propositional calculus we obtain a proof of
\begin{nscenter}
 $\prove_{\coresys} \aformulabis \iff (\aformulabis \land \inpath{\avariable}{\avariablebis}{\avariableter} \avariableter = \aterm)$
\end{nscenter}
and therefore, putting together the derivations above, we conclude that
\begin{nscenter}
$\prove_{\coresys} \inpath{\avariable}{\avariablebis}{\avariableter} \aformula \iff \aformulabis$
\end{nscenter}
ending the proof of (1). Therefore, let us show that $\prove_{\coresys} \aformulabis \implies \inpath{\avariable}{\avariablebis}{\avariableter} \avariableter = \aterm$.
By hypothesis, we have that
\begin{enumerate}[start=2,label=\textbf{\textsf{\alph*.}}]
\item $\sees{\avariable}{\avariablebis}{\emptyset} \inside \aformula$;
\item $\threeorliterals{\avariable = \avariableter}{\avariablebis = \avariableter}{\lnot \sees{\avariable}{\avariablebis}{\{\avariable,\avariableter,\avariablebis\}}} \inside \aformula$.
\end{enumerate}
Then, as $\aformula$ is a core type of $\coreformulae{\asetvar \cup \{\avariableter\}}{\bound}$, and $\avariableter = \aterm \inside \aformula$, we obtain that
\begin{nscenter}
$
\threeorliterals{\avariable = \aterm}{\avariablebis = \aterm}{\lnot \sees{\avariable}{\avariablebis}{\{\avariable,\aterm,\avariablebis\}}} \inside \aformula$.
\end{nscenter}
By definition of $\aformulabis$ we directly conclude that
\begin{enumerate}[start=4,label=\textbf{\textsf{\alph*.}}]
\item $\sees{\avariable}{\avariablebis}{\emptyset} \inside \aformulabis$;
\item $\threeorliterals{\avariable = \aterm}{\avariablebis = \aterm}{\lnot \sees{\avariable}{\avariablebis}{\{\avariable,\aterm,\avariablebis\}}} \inside \aformulabis$.
\end{enumerate}
Then, we prove the derivability of $\aformulabis \implies \inpath{\avariable}{\avariablebis}{\avariableter} \avariableter = \aterm$ by cases on which formula among  $\avariable = \aterm$, $\avariablebis = \aterm$ and
$\lnot\sees{\avariable}{\avariablebis}{\{\avariable,\aterm,\avariablebis\}}$ appears (positively) in $\aformulabis$.
\begin{description}
\item[case $\avariable = \aterm \inside \aformulabis$.]
Then,
\[
\begin{nd}
\hypo {1} {\aformulabis}
\hypo {2} {\avariable = \aterm}
\have {3} {\sees{\avariable}{\avariablebis}{\emptyset}} \by{$\sees{\avariable}{\avariablebis}{\emptyset} \inside \aformulabis$, (d)}{1}
\have {4} {\inpath{\avariable}{\avariablebis}{\avariableter}\ \avariableter = \avariable} \by{\ref{existsAx:ZeroStep}}{3}
\have {5} {\inpath{\avariable}{\avariablebis}{\avariableter}\ (\avariableter = \avariable \land \avariable = \aterm)} \by{\ref{existsAx:Conjunction}, as $\avariableter \not \in \chars{\avariable,\aterm}$}{2,4}
\have {6} {\inpath{\avariable}{\avariablebis}{\avariableter}\ \avariableter = \aterm} \by{\ref{core2Ax:Substitute} and
\ref{rule:wierdexistsinference}}{5}
\end{nd}
\]
\item[case $\avariablebis = \aterm \inside \aformulabis$.]
Then,
\[
\begin{nd}
\hypo {1} {\aformulabis}
\hypo {2} {\avariablebis = \aterm}
\have {2b} {\sees{\avariable}{\avariablebis}{\emptyset}} \by{$\sees{\avariable}{\avariablebis}{\emptyset} \inside \aformulabis$, (d)}{1}
\have {3} {\sees{\avariable}{\aterm}{\emptyset}} \by{\ref{core2Ax:Substitute}}{2,2b}
\have {4} {\sees{\avariable}{\aterm}{\{\avariable,\aterm\}}} \by{\ref{core2Ax:SeesRef}}{3}
\have {5} {\sees{\avariable}{\aterm}{\{\aterm\}}} \by{\ref{core2Ax:SeesMono1}}{4}
\have {6} {\sees{\avariable}{\aterm}{\{\avariablebis,\aterm\}}} \by{\ref{core2Ax:SeesTermEq}}{2,5}
\have {7} {\sees{\avariable}{\aterm}{\{\avariablebis\}}} \by{\ref{core2Ax:SeesMono1}}{6}
\have {8} {
\inpath{\avariable}{\avariablebis}{\avariableter}\ \avariableter = \aterm} \by{\ref{existsAx:AtLeastOneStep}}{2b,7}
\end{nd}
\]
\item[case $\lnot \sees{\avariable}{\avariablebis}{\{\aterm\}} \inside \aformulabis$.]
Then,
\[
\begin{nd}
\hypo {1} {\aformulabis}
\hypo {2} {\lnot \sees{\avariable}{\avariablebis}{\{\aterm\}}}
\have {3} {\sees{\avariable}{\avariablebis}{\emptyset}} \by{$\sees{\avariable}{\avariablebis}{\emptyset} \inside \aformulabis$, (d)}{1}
\have {4} {\sees{\avariable}{\avariablebis}{\{\avariable,\avariablebis\}}} \by{\ref{core2Ax:SeesRef}}{3}
\have {5} {\sees{\avariable}{\avariablebis}{\{\avariablebis\}}} \by{\ref{core2Ax:SeesMono1}}{4}
\have {10} {\sees{\avariable}{\aterm}{\{\avariablebis\}}} \by{\ref{core2Ax:SeesNegSum}}{2,5}
\have {11} {\inpath{\avariable}{\avariablebis}{\avariableter}\ \avariableter = \aterm} \by{\ref{existsAx:AtLeastOneStep}}{3,10}
\end{nd}
\]
\end{description}
\item Let us now focus on the second case of the statement. The proof is very similar to the first case. Suppose $\aformula$ as in the hypothesis, and moreover that for every  $\aterm \in \atermset{\asetvar}$,
$\avariableter \neq \aterm \inside \aformula$.
Let $\aterm_1$ and $\aterm_2$ be the two terms in $\atermset{\asetvar}$ such that $\threeorliterals{\aterm_1 = \avariableter}{\aterm_2 = \avariableter}{\lnot \sees{\aterm_1}{\aterm_2}{\{\avariableter\}}} \inside \aformula$ (their existence holds directly by (II)).
From the hypothesis that for all $\aterm \in \atermset{\asetvar}$,
$\avariableter \neq \aterm \inside \aformula$, it must hold that
\begin{nscenter}
$\sees{\aterm_1}{\aterm_2}{\atermset{\asetvar}} \land \lnot \sees{\aterm_1}{\aterm_2}{\atermset{\asetvar} \cup \{\avariableter\}} \inside \aformula$.
\end{nscenter}
Then by Lemma~\ref{lemma:deterministicexistentialcompletion}
there are $\inbound_1,\inbound_2 \in \interval{1}{\bound}$ such that
\begin{itemize}
\item $\seesgeq{\aterm_1}{\avariableter}{\atermset{\asetvar}}{\inbound_1} \land \seesgeq{\avariableter}{\aterm_2}{\atermset{\asetvar}}{\inbound_2} \inside \aformula$;
\item $\seesgeq{\aterm_1}{\avariableter}{\atermset{\asetvar}}{\inbound_1+1} \not\inside \aformula$ and $\seesgeq{\avariableter}{\aterm_2}{\atermset{\asetvar}}{\inbound_2+1} \not\inside \aformula$.
\end{itemize}
Let $\sim_1,\sim_2\in\{\geq,=\}$ s.t. for every $i \in \{1,2\}$, $\sim_i$ is $=$ iff $\inbound_i < \bound$.
Then (again Lemma~\ref{lemma:deterministicexistentialcompletion})
\begin{nscenter}
$\prove_{\coresys} (\sees{\aterm_1}{\avariableter}{\atermset{\asetvar}}{\sim_1}{\inbound_1} \land \sees{\avariableter}{\aterm_2}{\atermset{\asetvar}}{\sim_2}{\inbound_2}
 \land \avariableter \not\in\{\aterm_1,\aterm_2\} \land \aformulabis) \iff \aformula$.
\end{nscenter}
where, again, $\aformulabis \egdef \bigwedge\{ \aformulater \inside \aformula \mid \aformulater \in \coreformulae{\asetvar}{\bound}\}$.
Now, if $\sim_1$ or $\sim_2$ is $\geq$, then we can apply the axiom~\ref{core2Ax:SeesSum}, whereas if $\sim_1$ and $\sim_2$ are both $=$ then we can apply the auxiliary tautology~\ref{axiom2:seeslengthsum}, in order to derive:
\begin{nscenter}
$\prove_{\coresys} \sees{\aterm_1}{\avariableter}{\atermset{\asetvar}}{\sim_1}{\inbound_1} \land \sees{\avariableter}{\aterm_2}{\atermset{\asetvar}}{\sim_1}{\inbound_2} \implies
 \sees{\aterm_1}{\aterm_2}{\atermset{\asetvar}}{\sim}{\inbound_1{+}\inbound_2}$.
\end{nscenter}
Hence, by propositional calculus, the formula
\begin{nscenter}
$\sees{\aterm_1}{\avariableter}{\atermset{\asetvar}}{\sim_1}{\inbound_1} \land \sees{\avariableter}{\aterm_2}{\atermset{\asetvar}}{\sim_2}{\inbound_2} \land \avariableter \not\in\{\aterm_1,\aterm_2\} \land \aformulabis$
\end{nscenter}
can be proved in $\coresys$ to be equivalent to the formula $\aformulater$ defined as
\begin{nscenter}
$\sees{\aterm_1}{\avariableter}{\atermset{\asetvar}}{\sim_1}{\inbound_1} \land \sees{\avariableter}{\aterm_2}{\atermset{\asetvar}}{\sim_2}{\inbound_2} \land
\land \sees{\aterm_1}{\aterm_2}{\atermset{\asetvar}}{\sim}{\inbound_1{+}\inbound_2}
\land
\avariableter \not\in\{\aterm_1,\aterm_2\} \land \aformulabis$
\end{nscenter}
Notice that $\sees{\aterm_1}{\aterm_2}{\atermset{\asetvar}}{\sim}{\inbound_1{+}\inbound_2}$ is a core formulae from $\coreformulae{\asetvar}{2\bound}$.

As done in the previous case of the proof, by~\ref{rule:wierdexistsinference} we deduce that
\begin{nscenter}
$\prove_{\coresys} \inpath{\avariable}{\avariablebis}{\avariableter} \aformula \iff  \inpath{\avariable}{\avariablebis}{\avariableter} \aformulater$
\end{nscenter}
Moreover, by the axiom~\ref{existsAx:Conjunction}
we obtain a proof of
\begin{nscenter}
$\prove_{\coresys} \inpath{\avariable}{\avariablebis}{\avariableter} \aformulater \iff
\begin{aligned}[t]
&\sees{\aterm_1}{\aterm_2}{\atermset{\asetvar}}{\sim}{\inbound_1{+}\inbound_2} \land \aformulabis \land\\ &\inpath{\avariable}{\avariablebis}{\avariableter}(
\sees{\aterm_1}{\avariableter}{\atermset{\asetvar}}{\sim_1}{\inbound_1} \land \sees{\avariableter}{\aterm_2}{\atermset{\asetvar}}{\sim_2}{\inbound_2} \land
\avariableter \not\in\{\aterm_1,\aterm_2\})
\end{aligned}$
\end{nscenter}
Therefore (again, similarly to what is done in the first case of the proof), to end the proof it is sufficient to prove that
\begin{nscenter}
$\prove_{\coresys(\weirdexists)} \sees{\aterm_1}{\aterm_2}{\atermset{\asetvar}}{\sim}{\inbound_1{+}\inbound_2} \land \aformulabis \implies \inpath{\avariable}{\avariablebis}{\avariableter}
(\sees{\aterm_1}{\avariableter}{\atermset{\asetvar}}{\sim_1}{\inbound_1} \land \sees{\avariableter}{\aterm_2}{\atermset{\asetvar}}{\sim_2}{\inbound_2} \land
\avariableter \not\in\{\aterm_1,\aterm_2\})$
\end{nscenter}
Briefly, this follows by applying the axiom~\ref{existsAx:Split}, where the conditions in the antecedents of the axiom
$({\avariable} {=} {\aterm_1} \lor \sees{\avariable}{\aterm_1}{\asetmeetvar'} ) \land
({\aterm_2}{=}{\avariablebis} \lor \sees{\aterm_2}{\avariablebis}{\asetmeetvar''})\land(\avariablebis {=} \aterm_1 \implies \avariable{=} \avariablebis)$, with $\{\avariable,\avariablebis,\aterm_1,\aterm_2\} \in \asetmeetvar' \cap \asetmeetvar''$
are easily provable to be implied by $\aformulabis$, and more precisely from
\begin{nscenter}
$\sees{\avariable}{\avariablebis}{\emptyset} \land \lnot \sees{\avariable}{\avariablebis}{\{\avariable,\avariableter,\avariablebis\}} \land
\sees{\aterm_1}{\aterm_2}{\atermset{\asetvar}}
\land \lnot \sees{\aterm_1}{\aterm_2}{\atermset{\asetvar} \cup \{\avariableter\}} \inside \aformula$
\end{nscenter}
which informally implies that models of $\aformulabis$ (and $\aformula$) must have a path from $\astore(\avariable)$ to $\astore(\avariablebis)$ of the form:
\begin{center}
 \scalebox{0.85}{
     \begin{tikzpicture}[baseline]
       \node[dot,label=above:$\avariable$] (i) at (0,0) {};
       \node[dot,label=above:{$\aterm_1$}] (m) [right = 2cm of i] {};
       \node[dot,label=above:$\aterm_2$] (j) [right=2cm of m] {};
       \node[dot,label=above:{$\avariable$}] (k) [right=2cm of j] {};

       \draw[reach] (i) -- (m);
       \draw[pto] (m) to node [below] {$+$} (j);
       \draw[reach] (j) -- (k);
     \end{tikzpicture}
 }
\end{center}
\qedhere
\end{enumerate}
\end{proof}

\lemmaaxiomseliminateexists*

\begin{proof}
Let $\aformula \in \boolcomb{\coreformulae{\asetvar \cup \{\avariableter\}}{\bound}}$ with $\avariableter \not \in \asetvar \supseteq \{\avariable,\avariablebis\}$.
By propositional calculus, exactly as done in Lemma~\ref{prop:corePSLone},
there is a disjunction $\aformulabis=\aformula_1\vee\cdots\vee\aformula_n$ of core types
such that $\prove_{\coresys} \aformula\Leftrightarrow\aformulabis$.
Then, by the rule~\ref{rule:wierdexistsinference},
$\prove_{\coresys(\weirdexists)} \inpath{\avariable}{\avariablebis}{\avariableter} \aformula \iff \inpath{\avariable}{\avariablebis}{\avariableter} \left(\bigvee_{i \in \interval{1}{n}} \aformula_i\right)$.
We can now apply axiom~\ref{existsAx:Disjunction} to obtain a proof of $ \inpath{\avariable}{\avariablebis}{\avariableter} \aformula \iff \bigvee_{i \in \interval{1}{n}} \inpath{\avariable}{\avariablebis}{\avariableter} \aformula_i$.
We now consider each core type in $\{ \aformula_i \mid i \in \interval{1}{n}\}$. There are three cases:
\begin{itemize}
\item If $\aformula_i$ is unsatisfiable then by Lemma~\ref{lemma:axiomtwoRCct} $\prove_{\coresys} \aformula_i \implies \bottom$.
Then by the axiom~\ref{existsAx:Bottom} and the rule~\ref{rule:wierdexistsinference},  we obtain
$\prove_{\coresys(\weirdexists)} \inpath{\avariable}{\avariablebis}{\avariableter} \aformula_i \implies \bottom$.
\item If $\lnot \sees{\avariable}{\avariablebis}{\emptyset} \inside \aformula_i$ or $\threeandliterals{\avariable = \avariableter}{\avariablebis = \avariableter}{\lnot \sees{\avariable}{\avariablebis}{\{\avariable,\avariableter,\avariablebis\}}} \inside \aformula_i$, then by axiom \ref{existsAx:SeesSem}
again we obtain
$\prove_{\coresys(\weirdexists)} \inpath{\avariable}{\avariablebis}{\avariableter} \aformula_i \implies \bottom$.
\item Suppose instead $\aformula_i$ satisfiable and such that
$\sees{\avariable}{\avariablebis}{\emptyset} \inside \aformula_i$ and
$\threeorliterals{\avariable = \avariableter}{\avariablebis = \avariableter}{\lnot \sees{\avariable}{\avariablebis}{\{\avariable,\avariableter,\avariablebis\}}} \inside \aformula_i$.
Then by Lemma~\ref{lemma:existscoretypeelim} there is a formula $\aformulater_i \in \conjcomb{\coreformulae{\asetvar}{2\bound}}$
such that $\prove_{\coresys(\weirdexists)} \inpath{\avariable}{\avariablebis}{\avariableter} \aformula_i \implies \aformulater_i$.
Then again, by propositional calculus (as done in Lemma~\ref{prop:corePSLone}), there is a Boolean combination $\overline{\aformulater_i}$ of core types from $\coretype{\asetvar}{2\bound}$ such that $\prove_{\coresys} \aformulater_i \iff \overline{\aformulater_i}$.
\end{itemize}
Hence, $\bigvee_{i \in \interval{1}{n}} \inpath{\avariable}{\avariablebis}{\avariableter} \aformula_i$ can be shown equivalent in $\coresys(\weirdexists)$ to a Boolean combination of core formulae $\aformulater \in \boolcomb{\coreformulae{\asetvar}{2\bound}}$. As
$\prove_{\coresys(\weirdexists)} \inpath{\avariable}{\avariablebis}{\avariableter} \aformula \iff \bigvee_{i \in \interval{1}{n}} \inpath{\avariable}{\avariablebis}{\avariableter} \aformula_i$ (from above), we conclude that
$\prove_{\coresys(\weirdexists)} \inpath{\avariable}{\avariablebis}{\avariableter} \aformula \iff \aformulater$, which proves the lemma.
\end{proof}
