# Supplementary material for: A Complete Axiomatisation for Quantifier-Free Separation Logic
Source: arXiv:2006.05156 source file (2021-08-09)
Supplement: Supplementary file 8 [file proof-lemma-axiomstwo-RCchar.tex]

We want to prove that $\coresys$ is sound and complete with respect to core types. Formally,

\lemmaaxiomtwoRCct*
We recall that a core type for $\pair{\asetvar}{\bound}$ is a formula of the set
\begin{nscenter}
$\coretype{\asetvar}{\bound}
\egdef
\scaledformulasubset{
 \aformula \in \conjcomb{\coreformulae{\asetvar}{\bound}}
}{
 \bmat[
   \forall\aformulabis{\in} \coreformulae{\asetvar}{\bound}, \orliterals{\aformulabis}{\lnot \aformulabis} \inside \aformula, \text{ and } (\aformulabis \land \lnot \aformulabis) \not\inside \aformula
 ]
}{0.9}{1}$.
\end{nscenter}
The proof of completeness is involved and heavily uses the notion of characteristic formulae.
Mainly, the proof is divied in the following steps:
\begin{enumerate}
\item First, we show that the system is sound and complete for characteristic formulae (Lemma~\ref{lemma:axiomstwoRCchars}).
This proof, despite using standard techniques, is technically involved and uses most of the syntactical derivations shown in Appendix~\ref{appendix:DerivedTautologies}.
\item Second, we show that every satisfiable characteristic formula $\charsymbform(\asms)$ of a symbolic memory state $\asms$ over
$\pair{\asetvar}{\bound}$ is provably equivalent in $\coresys$ to exactly one core type in $\coretype{\asetvar}{\bound}$:
$\charsymbform(\asms)$ is as informative as the core type.
This is done in Lemma~\ref{corr:typeuniquesymb}, which relies on intermediate lemmata (from Lemma~\ref{lemma:closingsees} to  Lemma~\ref{lemma:charsubsettype}).
\item Lastly, from the two previous point we prove Lemma~\ref{lemma:axiomtwoRCct}.
\end{enumerate}
Let us be a little more precise on the second point of the proof.
We said that a characteristic formula is as informative as a core type.
For example, going back to the definition of characteristic formulae, we notice
that every literal involving the predicate $\mathtt{sees}$ has the index $\atermset{\asetvar}$.
Recall that if $\seesgeq{\aterm_1}{\aterm_2}{\atermset{\asetvar}}{\inbound} \inside \charsymbform(\asms)$, then in every memory state $\pair{\astore}{\aheap}$ satisfying $\charsymbform(\asms)$, there is a path of length at least $\inbound$ from $\semantics{\aterm_1}_{\astore,\aheap}$ to  $\semantics{\aterm_2}_{\astore,\aheap}$
without passing through elements assigned to $\atermset{\asetvar}$.
Such a memory state satisfies $\seesgeq{\aterm_1}{\aterm_2}{\asetmeetvar}\inbound$ for every
 $\asetmeetvar\subseteq \atermset{\asetvar}$.
%% (see also the axiom~\ref{core2Ax:SeesMono1}).
From a characteristic formula, we can then derive core formulae until we obtain a core type.
The converse also holds: given a core type, we can derive a characteristic formula by removing superfluous literals.
\LongVersionOnly{ (e.g.\ by only keeping $\mathtt{sees}$ predicates indexed by $\terms{\asetvar}$).}
For this reason, the
completeness of $\coresys$ can be shown  by first proving that the system is  complete w.r.t. characteristic formulae (point (1) above).

\subsubsection{Completeness of $\coresys$ for characteristic formulae}

\begin{restatable}{lemma}{lemmaaxiomstwoRCchars}\label{lemma:axiomstwoRCchars}
Let $\asms$ be a symb. memory state over $\pair{\asetvar}{\bound}$.
$\neg \charsymbform(\asms)$ is valid iff $\prove_{\coresys} \neg \charsymbform(\asms)$ where all derivation steps only have formulae in $\boolcomb{\coreformulae{\asetvar}{\bound}}$.
%% $\charsymbform(\asms)$ is unsatisfiable if and only if $\prove_{\coresys} \charsymbform(\asms) \implies \bottom$ where all derivation steps only have formulae in $\boolcomb{\coreformulae{\asetvar}{\bound}}$.
\end{restatable}
\begin{proof}
The ``only if'' part follows from Lemma~\ref{lemma:axiomstwocoresound}, so we just prove the ``if'' part.
Let $\asms$ a symbolic memory state over $\pair{\asetvar}{\bound}$ so that it is not possible to derive in $\coresys$,
the formula  $\charsymbform(\asms)\Rightarrow \bot$, with any proof using derivation step schemata instantiated with formulae from $\coreformulae{\asetvar}{\bound}$.
Let us prove that then
$\aformula \egdef \charsymbform(\asms)$ is satisfiable.
Notice that because of the constraint on the derivation steps, during the proof we need to be careful to use only formulae of $\coreformulae{\asetvar}{\bound}$.

Before beginning the proof, we state some properties of the characteristic formula $\aformula$ that immediately follow from its definition.
\begin{itemize}
\item for every two terms $\aterm_1,\aterm_2 \in \atermset{\asetvar}$, $\orliterals{\aterm_1 = \aterm_2}{\aterm_1 \neq \aterm_2} \inside \aformula$;
\item for every two terms $\aterm_1,\aterm_2 \in \atermset{\asetvar}$,
 $\lnot\sees{\aterm_1}{\aterm_2}{\atermset{\asetvar}} \inside \aformula$ or (otherwise) there is exactly one $\inbound \in \interval{1}{\bound}$ such that
${\seesgeq{\aterm_1}{\aterm_2}{\atermset{\asetvar}}{\inbound}} \inside \aformula$. Moreover, in the second case, if $\inbound < \bound$ then
$\lnot \seesgeq{\aterm_1}{\aterm_2}{\atermset{\asetvar}}{\inbound{+}1} \inside \aformula$.
For the same $\aterm_1,\aterm_2$, no other $\lnot\seesgeq{\aterm_1}{\aterm_2}{\asetmeetvar}{\inbound'}$ belongs to $\literals{\aformula}$.
\item there is exacly one $\inbound \in \interval{0}{\bound}$ such that
$\remgeq{\atermset{\asetvar}\times\atermset{\asetvar}}{\inbound} \inside \aformula$, and if $\inbound < \bound$ then $\lnot
\remgeq{\atermset{\asetvar}\times\terms{\asetvar}}{\inbound{+}1} \inside \aformula$.
No other $\lnot\remgeq{\asetpath}{\inbound'}$ is in $\literals{\aformula}$.
\end{itemize}

During the proof, we write ``\elseabsurd{(statement$_1$)}{(statement$_2$)}'' as a shortcut for
\begin{nscenter}
``if (statement$_2$) does not hold then $\prove_{\coresys} \aformula\Rightarrow \bot$ by (statement$_1$), contradiction''.
\end{nscenter}
For example, ``\elseabsurd{axioms~\ref{core2Ax:Self} and~\ref{core2Ax:Substitute}}{for every $\avariable \in \asetvar$, $\avariable = \avariable \inside \aformula$}'' is a shortcut for
``if (for every $\avariable \in \asetvar$, $\avariable = \avariable \inside \aformula$) does not hold then $\prove_{\coresys} \aformula\Rightarrow \bot$ by (axioms~\ref{core2Ax:Self} and~\ref{core2Ax:Substitute}),
 contradiction''.
Often, to be completely precise, in (statement$_1$) we should write that we also need propositional calculus. However, if we use classical reasoning in a trivial way, this is omitted.
For instance, the statement provided above as an example is proved as follows:
\[
\begin{nd}
\hypo {0} {\true}
\have {1} {\avariable = \ameetvar{\avariable}{\avariable}{\avariable}} \by{\ref{core2Ax:Self}}{}
\have {2} {\avariable = \ameetvar{\avariable}{\avariable}{\avariable} \land \avariable = \ameetvar{\avariable}{\avariable}{\avariable}} \by{$\aformula \implies \aformula \land \aformula$}{1}
\have {3} {\avariable = \avariable} \by{\ref{core2Ax:Substitute}}{2}
\end{nd}
\]
Hence, we clearly need propositional calculus to prove that for every $\avariable \in \asetvar$, $\avariable = \avariable \inside \aformula$. However, in (statement$_1$), we prefer to focus on the axioms of $\coresys$.
In this way, we hope to improve the readability of the proof, which is mainly composed of a series of results shown by contradiction.
The proof is divided into multiple steps, identified by numbers (and a small $\boxed{\text{title}}$).
So, the readed should refer to these identifiers when we say, for example, ``from the previous point of the proof''.
Lastly, in this proof we heavily rely on the auxiliary tautologies proved in Section~\ref{appendix:DerivedTautologies}.
We start the proof by studying the equivalence between terms. Recall that, as said above, for all terms $\aterm_1,\aterm_2 \in \terms{\asetvar}$, $\orliterals{\aterm_1 = \aterm_2}{\aterm_1 \neq \aterm_2} \inside \aformula$.
\begin{enumerate}
\item $\boxed{\text{Equiv. relation}}$ \elseabsurd{axioms~\ref{core2Ax:Self} and~\ref{core2Ax:Substitute}}{for every $\avariable \in \asetvar$, $\avariable = \avariable \inside \aformula$}. The proof is given just above. Moreover,
\elseabsurd{axioms~\ref{core2Ax:EqSymm} and~\ref{core2Ax:Substitute}}{there is an equivalence relation $\approx$ on the \emph{defined terms} of $\terms{\asetvar}$, i.e. the set of terms $\{\aterm \mid \aterm = \aterm \inside \aformula\}$, such that
$\aterm_1\approx\aterm_2$ iff $\aterm_1=\aterm_2$ occurs positively
in $\aformula$}
We write $[\aterm]$ to denote the equivalence class of $\aterm$
with respect to $\approx$. As for every variable $\avariable \in \asetvar$ it holds that $\avariable \approx \ameetvar{\avariable}{\avariable}{\avariable}$ (by axiom~\ref{core2Ax:Self}), when possible we reason exclusively with meet-points, knowing that a similar reasoning can be trivially adapted for variables.
\item\label{proofcomp:point2} $\boxed{\text{Order of a variable}}$ We now focus on one variable $\avariable \in \asetvar$ and one \emph{defined} meet-point $\ameetvar{\avariable}{\avariablebis}{\avariableter}$, i.e. a meet-point such that $\ameetvar{\avariable}{\avariablebis}{\avariableter} \approx \ameetvar{\avariable}{\avariablebis}{\avariableter}$.
Notice that $\avariable$ appears in the ``first position'' of $\ameetvar{\avariable}{\avariablebis}{\avariableter}$.
\elseabsurd{(\ref{axiom2:auxlemma3})}{$\avariable \approx \ameetvar{\avariable}{\avariablebis}{\avariableter}$ or $\before{\avariable}{\ameetvar{\avariable}{\avariablebis}{\avariableter}}\inside \aformula$}
Moreover, \elseabsurd{the tautology~\ref{axiom2:auxlemma11}}{if $\ameetvar{\avariable}{\avariablebis}{\avariableter} \approx \ameetvar{\avariablefour}{\avariablefifth}{\avariablesix}$ then the following meet-points are all in the same equivalence class: $\ameetvar{\avariable}{\avariablebis}{\avariableter}$,
$\ameetvar{\avariable}{\avariablebis}{\avariablesix}$,
$\ameetvar{\avariablefour}{\avariablefifth}{\avariableter}$,
$\ameetvar{\avariablefour}{\avariablefifth}{\avariablesix}$}

Consider now the set of defined meet-points $M_\avariable = \{\ameetvar{\avariable}{\avariablebis}{\avariableter} \mid \avariablebis,\avariableter \in \asetvar\ \text{and}\ \ameetvar{\avariable}{\avariablebis}{\avariableter} \approx \ameetvar{\avariable}{\avariablebis}{\avariableter} \}$.
Notice that $M_\avariable$ contains one element of the equivalence class of $\avariable$, as $\avariable \approx \ameetvar{\avariable}{\avariable}{\avariable}$ (from axiom~\ref{core2Ax:Self}) and then
\elseabsurd{\ref{core2Ax:Substitute}}{$\ameetvar{\avariable}{\avariable}{\avariable} \approx \ameetvar{\avariable}{\avariable}{\avariable}$}.
Indeed, this last statement is proved by showing $\ameetvar{\avariable}{\avariable}{\avariable} = \ameetvar{\avariable}{\avariable}{\avariable} \inside \aformula$:
\[
\begin{nd}
\hypo {0} {\true}
\have {1} {\avariable = \ameetvar{\avariable}{\avariable}{\avariable}} \by{\ref{core2Ax:Self}}{}
\have {2} {\avariable = \ameetvar{\avariable}{\avariable}{\avariable} \land \avariable = \ameetvar{\avariable}{\avariable}{\avariable}} \by{\landtwo}{1}
\have {3} {\ameetvar{\avariable}{\avariable}{\avariable} = \ameetvar{\avariable}{\avariable}{\avariable}} \by{\ref{core2Ax:Substitute}}{2}
\end{nd}
\]
In Section~\ref{subsection-intermediate-tautologies-eq} we proved the proofs of the following properties of $\mathtt{before}$:
\begin{itemize}
\item\ref{axiom2:beforelemma1}:
$\lnot \before{\aterm}{\aterm}$
\item\ref{axiom2:beforelemma2}:
$\before{\aterm_1}{\aterm_2} \implies \lnot \before{\aterm_2}{\aterm_1}$
\item\ref{axiom2:beforelemma3}:
$\before{\aterm_1}{\aterm_2} \land \before{\aterm_2}{\aterm_3} \implies \before{\aterm_1}{\aterm_3}$
\item\ref{axiom2:beforefunc}:
$
\before{\aterm_1}{\aterm_2} {\land} \before{\aterm_1}{\aterm_3} {\land} \aterm_2 {\neq} \aterm_3 \implies \before{\aterm_2}{\aterm_3} \lor \before{\aterm_3}{\aterm_2}
$
\item\ref{axiom2:beforelemma0two}:
$
\before{\aterm_1}{\aterm_2} \land \aterm_2 = \aterm_3 \implies \before{\aterm_1}{\aterm_3}
$
\item\ref{axiom2:beforelemma0}:
$
\before{\aterm_1}{\aterm_2} \land \aterm_1 = \aterm_3 \implies \before{\aterm_3}{\aterm_2}
$
\end{itemize}
\elseabsurd{these six properties and for all $\ameetvar{\avariable}{\avariablebis}{\avariableter} \in M_\avariable, \avariable \approx \ameetvar{\avariable}{\avariablebis}{\avariableter}$ or $\before{\avariable}{\ameetvar{\avariable}{\avariablebis}{\avariableter}}\inside \aformula$ (proved above)}
{there is a total order $>_\avariable$ on $M_\avariable/\approx$, such that $[\ameetvar{\avariable}{\avariablebis}{\avariableter}] >_\avariable [\ameetvar{\avariable}{\avariablefour}{\avariablefifth}]$ if and only if $\before{\ameetvar{\avariable}{\avariablebis}{\avariableter}}{\ameetvar{\avariable}{\avariablefour}{\avariablefifth}} \inside \aformula$}
As the set of terms in $\atermset{\asetvar}$ is finite, we hence proved that there is a finite chain:
\begin{nscenter}
$[\ameetvar{\avariable}{\avariablebis_0}{\avariableter_0}] >_\avariable [\ameetvar{\avariable}{\avariablebis_1}{\avariableter_1}] >_\avariable [\ameetvar{\avariable}{\avariablebis_2}{\avariableter_2}] >_\avariable \dots >_\avariable [\ameetvar{\avariable}{\avariablebis_n}{\avariableter_n}]$
\end{nscenter}
We build the partial function $\pred_\avariable: {M_\avariable/\approx} \to {M_\avariable/\approx}$ that models the predecessor function coherent with $>_\avariable$,
i.e. given an element of $M_\avariable/\approx$ returns the predecessor of that element in the order, if it exists. Formally, for every $\asymbterm_1,\asymbterm_2 \in M_\avariable/\approx$
\begin{nscenter}
$\pred_\asetvar(\asymbterm_1) \egdef \asymbterm_2$ iff $\asymbterm_1 >_\avariable \asymbterm_2$ and there is no $\asymbterm_3 \in M_\avariable/\approx$ such that $\asymbterm_1 >_\avariable \asymbterm_3 >_\avariable \asymbterm_2$.
\end{nscenter}
The order $>_\avariable$ and $\pred_\avariable$ have the following properties (that are later needed):
\begin{enumerate}
\item\label{pathx:1} $[\avariable] = [\ameetvar{\avariable}{\avariablebis_0}{\avariableter_0}]$, as
$\forall \ameetvar{\avariable}{\avariablebis}{\avariableter} \in M_\avariable, \avariable \approx \ameetvar{\avariable}{\avariablebis}{\avariableter}$ or $\before{\avariable}{\ameetvar{\avariable}{\avariablebis}{\avariableter}}\inside \aformula$;
\item\label{pathx:1b} From the definition of $>_\avariable$, given two $\asymbterm_1,\asymbterm_2 \in M_\avariable/\approx$, if $\pred_\avariable(\asymbterm_1)=\asymbterm_2$
then there is no $\asymbterm_3 \in M_\avariable$, $\aterm_1 \in \asymbterm_1$, $\aterm_2 \in \asymbterm_2$ and no $\aterm_3 \in \asymbterm_3$ such that $\before{\aterm_1}{\aterm_3} \land \before{\aterm_3}{\aterm_2} \inside \aformula$, and viceversa.
\item\label{pathx:2} \elseabsurd{axiom~\ref{core2Ax:BothAsym} and~\ref{axiom2:auxlemma7}}{if there is a meet-point $\ameetvar{\avariable}{\avariablebis}{\avariableter} \in M_\avariable$ such that $\asymmetric{\ameetvar{\avariable}{\avariablebis}{\avariableter}} \inside \aformula$
then $[\ameetvar{\avariable}{\avariablebis}{\avariableter}]$ is smallest w.r.t\ $>_\avariable$, i.e.\ $[\ameetvar{\avariable}{\avariablebis_n}{\avariableter_n}]$ in the representation above}
As a result, asymmetric meet-points of $M_\avariable$ are all in the same equivalence class of $\approx$, and all their descendants in $>_\avariable$ are hence symmetric meet-points. Here, we say that $\aterm_1$ is a descendant of $\aterm_2$ iff $[\aterm_1] >_\avariable [\aterm_2]$. We use the term ``descendants'' as we will later use this order to build a tree.
\item\label{pathx:3} \elseabsurd{$\before{\ameetvar{\avariable}{\avariablebis}{\avariableter}}{\ameetvar{\avariable}{\avariablefour}{\avariablefifth}} \implies \defined{\ameetvar{\avariable}{\avariablebis}{\avariablefifth}}$ by definition of $\mathtt{before}$}{%
for every $\ameetvar{\avariable}{\avariablebis}{\avariableter},\ameetvar{\avariable}{\avariablefour}{\avariablefifth}$, if $[\ameetvar{\avariable}{\avariablebis}{\avariableter}] >_{\avariable} [\ameetvar{\avariable}{\avariablefour}{\avariablefifth}]$
then $\ameetvar{\avariable}{\avariablebis}{\avariableter} \approx \ameetvar{\avariable}{\avariablebis}{\avariablefifth}$
}
This means that, given two equivalence classes $\asymbterm_1,\asymbterm_2 \in M_\avariable/\approx$, if $\asymbterm_1 >_\avariable \asymbterm_2$ then the set of subscripts $\{\avariableter \mid \ameetvar{\avariable}{\avariablebis}{\avariableter} \in \asymbterm_1\}$ contains every subscript of $\{\avariablefifth \mid \ameetvar{\avariable}{\avariablefour}{\avariablefifth} \in \asymbterm_2\}$.
Hence, the set of subscripts is weakly increasing when considering descendants in the chain.
\end{enumerate}
We define a similar total order $>_\avariablebis$ and predecessor function $\pred_\avariablebis$ on every variable $\avariablebis \in \asetvar$.
\item\label{proofcomp:point3} $\boxed{\text{Two orders meet}}$ We now consider two distinct variables $\avariable,\avariablebis \in \asetvar$ such that there exists $\avariableter \in \asetvar$ such that $\ameetvar{\avariable}{\avariablebis}{\avariableter}$ is defined and symmetric (i.e. $\symmetric{\ameetvar{\avariable}{\avariablebis}{\avariableter}} \inside \aformula$).

\elseabsurd{\ref{axiom2:auxlemma5}}{for every $\alength \geq 0$, if $\pred_\avariable^\alength([\ameetvar{\avariable}{\avariablebis}{\avariableter}])$ is defined then
$\pred_\avariable^\alength([\ameetvar{\avariable}{\avariablebis}{\avariableter}]) = \pred_\avariablebis^\alength([\ameetvar{\avariable}{\avariablebis}{\avariableter}])$}
Moreover, again \elseabsurd{\ref{axiom2:auxlemma5}}{for every $\avariablefour,\avariablefifth \in \asetvar$, if $[\ameetvar{\avariable}{\avariablebis}{\avariableter}] >_\avariable [\ameetvar{\avariable}{\avariablefour}{\avariablefifth}]$ then $\ameetvar{\avariable}{\avariablefour}{\avariablefifth} \approx \ameetvar{\avariablebis}{\avariablefour}{\avariablefifth}$}
Thank to this property we obtain that,
\begin{itemize}
\item[($\star$)] for every variable $\avariable,\avariablebis,\avariableter,\avariablefour,\avariablefifth,\avariablesix \in \asetvar$,
if $\ameetvar{\avariable}{\avariablebis}{\avariableter} \approx \ameetvar{\avariable}{\avariablefour}{\avariableter}$ and $[\ameetvar{\avariable}{\avariablebis}{\avariableter}] >_\avariable [\ameetvar{\avariable}{\avariablefifth}{\avariablesix}]$
then
$\ameetvar{\avariable}{\avariablefifth}{\avariablesix} \approx \ameetvar{\avariablebis}{\avariablefifth}{\avariablesix} \approx \ameetvar{\avariablefour}{\avariablefifth}{\avariablesix}$.
\end{itemize}
This is an important property that we will recall later.

Continuing the comparison on the orders $>_\avariable$ and $>_\avariablebis$ of $\avariable$ and $\avariablebis$,
\elseabsurd{\ref{axiom2:diffbeforemeet}}{for every element $\asymbterm_1 \in M_\avariable/\approx$ and $\asymbterm_2 \in M_\avariablebis/\approx$, if $\asymbterm_1 >_\avariable [\ameetvar{\avariable}{\avariablebis}{\avariableter}]$ and
$\asymbterm_2 >_\avariablebis [\ameetvar{\avariable}{\avariablebis}{\avariableter}]$ then
$\asymbterm_1 \cap \asymbterm_2 = \emptyset$}
For what we proved so far, we can represent the two orders $>_\avariable$ and $>\avariablebis$ in the following way:
\begin{center}
\scalebox{0.85}{
    \begin{tikzpicture}[baseline]
      \node (a) at (0,0) {$[\avariable]$};
      \node (b) [right = 0.65cm of a] {$[\ameetvar{\avariable}{\avariablefour_1}{\avariableter_1}]$};
      \node (c) [right = 0.65cm of b] {$\dots$};
      \node (d) [right = 0.65cm of c] {$[\ameetvar{\avariable}{\avariablefour_i}{\avariableter_i}]$};
      \node (e) [right = 0.65cm of d] {$[\ameetvar{\avariable}{\avariablebis}{\avariableter}]$};
      \node (f) [right = 0.65cm of e] {$[\ameetvar{\avariable}{\avariablesept_1}{\avariableoct_1}]$};
      \node (g) [right = 0.65cm of f] {$\dots$};
      \node (h) [right = 0.65cm of g] {$[\ameetvar{\avariable}{\avariablesept_k}{\avariableoct_k}]$};

      \node (a1) [below =  0.65cm of a] {$[\avariablebis]$};
      \node (a2) [right =  0.65cm of a1] {$[\ameetvar{\avariablebis}{\avariablefifth_1}{\avariablesix_1}]$};
      \node (a3) [right =  0.65cm of a2] {$\dots$};
      \node (a4) [right =  0.65cm of a3] {$[\ameetvar{\avariablebis}{\avariablefifth_j}{\avariablesix_j}]$};

      \path (a4) -- node[sloped, anchor=center, yshift=-5pt] {$>_\avariablebis$} (e);
      \path (a) -- node {$>_\avariable$} (b);
      \path (b) -- node {$>_\avariable$} (c);
      \path (c) -- node {$>_\avariable$} (d);
      \path (d) -- node {$>_\avariable$} (e);

      \path (a1) -- node {$>_\avariablebis$} (a2);
      \path (a2) -- node {$>_\avariablebis$} (a3);
      \path (a3) -- node {$>_\avariablebis$} (a4);

      \draw[->] (e) -- node[label=above:{$\substack{\pred_\avariable\\ \pred_\avariablebis}$}] {} (f);
      \draw[->] (f) -- node[label=above:{$\substack{\pred_\avariable\\ \pred_\avariablebis}$}] {} (g);
      \draw[->] (g) -- node[label=above:{$\substack{\pred_\avariable\\ \pred_\avariablebis}$}] {} (h);
    \end{tikzpicture}
    }
\end{center}
where different equivalence classes in the drawing are indeed different. Notice that it could be that $\avariable \approx \ameetvar{\avariable}{\avariablebis}{\avariableter}$, resulting the above shape to collapse to a single linear order (i.e. $>_\avariablebis$). Similarly, it could hold that $\avariablebis \approx \ameetvar{\avariable}{\avariablebis}{\avariableter}$ and then the representation above would be equivalent to $>_\avariable$.
\item\label{proofcomp:point4} $\boxed{\text{Trees}}$
We now consider three variables, $\avariable$, $\avariablebis$ and $\avariablefour$ so that, for some $\avariableter \in \asetvar$, we have $\symmetric{\ameetvar{\avariable}{\avariablebis}{\avariableter}} \land \symmetric{\ameetvar{\avariable}{\avariablefour}{\avariableter}} \inside \aformula$.

Then \elseabsurd{\ref{axiom2:auxlemma6}}{$\symmetric{\ameetvar{\avariablebis}{\avariablefour}{\avariableter}} \inside \aformula$}
We consider the three order $>_\avariable$, $>_\avariablebis$, $>_\avariablefour$. The properties expressed in the last point of the proof hold for any two of these orders.
Then, \elseabsurd{\ref{axiom2:auxlemma5}}{ $[\ameetvar{\avariable}{\avariablefour}{\avariableter}] >_\avariable [\ameetvar{\avariable}{\avariablebis}{\avariableter}]$ implies
$[\ameetvar{\avariablebis}{\avariablefour}{\avariableter}] \not>_\avariable [\ameetvar{\avariable}{\avariablebis}{\avariableter}]$, and viceversa}
Indeed, let us show this statement. Suppose
$[\ameetvar{\avariable}{\avariablefour}{\avariableter}] >_\avariable [\ameetvar{\avariable}{\avariablebis}{\avariableter}]$. Therefore, by definition we have $\before{\ameetvar{\avariable}{\avariablefour}{\avariableter}}{\ameetvar{\avariable}{\avariablebis}{\avariableter}} \inside \aformula$.
Then, \elseabsurd{\ref{axiom2:auxlemma5}}{$\ameetvar{\avariable}{\avariablebis}{\avariableter} = \ameetvar{\avariablefour}{\avariablebis}{\avariableter} \inside \aformula$ and hence $\ameetvar{\avariable}{\avariablebis}{\avariableter} \approx \ameetvar{\avariablefour}{\avariablebis}{\avariableter}$}
By symmetry of $\ameetvar{\avariablebis}{\avariablefour}{\avariableter}$ (deduced above), we then obtain $\ameetvar{\avariable}{\avariablebis}{\avariableter} \approx \ameetvar{\avariablefour}{\avariablebis}{\avariableter}$ and therefore $[\ameetvar{\avariablebis}{\avariablefour}{\avariableter}] \not>_\avariable [\ameetvar{\avariable}{\avariablebis}{\avariableter}]$. The other direction holds by symmetry.
We then obtain that the union of the three orders $>_\avariable \cup >_\avariablebis \cup >_\avariableter$ form a ``tree shaped'' partial order, i.e. the union of the relations $\pred_\avariable$, $\pred_\avariablebis$, $\pred_\avariableter$ is still a functional relation, it is acyclic and it has a bottom element (the root of the tree).

We now generalise this statement: given a variable $\avariable \in \asetvar$ we consider the set of variables $G_\avariable = \{\avariablebis \in \asetvar \mid \exists \avariableter \in \asetvar \text{ s.t.\ } \symmetric{\ameetvar{\avariable}{\avariablebis}{\avariableter}} \inside \aformula \}$.
Notice that by definition $\avariable \in G_\avariable$ (indeed, $\avariable \approx \ameetvar{\avariable}{\avariable}{\avariable}$ follows from \ref{core2Ax:Self} and $\ameetvar{\avariable}{\avariable}{\avariable}$ is symmetric by definition)
From the properties above, we obtain that the orders $\{>_i \mid i \in G_\avariable\}$ form a tree shaped partial order.
Moreover, by symmetry  have that, for every $\avariablebis,\avariablefour \in G_\avariable$,
the sets
\begin{itemize}
\item $G_\avariablebis = \{\avariablefifth \in \asetvar \mid \exists \avariableter \in \asetvar \text{ s.t.\ } \symmetric{\ameetvar{\avariablebis}{\avariablefifth}{\avariableter}} \inside \aformula \}$ and
\item $G_\avariablefour = \{\avariablefifth \in \asetvar \mid \exists \avariableter \in \asetvar \text{ s.t.\ } \symmetric{\ameetvar{\avariablefour}{\avariablefifth}{\avariableter}} \inside \aformula \}$
\end{itemize}
are such that $G_\avariablebis = G_\avariablefour = G_\avariable$.
Then, let $\atree_{G_\avariable}$ be the partial function with domain and codomain $\bigcup_{i \in G_\avariable} M_i$, encoding the parent relation of the tree subsumed by $\{>_i \mid i \in G_\avariable\}$. Formally,
given an element $\ameetvar{\avariablesept}{\avariableoct}{\avariablenine} \in \bigcup_{i \in G_\avariable} M_i$
$\atree_{G_\avariable}([\ameetvar{\avariablesept}{\avariableoct}{\avariablenine}]) \egdef \pred_\avariablesept([\ameetvar{\avariablesept}{\avariableoct}{\avariablenine}])$.
Suppose $\ameetvar{\avariablesept}{\avariableoct}{\avariablenine},\ameetvar{\avariablesept'}{\avariableoct'}{\avariablenine'} \in \bigcup_{i \in G_\avariable} M_i$, then if $\ameetvar{\avariablesept}{\avariableoct}{\avariablenine} \approx \ameetvar{\avariablesept'}{\avariableoct'}{\avariablenine'}$, by the previous point of the proof we have
$\pred_\avariablesept([\ameetvar{\avariablesept}{\avariableoct}{\avariablenine}]) = \pred_{\avariablesept'}([\ameetvar{\avariablesept'}{\avariableoct'}{\avariablenine'}])$.
Hence, $\atree_{G_\avariable}$ is well-defined.

Given two elements $\asymbterm_1,\asymbterm_2 \in \domain{\atree_{G_\avariable}}$ and an element $\asymbterm \in \range{\atree_{G_\avariable}}$, we say that $\asymbterm$ is the lowest common ancestor of $\asymbterm_1$ and $\asymbterm_2$
if and only if there is no $\asymbterm'$ such that, for some $\alength_1,\alength_2\geq 1$,
$\atree_{G_\avariable}^{\alength_1}(\asymbterm_1) = \asymbterm'$, $\atree_{G_\avariable}^{\alength_2}(\asymbterm_2) = \asymbterm'$ and
$\atree_{G_\avariable}(\asymbterm') = \asymbterm$.

We now state one of the main properties of $\atree_{G_\avariable}$, that follows directly from ($\star$).
For $\avariableten,\avariablebis,\avariableter,\avariablefour,\avariablefifth,\avariablesix \in \asetvar$,
let $\ameetvar{\avariableten}{\avariablebis}{\avariableter}$ and $\ameetvar{\avariablefour}{\avariablefifth}{\avariablesix}$ two meet-points, such that $[\ameetvar{\avariableten}{\avariablebis}{\avariableter}]$ and $[\ameetvar{\avariablefour}{\avariablefifth}{\avariablesix}]$ are in
$\domain{\atree_{G_\avariable}}$.
Let $\ameetvar{\avariablesept}{\avariableoct}{\avariablenine}$ such that $\ameetvar{\avariablesept}{\avariableoct}{\avariablenine} \in \range{\atree_{G_\avariable}}$ and $[\ameetvar{\avariablesept}{\avariableoct}{\avariablenine}]$ is the least common ancestor of
$[\ameetvar{\avariableten}{\avariablebis}{\avariableter}]$ and $[\ameetvar{\avariablefour}{\avariablefifth}{\avariablesix}]$ in
$\atree_{G_\avariable}$. Then:
\[
\{ \ameetvar{a}{b}{\avariablenine}, \ameetvar{b}{a}{\avariablenine} \mid a\in\{\avariableten,\avariablebis\},\ b\in\{\avariablefour,\avariablefifth\} \} \subseteq [\ameetvar{\avariablesept}{\avariableoct}{\avariablenine}]
\]
Informally, this means that, while the set of subscripts appearing in equivalence classes weakly increases when descending $\atree_{G_\avariable}$ (this follows from the property in \textbf{(\ref{pathx:3})}, in the point~\textbf{\ref{proofcomp:point2}} of the proof), the set of variables $\{\avariable_1,\avariable_2 \mid \ameetvar{\avariable_1}{\avariable_2}{\avariable_3} \in \asymbterm\}$ of a
$\asymbterm \in \bigcup_{i \in G_\avariable} M_i$ strictly increases when considering ancestors of $\asymbterm$ in the tree.

As a last remark, the set $\{\atree_{G_\avariable} \mid \avariable \in \asetvar\}$ represents a forest.
Informally, the next point of the proof we deal with the fact that roots of some of the trees in this forest can be linked together in a cycle.
\item\label{proofcomp:point5} $\boxed{\text{Two trees in the same cycle}}$ Let $\ameetvar{\avariable}{\avariablebis}{\avariableter} \in \atermset{\asetvar}$ such that $\asymmetric{\ameetvar{\avariable}{\avariablebis}{\avariableter}} \inside \aformula$.
Then by definition of $\asymmetric{\ameetvar{\avariable}{\avariablebis}{\avariableter}}$ and $\approx$, we have $\ameetvar{\avariable}{\avariablebis}{\avariableter} \not\approx \ameetvar{\avariablebis}{\avariable}{\avariableter}$.
\elseabsurd{the property  \textbf{(\ref{pathx:2})}, in the point~\textbf{\ref{proofcomp:point2}} of the proof}{$\ameetvar{\avariable}{\avariablebis}{\avariableter}$ is the root of the tree represented by $\atree_{G_\avariable}$,
whereas $\ameetvar{\avariablebis}{\avariable}{\avariableter}$ is the root of the tree represented by $\atree_{G_\avariablebis}$}
As $\ameetvar{\avariable}{\avariablebis}{\avariableter} \not\approx \ameetvar{\avariablebis}{\avariable}{\avariableter}$, the two trees must be disjoint.
\elseabsurd{\ref{axiom2:samelooplemma0two}}{
$\sameloop{\ameetvar{\avariable}{\avariablebis}{\avariableter}}{\ameetvar{\avariablebis}{\avariable}{\avariableter}}$}
Moreover, \elseabsurd{the axioms~\ref{core2Ax:OneAsym}, \ref{core2Ax:BothAsym} and~\ref{core2Ax:Symmetric}}{
\begin{itemize}
\item $\{\ameetvar{a}{b}{\avariableter} \mid \exists \avariablefour, \avariablefifth, \avariablesix, \avariablesept {\in} \atermset{\asetvar}:
\ameetvar{a}{\avariablefour}{\avariablefifth} \in {\bigcup_{j \in G_\avariable} M_j} \text{ and } \ameetvar{b}{\avariablesix}{\avariablesept} \in {\bigcup_{j \in G_\avariablebis} M_j}\} \subseteq [\ameetvar{\avariable}{\avariablebis}{\avariableter}]$
\item $\{\ameetvar{a}{b}{\avariableter} \mid \exists \avariablefour, \avariablefifth, \avariablesix, \avariablesept {\in} \atermset{\asetvar}:
\ameetvar{a}{\avariablefour}{\avariablefifth} \in {\bigcup_{j \in G_\avariablebis} M_j} \text{ and } \ameetvar{b}{\avariablesix}{\avariablesept} \in {\bigcup_{j \in G_\avariable} M_j}\} \subseteq [\ameetvar{\avariablebis}{\avariable}{\avariableter}]$
\end{itemize}
}
This last statement seems a little bit obscure, so let us draw a picture to better understand it.
Suppose $\ameetvar{\avariable}{\avariablebis}{\avariableter}$ asymmetric and $\ameetvar{\avariablefour}{\avariablefifth}{\avariablesix}  \in {\bigcup_{i \in G_\avariable} M_i}$, so that $\ameetvar{\avariable}{\avariablebis}{\avariableter}$ and $\ameetvar{\avariablefour}{\avariablesix}{\avariablesept}$ belongs to the same tree.
Similarly, suppose $\ameetvar{\avariablesept}{\avariableoct}{\avariablenine}  \in {\bigcup_{i \in G_\avariablebis} M_i}$, so that
$\ameetvar{\avariablesept}{\avariableoct}{\avariablenine}$ and $\ameetvar{\avariablebis}{\avariable}{\avariableter}$ belong to the same tree.
Lastly, by asymmetry of $\ameetvar{\avariable}{\avariablebis}{\avariableter}$ we now know that $\ameetvar{\avariable}{\avariablebis}{\avariableter}$ and $\ameetvar{\avariablebis}{\avariable}{\avariableter}$ belong to
one cycle (by~\ref{axiom2:samelooplemma0two}).
Then, the statement above basically says that the equivalence classes of meet-points are so that:
\begin{center}
\scalebox{0.85}{
    \begin{tikzpicture}[baseline]
  \node (x) [label=left:{$\ameetvar{\avariable}{\avariablesept}{\avariableter}, \ameetvar{\avariablefour}{\avariablebis}{\avariableter}, \ameetvar{\avariablefour}{\avariablesept}{\avariableter} \in$}] at (0,0) {$[\ameetvar{\avariable}{\avariablebis}{\avariableter}]$};
  \node (u) [above left=1.5cm and 0.2cm of x, xshift=30pt] {$[\ameetvar{\avariablefour}{\avariablefifth}{\avariablesix}]$};
  \node (y) [right =2cm of x,label=right:{$\ni  \ameetvar{\avariablesept}{\avariable}{\avariableter}, \ameetvar{\avariablebis}{\avariablefour}{\avariableter}, \ameetvar{\avariablesept}{\avariablefour}{\avariableter}$}] {$[\ameetvar{\avariablebis}{\avariable}{\avariableter}]$};
  \node (i) [above right=1.5cm and 0.2cm of y, xshift=-30pt] {$[\ameetvar{\avariablesept}{\avariableoct}{\avariablenine}]$};

  \node (tgx) [above = 0.3cm of u] {$\atree_{G_\avariable}$};
  \node (tgy) [above = 0.3cm of i] {$\atree_{G_\avariablebis}$};

  \draw[reach] (u) -- (x);
  \draw[reach] (i) -- (y);
  \draw[reach] (x) to [bend left=60] node[label=below:{$\mathtt{sameloop}$}] {} (y);
  \draw[reach] (y) to [bend left=60] (x);

  \node (h2) [above right = 0.3cm of u] {};
  \node (h1) [left = 2.5cm of h2] {};

  \node (h3) [above left = 0.3cm of i] {};
  \node (h4) [right = 2.5cm of h3] {};

  \draw (h1.center) -- (x);
  \draw (h2.center) -- (x);
  \draw (h1.center) -- (h2.center);

  \draw (h3.center) -- (y);
  \draw (h4.center) -- (y);
  \draw (h3.center) -- (h4.center);
\end{tikzpicture}
}
\end{center}
Here notice that, if $\ameetvar{\avariablefour}{\avariablefifth}{\avariablesix}$ above is symmetric, in particular from $\ameetvar{\avariablefour}{\avariablefifth}{\avariablesix} \approx \ameetvar{\avariablefifth}{\avariablefour}{\avariablesix}$ we obtain that also $\ameetvar{\avariablefifth}{\avariablefour}{\avariablesix}$ is in ${\bigcup_{i \in G_\avariable} M_i}$ and hence also
$\ameetvar{\avariablefifth}{\avariablebis}{\avariableter}$ and $ \ameetvar{\avariablefifth}{\avariablesept}{\avariableter}$ are in $[\ameetvar{\avariable}{\avariablebis}{\avariableter}]$.
The same reasoning holds for $\ameetvar{\avariablesept}{\avariableoct}{\avariablenine}$ (if symmetric) with respect to $\ameetvar{\avariablebis}{\avariable}{\avariableter}$.

\item\label{proofcomp:point6} $\boxed{\text{Cycles}}$ Given $\avariable \in \asetvar$, we define the following subset of defined meet-points
\begin{nscenter}
$S_\avariable =\{ \ameetvar{\avariablefour}{\avariablefifth}{\avariablesix} \mid \avariablefour \in G_\avariable \text{ and } \asymmetric{\ameetvar{\avariablefour}{\avariablefifth}{\avariablesix}} \inside \aformula\}.$
\end{nscenter}
As the definition of $G_\avariable$ is so that $\avariable \in G_\avariable$ and for every $\avariablebis \in G_\avariable$, $G_\avariablebis = G_\avariable$ (see point~\ref{proofcomp:point4} of the proof) we conclude by definition that for every $\avariablebis \in G_\avariable$, $S_\avariable = S_\avariablebis$.
This can also be seen from the property~\ref{pathx:2} described in point~\ref{proofcomp:point2} of the proof: if an asymmetric meet-point $\ameetvar{\avariablefour}{\avariablefifth}{\avariablesix}$ is defined, then it is minimal for the order $>_\avariablefour$ (whereas
$\ameetvar{\avariablefifth}{\avariablefour}{\avariablesix}$ is minimal for the order $>_\avariablefifth$). By definition, then it is the root of the tree represented by $\atree_{G_\avariablefour}$.

Recall that $G_\avariable$ are all the variables appearing in the same tree $\atree_{G_\avariable}$.
Hence (see again point~\ref{proofcomp:point4}), given any two $\avariablebis,\avariablefour\in G_\avariable$ there exists
$\avariableter \in \asetvar$ such that $\ameetvar{\avariablebis}{\avariablefour}{\avariableter}$ is defined and symmetric.
\elseabsurd{the previous point of the construction (where we used in particular \ref{core2Ax:OneAsym})}{if $\ameetvar{\avariablebis}{\avariablefifth}{\avariablesix}$ is asymmetric then so is $\ameetvar{\avariablefour}{\avariablefifth}{\avariablesix}$ and $\ameetvar{\avariablebis}{\avariablefifth}{\avariablesix} \approx \ameetvar{\avariablefour}{\avariablefifth}{\avariablesix}$
(for some $\avariablefifth,\avariablesix \in \asetvar$)}
Thanks to this, by definition of $S_\avariable$ we obtain that for every $\asymbterm_1,\asymbterm_2 \in S_\avariable$, $\asymbterm_1 \approx \asymbterm_2$.

We now use the following properties of $\mathtt{sameloop}$, proved again in Section~\ref{subsection-intermediate-tautologies-eq}:
\begin{itemize}
\item \ref{axiom2:samelooplemma0}
$
\lnot\sameloop{\aterm}{\aterm}
$
\item \ref{axiom2:samelooplemma1}
$
\sameloop{\aterm_1}{\aterm_2} \implies \sameloop{\aterm_2}{\aterm_1}
$
\item \ref{axiom2:samelooplemma2}
$
\sameloop{\aterm_1}{\aterm_2} \land \sameloop{\aterm_2}{\aterm_3} \land \aterm_1 \neq \aterm_3 \implies \sameloop{\aterm_1}{\aterm_3}
$
\item \ref{axiom2:sameloopsubr}
$
\sameloop{\aterm_1}{\aterm_2} \land \aterm_2 = \aterm_3 \implies \sameloop{\aterm_1}{\aterm_3}
$
\item
\ref{axiom2:sameloopsubl}
$
\sameloop{\aterm_1}{\aterm_2} \land \aterm_1 = \aterm_3 \implies \sameloop{\aterm_3}{\aterm_2}
$
\end{itemize}
Consider $\avariable,\avariablebis,\avariableter \in \asetvar$ such that $S_\avariable \neq S_\avariablebis \neq S_\avariableter$ and such that there are two meet-points $\ameetvar{\avariablefour}{\avariablefifth}{\avariablesix}, \ameetvar{\avariablesept}{\avariableoct}{\avariablenine}$ such that
\begin{itemize}
\item $\ameetvar{\avariablefour}{\avariablefifth}{\avariablesix} \in S_\avariable$ and $\ameetvar{\avariablefifth}{\avariablefour}{\avariablesix} \in S_\avariablebis$
\item $\ameetvar{\avariablesept}{\avariableoct}{\avariablenine} \in S_\avariablebis$ and $\ameetvar{\avariableoct}{\avariablesept}{\avariablenine} \in S_\avariableter$
\end{itemize}
Then \elseabsurd{the five properties of $\mathtt{sameloop}$ written above}{
\begin{itemize}
\item for every $a \in \{\avariable,\avariablebis,\avariableter\}$ and $\aterm,\aterm' \in S_a$, $\sameloop{\aterm}{\aterm'} \not\inside \aformula$;
\item for every $\aterm \in S_\avariable$ and $\aterm' \in S_\avariablebis$, $\sameloop{\aterm}{\aterm'}\land\sameloop{\aterm'}{\aterm}\ \inside \aformula$ and $\aterm_1 \not\approx \aterm_2$;
\item for every $\aterm \in S_\avariablebis$ and $\aterm' \in S_\avariableter$, $\sameloop{\aterm}{\aterm'}\land\sameloop{\aterm'}{\aterm} \inside \aformula$ and $\aterm_1 \not\approx \aterm_2$;
\item if moreover $S_\avariable \neq S_\avariableter$, then for every  $\aterm \in S_\avariable$ and $\aterm' \in S_\avariableter$, $\sameloop{\aterm}{\aterm'} \inside \aformula$ (by~\ref{axiom2:samelooplemma2}) and $\aterm_1 \not\approx \aterm_2$
\end{itemize}
}
Then, given a variable $\avariable \in \asetvar$, we define
$C_\avariable = \{ S_\avariablebis \mid \text{there are }\avariablefour,\avariableter\in\asetvar\ \text{s.t.}\ \ameetvar{\avariablefour}{\avariablebis}{\avariableter} \in S_\avariable\}$. We call $C_\avariable$ a \emph{cluster}.
From the properties above, for every two $\avariable,\avariablebis\in\asetvar$ such that
\begin{itemize}
\item $S_\avariable \neq S_\avariablebis$ and
\item there is a meet-point
$\ameetvar{\avariablefour}{\avariablefifth}{\avariablesix}$ such that $\ameetvar{\avariablefour}{\avariablefifth}{\avariablesix} \in S_\avariable$ and $\ameetvar{\avariablefifth}{\avariablefour}{\avariablesix} \in S_\avariablebis$
\end{itemize}
it must hold that $S_\avariablebis \in C_\avariable$, $S_\avariable \in C_\avariablebis$ and $C_\avariable \cup \{S_\avariable\} = C_\avariablebis \cup \{S_\avariablebis\}$.
In the model that we will later build, elements in the cluster $C_\avariable \cup \{S_\avariable\}$ ($\avariable \in \asetvar$)  will form a cycle.
It is important to recall two things, said previously in this point of the proof:
\begin{itemize}
\item for all $\avariable \in \asetvar$ and all $\asymbterm_1,\asymbterm_2 \in S_\avariablefour$, $\asymbterm_1 \approx \asymbterm_2$.
\item for all $\avariable \in \asetvar$, all $S_1,S_2 \in C_\avariable \cup \{S_\avariable\}$ and every $\asymbterm_1 \in S_1,\ \asymbterm_2 \in S_2$, $\asymbterm_1 \not\approx \asymbterm_2$.
\end{itemize}
Lastly, recall that, given $\avariable \in \asetvar$ and two terms,  the tree $\atree_{G_\avariable}$ is defined so that $\asymbterm_1$ is a descendant of $\asymbterm_2$ in the tree if and only if
$\before{\aterm_1}{\aterm_2} \inside \aformula$ for every two terms $\aterm_1 \in \asymbterm_1$ and $\aterm_2 \in \asymbterm_2$. Similarly, for every $\asymbterm \in C_\avariable$, $\sameloop{\aterm_1}{\aterm_2}$ for every two terms $\aterm_1 \in S_\avariable$ and $\aterm_2 \in \asymbterm$.
Then, \elseabsurd{\ref{core2Ax:SeesBefore}, \ref{core2Ax:SeesEWCycl}, \ref{core2Ax:SeesNegSum} and \ref{core2Ax:SeesSum}}{
for every $\asymbterm_1\in \bigcup_{i \in G_\avariable} M_i$ and every $\asymbterm_2 \in C_\avariable \cup \{S_\avariable\}$, $\prove_{\coresys} \aformula\implies\sees{\aterm_1}{\aterm_2}{\emptyset}$
for every $\aterm_1 \in \asymbterm_1$ and $\aterm_2 \in \asymbterm_2$
} With the figure of the previous point of the proof as a reference, this means for example that $\ameetvar{\avariablefour}{\avariablefifth}{\avariablesix}$ reaches $\ameetvar{\avariablebis}{\avariable}{\avariableter}$.
A similar statement is proved completely formally in~\ref{axiom2:beforesameloopsees}.
\item $\boxed{\text{Subscripts are reachable}}$ Before moving to $\mathtt{sees}$ and $\mathtt{rem}$ predicates, we show a last property about subscripts of meet-points, i.e. ``$\avariableter$''
 in $\ameetvar{\avariable}{\avariablebis}{\avariableter}$.
Let $\ameetvar{\avariable}{\avariablebis}{\avariableter} \in \atermset{\asetvar}$ be a defined meet-point.
\elseabsurd{\ref{axiom2:subscriptforward} and the definitions of $\atree_{G_\avariable}$ and $C_\avariable$}{there exists $\alength \geq 0$ such that $\atree_{G_\avariable}^\alength([\ameetvar{\avariable}{\avariablebis}{\avariableter}]) = [\avariableter]$ or $[\avariableter] \in C_\avariable$}.
\end{enumerate}
We now consider $\mathtt{sees}$ predicates. Recall that by definition of characteristic formula, for all terms $\aterm_1,\aterm_2 \in \atermset{\asetvar}$,
\begin{itemize}
\item
 $\lnot\sees{\aterm_1}{\aterm_2}{\atermset{\asetvar}} \inside \aformula$ or (otherwise) there is exactly one $\inbound \in \interval{1}{\bound}$ such that\\
${\seesgeq{\aterm_1}{\aterm_2}{\atermset{\asetvar}}{\inbound}} \inside \aformula$. Moreover, in the second case, if $\inbound < \bound$ then\\
$\lnot \seesgeq{\aterm_1}{\aterm_2}{\atermset{\asetvar}}{\inbound{+}1} \inside \aformula$.
No other $\lnot\seesgeq{\aterm_1}{\aterm_2}{\asetmeetvar}{\inbound'}$ belongs to $\literals{\aformula}$.
\end{itemize}

For now, we only care about whether or not a predicate $\seesgeq{\aterm_1}{\aterm_2}{\atermset{\asetvar}}{\inbound}$ holds or not, disregarding its length $\inbound$.
Indeed, by axiom~\ref{core2Ax:SeesMono2}, from such a predicate we can deduce $\sees{\aterm_1}{\aterm_2}{\atermset{\asetvar}}$.
Hence, in what follows, we write ``$\prove_{\coresys} \aformula \supseteq \sees{\aterm_1}{\aterm_2}{\atermset{\asetvar}}$'' to say that, for a certain $\inbound \in \interval{1}{\bound}$ we have
$\seesgeq{\aterm_1}{\aterm_2}{\atermset{\asetvar}}{\inbound} \inside \aformula$ and we proved
$\prove_{\coresys} \aformula \implies \sees{\aterm_1}{\aterm_2}{\atermset{\asetvar}}$ with~\ref{core2Ax:SeesMono2}. Notice that the derivation of this proof only uses formulae from $\coreformulae{\asetvar}{\bound}$.
We recall again that, from $\avariable \approx \ameetvar{\avariable}{\avariable}{\avariable}$, we can reason with meet-points knowing that the same reasoning holds for variables.
\begin{enumerate}
\setcounter{enumi}{7}
\item\label{proofcomp:point8} $\boxed{\text{Sees}}$
Suppose that $\prove_{\coresys} \aformula \supseteq \sees{\ameetvar{\avariable}{\avariablebis}{\avariableter}}{\ameetvar{\avariablefour}{\avariablefifth}{\avariablesix}}{\atermset{\asetvar}}$. Then, we want to prove that
\begin{enumerate}
\item if $[\ameetvar{\avariable}{\avariablebis}{\avariableter}] \in \domain{\atree_{G_\avariable}}$ then $\atree_{G_\avariable}([\ameetvar{\avariable}{\avariablebis}{\avariableter}]) =
[\ameetvar{\avariablefour}{\avariablefifth}{\avariablesix}]$,
\item otherwise if $[\ameetvar{\avariable}{\avariablebis}{\avariableter}] \not\in \domain{\atree_{G_\avariable}}$ and $\ameetvar{\avariable}{\avariablebis}{\avariableter} \neq \ameetvar{\avariablefour}{\avariablefifth}{\avariablesix} \inside \aformula$
then $S_\avariablefour \in C_\avariable$,
\item otherwise ($[\ameetvar{\avariable}{\avariablebis}{\avariableter}] \not\in \domain{\atree_{G_\avariable}}$ and $\ameetvar{\avariable}{\avariablebis}{\avariableter} = \ameetvar{\avariablefour}{\avariablefifth}{\avariablesix} \inside \aformula$)
then $C_\avariable = \emptyset$.
\end{enumerate}

(a) For the first case, suppose by contradiction $\atree_{G_\avariable}([\ameetvar{\avariable}{\avariablebis}{\avariableter}]) = \asymbterm \neq
[\ameetvar{\avariablefour}{\avariablefifth}{\avariablesix}]$.
Let $\aterm_1 \in \asymbterm$.
By definition of $\atree_{G_\avariable}$, and the property~\ref{pathx:1b} in point~\ref{proofcomp:point2} of the proof, $\before{\ameetvar{\avariable}{\avariablebis}{\avariableter}}{\aterm_1} \inside \aformula$ and there is no $\aterm \in \atermset{\asetvar}$ such that
$\before{\ameetvar{\avariable}{\avariablebis}{\avariableter}}{\aterm} \land \before{\aterm}{\aterm_1} \inside \aformula$.

By the axiom~\ref{core2Ax:SeesBefore}, it holds that $\prove_{\coresys} \aformula \implies \sees{\ameetvar{\avariable}{\avariablebis}{\avariableter}}{\aterm_1}{\emptyset}$.
From $\asymbterm \neq
[\ameetvar{\avariablefour}{\avariablefifth}{\avariablesix}]$ it then holds that $\aterm_1 \neq \ameetvar{\avariablefour}{\avariablefifth}{\avariablesix} \inside \aformula$.
By axioms~\ref{core2Ax:SeesFunc} and \ref{core2Ax:SeesMono1}, from $\aterm_1 \neq \ameetvar{\avariablefour}{\avariablefifth}{\avariablesix} \inside \aformula$ and
$\prove_{\coresys} \aformula \supseteq \sees{\ameetvar{\avariable}{\avariablebis}{\avariableter}}{\ameetvar{\avariablefour}{\avariablefifth}{\avariablesix}}{\atermset{\asetvar}}$
and $\prove_{\coresys} \implies \sees{\ameetvar{\avariable}{\avariablebis}{\avariableter}}{\aterm_1}{\emptyset}$
we deduce that $\prove_{\coresys} \aformula \implies \lnot\sees{\ameetvar{\avariable}{\avariablebis}{\avariableter}}{\aterm_1}{\{\ameetvar{\avariablefour}{\avariablefifth}{\avariablesix}\}}$.
Then, by axioms~\ref{core2Ax:SeesElsewhere}, \ref{axiom2:beforefunc} and~\ref{core2Ax:SeesBefore} it is easy to conclude that
$\prove_{\coresys} \aformula \implies \before{\ameetvar{\avariable}{\avariablebis}{\avariableter}}{\ameetvar{\avariablefour}{\avariablefifth}{\avariablesix}} \land \before{\ameetvar{\avariablefour}{\avariablefifth}{\avariablesix}}{{\aterm_1}}$. We reach then a contradiction: as $\aformula$ is a characteristic formula, every equality between two terms appears as a litteral in it (as written at the beginning of the proof). Then
$\before{\ameetvar{\avariable}{\avariablebis}{\avariableter}}{\ameetvar{\avariablefour}{\avariablefifth}{\avariablesix}} \land \before{\ameetvar{\avariablefour}{\avariablefifth}{\avariablesix}}{{\aterm_1}} \inside \aformula$,
in contradiction with the definition of  $\atree_{G_\avariable}$ (again, see property~\ref{pathx:1b} in point~\ref{proofcomp:point2} of the proof).
 Hence,
$\atree_{G_\avariable}([\ameetvar{\avariable}{\avariablebis}{\avariableter}]) =
[\ameetvar{\avariablefour}{\avariablefifth}{\avariablesix}]$.

(b) For the second case \elseabsurd{\ref{core2Ax:SeesDef}}{$\defined{\ameetvar{\avariable}{\avariablebis}{\avariableter}} \inside \aformula$}
\elseabsurd{$[\ameetvar{\avariable}{\avariablebis}{\avariableter}] \not\in \domain{\atree_{G_\avariable}}$}{$\asymmetric{\ameetvar{\avariable}{\avariablebis}{\avariableter}} \inside \aformula$}
\elseabsurd{\ref{axiom2:seessameloop}}{$S_\avariablefour \in C_\avariable$}

(c) For the last case, suppose {\em ad absurdum} that there is an element $S_\avariablesept \in C_\avariable$.
Then by definition there is an element $\ameetvar{\avariable}{\avariablesept}{\avariableoct} \in [\ameetvar{\avariable}{\avariablebis}{\avariableter}]$ such that $\asymmetric{\ameetvar{\avariable}{\avariablesept}{\avariableoct}} \inside \aformula$.
\elseabsurd{\ref{axiom2:samelooplemma0two} and~\ref{axiom2:sameloopsubl}}{$\sameloop{\ameetvar{\avariable}{\avariablebis}{\avariableter}}{\ameetvar{\avariablesept}{\avariable}{\avariableoct}} \inside \aformula$} Then,
\elseabsurd{\ref{core2Ax:SeesEWCycl}}{$\prove_{\coresys} \aformula \implies \lnot \sees{\ameetvar{\avariable}{\avariablebis}{\avariableter}}{\ameetvar{\avariable}{\avariablebis}{\avariableter}}{\{\ameetvar{\avariablesept}{\avariable}{\avariableoct}\}}$}
However, as we supposed $\prove_{\coresys} \aformula \supseteq \sees{\ameetvar{\avariable}{\avariablebis}{\avariableter}}{\ameetvar{\avariablefour}{\avariablefifth}{\avariablesix}}{\atermset{\asetvar}}$ and
$\ameetvar{\avariable}{\avariablebis}{\avariableter} = \ameetvar{\avariablefour}{\avariablefifth}{\avariablesix} \inside \aformula$ (hypothesis of case (c)), by~\ref{core2Ax:Substitute} and~\ref{core2Ax:SeesMono1} we can prove that
\begin{nscenter}
$\prove_{\coresys} \aformula \implies
\sees{\ameetvar{\avariable}{\avariablebis}{\avariableter}}{\ameetvar{\avariable}{\avariablebis}{\avariableter}}{\{\ameetvar{\avariablesept}{\avariable}{\avariableoct}\}}$,
\end{nscenter}
Then by propositional calculus, we obtain
\begin{nscenter}
$\prove_{\coresys} \aformula \supseteq \sees{\ameetvar{\avariable}{\avariablebis}{\avariableter}}{\ameetvar{\avariablefour}{\avariablefifth}{\avariablesix}}{\terms{\asetvar}}
\land \sees{\ameetvar{\avariable}{\avariablebis}{\avariableter}}{\ameetvar{\avariable}{\avariablebis}{\avariableter}}{\{\ameetvar{\avariablesept}{\avariable}{\avariableoct}\}}$
\end{nscenter}
and therefore (again by propositional reasoning) $\prove_{\coresys} \aformula \implies \true$, a contradiction.
Then  $C_\avariable = \emptyset$.

\item\label{proofcomp:point9} $\boxed{\text{Sees in a cycle}}$ We now consider a cluster $C_\avariable \cup \{S_\avariable\}$ ($\avariable \in \asetvar$) with $S_\avariable \neq \emptyset$.
By definition $C_\avariable \cup \{S_\avariable\}$ has then cardinality at least $2$.
 Let $\asetmeetvar = \{\aterm_1,\dots,\aterm_n\}$ a set containing exactly one representative for each set in $C_\avariable \cup \{S_\avariable\}$. We want to show
that, if $\not\prove_{\coresys} \aformula \implies \bottom$ then there exists a cyclic order $\aterm_{i_1} \to \aterm_{i_2} \to \dots \to \aterm_{i_n} \to \aterm_{i_1}$ of all the elements in $\asetmeetvar$ so that for every $j \in \interval{1}{n-1}$,
$\prove_{\coresys} \aformula \implies \sees{\aterm_{i_j}}{\aterm_{i_{j+1}}}{\asetmeetvar}$ and $\prove_{\coresys} \aformula \implies \sees{\aterm_{i_n}}{\aterm_{i_{1}}}{\asetmeetvar}$.
The main ingredient to show this property, which we call \emph{cycle order property}, is axiom~\ref{core2Ax:SeesLoopOrder}.
Here, we start by showing the property for a ``cluster'' of two elements (in doing this, we do not use~\ref{core2Ax:SeesLoopOrder}). Then, we show as an example the case for three elements, to better understanding the process. Then, we then reason inductively for the general result.
We know already (point~\ref{proofcomp:point6} of the proof) that for every two distinct elements of $\asymbterm_1,\asymbterm_2 \in C_\avariable \cup \{S_\avariable\}$ we have, for every $\aterm_1 \in \asymbterm_1$ and $\aterm_2 \in \asymbterm_2$,
$\sameloop{\aterm_1}{\aterm_2} \inside \aformula$. Then \elseabsurd{\ref{core2Ax:SeesEWCycl}}
{$\prove_{\coresys} \aformula \implies \sees{\aterm_1}{\aterm_1}{\emptyset} \land \lnot \sees{\aterm_1}{\aterm_1}{\{\aterm_2\}}$}
Then, by \ref{core2Ax:SeesNegSum} it is easy to see that
$\prove_{\coresys} \aformula \implies \sees{\aterm_1}{\aterm_2}{\emptyset} \land \sees{\aterm_2}{\aterm_1}{\emptyset}$.
We can then use \ref{core2Ax:SeesRef} to conclude
$\prove_{\coresys} \aformula \implies \sees{\aterm_1}{\aterm_2}{\{\aterm_1,\aterm_2\}} \land \sees{\aterm_2}{\aterm_1}{\{\aterm_1,\aterm_2\}}$.
This establishes a proof of the cycle order property for cycles of only two elements.

Suppose now $\asymbterm_1,\asymbterm_2,\asymbterm_3$ three distinct elements of $C_\avariable \cup \{S_\avariable\}$ and $\aterm_1 \in \asymbterm_1$, $\aterm_2 \in \asymbterm_2$ and $\aterm_3 \in \asymbterm_3$.
Using axioms~\ref{core2Ax:SeesLoopOrder},~\ref{core2Ax:SeesEWCycl},~\ref{core2Ax:SeesSum} and~\ref{axiom2:samelooplemma1}
we now prove that one of the following must hold
(as otherwise we would reach a contradiction by proving $\prove_{\coresys} \aformula \implies \bottom$):
\begin{itemize}
\item $\prove_{\coresys} \aformula \implies \sees{\aterm_1}{\aterm_2}{\{\aterm_3\}} \land \sees{\aterm_2}{\aterm_3}{\{\aterm_1\}} \land \sees{\aterm_3}{\aterm_1}{\{\aterm_2\}}$ or
\item $\prove_{\coresys} \aformula \implies \sees{\aterm_1}{\aterm_3}{\{\aterm_2\}} \land \sees{\aterm_3}{\aterm_2}{\{\aterm_1\}} \land \sees{\aterm_2}{\aterm_1}{\{\aterm_3\}}$.
\end{itemize}
Indeed, \elseabsurd{\ref{core2Ax:SeesLoopOrder}}{$\prove_{\coresys} \aformula \implies \sees{\aterm_1}{\aterm_3}{\aterm_2} \lxor \sees{\aterm_3}{\aterm_1}{\aterm_2}$}
There are then two cases: $\prove_{\coresys} \aformula \implies \sees{\aterm_1}{\aterm_3}{\{\aterm_2\}} \land \lnot \sees{\aterm_3}{\aterm_1}{\{\aterm_2\}}$ or
$\prove_{\coresys} \aformula \implies \lnot \sees{\aterm_1}{\aterm_3}{\{\aterm_2\}} \land \sees{\aterm_3}{\aterm_1}{\{\aterm_2\}}$.

We now investigate the case for
$\prove_{\coresys} \aformula \implies \sees{\aterm_1}{\aterm_3}{\{\aterm_2\}} \land \lnot \sees{\aterm_3}{\aterm_1}{\{\aterm_2\}}$.
\[
\begin{nd}
\hypo {1} {\sameloop{\aterm_1}{\aterm_2}}
\hypo {2} {\sameloop{\aterm_2}{\aterm_3}}
\hypo {3} {\sameloop{\aterm_3}{\aterm_1}}
\hypo {4} {\boxed{\sees{\aterm_1}{\aterm_3}{\{\aterm_2\}}}}
\hypo {5} {\lnot \sees{\aterm_3}{\aterm_1}{\{\aterm_2\}}}
\hypo {6} {\aterm_1 \neq \aterm_2} \ae{1}
\hypo {7} {\aterm_2 \neq \aterm_3} \ae{2}
\hypo {8} {\aterm_1 \neq \aterm_3} \ae{3}
\have {9} {\sees{\aterm_1}{\aterm_2}{\{\aterm_3\}} \iff \lnot \sees{\aterm_2}{\aterm_1}{\{\aterm_3\}}} \by{\ref{core2Ax:SeesLoopOrder}}{2,3,6}
\open
\hypo {10} {\sees{\aterm_1}{\aterm_2}{\{\aterm_3\}} \land \lnot \sees{\aterm_2}{\aterm_1}{\{\aterm_3\}}}
\have {11} {\aterm_2 = \aterm_3} \by{\ref{core2Ax:SeesFunc}}{4,10}
\have {12} {\bottom} \by{\landcontr}{7,11}
\close
\have {13} {\boxed{\sees{\aterm_2}{\aterm_1}{\{\aterm_3\}}} \land \lnot \sees{\aterm_1}{\aterm_2}{\{\aterm_3\}}}
\by{\modusponens}{9,10-12}
\have {14} {\sees{\aterm_2}{\aterm_3}{\{\aterm_1\}} \iff \lnot \sees{\aterm_3}{\aterm_2}{\{\aterm_1\}}}
\by{\ref{core2Ax:SeesLoopOrder} and \ref{axiom2:samelooplemma1}}{1,4,7}
\open
\hypo {15} {\sees{\aterm_2}{\aterm_3}{\{\aterm_1\}} \land \lnot \sees{\aterm_3}{\aterm_2}{\{\aterm_1\}}}
\have {16} {\aterm_1 = \aterm_3} \by{\ref{core2Ax:SeesFunc}}{13,15}
\have {17} {\bottom} \by{\landcontr}{3,16}
\close
\have {18} {\boxed{\sees{\aterm_3}{\aterm_2}{\{\aterm_1\}}} \land \lnot \sees{\aterm_2}{\aterm_3}{\{\aterm_1\}}}
\by{\modusponens}{14,15-17}
\have {19}
{\sees{\aterm_1}{\aterm_3}{\{\aterm_2\}} \land \sees{\aterm_3}{\aterm_2}{\{\aterm_1\}} \land \sees{\aterm_2}{\aterm_1}{\{\aterm_3\}}}
\by{\ndref{4} $\land$ \ndref{13} $\land$ \ndref{18}}{}
\end{nd}
\]
The other case, i.e. $\prove_{\coresys} \aformula \implies \lnot \sees{\aterm_1}{\aterm_3}{\{\aterm_2\}} \land \sees{\aterm_3}{\aterm_1}{\{\aterm_2\}}$ is analogous and instead leads to
\begin{nscenter}
$\prove_{\coresys} \aformula \implies \sees{\aterm_1}{\aterm_2}{\{\aterm_3\}} \land \sees{\aterm_2}{\aterm_3}{\{\aterm_1\}} \land \sees{\aterm_3}{\aterm_1}{\{\aterm_2\}}$.
\end{nscenter}
By using again~\ref{core2Ax:SeesRef}, we obtain a proof of the cycle order property for clusters of three elements.
From this case, it should be clear what is the ``meaning'' of axiom~\ref{core2Ax:SeesLoopOrder}: given two elements $\aterm$ and $\aterm'$ in a loop, it states that a third (different) element of the cycle must be or in the path from $\aterm$ to $\aterm'$ or in the path from $\aterm'$ to $\aterm$. Therefore, axiom~\ref{core2Ax:SeesLoopOrder} given an order to the elements of the cycle.
We prove the cycle order property by induction, with hypothesis: given a set  $\asetmeetvar$ containing at most one representative for each set of a cluster $C_\avariable \cup \{S_\avariable\}$ ($\avariable \in \asetvar$, $S_\avariable \neq \emptyset$)
\begin{itemize}
\item[] for each strict subset $\asetmeetvar'\subset\asetmeetvar$ of at least $2$ elements there exists a cyclic order $\aterm_1\to,\dots,\to\aterm_i\to\aterm_1$ so that for every $j \in \interval{1}{i-1}$,
$\prove_{\coresys} \aformula \implies \sees{\aterm_{j}}{\aterm_{{j+1}}}{\asetmeetvar'}$ and $\prove_{\coresys} \aformula \implies \sees{\aterm_{i}}{\aterm_{1}}{\asetmeetvar'}$.
\end{itemize}
We have already shown the case for $\asetmeetvar$ of  cardinality $2$ (base case), and we also shown the case for $3$ to have a better understanding of axiom~\ref{core2Ax:SeesLoopOrder}.

For the inductive case, suppose $\asetmeetvar' = \asetmeetvar \setminus \{\aterm\}$ with $\aterm \in \asetmeetvar$ and $\asetmeetvar' = \{\aterm_1,\dots,\aterm_i\}$. Then by inductive hypothesis
there exists a cyclic order $\aterm_1\to\dots\to\aterm_i\to\aterm_1$ so that for every $j \in \interval{1}{i-1}$,
$\prove_{\coresys} \aformula \implies \sees{\aterm_{j}}{\aterm_{{j+1}}}{\asetmeetvar'}$ and $\prove_{\coresys} \aformula \implies \sees{\aterm_{i}}{\aterm_{1}}{\asetmeetvar'}$.

\elseabsurd{\ref{core2Ax:SeesLoopOrder}}{there must be two elements $\aterm_j \to \aterm_{(j \mod i)+1}$ so that,
$\prove_{\coresys} \aformula \implies \lnot \sees{\aterm_j}{\aterm_{(j \mod i)+1}}{\{\aterm\}} \land \sees{\aterm_{(j \mod i)+1}}{\aterm_j}{\{\aterm\}}$}. From the inductive hypothesis we have
$\prove_{\coresys} \aformula \implies \lnot \sees{\aterm_j}{\aterm_{(j \mod i)+1}}{\asetmeetvar'}$.
Then, \elseabsurd{\ref{core2Ax:SeesNegSum} followed by~\ref{core2Ax:SeesRef}}{
$\prove_{\coresys} \aformula \implies \sees{\aterm_j}{\aterm}{\{\aterm\}\cup\asetmeetvar'}
\land \sees{\aterm}{\aterm_{(j \mod i)+1}}{\{\aterm\}\cup\asetmeetvar'}$}.

Suppose now that there exists a second pair of elements (i.e. $j \neq k$) $\aterm_k \to \aterm_{(k \mod i)+1}$ such that $\prove_{\coresys} \aformula \implies \lnot \sees{\aterm_{k}}{\aterm_{(k \mod i)+1}}{\{\aterm\}}$. Then with the same reasoning as before we obtain
$\prove_{\coresys} \aformula \implies \sees{\aterm}{\aterm_{(k \mod i)+1}}{\{\aterm\}\cup\asetmeetvar'}$.
By definition, $\asetmeetvar'$ contains both $\aterm_{(k \mod i)+1}$ and $\aterm_{(j \mod i)+1}$, for which it must hold that $\aterm_{(k \mod i)+1}\neq\aterm_{(j \mod i)+1} \inside \aformula$, as by hypothesis $\asetmeetvar'$ contains at most one representative for each set of the cluster.
However, by repeated application of~\ref{core2Ax:SeesMono1} we obtain
$\prove_{\coresys} \aformula \implies \sees{\aterm}{\aterm_{(j \mod i)+1}}{\{\aterm_{(k \mod i)+1}\}} \land \sees{\aterm}{\aterm_{(k \mod i)+1}}{\{\aterm_{(j \mod i)+1}\}}$ and then by \ref{core2Ax:SeesFunc} we obtain
$\prove_{\coresys} \aformula \implies {\aterm_{(j \mod i)+1}} = {\aterm_{(k \mod i)+1}}$: a contradiction.
Hence, for every other pair of elements  (i.e. $j \neq k$) $\aterm_k \to \aterm_{(k \mod i)+1}$, $\prove_{\coresys} \aformula \implies \sees{\aterm_{k}}{\aterm_{(k \mod i)+1}}{\{\aterm\}}$. Then the cycle order property of $\asetmeetvar$ holds  for the cyclic order
$\aterm_1\dots\aterm_j \to \aterm \to \aterm_{(j \mod i) + 1}\dots\aterm_i\to\aterm_1$, which concludes the proof.

As a last step, suppose now $\asetmeetvar$ to contain exactly one representative for each set of a cluster, and let
$\aterm_1\to\dots\to\aterm_n\to\aterm_1$ be its cyclic order. Then, \elseabsurd{\ref{axiom2:outsideloopsees}}{
$\forall j \in \interval{1}{n-1}$,
$\prove_{\coresys} \aformula \implies \sees{\aterm_{j}}{\aterm_{{j+1}}}{\terms{\asetvar}}$ and $\prove_{\coresys} \aformula \implies \sees{\aterm_{n}}{\aterm_{1}}{\terms{\asetvar}}$}
Here, notice the subscripts of sees predicates.
For each of these predicates,
say $\sees{\aterm}{\aterm'}{\atermset{\asetvar}}$, we then must have that $\seesgeq{\aterm}{\aterm'}{\atermset{\asetvar}}{\inbound} \inside \aformula$, otherwise $\prove_{\coresys} \aformula \implies \bottom$ follows
 from~\ref{core2Ax:SeesMono2}.

\item\label{proofcomp:point10} $\boxed{\text{Not Sees}}$
From the previous point of the proof, we already know that given two terms $\aterm_1$ and $\aterm_2$ such that $[\aterm_1],[\aterm_2] \inside C_\avariable$ ($\avariable \in \asetvar$),
if $\aterm_2$ is the successor of $\aterm_1$ in the cyclic order then
$\prove_{\coresys} \aformula \implies \sees{\aterm_1}{\aterm_{2}}{\atermset{\asetvar}}$.
Hence, it cannot be that $\lnot \sees{\aterm_1}{\aterm_{2}}{\atermset{\asetvar}} \inside \aformula$ as otherwise by classical reasoning $\prove_{\coresys} \aformula \implies \bottom$ in contradiction with the hypothesis.

We need a similar result for the elements of a tree: given $\avariable \in \asetvar$ and $\aterm_1,\aterm_2 \in \atermset{\asetvar}$ such that $[\aterm_1] \in \domain{\atree_{G_\avariable}}$
 and $\atree_{G_\avariable}([\aterm_1]) = [\aterm_2]$, we show that
$\prove_{\coresys} \aformula \implies \sees{\aterm_1}{\aterm_{2}}{\atermset{\asetvar}}$.
Recall that, from the property of the characteristic formula it holds that:
\begin{itemize}
\item
 $\lnot\sees{\aterm_1}{\aterm_2}{\terms{\asetvar}} \inside \aformula$ or (otherwise) there is exactly one $\inbound \in \interval{1}{\bound}$ such that
${\seesgeq{\aterm_1}{\aterm_2}{\terms{\asetvar}}{\inbound}} \inside \aformula$. Moreover, in the second case, if $\inbound < \bound$ then\\
$\lnot \seesgeq{\aterm_1}{\aterm_2}{\terms{\asetvar}}{\inbound{+}1} \inside \aformula$.
No other $\lnot\seesgeq{\aterm_1}{\aterm_2}{\asetmeetvar}{\inbound'}$ belongs to $\literals{\aformula}$.
\end{itemize}
Moreover, as we said previously, if for some $\inbound$ it holds that $\seesgeq{\aterm_1}{\aterm_2}{\terms{\asetvar}}{\inbound} \inside \aformula$ then we are able to conclude $\prove_{\coresys} \aformula \implies \sees{\aterm_1}{\aterm_{2}}{\terms{\asetvar}}$ by axiom~\ref{core2Ax:SeesMono1}.
Hence, to prove the statement above we can equivalently prove that \elseabsurd{$\atree_{G_\avariable}([\aterm_1]) = [\aterm_2]$}{ $\lnot\sees{\aterm_1}{\aterm_2}{\terms{\asetvar}} \not\inside\aformula$}
By absurd, suppose $\lnot\sees{\aterm_1}{\aterm_2}{\terms{\asetvar}} \inside\aformula$.
As we have by hypothesis $\atree_{G_\avariable}([\aterm_1]) = [\aterm_2]$, from the points~\ref{proofcomp:point3} and~\ref{proofcomp:point4} of the proof, there is  $\avariablebis \in G_\avariable$ such that
$[\aterm_1],[\aterm_2] \in M_\avariablebis/\approx$.
By definition of $\atree_{G_\avariable}$ (see also  the property~\ref{pathx:1b} in point~\ref{proofcomp:point2} of the proof), $\before{\aterm_1}{\aterm_2} \inside \aformula$ and there is no $\aterm \in \terms{\asetvar}$ such that $[\aterm] \in M_\avariablebis/\approx$ and
$\before{\aterm_1}{\aterm} \land \before{\aterm}{\aterm_2} \inside \aformula$.
\elseabsurd{$\before{\aterm_1}{\aterm_2} \inside \aformula$ and~\ref{core2Ax:SeesBefore}}{$\prove_{\coresys} \aformula \implies \sees{\aterm_1}{\aterm_2}{\emptyset}$}
By propositional calculus, we have
$\prove_{\coresys} \aformula \implies \bigwedge_{\aterm' \in \terms{\asetvar}} \sees{\aterm_1}{\aterm_2}{\{\aterm'\}} \lor \bigvee_{\aterm' \in \terms{\asetvar}} \lnot\sees{\aterm_1}{\aterm_2}{\{\aterm'\}}$.
However, if  we suppose that we are able to derive the first dijunct ($\bigwedge_{\aterm' \in \terms{\asetvar}} \sees{\aterm_1}{\aterm_2}{\{\aterm'\}}$), then by~\ref{core2Ax:SeesMax} we obtain $\prove_{\coresys} \aformula \implies \sees{\aterm_1}{\aterm_2}{\terms{\asetvar}}$,
in contradiction with the hypothesis $\lnot\sees{\aterm_1}{\aterm_2}{\terms{\asetvar}} \inside\aformula$.
Then, we conclude that $\prove_{\coresys} \aformula \implies \bigvee_{\aterm' \in \terms{\asetvar}} \lnot\sees{\aterm_1}{\aterm_2}{\{\aterm'\}}$.
Therefore there is $\aterm \in \terms{\asetvar}$ such that $\prove_{\coresys} \aformula \implies \lnot\sees{\aterm_1}{\aterm_2}{\{\aterm\}}$.
\elseabsurd{\ref{core2Ax:SeesElsewhere}, as we also have $\before{\aterm_1}{\aterm_2} \inside \aformula$}{
$\prove_{\coresys} \aformula \implies \before{\aterm_1}{\aterm} \land \lnot \sees{\aterm_2}{\aterm}{\emptyset}$}
Moreover,
\elseabsurd{\ref{core2Ax:Self} and \ref{core2Ax:SeesTermEq}, as $\prove_{\coresys} \aformula \implies \lnot\sees{\aterm_1}{\aterm_2}{\{\aterm\}}$}{$\aterm \neq \aterm_2 \inside \aformula$}
Now, $\before{\aterm_1}{\aterm} \inside \aformula$ implies from the point~\ref{proofcomp:point3} of the proof that $[\aterm ]\in M_\avariablebis/\approx$.
\elseabsurd{\ref{axiom2:beforefunc}}{$\prove_{\coresys} \aformula \implies \before{\aterm}{\aterm_2} \lor \before{\aterm_2}{\aterm}$}
As we already have that $\prove_{\coresys} \aformula \implies \lnot\sees{\aterm_2}{\aterm}{\emptyset}$, the second disjunct (i.e. $\before{\aterm_2}{\aterm}$) cannot hold as otherwise by axiom \ref{core2Ax:SeesBefore}
we would be able to derive $\prove_{\coresys} \aformula \implies \sees{\aterm_2}{\aterm}{\emptyset}$ and then by propositional calculus $\prove_{\coresys} \aformula \implies \bottom$.
Then, we have $\prove_{\coresys} \aformula \implies \before{\aterm}{\aterm_2}$.
However, we now proved that there exists a term $\aterm \in \terms{\asetvar}$ such that
$[\aterm] \in M_\avariablebis/\approx$ and
$\before{\aterm_1}{\aterm} \land \before{\aterm}{\aterm_2} \inside \aformula$, which is absurd as $\atree_{G_\avariable}([\aterm_1]) = [\aterm_2]$.
Hence, $\lnot\sees{\aterm_1}{\aterm_2}{\terms{\asetvar}} \not\inside\aformula$.

\item $\boxed{\text{Path length and Rem}}$ Due to the fact that in the characteristic formula $\aformula$ subscripts of
$\mathtt{sees}$ and $\mathtt{rem}$ predicates are only indexed respectively by $\atermset{\asetvar}$ and $\atermset{\asetvar} \times \atermset{\asetvar}$
and
\begin{itemize}
\item for all terms $\aterm_1,\aterm_2 \in \terms{\asetvar}$,
 $\lnot\sees{\aterm_1}{\aterm_2}{\terms{\asetvar}} \inside \aformula$ or (otherwise) there is exactly one $\inbound \in \interval{1}{\bound}$ such that
${\seesgeq{\aterm_1}{\aterm_2}{\terms{\asetvar}}{\inbound}} \inside \aformula$. Moreover, in the second case, if $\inbound < \bound$ then
$\lnot \seesgeq{\aterm_1}{\aterm_2}{\terms{\asetvar}}{\inbound{+}1} \inside \aformula$.
For the same $\aterm_1,\aterm_2$,  no other $\lnot\seesgeq{\aterm_1}{\aterm_2}{\asetmeetvar}{\inbound'}$ belongs to $\literals{\aformula}$.
\item there is exacly one $\inbound \in \interval{0}{\bound}$ such that
$\remgeq{\atermset{\asetvar}\times\terms{\asetvar}}{\inbound} \inside \aformula$, and if $\inbound < \bound$ then $\lnot \remgeq{\atermset{\asetvar}\times\terms{\asetvar}}{\inbound{+}1} \inside \aformula$.
No other $\lnot\remgeq{\asetpath}{\inbound'}$ belongs to $\literals{\aformula}$.
\end{itemize}
The magnitude of $\inbound$ in $\seesgeq{\aterm}{\aterm'}{\atermset{\asetvar}}{\inbound}$ or $\remgeq{\atermset{\asetvar}\times\atermset{\asetvar}}\inbound$ does not play a role in the (un)satisfiablity of $\aformula$.
\end{enumerate}

Let $\atree$ be the union of all $(\atree_{G_\avariable})_{\avariable \in \asetvar}$. From the definition of $\atree_{G_\avariable}$ ($\avariable \in \asetvar$), $\atree$ is still a functional and acyclic relation (i.e.\ it represent a forest of trees).
Let $\aloop$ be partial function from $\atermset{\asetvar}/\approx$ to $\atermset{\asetvar}/\approx$ such that $\aloop(\asymbterm_1) = \asymbterm_2$ iff $\asymbterm_1 \not \in \domain{\atree}$ and
\begin{itemize}
\item $\ameetvar{\avariable}{\avariablebis}{\avariableter} \in \asymbterm_1$, $C_\avariable = \emptyset$ and there is $\inbound \in \interval{1}{\bound}$ such that
$\seesgeq{\ameetvar{\avariable}{\avariablebis}{\avariableter}}{\ameetvar{\avariable}{\avariablebis}{\avariableter}}{\atermset{\asetvar}}{\inbound} \inside \aformula$
\item or $C_\avariable \neq \emptyset$ and there is $\ameetvar{\avariablefour}{\avariablefifth}{\avariablesix} \in \asymbterm_2$ such that
$\ameetvar{\avariable}{\avariablebis}{\avariableter} \to \ameetvar{\avariablefour}{\avariablefifth}{\avariablesix}$ is the successor in the cyclic order of $C_\avariable \cup \{S_\avariable\}$ such that $\seesgeq{\ameetvar{\avariable}{\avariablebis}{\avariableter}}{\ameetvar{\avariablefour}{\avariablefifth}{\avariablesix}}{\terms{\asetvar}}{\inbound} \inside \aformula$, for some $\inbound \in \interval{1}{\bound}$.
\end{itemize}
From the points~\ref{proofcomp:point8},~\ref{proofcomp:point9} and~\ref{proofcomp:point10} of the proof, $\aloop$ is well-defined and functional.
As by definition $\domain{\atree} \cap \domain{\aloop} = \emptyset$, we denote with $\atree + \aloop$ their union

We now have all the ingredients to build a model for $\aformula$.
\begin{itemize}
\item Let $A = \{\alocation_{\asymbterm_1},\alocation_{\asymbterm_2},\dots,\alocation_{\asymbterm_n}\}\subseteq\LOC$ be $n$ distinct locations, where $\{\asymbterm_1,\dots,\asymbterm_n\}$ is the set of equialence classes of $\approx$.
Here, the subscript $\asymbterm_i$ is just used to distinguish between the locations of different equivalence classes and should be understood as an index.
\item Let $\asymbterm \in \domain{\atree+\aloop}$. From the points~\ref{proofcomp:point8},~\ref{proofcomp:point9} and~\ref{proofcomp:point10} of the proof, there is exactly one $\inbound \in \interval{1}{\bound}$
such that
$\seesgeq{\aterm_1}{\aterm_2}{\terms{\asetvar}}{\inbound} \in \aformula$ where $\aterm_1 \in \asymbterm$ and $\aterm_2 \in (\atree+\aloop)(\asymbterm)$. Let
$B_{\asymbterm} = \{\alocation_{(\asymbterm,1),\dots,\alocation_{(\asymbterm,\inbound-1)}}\}$
be $\inbound-1$ distinct locations (again, the subscripts $(\asymbterm,i)$ should be understood just as indices).
\item Let $R = \{\alocation^r_1,\dots,\alocation^r_\inbound\}$ a set of $\inbound$ different locations, where $\inbound \in \interval{1}{\bound}$ is such that
$\remgeq{\atermset{\asetvar}\times\atermset{\asetvar}}{\inbound} \inside \aformula$.
\end{itemize}
As $\LOC$ is countably infinite, we suppose moreover that we always selected different locations between each set that we introduced, i.e.
$R \cap A = \emptyset$, and for each $\asymbterm,\asymbterm' \in \domain{\atree+\aloop}$, $R \cap B_\asymbterm = \emptyset$, $B_\asymbterm \cap A = \emptyset$ and if $\asymbterm\neq\asymbterm'$ then $B_\asymbterm \cap B_{\asymbterm'} = \emptyset$.

A memory state satisfying $\aformula$ is $\pair{\astore}{\aheap}$ such that:
\begin{itemize}
\item $\astore(\avariable) = \alocation_{[\avariable]}$;
\item $\domain{\aheap} = R \cup \bigcup_{\asymbterm \in \domain{\atree+\aloop}} (\{\alocation_\asymbterm \} \cup B_{\asymbterm})$;
\item for every $\asymbterm \in \domain{\atree+\aloop}$,
\begin{itemize}
\item if $B_\asymbterm = \emptyset$ then $\aheap(\alocation_\asymbterm) = \alocation_{(\atree+\aloop)(\asymbterm)}$,
\item otherwise $\aheap(\alocation_\asymbterm) = \alocation_{(\asymbterm,1)}$, for each $i \in \interval{1}{\card{B_\asymbterm}-1}$, $\aheap(\alocation_{(\asymbterm,i)}) = \alocation_{(\asymbterm,i+1)}$ and
$\aheap(\alocation_{(\asymbterm,\card{B_\asymbterm})}) = \alocation_{(\atree+\aloop)(\asymbterm)}$;
\end{itemize}
\item for every $\alocation \in R$, $\aheap(\alocation) = \alocation$.
\end{itemize}
\end{proof}
