# Supplementary material for: A Complete Axiomatisation for Quantifier-Free Separation Logic
Source: arXiv:2006.05156 source file (2021-08-09)
Supplement: Supplementary file 9 [file proof-lemma-axiomstwosound.tex]

\begin{proof} A great amount of the axioms from System~\ref{axioms2:coreaxioms} can be easily proved sound. Below, we prove the soundness for
a selection of axioms whose proof requires more developments.

\textbf{Axioms from \ref{core2Ax:Self} to \ref{core2Ax:BothAsym}}
\begin{itemize}
\item The soundness of the  axioms from~\ref{core2Ax:Self} to~\ref{core2Ax:Bothdef}, as well as for the axiom~\ref{core2Ax:PedInv}, is straightforward.
\item Soundness of the axiom~\ref{core2Ax:EqDef}:
$\defined{\ameetvar{\avariable}{\avariablebis}{\avariableter}} \land
  \defined{\ameetvar{\avariable}{\avariablebis}{\avariablefour}} \Rightarrow \ameetvar{\avariable}{\avariablebis}{\avariableter} = \ameetvar{\avariable}{\avariablebis}{\avariablefour}
$.\\
Let $\pair{\astore}{\aheap}$ be a memory state s.t. $\pair{\astore}{\aheap} \models  \defined{\ameetvar{\avariable}{\avariablebis}{\avariableter}} \land
  \defined{\ameetvar{\avariable}{\avariablebis}{\avariablefour}}$.
As $\semantics{\ameetvar{\avariable}{\avariablebis}{\avariableter}}_{\astore,\aheap}$ is defined  (say equal to $\alocation$),
there are $\alength_1,\alength_2 \geq 0$ such that
\begin{itemize}
\item $\aheap^{\alength_1}(\astore(\avariable)) = \aheap^{\alength_2}(\astore(\avariablebis)) = \alocation$ and there is $\alength \geq 0$ such that  $\aheap^\alength(\alocation) = \astore(\avariableter)$;
\item for every $\alength_1' \in \interval{0}{\alength_1-1}$ and $\alength_2' \geq 0$,
$\aheap^{\alength_1'}(\astore(\avariable)) \neq \aheap^{\alength_2'}(\astore(\avariablebis))$.
\end{itemize}
As $\semantics{\ameetvar{\avariable}{\avariablebis}{\avariablefour}}_{\astore,\aheap}$ is defined  (say equal to $\alocation'$) ,
there are $\gamma_1,\gamma_2 \geq 0$ such that
\begin{itemize}
\item $\aheap^{\gamma_1}(\astore(\avariable)) = \aheap^{\gamma_2}(\astore(\avariablebis)) = \alocation'$ and there is $\alength' \geq 0$ such that  $\aheap^{\alength'}(\alocation') = \astore(\avariablefour)$;
\item for every $\gamma_1' \in \interval{0}{\gamma_1-1}$ and $\gamma_2' \geq 0$,
$\aheap^{\gamma_1'}(\astore(\avariable)) \neq \aheap^{\gamma_2'}(\astore(\avariablebis))$.
\end{itemize}
Combining the two types of inequality constraints, we can conclude that $\alength_1 = \gamma_1$ and therefore $\alocation = \alocation'$, i.e.
$\pair{\astore}{\aheap} \models \ameetvar{\avariable}{\avariablebis}{\avariableter} = \ameetvar{\avariable}{\avariablebis}{\avariablefour}$.

\item Soundness of the axiom~\ref{core2Ax:Pedix}:
$
\defined{\ameetvar{\avariable}{\avariablebis}{\avariableter}} \land \defined{\ameetvar{\avariableter}{\avariableter}{\avariablefifth}}
\Rightarrow \defined{\ameetvar{\avariable}{\avariablebis}{\avariablefifth}}
$.\\
Let $\pair{\astore}{\aheap}$ be a memory state such that $\pair{\astore}{\aheap} \models
\defined{\ameetvar{\avariable}{\avariablebis}{\avariableter}} \land \defined{\ameetvar{\avariableter}{\avariableter}{\avariablefifth}}$.
As $\defined{\ameetvar{\avariableter}{\avariableter}{\avariablefifth}}$ holds, there is a path from $\semantics{\avariableter}_{\astore,\aheap}$ to
 $\semantics{\avariablefifth}_{\astore,\aheap}$. As $\defined{\ameetvar{\avariable}{\avariablebis}{\avariableter}}$ holds,
$\semantics{\ameetvar{\avariable}{\avariablebis}{\avariableter}}_{\astore,\aheap}$ is defined, and
there are paths from $\semantics{\avariable}_{\astore,\aheap}$ to
 $\semantics{\avariableter}_{\astore,\aheap}$ and from $\semantics{\avariablebis}_{\astore,\aheap}$ to
 $\semantics{\avariableter}_{\astore,\aheap}$. By transitivity, there are paths
from $\semantics{\avariable}_{\astore,\aheap}$ to
 $\semantics{\avariablefifth}_{\astore,\aheap}$ and from $\semantics{\avariablebis}_{\astore,\aheap}$ to
 $\semantics{\avariablefifth}_{\astore,\aheap}$. So, $\semantics{\ameetvar{\avariable}{\avariablebis}{\avariablefifth}}_{\astore,\aheap}$ is defined, and
therefore  $\pair{\astore}{\aheap} \models \defined{\ameetvar{\avariable}{\avariablebis}{\avariablefifth}}$.

\item Soundness of the axiom~\ref{core2Ax:PedLinear}:
$$\defined{\ameetvar{\avariable}{\avariablebis}{\avariableter}} \land \defined{\ameetvar{\avariable}{\avariablefour}{\avariablefifth}} \Rightarrow \defined{\ameetvar{\avariableter}{\avariableter}{\avariablefifth}} \lor \defined{\ameetvar{\avariablefifth}{\avariablefifth}{\avariableter}}
$$
Let $\pair{\astore}{\aheap}$ be a memory state such that $\pair{\astore}{\aheap} \models
\defined{\ameetvar{\avariable}{\avariablebis}{\avariableter}} \land \defined{\ameetvar{\avariable}{\avariablefour}{\avariablefifth}}$.
Consequently, there are paths
\begin{itemize}
\item from $\semantics{\avariable}_{\astore,\aheap}$ to $\semantics{\avariableter}_{\astore,\aheap}$,
\item from $\semantics{\avariablebis}_{\astore,\aheap}$ to $\semantics{\avariableter}_{\astore,\aheap}$,
\item from $\semantics{\avariable}_{\astore,\aheap}$ to $\semantics{\avariablefifth}_{\astore,\aheap}$,
\item from $\semantics{\avariablefour}_{\astore,\aheap}$ to $\semantics{\avariablefifth}_{\astore,\aheap}$.
\end{itemize}
By functionality, one of the two situations occur:
\begin{enumerate}
\item There is a path from $\semantics{\avariable}_{\astore,\aheap}$ to $\semantics{\avariableter}_{\astore,\aheap}$ passing via
$\semantics{\avariablefifth}_{\astore,\aheap}$.
\item There is a path from $\semantics{\avariable}_{\astore,\aheap}$ to $\semantics{\avariablefifth}_{\astore,\aheap}$ passing via
$\semantics{\avariableter}_{\astore,\aheap}$.
\end{enumerate}
Hence, either there is a path from $\semantics{\avariableter}_{\astore,\aheap}$ to $\semantics{\avariablefifth}_{\astore,\aheap}$
(which can be expressed with $\defined{\ameetvar{\avariableter}{\avariableter}{\avariablefifth}}$)
or there is a path from $\semantics{\avariablefifth}_{\astore,\aheap}$ to $\semantics{\avariableter}_{\astore,\aheap}$
(which can be expressed with $\defined{\ameetvar{\avariablefifth}{\avariablefifth}{\avariableter}}$),
whence $\pair{\astore}{\aheap} \models \defined{\ameetvar{\avariableter}{\avariableter}{\avariablefifth}} \lor \defined{\ameetvar{\avariablefifth}{\avariablefifth}{\avariableter}}$.

\item Soundness of the axiom~\ref{core2Ax:PedDefines}: $\defined{\ameetvar{\avariable}{\avariablebis}{\avariableter}} \land \defined{\ameetvar{\avariablefour}{\avariablefifth}{\avariableter}} \Rightarrow \defined{\ameetvar{\avariable}{\avariablefour}{\avariableter}}$.

Let $\pair{\astore}{\aheap}$ be a memory state s.t.\ $\pair{\astore}{\aheap} \models  \defined{\ameetvar{\avariable}{\avariablebis}{\avariableter}} \land
  \defined{\ameetvar{\avariablefour}{\avariablefifth}{\avariableter}}$.
As $\semantics{\ameetvar{\avariable}{\avariablebis}{\avariableter}}_{\astore,\aheap}$ is defined (say equal to $\alocation$),
there are $\alength_1,\alength_2 \geq 0$ such that
\begin{itemize}
\item $\aheap^{\alength_1}(\astore(\avariable)) = \aheap^{\alength_2}(\astore(\avariablebis)) = \alocation$ and there is $\alength \geq 0$ such that  $\aheap^\alength(\alocation) = \astore(\avariableter)$;
\item for every $\alength_1' \in \interval{0}{\alength_1-1}$ and $\alength_2' \geq 0$,
$\aheap^{\alength_1'}(\astore(\avariable)) \neq \aheap^{\alength_2'}(\astore(\avariablebis))$.
\end{itemize}
As $\semantics{\ameetvar{\avariablefour}{\avariablefifth}{\avariableter}}_{\astore,\aheap}$ is defined  (say equal to $\alocation'$) ,
there are $\gamma_1,\gamma_2 \geq 0$ such that
\begin{itemize}
\item $\aheap^{\gamma_1}(\astore(\avariablefour)) = \aheap^{\gamma_2}(\astore(\avariablefifth)) = \alocation'$ and there is $\alength' \geq 0$ such that  $\aheap^{\alength'}(\alocation') = \astore(\avariableter)$;
\item for every $\gamma_1' \in \interval{0}{\gamma_1-1}$ and $\gamma_2' \geq 0$,
$\aheap^{\gamma_1'}(\astore(\avariablefour)) \neq \aheap^{\gamma_2'}(\astore(\avariablefifth))$.
\end{itemize}

Therefore, it holds that $\aheap^{\alength_1 + \alength}(\astore(\avariable)) = \astore(\avariableter)$ and $\aheap^{\gamma_1 + \alength'}(\astore(\avariablefour)) = \astore(\avariableter)$.
This is enough to conclude that there is $\widehat{\alocation}$ such that $\widehat{\alocation} = \semantics{\ameetvar{\avariable}{\avariablefour}{\avariableter}}_{\astore,\aheap}$. Indeed, there must be a location $\widehat{\alocation}$ in the minimal path from $\astore(\avariable)$ to $\astore(\avariableter)$ that is also reached by $\astore(\avariablefour)$ and such that its predecessor in the path is not reached by $\astore(\avariablefour)$. Then
$\widehat{\alocation} = \semantics{\ameetvar{\avariable}{\avariablefour}{\avariableter}}_{\astore,\aheap}$.

\item Soundness of the axiom~\ref{core2Ax:Before}:
$$\symmetric{\ameetvar{\avariable}{\avariablebis}{\avariableter}} \land \defined{\ameetvar{\avariable}{\avariablefour}{\avariableter}} \land
\ameetvar{\avariable}{\avariablefour}{\avariableter} \neq \ameetvar{\avariablebis}{\avariablefour}{\avariableter}
 \Rightarrow (
 \ameetvar{\avariable}{\avariablebis}{\avariableter} = \ameetvar{\avariable}{\avariablefour}{\avariableter}
 \lor
 \ameetvar{\avariable}{\avariablebis}{\avariableter} = \ameetvar{\avariablebis}{\avariablefour}{\avariableter}
 )$$

Suppose $\pair{\astore}{\aheap} \models \symmetric{\ameetvar{\avariable}{\avariablebis}{\avariableter}} \land \defined{\ameetvar{\avariable}{\avariablefour}{\avariableter}} \land
\ameetvar{\avariable}{\avariablefour}{\avariableter} \neq \ameetvar{\avariablebis}{\avariablefour}{\avariableter}
 \Rightarrow (
 \ameetvar{\avariable}{\avariablebis}{\avariableter} = \ameetvar{\avariable}{\avariablefour}{\avariableter}
 \lor
 \ameetvar{\avariable}{\avariablebis}{\avariableter} = \ameetvar{\avariablebis}{\avariablefour}{\avariableter}
 )$.
From $\pair{\astore}{\aheap} \models \symmetric{\ameetvar{\avariable}{\avariablebis}{\avariableter}}$, we conclude that one of the following two patterns must hold in $\aheap$:
\begin{center}
 \scalebox{0.85}{
     \begin{tikzpicture}[baseline]
       \node[dot,label=above:$\avariable$] (i) at (0,0) {};
       \node[dot,label=left:{$\ameetvar{\avariable}{\avariablebis}{\avariableter}$}] (m) [below right = 1.5cm and 0.5cm of i] {};
       \node[dot,label=above:$\avariablebis$] (j) [above right=1.5cm and 0.5cm of m] {};
       \node[dot,label=below:{$\avariableter$\\$\avariableter$ not inside a loop}] (k) [below of=m] {};

       \draw[reach] (i) -- (m);
       \draw[reach] (j) -- (m);
       \draw[reach] (m) -- (k);
     \end{tikzpicture}
     \quad
     \begin{tikzpicture}[baseline]
       \node[dot,label=above:$\avariable$] (i) at (0,0) {};
       \node[dot,label=left:{$\ameetvar{\avariable}{\avariablebis}{\avariableter}$}] (m) [below right = 1.5cm and 0.5cm of i] {};
       \node[dot,label=above:$\avariablebis$] (j) [above right=1.5cm and 0.5cm of m] {};
       \node[dot] (mid) [below=0.8cm of m] {};
       \node[dot,label=below:{$\avariableter$}] (k) [below=1.65cm of m] {};

       \draw[reach] (i) -- (m);
       \draw[reach] (j) -- (m);
       \draw[reach] (m) -- (mid);
       \draw[reach] (mid) to [out=-35,in=35] (k);
       \draw[pto] (k) to [out=155,in=-155] node [left] {$+$} (mid);
     \end{tikzpicture}
 }
\end{center}
Then, from $\pair{\astore}{\aheap} \models \defined{\ameetvar{\avariable}{\avariablefour}{\avariableter}}$
it holds that $\semantics{\ameetvar{\avariable}{\avariablefour}{\avariableter}}_{\astore,\aheap}$
must be a location reachable from $\astore(\avariable)$ ($\astore(\avariable)$ included).
By  $\pair{\astore}{\aheap} \models
\ameetvar{\avariable}{\avariablefour}{\avariableter} \neq \ameetvar{\avariablebis}{\avariablefour}{\avariableter}$,
it is easy to see that
$\semantics{\ameetvar{\avariable}{\avariablefour}{\avariableter}}_{\astore,\aheap}$
cannot be a location reachable from $\semantics{\ameetvar{\avariable}{\avariablebis}{\avariableter}}_{\astore,\aheap}$ in at least one step.
Hence, $\semantics{\ameetvar{\avariable}{\avariablefour}{\avariableter}}_{\astore,\aheap}$ must be a location in the path from $\astore(\avariable)$ to $\semantics{\ameetvar{\avariable}{\avariablebis}{\avariableter}}_{\astore,\aheap}$ (both ends included).
We distinguish two cases.
\begin{itemize}
\item If $\semantics{\ameetvar{\avariable}{\avariablebis}{\avariableter}}_{\astore,\aheap} = 
\semantics{\ameetvar{\avariable}{\avariablefour}{\avariableter}}_{\astore,\aheap}$,
then $\pair{\astore}{\aheap} \models \ameetvar{\avariable}{\avariablebis}{\avariableter} = \ameetvar{\avariable}{\avariablefour}{\avariableter}$.
\item Otherwise ($\semantics{\ameetvar{\avariable}{\avariablebis}{\avariableter}}_{\astore,\aheap} \neq \semantics{\ameetvar{\avariable}{\avariablefour}{\avariableter}}_{\astore,\aheap}$),
clearly $\semantics{\ameetvar{\avariable}{\avariablebis}{\avariableter}}_{\astore,\aheap}$ is the first location reached from $\astore(\avariablebis)$ that is also reached by $\astore(\avariablefour)$ (and reaches $\astore(\avariableter)$).
Hence, by definition of the meet-points, we have  $\semantics{\ameetvar{\avariable}{\avariablebis}{\avariableter}}_{\astore,\aheap} = \semantics{\ameetvar{\avariablebis}{\avariablefour}{\avariableter}}_{\astore,\aheap}$ and therefore
$\pair{\astore}{\aheap} \models \ameetvar{\avariable}{\avariablebis}{\avariableter} = \ameetvar{\avariablebis}{\avariablefour}{\avariableter}$.
\end{itemize}
We conclude that $\pair{\astore}{\aheap} \models  \ameetvar{\avariable}{\avariablebis}{\avariableter} = \ameetvar{\avariable}{\avariablefour}{\avariableter}
 \lor
 \ameetvar{\avariable}{\avariablebis}{\avariableter} = \ameetvar{\avariablebis}{\avariablefour}{\avariableter}$.

\item Soundness of the axiom~\ref{core2Ax:Symmetric}
$$\ameetvar{\avariable}{\avariablebis}{\avariableter} = \ameetvar{\avariablefour}{\avariablefifth}{\avariableter} \Rightarrow \symmetric{\ameetvar{\avariable}{\avariablefour}{\avariableter}} \land
(
\ameetvar{\avariable}{\avariablebis}{\avariableter} = \ameetvar{\avariable}{\avariablefour}{\avariableter} \lor
\ameetvar{\avariable}{\avariablebis}{\avariableter} = \ameetvar{\avariable}{\avariablefifth}{\avariableter}
)$$

Suppose $\pair{\astore}{\aheap} \models \ameetvar{\avariable}{\avariablebis}{\avariableter} = \ameetvar{\avariablefour}{\avariablefifth}{\avariableter}$.
By definition, $\semantics{\ameetvar{\avariable}{\avariablebis}{\avariableter}}_{\astore,\aheap}$ and $\semantics{\ameetvar{\avariablefour}{\avariablefifth}{\avariableter}}_{\astore,\aheap}$ are both defined (and equal).
Then, it is easy to see that $\pair{\astore}{\aheap} \models \defined{\ameetvar{\avariable}{\avariablefour}{\avariableter}}$, as it can be derived from 
the axiom~\ref{core2Ax:PedDefines} together with propositional reasoning.
Let us suppose by contradiction that $\pair{\astore}{\aheap} \not\models  \symmetric{\ameetvar{\avariable}{\avariablefour}{\avariableter}}$ and that, therefore (by definition of $\symmetric{\aterm}$ and $\asymmetric{\aterm}$) $\pair{\astore}{\aheap} \models \asymmetric{\ameetvar{\avariable}{\avariablefour}{\avariableter}}$.
Then, we concude that one of the following two patterns must hold in $\aheap$:
\begin{center}
\begin{tikzpicture}[baseline]
  \node[dot,label=above:$\avariable$] (i) at (0,0) {};
  \node[dot,label=left:{$\ameetvar{\avariable}{\avariablefour}{\avariablefifth}$}]
  (m1) [below right = 1.5cm and 0.4cm of i] {};
  \node[dot,label=right:{$\ameetvar{\avariablefour}{\avariable}{\avariablefifth}$}] (m2) [below right = 1.7cm and 0.4cm of m1] {};
  \node[dot,label=above:$\avariablefour$] (j) [above right=1.5cm and 0.5cm of m2] {};
  \node[dot,label=left:{$\avariablefifth$}] (k) [below right= 2.7cm and 0.1 of i] {};

  \draw[reach] (i) -- (m1);
  \draw[pto] (m1) to node [above right] {$+$} (m2);
  \draw[reach] (j) -- (m2);
  \draw[reach] (m2) to [out=180,in=-75] (k);
  \draw[pto] (k) to [bend left=30] node [left] {$+$} (m1);

\end{tikzpicture}
\qquad\qquad
\begin{tikzpicture}[baseline]
  \node[dot,label=above:$\avariablefour$] (i) at (0,0) {};
  \node[dot,label=left:{$\ameetvar{\avariablefour}{\avariable}{\avariablefifth}$}]
  (m1) [below right = 1.5cm and 0.4cm of i] {};
  \node[dot,label=right:{$\ameetvar{\avariable}{\avariablefour}{\avariablefifth}$}] (m2) [below right = 1.7cm and 0.4cm of m1] {};
  \node[dot,label=above:$\avariable$] (j) [above right=1.5cm and 0.5cm of m2] {};
  \node[dot,label=left:{$\avariablefifth$}] (k) [below right= 2.7cm and 0.1 of i] {};

  \draw[reach] (i) -- (m1);
  \draw[pto] (m1) to node [above right] {$+$} (m2);
  \draw[reach] (j) -- (m2);
  \draw[reach] (m2) to [out=180,in=-75] (k);
  \draw[pto] (k) to [bend left=30] node [left] {$+$} (m1);
\end{tikzpicture}
\end{center}
We recall that, informally, a meet-point of the form $\ameetvar{\avariable}{\avariablefifth}{\avariablesix}$, whenever defined w.r.t. $\pair{\astore}{\aheap}$, corresponds to the \emph{first} location reachable from $\astore(\avariable)$ that is also reached by $\astore(\avariablefifth)$ and reaches $\astore(\avariablesix)$.
It is therefore clear that (I) $\semantics{\ameetvar{\avariable}{\avariablebis}{\avariableter}}_{\astore,\aheap}$
must be a location in the path from $\astore(\avariable)$ to $\semantics{\ameetvar{\avariable}{\avariablefour}{\avariableter}}_{\astore,\aheap}$ (both ends included), as every other location reachable from $\astore(\avariable)$ belongs to a cycle but
it cannot be the first location of the cycle that is reachable from $\astore(\avariable)$ (as this location is
$\semantics{\ameetvar{\avariable}{\avariablefour}{\avariableter}}_{\astore,\aheap}$); hence it cannot correspond to meet-points of the form $\ameetvar{\avariable}{\avariablefifth}{\avariablesix}$.
Similarly, (II) $\semantics{\ameetvar{\avariablefour}{\avariablefifth}{\avariableter}}_{\astore,\aheap}$ must be a location in the path from $\astore(\avariablefour)$ to $\semantics{\ameetvar{\avariablefour}{\avariable}{\avariableter}}_{\astore,\aheap}$.
However, the two paths considered in (I) and (II) do not have any location in common, and therefore we conclude that  $\semantics{\ameetvar{\avariable}{\avariablebis}{\avariableter}}_{\astore,\aheap} \neq \semantics{\ameetvar{\avariablefour}{\avariablefifth}{\avariableter}}_{\astore,\aheap}$, in contradiction with
$\pair{\astore}{\aheap} \models \ameetvar{\avariable}{\avariablebis}{\avariableter} = \ameetvar{\avariablefour}{\avariablefifth}{\avariableter}$.
Hence, $\pair{\astore}{\aheap} \models \symmetric{\ameetvar{\avariable}{\avariablefour}{\avariableter}}$.

Now, we  show that $\pair{\astore}{\aheap} \models \ameetvar{\avariable}{\avariablebis}{\avariableter} = \ameetvar{\avariable}{\avariablefour}{\avariableter} \lor
\ameetvar{\avariable}{\avariablebis}{\avariableter} = \ameetvar{\avariable}{\avariablefifth}{\avariableter}$.
Let us consider the meet-point $\semantics{\ameetvar{\avariable}{\avariablebis}{\avariableter}}_{\astore,\aheap}$.
The possible patterns occurring in $\aheap$ w.r.t. these meet-points are depicted as follows:
\begin{center}
 \scalebox{0.85}{
     \begin{tikzpicture}[baseline]
       \node[dot,label=above:$\avariable$] (i) at (0,0) {};
       \node[dot,label=left:{$\ameetvar{\avariable}{\avariablebis}{\avariableter}$}] (m) [below right = 1.5cm and 0.5cm of i] {};
       \node[dot,label=above:$\avariablebis$] (j) [above right=1.5cm and 0.5cm of m] {};
       \node[dot,label=below:{$\avariableter$}] (k) [below of=m] {};

       \draw[reach] (i) -- (m);
       \draw[reach] (j) -- (m);
       \draw[reach] (m) -- (k);
     \end{tikzpicture}
     \qquad
     \begin{tikzpicture}[baseline]
       \node[dot,label=above:$\avariable$] (i) at (0,0) {};
       \node[dot,label=left:{$\ameetvar{\avariable}{\avariablebis}{\avariableter}$}]
       (m1) [below right = 1.5cm and 0.4cm of i] {};
       \node[dot,label=right:{$\ameetvar{\avariablebis}{\avariable}{\avariableter}$}] (m2) [below right = 1.7cm and 0.4cm of m1] {};
       \node[dot,label=above:$\avariablebis$] (j) [above right=1.5cm and 0.5cm of m2] {};
       \node[dot,label=left:{$\avariableter$}] (k) [below right= 2.7cm and 0.1 of i] {};

       \draw[reach] (i) -- (m1);
       \draw[pto] (m1) to node [above right] {$+$} (m2);
       \draw[reach] (j) -- (m2);
       \draw[reach] (m2) to [out=180,in=-75] (k);
       \draw[pto] (k) to [bend left=30] node [left] {$+$} (m1);
     \end{tikzpicture}
     \qquad
     \begin{tikzpicture}[baseline]
       \node[dot,label=above:$\avariablebis$] (i) at (0,0) {};
       \node[dot,label=left:{$\ameetvar{\avariablebis}{\avariable}{\avariableter}$}]
       (m1) [below right = 1.5cm and 0.4cm of i] {};
       \node[dot,label=right:{$\ameetvar{\avariable}{\avariablebis}{\avariableter}$}] (m2) [below right = 1.7cm and 0.4cm of m1] {};
       \node[dot,label=above:$\avariable$] (j) [above right=1.5cm and 0.5cm of m2] {};
       \node[dot,label=left:{$\avariableter$}] (k) [below right= 2.7cm and 0.1 of i] {};

       \draw[reach] (i) -- (m1);
       \draw[pto] (m1) to node [above right] {$+$} (m2);
       \draw[reach] (j) -- (m2);
       \draw[reach] (m2) to [out=180,in=-75] (k);
       \draw[pto] (k) to [bend left=30] node [left] {$+$} (m1);

     \end{tikzpicture}
 }
\end{center}
where the last two cases are essentially the same, the sole difference being whether $\astore(\avariable)$ reaches first the location correponding to $\ameetvar{\avariable}{\avariablebis}{\avariableter}$ or the one corresponding to $\ameetvar{\avariablebis}{\avariable}{\avariableter}$ (which does not play a role in the proof).
Let us consider the first case. In order to satisfy $\ameetvar{\avariable}{\avariablebis}{\avariableter} = \ameetvar{\avariablefour}{\avariablefifth}{\avariableter}$ (the hypothesis) one of the following must hold:
\begin{itemize}
  \item $\ameetvar{\avariable}{\avariablefour}{\avariableter}$ corresponds to a location in the path from $\astore(\avariable)$ to $\semantics{\ameetvar{\avariable}{\avariablebis}{\avariableter}}_{\astore,\aheap}$, and $\ameetvar{\avariablebis}{\avariablefifth}{\avariableter}$ corresponds to a location in the path from $\astore(\avariablebis)$ to
  $\semantics{\ameetvar{\avariable}{\avariablebis}{\avariableter}}_{\astore,\aheap}$.
  This case can be depicted as follows:
  \begin{center}
   \scalebox{0.85}{
       \begin{tikzpicture}[baseline]
         \node[dot,label=above:$\avariable$] (i) at (0,0) {};
         \node[dot,label=left:{$\ameetvar{\avariable}{\avariablebis}{\avariableter}$}] (m) [below right = 1.5cm and 0.5cm of i] {};
         \node[dot] (uu) [below right = 0.7cm and 0.2cm of i] {};
         \node[dot,label=above:$\avariablebis$] (j) [above right=1.5cm and 0.5cm of m] {};
         \node[dot] (vv) [below left = 0.7cm and 0.2cm of j] {};
         \node[dot,label=below:{$\avariableter$}] (k) [below of=m] {};

         \node[dot,label=left:$\avariablefour$] (u) [left = 1cm of uu] {};
         \node[dot,label=right:$\avariablefifth$] (v) [right = 1cm of vv] {};

         \draw[reach] (i) -- (uu);
         \draw[reach] (uu) -- (m);
         \draw[reach] (j) -- (vv);
         \draw[reach] (vv) -- (m);
         \draw[reach] (m) -- (k);
         \draw[reach] (u) -- (uu);
         \draw[reach] (v) -- (vv);
       \end{tikzpicture}
   }
  \end{center}
  Then, it is easy to show that $\semantics{\ameetvar{\avariable}{\avariablebis}{\avariableter}}_{\astore,\aheap} = \semantics{\ameetvar{\avariable}{\avariablefifth}{\avariableter}}_{\astore,\aheap}$.
  \item $\ameetvar{\avariable}{\avariablefifth}{\avariableter}$ corresponds to a location in the path from $\astore(\avariable)$ to $\semantics{\ameetvar{\avariable}{\avariablebis}{\avariableter}}_{\astore,\aheap}$, and $\ameetvar{\avariablebis}{\avariablefour}{\avariableter}$ corresponds to a location in the path from $\astore(\avariablebis)$ to
  $\semantics{\ameetvar{\avariable}{\avariablebis}{\avariableter}}_{\astore,\aheap}$.
  This case can be depicted as follows:
  \begin{center}
   \scalebox{0.85}{
       \begin{tikzpicture}[baseline]
         \node[dot,label=above:$\avariable$] (i) at (0,0) {};
         \node[dot,label=left:{$\ameetvar{\avariable}{\avariablebis}{\avariableter}$}] (m) [below right = 1.5cm and 0.5cm of i] {};
         \node[dot] (uu) [below right = 0.7cm and 0.2cm of i] {};
         \node[dot,label=above:$\avariablebis$] (j) [above right=1.5cm and 0.5cm of m] {};
         \node[dot] (vv) [below left = 0.7cm and 0.2cm of j] {};
         \node[dot,label=below:{$\avariableter$}] (k) [below of=m] {};

         \node[dot,label=left:$\avariablefifth$] (u) [left = 1cm of uu] {};
         \node[dot,label=right:$\avariablefour$] (v) [right = 1cm of vv] {};

         \draw[reach] (i) -- (uu);
         \draw[reach] (uu) -- (m);
         \draw[reach] (j) -- (vv);
         \draw[reach] (vv) -- (m);
         \draw[reach] (m) -- (k);
         \draw[reach] (u) -- (uu);
         \draw[reach] (v) -- (vv);
       \end{tikzpicture}
   }
  \end{center}
  Then, it is easy to show that $\semantics{\ameetvar{\avariable}{\avariablebis}{\avariableter}}_{\astore,\aheap} = \semantics{\ameetvar{\avariable}{\avariablefour}{\avariableter}}_{\astore,\aheap}$.
\end{itemize}
Then, for the first pattern we have $\pair{\astore}{\aheap} \models \ameetvar{\avariable}{\avariablebis}{\avariableter} = \ameetvar{\avariable}{\avariablefour}{\avariableter} \lor \ameetvar{\avariable}{\avariablebis}{\avariableter} = \ameetvar{\avariable}{\avariablefifth}{\avariableter}$.

Let us now consider (together) the second and third patterns.
As $\symmetric{\ameetvar{\avariable}{\avariablefour}{\avariableter}}$ holds in $\pair{\astore}{\aheap}$, it is easy to see that $\semantics{\ameetvar{\avariable}{\avariablefour}{\avariableter}}_{\astore,\aheap}$ must be a location in the path from $\astore(\avariable)$ to $\semantics{\ameetvar{\avariable}{\avariablebis}{\avariableter}}_{\astore,\aheap}$.
We then distinguish two cases:
\begin{itemize}
  \item $\semantics{\ameetvar{\avariable}{\avariablebis}{\avariableter}}_{\astore,\aheap} = \semantics{\ameetvar{\avariable}{\avariablefour}{\avariableter}}_{\astore,\aheap}$,
  which directly implies $\pair{\astore}{\aheap} \models \ameetvar{\avariable}{\avariablebis}{\avariableter} = \ameetvar{\avariable}{\avariablefour}{\avariableter} \lor \ameetvar{\avariable}{\avariablebis}{\avariableter} = \ameetvar{\avariable}{\avariablefifth}{\avariableter}$.
  \item $\semantics{\ameetvar{\avariable}{\avariablebis}{\avariableter}}_{\astore,\aheap} \neq \semantics{\ameetvar{\avariable}{\avariablefour}{\avariableter}}_{\astore,\aheap}$. Then, one of the following two patterns must occur in $\aheap$:
  \begin{center}
   \scalebox{0.85}{
       \begin{tikzpicture}[baseline]
         \node[dot,label=above:$\avariable$] (i) at (0,0) {};
         \node[dot]
         (uu) [below right = 0.7cm and 0.2cm of i] {};
         \node[dot,label=left:{$\avariablefour$}]
         (u) [left = 1cm of uu] {};
         \node[dot,label=left:{$\ameetvar{\avariable}{\avariablebis}{\avariableter}$}]
         (m1) [below right = 1.5cm and 0.4cm of i] {};
         \node[dot,label=right:{$\ameetvar{\avariablebis}{\avariable}{\avariableter}$}] (m2) [below right = 1.7cm and 0.4cm of m1] {};
         \node[dot,label=above:$\avariablebis$] (j) [above right=1.5cm and 0.5cm of m2] {};
         \node[dot,label=left:{$\avariableter$}] (k) [below right= 2.7cm and 0.1 of i] {};

         \draw[reach] (i) -- (uu);
         \draw[reach] (u) -- (uu);
         \draw[pto] (uu) to node [above right] {$+$} (m1);
         \draw[pto] (m1) to node [above right] {$+$} (m2);
         \draw[reach] (j) -- (m2);
         \draw[reach] (m2) to [out=180,in=-75] (k);
         \draw[pto] (k) to [bend left=30] node [left] {$+$} (m1);
       \end{tikzpicture}
       \qquad
       \begin{tikzpicture}[baseline]
         \node[dot,label=above:$\avariablebis$] (i) at (0,0) {};
         \node[dot,label=left:{$\ameetvar{\avariablebis}{\avariable}{\avariableter}$}]
         (m1) [below right = 1.5cm and 0.4cm of i] {};
         \node[dot,label=right:{$\ameetvar{\avariable}{\avariablebis}{\avariableter}$}] (m2) [below right = 1.7cm and 0.4cm of m1] {};
         \node[dot,label=above:$\avariable$] (j) [above right=1.5cm and 0.5cm of m2] {};
         \node[dot,label=left:{$\avariableter$}] (k) [below right= 2.7cm and 0.1 of i] {};
         \node[dot]
         (uu) [below left = 0.7cm and 0.2cm of j] {};
         \node[dot,label=right:{$\avariablefour$}]
         (u) [right = 1cm of uu] {};

        \draw[reach] (i) -- (m1);
        \draw[reach] (j) -- (uu);
        \draw[reach] (u) -- (uu);
        \draw[pto] (uu) to node [right] {$+$} (m2);
         \draw[pto] (m1) to node [above right] {$+$} (m2);
         \draw[reach] (m2) to [out=180,in=-75] (k);
         \draw[pto] (k) to [bend left=30] node [left] {$+$} (m1);

       \end{tikzpicture}
   }
  \end{center}
  Then, $\ameetvar{\avariable}{\avariablefifth}{\avariableter}$ corresponds to the location $\semantics{\ameetvar{\avariable}{\avariablebis}{\avariableter}}_{\astore,\aheap}$, as otherwise the hypothesis $\ameetvar{\avariable}{\avariablebis}{\avariableter} = \ameetvar{\avariablefour}{\avariablefifth}{\avariableter}$ is violated.
  Again, we obtain
  \begin{nscenter}
   $\pair{\astore}{\aheap} \models \ameetvar{\avariable}{\avariablebis}{\avariableter} = \ameetvar{\avariable}{\avariablefour}{\avariableter} \lor \ameetvar{\avariable}{\avariablebis}{\avariableter} = \ameetvar{\avariable}{\avariablefifth}{\avariableter}$,
   \end{nscenter}
   concluding the proof.
\end{itemize}

\item Soundness of the axiom~\ref{core2Ax:OneAsym}:
$$\symmetric{\ameetvar{\avariable}{\avariablebis}{\avariableter}} \land \asymmetric{\ameetvar{\avariable}{\avariablefour}{\avariablefifth}}
\Rightarrow \ameetvar{\avariablebis}{\avariablefour}{\avariablefifth} = \ameetvar{\avariable}{\avariablefour}{\avariablefifth} \land \ameetvar{\avariablefour}{\avariablebis}{\avariablefifth} = \ameetvar{\avariablefour}{\avariable}{\avariablefifth}$$

Suppose $\pair{\astore}{\aheap} \models \symmetric{\ameetvar{\avariable}{\avariablebis}{\avariableter}} \land \asymmetric{\ameetvar{\avariable}{\avariablefour}{\avariablefifth}}$.
From $\asymmetric{\ameetvar{\avariable}{\avariablefour}{\avariablefifth}}$, we conclude that one of the following patterns must hold in $\aheap$:
\begin{center}
\begin{tikzpicture}[baseline]
  \node[dot,label=above:$\avariable$] (i) at (0,0) {};
  \node[dot,label=left:{$\ameetvar{\avariable}{\avariablefour}{\avariablefifth}$}]
  (m1) [below right = 1.5cm and 0.4cm of i] {};
  \node[dot,label=right:{$\ameetvar{\avariablefour}{\avariable}{\avariablefifth}$}] (m2) [below right = 1.7cm and 0.4cm of m1] {};
  \node[dot,label=above:$\avariablefour$] (j) [above right=1.5cm and 0.5cm of m2] {};
  \node[dot,label=left:{$\avariablefifth$}] (k) [below right= 2.7cm and 0.1 of i] {};

  \draw[reach] (i) -- (m1);
  \draw[pto] (m1) to node [above right] {$+$} (m2);
  \draw[reach] (j) -- (m2);
  \draw[reach] (m2) to [out=180,in=-75] (k);
  \draw[pto] (k) to [bend left=30] node [left] {$+$} (m1);

\end{tikzpicture}
\qquad\qquad
\begin{tikzpicture}[baseline]
  \node[dot,label=above:$\avariablefour$] (i) at (0,0) {};
  \node[dot,label=left:{$\ameetvar{\avariablefour}{\avariable}{\avariablefifth}$}]
  (m1) [below right = 1.5cm and 0.4cm of i] {};
  \node[dot,label=right:{$\ameetvar{\avariable}{\avariablefour}{\avariablefifth}$}] (m2) [below right = 1.7cm and 0.4cm of m1] {};
  \node[dot,label=above:$\avariable$] (j) [above right=1.5cm and 0.5cm of m2] {};
  \node[dot,label=left:{$\avariablefifth$}] (k) [below right= 2.7cm and 0.1 of i] {};

  \draw[reach] (i) -- (m1);
  \draw[pto] (m1) to node [above right] {$+$} (m2);
  \draw[reach] (j) -- (m2);
  \draw[reach] (m2) to [out=180,in=-75] (k);
  \draw[pto] (k) to [bend left=30] node [left] {$+$} (m1);
\end{tikzpicture}
\end{center}
Now, since $\pair{\astore}{\aheap} \models \symmetric{\ameetvar{\avariable}{\avariablebis}{\avariableter}}$,
the location $\semantics{\ameetvar{\avariable}{\avariablebis}{\avariableter}}_{\astore,\aheap}$ must be in the path from $\astore(\avariable)$ to $\semantics{\ameetvar{\avariable}{\avariablefour}{\avariablefifth}}_{\astore,\aheap}$.
Because of this, since (informally) $\semantics{\ameetvar{\avariablebis}{\avariablefour}{\avariablefifth}}_{\astore,\aheap}$ is
the first location reachable from $\astore(\avariablebis)$ that reaches $\astore(\avariablefifth)$ and is reached by $\astore(\avariablefour)$, it must hold that $\semantics{\ameetvar{\avariablebis}{\avariablefour}{\avariablefifth}}_{\astore,\aheap} = \semantics{\ameetvar{\avariable}{\avariablefour}{\avariablefifth}}$.
Similarly, as $\semantics{\ameetvar{\avariablefour}{\avariablebis}{\avariablefifth}}_{\astore,\aheap}$ is the first location reachable from $\astore(\avariablefour)$ that reaches $\astore(\avariablefifth)$ and is reached by $\astore(\avariablebis)$, it is possible to show that
$\semantics{\ameetvar{\avariablefour}{\avariablebis}{\avariablefifth}}_{\astore,\aheap} = \semantics{\ameetvar{\avariablefour}{\avariable}{\avariablefifth}}$.
Hence, $\pair{\astore}{\aheap} \models \ameetvar{\avariablefour}{\avariablebis}{\avariablefifth} = \ameetvar{\avariablefour}{\avariable}{\avariablefifth}$.

\item Soundness of the axiom~\ref{core2Ax:BothAsym}:
$$
\asymmetric{\ameetvar{\avariable}{\avariablebis}{\avariableter}} \land \asymmetric{\ameetvar{\avariable}{\avariablefour}{\avariablefifth}} \Rightarrow \ameetvar{\avariable}{\avariablebis}{\avariableter} = \ameetvar{\avariable}{\avariablefour}{\avariablefifth}.
$$

This axiom is pretty straightforward.
Suppose $\pair{\astore}{\aheap} \models \asymmetric{\ameetvar{\avariable}{\avariablebis}{\avariableter}} \land \asymmetric{\ameetvar{\avariable}{\avariablefour}{\avariablefifth}}$.
From $\asymmetric{\ameetvar{\avariable}{\avariablebis}{\avariableter}}$, we can easily deduce that $\semantics{\ameetvar{\avariable}{\avariablebis}{\avariableter}}_{\astore,\aheap}$ is defined and it is such that
$\semantics{\ameetvar{\avariable}{\avariablebis}{\avariableter}}_{\astore,\aheap} \neq \semantics{\ameetvar{\avariablebis}{\avariable}{\avariableter}}_{\astore,\aheap}$.
Then, from the definition of meet-point, we conclude that one of the following patterns must hold in $\aheap$:
\begin{center}
\begin{tikzpicture}[baseline]
  \node[dot,label=above:$\avariable$] (i) at (0,0) {};
  \node[dot,label=left:{$\ameetvar{\avariable}{\avariablebis}{\avariableter}$}]
  (m1) [below right = 1.5cm and 0.4cm of i] {};
  \node[dot,label=right:{$\ameetvar{\avariablebis}{\avariable}{\avariableter}$}] (m2) [below right = 1.7cm and 0.4cm of m1] {};
  \node[dot,label=above:$\avariablebis$] (j) [above right=1.5cm and 0.5cm of m2] {};
  \node[dot,label=left:{$\avariableter$}] (k) [below right= 2.7cm and 0.1 of i] {};

  \draw[reach] (i) -- (m1);
  \draw[pto] (m1) to node [above right] {$+$} (m2);
  \draw[reach] (j) -- (m2);
  \draw[reach] (m2) to [out=180,in=-75] (k);
  \draw[pto] (k) to [bend left=30] node [left] {$+$} (m1);

\end{tikzpicture}
\qquad\qquad
\begin{tikzpicture}[baseline]
  \node[dot,label=above:$\avariablebis$] (i) at (0,0) {};
  \node[dot,label=left:{$\ameetvar{\avariablebis}{\avariable}{\avariableter}$}]
  (m1) [below right = 1.5cm and 0.4cm of i] {};
  \node[dot,label=right:{$\ameetvar{\avariable}{\avariablebis}{\avariableter}$}] (m2) [below right = 1.7cm and 0.4cm of m1] {};
  \node[dot,label=above:$\avariable$] (j) [above right=1.5cm and 0.5cm of m2] {};
  \node[dot,label=left:{$\avariableter$}] (k) [below right= 2.7cm and 0.1 of i] {};

  \draw[reach] (i) -- (m1);
  \draw[pto] (m1) to node [above right] {$+$} (m2);
  \draw[reach] (j) -- (m2);
  \draw[reach] (m2) to [out=180,in=-75] (k);
  \draw[pto] (k) to [bend left=30] node [left] {$+$} (m1);

\end{tikzpicture}
\end{center}
Specifically, $\semantics{\ameetvar{\avariable}{\avariablebis}{\avariableter}}_{\astore,\aheap}$ must be the first location reachable from $\astore(\avariable)$ that belongs to a cycle. Since $\asymmetric{\ameetvar{\avariable}{\avariablefour}{\avariablefifth}}$ is satisfied by $\pair{\astore}{\aheap}$, can apply the same reasoning on $\semantics{\ameetvar{\avariable}{\avariablefour}{\avariablefifth}}$ and conclude that it must again be the first location reachable from $\astore(\avariable)$
that belongs to a cycle. By functionality of our models, we then conclude:
$\semantics{\ameetvar{\avariable}{\avariablebis}{\avariableter}}_{\astore,\aheap} = \semantics{\ameetvar{\avariable}{\avariablefour}{\avariablefifth}}$ and therefore $\pair{\astore}{\aheap} \models
\ameetvar{\avariable}{\avariablebis}{\avariableter} = \ameetvar{\avariable}{\avariablefour}{\avariablefifth}$.

\end{itemize}

\textbf{Axioms from \ref{core2Ax:SeesTermEq} to \ref{core2Ax:SeesLoopOrder}}
\begin{itemize}
\item The soundness for the axioms from~\ref{core2Ax:SeesTermEq} to~\ref{core2Ax:SeesMono2}, as well as for
the axioms~\ref{core2Ax:SeesDef},~\ref{core2Ax:SeesMax} is straightforward.
\item Soundness of the axiom~\ref{core2Ax:SeesFunc}:
$
\sees{\aterm_1}{\aterm_2}{\{\aterm_3\}} \land \sees{\aterm_1}{\aterm_3}{\{\aterm_2\}} \Rightarrow \aterm_2 = \aterm_3
$.

Let $\pair{\astore}{\aheap}$ be a memory state such that $\pair{\astore}{\aheap} \models
\sees{\aterm_1}{\aterm_2}{\{\aterm_3\}} \land \sees{\aterm_1}{\aterm_3}{\{\aterm_2\}}$.
So there is a path $\alocation_1 = \semantics{\aterm_1}_{\astore,\aheap} \mapsto \alocation_2 \mapsto \cdots \mapsto \alocation_{N_1} = \semantics{\aterm_2}_{\astore,\aheap}$
such that $N_1 > 1$ and $\semantics{\aterm_3}_{\astore,\aheap},\semantics{\aterm_2}_{\astore,\aheap}   \not \in \set{\alocation_2, \ldots, \alocation_{N_1-1}}$.
Similarly, there is a path $\alocation_1' = \semantics{\aterm_1}_{\astore,\aheap} \mapsto \alocation_2' \mapsto \cdots \mapsto \alocation_{N_2}' = \semantics{\aterm_3}_{\astore,\aheap}$
such that $N_2 > 1$ and $\semantics{\aterm_2}_{\astore,\aheap},\semantics{\aterm_3}_{\astore,\aheap} \not \in \set{\alocation_2', \ldots, \alocation_{N_2-1}'}$.
Because of functionality, we have $\alocation_1 = \alocation_1'$, \ldots, $\alocation_N = \alocation_N'$ with $N = \min(N_1,N_2)$. Then, the constraints
about the non-occurrences of $\semantics{\aterm_3}_{\astore,\aheap}$ and $\semantics{\aterm_2}_{\astore,\aheap}$ lead to $N_1 = N_2$. Hence,
$\semantics{\aterm_2}_{\astore,\aheap} = \semantics{\aterm_3}_{\astore,\aheap}$ and therefore $\pair{\astore}{\aheap} \models \aterm_2 = \aterm_3$.

\item Soundness of the axiom~\ref{core2Ax:SeesEWCycl}:
$
\sees{\aterm_1}{\aterm_1}{\emptyset} {\land} \lnot \sees{\aterm_1}{\aterm_1}{\{\aterm_2\}}  \iff \sameloop{\aterm_1}{\aterm_2}
$.\\
Let $\pair{\astore}{\aheap}$ be a memory state such that $\pair{\astore}{\aheap} \models
\sees{\aterm_1}{\aterm_1}{\emptyset} {\land} \lnot \sees{\aterm_1}{\aterm_1}{\{\aterm_2\}}$.
The satisfaction of $\sees{\aterm_1}{\aterm_1}{\emptyset}$ enforces that
$\semantics{\aterm_1}_{\astore,\aheap}$ belongs to a cycle and the satisfaction of $\neg \sees{\aterm_1}{\aterm_1}{\{\aterm_2\}}$
enforces that $\semantics{\aterm_2}_{\astore,\aheap}$ belongs to that cycle. Consequently,
$\semantics{\aterm_1}_{\astore,\aheap} {\neq} \semantics{\aterm_2}_{\astore,\aheap}$ and
there is a cycle  with both $\semantics{\aterm_1}_{\astore,\aheap}$, $\semantics{\aterm_2}_{\astore,\aheap}$, which precisely means
that $\sameloop{\aterm_1}{\aterm_2}$ holds. The other direction is proved in a similar way.

\item Soundness of the axiom~\ref{core2Ax:SeesBefore}:
$
\before{\aterm_1}{\aterm_2} \Rightarrow \sees{\aterm_1}{\aterm_2}{\emptyset}
$.\\
Let $\pair{\astore}{\aheap}$ be a memory state such that $\pair{\astore}{\aheap} \models \before{\aterm_1}{\aterm_2}$.
This means that $\semantics{\aterm_1}_{\astore,\aheap} {\neq} \semantics{\aterm_2}_{\astore,\aheap}$ and,
there is a path from $\semantics{\aterm_1}_{\astore,\aheap}$ to $\semantics{\aterm_2}_{\astore,\aheap}$
such that the only location on the path that may belong to a cycle is $\semantics{\aterm_2}_{\astore,\aheap}$. Obviously, the path is of length
at least one, and therefore there is $\delta \geq 1$ such that (a) $\aheap^{\delta}(\semantics{\aterm_1}_{\astore,\aheap}) = \semantics{\aterm_2}_{\astore,\aheap}$
and (b) for all $\delta' \in \interval{1}{\delta-1}$, $\aheap^{\delta'}(\semantics{\aterm_1}_{\astore,\aheap}) \not \in
\set{\semantics{\aterm_2}_{\astore,\aheap}} \cup \emptyset$. This means precisely that $\sees{\aterm_1}{\aterm_2}{\emptyset}$ on $\pair{\astore}{\aheap}$.

\item Soundness of the axiom~\ref{core2Ax:SeesSum}:
\begin{nscenter}
$
\begin{aligned}[t]
&\seesgeq{\aterm_1}{\aterm_2}{\asetmeetvar}{\inbound_1}\!\land \seesgeq{\aterm_2}{\aterm_3}{\asetmeetvar}{\inbound_2} \land \aterm_2 {\not\in}\asetmeetvar \land \aterm_3 {\in} \asetmeetvar\\
  &\qquad\qquad
  \Rightarrow \seesgeq{\aterm_1}{\aterm_3}{\asetmeetvar}{\inbound_1{+}\inbound_2} \land \lnot \sees{\aterm_1}{\aterm_3}{\{\aterm_2\}}
\end{aligned}$
\end{nscenter}

Let $\pair{\astore}{\aheap}$ be a memory state such that $\pair{\astore}{\aheap} \models
\seesgeq{\aterm_1}{\aterm_2}{\asetmeetvar}{\inbound_1}\!\land \seesgeq{\aterm_2}{\aterm_3}{\asetmeetvar}{\inbound_2} \land \aterm_2 {\not\in}\asetmeetvar \land \aterm_3 {\in} \asetmeetvar$.
So there is a path $\alocation_1 = \semantics{\aterm_1}_{\astore,\aheap} \mapsto \alocation_2 \mapsto \cdots \mapsto \alocation_{\inbound_1+1} = \semantics{\aterm_2}_{\astore,\aheap}$
such that $\inbound_1 \geq 1$ (hence the path is of length $\inbound_1$) and $\semantics{\aterm_2}_{\astore,\aheap} \not \in \set{\alocation_2, \ldots, \alocation_{\inbound_1}}$.
Similarly, there is a path $\alocation_1' = \semantics{\aterm_2}_{\astore,\aheap} \mapsto \alocation_2' \mapsto \cdots \mapsto \alocation_{\inbound_2+1}' = \semantics{\aterm_3}_{\astore,\aheap}$
such that $\inbound_2 \geq 1$ (hence the path is of length $\inbound_2$) and $\semantics{\aterm_3}_{\astore,\aheap} \not \in \set{\alocation_2', \ldots, \alocation_{\inbound_2}'}$.
From $\pair{\astore}{\aheap} \models \aterm_3 {\in} \asetmeetvar$ we conclude that $\semantics{\aterm_3}_{\astore,\aheap} \not \in \set{\alocation_2, \ldots, \alocation_{\inbound_1}}$
and, as instead $\pair{\astore}{\aheap} \models \aterm_2 {\not\in} \asetmeetvar$, we obtain also that $\semantics{\aterm_3}_{\astore,\aheap} \neq \semantics{\aterm_2}_{\astore,\aheap}$. Hence, \textbf{($\dagger$)}
$\semantics{\aterm_3}_{\astore,\aheap} \not \in \set{\alocation_2, \ldots, \alocation_{\inbound_1}, \alocation_{\inbound_1+1} = \alocation_1' , \alocation_2', \ldots, \alocation_{\inbound_2}'}$.
Moreover, for every term $\widehat{\aterm} \in \asetmeetvar$ it also holds that
$\semantics{\widehat{\aterm}}_{\astore,\aheap} \not \in \set{\alocation_2, \ldots, \alocation_{\inbound_1}, \alocation_{\inbound_1+1} = \alocation_1' , \alocation_2', \ldots, \alocation_{\inbound_2}'}$.
This, together with \textbf{($\dagger$)} allows us to concldue that
$\pair{\astore}{\aheap} \models \seesgeq{\aterm_1}{\aterm_3}{\asetmeetvar}{\inbound_1{+}\inbound_2}$.

Now, to show that $\pair{\astore}{\aheap} \models \lnot \sees{\aterm_1}{\aterm_3}{\{\aterm_2\}}$, suppose ad absurdum the opposite, i.e.\ $\pair{\astore}{\aheap} \models \sees{\aterm_1}{\aterm_3}{\{\aterm_2\}}$.
As
$\pair{\astore}{\aheap} \models
\seesgeq{\aterm_1}{\aterm_2}{\asetmeetvar}{\inbound_1}\!\land \seesgeq{\aterm_2}{\aterm_3}{\asetmeetvar}{\inbound_2}$, this
 implies that $\semantics{\aterm_1}_{\astore,\aheap} = \semantics{\aterm_2}_{\astore,\aheap}$ or  $\semantics{\aterm_2}_{\astore,\aheap} = \semantics{\aterm_3}_{\astore,\aheap}$.
 However from $\pair{\astore}{\aheap} \models \aterm_2 {\not\in}\asetmeetvar \land \aterm_3 {\in} \asetmeetvar$
it follows that $\semantics{\aterm_2}_{\astore,\aheap} \neq \semantics{\aterm_3}_{\astore,\aheap}$ and therefore it should hold that
$\semantics{\aterm_1}_{\astore,\aheap} = \semantics{\aterm_2}_{\astore,\aheap}$.
Thanks to this, we derive that
 $\pair{\astore}{\aheap} \models
\seesgeq{\aterm_1}{\aterm_1}{\asetmeetvar}{\inbound_1}\!\land \seesgeq{\aterm_1}{\aterm_3}{\asetmeetvar}{\inbound_2} \land \aterm_1 \neq \aterm_3$, meaning that $\aterm_3$ is strictly in between the minimal path from
$\semantics{\aterm_1}_{\astore,\aheap}$ and $\semantics{\aterm_2}_{\astore,\aheap}$. This is impossible as
$\pair{\astore}{\aheap} \models
\seesgeq{\aterm_1}{\aterm_2}{\asetmeetvar}{\inbound_1} \land \aterm_3 {\in} \asetmeetvar$. Hence, we reached a contradiction and therefore  $\pair{\astore}{\aheap} \models \lnot \sees{\aterm_1}{\aterm_3}{\{\aterm_2\}}$.

\item Soundness of the axiom~\ref{core2Ax:SeesNegSum}:
$$
\seesgeq{\aterm_1}{\aterm_3}{\asetmeetvar}{\inbound} \land \lnot \sees{\aterm_1}{\aterm_3}{\{\aterm_2\}} \Rightarrow
{\bigvee_{\mathrlap{
  \raisebox{-0.2cm}[0pt][0pt]{$\kern-1em\scriptstyle{\inbound_1+\inbound_2=\max(2,\inbound)-2}$}}}
}
(\seesgeq{\aterm_1}{\aterm_2}{\asetmeetvar}{\inbound_1{+}1} \land \seesgeq{\aterm_2}{\aterm_3}{\asetmeetvar}{\inbound_2{+}1})
$$
Let $\pair{\astore}{\aheap}$ be a memory state such that $\pair{\astore}{\aheap} \models
\seesgeq{\aterm_1}{\aterm_3}{\asetmeetvar}{\inbound} \land \lnot \sees{\aterm_1}{\aterm_3}{\{\aterm_2\}}$.
By definition of $\models$,  there is $\delta \geq \inbound$ such that (a)
$\aheap^{\delta}(\semantics{\aterm_1}_{\astore,\aheap}) = \semantics{\aterm_3}_{\astore,\aheap}$
and (b) for all $\delta' \in \interval{1}{\delta-1}$, $\aheap^{\delta'}(\semantics{\aterm_1}_{\astore,\aheap}) \not \in
\set{\semantics{\aterm_3}_{\astore,\aheap}} \cup \set{\semantics{\aterm}_{\astore,\aheap} \mid \aterm \in \asetmeetvar}$.
Moreover, there is $\delta_0 \in \interval{1}{\delta-1}$ such that $\aheap^{\delta_0}(\semantics{\aterm_1}_{\astore,\aheap}) =
\semantics{\aterm_2}_{\astore,\aheap}$.
Hence,
\begin{itemize}
\item $\inbound \geq 2$,
\item for all $\delta' \in \interval{1}{\delta_0-1}$, $\aheap^{\delta'}(\semantics{\aterm_1}_{\astore,\aheap}) \not \in
\set{\semantics{\aterm_3}_{\astore,\aheap}} \cup \set{\semantics{\aterm}_{\astore,\aheap} \mid \aterm \in \asetmeetvar}$,
\item for all $\delta' \in \interval{1}{(\delta - \delta_0)-1}$, $\aheap^{\delta'}(\semantics{\aterm_3}_{\astore,\aheap}) \not \in
\set{\semantics{\aterm_2}_{\astore,\aheap}} \cup \set{\semantics{\aterm}_{\astore,\aheap} \mid \aterm \in \asetmeetvar}$.
\end{itemize}
So, $\pair{\astore}{\aheap} \models \sees{\aterm_1}{\aterm_2}{\asetmeetvar} \land \sees{\aterm_2}{\aterm_3}{\asetmeetvar}$.
Let us handle now the quantities.
\begin{enumerate}
\item If $\delta_0 \geq \inbound$, then let us define $\inbound_1 = \inbound -2$ and $\inbound_2 = 0$.
\item Otherwise, we define $\inbound_1 = \delta_0 -1$ and $\inbound_2 = \inbound -\delta_0 -1$.
\end{enumerate}
In both cases, one can check that $\inbound_1 + \inbound_2 = \inbound -2 = \max(2,\inbound)-2$
and moreover, we have $\pair{\astore}{\aheap} \models
\seesgeq{\aterm_1}{\aterm_2}{\asetmeetvar}{\inbound_1{+}1} \land \seesgeq{\aterm_2}{\aterm_3}{\asetmeetvar}{\inbound_2{+}1}$.

\item Soundenss of the axiom~\ref{core2Ax:SeesSubscript}:
$\sees{\ameetvar{\avariable}{\avariablebis}{\avariableter}}{\ameetvar{\avariablefour}{\avariablefifth}{\avariablesix}}{\asetmeetvar} \implies \defined{\ameetvar{\avariable}{\avariablebis}{\avariablesix}}$.\\

Suppose $\pair{\astore}{\aheap} \models \sees{\ameetvar{\avariable}{\avariablebis}{\avariableter}}{\ameetvar{\avariablefour}{\avariablefifth}{\avariablesix}}{\asetmeetvar}$.
By definition, there is $\alength \geq 1$ such that $\aheap^\alength(\semantics{\ameetvar{\avariable}{\avariablebis}{\avariableter}}_{\astore,\aheap}) = \semantics{\ameetvar{\avariablefour}{\avariablefifth}{\avariablesix}}_{\astore,\aheap}$.
Hence, $\semantics{\ameetvar{\avariable}{\avariablebis}{\avariableter}}_{\astore,\aheap}$
and $\semantics{\ameetvar{\avariablefour}{\avariablefifth}{\avariablesix}}_{\astore,\aheap}$
are defined (as also reflected by axiom~\ref{core2Ax:SeesDef}).
There are $\alength' \geq 0$, $\alength'' \geq 0$ and $\alength''' \geq 0$ such that
$\aheap^{\alength'}(\astore(\avariable)) = \semantics{\ameetvar{\avariable}{\avariablebis}{\avariableter}}_{\astore,\aheap}$,
$\aheap^{\alength''}(\astore(\avariablebis)) = \semantics{\ameetvar{\avariable}{\avariablebis}{\avariableter}}_{\astore,\aheap}$
and $\aheap^{\alength'''}(\semantics{\ameetvar{\avariablefour}{\avariablefifth}{\avariablesix}}_{\astore,\aheap}) = \astore(\avariablesix)$.
Hence there is a path of length $\alength'+\alength+\alength''' \geq 1$ from $\astore(\avariable)$ to $\astore(\avariablesix)$.
Similarly, there is a path of length $\alength''+\alength+\alength''' \geq 1$ from $\astore(\avariablebis)$ to $\astore(\avariablesix)$.
We then conclude that $\semantics{\ameetvar{\avariable}{\avariablebis}{\avariablesix}}_{\astore,\aheap}$ must be
defined and therefore $\pair{\astore}{\aheap} \models \defined{\ameetvar{\avariable}{\avariablebis}{\avariablesix}}$.

\item Soundness of the axiom~\ref{core2Ax:SeesToLoop}:
$$
\sees{\ameetvar{\avariable}{\avariablebis}{\avariableter}}{\ameetvar{\avariablefour}{\avariablefifth}{\avariablesix}}{\asetmeetvar} \land \asymmetric{\ameetvar{\avariable}{\avariablefour}{\avariablesix}}
\implies \ameetvar{\avariablefour}{\avariablefifth}{\avariablesix} = \ameetvar{\avariablefour}{\avariable}{\avariablesix}
$$

Briefly, suppose $\pair{\astore}{\aheap} \models \sees{\ameetvar{\avariable}{\avariablebis}{\avariableter}}{\ameetvar{\avariablefour}{\avariablefifth}{\avariablesix}}{\asetmeetvar} \land \asymmetric{\ameetvar{\avariable}{\avariablefour}{\avariablesix}}$.
Since $\asymmetric{\ameetvar{\avariable}{\avariablefour}{\avariablesix}}$ holds, then we obtain that one of the two following pattens must hold in the heap:
\begin{center}
\begin{tikzpicture}[baseline]
  \node[dot,label=above:$\avariable$] (i) at (0,0) {};
  \node[dot,label=left:{$\ameetvar{\avariable}{\avariablefour}{\avariablesix}$}]
  (m1) [below right = 1.5cm and 0.4cm of i] {};
  \node[dot,label=right:{$\ameetvar{\avariablefour}{\avariable}{\avariablesix}$}] (m2) [below right = 1.7cm and 0.4cm of m1] {};
  \node[dot,label=above:$\avariablefour$] (j) [above right=1.5cm and 0.5cm of m2] {};
  \node[dot,label=left:{$\avariablesix$}] (k) [below right= 2.7cm and 0.1 of i] {};

  \draw[reach] (i) -- (m1);
  \draw[pto] (m1) to node [above right] {$+$} (m2);
  \draw[reach] (j) -- (m2);
  \draw[reach] (m2) to [out=180,in=-75] (k);
  \draw[pto] (k) to [bend left=30] node [left] {$+$} (m1);

\end{tikzpicture}
\qquad\qquad
\begin{tikzpicture}[baseline]
  \node[dot,label=above:$\avariablefour$] (i) at (0,0) {};
  \node[dot,label=left:{$\ameetvar{\avariablefour}{\avariable}{\avariablesix}$}]
  (m1) [below right = 1.5cm and 0.4cm of i] {};
  \node[dot,label=right:{$\ameetvar{\avariable}{\avariablefour}{\avariablesix}$}] (m2) [below right = 1.7cm and 0.4cm of m1] {};
  \node[dot,label=above:$\avariable$] (j) [above right=1.5cm and 0.5cm of m2] {};
  \node[dot,label=left:{$\avariablesix$}] (k) [below right= 2.7cm and 0.1 of i] {};

  \draw[reach] (i) -- (m1);
  \draw[pto] (m1) to node [above right] {$+$} (m2);
  \draw[reach] (j) -- (m2);
  \draw[reach] (m2) to [out=180,in=-75] (k);
  \draw[pto] (k) to [bend left=30] node [left] {$+$} (m1);
\end{tikzpicture}
\end{center}
As $\sees{\ameetvar{\avariable}{\avariablebis}{\avariableter}}{\ameetvar{\avariablefour}{\avariablefifth}{\avariablesix}}{\asetmeetvar}$ holds, we 
obtain that there must be $\alength \geq 1$ such that  $\aheap^\alength(\astore(\avariable))
= \semantics{\ameetvar{\avariablefour}{\avariablefifth}{\avariablesix}}_{\astore,\aheap}$.
Then, it is easy to see (from the two diagram above) that $\semantics{\ameetvar{\avariablefour}{\avariablefifth}{\avariablesix}}_{\astore,\aheap}$ must be a location in the cycle that contains $\semantics{\ameetvar{\avariablefour}{\avariable}{\avariablesix}}_{\astore,\aheap}$.
Moreover, as $\semantics{\ameetvar{\avariablefour}{\avariablefifth}{\avariablesix}}_{\astore,\aheap}$ is defined,
there are $\alength_1,\alength_2 \geq 0$ such that
\begin{enumerate}[label=\alph*.]
\item $\aheap^{\alength_1}(\astore(\avariablefour)) = \aheap^{\alength_2}(\astore(\avariablefifth)) = \semantics{\ameetvar{\avariablefour}{\avariablefifth}{\avariablesix}}_{\astore,\aheap}$ and there is $\alength \geq 0$ s.t.\
$\aheap^\alength(\semantics{\ameetvar{\avariablefour}{\avariablefifth}{\avariablesix}}_{\astore,\aheap}) = \astore(\avariablesix)$;
\item for every $\alength_1' \in \interval{0}{\alength_1-1}$ and $\alength_2' \geq 0$,
$\aheap^{\alength_1'}(\astore(\avariablefour)) \neq \aheap^{\alength_2'}(\astore(\avariablefifth))$.
\end{enumerate}
By contradiction, suppose that  $\semantics{\ameetvar{\avariablefour}{\avariablefifth}{\avariablesix}}_{\astore,\aheap} \neq \semantics{\ameetvar{\avariablefour}{\avariable}{\avariablesix}}_{\astore,\aheap}$.
Then, as $\semantics{\ameetvar{\avariablefour}{\avariablefifth}{\avariablesix}}_{\astore,\aheap}$ we directly obtain that (b) cannot hold, as $\semantics{\ameetvar{\avariablefour}{\avariable}{\avariablesix}}_{\astore,\aheap}$ is such that
$\aheap^{\alength_1'}(\astore(\avariablefour)) = \semantics{\ameetvar{\avariablefour}{\avariable}{\avariablesix}}_{\astore,\aheap} =  \aheap^{\alength_2'}(\astore(\avariablefifth))$
for some $\alength_1' \in \interval{0}{\alength_1-1}$ and $\alength_2' \geq 0$.
Hence $\pair{\astore}{\aheap} \models  \ameetvar{\avariablefour}{\avariablefifth}{\avariablesix} = \ameetvar{\avariablefour}{\avariable}{\avariablesix}$.

\item Soundness of the axiom~\ref{core2Ax:SeesToBefore}:
$$
\sees{\ameetvar{\avariable}{\avariablebis}{\avariableter}}{\ameetvar{\avariablefour}{\avariablefifth}{\avariablesix}}{\asetmeetvar} \land \symmetric{\ameetvar{\avariable}{\avariablefour}{\avariablesix}}
\land \ameetvar{\avariable}{\avariablebis}{\avariableter} \neq \ameetvar{\avariablefour}{\avariablefifth}{\avariablesix}
\Rightarrow \before{\ameetvar{\avariable}{\avariablebis}{\avariableter}}{\ameetvar{\avariablefour}{\avariablefifth}{\avariablesix}}
$$

Suppose $\pair{\astore}{\aheap} \models \sees{\ameetvar{\avariable}{\avariablebis}{\avariableter}}{\ameetvar{\avariablefour}{\avariablefifth}{\avariablesix}}{\asetmeetvar} \land \symmetric{\ameetvar{\avariable}{\avariablefour}{\avariablesix}}
\land \ameetvar{\avariable}{\avariablebis}{\avariableter} \neq \ameetvar{\avariablefour}{\avariablefifth}{\avariablesix}$.

First, from $\sees{\ameetvar{\avariable}{\avariablebis}{\avariableter}}{\ameetvar{\avariablefour}{\avariablefifth}{\avariablesix}}{\asetmeetvar}$ we conclude that
$\semantics{\ameetvar{\avariable}{\avariablebis}{\avariableter}}_{\astore,\aheap}$ and
$\semantics{\ameetvar{\avariablefour}{\avariablefifth}{\avariablesix}}_{\astore,\aheap}$ are both defined.
From $\symmetric{\ameetvar{\avariable}{\avariablefour}{\avariablesix}}$ we obtain that one of the following two patterns holds in $\aheap$:
\begin{nscenter}
\begin{tikzpicture}[baseline]
  \node[dot,label=above:$\avariable$] (i) at (0,0) {};
  \node[dot,label=left:{$\ameetvar{\avariable}{\avariablefour}{\avariablesix}$, $\ameetvar{\avariablefour}{\avariable}{\avariablesix}$}] (m) [below right = 1.5cm and 0.5cm of i] {};
  \node[dot,label=above:$\avariablefour$] (j) [above right=1.5cm and 0.5cm of m] {};
  \node[dot,label=below:{$\avariablesix$\\$\avariablesix$ not inside a loop}] (k) [below of=m] {};

  \draw[reach] (i) -- (m);
  \draw[reach] (j) -- (m);
  \draw[reach] (m) -- (k);
\end{tikzpicture}
\qquad\qquad
\begin{tikzpicture}[baseline]
  \node[dot,label=above:$\avariable$] (i) at (0,0) {};
  \node[dot,label=left:{$\ameetvar{\avariable}{\avariablefour}{\avariablesix}$, $\ameetvar{\avariablefour}{\avariable}{\avariablesix}$}] (m) [below right = 1.5cm and 0.5cm of i] {};
  \node[dot,label=above:$\avariablefour$] (j) [above right=1.5cm and 0.5cm of m] {};
  \node[dot] (mid) [below=0.8cm of m] {};
  \node[dot,label=below:{$\avariablesix$}] (k) [below=1.65cm of m] {};

  \draw[reach] (i) -- (m);
  \draw[reach] (j) -- (m);
  \draw[reach] (m) -- (mid);
  \draw[reach] (mid) to [out=-35,in=35] (k);
  \draw[pto] (k) to [out=155,in=-155] node [left] {$+$} (mid);
\end{tikzpicture}
\end{nscenter}
If the first pattern holds, then trivially we conclude that
$\semantics{\ameetvar{\avariable}{\avariablebis}{\avariableter}}_{\astore,\aheap}$ and
$\semantics{\ameetvar{\avariablefour}{\avariablefifth}{\avariablesix}}_{\astore,\aheap}$
must lay on the path from $\astore(\avariable)$ to $\astore(\avariablesix)$ and on the
path from $\astore(\avariablefour)$ to $\astore(\avariablesix)$, respectively.
Hence, from $\sees{\ameetvar{\avariable}{\avariablebis}{\avariableter}}{\ameetvar{\avariablefour}{\avariablefifth}{\avariablesix}}{\asetmeetvar}$ it is easy to see that $\before{\ameetvar{\avariable}{\avariablebis}{\avariableter}}{\ameetvar{\avariablefour}{\avariablefifth}{\avariablesix}}$ holds (we recall that, informally, this formula holds whenever
$\semantics{\ameetvar{\avariable}{\avariablebis}{\avariableter}}_{\astore,\aheap}$ and
$\semantics{\ameetvar{\avariablefour}{\avariablefifth}{\avariablesix}}_{\astore,\aheap}$
are in a path where at most the location
$\semantics{\ameetvar{\avariablefour}{\avariablefifth}{\avariablesix}}_{\astore,\aheap}$ can belong to a cycle, and from $\semantics{\ameetvar{\avariable}{\avariablebis}{\avariableter}}_{\astore,\aheap}$ it is possible to reach  $\semantics{\ameetvar{\avariablefour}{\avariablefifth}{\avariablesix}}_{\astore,\aheap}$ in at least one step).

Suppose instead that the second pattern holds. Then we argue that $\symmetric{\ameetvar{\avariable}{\avariablefour}{\avariablesix}}
\land \ameetvar{\avariable}{\avariablebis}{\avariableter} \neq \ameetvar{\avariablefour}{\avariablefifth}{\avariablesix}$ implies that
$\semantics{\ameetvar{\avariable}{\avariablebis}{\avariableter}}_{\astore,\aheap}$ and
$\semantics{\ameetvar{\avariablefour}{\avariablefifth}{\avariablesix}}_{\astore,\aheap}$
cannot be together in the cycle. Indeed, from
$\symmetric{\ameetvar{\avariable}{\avariablefour}{\avariablesix}}$,
if this was the case, then we obtain
$\ameetvar{\avariable}{\avariablebis}{\avariableter} = \ameetvar{\avariablefour}{\avariablefifth}{\avariablesix}$ (contradiction)
as the first location in the cycle that is reachable from $\astore(\avariable)$ is also the first location in the cycle reachable from $\astore(\avariablefour)$.
Then, at most one location between $\semantics{\ameetvar{\avariable}{\avariablebis}{\avariableter}}_{\astore,\aheap}$ and
$\semantics{\ameetvar{\avariablefour}{\avariablefifth}{\avariablesix}}_{\astore,\aheap}$
can be in the cycle, and (if it does belong to the cycle) it must correspond to the first location in the cycle that is reachable from $\astore(\avariable)$ (or alternatively $\astore(\avariablefour)$).
Then, from $\sees{\ameetvar{\avariable}{\avariablebis}{\avariableter}}{\ameetvar{\avariablefour}{\avariablefifth}{\avariablesix}}{\asetmeetvar}$ we conclude that, in the case that one of the two locations is in the cycle, it is
$\semantics{\ameetvar{\avariablefour}{\avariablefifth}{\avariablesix}}_{\astore,\aheap}$.
As in the previous case, it is then easy to see that
$\before{\ameetvar{\avariable}{\avariablebis}{\avariableter}}{\ameetvar{\avariablefour}{\avariablefifth}{\avariablesix}}$ must hold.

\item Soundness of the axiom~\ref{core2Ax:SeesElsewhere}:
$$\before{\aterm_1}{\aterm_2} \land \lnot \sees{\aterm_1}{\aterm_2}{\{\aterm_3\}} \implies \lnot \sees{\aterm_2}{\aterm_3}{\emptyset} \land \before{\aterm_1}{\aterm_3}
$$
Let $\pair{\astore}{\aheap}$ be a memory state such that $\pair{\astore}{\aheap} \models \before{\aterm_1}{\aterm_2} \land \lnot \sees{\aterm_1}{\aterm_2}{\{\aterm_3\}}$.
So, $\semantics{\aterm_1}_{\astore,\aheap} {\neq} \semantics{\aterm_2}_{\astore,\aheap}$ and,
there is a path
$\alocation_1 = \semantics{\aterm_1}_{\astore,\aheap} \mapsto \alocation_2 \mapsto \cdots \mapsto \alocation_{N} = \semantics{\aterm_2}_{\astore,\aheap}$ ($N \geq 1$)
such that the only location on the path that may belong to a cycle is $\semantics{\aterm_2}_{\astore,\aheap}$
and $\semantics{\aterm_3}_{\astore,\aheap} \in \set{\alocation_2, \ldots, \alocation_{N-1}}$.
This means that $\semantics{\aterm_1}_{\astore,\aheap} {\neq} \semantics{\aterm_3}_{\astore,\aheap}$ and,
there is a path from $\semantics{\aterm_1}_{\astore,\aheap}$ to $\semantics{\aterm_3}_{\astore,\aheap}$
such that none of the locations on the path   belongs to a cycle.
So, $\pair{\astore}{\aheap} \models \before{\aterm_1}{\aterm_3}$.
As $\semantics{\aterm_3}_{\astore,\aheap}$ does not belong to a cycle, $\sees{\aterm_2}{\aterm_3}{\emptyset}$ cannot hold on $\pair{\astore}{\aheap}$.

\item Soundness of the axiom~\ref{core2Ax:SeesLoopOrder}:
$$\sameloop{\aterm_1}{\aterm_2} \land \sameloop{\aterm_2}{\aterm_3} \land \aterm_1\neq\aterm_3 \Rightarrow
\sees{\aterm_1}{\aterm_3}{\{\aterm_2\}} \iff \lnot \sees{\aterm_3}{\aterm_1}{\{\aterm_2\}}
$$
Let $\pair{\astore}{\aheap}$ be a memory state such that $\pair{\astore}{\aheap} \models \sameloop{\aterm_1}{\aterm_2} \land \sameloop{\aterm_2}{\aterm_3}
\land  \aterm_1\neq\aterm_3$.
So $\semantics{\aterm_1}_{\astore, \aheap} \neq \semantics{\aterm_2}_{\astore, \aheap}$,
   $\semantics{\aterm_2}_{\astore, \aheap} \neq \semantics{\aterm_3}_{\astore, \aheap}$ and,
$\semantics{\aterm_1}_{\astore, \aheap}$,$\semantics{\aterm_2}_{\astore, \aheap}$, $\semantics{\aterm_3}_{\astore, \aheap}$  belong
to the same cycle having at least three elements.
\begin{itemize}
\item In the case, there is a path from $\semantics{\aterm_1}_{\astore, \aheap}$ to $\semantics{\aterm_2}_{\astore, \aheap}$ that does not
visit $\semantics{\aterm_3}_{\astore, \aheap}$, there is necessarily a path
from $\semantics{\aterm_3}_{\astore, \aheap}$ to $\semantics{\aterm_1}_{\astore, \aheap}$ that does not
visit $\semantics{\aterm_2}_{\astore, \aheap}$. Consequently, $\pair{\astore}{\aheap} \models
 \sees{\aterm_3}{\aterm_1}{\{\aterm_2\}} \wedge \neg \sees{\aterm_1}{\aterm_3}{\{\aterm_2\}}$.
\item Similarly, if there is a path from $\semantics{\aterm_1}_{\astore, \aheap}$ to $\semantics{\aterm_2}_{\astore, \aheap}$ that
visits $\semantics{\aterm_3}_{\astore, \aheap}$, then there is  a path
from $\semantics{\aterm_1}_{\astore, \aheap}$ to $\semantics{\aterm_3}_{\astore, \aheap}$ that does not
visit $\semantics{\aterm_2}_{\astore, \aheap}$. Consequently, $\pair{\astore}{\aheap} \models
 \neg \sees{\aterm_3}{\aterm_1}{\{\aterm_2\}} \wedge  \sees{\aterm_1}{\aterm_3}{\{\aterm_2\}}$.
\end{itemize}
We can conclude that  $\pair{\astore}{\aheap} \models \sees{\aterm_1}{\aterm_3}{\{\aterm_2\}} \iff \lnot \sees{\aterm_3}{\aterm_1}{\{\aterm_2\}}$.
\end{itemize}

\textbf{Axioms from \ref{core2Ax:RemPos} to \ref{core2Ax:RemShort}}

\begin{itemize}
\item Axioms from~\ref{core2Ax:RemPos} to~\ref{core2Ax:RemTEq2} are straightforward.
\item
 Soundness of the axiom~\ref{core2Ax:RemNotSees}:
$$\lnot \seesgeq{\aterm_1}{\aterm_2}{\emptyset}{\beta_2{+}1} \land \remgeq{\asetpath}{\inbound_1}
   \implies
     \remgeq{\asetpath \cup \{\pair{\aterm_1}{\aterm_2}\}}{\inbound_1{\dotminus}\inbound_2}$$
Let $\pair{\astore}{\aheap}$ be a memory state such that $\pair{\astore}{\aheap} \models \lnot \seesgeq{\aterm_1}{\aterm_2}{\emptyset}{\beta_2{+}1} \land \remgeq{\asetpath}{\inbound_1}$.
So, $\card{\domain{\aheap}  \setminus \bigcup_{\pair{\aterm_3}{\aterm_4}\in\asetpath} \minpath{\semantics{\aterm_3}_{\astore,\aheap}}{\semantics{\aterm_4}_{\astore,\aheap}}{\aheap}} \geq  \inbound_1$.
Trivially, since $\pair{\astore}{\aheap} \models \lnot \seesgeq{\aterm_1}{\aterm_2}{\emptyset}{\inbound_2{+}1}$ then the minimal path the minimal path between $\semantics{\aterm_1}_{\astore,\aheap}$ and $\semantics{\aterm_2}_{\astore,\aheap}$ (if it exists)
has at most $\inbound_2$ locations, i.e. $\card{\minpath{\semantics{\aterm_3}_{\astore,\aheap}}{\semantics{\aterm_4}_{\astore,\aheap}}{\aheap}} \leq \inbound_2$.
Then by properties of sets it can be easily shown that $$\card{\domain{\aheap}  \setminus \bigcup_{\pair{\aterm_3}{\aterm_4}\in\asetpath \cup \{\pair{\aterm_1}{\aterm_2} \}} \minpath{\semantics{\aterm_3}_{\astore,\aheap}}{\semantics{\aterm_4}_{\astore,\aheap}}{\aheap}} \geq \inbound_1{\dotminus}\inbound_2,$$
i.e. $\pair{\astore}{\aheap} \models  \remgeq{\asetpath \cup \{\pair{\aterm_1}{\aterm_2}\}}{\inbound_1{\dotminus}\inbound_2}$.

\item Soundness of the axiom~\ref{core2Ax:RemBetween}:
$$
  \sees{\aterm_1}{\aterm_2}{\asetmeetvar} \land \lnot \sees{\aterm_1}{\aterm_2}{\{\aterm_3\}} \land
  \remgeq{\{\pair{\aterm_1}{\aterm_3},\pair{\aterm_3}{\aterm_2}\}\cup\asetpath}{\inbound}
  \implies \remgeq{\{\pair{\aterm_1}{\aterm_2}\}\cup\asetpath}{\inbound}
$$

Let  $\pair{\astore}{\aheap}$ be a memory state such that
$$\pair{\astore}{\aheap} \models
\sees{\aterm_1}{\aterm_2}{\asetmeetvar} \land \lnot \sees{\aterm_1}{\aterm_2}{\{\aterm_3\}} \land
\remgeq{\{\pair{\aterm_1}{\aterm_3},\pair{\aterm_3}{\aterm_2}\}\cup\asetpath}{\inbound}
$$
By definition of $\models$,  there is $\delta \geq 1$ such that (a)
$\aheap^{\delta}(\semantics{\aterm_1}_{\astore,\aheap}) = \semantics{\aterm_2}_{\astore,\aheap}$
and (b) for all $\delta' \in \interval{1}{\delta-1}$, $\aheap^{\delta'}(\semantics{\aterm_1}_{\astore,\aheap}) \not \in
\set{\semantics{\aterm_2}_{\astore,\aheap}} \cup \set{\semantics{\aterm}_{\astore,\aheap} \mid \aterm \in \asetmeetvar}$.
Moreover, there is $\delta_0 \in \interval{1}{\delta-1}$ such that $\aheap^{\delta_0}(\semantics{\aterm_1}_{\astore,\aheap}) =
\semantics{\aterm_3}_{\astore,\aheap}$.
Hence,
\begin{itemize}
\item for all $\delta' \in \interval{1}{\delta_0-1}$, $\aheap^{\delta'}(\semantics{\aterm_1}_{\astore,\aheap}) \not \in
\set{\semantics{\aterm_3}_{\astore,\aheap}} \cup \set{\semantics{\aterm}_{\astore,\aheap} \mid \aterm \in \asetmeetvar}$,
\item for all $\delta' \in \interval{1}{(\delta - \delta_0)-1}$, $\aheap^{\delta'}(\semantics{\aterm_3}_{\astore,\aheap}) \not \in
\set{\semantics{\aterm_2}_{\astore,\aheap}} \cup \set{\semantics{\aterm}_{\astore,\aheap} \mid \aterm \in \asetmeetvar}$,
\item $\aheap^{\alength - \alength_0}(\semantics{\aterm_3}_{\astore,\aheap}) = \semantics{\aterm_2}_{\astore,\aheap}$.
\end{itemize}
We then obtain the following equality:
$$
\minpath{\semantics{\aterm_1}_{\astore,\aheap}}{\semantics{\aterm_2}_{\astore,\aheap}}{\aheap}
=
\minpath{\semantics{\aterm_1}_{\astore,\aheap}}{\semantics{\aterm_3}_{\astore,\aheap}}{\aheap} \cup
\minpath{\semantics{\aterm_3}_{\astore,\aheap}}{\semantics{\aterm_2}_{\astore,\aheap}}{\aheap}
$$
And therefore, by considering
$\asetpath' = \{\pair{\aterm_1}{\aterm_3},\pair{\aterm_3}{\aterm_2}\}\cup\asetpath$ and
$\asetpath'' = \{\pair{\aterm_1}{\aterm_2}\}\cup\asetpath$ we get
$$
\bigcup_{\pair{\aterm}{\aterm'}\in\asetpath'}
\minpath{\semantics{\aterm}_{\astore,\aheap}}{\semantics{\aterm'}_{\astore,\aheap}}{\aheap}
=
\bigcup_{\pair{\aterm}{\aterm'}\in\asetpath''}
\minpath{\semantics{\aterm}_{\astore,\aheap}}{\semantics{\aterm'}_{\astore,\aheap}}{\aheap}
$$
Hence,
$$\domain{\aheap}  \setminus \bigcup_{\pair{\aterm}{\aterm'}\in\asetpath'}
\minpath{\semantics{\aterm}_{\astore,\aheap}}{\semantics{\aterm'}_{\astore,\aheap}}{\aheap}
=
\domain{\aheap}  \setminus \bigcup_{\pair{\aterm}{\aterm'}\in\asetpath''}
\minpath{\semantics{\aterm}_{\astore,\aheap}}{\semantics{\aterm'}_{\astore,\aheap}}{\aheap}.
$$
From
$\pair{\astore}{\aheap} \models
\remgeq{\{\pair{\aterm_1}{\aterm_3},\pair{\aterm_3}{\aterm_2}\}\cup\asetpath}{\inbound}$, the set above has cardinality at least $\inbound$, and therefore
we conclude that
$\pair{\astore}{\aheap} \models
\remgeq{\{\pair{\aterm_1}{\aterm_2}\}\cup\asetpath}{\inbound}$.

\item Soundness of the axiom~\ref{core2Ax:RemBetweenTwo}:
  $$
    \sees{\aterm_1}{\aterm_2}{\asetmeetvar} \land \lnot \sees{\aterm_1}{\aterm_2}{\{\aterm_3\}} \land
    \remgeq{\{\pair{\aterm_1}{\aterm_2}\}\cup\asetpath}{\inbound} \implies \remgeq{\{\pair{\aterm_1}{\aterm_2},\pair{\aterm_1}{\aterm_3},\pair{\aterm_3}{\aterm_2}\}\cup\asetpath}{\inbound}
  $$
The proof of validity of this formula is very similar to the one for \ref{core2Ax:RemBetween} (previous axiom), and can be obtained from this latter proof by simply updating the definition of $\asetpath'$ from
$\{\pair{\aterm_1}{\aterm_3},\pair{\aterm_3}{\aterm_2}\}\cup\asetpath$ to
$\{\pair{\aterm_1}{\aterm_2},\pair{\aterm_1}{\aterm_3},\pair{\aterm_3}{\aterm_2}\}\cup\asetpath$.
We then obtain again
$$\domain{\aheap}  \setminus \bigcup_{\pair{\aterm}{\aterm'}\in\asetpath'}
\minpath{\semantics{\aterm}_{\astore,\aheap}}{\semantics{\aterm'}_{\astore,\aheap}}{\aheap}
=
\domain{\aheap}  \setminus \bigcup_{\pair{\aterm}{\aterm'}\in\asetpath''}
\minpath{\semantics{\aterm}_{\astore,\aheap}}{\semantics{\aterm'}_{\astore,\aheap}}{\aheap}.
$$
and from
$\pair{\astore}{\aheap} \models
\remgeq{\{\pair{\aterm_1}{\aterm_2}\}\cup\asetpath}{\inbound}$
we conclude that
$\pair{\astore}{\aheap} \models
\remgeq{\{\pair{\aterm_1}{\aterm_2},\pair{\aterm_1}{\aterm_3},\pair{\aterm_3}{\aterm_2}\}\cup\asetpath}{\inbound}$.

\item Soundness of the axiom~\ref{core2Ax:RemShort}:
$$\begin{aligned}[t]
&\big(\seesgeq{\aterm_1}{\aterm_2}{\emptyset}{\beta_2}
    \land
      \textstyle\bigwedge_{
      \scriptstyle{\pair{\aterm_3}{\aterm_4} \in \asetpath}}
      (\sees{\aterm_3}{\aterm_4}{\emptyset} \implies \sees{\aterm_1}{\aterm_2}{\{\aterm_3,\aterm_4\}} \land \sees{\aterm_3}{\aterm_4}{\{\aterm_1,\aterm_2\}} \land \aterm_3 {\neq} \aterm_1 )\\
& \land \remgeq{\asetpath \cup \{\pair{\aterm_1}{\aterm_2}\}}{\inbound_1} \big) \implies
    \remgeq{\asetpath}{\inbound_1{+}\inbound_2}
\end{aligned}$$

Let $\pair{\astore}{\aheap}$ be a memory state satisfying the antecedent of the implication.
By definition of $\models$,  there is $\delta \geq \inbound_2$ such that (a)
$\aheap^{\delta}(\semantics{\aterm_1}_{\astore,\aheap}) = \semantics{\aterm_2}_{\astore,\aheap}$
and (b) for all $\delta' \in \interval{1}{\delta-1}$, $\aheap^{\delta'}(\semantics{\aterm_1}_{\astore,\aheap}) \not \semantics{\aterm_2}_{\astore,\aheap}$.
Moreover, we have
$$
\card{\domain{\aheap}  \setminus \bigcup_{\pair{\aterm}{\aterm'}\in\asetpath \cup \set{\pair{\aterm_1}{\aterm_2}}}
\minpath{\semantics{\aterm}_{\astore,\aheap}}{\semantics{\aterm'}_{\astore,\aheap}}{\aheap}}
\geq \inbound_1.
$$
The satisfaction of
$$
\remgeq{\asetpath \cup \{\pair{\aterm_1}{\aterm_2}\}}{\inbound_1} \land
\textstyle\bigwedge_{\mathclap{
      \raisebox{-0.15cm}[0pt][0pt]{$\scriptstyle{\pair{\aterm_3}{\aterm_4} \in \asetpath}$}}}
      (\sees{\aterm_3}{\aterm_4}{\emptyset} \implies \sees{\aterm_3}{\aterm_4}{\{\aterm_1,\aterm_2\}} \land \aterm_3 {\neq} \aterm_1 )
$$
on $\pair{\astore}{\aheap}$ guarantees that
$$
(\bigcup_{\pair{\aterm}{\aterm'}\in\asetpath}
\minpath{\semantics{\aterm}_{\astore,\aheap}}{\semantics{\aterm'}_{\astore,\aheap}}{\aheap})
\cap \minpath{\semantics{\aterm_1}_{\astore,\aheap}}{\semantics{\aterm_2}_{\astore,\aheap}}{\aheap}
= \emptyset
$$
Consequently,
$$
\card{\domain{\aheap}  \setminus \bigcup_{\pair{\aterm}{\aterm'}\in\asetpath}
\minpath{\semantics{\aterm}_{\astore,\aheap}}{\semantics{\aterm'}_{\astore,\aheap}}{\aheap}}
\geq
$$
$$
\inbound_2
+
\card{\domain{\aheap}  \setminus \bigcup_{\pair{\aterm}{\aterm'}\in\asetpath \cup \set{\pair{\aterm_1}{\aterm_2}}}
\minpath{\semantics{\aterm}_{\astore,\aheap}}{\semantics{\aterm'}_{\astore,\aheap}}{\aheap}}.
$$
In conclusion, $\pair{\astore}{\aheap} \models \remgeq{\asetpath}{\inbound_1{+}\inbound_2}$.

\end{itemize}

\end{proof}
