# Supplementary material for: A Complete Axiomatisation for Quantifier-Free Separation Logic
Source: arXiv:2006.05156 source file (2021-08-09)
Supplement: Supplementary file 10 [file proof-lemma-axiomtwo-StarElimination.tex]

\lemmaaxiomtwoStarElimination*

\begin{proof}
Let $\aformula \in \boolcomb{\coreformulae{\asetvar}{\bound_1}}$
and $\aformulabis \in \boolcomb{\coreformulae{\asetvar}{\bound_2}}$.
As shown in the proof of Lemma~\ref{prop:corePSLone} (whose proof works also for the family of core types of \intervalSL),
there are two disjunctions $\aformula_1\lor\dots\lor\aformula_n$ and $\aformulabis_1\lor\dots\lor\aformulabis_m$, where $\aformula_i \in \coretype{\asetvar}{\bound_1}$ and $\aformulabis_i \in \coretype{\asetvar}{\bound_2}$, such that
$\prove_{\coresys} \aformula \iff \aformula_1\lor\dots\lor\aformula_n$ and
$\prove_{\coresys} \aformulabis \iff \aformulabis_1\lor\dots\lor\aformulabis_m$. Then, by the rule~\ref{rule:star2inference} we deduce that
$\aformula \separate \aformulabis \iff (\bigvee_{i \in \interval{1}{n}}\aformula_i) \separate (\bigvee_{j \in \interval{1}{m}} \aformulabis_j)$ is derivable in $\coresys(\separate,\weirdexists)$.
As $\separate$ distributes w.r.t\ disjunctions (axiom~\ref{starAx2:DistrOr}) and is commutative (axiom~\ref{starAx2:StarCommute}), then we obtain that
$\aformula \separate \aformulabis \iff \bigvee_{i \in \interval{1}{n}}\bigvee_{j \in \interval{1}{m}} (\aformula_i \separate \aformulabis_j)$ is derivable in $\coresys(\separate,\weirdexists)$.
To conclude the proof it is then sufficient to focus on a single disjunct $\aformula_i \separate \aformulabis_j$ of the formula above, and show that it is equivalent to a Boolean combination of core formulae $\boolcomb{\coreformulae{\asetvar}{\bound_1+\bound_2}}$.
If $\aformula_i$ or $\aformulabis_j$ are unsatisfiable, say $\aformula_i$, then by Lemma~\ref{lemma:axiomtwoRCct}
$\prove_{\coresys} \aformula_i \implies \bottom$ and by axiom~\ref{starAx2:False} we conclude that $\prove_{\coresys(\separate,\weirdexists)} \aformula_i \separate \aformulabis_j \implies \bottom$ (which is equivalent to any unsatisfiable core type, as for example one containing $\lnot \remgeq{\emptyset}{0}$).

Suppose that both $\aformula_i$ and $\aformulabis_j$ are satisfiable.
By Lemma~\ref{corr:typeuniquesymb} then there are two symbolic memory states $\asms_1$, $\asms_2$, respectively over $\pair{\asetvar}{\bound_1}$ and $\pair{\asetvar}{\bound_2}$ such that
$\prove_{\coresys} \aformula_i \iff \charsymbform(\asms_1)$
and
$\prove_{\coresys} \aformulabis_j \iff \charsymbform(\asms_2)$.
Hence, by the rule~\ref{rule:star2inference}, we obtain $\prove_{\coresys(\separate,\weirdexists)} \aformula_i \separate \aformulabis_j \iff \charsymbform(\asms_1) \separate \charsymbform(\asms_2)$.
We can now apply axiom~\ref{starAx2:StarElim} and derive from $\charsymbform(\asms_1) \separate \charsymbform(\asms_2)$ an equivalent Boolean combination of core formulae ${\textstyle\bigvee_{\asms\ \text{s.t.}\
\symbunion{\asms_1}{\asms_2}{\asms}}}
{\charsymbform(\asms)}$ from $\boolcomb{\coreformulae{\asetvar}{\bound_1+\bound_2}}$.
Therefore, by propositional calculus we obtain that the following equivalence is derivable in $\coresys(\separate,\weirdexists)$:
\begin{nscenter}
$\aformula_i \separate \aformulabis_j \iff {\textstyle\bigvee_{\asms\ \text{s.t.}\
\symbunion{\asms_1}{\asms_2}{\asms}}} \
{\charsymbform(\asms)}$.
\end{nscenter}
This concludes the proof.

\end{proof}
