# Supplementary material for: A Complete Axiomatisation for Quantifier-Free Separation Logic
Source: arXiv:2006.05156 source file (2021-08-09)
Supplement: Supplementary file 11 [file proof-lemma-axiomtwo-StarSound.tex]

\begin{restatable}{lemma}{lemmaaxiomtwoStarSound}\label{lemma:axiomtwoStarSound}
$\coresys(\separate,\weirdexists)$ is sound.
\end{restatable}
\begin{proof}
We proved the validity of the axioms for $\weirdexists$ in Lemma~\ref{lemma:existsaxiomsvalid}.
The validity of axioms~\ref{starAx2:False},~\ref{starAx2:DistrOr} and of~\ref{rule:star2inference} follows from propositional separation logic. Then, we focus on the axiom~\ref{starAx2:StarElim}.
\begin{itemize}
\item[\ref{starAx2:StarElim}]
The proof of validity of this axiom relies on Lemmata~\ref{lemma:msmodelsabs}, \ref{lemma:compositionisok} and \ref{lemma:CompositionVsStar}. Let us start by recalling the axiom:
\begin{nscenter}
$
\charsymbform(\asms_1) \separate \charsymbform(\asms_2) \iff {\textstyle\bigvee_{\asms\ \text{s.t.}\
\symbunion{\asms_1}{\asms_2}{\asms}}}
{\charsymbform(\asms)}
\assuming{{\asms_1}, {\asms_2}\ \text{resp. over}\
\pair{\asetvar}{\bound_1}\ \text{and}\ \pair{\asetvar}{\bound_2}}
$
\end{nscenter}
In the following, $\asms_1 = \triple{\symbterms_1}{\amap_1}{\symbrem_1}$ and $\asms_2 = \triple{\symbterms_2}{\amap_2}{\symbrem_2}$.

It is easy to see that the right to left direction is just an application of Lemma~\ref{lemma:CompositionVsStar}.
Indeed, suppose
\begin{nscenter}
$\pair{\astore}{\aheap} \models {\textstyle\bigvee_{\asms\ \text{s.t.}\
\symbunion{\asms_1}{\asms_2}{\asms}}}
{\charsymbform(\asms)}$.
\end{nscenter}
Then the disjunction is not empty and
there is $\asms$ such that $\symbunion{\asms_1}{\asms_2}{\asms}$.
Thanks to the assumption of the axiom we can then apply Lemma~\ref{lemma:CompositionVsStar} and conclude that $\pair{\astore}{\aheap} \models \charsymbform(\asms_1) \separate \charsymbform(\asms_2)$.

We now prove the left to right direction.
Suppose $\pair{\astore}{\aheap} \models \charsymbform(\asms_1) \separate \charsymbform(\asms_2)$.
By Lemma~\ref{lemma:msmodelsabs} we have that $\pair{\astore}{\aheap} \models \charsymbform(\symbms{\astore}{\aheap}{\asetvar}{\bound_1+\bound_2})$.
Then to prove that the result, it is sufficient to show that
\begin{nscenter}
$\symbunion{\triple{\symbterms_1}{\amap_1}{\symbrem_1}}{\triple{\symbterms_2}{\amap_2}{\symbrem_2}}{\symbms{\astore}{\aheap}{\asetvar}{\bound_1+\bound_2}}$,
\end{nscenter}
therefore proving that $\charsymbform(\symbms{\astore}{\aheap}{\asetvar}{\bound_1+\bound_2})$
is a disjunct of
\begin{nscenter}
${\textstyle\bigvee_{\triple{\symbterms}{\amap}{\symbrem}\ \text{s.t.}\
\symbunion{\triple{\symbterms_1}{\amap_1}{\symbrem_1}}{\triple{\symbterms_2}{\amap_2}{\symbrem_2}}{\triple{\symbterms}{\amap}{\symbrem}}}}
{\charsymbform({\triple{\symbterms}{\amap}{\symbrem}})}$.
\end{nscenter}

By $\pair{\astore}{\aheap} \models \charsymbform(\asms_1) \separate \charsymbform(\asms_2)$,
there are $\aheap_1$ and $\aheap_2$ such that
\begin{itemize}
\item $\aheap = \aheap_1 + \aheap_2$;
\item $\pair{\astore}{\aheap_1} \models  \charsymbform(\asms_1) $;
\item $\pair{\astore}{\aheap_2} \models  \charsymbform(\asms_2) $.
\end{itemize}
By Lemma~\ref{lemma:msmodelsabs} we obtain:
\begin{itemize}
\item $\asms_1 = \symbms{\astore}{\aheap_1}{\asetvar}{\bound_1}$;
\item $\asms_2 = \symbms{\astore}{\aheap_1}{\asetvar}{\bound_2}$.
\end{itemize}
We now apply Lemma~\ref{lemma:compositionisok} and conclude that then
\begin{nscenter}
$\symbunion{\asms_1}{\asms_2}{\symbms{\astore}{\aheap}{\asetvar}{\bound_1+\bound_2}}$.
\end{nscenter}
Axiom~\ref{starAx2:StarElim} is therefore valid.\qedhere
\end{itemize}
\end{proof}
