# Supplementary material for: A Complete Axiomatisation for Quantifier-Free Separation Logic
Source: arXiv:2006.05156 source file (2021-08-09)
Supplement: Supplementary file 12 [file proof-lemma-exists-axioms-valid.tex]

\begin{restatable}{lemma}{lemmaexistsaxiomsvalid}\label{lemma:existsaxiomsvalid}
$\coresys(\weirdexists)$ is sound.
\end{restatable}

\begin{proof}
As said previously, the axioms~\ref{existsAx:Renaming}, \ref{existsAx:Conjunction}, \ref{existsAx:Disjunction}, \ref{existsAx:Bottom}, and the introduction rule
are classical tautologies of first-order quantifiers and it is not surprising that they still hold for the  quantifier $\weirdexists$.
Hence, we omit the proof and focus on the validity of the axioms~\ref{existsAx:ZeroStep}, \ref{existsAx:AtLeastOneStep}, \ref{existsAx:Split} and \ref{existsAx:SeesSem}.

\begin{enumerate}
\item[\ref{existsAx:ZeroStep}]  $\sees{\avariable}{\avariablebis}{\emptyset} \implies \inpath{\avariable}{\avariablebis}{\avariableter}\ \avariableter = \avariable$ $\assuming{\avariableter\not\in\{\avariable,\avariablebis\}}$.

Suppose $\pair{\astore}{\aheap} \models \sees{\avariable}{\avariablebis}{\emptyset}$. Then by definition the following two properties hold:
\begin{enumerate}
\item $\card{\minpath{\astore(\avariable)}{\astore(\avariablebis)}{\aheap}} \geq 1$
\item $\minpath{\astore(\avariable)}{\astore(\avariablebis)}{\aheap} \subseteq
      \pathset{\astore(\avariable)}{\astore,\aheap}{\asetmeetvar}$ ($\pathset{\astore(\avariable)}{\astore,\aheap}{\asetmeetvar}$ is introduced
      in Appendix~\ref{appendix:ExpressingCoreFormulae}).
\end{enumerate}
Given $\avariableter \not \in \{\avariable,\avariablebis\}$ it holds that $\pair{\astore[\avariableter \gets \astore(\avariable)]}{\aheap} \models \avariableter = \avariable$.
Moreover, from the first property we obtain $\minpath{\astore(\avariable)}{\astore(\avariablebis)}{\aheap} \neq \emptyset$.
By definition,  $\minpath{\astore(\avariable)}{\astore(\avariablebis)}{\aheap}$  contains $\astore(\avariable)$ whenever it is not empty.
Hence,   $\pair{\astore}{\aheap} \models \inpath{\avariable}{\avariablebis}{\avariableter}\ \avariableter = \avariable$.
\item[\ref{existsAx:AtLeastOneStep}]
 $\sees{\avariable}{\avariablebis}{\emptyset} \land \sees{\avariable}{\aterm_1}{\{\avariablebis\}}
\implies
\inpath{\avariable}{\avariablebis}{\avariableter}\ \avariableter = \aterm_1$ $\assuming{\avariableter\not\in\chars{\{\avariable,\avariablebis,\aterm_1\}}}$.

Suppose $\pair{\astore}{\aheap} \models \sees{\avariable}{\avariablebis}{\emptyset} \land \sees{\avariable}{\aterm_1}{\{\avariablebis\}}$.
Then, by definition of the sees predicate, it is easy to see that
$\emptyset \neq \minpath{\astore(\avariable)}{\semantics{\aterm_1}_{\astore,\aheap}}{\aheap} \subseteq \minpath{\astore(\avariable)}{\astore(\avariablebis)}{\aheap}$.
This also implies that $\semantics{\aterm_1}_{\astore,\aheap}$ is defined.
Given $\avariableter \not \in\chars{\{\avariable,\avariablebis,\aterm_1\}}$ it holds that $\pair{\astore[\avariableter \gets \semantics{\aterm_1}_{\astore,\aheap}]}{\aheap} \models \avariableter = \aterm_1$.
Notice that this only holds if we pick $\avariableter$ to be a program variable not in $\chars{\aterm_1}$ as then we are guaranteed that $\semantics{\aterm_1}_{\astore,\aheap} = \semantics{\aterm_1}_{\astore[\avariableter \gets \semantics{\aterm_1}_{\astore,\aheap}],\aheap}$.
From $\emptyset \neq \minpath{\astore(\avariable)}{\semantics{\aterm_1}_{\astore,\aheap}}{\aheap} \subseteq \minpath{\astore(\avariable)}{\astore(\avariablebis)}{\aheap}$
we can conclude that
 $\minpath{\astore(\avariable)}{\astore(\avariablebis)}{\aheap} \neq \emptyset$ and that $\semantics{\aterm_1}_{\astore,\aheap}$ belongs to $\minpath{\astore(\avariable)}{\astore(\avariablebis)}{\aheap} \cup \{\astore(\avariablebis)\}$.
Therefore, $\pair{\astore}{\aheap} \models \inpath{\avariable}{\avariablebis}{\avariableter}\ \avariableter = \aterm_1$.
\item[\ref{existsAx:Split}]
$
\begin{aligned}[t]
&\assuming{\{\avariable,\avariablebis,\aterm_1,\aterm_2\} \subseteq \asetmeetvar,\asetmeetvar',\asetmeetvar''\ \avariableter\not\in\chars{\asetmeetvar},\ \inbound_1,\inbound_2 \in \Nat^+\!,\ \geq\ \in \{\sim_1,\sim_2\} \subseteq \{\geq,=\}}\\
&({\avariable} {=} {\aterm_1} \lor \sees{\avariable}{\aterm_1}{\asetmeetvar'} ) \land \seesgeq{\aterm_1}{\aterm_2}{\asetmeetvar}{\inbound_1{+}\inbound_2} \land
({\aterm_2}{=}{\avariablebis} \lor \sees{\aterm_2}{\avariablebis}{\asetmeetvar''})\land(\avariablebis {=} \aterm_1 \implies \avariable{=} \avariablebis)\\
&\implies
\inpath{\avariable}{\avariablebis}{\avariableter} (\sees{\aterm_1}{\avariableter}{\asetmeetvar} \sim_1 \inbound_1
\land
\sees{\avariableter}{\aterm_2}{\asetmeetvar} \sim_2 \inbound_2 \land \avariableter\neq\aterm_1 \land \avariableter\neq\aterm_2)
\end{aligned}$

The proof is divided by cases by considering all the combinations of the three disjunctions ${\avariable} {=} {\aterm_1} \lor \sees{\avariable}{\aterm_1}{\asetmeetvar'} $,  ${\aterm_2}{=}{\avariablebis} \lor \sees{\aterm_2}{\avariablebis}{\asetmeetvar''}$, $\avariablebis {=} \aterm_1 \implies \avariable{=} \avariablebis$ in the hypothesis.
As all cases are very similar, here we just show the case where $\sees{\avariable}{\aterm_1}{\asetmeetvar'}$ (for the first disjunct), $\sees{\aterm_2}{\avariablebis}{\asetmeetvar''}$ (second disjunct) and $\avariablebis \neq \aterm_1$ (third disjunct) are assumed. More precisely, we show that the following formula is a tautology:
\begin{nscenter}
$
\begin{aligned}[t]
&\sees{\avariable}{\aterm_1}{\asetmeetvar} \land \seesgeq{\aterm_1}{\aterm_2}{\asetmeetvar}{\inbound_1{+}\inbound_2} \land
\sees{\aterm_2}{\avariablebis}{\asetmeetvar}\land\avariablebis \neq \aterm_1\\
&\implies
\inpath{\avariable}{\avariablebis}{\avariableter} (\sees{\aterm_1}{\avariableter}{\asetmeetvar} = \inbound_1
\land
\sees{\avariableter}{\aterm_2}{\asetmeetvar} \geq \inbound_2 \land \avariableter\neq\aterm_1 \land \avariableter\neq\aterm_2)
\end{aligned}$
\end{nscenter}
Suppose the memory state $\pair{\astore}{\aheap}$  satisfies
\begin{nscenter}
$\sees{\avariable}{\aterm_1}{\asetmeetvar'} \land \seesgeq{\aterm_1}{\aterm_2}{\asetmeetvar}{\inbound_1{+}\inbound_2} \land
\sees{\aterm_2}{\avariablebis}{\asetmeetvar''}\land\avariablebis \neq \aterm_1$
\end{nscenter}
First, we derive in $\coresys$ that  $\aterm_1 \neq \aterm_2$ (from weaker hypothesis than the ones that we have):
\[
\begin{nd}
\hypo {1} {\sees{\aterm_1}{\aterm_2}{\asetmeetvar}}
\hypo {2} {\sees{\aterm_2}{\avariablebis}{\asetmeetvar''}}
\hypo {2b} {\avariablebis \neq \aterm_1}
\hypo {3} {\aterm_1 = \aterm_2}
\have {4} {\sees{\aterm_1}{\aterm_2}{\{\avariablebis\}}} \by{\ref{core2Ax:SeesMono1}, as $\avariablebis \in \asetmeetvar$}{1}
\have {5} {\sees{\aterm_2}{\avariablebis}{\{\aterm_2\}}} \by{\ref{core2Ax:SeesMono1}, as $\aterm_2 \in \asetmeetvar''$}{2}
\have {6} {\sees{\aterm_2}{\aterm_2}{\{\aterm_2\}}} \by{\ref{core2Ax:Substitute}}{1,3}
\have {7} {\avariablebis = \aterm_2} \by{\ref{core2Ax:SeesFunc}}{5,6}
\have {8} {\avariablebis = \aterm_1} \by{\ref{core2Ax:Substitute}}{3,7}
\have {9} {\bottom} \by{\landcontr}{2b,8}
\end{nd}
\]
Then $\aterm_1 \neq \aterm_2$.
Similarly, we can prove that $\aterm_2 \neq \avariable$ (we do this semantically for conciseness).
Suppose $\aterm_2 = \avariable$. As we just proved that $\aterm_1 \neq \aterm_2$, there must be a loop involving $\avariable$, $\aterm_1$ and $\aterm_2$, here represented:
\begin{center}
     \begin{tikzpicture}[baseline]
       \node[dot,label=above:{$\avariable=\aterm_2$}] (ex) at (0,0) {};
       \node[dot,label=below:{$\aterm_1$}] (t1) [below = 1.2cm of ex] {};

       \draw[reach] (ex)  to [bend left=90] node [right] {$+$} (t1);
       \draw[reach] (t1)  to [bend left=90] node [left] {$+$} (ex);

     \end{tikzpicture}
\end{center}
Then, as the memory state satisfies $\sees{\avariable}{\aterm_1}{\asetmeetvar'} \land \sees{\aterm_1}{\aterm_2}{\asetmeetvar} \land \sees{\aterm_2}{\avariablebis}{\asetmeetvar''}$, where $\avariablebis$ is a member of $\asetmeetvar$, $\asetmeetvar'$ and $\asetmeetvar''$, the only possible location that can correspond to $\avariablebis$ is $\semantics{\aterm_1}_{\astore,\aheap}$.
However, $\pair{\astore}{\aheap}$ also satisfies $\aterm_1 \neq \avariablebis$.
We then conclude that $\aterm_2 \neq \avariable$.
Moreover, it also holds that $\avariable \neq \aterm_1$.
Again, by contradiction, suppose otherwise, i.e.\ $\avariable = \aterm_1$.
Then there is a loop involving $\avariable$, $\aterm_1$ and $\aterm_2$ and, by $\pair{\astore}{\aheap} \models \sees{\avariable}{\aterm_1}{\asetmeetvar}$ where $\aterm_2 \in \asetmeetvar$, it must hold that $\aterm_1 = \aterm_2$: a contradiction.
We conclude that one of the following possibilities needs to hold:
\begin{center}
 \scalebox{0.85}{
     \begin{tikzpicture}[baseline]
       \node[dot,label=above:{$\avariable$}] (x) at (0,0) {};
       \node[dot,label=above:{$\aterm_1$}] (t1) [right = 1cm of x] {};
       \node[dot,label=above:{$\aterm_2$}] (t2) [right = 1cm of t1] {};
       \node[dot,label=above:{$\avariablebis$}] (y) [right = 1cm of t2] {};

       \draw[reach] (x) -- node [above] {$+$} (t1);
       \draw[reach] (t1) -- node [above] {$+$} (t2);
       \draw[reach] (t2) -- node [above] {$+$} (y);
     \end{tikzpicture}
     \qquad\qquad
     \begin{tikzpicture}[baseline]
       \node[dot,label=above:{$\avariable$}] (x) at (0,0) {};
       \node[dot,label=above:{$\aterm_1$}] (t1) [right = 1.2cm of x] {};
       \node[dot,label=above:{$\aterm_2=\avariablebis$}] (t2) [right = 1cm of t1] {};

        \draw[reach] (x) -- node [above] {$+$} (t1);
        \draw[reach] (t1) -- node [above] {$+$} (t2);
        \draw[reach] (t2) to [out=0,in=-90,min distance=10mm,looseness=10] node [below] {$+$} (t2);
     \end{tikzpicture}
     \qquad\qquad
     \begin{tikzpicture}[baseline]
       \node[dot,label=above:{$\avariable=\avariablebis$}] (x) at (0,0) {};
       \node[dot,label=above:{$\aterm_1$}] (t1) [right = 1.2cm of x] {};
       \node[dot,label=above:{$\aterm_2$}] (t2) [right = 1cm of t1] {};

       \draw[reach] (x) -- node [above] {$+$} (t1);
       \draw[reach] (t1) -- node [above] {$+$} (t2);
       \draw[reach] (t2) to [bend left=90] node [below] {$+$} (x);
     \end{tikzpicture}
 }
\end{center}
For all three possibilities, we notice that
$\minpath{\astore(\avariable)}{\astore(\avariablebis)}{\aheap} \neq \emptyset$ and $$\minpath{\semantics{\aterm_1}_{\astore,\aheap}}{\semantics{\aterm_2}_{\astore,\aheap}}{\aheap} \subseteq \minpath{\astore(\avariable)}{\astore(\avariablebis)}{\aheap}$$
Moreover, by $\pair{\astore}{\aheap} \models \sees{\aterm_1}{\aterm_2}{\asetmeetvar} \geq \inbound_1{+}\inbound_2$ we have
that $\minpath{\semantics{\aterm_1}_{\astore,\aheap}}{\semantics{\aterm_2}_{\astore,\aheap}}{\aheap}$ has at least $\inbound_1{+}\inbound_2$ elements, where $\inbound_1$ and $\inbound_2$ are both at least $1$ (from the assumptions of the axiom).
Then, let $\alocation$ be such that $\aheap^{\beta_1}(\semantics{\aterm_1}_{\astore,\aheap}) = \alocation$.
As $\inbound_1$ is greater than $1$ and is strictly less than the cardinality of $\minpath{\semantics{\aterm_1}_{\astore,\aheap}}{\semantics{\aterm_2}_{\astore,\aheap}}{\aheap}$, we obtain:
\begin{itemize}
\item $\alocation \in \minpath{\semantics{\aterm_1}_{\astore,\aheap}}{\semantics{\aterm_2}_{\astore,\aheap}}{\aheap}$ and from the inclusion above $\alocation \in \minpath{\astore(\avariable)}{\astore(\avariablebis)}{\aheap}$.
\item $\alocation \neq \semantics{\aterm_1}_{\astore,\aheap}$ and $\alocation \neq \semantics{\aterm_2}_{\astore,\aheap}$.
\end{itemize}
Moreover, as $\minpath{\semantics{\aterm_1}_{\astore,\aheap}}{\semantics{\aterm_2}_{\astore,\aheap}}{\aheap}$ contains at least $\inbound_1+\inbound_2$ elements, the set $\minpath{\alocation}{\semantics{\aterm_2}_{\astore,\aheap}}{\aheap}$ contains at least $\inbound_2$ elements.
It is then easy to see that  the following holds:
\begin{nscenter}
$
\pair{\astore[\avariableter \gets \alocation]}{\aheap} \models \sees{\aterm_1}{\avariableter}{\asetmeetvar} = \inbound_1
\land
\sees{\avariableter}{\aterm_2}{\asetmeetvar} \geq \inbound_2 \land \avariableter\neq\aterm_1 \land \avariableter\neq\aterm_2
$
\end{nscenter}
where $\avariableter$ is a program variable not appearing in $\asetmeetvar$.
As $\alocation$ belongs to $\minpath{\astore(\avariable)}{\astore(\avariablebis)}{\aheap} \neq \emptyset$, by the semantics of the $\weirdexists$ quantifier we conclude:
\begin{nscenter}
$
\pair{\astore}{\aheap} \models \inpath{\avariable}{\avariablebis}{\avariableter}(\sees{\aterm_1}{\avariableter}{\asetmeetvar} = \inbound_1
\land
\sees{\avariableter}{\aterm_2}{\asetmeetvar} \geq \inbound_2 \land \avariableter\neq\aterm_1 \land \avariableter\neq\aterm_2)
$
\end{nscenter}
\item[\ref{existsAx:SeesSem}]
$\lnot \inpath{\avariable}{\avariablebis}{\avariableter}((\avariable \neq \avariableter \land \avariablebis \neq \avariableter \land \sees{\avariable}{\avariablebis}{\{\avariable,\avariableter,\avariablebis\}})
\lor \lnot \sees{\avariable}{\avariablebis}{\emptyset})$ $\assuming{\avariableter \not\in \set{\avariable,\avariablebis}}$.

Suppose $(\astore,\aheap) \models \inpath{\avariable}{\avariablebis}{\avariableter}((\avariable \neq \avariableter \land \avariablebis \neq \avariableter \land \sees{\avariable}{\avariablebis}{\{\avariable,\avariableter,\avariablebis\}})
\lor \lnot \sees{\avariable}{\avariablebis}{\emptyset})$ where $\avariableter \not\in\{\avariable,\avariablebis\}$.
Then by definition $\minpath{\astore(\avariable)}{\astore(\avariablebis)}{\aheap} \neq \emptyset$ and
there is $\alocation$ in $\minpath{\astore(\avariable)}{\astore(\avariablebis)}{\aheap}\cup\{\astore(\avariablebis)\}$ such that
$\pair{\astore[\avariableter \gets \alocation]}{\aheap} \models (\avariable \neq \avariableter \land \avariablebis \neq \avariableter \land \sees{\avariable}{\avariablebis}{\{\avariable,\avariableter,\avariablebis\}})
\lor \lnot \sees{\avariable}{\avariablebis}{\emptyset})$.
As $\minpath{\astore(\avariable)}{\astore(\avariablebis)}{\aheap} \neq \emptyset$ we obtain that $\pair{\astore}{\aheap} \models \sees{\avariable}{\avariablebis}{\emptyset}$.
Then, since $\avariableter \not \in\{\avariable,\avariablebis\}$ we conclude that
$\pair{\astore[\avariableter \gets \alocation]}{\aheap} \models \sees{\avariable}{\avariablebis}{\emptyset}$.
This implies that the second disjunct of the disjunction above is false and therefore it must hold that
\begin{nscenter}
$\pair{\astore[\avariableter \gets \alocation]}{\aheap} \models (\avariable \neq \avariableter \land \avariablebis \neq \avariableter \land \sees{\avariable}{\avariablebis}{\{\avariable,\avariableter,\avariablebis\}})$
\end{nscenter}
However, as  $\alocation$ is in $\minpath{\astore(\avariable)}{\astore(\avariablebis)}{\aheap}\cup\{\astore(\avariablebis)\}$, from the statement above we can easily derive a contradiction, as we show that
 $\avariable \neq \avariableter$ and $\avariablebis \neq \avariableter$ imply $\lnot\sees{\avariable}{\avariablebis}{\{\avariable,\avariableter,\avariablebis\}}$.
From the formula above, we have $\pair{\astore[\avariableter \gets \alocation]}{\aheap} \models \avariable \neq \avariableter \land \avariablebis \neq \avariableter$.
Then $\astore(\avariable) \neq \alocation \neq \astore(\avariablebis)$ and $\astore[\avariableter \gets \alocation](\avariableter) \in \minpath{\astore(\avariable)}{\astore(\avariablebis)}{\aheap}\setminus\{\astore(\avariable)\}$.
Hence, by definition $\minpath{\astore(\avariable)}{\astore[\avariableter \gets \alocation](\avariableter)}{\aheap} \subset \minpath{\astore(\avariable)}{\astore(\avariablebis)}{\aheap}$.
Then by definition of the sees operator, it holds that $(\astore[\avariableter \gets \alocation],\aheap) \models \sees{\avariable}{\avariableter}{\{\avariablebis\}}$.
Putting all together, we prove that
\begin{nscenter}
$(\astore[\avariableter \gets \alocation],\aheap) \models \avariablebis \neq \avariableter \land \sees{\avariable}{\avariablebis}{\{\avariable,\avariableter,\avariablebis\}} \land \sees{\avariable}{\avariableter}{\{\avariablebis\}}$
\end{nscenter}
However, this is contradictory in $\coresys$:
\[
\begin{nd}
\hypo {1} {\avariablebis \neq \avariableter}
\hypo {2} {\sees{\avariable}{\avariablebis}{\{\avariable,\avariableter,\avariablebis\}}}
\hypo {3} {\sees{\avariable}{\avariableter}{\{\avariablebis\}}}
\have {4} {\sees{\avariable}{\avariablebis}{\{\avariable,\avariableter\}}} \by{\ref{core2Ax:SeesMono1}}{2}
\have {5} {\sees{\avariable}{\avariablebis}{\{\avariableter\}}} \by{\ref{core2Ax:SeesMono1}}{4}
\have {6} {\avariablebis = \avariableter} \by{\ref{core2Ax:SeesFunc}}{3,5}
\have {7} {\bottom} \by{\landcontr}{1,6}
\end{nd}
\]
Therefore, the axiom~\ref{existsAx:SeesSem} is valid.
\end{enumerate}
\end{proof}
