# Supplementary material for: A Complete Axiomatisation for Quantifier-Free Separation Logic
Source: arXiv:2006.05156 source file (2021-08-09)
Supplement: Supplementary file 13 [file proof-lemma-ms-models-abs.tex]

In order to proof the completeness of $\coresys$, we use the notion of symbolic memory state defined in Section~\ref{section:axiom2starelim}.
Let us first recall the definition of symbolic memory states, which is a structure that simply
highlights the properties of a memory state that are expressible through core formulae, while removing the ones that are not expressible.
Given $\asetvar \subseteq_{\fin} \PVAR$ and $\bound \in \Nat^+$,
a \defstyle{symbolic memory states} $\asms$ over $\pair{\asetvar}{\bound}$ is
defined as a finite structure $\triple{\symbterms}{\amap}{\symbrem}$ such that
\begin{itemize}
\margindown
\item $\symbterms$ is a partition of a subset of $\atermset{\asetvar}$, encoding (dis)equalities. We introduce
the partial function $\equivclass{\ .\ }{\symbterms}: \atermset{\asetvar} \to \symbterms$ such that
given $\aterm \in \atermset{\asetvar}$ returns $\asymbterm \in \symbterms$ and $\aterm \in \asymbterm$, if it exists.
\item $\amap$ is a partial function from $\symbterms$ to $\symbterms\times\interval{1}{\bound}$, encoding paths between terms and their length. Then, $\pi_i \circ \amap$ is the projection of $\amap$ that goes from $\symbterms$ the $i$-th element of $\symbterms\times\interval{1}{\bound}$.
\item $\symbrem {\in} \interval{0}{\bound}$, encoding the number of memory cells (up to $\bound$)
not in paths between terms.
\margindown
\end{itemize}
We denote with $\symbdomain{\asetvar}{\bound}$ the domain of these structures.
The \defstyle{abstraction} $\symbms{\astore}{\aheap}{\asetvar}{\bound}$ of a memory state $\pair{\astore}{\aheap}$ is defined as the symbolic memory state $\triple{\symbterms}{\amap}{\symbrem}$ over $\pair{\asetvar}{\bound}$ such that
\begin{itemize}
\margindown
\item $\symbterms \egdef \{ \{ \aterm_1 \in \atermset{\asetvar} \mid \pair{\astore}{\aheap} \models \aterm_1 = \aterm_2 \} \mid \aterm_2 \in \atermset{\asetvar} \}$;
\item $\amap(\asymbterm) = (\asymbterm',\inbound)$ $\equivdef$ there are $\aterm_1 {\in} \asymbterm$ and $\aterm_2 {\in} \asymbterm'$ such that $\pair{\astore}{\aheap} \models \seesgeq{\aterm_1}{\aterm_2}{\atermset{\asetvar}}{\inbound}$ and if $\inbound < \bound$ then
$\pair{\astore}{\aheap} \models \lnot \seesgeq{\aterm_1}{\aterm_2}{\atermset{\asetvar}}{\inbound{+}1}$;
\item $\symbrem = \inbound$ $\equivdef$ $\pair{\astore}{\aheap} \models \remgeq{\atermset{\asetvar}\times\atermset{\asetvar}}{\inbound}$ and if $\inbound < \bound$ then
$\pair{\astore}{\aheap} \models \lnot\remgeq{\atermset{\asetvar}\times\atermset{\asetvar}}{\inbound{+}1}$.
\margindown
\end{itemize}
The semantics of a symbolic memory state $\triple{\symbterms}{\amap}{\symbrem}$ over $\pair{\asetvar}{\bound}$
is given through
%%  the following formula of $\conjcomb{\coreformulae{\asetvar}{\bound}}$, denoted with
the \defstyle{characteristic formula} $\charsymbform\triple{\symbterms}{\amap}{\symbrem}$ defined below:
\begin{nscenter}
$
\begin{aligned}[t]
&
\formulasubset{\rem{\atermset{\asetvar}\times\atermset{\asetvar}}{\sim}{\symbrem}}{\bmat[\text{if } \symbrem {\neq} \bound \text{ then } (\sim \text{ is } =) \text{ else } (\sim \text{ is } \geq)]}
\land\formulasubset{\aterm_1 \neq \aterm_2}{\bmat[\equivclass{\aterm_1}{\symbterms}\ \text{or}\ \equivclass{\aterm_2}{\symbterms}\ \text{undefined, or}\ \equivclass{\aterm_1}{\symbterms}\neq\equivclass{\aterm_2}{\symbterms}]}
 \\
& {\land}\formulasubset{\aterm_1 = \aterm_2}{\bmat[\equivclass{\aterm_1}{\symbterms}=\equivclass{\aterm_2}{\symbterms} \ \text{defined}]}
  \land
  \formulasubset{\lnot\sees{\aterm_1}{\aterm_2}{\atermset{\asetvar}}}{\bmat[
  \equivclass{\aterm_1}{\symbterms}\ \text{undefined or}\
  \forall\inbound\in\interval{1}{\bound}: \amap(\equivclass{\aterm_1}{\symbterms}) \neq (\equivclass{\aterm_2}{\symbterms},\inbound)]}
  \\
&{\land}
\formulasubset{\sees{\aterm_1}{\aterm_2}{\atermset{\asetvar}}{=}{\inbound}}{\bmat[
\amap(\equivclass{\aterm_1}{\symbterms}) = (\equivclass{\aterm_2}{\symbterms},\inbound)\ \text{and}\ \inbound < \bound]}
\land
\formulasubset{\seesgeq{\aterm_1}{\aterm_2}{\atermset{\asetvar}}{\inbound}}{\bmat[
\amap(\equivclass{\aterm_1}{\symbterms}) = (\equivclass{\aterm_2}{\symbterms},\inbound)\ \text{and}\ \inbound = \bound]}
\end{aligned}
$
\end{nscenter}
We want to prove the following result.
\lemmamsmodelsabs*

Which is essentially proved with the following two intermediate lemmata (Lemma~\ref{lemma:nosumdiffsms} and Lemma~\ref{lemma:absmsmodelchar}).

\begin{lemma}\label{lemma:nosumdiffsms}
Let $\triple{\symbterms}{\amap}{\symbrem}$ and $\triple{\symbterms'}{\amap'}{\symbrem'}$ be two symbolic memory state over $\pair{\asetvar}{\bound}$ such that $\charsymbform{\triple{\symbterms}{\amap}{\symbrem}}$ and $\charsymbform{\triple{\symbterms'}{\amap'}{\symbrem'}}$
are satisfiable. Then
\begin{nscenter}
$\charsymbform{\triple{\symbterms}{\amap}{\symbrem}} \land \charsymbform{\triple{\symbterms'}{\amap'}{\symbrem'}}$ is satisfiable if and only if
$\triple{\symbterms}{\amap}{\symbrem} = \triple{\symbterms'}{\amap'}{\symbrem'}$.
\end{nscenter}
\end{lemma}
\begin{proof}
The right to left direction is trivial (recall that from the hypothesis $\charsymbform{\triple{\symbterms}{\amap}{\symbrem}}$ is satisfiable and $\aformula \implies \aformula \land \aformula$ is tautological in propositional calculus).
We then focus on the left to right direction:
Suppose $\charsymbform{\triple{\symbterms}{\amap}{\symbrem}} \land \charsymbform{\triple{\symbterms'}{\amap'}{\symbrem'}}$ satisfiable. Then, we show that $\charsymbform{\triple{\symbterms}{\amap}{\symbrem}} \inside \charsymbform{\triple{\symbterms'}{\amap'}{\symbrem'}}$ and viceversa, i.e. the two characteristic formulae are syntactically equivalent.
This is sufficient to prove the lemma as by definition of the characteristic formula it is easy to conclude that two distinct symbolic memory states over
$\pair{\asetvar}{\bound}$  have distinct characteristic formulae.
By symmetry, it is sufficient to show $\charsymbform{\triple{\symbterms}{\amap}{\symbrem}} \inside \charsymbform{\triple{\symbterms'}{\amap'}{\symbrem'}}$.
\begin{itemize}
\item Suppose that there is $\inbound_1 \in \interval{0}{\bound}$ such that $\remgeq{\atermset{\asetvar}\times\atermset{\asetvar}}{\inbound_1} \inside \charsymbform{\triple{\symbterms}{\amap}{\symbrem}}$
whereas $\remgeq{\atermset{\asetvar}\times\atermset{\asetvar}}{\inbound_1} \not\inside \charsymbform\triple{\symbterms'}{\amap'}{\symbrem'}$.
Then, by definition of the characteristic formula, there is a different $\inbound_2 \in \interval{0}{\bound}\setminus\{\inbound_1\}$ such that
$\remgeq{\atermset{\asetvar}\times\atermset{\asetvar}}{\inbound_2} \inside \charsymbform(\triple{\symbterms'}{\amap'}{\symbrem'})$.
We assume $\inbound_1 < \inbound_2$ (the other case is analogous). Then it must hold that $\inbound_1 < \bound$ and hence by definition of characteristic formula
$\lnot\remgeq{\atermset{\asetvar}\times\atermset{\asetvar}}{\inbound_1+1} \inside \charsymbform{\triple{\symbterms}{\amap}{\symbrem}}$.
This leads to a contradiction as a set with at least $\inbound_2$ elements, but stricty less than $\inbound_1$ with $\inbound_1 < \inbound_2$
does not exist.
%%
%% This is contradictory, as can be seen by applying axiom~\ref{core2Ax:RemMono1}.
%% Indeed, from $\remgeq{\atermset{\asetvar}\times\terms{\asetvar}}{\inbound_2}$ and $\inbound_2 \geq \inbound_1+1$, by applying~\ref{core2Ax:RemMono1} $\inbound_2-(\inbound_1+1)$
%% times we obtain $\remgeq{\terms{\asetvar}\times\terms{\asetvar}}{\inbound_1+1}$, in contradiction with $\lnot\remgeq{\terms{\asetvar}\times\terms{\asetvar}}{\inbound_1+1}$ as by hypothesis
%% $\charsymbform{\triple{\symbterms}{\amap}{\symbrem}} \land \charsymbform{\triple{\symbterms'}{\amap'}{\symbrem'}}$ satisfiable.
Hence, for every $\inbound \in \interval{0}{\bound}$,
$\remgeq{\terms{\asetvar}\times\atermset{\asetvar}}{\inbound} \inside \charsymbform\triple{\symbterms}{\amap}{\symbrem}$ implies
$\remgeq{\terms{\asetvar}\times\atermset{\asetvar}}{\inbound} \inside \charsymbform\triple{\symbterms'}{\amap'}{\symbrem'}$.
Thanks to this, we can also prove that for every $\inbound \in \interval{0}{\bound}$
\begin{nscenter}
$\lnot \remgeq{\atermset{\asetvar}\times\atermset{\asetvar}}{\inbound} \inside \charsymbform\triple{\symbterms}{\amap}{\symbrem}$ implies
$\lnot \remgeq{\atermset{\asetvar}\times\atermset{\asetvar}}{\inbound} \inside \charsymbform\triple{\symbterms'}{\amap'}{\symbrem'}$.
\end{nscenter}
Indeed, suppose $\lnot \remgeq{\atermset{\asetvar}\times\atermset{\asetvar}}{\inbound} \inside \charsymbform\triple{\symbterms}{\amap}{\symbrem}$.
$\inbound$ must be at least $1$, as otherwise $\charsymbform\triple{\symbterms}{\amap}{\symbrem}$ will not be satisfiable (a contradiction).
%%  by axiom~\ref{core2Ax:RemPos}.
 Then by definition of the characteristic formula we have $\remgeq{\atermset{\asetvar}\times\atermset{\asetvar}}{\inbound-1} \inside \charsymbform\triple{\symbterms}{\amap}{\symbrem}$,
with $\inbound-1<\bound$, and therefore $\remgeq{\atermset{\asetvar}\times\atermset{\asetvar}}{\inbound-1} \inside \charsymbform\triple{\symbterms'}{\amap'}{\symbrem'}$.
Again by definition of the characteristic formula, as $\inbound-1<\bound$, we conclude that
$\lnot \remgeq{\atermset{\asetvar}\times\atermset{\asetvar}}{\inbound} \inside \charsymbform\triple{\symbterms'}{\amap'}{\symbrem'}$.
\item Suppose there are two terms $\aterm_1,\aterm_2 \in \atermset{\asetvar}$ such that ${\aterm_1 = \aterm_2} \inside \charsymbform{\triple{\symbterms}{\amap}{\symbrem}}$
whereas ${\aterm_1 = \aterm_2} \not\inside  \charsymbform{\triple{\symbterms'}{\amap'}{\symbrem'}}$.
Then by definition of the characteristic formula, ${\aterm_1 \neq \aterm_2} \inside  \charsymbform{\triple{\symbterms'}{\amap'}{\symbrem'}}$ and we conclude that $\charsymbform\triple{\symbterms}{\amap}{\symbrem} \land \charsymbform{\triple{\symbterms'}{\amap'}{\symbrem'}}$ is unsatisfiable: a contradiction.
A similar contradiction is found when we suppose ${\aterm_1 \neq \aterm_2} \inside \charsymbform{\triple{\symbterms}{\amap}{\symbrem}}$
whereas ${\aterm_1 \neq \aterm_2} \not\inside  \charsymbform{\triple{\symbterms'}{\amap'}{\symbrem'}}$, as then by definition of the characteristic formula it follows that ${\aterm_1 = \aterm_2} \inside  \charsymbform{\triple{\symbterms'}{\amap'}{\symbrem'}}$.
\item Suppose that there are two terms $\aterm_1,\aterm_2 \in \atermset{\asetvar}$ and $\inbound_1 \in \interval{1}{\bound}$ s.t.\
$\seesgeq{\aterm_1}{\aterm_2}{\atermset{\asetvar}}{\inbound_1} \inside \charsymbform{\triple{\symbterms}{\amap}{\symbrem}}$ whereas
$\seesgeq{\aterm_1}{\aterm_2}{\atermset{\asetvar}}{\inbound_1} \not\inside \charsymbform{\triple{\symbterms'}{\amap'}{\symbrem'}}$. Then by definition of the characteristic formula there are two possibilities:
\begin{enumerate}
\item There is a different $\inbound_2 \in \interval{1}{\bound}\setminus\{\inbound_1\}$ such that
$\seesgeq{\aterm_1}{\aterm_2}{\atermset{\asetvar}}{\inbound_2} \inside \charsymbform{\triple{\symbterms'}{\amap'}{\symbrem'}}$.
Then the proof is similar to the first case above. We assume $\inbound_1 < \inbound_2$ (the other case is analogous).
Then it must hold that $\inbound_1 < \bound$ and hence by definition of characteristic formula $\lnot\seesgeq{\aterm_1}{\aterm_2}{\atermset{\asetvar}}{\inbound_1+1} \inside \charsymbform{\triple{\symbterms}{\amap}{\symbrem}}$.
This leads to a contradiction as a set with at least $\inbound_2$ elements, but stricty less than $\inbound_1$ with $\inbound_1 < \inbound_2$
does not exist.
%% This is contradictory, as can be seen by applying axiom~\ref{core2Ax:SeesMono2}.
%% Indeed, from $\seesgeq{\aterm_1}{\aterm_2}{\terms{\asetvar}}{\inbound_2}$ and $\inbound_2 \geq \inbound_1+1 \geq 2$, by applying~\ref{core2Ax:RemMono1} $\inbound_2-(\inbound_1+1)$
%% times we obtain $\seesgeq{\aterm_1}{\aterm_2}{\atermset{\asetvar}}{\inbound_1+1}$, in contradiction with $\lnot \seesgeq{\aterm_1}{\aterm_2}{\atermset{\asetvar}}{\inbound_1+1}$ as by hypothesis
%% $\charsymbform{\triple{\symbterms}{\amap}{\symbrem}} \land \charsymbform{\triple{\symbterms'}{\amap'}{\symbrem'}}$ satisfiable.
\item $\lnot \sees{\aterm_1}{\aterm_2}{\atermset{\asetvar}} \inside \charsymbform{\triple{\symbterms'}{\amap'}{\symbrem'}}$. Again, this is contradictory by the axiom~\ref{core2Ax:SeesMono2} and
$\charsymbform{\triple{\symbterms}{\amap}{\symbrem}} \land \charsymbform{\triple{\symbterms'}{\amap'}{\symbrem'}}$ satisfiable by hypothesis.
Indeed, from $\seesgeq{\aterm_1}{\aterm_2}{\atermset{\asetvar}}{\inbound_1}$ we can apply $\inbound_1-1$ times axiom~\ref{core2Ax:SeesMono2} and obtain $\sees{\aterm_1}{\aterm_2}{\atermset{\asetvar}}$.
\end{enumerate}
We then conclude that
for all terms $\aterm_1,\aterm_2 \in \atermset{\asetvar}$ and $\inbound_1 \in \interval{1}{\bound}$,
\begin{nscenter}
$\seesgeq{\aterm_1}{\aterm_2}{\atermset{\asetvar}}{\inbound_1} \inside \charsymbform{\triple{\symbterms}{\amap}{\symbrem}}$ implies
$\seesgeq{\aterm_1}{\aterm_2}{\atermset{\asetvar}}{\inbound_1} \inside \charsymbform{\triple{\symbterms'}{\amap'}{\symbrem'}}$.
\end{nscenter}
Thanks to this we can also prove that for every $\inbound \in \interval{1}{\bound}$,
\begin{nscenter}
$\lnot\seesgeq{\aterm_1}{\aterm_2}{\atermset{\asetvar}}{\inbound} \inside \charsymbform{\triple{\symbterms}{\amap}{\symbrem}}$ implies
$\lnot\seesgeq{\aterm_1}{\aterm_2}{\atermset{\asetvar}}{\inbound} \inside \charsymbform{\triple{\symbterms'}{\amap'}{\symbrem'}}$.
\end{nscenter}
Indeed, suppose $\seesgeq{\aterm_1}{\aterm_2}{\atermset{\asetvar}}{\inbound} \inside \charsymbform{\triple{\symbterms}{\amap}{\symbrem}}$.
If $\inbound = 1$ then, as $\charsymbform{\triple{\symbterms}{\amap}{\symbrem}} \land \charsymbform{\triple{\symbterms'}{\amap'}{\symbrem'}}$ is satisfiable and by axiom~\ref{core2Ax:SeesMono2}, it cannot be that there is $\inbound_1 \in\interval{1}{\bound}$ such that
$\seesgeq{\aterm_1}{\aterm_2}{\atermset{\asetvar}}{\inbound_1} \inside \charsymbform{\triple{\symbterms'}{\amap'}{\symbrem'}}$.
Hence by definition of the characteristic formula we obtain $\lnot\seesgeq{\aterm_1}{\aterm_2}{\atermset{\asetvar}}{\inbound} \inside \charsymbform{\triple{\symbterms'}{\amap'}{\symbrem'}}$.
Suppose instead $\inbound \geq 2$. Then by definition of the characteristic formula
$\seesgeq{\aterm_1}{\aterm_2}{\atermset{\asetvar}}{\inbound-1} \inside \charsymbform{\triple{\symbterms}{\amap}{\symbrem}}$ and therefore
$\seesgeq{\aterm_1}{\aterm_2}{\atermset{\asetvar}}{\inbound-1} \inside \charsymbform{\triple{\symbterms'}{\amap'}{\symbrem'}}$.
Again by definition of the characteristic formula
$\lnot\seesgeq{\aterm_1}{\aterm_2}{\atermset{\asetvar}}{\inbound} \inside \charsymbform{\triple{\symbterms'}{\amap'}{\symbrem'}}$.
\qedhere
\end{itemize}
\end{proof}

\begin{lemma}\label{lemma:absmsmodelchar}
Let $\pair{\astore}{\aheap}$ be a memory state, $\asetvar\subseteq_\fin\PVAR$ and $\bound \in \Nat^+$.
It holds that $\pair{\astore}{\aheap} \models \charsymbform({\symbms{\astore}{\aheap}{\asetvar}{\bound}})$.
\end{lemma}
\begin{proof}
We sketch the proof, that can easily be shown from
the definitions of $\symbms{\astore}{\aheap}{\asetvar}{\bound}$  and $\charsymbform{\triple{\symbterms}{\amap}{\symbrem}}$,
by developing the case for the first conjunct of the characteristic formula, i.e. we prove that
\begin{nscenter}
$\pair{\astore}{\aheap} \models \formulasubset{\rem{\atermset{\asetvar}\times\atermset{\asetvar}}{\sim}{\symbrem}}{\bmat[\text{if } \symbrem {=} \bound \text{ then } (\sim \text{ is } =) \text{ else } (\sim \text{ is } \geq)]}$
\end{nscenter}
so that the relation between abstraction of a symbolic memory state and its characteristic formula will become transparent.
\emph{All other conjuncts can be shown in a similar way}.

Suppose $\pair{\astore}{\aheap} \models \remgeq{\atermset{\asetvar}\times\atermset{\asetvar}}{\inbound}$ for $\inbound < \bound$ and
$\pair{\astore}{\aheap} \models \lnot\remgeq{\atermset{\asetvar}\times\atermset{\asetvar}}{\inbound{+}1}$.
Then by definition $\charsymbform({\symbms{\astore}{\aheap}{\asetvar}{\bound}})$ is a symbolic memory state $\triple{\symbterms}{\amap}{\symbrem}$ over $\pair{\asetvar}{\bound}$ such that $\symbrem = \inbound$.
Hence, in the characteristic formula of $\triple{\symbterms}{\amap}{\symbrem}$, it holds that the conjunction
$\formulasubset{\rem{\atermset{\asetvar}\times\atermset{\asetvar}}{\sim}{\symbrem}}{\bmat[\text{if } \symbrem {=} \bound \text{ then } (\sim \text{ is } =) \text{ else } (\sim \text{ is } \geq)]}$
is
$\rem{\atermset{\asetvar}\times\atermset{\asetvar}}{=}{\inbound}$, which is defined as
$$\remgeq{\atermset{\asetvar}\times\atermset{\asetvar}}{\inbound} \land \lnot\remgeq{\atermset{\asetvar}\times\atermset{\asetvar}}{\inbound{+}1}.
$$
As we have that $\pair{\astore}{\aheap}$ satisfies $\remgeq{\atermset{\asetvar}\times\atermset{\asetvar}}{\inbound}$ and
$\lnot\remgeq{\atermset{\asetvar}\times\atermset{\asetvar}}{\inbound{+}1}$, we obtain
$\pair{\astore}{\aheap} \models \remgeq{\atermset{\asetvar}\times\atermset{\asetvar}}{\inbound} \land \lnot\remgeq{\atermset{\asetvar}\times\atermset{\asetvar}}{\inbound{+}1}$ and therefore
\begin{nscenter}
$\pair{\astore}{\aheap} \models \formulasubset{\rem{\atermset{\asetvar}\times\atermset{\asetvar}}{\sim}{\symbrem}}{\bmat[\text{if } \symbrem {=} \bound \text{ then } (\sim \text{ is } =) \text{ else } (\sim \text{ is } \geq)]}$
\end{nscenter}
If instead $\pair{\astore}{\aheap} \models \remgeq{\atermset{\asetvar}\times\atermset{\asetvar}}{\bound}$, then by definition
$\charsymbform({\symbms{\astore}{\aheap}{\asetvar}{\bound}})$ is a symbolic memory state $\triple{\symbterms}{\amap}{\symbrem}$ over $\pair{\asetvar}{\bound}$ such that $\symbrem = \bound$.
Hence, in the characteristic formula of $\triple{\symbterms}{\amap}{\symbrem}$, it holds that the conjunction
$\formulasubset{\rem{\atermset{\asetvar}\times\atermset{\asetvar}}{\sim}{\symbrem}}{\bmat[\text{if } \symbrem {=} \bound \text{ then } (\sim \text{ is } =) \text{ else } (\sim \text{ is } \geq)]}$
is
$\remgeq{\atermset{\asetvar}\times\atermset{\asetvar}}{\bound}$, which is satisfied by $\pair{\astore}{\aheap}$. Again,
\begin{nscenter}
$\pair{\astore}{\aheap} \models \formulasubset{\rem{\atermset{\asetvar}\times\atermset{\asetvar}}{\sim}{\symbrem}}{\bmat[\text{if } \symbrem {=} \bound \text{ then } (\sim \text{ is } =) \text{ else } (\sim \text{ is } \geq)]}$
\qedhere
\end{nscenter}
\end{proof}

Then, Lemma~\ref{lemma:msmodelsabs} can be easily shown as follows.

\begin{proof}
For the left to right direction,
suppose that
$\pair{\astore}{\aheap} \models \charsymbform(\asms)$ where $\asms$ is a symbolic memory state over $\pair{\asetvar}{\bound}$.
By Lemma~\ref{lemma:absmsmodelchar} it holds that $\pair{\astore}{\aheap} \models \charsymbform({\symbms{\astore}{\aheap}{\asetvar}{\bound}})$.
Then it must hold that
$\pair{\astore}{\aheap} \models \charsymbform(\asms) \land \charsymbform({\symbms{\astore}{\aheap}{\asetvar}{\bound}})$. As
$\charsymbform(\asms) \land \charsymbform({\symbms{\astore}{\aheap}{\asetvar}{\bound}})$
is then satisfiable, by applying
Lemma~\ref{lemma:nosumdiffsms} we conclude that $\asms = \symbms{\astore}{\aheap}{\asetvar}{\bound}$.

The right to left direction is instead exactly Lemma~\ref{lemma:absmsmodelchar}.
\end{proof}
