# Supplementary material for: A Complete Axiomatisation for Quantifier-Free Separation Logic
Source: arXiv:2006.05156 source file (2021-08-09)
Supplement: Supplementary file 14 [file proof-lemmaaxiomtwoRCct.tex]

We finally have all the ingredients we need in order to prove Lemma~\ref{lemma:axiomtwoRCct}.

\begin{proof}
As in Lemma~\ref{prop:corePSLtwo},
the ``only if'' part follows from the validity of the axioms, proved in Lemma~\ref{lemma:axiomstwocoresound}.
Therefore, we prove the ``if'' part. Let $\aformula \in \coretype{\asetvar}{\bound}$ be fixed such that
the system $\coresys$ cannot prove $\aformula \implies \bottom$ with any proof having formulae from $\coreformulae{\asetvar}{\bound}$, and let us prove that $\aformula$ is satisfiable.
We use the same shortcut
``\elseabsurd{(statement$_1$)}{(statement$_2$)}'' introduced in the proof of Lemma~\ref{lemma:axiomstwoRCchars} (and refer to this proof to the description of this schortcut).
We start by deriving four properties of $\aformula$:
\begin{enumerate}
\item
\elseabsurd{axiom~\ref{core2Ax:Self},
\ref{core2Ax:EqSymm} and
\ref{core2Ax:Substitute}}{%
there is an equivalence relation $\approx$ on the defined terms of $\atermset{\asetvar}$, i.e. the set of terms $\{\aterm \mid \aterm = \aterm \inside \aformula\}$, such that
$\aterm_1\approx\aterm_2$ iff $\aterm_1=\aterm_2$ occurs positively
in $\aformula$}
We write $[\aterm]$ to denote the equivalence class of $\aterm$
with respect to $\approx$.
\item \elseabsurd{\ref{core2Ax:SeesMono1} and \ref{core2Ax:SeesFunc}}{the axiom system induces a functional relation of the sees predicate, that is
$\sees{\aterm_1}{\aterm_2}{\terms{\asetvar}} \inside \aformula$ and $\sees{\aterm_1}{\aterm_3}{\terms{\asetvar}} \inside \aformula$ imply $\aterm_2 \approx \aterm_3$}
Indeed, suppose $\sees{\aterm_1}{\aterm_2}{\terms{\asetvar}} \inside \aformula$ and $\sees{\aterm_1}{\aterm_3}{\terms{\asetvar}} \inside \aformula$.
Then, by repeated application of \ref{core2Ax:SeesMono1} we conclude that $\sees{\aterm_1}{\aterm_2}{\{\aterm_3\}}$ and $\sees{\aterm_1}{\aterm_3}{\{\aterm_2\}}$ must occur positively in $\aformula$ as otherwise $\prove_{\coresys}\aformula \implies \bottom$ (by only using derivation steps with formulae from $\coreformulae{\asetvar}{1}$).
\elseabsurd{axiom \ref{core2Ax:SeesFunc}}{$\aterm_2 = \aterm_3 \inside \aformula$}
Then, $\aterm_2 \approx \aterm_3$ by definition of $\approx$.
Moreover, \elseabsurd{axiom \ref{core2Ax:Substitute}}{if $\sees{\aterm_1}{\aterm_2}{\atermset{\asetvar}} \inside \aformula$ and $\aterm_1 \approx \aterm_3$ then $\sees{\aterm_3}{\aterm_2}{\atermset{\asetvar}} \inside \aformula$}
\item For each $\sees{\aterm_1}{\aterm_2}{\atermset{\asetvar}}$ occurring positively in $\aformula$ there is a bound, denoted here $\inbound_{\aterm_1,\aterm_2}$, maximal in $\interval{1}{\bound}$
and such that for every $\inbound' \leq \inbound_{\aterm_1,\aterm_2}$ $\seesgeq{\aterm_1}{\aterm_2}{\atermset{\asetvar}}{\inbound'} \inside \aformula$.
Indeed, this holds by axiom \ref{core2Ax:SeesMono2}.
\item
\elseabsurd{\ref{core2Ax:RemPos} and \ref{core2Ax:RemMono1} (instantiated so that $\asetpath = \atermset{\asetvar}\times\terms{\asetvar}$)}{
there is a bound, denoted here $\inbound_{\mathtt{rem}}$, maximal in $\interval{0}{\bound}$ and such that for every $\inbound \leq \inbound_{\mathtt{rem}}$
$\remgeq{\atermset{\asetvar}\times\atermset{\asetvar}}{\inbound_{\mathtt{rem}}} \inside \aformula$}
\end{enumerate}
Notice that, whenever one of these four properties is violated we  obtain (in contradiction with the hypothesis) a proof of
$\aformula \implies \bottom$ (this is the meaning of the shortcut ``\elseabsurd{(statement$_1$)}{(statement$_2$)}'') where all derivation steps only have formulae from $\coreformulae{\asetvar}{\bound}$, as all axiom schema used above are instantiated with formulae of this set.
By the second and third properties of $\aformula$ we conclude that
there is a partial map
\begin{nscenter}
$\amap: (\atermset{\asetvar}/\!\approx)\to\pair{\atermset{\asetvar}/\!\approx}{\interval{1}{\bound}}$
\end{nscenter}
on equivalence classes such
that $\seesgeq{\aterm_1}{\aterm_2}{\atermset{\asetvar}}{\inbound_{\aterm_1,\aterm_2}} \inside \aformula$ iff $f([\aterm_1])$ is defined and $f([\aterm_1])=([\aterm_2],\inbound_{\aterm_1,\aterm_2})$, where
$\inbound_{\aterm_1,\aterm_2}$ is again the maximal bound s.t.\ $\seesgeq{\aterm_1}{\aterm_2}{\atermset{\asetvar}}{\inbound_{\aterm_1,\aterm_2}}$ occurs positively in $\aformula$.
Hence, we conclude that the structure $\triple{\atermset{\asetvar}/\!\approx}{\amap}{\inbound_{\mathtt{rem}}}$ is a symbolic memory state over $\pair{\asetvar}{\bound}$.
In what follows, we apply Lemmata~\ref{lemma:axiomstwoRCchars} and \ref{lemma:coretypecharsms} to conclude that $\aformula$ is satisfiable.

The characteristic formula $\charsymbform{\triple{\terms{\asetvar}/\!\approx}{\amap}{\inbound_{\mathtt{rem}}}}$ is defined as
\begin{nscenter}
$
\begin{aligned}[t]
&
\formulasubset{\rem{\atermset{\asetvar}\times\atermset{\asetvar}}{\sim}{\inbound_{\mathtt{rem}}}}{\bmat[\text{if}\
\inbound_{\mathtt{rem}} {=} \bound\ \text{then}\ (\sim\ \text{is}\ =)\ \text{else}\ (\sim\ \text{is}\ \geq)]}
\land\formulasubset{\aterm_1 \neq \aterm_2}{\bmat[{[\aterm_1]}\ \text{or}\ {[\aterm_2]}\ \text{undefined, or}\ \aterm_1\not\approx\aterm_2]}
\\
&{\land} \formulasubset{\aterm_1 = \aterm_2}{\bmat[\aterm_1 \approx \aterm_2]}
  \land
  \formulasubset{\lnot\sees{\aterm_1}{\aterm_2}{\atermset{\asetvar}}}{\bmat[
  {[\aterm_1]}\ \text{undefined or}\
  \forall\inbound\in\interval{1}{\bound}: \amap({[\aterm_1]}) \neq ({[\aterm_2]},\inbound)]}
  \\
&{\land}
\formulasubset{\sees{\aterm_1}{\aterm_2}{\atermset{\asetvar}}{\sim}{\inbound_{\aterm_1,\aterm_2}}}
{\bmat[
\amap({[\aterm_1]}) = ({[\aterm_2]},\inbound_{\aterm_1,\aterm_2})\ \text{and if}\
\inbound_{\aterm_1,\aterm_2} = \bound \ \text{then}\ (\sim\ \text{is}\ =)\ \text{else}\ (\sim\ \text{is}\ \geq)]}
\end{aligned}
$
\end{nscenter}
By definition, it is easy to see that $\charsymbform{\triple{\terms{\asetvar}/\!\approx}{\amap}{\inbound_{\mathtt{rem}}}} \inside \aformula$.
By propositional calculus we obtain
$\prove_{\coresys} \aformula \implies \charsymbform{\triple{\terms{\asetvar}/\!\approx}{\amap}{\inbound_{\mathtt{rem}}}}$
and, as by hypothesis $\coresys$ cannot prove $\aformula \implies \bottom$ with any proof having formulae from $\coreformulae{\asetvar}{\bound}$, the same statement holds for $\charsymbform{\triple{\terms{\asetvar}/\!\approx}{\amap}{\inbound_{\mathtt{rem}}}} \implies \bottom$.
Then, by Lemma~\ref{lemma:axiomstwoRCchars},
$\charsymbform{\triple{\terms{\asetvar}/\!\approx}{\amap}{\inbound_{\mathtt{rem}}}}$ is satisfiable.

We now apply Lemma~\ref{lemma:coretypecharsms}.
As $\charsymbform{\triple{\terms{\asetvar}/\!\approx}{\amap}{\inbound_{\mathtt{rem}}}}$ is satisfiable, there is exactly one core type $\aformulabis \in \coretype{\asetvar}{\bound}$ such that
$\prove_{\coresys} \charsymbform{\triple{\terms{\asetvar}/\!\approx}{\amap}{\inbound_{\mathtt{rem}}}} \Leftrightarrow \aformulabis$.
Again, the proof of
$\charsymbform{\triple{\terms{\asetvar}/\!\approx}{\amap}{\inbound_{\mathtt{rem}}}} \Leftrightarrow \aformulabis$
only uses formulae from $\coreformulae{\asetvar}{\bound}$.
Notice that then $\aformulabis$ is also satisfiable.
By propositional calculus we have $\prove_{\coresys} \aformula \implies \aformula \land \aformulabis$.

Recall that, by definition of core types, $\literals{\aformula}$ and $\literals{\aformulabis}$ both include every core formula from $\coreformulae{\asetvar}{\bound}$.
Suppose then that there is a core formula $\aformulater \in \coreformulae{\asetvar}{\bound}$ that appears positively in one of the two formulae $\aformula$, $\aformulabis$ and negatively in the other. Then by propositional calculus $\prove_{\coresys} \aformula \land \aformulabis \implies \bottom$.
However, from $\prove_{\coresys} \aformula  \implies \aformula \land \aformulabis$ we then conclude $\prove_{\coresys} \aformula \implies \bottom$, in contradiction with the hypothesis.
Hence $\aformula$ and $\aformulabis$ agree on the satisfaction of every core formulae.
More precisely, as they are core types, $\aformulabis$ is syntactically equivalent to $\aformula$ up to commutativity and associativity of $\land$.
Then $\prove_{\coresys} \aformula \iff \aformulabis$.
As $\aformulabis$ is satisfiable, we conclude that $\aformula$ is satisfiable.
\end{proof}
