# Supplementary material for: A Complete Axiomatisation for Quantifier-Free Separation Logic
Source: arXiv:2006.05156 source file (2021-08-09)
Supplement: Supplementary file 15 [file proof-lemmacoretypecharsms.tex]

We start by extending the definition of \emph{types} to arbitrary finite sets of formulae of \intervalSL.
Let $F$ be a finite set of formulae. We say that a formula $\aformula$ is a \emph{type} for $F$ if and only if
it is a conjunction of the form $\aliteral_1 \land \dots \land \aliteral_n$ where
\begin{itemize}
 \item for every $i \in \interval{1}{n}$, $\aliteral_i$ is a formula from  $F$ or its negation;
 \item for every formula $\aformulabis \in F$, there is $i \in \interval{1}{n}$ such that $\aliteral_i = \aformulabis$ or $\aliteral_i = \lnot \aformulabis$;
 \item for every $i,j \in \interval{1}{n}$ $\aliteral_i \neq \lnot \aliteral_j$.
\end{itemize}
It is easy to see that in \intervalSL, a core type $\aformula \in \coretype{\asetvar}{\bound}$ is a type
for $\coreformulae{\asetvar}{\bound}$, with the meaning provided in the above definition. 
From this definition, it is clear that given two types $\aformula$ and $\aformulabis$ for $F$, the formula
$\aformula \land \aformulabis$ is satisfiable if and only if $\aformula$ and $\aformulabis$ are satisfiable and they are syntactically equivalent up to commutativity and associativity of $\land$.

In this section we want to prove the following result

\begin{restatable}{lemma}{lemmacoretypecharsms}\label{lemma:coretypecharsms}
Let $\asms$ be a symbolic memory state over $\pair{\asetvar}{\bound}$.
There is $\aformulabis {\in} \coretype{\asetvar}{\bound}$ s.t.\ $\prove_{\coresys} \charsymbform(\asms)\Leftrightarrow \aformulabis$ where all derivation steps only have formulae from $\boolcomb{\coreformulae{\asetvar}{\bound}}$.
Moreover, if $\charsymbform(\asms)$ is satisfiable, then $\aformulabis$ is unique.
\end{restatable}

The proof is essentially split into several technical lemmata, each presenting a key step in obtaining the result.
In a sense, these technical lemmata describe a strategy (in terms of proofs in $\coresys$) that can be used to obtain a core type from a characteristic formula, where the $i$th lemma represent the $i$th step in this strategy.

First, we look at equalities between terms and $\mathtt{sees}$ predicates.
Let $\asetvar \subseteq_\fin \PVAR$ and $\bound \in \Nat^+$.
Given  $\asetmeetvar \subseteq \atermset{\asetvar}$, we denote with $\coreseeseq{\asetmeetvar}{\bound}$ the set
\begin{nscenter}
$\{ \aterm_1 = \aterm_2, \seesgeq{\aterm_1}{\aterm_2}{\asetmeetvar}{\inbound} \mid \aterm_1,\aterm_2 \in \asetmeetvar, \inbound \in \interval{1}{\bound} \}$.
\end{nscenter}
Essentially, the following technical lemma implies that, given a characteristic formula, it is possible to deterministically complete every instance of the $\mathtt{sees}$ predicates (as we make explicit in Lemma~\ref{lemma:completesees}, afterwards).
Then, just by using this result, from a characteristic formula, we can deduce almost a core type, the only exception being the $\mathtt{rem}$ formulae, essentially treated in Lemma~\ref{lemma:closingrem1}.

\begin{lemma}\label{lemma:closingsees}
Let $\aformula \in \conjcomb{\coreformulae{\asetvar}{\bound}}$ be a satisfiable type for $\coreseeseq{\asetmeetvar}{\bound}$.
Let $\aterm \in \asetmeetvar$ and $\asetmeetvar' = \asetmeetvar \setminus \{\aterm\}$.
There exists one and only one $\aformulabis \in \conjcomb{\coreformulae{\asetvar}{\bound}}$ type for $\coreseeseq{\asetmeetvar'}{\bound}$ such that $\prove_{\coresys} \aformula \implies \aformulabis$. Moreover, the proof can be done with derivation steps that only have formulae from $\boolcomb{\coreformulae{\asetvar}{\bound}}$.
\end{lemma}

\begin{proof}(sketch)
The proof distinguishes two cases, depending on whether or not there exists $\aterm' \in \asetmeetvar'$ such that $\aterm = \aterm' \inside \aformula$.
\begin{itemize}
\item
For the first case, suppose there exists $\aterm' \in \asetmeetvar'$ such that $\aterm = \aterm' \inside \aformula$.
Then $\aformulabis$ is
\begin{nscenter}
$\begin{aligned}[t]
&\formulasubset{\aterm_1 \sim \aterm_2}{\bmat[\aterm_1,\aterm_2 \in \asetmeetvar',\ \sim \in \{=,\neq\},\ \aterm_1\sim\aterm_2 \inside \aformula]}
\land
\formulasubset{\seesgeq{\aterm_1}{\aterm_2}{\asetmeetvar'}{\inbound}}{\bmat[ \aterm_1,\aterm_2 \in \asetmeetvar',\  \seesgeq{\aterm_1}{\aterm_2}{\asetmeetvar}{\inbound} \inside \aformula]}\\
&\land
\formulasubset{\lnot\seesgeq{\aterm_1}{\aterm_2}{\asetmeetvar'}{\inbound}}{\bmat[ \aterm_1,\aterm_2 \in \asetmeetvar',\  \lnot\seesgeq{\aterm_1}{\aterm_2}{\asetmeetvar}{\inbound} \inside \aformula]}.
\end{aligned}$
\end{nscenter}
It is trivial to check that this formula is a type for $\coreseeseq{\asetmeetvar'}{\bound}$.
Moreover, $\prove_{\coresys} \aformula \implies \aformulabis$ holds easily.
Indeed, the first set in the conjunction, i.e. $\formulasubset{\aterm_1 \sim \aterm_2}{\bmat[\aterm_1,\aterm_2 \in \asetmeetvar',\ \sim \in \{=,\neq\},\ \aterm_1\sim\aterm_2 \inside \aformula]}$, is made of subformulae of $\aformula$, hence simply by propositional calculus
\begin{nscenter}
$\prove_{\coresys} \aformula \implies \formulasubset{\aterm_1 \sim \aterm_2}{\bmat[\aterm_1,\aterm_2 \in \asetmeetvar',\ \sim \in \{=,\neq\},\ \aterm_1\sim\aterm_2 \inside \aformula]}.$
\end{nscenter}
The remaining part of the formula, instead, follows trivially by application of the tautology
\begin{nscenter}
$\aterm = \aterm' \implies (\seesgeq{\aterm_1}{\aterm_2}{\asetmeetvar\cup\{\aterm'\}}{\inbound} \iff \seesgeq{\aterm_1}{\aterm_2}{\asetmeetvar\cup\{\aterm,\aterm'\}}{\inbound}),$
\end{nscenter}
which can be easily proved. Indeed, the left to right direction of the double implication is by the axiom~\ref{core2Ax:SeesTermEq}
whereas the right to left direction is precisely the axiom~\ref{core2Ax:SeesMono1}.
\item Otherwise (second case), for every $\aterm' \in \asetmeetvar'$, $\aterm = \aterm' \not\inside \aformula$.
As $\aformula$ is a type for $\coreseeseq{\asetmeetvar}{\bound}$, $\aterm = \aterm' \not\inside \aformula$ iff $\aterm \neq \aterm' \inside \aformula$.
Therefore we have that for every  $\aterm' \in \asetmeetvar'$, $\aterm \neq \aterm' \inside \aformula$.
We show that $\prove_{\coresys} \aformula \implies \aformulabis$, where $\aformulabis$ is
\begin{nscenter}
$
\begin{aligned}[t]
&\formulasubset{\aterm_1 \sim \aterm_2}{\bmat[ \aterm_1,\aterm_2 \in \asetmeetvar',\ \sim \in \{=,\neq\},\ \aterm_1\sim\aterm_2 \inside \aformula]}
\\
&\land \formulasubset{\seesgeq{\aterm_1}{\aterm_2}{\asetmeetvar'}{\inbound}}{\bmat[ \aterm_1,\aterm_2 \in \asetmeetvar',\ \seesgeq{\aterm_1}{\aterm_2}{\asetmeetvar}{\inbound} \inside \aformula]}
\\
&\land \formulasubset{\lnot\seesgeq{\aterm_1}{\aterm_2}{\asetmeetvar'}{\inbound}}{\bmat[ \aterm_1,\aterm_2 \in \asetmeetvar',\
\sees{\aterm_1}{\aterm_2}{\asetmeetvar} \land \lnot\seesgeq{\aterm_1}{\aterm_2}{\asetmeetvar}{\inbound} \inside \aformula]}\\
&\land \formulasubset{\lnot\seesgeq{\aterm_1}{\aterm_2}{\asetmeetvar'}{\inbound}}{\bmat[\aterm_1,\aterm_2 \in \asetmeetvar', \inbound \in \interval{1}{\bound}, 
\lnot\sees{\aterm_1}{\aterm_2}{\asetmeetvar} \inside \aformula\ \text{and}\ \sees{\aterm_1}{\aterm}{\asetmeetvar} \land \sees{\aterm}{\aterm_2}{\asetmeetvar} \not\inside \aformula]}\\
&\land \formulasubset{\seesgeq{\aterm_1}{\aterm_2}{\asetmeetvar'}{\inbound_1+\inbound_2}}{\bmat[\aterm_1,\aterm_2 \in \asetmeetvar',\ \inbound_1+\inbound_2 \leq \bound,\
\lnot\sees{\aterm_1}{\aterm_2}{\asetmeetvar} \inside \aformula\ \text{and}\\ \seesgeq{\aterm_1}{\aterm}{\asetmeetvar}{\inbound'} \land \seesgeq{\aterm}{\aterm_2}{\asetmeetvar}{\inbound_2} \inside \aformula]}\\
&\land \formulasubset{\lnot\seesgeq{\aterm_1}{\aterm_2}{\asetmeetvar'}{\inbound_1+\inbound_2\dotminus 1}}{\bmat[\aterm_1,\aterm_2 \in \asetmeetvar',\ \inbound_1+\inbound_2 \leq \bound,\
\lnot\sees{\aterm_1}{\aterm_2}{\asetmeetvar} \inside \aformula\ \text{and}\\ \sees{\aterm_1}{\aterm}{\asetmeetvar} \land \sees{\aterm}{\aterm_2}{\asetmeetvar} \inside \aformula\ \text{and}\\
 \lnot\seesgeq{\aterm_1}{\aterm}{\asetmeetvar}{\inbound_1} \land \lnot\seesgeq{\aterm}{\aterm_2}{\asetmeetvar}{\inbound_2} \inside \aformula]}
\end{aligned}
$
\end{nscenter}
It is quite easy to see that $\aformulabis$ is a type for $\coreseeseq{\asetmeetvar'}{\bound}$.
\begin{itemize}
\item From the first conjunct we have that for all $\aterm_1,\aterm_2 \in \asetmeetvar'$, $\orliterals{\aterm_1 = \aterm_2}{\aterm_1 \neq \aterm_2} \inside \aformulabis$.
\item Fix now two terms $\aterm_1,\aterm_2 \in \asetmeetvar'$:
\begin{itemize}
\item if $\sees{\aterm_1}{\aterm_2}{\asetmeetvar} \inside \aformula$, then from the second and third sets in the conjunction $\aformulabis$,
we obtain that for every $\inbound \in \interval{1}{\bound}$,
$\orliterals{\seesgeq{\aterm_1}{\aterm_2}{\asetmeetvar'}{\inbound}}{\lnot\seesgeq{\aterm_1}{\aterm_2}{\asetmeetvar'}{\inbound}} \inside \aformulabis$.
\item if instead $\lnot\sees{\aterm_1}{\aterm_2}{\asetmeetvar} \inside \aformula$, we have two cases:
\begin{itemize}
\item if $\seesgeq{\aterm_1}{\aterm}{\asetmeetvar}{\inbound'} \land \seesgeq{\aterm}{\aterm_2}{\asetmeetvar}{\inbound_2} \not\inside \aformula$, then from the fourth set in the conjunction we obtain that for every
$\inbound \in \interval{1}{\bound}$, $\lnot\seesgeq{\aterm_1}{\aterm_2}{\asetmeetvar'}{\inbound} \inside \aformulabis$;
\item if instead $\seesgeq{\aterm_1}{\aterm}{\asetmeetvar}{\inbound'} \land \seesgeq{\aterm}{\aterm_2}{\asetmeetvar}{\inbound_2} \inside \aformula$, then for the fifth and sixth sets in the conjunction we have that for every $\inbound \in \interval{1}{\bound}$,
$\orliterals{\seesgeq{\aterm_1}{\aterm_2}{\asetmeetvar'}{\inbound}}{\lnot\seesgeq{\aterm_1}{\aterm_2}{\asetmeetvar'}{\inbound}} \inside \aformulabis$.
\end{itemize}
\end{itemize}
\end{itemize}
\end{itemize}
Hence, $\aformulabis$ is a type for $\coreseeseq{\asetmeetvar'}{\bound}$.
We now show that $\prove_{\coresys} \aformula \implies \aformulabis$.
For the first set in the conjunction, as in the previous case we have
\begin{nscenter}
$\prove_{\coresys} \aformula \implies \formulasubset{\aterm_1 \sim \aterm_2}{\bmat[\aterm_1,\aterm_2 \in \asetmeetvar',\ \sim \in \{=,\neq\},\ \aterm_1\sim\aterm_2 \inside \aformula]}$
\end{nscenter}
by propositional calculus, as the consequence of this implication is a subformula of $\aformula$.
The second and third sets of the conjunction can be derived instead from the tautologies
\begin{itemize}[align=left]
\item[\ref{core2Ax:SeesMono1}] $\seesgeq{\aterm_1}{\aterm_2}{\asetmeetvar' \cup \{\aterm\}}{\inbound} \implies \seesgeq{\aterm_1}{\aterm_2}{\asetmeetvar'}{\inbound}$;
\item[\ref{core2Ax:SeesMono2}] $\seesgeq{\aterm_1}{\aterm_2}{\asetmeetvar'}{\inbound+1} \implies \seesgeq{\aterm_1}{\aterm_2}{\asetmeetvar'}{\inbound}$;
\item[\ref{axiom2:seeslengthpreserved}]
$
\sees{\aterm_1}{\aterm_2}{\asetmeetvar\cup\{\aterm_3\}}{=}{\inbound} \implies \sees{\aterm_1}{\aterm_2}{\asetmeetvar}{=}{\inbound}
$
\end{itemize}
The fourth set can be derived from the tautologies
\begin{itemize}[align=left]
\item[\ref{axiom2:notseespreservedL}]
$\lnot \sees{\aterm_1}{\aterm_2}{\asetmeetvar\cup\{\aterm\}} \land \lnot \sees{\aterm_1}{\aterm_3}{\asetmeetvar\cup\{\aterm\}}
\implies \lnot\sees{\aterm_1}{\aterm_2}{\asetmeetvar}$
\item[\ref{axiom2:notseespreservedR}]
$\lnot \sees{\aterm_1}{\aterm_2}{\asetmeetvar\cup\{\aterm\}} \land \lnot \sees{\aterm_3}{\aterm_2}{\asetmeetvar\cup\{\aterm\}}
\implies \lnot\sees{\aterm_1}{\aterm_2}{\asetmeetvar}$
\end{itemize}
Lastly, the fifth and sixth sets can be derived from the tautologies
\begin{itemize}[align=left]
\item[\ref{core2Ax:SeesMono1}] $\seesgeq{\aterm_1}{\aterm_2}{\asetmeetvar' \cup \{\aterm\}}{\inbound} \implies \seesgeq{\aterm_1}{\aterm_2}{\asetmeetvar'}{\inbound}$;
\item[\ref{core2Ax:SeesMono2}] $\seesgeq{\aterm_1}{\aterm_2}{\asetmeetvar'}{\inbound+1} \implies \seesgeq{\aterm_1}{\aterm_2}{\asetmeetvar'}{\inbound}$;
\item[\ref{core2Ax:SeesSum}]
$
\begin{aligned}[t]
&\seesgeq{\aterm_1}{\aterm_2}{\asetmeetvar}{\inbound_1}\!\land \seesgeq{\aterm_2}{\aterm_3}{\asetmeetvar}{\inbound_2} \land \aterm_2 {\not\in}\asetmeetvar \land \aterm_3 {\in} \asetmeetvar\\
&\Rightarrow \seesgeq{\aterm_1}{\aterm_3}{\asetmeetvar}{\inbound_1{+}\inbound_2} \land \lnot \sees{\aterm_1}{\aterm_3}{\{\aterm_2\}}
\end{aligned}$
\item[\ref{axiom2:seeslengthsum}]
$
\begin{aligned}[t]
&\sees{\aterm_1}{\aterm_2}{\asetmeetvar}{=}{\inbound_1} \land  \sees{\aterm_2}{\aterm_3}{\asetmeetvar}{=}{\inbound_2}
\land \aterm_2 \not\in\asetmeetvar \land \aterm_3 \in \asetmeetvar\\
&\implies
\sees{\aterm_1}{\aterm_3}{\asetmeetvar}{=}{\inbound_1+\inbound_2} \land
\lnot \sees{\aterm_1}{\aterm_2}{\{\aterm_3\}}
\end{aligned}
$
\end{itemize}
Here, these schemas are instantiated so that $\inbound_1+\inbound_2 \leq \bound$. Notice that this can be done as $\aformula$ is a satisfiable type for $\coreseeseq{\asetmeetvar}{\bound}$ and hence, if for example it holds
\begin{nscenter}
$\seesgeq{\aterm_1}{\aterm_2}{\asetmeetvar}{\inbound_1}\!\land \seesgeq{\aterm_2}{\aterm_3}{\asetmeetvar}{\inbound_2} \inside \aformula$
\end{nscenter}
then by the axiom~\ref{core2Ax:SeesMono2} it also holds
\begin{nscenter}
$\seesgeq{\aterm_1}{\aterm_2}{\asetmeetvar}{\inbound_1'}\!\land \seesgeq{\aterm_2}{\aterm_3}{\asetmeetvar}{\inbound_2'} \inside \aformula,$
\end{nscenter}
for any $\inbound_1' \in \interval{1}{\inbound_1}$ and $\inbound_2' \in \interval{1}{\inbound_2}$. Hence, it is sufficient to use $\inbound_1'$ and $\inbound_2'$ so that $\inbound_1' + \inbound_2' \leq \bound$.
Moreover, if \ref{axiom2:seeslengthsum} can be applied but only for $\inbound_1 + \inbound_2 > \bound$, then 
the axiom~\ref{core2Ax:SeesSum}
should be applied instead (this can always be done as in the axiom~\ref{core2Ax:SeesSum} the antecedent is weaker than the one in \ref{axiom2:seeslengthsum}).
\end{proof}

We denote with $\fullcoreseeseq{\asetvar}{\bound}$ the set $\bigcup_{\asetmeetvar \subseteq \atermset{\asetvar}} \coreseeseq{\asetmeetvar}{\bound}$. It is equivalent to
\begin{nscenter}
$\{ \aterm_1 = \aterm_2, \seesgeq{\aterm_1}{\aterm_2}{\asetmeetvar}{\inbound} \mid \aterm_1,\aterm_2 \in \asetmeetvar, \inbound \in \interval{1}{\bound}, \asetmeetvar \subseteq \atermset{\asetvar} \}$.
\end{nscenter}
Informally, a type for $\fullcoreseeseq{\asetvar}{\bound}$ is almost a core type, the exception being $\mathtt{rem}$ predicates.

\begin{lemma}\label{lemma:completesees}
Let $\asetvar \subseteq_\fin \PVAR$, $\bound \in \Nat^+$.
Let $\asms$ be a symbolic memory state over $\pair{\asetvar}{\bound}$.
There is $\aformula$ type for $\fullcoreseeseq{\asetvar}{\bound}$ s.t.\ $\prove_{\coresys} \charsymbform(\asms) \implies \aformula$, where all derivation steps only have formulae from $\boolcomb{\coreformulae{\asetvar}{\bound}}$.
Moreover, if $\charsymbform(\asms)$ is satisfiable, then $\aformula$ is unique.
\end{lemma}

\begin{proof}
First, suppose
$
\charsymbform(\asms)
$
to be unsatisfiable.
Then
by Lemma~\ref{lemma:axiomstwoRCchars}, there is a proof of $\charsymbform{\asms} \implies \false$ where
all derivation steps only use formulae  from $\boolcomb{\coreformulae{\asetvar}{\bound}}$.
Then, trivially $\prove_{\coresys} \charsymbform(\asms) \implies \aformula$ for every  type $\aformula$
for $\fullcoreseeseq{\asetvar}{\bound}$. Since $\aformula$ only has formulae from $\boolcomb{\coreformulae{\asetvar}{\bound}}$, it is easy to see that, in this case, the proof can be done with only formulae from $\boolcomb{\coreformulae{\asetvar}{\bound}}$.

Suppose now $\asms$ to be a core type over $\pair{\asetvar}{\bound}$ such that $\charsymbform(\asms)$ is satisfiable.
Then, we show that  there is a  type $\aformula$ for $\fullcoreseeseq{\asetvar}{\bound}$ such that
$\prove_{\coresys} \charsymbform(\asms) \implies \aformula$.
The formula $\aformula$ is trivially the only formula in $\fullcoreseeseq{\asetvar}{\bound}$ (up to commutativity and associativity of $\land$) that can be implied by $\charsymbform(\asms)$ (both in the calculus).
Indeed, suppose that there is another type $\aformulabis$ for $\fullcoreseeseq{\asetvar}{\bound}$ such that
$\prove_{\coresys} \charsymbform(\asms) \implies \aformulabis$.
By propositional calculus we then obtain $\prove_{\coresys} \charsymbform(\asms) \implies \aformula \land \aformulabis$.
Since $\charsymbform(\asms)$ is satisfiable, $\aformula \land \aformulabis$ is satisfiable.
Then, by definition of type, $\aformula$ and $\aformulabis$ must be syntactically equivalent up to commutativity and associativity of $\land$.

Let us now show how to deduce $\aformula$ starting from (a satisfiable) $\charsymbform(\asms)$.
Essentially, (dis)equalities are easy to treat and the proof mainly shows how to ``complete the formula'' by adding the missing $\mathtt{sees}$ predicates.
We start by deriving a type $\aformulater$ for $\coreseeseq{\atermset{\asetvar}}{\bound}$ such that $\prove_{\coresys} \charsymbform(\asms) \implies \aformulater$. Indeed, from the definition of characteristic formula and the one of type for $\coreseeseq{\atermset{\asetvar}}{\bound}$, it is easy to see that this can be done just by using the axiom
\begin{itemize}[align=left]
\item[\ref{core2Ax:SeesMono2}] $\seesgeq{\aterm_1}{\aterm_2}{\asetmeetvar}{\inbound{+}2} \Rightarrow\! \seesgeq{\aterm_1}{\aterm_2}{\asetmeetvar}{\inbound{+}1}$
\end{itemize}
Indeed, given two terms $\aterm_1,\aterm_2 \in \atermset{\asetvar}$, by definition $\charsymbform(\asms)$ is such that:
\begin{itemize}
\item $\lnot \sees{\aterm_1}{\aterm_2}{\atermset{\asetvar}} \inside \charsymbform(\asms)$, or
\item $\seesgeq{\aterm_1}{\aterm_2}{\atermset{\asetvar}}{\inbound} \land \seesgeq{\aterm_1}{\aterm_2}{\atermset{\asetvar}}{\inbound{+}1} \inside \charsymbform(\asms)$ for some $\inbound \in \interval{1}{\bound-1}$, or
\item $\seesgeq{\aterm_1}{\aterm_2}{\atermset{\asetvar}}{\bound} \inside \charsymbform(\asms)$.
\end{itemize}
Hence, by using the axiom~\ref{core2Ax:SeesMono2} (and its contrapositive $\lnot \seesgeq{\aterm_1}{\aterm_2}{\asetmeetvar}{\inbound{+}1} \Rightarrow\! \lnot\seesgeq{\aterm_1}{\aterm_2}{\asetmeetvar}{\inbound{+}2}$) we can derive in $\coresys$,
$\charsymbform(\asms) \implies \aformulabis_{\mathtt{sees}}$,
where $\aformulabis_{\mathtt{sees}}$ is a type for
$\{\seesgeq{\aterm_1}{\aterm_2}{\atermset{\asetvar}}{\inbound} \mid \aterm_1,\aterm_2 \in \atermset{\asetvar}, \inbound \in \interval{1}{\bound}\}$.
Let $\aformulabis_{\mathtt{eq}}$ be the (conjunctive) subformula of $\aformulabis$ containing all (dis)equalities in $\aformulabis$.
Then we have $\prove_{\coresys} \aformulabis \implies \aformulabis_{\mathtt{eq}} \land \aformulabis_{\mathtt{sees}}$ and $\aformulabis_{\mathtt{eq}} \land \aformulabis_{\mathtt{sees}}$ is a type for $\coreseeseq{\atermset{\asetvar}}{\bound}$.
We can now iteratively apply Lemma~\ref{lemma:closingsees} as a closure operator that computes from
$\aformulabis_{\mathtt{eq}} \land \aformulabis_{\mathtt{sees}}$ the truth value for every $\mathtt{sees}$ predicate.
In this way, we obtain the formula $\aformula$ of the statement of the lemma, i.e. a type for $\fullcoreseeseq{\asetvar}{\bound}$ such that $\prove_{\coresys} \charsymbform(\asms) \implies \aformula$. Moreover, Lemma~\ref{lemma:closingsees} also allows us to conclude that such a derivation can be done by only using formulae from $\boolcomb{\coreformulae{\asetvar}{\bound}}$.
\end{proof}

\noindent Lemma~\ref{lemma:completesees} allows us to deduce the $\mathtt{sees}$ formulae. The following result does 
the same for $\mathtt{rem}$.

\begin{lemma}\label{lemma:closingrem1}
Let $\asetvar \subseteq_\fin \PVAR$, $\bound \in \Nat^+$.
Let $\asms$ be a symbolic memory state over $\pair{\asetvar}{\bound}$.
Let $\aformula$ be a type for $\fullcoreseeseq{\asetvar}{\bound}$ such that
$\prove_{\coresys} \charsymbform(\asms) \implies \aformula$.
Let $A,B \subseteq \atermset{\asetvar} \times \atermset{\asetvar}$ such that
\begin{enumerate}
\item for every
$\pair{\aterm}{\aterm'} \in A$: if $\sees{\aterm}{\aterm'}{\emptyset} \inside \aformula$, then
there are $n \geq 0$ and
\begin{nscenter} $\pair{\aterm_0'}{\aterm_1'},\pair{\aterm_1'}{\aterm_2'},\dots,\pair{\aterm_{n-1}'}{\aterm_{n}'},\pair{\aterm_{n}'}{\aterm_{n+1}'} \in B$
\end{nscenter}
such that $\aterm = \aterm_0' \land \aterm' = \aterm_{n+1}' \inside \aformula$.
 \item for every $\pair{\aterm_1}{\aterm_2} \in B$:
  \begin{itemize}
    \item $\sees{\aterm_1}{\aterm_2}{\pi_1(A)\cup \pi_2(A) \cup \pi_1(B) \cup \pi_2(B)} \inside \aformula$;
    \item for every $\pair{\aterm_3}{\aterm_4} \in B \setminus \{(\aterm_1,\aterm_2)\}$, $\aterm_1 \neq \aterm_3 \inside \aformula$;
    \item $\exists\pair{\aterm_3}{\aterm_4} \in A$ s.t.\ $\sees{\aterm_3}{\aterm_4}{\emptyset} \inside \aformula$ and ($\aterm_1 = \aterm_3 \inside \aformula$ or $\lnot \sees{\aterm_3}{\aterm_4}{\{\aterm_1\}} \inside \aformula$)
  \end{itemize}
\end{enumerate}
Then $\prove_{\coresys} \charsymbform(\asms) \implies \bigwedge_{\inbound \in \interval{0}{\bound}}( \remgeq{A}{\inbound} \iff \remgeq{B}{\inbound})$, where the proof in $\coresys$ can be done with only derivation steps having formulae from $\boolcomb{\coreformulae{\asetvar}{\bound}}$.
\end{lemma}

\begin{proof}
As we did for Lemma~\ref{lemma:completesees},
let us first suppose
$
\charsymbform(\asms)
$
to be unsatisfiable.
Then
by Lemma~\ref{lemma:axiomstwoRCchars}, there is a proof of $\charsymbform(\asms) \implies \false$ where all derivation steps have premises from $\boolcomb{\coreformulae{\asetvar}{\bound}}$.
Then, trivially $\prove_{\coresys} \charsymbform{\asms} \implies \bigwedge_{\inbound \in \interval{0}{\bound}}( \remgeq{A}{\inbound} \iff \remgeq{B}{\inbound})$
for every $\aformula$ type for $\fullcoreseeseq{\asetvar}{\bound}$. Since $\bigwedge_{\inbound \in \interval{0}{\bound}}( \remgeq{A}{\inbound} \iff \remgeq{B}{\inbound})$ only has formulae from $\boolcomb{\coreformulae{\asetvar}{\bound}}$, it is easy to see that, in this case, the proof can be done with only formulae from $\boolcomb{\coreformulae{\asetvar}{\bound}}$.

Suppose now $\charsymbform(\asms)$ to be satisfiable.
First, notice that by Lemma~\ref{lemma:completesees} the formula $\aformula$ of the statement exists and is unique.
Moreover, from $\prove_{\coresys} \charsymbform(\asms) \implies \aformula$ together with the satisfiability of $\charsymbform(\asms)$ and the soundness of $\coresys$, we conclude that $\aformula$ is satisfiable.
Then, the proof is essentially made of a series of theorems in $\coresys$ of the form $\prove_{\coresys} \aformula \implies \bigwedge_{\inbound \in \interval{0}{\bound}}( \remgeq{C}{\inbound} \iff \remgeq{D}{\inbound})$ in which the set $D$ is essentially defined from $C$. By putting together all the double implications of the form $\remgeq{C}{\inbound} \iff \remgeq{D}{\inbound}$ we then obtain a proof of
$\prove_{\coresys} \aformula \implies \bigwedge_{\inbound \in \interval{0}{\bound}}(\remgeq{A}{\inbound} \iff \remgeq{B}{\inbound})$. By propositional calculus and $\prove_{\coresys} \charsymbform(\asms) \implies \aformula$, this leads to
$\prove_{\coresys} \charsymbform(\asms) \implies \bigwedge_{\inbound \in \interval{0}{\bound}}( \remgeq{A}{\inbound} \iff \remgeq{B}{\inbound})$.
The proof, as it is presented here, can be seen as a strategy of rewriting $\mathtt{rem}$ formulae and it is split into 3 steps.
  We start (1) by treating the pairs $\pair{\aterm}{\aterm'} \in A$ ($A$ as in the statement) such that $\lnot \sees{\aterm}{\aterm'}{\emptyset} \inside \aformula$.
  Then, (2) we consider the pairs $\pair{\aterm}{\aterm'} \in A$ for which, by considering the sequence of terms $\pair{\aterm_0'}{\aterm_1'},\pair{\aterm_1'}{\aterm_2'},\dots,\pair{\aterm_{n-1}'}{\aterm_{n}'},\pair{\aterm_{n}'}{\aterm_{n+1}'} \in B$ in the first condition of the statement of the lemma,
  we syntactically have that $\aterm \neq \aterm_0'$ or $\aterm' \neq \aterm_{n+1}'$.
  From these two steps, we deduce the existence of a set $C$ from which
  \begin{itemize}
    \item $\prove_{\coresys} \aformula \implies \bigwedge_{\inbound \in \interval{0}{\bound}}( \remgeq{A}{\inbound} \iff \remgeq{C}{\inbound})$
    \item for every $\pair{\aterm_1}{\aterm_2} \in C$: $\sees{\aterm_1}{\aterm_2}{\emptyset} \inside \aformula$
    \item for every
    $\pair{\aterm}{\aterm'} \in C$:
    there are $\pair{\aterm_0'}{\aterm_1'},\pair{\aterm_1'}{\aterm_2'},\dots,\pair{\aterm_{n-1}'}{\aterm_{n}'},\pair{\aterm_{n}'}{\aterm_{n+1}'} \in B$
    where $\aterm = \aterm_0'$ and $\aterm' = \aterm_{n+1}'$, syntactically.
  \end{itemize}
  Lastly (3), we deduce $\prove_{\coresys} \aformula \implies \bigwedge_{\inbound \in \interval{0}{\bound}}( \remgeq{C}{\inbound} \iff \remgeq{B}{\inbound})$ by well-founded induction on a particular multiset of the lengths of the sequences
  $\pair{\aterm_0'}{\aterm_1'},\pair{\aterm_1'}{\aterm_2'},\dots,\pair{\aterm_{n-1}'}{\aterm_{n}'},\pair{\aterm_{n}'}{\aterm_{n+1}'}$ in $B$. To start, assume $\aformula$, $A$ and $B$ as in the statement of the lemma.
  \begin{enumerate}
  \item Let $\pair{\aterm}{\aterm'} \in A$ be such that $\lnot \sees{\aterm}{\aterm'}{\emptyset} \inside \aformula$ (recall that $\aformula$ is a type for every $\mathtt{sees}$ and $\mathtt{rem}$ predicates).
  By the axiom~\ref{core2Ax:RemNotSees} instantiated so that $\inbound_2 = 0$, it is easy to see that the following formula is a theorem in $\coresys$:
  \begin{nscenter}
    $\aformula \implies \bigwedge_{\inbound \in \interval{0}{\bound}}(\remgeq{A}{\inbound} \iff \remgeq{A \setminus \{\pair{\aterm}{\aterm'}\}}{\inbound})$.
  \end{nscenter}
  Hence, consider $A'$ to be the subset obtained from $A$ by removing every pair $\pair{\aterm''}{\aterm'''} \in A$ such that $\lnot \sees{\aterm_1}{\aterm_2}{\emptyset} \inside \aformula$.
  Formally, $A' = A \setminus \{\pair{\aterm}{\aterm'} \in A \mid \lnot \sees{\aterm}{\aterm'}{\emptyset} \inside \aformula\}$, which is equivalent to
  $A' = \{\pair{\aterm}{\aterm'} \in A \mid \sees{\aterm}{\aterm'}{\emptyset} \inside \aformula\}$ since by definition of type, $\aformula$ cannot contain both $\lnot \sees{\aterm}{\aterm'}{\emptyset}$ and $\sees{\aterm}{\aterm'}{\emptyset}$.
  By iterative application of the tautology above we conclude that
  \begin{nscenter}
    $\prove_{\coresys} \aformula \implies \bigwedge_{\inbound \in \interval{0}{\bound}}(\remgeq{A}{\inbound} \iff \remgeq{A'}{\inbound})$.
  \end{nscenter}
  \item We now consider $A'$ as defined above. Notice that it is a subset of $A$ and for every pair 
  $\pair{\aterm}{\aterm'} \in A'$ it holds that $\sees{\aterm}{\aterm'}{\emptyset} \inside \aformula$.
  We now consider a pair $\pair{\aterm}{\aterm'} \in A'$
  for which, by considering the sequence of terms $\pair{\aterm_0'}{\aterm_1'},\pair{\aterm_1'}{\aterm_2'},\dots,\pair{\aterm_{n-1}'}{\aterm_{n}'},\pair{\aterm_{n}'}{\aterm_{n+1}'} \in B$ in the first condition of the statement of the lemma,
  we syntactically have that $\aterm \neq \aterm_0'$ or $\aterm' \neq \aterm_{n+1}'$.
  From the statement of the lemma such a sequence always exists for elements in $A'$.
  Again by hypothesis on these sequences, it must hold that
  such that $\aterm = \aterm_0' \land \aterm' = \aterm_{n+1}' \inside \aformula$.
  From this, together with axioms \ref{core2Ax:RemTEq1} and \ref{core2Ax:RemTEq2} it is easy to derive the following theorem of $\coresys$:
  \begin{nscenter}
      $\aformula \implies \bigwedge_{\inbound \in \interval{0}{\bound}}(\remgeq{A'}{\inbound} \iff \remgeq{A' \cup \{\pair{\aterm_0'}{\aterm_{n+1}'}\}}{\inbound})$.
  \end{nscenter}
  Similarly, again from the axioms~\ref{core2Ax:RemTEq1} and~\ref{core2Ax:RemTEq2}, we can start from the set $(A' \setminus \{\pair{\aterm}{\aterm'}\}) \cup \{\pair{\aterm_0'}{\aterm_{n+1}'}\}$ and obtain the $\mathtt{rem}$ predicates for
  $A' \cup \{\pair{\aterm}{\aterm'}\}$, i.e. we can derive the following theorem
  \begin{nscenter}
      $\aformula \implies \bigwedge_{\inbound \in \interval{0}{\bound}}(\remgeq{(A' \setminus \{\pair{\aterm}{\aterm'}\}) \cup \{\pair{\aterm_0'}{\aterm_{n+1}'}\}}{\inbound} \iff \remgeq{A' \cup \{\pair{\aterm_0',\aterm_{n+1}'}\}}{\inbound})$.
  \end{nscenter}
  These two proofs allow then to prove the following theorem of $\coresys$:
  \begin{nscenter}
      $\aformula \implies \bigwedge_{\inbound \in \interval{0}{\bound}}(\remgeq{A'}{\inbound} \iff \remgeq{(A' \setminus \{\pair{\aterm}{\aterm'}\}) \cup \{\pair{\aterm_0'}{\aterm_{n+1}'}\}}{\inbound})$.
  \end{nscenter}
  In a sense, in this step we swapped a pair $\pair{\aterm}{\aterm'}$ for an equivalent pair $\pair{\aterm_0'}{\aterm_{n+1}'}$ which has a syntactical counterpart in $B$.
  By iterative application of the last tautology, we can swap every pair in $A'$ with pairs enjoying this syntactical condition and hence derive a set $C$ such that
  \begin{itemize}
    \item $\prove_{\coresys} \aformula \implies \bigwedge_{\inbound \in \interval{0}{\bound}}( \remgeq{A'}{\inbound} \iff \remgeq{C}{\inbound})$
    \item for every $\pair{\aterm_1}{\aterm_2} \in C$: $\sees{\aterm_1}{\aterm_2}{\emptyset} \inside \aformula$
    \item for every
    $\pair{\aterm}{\aterm'} \in C$:
    there are $\pair{\aterm_0'}{\aterm_1'},\pair{\aterm_1'}{\aterm_2'},\dots,\pair{\aterm_{n-1}'}{\aterm_{n}'},\pair{\aterm_{n}'}{\aterm_{n+1}'} \in B$
    such that $\aterm = \aterm_0'$ and $\aterm' = \aterm_{n+1}'$, syntactically.
  \end{itemize}
  Notice that from the first property of $C$ together with the properties of $A'$ (previous point of the construction), we conclude that
  \begin{nscenter}
    $\prove_{\coresys} \aformula \implies \bigwedge_{\inbound \in \interval{0}{\bound}}( \remgeq{A}{\inbound} \iff \remgeq{C}{\inbound}).$
  \end{nscenter}
  \item We now deduce $\aformula \implies \bigwedge_{\inbound \in \interval{0}{\bound}}( \remgeq{C}{\inbound} \iff \remgeq{B}{\inbound})$ in $\coresys$, which then terminates the proof directly from the last tautology proved in the previous point of the construction.
  Let us first analyse the Condition (2) in the statement of the lemma, i.e. for every $\pair{\aterm_1}{\aterm_2} \in B$:
   \begin{itemize}
     \item $\sees{\aterm_1}{\aterm_2}{\pi_1(A)\cup \pi_2(A) \cup \pi_1(B) \cup \pi_2(B)} \inside \aformula$;
     \item for every $\pair{\aterm_3}{\aterm_4} \in B \setminus \{(\aterm_1,\aterm_2)\}$, $\aterm_1 \neq \aterm_3 \inside \aformula$;
     \item $\exists\pair{\aterm_3}{\aterm_4} \in A$ s.t.\ $\sees{\aterm_3}{\aterm_4}{\emptyset} \inside \aformula$ and ($\aterm_1 = \aterm_3 \inside \aformula$ or $\lnot \sees{\aterm_3}{\aterm_4}{\{\aterm_1\}} \inside \aformula$)
   \end{itemize}
  Informally, the first two points of this condition states that every pair $\pair{\aterm_1}{\aterm_2} \in B$ uniquely represents a non-empty path from the location corresponding to $\aterm_1$ to the location corresponding to $\aterm_2$ and
  \begin{itemize}
   \item every location in this path ($\aterm_1$ and $\aterm_2$ excluded) does not correspond to terms in $A$;
   \item every location in this path ($\aterm_2$ excluded) does not correspond to terms in $B$.
  \end{itemize}
  The third point of the condition instead states that there is a path from a location corresponding to $\aterm_3$ to a location
corresponding to $\aterm_4$ (``for some $\pair{\aterm_3}{\aterm_4} \in A$'') that includes the path described by
$\pair{\aterm_1}{\aterm_2}$.
  Together with the 1st condition in the statement of the lemma, this implies that the pairs in $B$ in a sense represent non-overlapping paths that exactly cover the paths described by terms in $A$. To better understand this concept, let us consider the following picture of a path from $\aterm_1$ to $\aterm_6$ in a memory state.
  \begin{center}
   \scalebox{0.85}{
       \begin{tikzpicture}[baseline]
         \node[dot,label=above:$\aterm_1$] (a) at (0,0) {};
          \node[dot,label=above:$\aterm_2$] (b) [right=of a] {};
            \node[dot,label=above:$\aterm_3$] (c) [right=of b] {};
              \node[dot,label=above:$\aterm_4$] (d) [right=of c] {};
                \node[dot,label=above:$\aterm_5$] (e) [right=of d] {};
                  \node[dot,label=above:$\aterm_6$] (f) [right=of e] {};

         \draw[reach] (a) -- (b);
         \draw[reach] (b) -- (c);
         \draw[reach] (c) -- (d);
         \draw[reach] (d) -- (e);
         \draw[reach] (e) -- (f);

         \node[dot,red,fill=red] (aa) [below = 0.5cm of a] {};
         \node[dot,red,fill=red] (cc) [below = 0.5cm of c] {};

         \node[dot,red,fill=red] (bb) [below = 1cm of b] {};
         \node[dot,red,fill=red] (dd) [below = 1cm of d] {};

        \node[dot,red,fill=red] (ee) [below = 0.5cm of e] {};
        \node[dot,red,fill=red] (ff) [below = 0.5cm of f] {};

        \draw (aa) -- (cc);
              \draw (bb) -- (dd);
                    \draw (ee) -- (ff);
       \end{tikzpicture}
   }
  \end{center}
  In this figure, the segments below the path represent the pairs in $A$. Specifically, $A = \{\pair{\aterm_1}{\aterm_3},\pair{\aterm_2}{\aterm_4},\pair{\aterm_5}{\aterm_6}\}$.
  Notice that we cannot take $B$ to be equal to $A$, as this latter set does not satisfy
  the conditions we are imposing on $B$.
  In particular, $\aterm_2$ is inside the path from $\aterm_1$ to $\aterm_3$, and $\aterm_3$ is inside the path from $\aterm_2$ to $\aterm_4$, which violates the first constraint of Condition (2).
  A suitable $B$ that respects all the conditions for $A$ is $\{\pair{\aterm_1}{\aterm_2},\pair{\aterm_2}{\aterm_3},\pair{\aterm_3,\aterm_4},\pair{\aterm_5}{\aterm_6}\}$, and it is depicted as follows:
  \begin{center}
   \scalebox{0.85}{
       \begin{tikzpicture}[baseline]
         \node[dot,label=above:$\aterm_1$] (a) at (0,0) {};
          \node[dot,label=above:$\aterm_2$] (b) [right=of a] {};
            \node[dot,label=above:$\aterm_3$] (c) [right=of b] {};
              \node[dot,label=above:$\aterm_4$] (d) [right=of c] {};
                \node[dot,label=above:$\aterm_5$] (e) [right=of d] {};
                  \node[dot,label=above:$\aterm_6$] (f) [right=of e] {};

         \draw[reach] (a) -- (b);
         \draw[reach] (b) -- (c);
         \draw[reach] (c) -- (d);
         \draw[reach] (d) -- (e);
         \draw[reach] (e) -- (f);

         \node[dot,red,fill=red] (aa) [below = 0.5cm of a] {};
         \node[dot,red,fill=red] (bb) [below = 0.5cm of b] {};
         \node[dot,red,fill=red] (bb2) [below = 1cm of b] {};
         \node[dot,red,fill=red] (cc2) [below = 1cm of c] {};
         \node[dot,red,fill=red] (cc) [below = 0.5cm of c] {};
         \node[dot,red,fill=red] (dd) [below = 0.5cm of d] {};

        \node[dot,red,fill=red] (ee) [below = 0.5cm of e] {};
        \node[dot,red,fill=red] (ff) [below = 0.5cm of f] {};

          \draw (aa) -- (bb);
          \draw (bb2) -- (cc2);
          \draw (cc) -- (dd);
          \draw (ee) -- (ff);
       \end{tikzpicture}
   }
  \end{center}
  Indeed, $B$ exactly covers the paths in $A$ and only uses non-overlapping paths.
  We can now tackle the proof of
  $\prove_{\coresys} \aformula \implies \bigwedge_{\inbound \in \interval{0}{\bound}}( \remgeq{C}{\inbound} \iff \remgeq{B}{\inbound})$, which mainly revolves around modifying $C$ so that it does not have overlapping paths.

  Formally, we prove that for every $C'$ such that
  \begin{enumerate}
    \item $\prove_{\coresys} \aformula \implies \bigwedge_{\inbound \in \interval{0}{\bound}}( \remgeq{A}{\inbound} \iff \remgeq{C'}{\inbound})$
    \item for every $\pair{\aterm}{\aterm'} \in C'$: $\sees{\aterm}{\aterm'}{\emptyset} \inside \aformula$
    \item for every
    $\pair{\aterm}{\aterm'} \in C$:
    there are $\pair{\aterm_0'}{\aterm_1'},\pair{\aterm_1'}{\aterm_2'},\dots,\pair{\aterm_{n-1}'}{\aterm_{n}'},\pair{\aterm_{n}'}{\aterm_{n+1}'} \in B$
    such that $\aterm = \aterm_0'$ and $\aterm' = \aterm_{n+1}'$, syntactically.
  \end{enumerate}
  We have that $\prove_{\coresys} \aformula \implies \bigwedge_{\inbound \in \interval{0}{\bound}}( \remgeq{C'}{\inbound} \iff \remgeq{B}{\inbound})$.
  This statement indeed implies $\prove_{\coresys} \aformula \implies \bigwedge_{\inbound \in \interval{0}{\bound}}( \remgeq{C}{\inbound} \iff \remgeq{B}{\inbound})$ as $C$ satisfies the conditions (a)--(c).

  The proof is by induction on the well-founded domain of multisets over natural numbers, with the standard multiset ordering $<_{\text{mult}}$.
  We define a ranking function $\amapbis$ that, given $C'$, returns one of these multisets.
  Given $C'$ satisfying (a)--(c), $\amapbis$ is defined as
  \begin{nscenter}
    $\amapbis(C') \egdef \{\!| \#\pair{\aterm}{\aterm'} \mid  \pair{\aterm}{\aterm'} \in C' |\!\}$
  \end{nscenter}
  where $\#\pair{\aterm}{\aterm'} = n$ holds if and only if
  \begin{nscenter}
  \begin{tabular}{l}
  \hspace{-0.5cm} there are $\pair{\aterm_0'}{\aterm_1'},\pair{\aterm_1'}{\aterm_2'},\dots,\pair{\aterm_{n-1}'}{\aterm_{n}'},\pair{\aterm_{n}'}{\aterm_{n+1}'} \in B$
  such that $\aterm = \aterm_0'$ and $\aterm' = \aterm_{n+1}'$, syntactically.
  \end{tabular}
  \end{nscenter}
  The fact that $\amapbis$ is well-defined stems from (c) together with the property that every pair in $B$ is non-overlapping, meaning that the sequence $\pair{\aterm_0'}{\aterm_1'},\pair{\aterm_1'}{\aterm_2'},\dots,\pair{\aterm_{n-1}'}{\aterm_{n}'},\pair{\aterm_{n}'}{\aterm_{n+1}'}$ in $B$ that is associated to
  $\pair{\aterm}{\aterm'} \in C'$ is unique.
  We are now ready to perform the proof.
  \begin{description}
    \item[base case ($\amapbis(C')$ only contains $0$s)] For the base case, we consider any $C'$ such that for every $\pair{\aterm}{\aterm'} \in C'$ $\#\pair{\aterm}{\aterm'} = 0$. Then, from the property (c) of $C'$, it directly holds that $\pair{\aterm}{\aterm'} \in B$. As $B$ is non-overlapping and covers $A$, we directly conclude that $C' = B$ and therefore simply by propositional calculus
    \begin{nscenter}
    $\prove_{\coresys} \aformula \implies \bigwedge_{\inbound \in \interval{0}{\bound}}( \remgeq{C'}{\inbound} \iff \remgeq{B}{\inbound})$.
    \end{nscenter}
    \item[induction case] For the induction case, we suppose that there is $\pair{\aterm}{\aterm'} \in C'$ such that $\#\pair{\aterm}{\aterm'} = n > 0$. Then, again from the property (c) of $C'$, let
    \begin{nscenter}
    $\pair{\aterm_0'}{\aterm_1'},\pair{\aterm_1'}{\aterm_2'},\dots,\pair{\aterm_{n-1}'}{\aterm_{n}'},\pair{\aterm_{n}'}{\aterm_{n+1}'} \in B$
    \end{nscenter}
    such that $\aterm = \aterm_0'$ and $\aterm' = \aterm_{n+1}'$, syntactically.
    We consider $k \in \interval{1}{n}$.
    Condition (b) of $C'$ states that $\sees{\aterm}{\aterm'}{\emptyset} \inside \aformula$.
    Recall that $\aformula$ is satisfiable, since we assumed $\charsymbform(\asms)$ to be satisfiable.
    We can show that
    $\sees{\aterm_0'}{\aterm_i'}{\emptyset} \land \sees{\aterm_i'}{\aterm_{n+1}'}{\emptyset} \land \lnot \sees{\aterm_0'}{\aterm_{n+1}'}{\{\aterm_i'\}} \inside \aformula$.
    Indeed, $\sees{\aterm_0'}{\aterm_i'}{\emptyset}$ and $\sees{\aterm_i'}{\aterm_{n+1}'}{\emptyset}$ must hold from the hypothesis (1) on the pairs of $A$ (statement of the lemma) together with the fact that for every $\pair{\aterm_1}{\aterm_2} \in B$,
    $\sees{\aterm_1}{\aterm_2}{\pi_1(A)\cup \pi_2(A) \cup \pi_1(B) \cup \pi_2(B)} \inside \aformula$ (hypothesis (2) on the pairs of $B$ in the statement of the lemma). This latter property on the pairs of $B$ also proves that $\lnot \sees{\aterm_0'}{\aterm_{n+1}'}{\{\aterm_{i}'\}}$. Hence,
    $\sees{\aterm_0'}{\aterm_i'}{\emptyset} \land \sees{\aterm_i'}{\aterm_{n+1}'}{\emptyset} \land \lnot \sees{\aterm_0'}{\aterm_{n+1}'}{\{\aterm_i'\}} \inside \aformula$ must hold as otherwise $\aformula$ cannot be satisfiable, a contradiction.
    Now, we use the axioms~\ref{core2Ax:RemBetween},~\ref{core2Ax:RemBetweenTwo} and~\ref{core2Ax:RemMono2}, to deduce that
    \begin{nscenter}
      $\prove_{\coresys} \aformula \implies \bigwedge_{\inbound \in \interval{0}{\bound}}( \remgeq{C'}{\inbound} \iff \remgeq{(C' \setminus \{\pair{\aterm}{\aterm'}) \cup
      \{\pair{\aterm_0'}{\aterm_i'},\pair{\aterm_i'}{\aterm_{n+1}'}\}}{\inbound})$.
    \end{nscenter}
    Since $\sees{\aterm}{\aterm'}{\asetmeetvar} \land \lnot \sees{\aterm}{\aterm'}{\{\aterm_i'\}} \inside \aformula$
    (the first conjunct holds by properties of $C'$, the second conjunct holds from $\lnot \sees{\aterm_0'}{\aterm_{n+1}'}{\{\aterm_i'\}} \inside \aformula$ by recalling that $\aterm = \aterm_0'$ and $\aterm' = \aterm_{n+1}'$, syntactically), from the axiom \ref{core2Ax:RemBetweenTwo} we have
    \begin{nscenter}
      $\prove_{\coresys} \aformula \land \remgeq{C'}{\inbound} \implies \remgeq{C' \cup \{\pair{\aterm_0'}{\aterm_i'},\pair{\aterm_i'}{\aterm_{n+1}'}\}}{\inbound}$.
    \end{nscenter}
    Then, by the axiom~\ref{core2Ax:RemMono2} the pair $\pair{\aterm}{\aterm'}$ can be removed from $C' \cup \{\pair{\aterm_0'}{\aterm_i'},\pair{\aterm_i'}{\aterm_{n+1}'}\}$. As this pair is by definition different form
    $\pair{\aterm_0'}{\aterm_i'}$ and $\pair{\aterm_i'}{\aterm_{n+1}'}$, we obtain
    \begin{nscenter}
      $\prove_{\coresys} \aformula \land \remgeq{C' \cup \{\pair{\aterm_0'}{\aterm_i'},\pair{\aterm_i'}{\aterm_{n+1}'}\}}{\inbound} \implies
      \remgeq{(C'\setminus \{\pair{\aterm}{\aterm'}\})\cup \{\pair{\aterm_0'}{\aterm_i'},\pair{\aterm_i'}{\aterm_{n+1}'}\}}{\inbound}$.
    \end{nscenter}
    Lastly, we apply the axiom~\ref{core2Ax:RemBetween} to go 
    from $(C'\setminus \{\pair{\aterm}{\aterm'}\})\cup \{\pair{\aterm_0'}{\aterm_i'},\pair{\aterm_i'}{\aterm_{n+1}'}\}$ back to $C'$:
    \begin{nscenter}
      $\prove_{\coresys} \aformula \land \remgeq{(C'\setminus \{\pair{\aterm}{\aterm'}\})\cup \{\pair{\aterm_0'}{\aterm_i'},\pair{\aterm_i'}{\aterm_{n+1}'}\}}{\inbound} \implies
      \remgeq{C'}{\inbound}$.
    \end{nscenter}
    From these theorems, together with propositional calculus, we are able in $\coresys$ to obtain a derivation for the formula
    \begin{nscenter}
      $\aformula \implies \bigwedge_{\inbound \in \interval{0}{\bound}}( \remgeq{C'}{\inbound} \iff \remgeq{(C' \setminus \{\pair{\aterm}{\aterm'}) \cup
      \{\pair{\aterm_0'}{\aterm_i'},\pair{\aterm_i'}{\aterm_{n+1}'}\}}{\inbound})$.
    \end{nscenter}
    Again, notice that all the derivation steps only use formulae from $\boolcomb{\coreformulae{\asetvar}{\bound}}$.

    Let us now analyse the set $(C' \setminus \{\pair{\aterm}{\aterm'}) \cup
    \{\pair{\aterm_0'}{\aterm_i'},\pair{\aterm_i'}{\aterm_{n+1}'}\}$.
     It is easy to see that this set satisfies the properties (a)--(c).
     Moreover, we have that
     \begin{nscenter}
      $\amapbis((C' \setminus \{\pair{\aterm}{\aterm'}) \cup
     \{\pair{\aterm_0'}{\aterm_i'},\pair{\aterm_i'}{\aterm_{n+1}'}\}) = (\amapbis(C') \setminus \{ \#\pair{\aterm}{\aterm'} \})
     \cup \{ \#\pair{\aterm_0'}{\aterm_i'} \#\pair{\aterm_i'}{\aterm_{n+1}'}\}$.
     \end{nscenter}
     We then conclude that $\amapbis((C' \setminus \{\pair{\aterm}{\aterm'}) \cup
     \{\pair{\aterm_0'}{\aterm_i'},\pair{\aterm_i'}{\aterm_{n+1}'}\}) <_{\text{mult}} \amapbis(C')$,
     as we are removing from the multiset $\#\pair{\aterm}{\aterm'} = n$ in favor of $\#\pair{\aterm_0'}{\aterm_i'}$ and $ \#\pair{\aterm_i'}{\aterm_{n+1}'}$ we are both strictly smaller than $n$.
     Hence, we can apply the inductive hypothesis in order to obtain a proof in $\coresys$ of
     \begin{nscenter}
       $\aformula \implies \bigwedge_{\inbound \in \interval{0}{\bound}}(\remgeq{(C' \setminus \{\pair{\aterm}{\aterm'}) \cup
       \{\pair{\aterm_0'}{\aterm_i'},\pair{\aterm_i'}{\aterm_{n+1}'}\}}{\inbound} \iff \remgeq{B}{\inbound})$.
     \end{nscenter}
     Together with the previous formula we derived, by propositional calculus we conclude that
     \begin{nscenter}
       $\prove_{\coresys} \aformula \implies \bigwedge_{\inbound \in \interval{0}{\bound}}(\remgeq{C'}{\inbound} \iff \remgeq{B}{\inbound})$,
     \end{nscenter}
     which ends the proof. \qedhere
  \end{description}
  \end{enumerate}
\end{proof}

Before dealing with the proof of Lemma~\ref{lemma:coretypecharsms}, let us state a simple result on the existence of the set $B$ appearing in Lemma~\ref{lemma:closingrem1}.

\begin{lemma}\label{lemma:closingremaux}
Let $\asetvar \subseteq_\fin \PVAR$, $\bound \in \Nat^+$.
Let $\aformula$ be a type for $\fullcoreseeseq{\asetvar}{\bound}$
and $A \subseteq \atermset{\asetvar} \times \atermset{\asetvar}$.
There is $B \subseteq \atermset{\asetvar} \times \atermset{\asetvar}$ such that
\begin{enumerate}
\item for every
$\pair{\aterm}{\aterm'} \in A$: if $\sees{\aterm}{\aterm'}{\emptyset} \inside \aformula$, then
there are $n \geq 0$ and
\begin{nscenter} $\pair{\aterm_0'}{\aterm_1'},\pair{\aterm_1'}{\aterm_2'},\dots,\pair{\aterm_{n-1}'}{\aterm_{n}'},\pair{\aterm_{n}'}{\aterm_{n+1}'} \in B$
\end{nscenter}
such that $\aterm = \aterm_0' \land \aterm' = \aterm_{n+1}' \inside \aformula$.
 \item for every $\pair{\aterm_1}{\aterm_2} \in B$:
  \begin{enumerate}
    \item $\sees{\aterm_1}{\aterm_2}{\atermset{\asetvar}} \inside \aformula$;
    \item for every $\pair{\aterm_3}{\aterm_4} \in B \setminus \{(\aterm_1,\aterm_2)\}$, $\aterm_1 \neq \aterm_3 \inside \aformula$;
    \item $\exists\pair{\aterm_3}{\aterm_4} \in A$ such that $\sees{\aterm_3}{\aterm_4}{\emptyset} \inside \aformula$ and ($\aterm_1 = \aterm_3 \inside \aformula$ or $\lnot \sees{\aterm_3}{\aterm_4}{\{\aterm_1\}} \inside \aformula$).
  \end{enumerate}
\end{enumerate}
\end{lemma}

\begin{proof}(sketch)
We show how to deduce $B$ starting from $A$.
First of, we remove from $A$ every pair $\pair{\aterm}{\aterm'}$ such that $\lnot \sees{\aterm}{\aterm'}{\emptyset} \inside \aformula$. Let us denote with $A'$ the set we obtain from this set of the construction.
Notice that for all $\pair{\aterm}{\aterm'} \in A'$, $\sees{\aterm}{\aterm'}{\emptyset} \inside \aformula$.

We want now to prove that for every $C$ such that for all $\pair{\aterm}{\aterm'} \in C$, $\sees{\aterm}{\aterm'}{\emptyset} \inside \aformula$, there is a set $D$ such that
\begin{enumerate}[label=(\Roman*)]
\item for every
$\pair{\aterm}{\aterm'} \in C$
there are $n \geq 0$ and
\begin{nscenter} $\pair{\aterm_0'}{\aterm_1'},\pair{\aterm_1'}{\aterm_2'},\dots,\pair{\aterm_{n-1}'}{\aterm_{n}'},\pair{\aterm_{n}'}{\aterm_{n+1}'} \in D$
\end{nscenter}
such that $\aterm = \aterm_0' \land \aterm' = \aterm_{n+1}' \inside \aformula$.
 \item for every $\pair{\aterm_1}{\aterm_2} \in D$:
  \begin{itemize}
    \item $\sees{\aterm_1}{\aterm_2}{\atermset{\asetvar}} \inside \aformula$;
    \item $\exists\pair{\aterm_3}{\aterm_4} \in C$ such that ($\aterm_1 = \aterm_3 \inside \aformula$ or $\lnot \sees{\aterm_3}{\aterm_4}{\{\aterm_1\}} \inside \aformula$).
  \end{itemize}
\end{enumerate}
Similarly to the previous lemma, the proof is by induction on the well-founded domain of multisets over natural numbers, with the standard multiset ordering $<_{\text{mult}}$.
As usual, we define a ranking function $\amapbis$ that, given a set of pairs of terms, returns one of these multisets.
Given $C \subseteq  \atermset{\asetvar} \times \atermset{\asetvar}$, we define
\begin{nscenter}
  $\amapbis(C) \egdef \{\!| \#\pair{\aterm}{\aterm'} \mid  \pair{\aterm}{\aterm'} \in C |\!\}$,
\end{nscenter}
where $\#\pair{\aterm}{\aterm'} = \card{\atermset{\asetvar} \setminus \asetmeetvar}$ where $\asetmeetvar$ is the maximal subset of $\atermset{\asetvar}$ such that $\sees{\aterm}{\aterm'}{\asetmeetvar} \inside \aformula$.
Notice that this function is well-founded as the maximal sets we require in the definition ($\asetmeetvar$ above) exists directly by 
the axiom~\ref{core2Ax:SeesMax}.
\begin{description}
\item[base case ($\amapbis(C)$ only contains $0$s)] For the base case, we consider any $C$ such that for every $\pair{\aterm}{\aterm'} \in C$ $\#\pair{\aterm}{\aterm'} = 0$. Then, we take $D = C$. All the constraints required on $D$ are trivially satisfied.
\item[induction case] For the induction case, we suppose that there is $\pair{\aterm}{\aterm'} \in C$ such that $\#\pair{\aterm}{\aterm'} = n > 0$. Then, let $\asetmeetvar$ be the maximal subset of $\atermset{\asetvar}$ such that
$\sees{\aterm}{\aterm'}{\asetmeetvar} \inside \aformula$.
By definition of $\#\pair{\aterm}{\aterm'}$, there is $\aterm'' \in \atermset{\asetvar} \setminus \asetmeetvar$ such that
$\lnot\sees{\aterm}{\aterm'}{ \asetmeetvar \cup \{\aterm''\}} \inside \aformula$.
By the axiom~\ref{core2Ax:SeesNegSum}, we conclude that $\sees{\aterm}{\aterm''}{\asetmeetvar \cup \{\aterm''\}} \inside \aformula$ and $\sees{\aterm''}{\aterm'}{\asetmeetvar \cup \{\aterm''\}} \inside \aformula$.
Then, let us consider the set $C' \egdef (C \setminus \pair{\aterm}{\aterm'}) \cup \{ \pair{\aterm}{\aterm''}, \pair{\aterm''}{\aterm'} \}$.
As we have $\#\pair{\aterm}{\aterm'} > \#\pair{\aterm}{\aterm''}$ and $\#\pair{\aterm}{\aterm'} > \#\pair{\aterm''}{\aterm'}$
we conclude that $\amapbis(C') <_{\text{mult}} \amapbis(C)$ and therefore we can apply the induction hypothesis.
We derive $D$ that satisfies the properties (I) and (II) above w.r.t. $C'$.
By definition of $C'$ and $\sees{\aterm}{\aterm''}{\asetmeetvar \cup \{\aterm''\}} \land \sees{\aterm''}{\aterm'}{\asetmeetvar \cup \{\aterm''\}} \inside \aformula$, we can easily show that $D$ also satisfies (I) and (II) w.r.t. $C$.
\end{description}
As $A'$ is such that for all $\pair{\aterm}{\aterm'} \in A'$, $\sees{\aterm}{\aterm'}{\emptyset} \inside \aformula$, from the statement we just proved we conclude that there 
is $D$ that satisfies (I) and (II) w.r.t. $A'$.
In order to conclude the proof, we just need to derive from $D$ a set $B$ that also satisfies the condition 2(b) of the statement. Consider (if they exist) two distinct pairs $\pair{\aterm_1}{\aterm_2},\pair{\aterm_3}{\aterm_4} \in D$
such that $\aterm_1 = \aterm_3 \inside \aformula$. By (II), more precisely from
$\sees{\aterm_1}{\aterm_2}{\pi_1(C)\cup \pi_2(C) \cup \pi_1(D) \cup \pi_2(D)} \inside \aformula$ and $\sees{\aterm_3}{\aterm_4}{\pi_1(C)\cup \pi_2(C) \cup \pi_1(D) \cup \pi_2(D)} \inside \aformula$,
it is easy to see that then also $\aterm_2 = \aterm_4 \inside \aformula$.
Hence, given two pairs $\pair{\aterm_1}{\aterm_2},\pair{\aterm_3}{\aterm_4} \in D$ not satisfying 2(b),
$\aterm_1 = \aterm_3 \land \aterm_2 = \aterm_4 \inside \aformula$.
In order to derive $B$ it is therefore sufficient to iteratively remove one of these two pairs until no more pairs violating 2(b) are found.
By construction, the set $B$ derived in this way satisfies the conditions $1$ and $2$ in the statement of the lemma, w.r.t.\ the set $A'$.
However, as $A'$ is obtained form $A$ by removing the pairs $\pair{\aterm}{\aterm'}$ such that $\lnot \sees{\aterm}{\aterm'}{\emptyset} \inside \aformula$, it is easy to see that $B$  satisfies the conditions $1$ and $2$ also w.r.t.\ the initial set $A$.
\end{proof}

We are now finally ready to tackle the proof of Lemma~\ref{lemma:coretypecharsms}

\lemmacoretypecharsms*

\begin{proof}
First, suppose
$
\charsymbform(\asms)
$
to be unsatisfiable.
Then
by Lemma~\ref{lemma:axiomstwoRCchars}, there is a proof (in $\coresys$) of $\charsymbform{\asms} \implies \false$ where all derivation steps only use formulae from  $\boolcomb{\coreformulae{\asetvar}{\bound}}$.
The characteristic formula can be proved equivalent to any unsatisfiable core type, as for example one containing the literal $\lnot \remgeq{\atermset{\asetvar}\times\atermset{\asetvar}}{0}$.
Indeed, a contradiction of such a core type can be derived directly by the axiom~\ref{core2Ax:RemPos} and propositional calculus, and the derivation trivially uses only formulae from $\boolcomb{\coreformulae{\asetvar}{\bound}}$.
The lemma then holds for unsatisfiable characteristic formulae.

Suppose then $\charsymbform(\asms)$ to be a satisfiable characteristic formula.
By Lemma~\ref{lemma:completesees}, there is a type $\aformula$ for $\fullcoreseeseq{\asetvar}{\bound}$
such that $\prove_{\coresys} \models \charsymbform(\asms) \implies \aformula$.
Moreover, the proof in $\coresys$ of this last theorem can be done by using only derivation steps with formulae from $\boolcomb{\coreformulae{\asetvar}{\bound}}$, and $\aformula$ is the only type for $\fullcoreseeseq{\asetvar}{\bound}$ that is entailed by $\charsymbform(\asms)$.

We are almost done, as $\aformula$ is already a type for all equivalences and $\mathtt{sees}$ predicates, and we just need to derive a type for the $\mathtt{rem}$ predicates.
Recall that, from the definition of $\charsymbform(\asms)$, one of the following holds:
\begin{itemize}
\item $\remgeq{\atermset{\asetvar}\times\atermset{\asetvar}}{\bound} \inside\charsymbform(\asms)$, or
\item $\remgeq{\atermset{\asetvar}\times\atermset{\asetvar}}{\inbound} \land \lnot \remgeq{\atermset{\asetvar}\times\atermset{\asetvar}}{\inbound{+}1} \inside \charsymbform(\asms)$ for some $\inbound \in \interval{0}{\bound-1}$.
\end{itemize}
As a first step then, let us prove that there is a type
$\aformulater_{\atermset{\asetvar} \times \atermset{\asetvar}}$ for $\{ \remgeq{\atermset{\asetvar} \times \atermset{\asetvar}}{\inbound} \mid \inbound \in \interval{0}{\bound}\}$ such that
$\prove_{\coresys} \charsymbform(\asms) \implies \aformulater_{\atermset{\asetvar}}$.
This is easy to show:
\begin{itemize}
\item if $\remgeq{\atermset{\asetvar}\times\atermset{\asetvar}}{\bound} \inside\charsymbform(\asms)$, then by repeated applications of 
the axiom~\ref{core2Ax:RemMono1}, we conclude that
$\prove_{\coresys} \charsymbform(\asms) \implies \remgeq{\atermset{\asetvar}\times\atermset{\asetvar}}{\inbound}$ for every $\inbound \in \interval{0}{\bound}$.
\item if instead there is $\inbound \in \interval{0}{\bound-1}$ such that $\remgeq{\atermset{\asetvar}\times\atermset{\asetvar}}{\inbound} \land \lnot \remgeq{\atermset{\asetvar}\times\atermset{\asetvar}}{\inbound{+}1} \inside \charsymbform(\asms)$, then
again by repeated applications of the axiom~\ref{core2Ax:RemMono1} and of its contrapositive (which is a theorem in $\coresys$ by propositional calculus) $\lnot \remgeq{\asetpath}{\inbound} \implies \lnot \remgeq{\asetpath}{\inbound+1}$, we conclude that
$\prove_{\coresys} \charsymbform(\asms) \implies \remgeq{\atermset{\asetvar}\times\atermset{\asetvar}}{\inbound'}$ for every $\inbound' \in \interval{0}{\inbound}$
and $\prove_{\coresys} \charsymbform(\asms) \implies \lnot\remgeq{\atermset{\asetvar}\times\atermset{\asetvar}}{\inbound'}$ for every $\inbound' \in \interval{\inbound+1}{\bound}$.
\end{itemize}
Hence, by propositional calculus and the axiom~\ref{core2Ax:RemMono1}, $\prove_{\coresys} \charsymbform(\asms) \implies \aformulater_{\atermset{\asetvar} \times \atermset{\asetvar}}$, where
$\aformulater_{\atermset{\asetvar} \times \atermset{\asetvar}}$ is a type for $\{ \remgeq{\atermset{\asetvar} \times \atermset{\asetvar}}{\inbound} \mid \inbound \in \interval{0}{\bound}\}$.
We now generalise this fact and show that, given an arbitrary $\asetpath \subseteq \atermset{\asetvar} \times \atermset{\asetvar}$, there is a type $\aformulater_{\asetpath}$ for $\{ \remgeq{\asetpath}{\inbound} \mid \inbound \in \interval{0}{\bound}\}$ such that
$\prove_{\coresys} \charsymbform(\asms) \implies \aformulater_{\asetpath}$.
Notice that, in order to prove this result, we just need to derive, in $\coresys$ one of the two following formulae (which cannot hold simultaneously)
\begin{enumerate}[label=(\Roman*)]
\item $\charsymbform(\asms) \implies\remgeq{\asetpath}{\bound}$, or
\item $\charsymbform(\asms) \implies \remgeq{\asetpath}{\inbound} \land \lnot \remgeq{\asetpath}{\inbound{+}1}$, for some $\inbound \in \interval{0}{\bound-1}$,
\end{enumerate}
as then we can use the axiom~\ref{core2Ax:RemMono1} as we did just above in order to derive a type for $\{ \remgeq{\asetpath}{\inbound} \mid \inbound \in \interval{0}{\bound}\}$.
Most importantly, by showing that such an $\aformulater_{\asetpath}$ is derivable in the calculus starting from $\charsymbform(\asms)$, we end the proof.
Indeed, together with $\prove_{\coresys} \charsymbform(\asms) \implies \aformula$ (recall that $\aformula$ is a type for $\fullcoreseeseq{\asetvar}{\bound}$) we then obtain that
\begin{nscenter}
  $\prove_{\coresys} \charsymbform(\asms) \implies \aformula \land \bigwedge_{\asetpath \subseteq \atermset{\asetvar} \times \atermset{\asetvar}} \aformulater_{\asetpath}$,
\end{nscenter}
where, by definition, $\aformula \land \bigwedge_{\asetpath \subseteq \atermset{\asetvar} \times \atermset{\asetvar}} \aformulater_{\asetpath}$ is a core type for $\pair{\asetvar}{\bound}$.
Hence, let $\asetpath \subseteq \atermset{\asetvar} \times \atermset{\asetvar}$ and let us show how to derive a formula shaped as  in (I) or (II).
The proof is divided essentially in three steps.
We first (1) derive from $\atermset{\asetvar} \times \atermset{\asetvar}$ a set $B$ enjoying the properties specified in Lemma~\ref{lemma:closingremaux}.
We then (2) do the same for $\asetpath$, obtaining a set $C$. Lastly (3), we derive the formulae (I) or (II) by focusing $B$ and $C$. Everything is done in $\coresys$ and only uses derivation steps having formulae from $\boolcomb{\coreformulae{\asetvar}{\bound}}$.
Let us also assume that $\asetpath$ is different from $\atermset{\asetvar} \times \atermset{\asetvar}$, as the case for $\asetpath = \atermset{\asetvar} \times \atermset{\asetvar}$ has been treated already and leads to the formula $\aformulater_{\atermset{\asetvar} \times \atermset{\asetvar}}$.
\begin{description}
\item[step 1.] W.r.t. the set $\atermset{\asetvar} \times \atermset{\asetvar}$,
by Lemma~\ref{lemma:closingremaux}
there is $B \subseteq \atermset{\asetvar} \times \atermset{\asetvar}$ such that
\begin{enumerate}
\item for every
$\pair{\aterm}{\aterm'} \in \atermset{\asetvar} \times \atermset{\asetvar}$: if $\sees{\aterm}{\aterm'}{\emptyset} \inside \aformula$, then
there are $n \geq 0$ and
\begin{nscenter} $\pair{\aterm_0'}{\aterm_1'},\pair{\aterm_1'}{\aterm_2'},\dots,\pair{\aterm_{n-1}'}{\aterm_{n}'},\pair{\aterm_{n}'}{\aterm_{n+1}'} \in B$
\end{nscenter}
such that $\aterm = \aterm_0' \land \aterm' = \aterm_{n+1}' \inside \aformula$.
 \item for every $\pair{\aterm_1}{\aterm_2} \in B$:
  \begin{enumerate}
    \item $\sees{\aterm_1}{\aterm_2}{\atermset{\asetvar}} \inside \aformula$;
    \item for every $\pair{\aterm_3}{\aterm_4} \in B \setminus \{(\aterm_1,\aterm_2)\}$, $\aterm_1 \neq \aterm_3 \inside \aformula$;
    \item $\exists\pair{\aterm_3}{\aterm_4} \in \atermset{\asetvar} \times \atermset{\asetvar}$ s.t.\ $\sees{\aterm_3}{\aterm_4}{\emptyset} \inside \aformula$ and

    ($\aterm_1 = \aterm_3 \inside \aformula$ or $\lnot \sees{\aterm_3}{\aterm_4}{\{\aterm_1\}} \inside \aformula$).
  \end{enumerate}
\end{enumerate}
By Lemma~\ref{lemma:closingrem1}, we  obtain
$\prove_{\coresys} \charsymbform(\asms) \implies \bigwedge_{\inbound \in \interval{0}{\bound}}( \remgeq{\atermset{\asetvar} \times \atermset{\asetvar}}{\inbound} \iff \remgeq{B}{\inbound})$, where the proof in $\coresys$ can be done with only derivation steps having formulae from $\boolcomb{\coreformulae{\asetvar}{\bound}}$.
Then, from $\prove_{\coresys} \charsymbform(\asms) \implies \aformulater_{\atermset{\asetvar} \times \atermset{\asetvar}}$
we deduce that
\begin{nscenter}
\begin{tabular}{l}
$\prove_{\coresys} \charsymbform(\asms) \implies \bigwedge
\{\remgeq{B}{\inbound} \mid \remgeq{B}{\inbound} \inside \aformulater_{\atermset{\asetvar} \times \atermset{\asetvar}}\}
\land \bigwedge
\{\lnot \remgeq{B}{\inbound} \mid \lnot \remgeq{B}{\inbound} \inside \aformulater_{\atermset{\asetvar} \times \atermset{\asetvar}}\}$.
\end{tabular}
\end{nscenter}
\item[step 2.] Now, we  define a similar set for $\asetpath$.
By Lemma~\ref{lemma:closingremaux}
there is $C \subseteq \atermset{\asetvar} \times \atermset{\asetvar}$ such that
\begin{enumerate}
\item for every
$\pair{\aterm}{\aterm'} \in \asetpath$: if $\sees{\aterm}{\aterm'}{\emptyset} \inside \aformula$, then
there are $n \geq 0$ and
\begin{nscenter} $\pair{\aterm_0'}{\aterm_1'},\pair{\aterm_1'}{\aterm_2'},\dots,\pair{\aterm_{n-1}'}{\aterm_{n}'},\pair{\aterm_{n}'}{\aterm_{n+1}'} \in C$
\end{nscenter}
such that $\aterm = \aterm_0' \land \aterm' = \aterm_{n+1}' \inside \aformula$.
 \item for every $\pair{\aterm_1}{\aterm_2} \in C$:
  \begin{enumerate}
    \item $\sees{\aterm_1}{\aterm_2}{\atermset{\asetvar}} \inside \aformula$;
    \item for every $\pair{\aterm_3}{\aterm_4} \in C \setminus \{(\aterm_1,\aterm_2)\}$, $\aterm_1 \neq \aterm_3 \inside \aformula$;
    \item $\exists\pair{\aterm_3}{\aterm_4} \in \asetpath$ s.t.\ $\sees{\aterm_3}{\aterm_4}{\emptyset} \inside \aformula$ and

    ($\aterm_1 = \aterm_3 \inside \aformula$ or $\lnot \sees{\aterm_3}{\aterm_4}{\{\aterm_1\}} \inside \aformula$)
  \end{enumerate}
\end{enumerate}
By Lemma~\ref{lemma:closingrem1}, we  obtain
$\prove_{\coresys} \charsymbform(\asms) \implies \bigwedge_{\inbound \in \interval{0}{\bound}}( \remgeq{\asetpath}{\inbound} \iff \remgeq{C}{\inbound})$, where the proof in $\coresys$ can be done with only derivation steps having formulae from $\boolcomb{\coreformulae{\asetvar}{\bound}}$.
\item[step 3.]
Let us now consider the sets $B$ and $C$ defined in the previous two steps.
An important property of $B$ is that
for every $\pair{\aterm}{\aterm'} \in C$ there is a pair $\pair{\aterm_0'}{\aterm_1'} \in B$ such that $\aterm = \aterm_0' \land \aterm' = \aterm_1' \inside \aformula$.
This holds since $B$ is derived from $\atermset{\asetvar} \times \atermset{\asetvar}$ whereas $C$ is derived from
$\asetpath \subset \atermset{\asetvar} \times \atermset{\asetvar}$.
Indeed, suppose $\pair{\aterm}{\aterm'} \in C$. Then by property 2(a) on this set,  $\sees{\aterm}{\aterm'}{\atermset{\asetvar}} \inside \aformula$. Moreover, by definition, $\pair{\aterm}{\aterm'}$ also belongs to $\atermset{\asetvar} \times \atermset{\asetvar}$ and hence from the first property of $B$ it holds that
there are $n \geq 0$ and
\begin{nscenter} $\pair{\aterm_0'}{\aterm_1'},\pair{\aterm_1'}{\aterm_2'},\dots,\pair{\aterm_{n-1}'}{\aterm_{n}'},\pair{\aterm_{n}'}{\aterm_{n+1}'} \in B$
\end{nscenter}
such that $\aterm = \aterm_0' \land \aterm' = \aterm_{n+1}' \inside \aformula$.
Suppose that $n$ is at least $1$. Then, from the property 2(a) of $B$ it is easy to see that it must hold that, for every $i \in \interval{1}{n}$, $\lnot \sees{\aterm}{\aterm'}{\{\aterm_i'\}} \inside \aformula$, in contradiction with $\sees{\aterm}{\aterm'}{\atermset{\asetvar}} \inside \aformula$ (by properties of types)
Hence $n = 0$ and therefore there is a pair $\pair{\aterm_0'}{\aterm_1'} \in B$ such that
$\aterm = \aterm_0' \land \aterm' = \aterm_1' \inside \aformula$.

Hence, in order to conclude the proof, it is sufficient to consider the set of pairs in $B$ that are not equivalent to pairs in $C$ and show how the $\mathtt{rem}$ predicate is updated when these pairs are removed from $B$. Recall that we are searching for derivations of the form

\begin{enumerate}[label=(\Roman*)]
\item $\charsymbform(\asms) \implies\remgeq{\asetpath}{\bound}$, or
\item $\charsymbform(\asms) \implies \remgeq{\asetpath}{\inbound} \land \lnot \remgeq{\asetpath}{\inbound{+}1}$, for some $\inbound \in \interval{0}{\bound-1}$,
\end{enumerate}

Formally, we define $\Delta_C(B) \egdef \{\pair{\aterm}{\aterm'} \in B \mid \forall \pair{\aterm_1}{\aterm_2} \in C, \aterm = \aterm_1 \land \aterm' = \aterm_2 \inside \aformula\}$.
We also denote with $\Phi(B)$ the formula
\begin{nscenter}
\begin{tabular}{l}
$\charsymbform(\asms) \implies \bigwedge
\{\remgeq{B}{\inbound} \mid \remgeq{B}{\inbound} \inside \aformulater_{\atermset{\asetvar} \times \atermset{\asetvar}}\}
\land \bigwedge
\{\lnot \remgeq{B}{\inbound} \mid \lnot \remgeq{B}{\inbound} \inside \aformulater_{\atermset{\asetvar} \times \atermset{\asetvar}}\}$,
\end{tabular}
\end{nscenter}
which is shown to be a theorem of $\coresys$ at the end of (step 1).
We perform the following construction.
\begin{description}
\item[C1] If $\card{\Delta_C(B)} = 0$, then every pair of $B$ has an equivalent pair in $C$. Hence, as done in Lemma~\ref{lemma:closingrem1}, 
by the axioms~\ref{core2Ax:RemTEq1},~\ref{core2Ax:RemTEq2} and~\ref{core2Ax:RemMono2}, we derive
\begin{nscenter}
   $\prove_{\coresys} \charsymbform(\asms) \implies \bigwedge_{\inbound \in \interval{0}{\bound}}( \remgeq{B}{\inbound} \iff \remgeq{C}{\inbound})$
\end{nscenter}
Then, from the last part of (step 2) we obtain
\begin{nscenter}
  $\prove_{\coresys} \charsymbform(\asms) \implies \bigwedge_{\inbound \in \interval{0}{\bound}}( \remgeq{B}{\inbound} \iff \remgeq{\asetpath}{\inbound})$,
\end{nscenter}
which concludes the proof directly from $\Phi(B)$, together with propositional calculus.
\item[C2] If instead $\card{\Delta_C(B)} > 1$, we distinguish two cases.

If $\Phi(B)$ entails
$\charsymbform(\asms) \implies \remgeq{B}{\bound}$,
then we can simply
use the axiom~\ref{core2Ax:RemMono2} to remove every pair of $\Delta_C(B)$ and obtain a proof in $\coresys$ of
$\prove_{\coresys} \charsymbform(\asms) \implies \remgeq{B \setminus \Delta_C(B)}{\bound}$.
Then as done for the case $\card{\Delta_C(B)} = 0$, we are able to conclude that
$\prove_{\coresys} \charsymbform(\asms) \implies \remgeq{C}{\bound}$, which leads to
$\prove_{\coresys} \charsymbform(\asms) \implies \remgeq{\asetpath}{\bound}$
directly from the theorem of $\coresys$ shown at the end of (step 2).

Suppose instead that $\Phi(B)$ entails
$\charsymbform(\asms) \implies \remgeq{B}{\inbound} \land \lnot \remgeq{B}{\inbound+1}$
for some $\inbound \in \interval{0}{\bound-1}$.
Let $\pair{\aterm}{\aterm'} \in \Delta_C(B)$.
We first notice that, directly by the properties 2(a) and 2(b) of $B$, $\Phi(B)$ and the axiom\ref{core2Ax:RemShort}, we obtain

\lemmalab{($\star$)}{propB:Geqrem} \qquad
$
\prove_{\coresys}  \charsymbform(\asms)  \implies
\big(\seesgeq{\aterm_1}{\aterm_2}{\emptyset}{\beta_2}
\land \remgeq{B}{\inbound_1}  \implies
    \remgeq{B \setminus \{\pair{\aterm}{\aterm'}\}}{\inbound_1{+}\inbound_2}
    \big).
$

\noindent Similarly, by also using the axiom~\ref{core2Ax:RemNotSees}, we can show that

\lemmalab{($\dagger$)}{propB:EQrem} \qquad
$
\prove_{\coresys}  \charsymbform(\asms)  \implies
\big(\sees{\aterm_1}{\aterm_2}{\emptyset}={\beta_2}
\land \rem{B}={\inbound_1}  \implies
    \rem{B \setminus \{\pair{\aterm}{\aterm'}\}}={\inbound_1{+}\inbound_2}
    \big).
$

\noindent
Laslty, as $\aformula$ is a type for $\fullcoreseeseq{\asetvar}{\bound}$ and $\sees{\aterm}{\aterm'}{\atermset{\asetvar}} \inside \aformula$, one of the following must hold
\begin{enumerate}[label=(\roman*)]
\item $\seesgeq{\aterm}{\aterm'}{\atermset{\asetvar}}{\bound} \inside \aformula$, or
\item $\sees{\aterm}{\aterm'}{\atermset{\asetvar}}=\inbound' \inside \aformula$ for some $\inbound' \in \interval{0}{\bound-1}$.
\end{enumerate}
If (i) holds, then we take $\inbound_1 \leq \inbound$ and $\inbound_2 \leq \inbound'$ such that $\inbound_1 + \inbound_2 = \bound$ and derive in $\coresys$, by \ref{propB:Geqrem} together with $\Phi(B)$, the formula
\begin{nscenter}
$\Phi(B \setminus \{\pair{\aterm}{\aterm'}\}) \egdef \charsymbform(\asms) \implies \remgeq{B \setminus \{\pair{\aterm}{\aterm'}\}}{\bound}$.
\end{nscenter}
This guarantees the proof to be made of derivation steps with only formulae from $\boolcomb{\coreformulae{\asetvar}{\bound}}$.
We can then iterate the (C1)--(C2) construction on $\Delta_C(B \setminus \{\pair{\aterm}{\aterm'}\})$ and $\Phi(B \setminus \{\pair{\aterm}{\aterm'}\})$. In particular, as $\remgeq{B \setminus \{\pair{\aterm}{\aterm'}\}}{\bound}$ is entailed by
$\charsymbform(\asms)$, the construction leads to
$\prove_{\coresys} \charsymbform(\asms) \implies \remgeq{C}{\bound}$, either as $\card{\Delta_C(B \setminus \{\pair{\aterm}{\aterm'}\})} = 0$ or from the first case in step (C2). Then, directly from the theorem of $\coresys$ shown at the end of (step 2), we conclude that
$\prove_{\coresys} \charsymbform(\asms) \implies \remgeq{\asetpath}{\bound}$.

If (ii) holds and $\inbound + \inbound' \geq \bound$, we perform the same construction as in (i), in order to obtain a proof of $\prove_{\coresys} \charsymbform(\asms) \implies \remgeq{\asetpath}{\bound}$ that only uses derivations with formulae from
$\boolcomb{\coreformulae{\asetvar}{\bound}}$.
Lastly, if (ii) holds and $\inbound + \inbound' < \bound$, by \ref{propB:EQrem} together with
$\Phi(B)$ we derive in $\coresys$ the formula
\begin{nscenter}
$\Phi(B \setminus \{\pair{\aterm}{\aterm'}\}) \egdef \charsymbform(\asms) \implies \remgeq{B \setminus \{\pair{\aterm}{\aterm'}\}}{\inbound+\inbound'}$.
\end{nscenter}
We can then iterate the (C1)--(C2) construction on $\Delta_C(B \setminus \{\pair{\aterm}{\aterm'}\})$ and $\Phi(B \setminus \{\pair{\aterm}{\aterm'}\})$. As $\card{\Delta_C(B \setminus \{\pair{\aterm}{\aterm'}\})} < \card{\Delta_C(B)}$ this construction is guaranteed to terminate.
We then obtain that exactly one of the following holds:
\begin{enumerate}
\item $\prove_{\coresys} \charsymbform(\asms) \implies\remgeq{C}{\bound}$, or
\item $\prove_{\coresys} \charsymbform(\asms) \implies \remgeq{C}{\inbound} \land \lnot \remgeq{C}{\inbound{+}1}$, for some $\inbound \in \interval{0}{\bound-1}$.
\end{enumerate}
Then, directly from the theorem of $\coresys$ shown at the end of (step 2), we conclude that (I) or (II) are provable in $\coresys$. 
Moreover, as we used only formulae from  $\boolcomb{\coreformulae{\asetvar}{\bound}}$, the lemma is proved. \qedhere
\end{description}
\end{description}
\end{proof}

\begin{lemma}\label{lemma:charsubsettype}
Let $\aformula \in \coretype{\asetvar}{\bound}$ satisfiable and let $\asms$ be a symbolic memory state over $\pair{\asetvar}{\bound}$.
$\models \aformula \iff \charsymbform(\asms)$ if and only if $\charsymbform(\asms) \inside \aformula$. Moreover, $\prove_{\coresys} \aformula \iff \charsymbform(\asms)$ where all derivation steps only have formulae from $\boolcomb{\coreformulae{\asetvar}{\bound}}$.
\end{lemma}
\begin{proof}
Recall that, since $\aformula \in \coretype{\asetvar}{\bound}$ is a core type, by definition $\literals{\aformula}$ includes 
every core formula of $\coreformulae{\asetvar}{\bound}$.
Then, as $\charsymbform(\asms) \in \conjcomb{\coreformulae{\asetvar}{\bound}}$, by propositional reasoning we trivially conclude that
$\models \aformula \implies \charsymbform(\asms)$ if and only if $\charsymbform(\asms) \inside \aformula$.

It is then sufficient to prove that
$\charsymbform(\asms) \inside \aformula$ implies
$\models \charsymbform(\asms) \implies \aformula$.
As $\aformula$ is satisfiable and $\charsymbform(\asms) \inside \aformula$, we then conclude that $\charsymbform(\asms)$ is satisfiable.
Hence, by Lemma~\ref{lemma:coretypecharsms} where is a unique core type $\aformulabis \in \coretype{\asetvar}{\bound}$
equivalent to $\charsymbform(\asms)$.
From
``$\models \aformula \implies \charsymbform(\asms)$ if and only if $\charsymbform(\asms) \inside \aformula$'',
we then conclude that $\models \aformula \implies \aformulabis$. By propositional reasoning, $\models \aformula \implies \aformula \land \aformulabis$. However, by definition of core types, $\aformula \land \aformulabis$ is satisfiable if and only if $\aformula$ and $\aformulabis$ are equivalent up to commutativity and associativity of $\land$.
As $\aformula$ is satisfiable and $\models \aformula \implies \aformula \land \aformulabis$, we obtain that $\aformulabis$ is equivalent to $\aformula$ and hence $\models \charsymbform(\asms)  \implies \aformula$.
Provability in $\coresys$ stems directly from Lemma~\ref{lemma:coretypecharsms} and the fact that the set of symbolic memory states over $\pair{\asetvar}{\bound}$ is finite.
\end{proof}

\begin{lemma}\label{corr:typeuniquesymb}
Let $\aformula \in \coretype{\asetvar}{\bound}$ satisfiable. Then there exists exactly one symbolic memory state $\asms$ over $\pair{\asetvar}{\bound}$ such that $\models \aformula \iff \charsymbform(\asms)$.
Moreover, $\prove_{\coresys} \aformula \iff \charsymbform(\asms)$ where all derivation steps only have formulae from $\boolcomb{\coreformulae{\asetvar}{\bound}}$.
\end{lemma}

\begin{proof}
As $\aformula$ is satisfiable, suppose $\pair{\astore}{\aheap}$ is a memory state such that $\pair{\astore}{\aheap} \models \aformula$.
As $\aformula \in \coretype{\asetvar}{\bound}$  and $\charsymbform(\symbms{\astore}{\aheap}{\asetvar}{\bound}) \in \conjcomb{\coreformulae{\asetvar}{\bound}}$, it holds that $\charsymbform(\symbms{\astore}{\aheap}{\asetvar}{\bound}) \inside \aformula$.
The result then follows directly by Lemma~\ref{lemma:charsubsettype}.
\end{proof}
