# Supplementary material for: A Complete Axiomatisation for Quantifier-Free Separation Logic
Source: arXiv:2006.05156 source file (2021-08-09)
Supplement: Supplementary file 16 [file proof-lemmaintcoreexpress.tex]

In this section, we explain how to encode the core formulae within \intervalSL, so that
such core formulae can be also understood as mere abbreviations.
We start by proving an auxiliary lemma that will later be useful in order to prove this result.
\begin{lemma}\label{lemma:meetinsideminpath}
Let $\pair{\astore}{\aheap}$ a memory state and $\avariable,\avariablebis,\avariableter \in \PVAR$. If $\semantics{\ameetvar{\avariable}{\avariablebis}{\avariableter}}_{\astore,\aheap}$ is defined then $\semantics{\ameetvar{\avariable}{\avariablebis}{\avariableter}}_{\astore,\aheap} \in
\minpath{\astore(\avariable)}{\astore(\avariableter)}{\aheap}\cup\{\astore(\avariableter)\}$.
\end{lemma}
\begin{proof}
Suppose $\semantics{\ameetvar{\avariable}{\avariablebis}{\avariableter}}_{\astore,\aheap}$ defined and equal to $\alocation$. Then by definition
$\alocation$ is such that
there are $\alength_1,\alength_2 \geq 0$ s.t.
\begin{itemize}
\item $\aheap^{\alength_1}(\astore(\avariable)) = \aheap^{\alength_2}(\astore(\avariablebis)) = \alocation$,
\item for every $\alength_1' \in \interval{0}{\alength_1-1}$ and $\alength_2' \geq 0$,
$\aheap^{\alength_1'}(\astore(\avariable)) \neq \aheap^{\alength_2'}(\astore(\avariablebis))$,
\item there is $\alength \geq 0$ such that  $\aheap^\alength(\alocation) = \astore(\avariableter)$.
\end{itemize}
Trivially by definition, every $\alocation'$ that is reachable from $\astore(\avariable)$ but not in $\minpath{\astore(\avariable)}{\astore(\avariableter)}{\aheap}\cup\{\astore(\avariableter)\}$
is such that the length of the minimal path from $\astore(\avariable)$ to $\alocation'$ is greater than the length of the minimal path from $\astore(\avariable)$ to $\alocation''$, for every $\alocation'' \in \minpath{\astore(\avariable)}{\astore(\avariableter)}{\aheap}\cup\{\astore(\avariableter)\}$.
Suppose by absurd that
$\semantics{\ameetvar{\avariable}{\avariablebis}{\avariableter}}_{\astore,\aheap} \not\in
\minpath{\astore(\avariable)}{\astore(\avariableter)}{\aheap}\cup\{\astore(\avariableter)\}$.
Then, as $\alocation$ reaches $\astore(\avariableter)$ (third condition in the definition of meet-points) and the same holds true for $\astore(\avariable)$ and $\astore(\avariablebis)$ (first condition in the definition of meet-points, plus transitivity of the reachability relation),
from the statement above we conclude that there is $\alength_1' \in \interval{0}{\alength_1-1}$ and $\alength_2' \geq 0$,
$\aheap^{\alength_1'}(\astore(\avariable)) = \aheap^{\alength_2'}(\astore(\avariablebis))$: a contradiction.
Hence, $\semantics{\ameetvar{\avariable}{\avariablebis}{\avariableter}}_{\astore,\aheap} \in
\minpath{\astore(\avariable)}{\astore(\avariableter)}{\aheap}\cup\{\astore(\avariableter)\}$.
\end{proof}

%% SD 27/06/19 -- Now earlier in the appendix B
%%
\cut{
First, we need to introduce preliminary definitions. Given an arbitrary object $\mathtt{O}$ (for instance, this can be a term
in $\atermset{\PVAR}$, a set of terms --or of pairs of terms--), we write $\chars{\mathtt{O}}$ to denote the set of program
variables occurring in $\mathtt{O}$. For instance, by definition,
$\chars{\ameetvar{\avariable}{\avariablebis}{\avariableter}} = \{\avariable,\avariablebis,\avariableter\}$.
By contrast, we write $\vars{\mathtt{O}}$ to denote the subset of $\chars{\mathtt{O}}$ made of the program variables
occurring in $\mathtt{O}$ truncated by all the meet-point terms. For instance, by definition,
$\vars{\set{\avariableter, \ameetvar{\avariable}{\avariablebis}{\avariableter}}} = \set{\avariableter}$.
Similarly, we write $\meets{\mathtt{O}}$ to denote the set of meet-point terms  occurring in $\mathtt{O}$.
For example, by definition, $\meets{\set{\avariableter, \ameetvar{\avariable}{\avariablebis}{\avariableter}}} =
\set{\ameetvar{\avariable}{\avariablebis}{\avariableter}}$.
}

Below, we provide the definitions for the different core formulae.
For each core formula $\aformulabis$, we define its extension $\extension{\aformulabis}$ in \intervalSL
that is logically equivalent. The notation $\extension{\aformulabis}$ is used for formal statements but by slight abuse,
we avoid it when there is no confusion.
As a rule of thumb, when core formulae
are used to define other core formulae, their expansion in \intervalSL has been defined above. For example,
equalities are defined firstly when at least one variable is involved and then we consider equalities
when two meet-point terms are involved.
A similar principle applies for other core formulae, and moreover, for the core formulae involving a finite set
of terms, our definitions are done inductively involving strictly smaller subsets. Let us start by the equalities.

\begin{itemize}
\itemsep 0 cm
\item $\avariable = \avariablebis$ belongs to \intervalSL whereas $\avariable = \ameetvar{\avariablebis}{\avariableter}{\avariablefour}$ and $\ameetvar{\avariablebis}{\avariableter}{\avariablefour} = \avariable$ are both equal to
\begin{nscenter}
$
\reach(\avariable,\avariablefour) \land
(\reach(\avariablebis,\avariable)\separate \reach(\avariableter,\avariable)) \land
(\reachplus(\avariable,\avariable) \implies (\reach(\avariablebis,\avariable) \separate \reachplus(\avariable,\avariable))).
$
\end{nscenter}
\item $\ameetvar{\avariable}{\avariablebis}{\avariableter} {=} \ameetvar{\avariablefour}{\avariablefifth}{\avariablesix}$
$\equivbydef$
$
\inpath{\avariable}{\avariableter}{\avariableoct} (\ameetvar{\avariable}{\avariablebis}{\avariableter} = \avariableoct \land \avariableoct = \ameetvar{\avariablefour}{\avariablefifth}{\avariablesix})$,
where $\avariableoct \not \in \set{\avariable,\avariablebis,\avariableter,\avariablefour,\avariablefifth,\avariablesix}$.
\end{itemize}

Now, let us define the core formulae with the predicate $\mathtt{sees}$ but only those involving as main arguments
program variables only. We use $\strict{\aformula}$ as a shortcut for $\aformula \land \lnot (\lnot\emp \separate \aformula)$.

\begin{itemize}
\item $\seesgeq{\avariable}{\avariablebis}{\emptyset}{\inbound}$ is equal to
$(\strict{\reachplus(\avariable,\avariablebis)} \land \sizegeq{\inbound}) \separate \true$.
\item $\seesgeq{\avariable}{\avariablebis}{\asetmeetvar \cup \{\avariableter\}}{\inbound}$ is equal to:
\begin{nscenter}
 $\seesgeq{\avariable}{\avariablebis}{\asetmeetvar}{\inbound} \land
\big(\avariableter = \avariable \lor \avariableter = \avariablebis \lor (\true \separate (\reachplus(\avariable,\avariablebis) \land \lnot \reachplus(\avariable,\avariableter)))\big).
$
\end{nscenter}
\item $\seesgeq{\avariable}{\avariablebis}{\asetmeetvar \cup \{\ameetvar{\avariableter}{\avariablefour}{\avariablefifth}\}}{\inbound}$
is equal to
\begin{nscenter}
$\seesgeq{\avariable}{\avariablebis}{\asetmeetvar}{\inbound} \land
 ( \ameetvar{\avariableter}{\avariablefour}{\avariablefifth} = \avariable \lor \ameetvar{\avariableter}{\avariablefour}{\avariablefifth} = \avariablebis \lor
  \lnot \inpath{\avariable}{\avariablebis}{\avariablesept} \ameetvar{\avariableter}{\avariablefour}{\avariablefifth} = \avariablesept
  )$
\end{nscenter}
  where $\avariablesept$ is a program variable that does not appear in $\set{\avariable,\avariablebis,\avariableter,\avariablefour,\avariablefifth} \cup\chars{\asetmeetvar}$.
\end{itemize}
Now, let us define the core formulae with the predicate $\mathtt{sees}$ involving at least one meet-point term.
They can be reduced easily to the previous ones by using the $\weirdexists$ quantifier.
\begin{itemize}
\item $\seesgeq{\avariable}{\ameetvar{\avariablebis}{\avariableter}{\avariablefour}}{\asetmeetvar}{\inbound}$ is equal to
\begin{nscenter}
$(
\avariablebis = \ameetvar{\avariablebis}{\avariableter}{\avariablefour} \land \seesgeq{\avariable}{\avariablebis}{\asetmeetvar}{\inbound}) \lor
 \inpath{\avariablebis}{\avariablefour}{\avariablesept} (\avariablesept = \ameetvar{\avariablebis}{\avariableter}{\avariablefour} \land \seesgeq{\avariable}{\avariablesept}{\asetmeetvar}{\inbound}),
$
\end{nscenter}
where $\avariablesept$ is a program variable that is not in $\set{\avariable,\avariablebis,\avariableter,\avariablefour} \cup \chars{\asetmeetvar}$.
It is worth noting that the atomic predicates involved in these expansions only
contains program variables.
\item Similarly, the formula $\seesgeq{\ameetvar{\avariablebis}{\avariableter}{\avariablefour}}{\avariable}{\asetmeetvar}{\inbound}$ is equal to
\begin{nscenter}
$(
\avariablebis = \ameetvar{\avariablebis}{\avariableter}{\avariablefour} \land \seesgeq{\avariablebis}{\avariable}{\asetmeetvar}{\inbound}) \lor \inpath{\avariablebis}{\avariablefour}{\avariablesept} (\avariablesept = \ameetvar{\avariablebis}{\avariableter}{\avariablefour} \land \seesgeq{\avariablesept}{\avariable}{\asetmeetvar}{\inbound})$,
\end{nscenter}
where $\avariablesept$ is a program variable that does not appear in $\set{\avariable,\avariablebis,\avariableter,\avariablefour} \cup \chars{\asetmeetvar}$.
\item Lastly, $\seesgeq{\ameetvar{\avariable}{\avariablebis}{\avariableter}}{\ameetvar{\avariablefour}{\avariablefifth}{\avariablesix}}{\asetmeetvar}{\inbound}$ is equal to
\begin{nscenter}
$
(\avariable = \ameetvar{\avariable}{\avariablebis}{\avariableter} \land \seesgeq{\avariable}{\ameetvar{\avariablefour}{\avariablefifth}{\avariablesix}}{\asetmeetvar}{\inbound}) \lor
\inpath{\avariable}{\avariableter}{\avariablesept} (\avariablesept = \ameetvar{\avariable}{\avariablebis}{\avariableter} \land
\seesgeq{\avariablesept}{\ameetvar{\avariablefour}{\avariablefifth}{\avariablesix}}{\asetmeetvar}{\inbound}),
$
\end{nscenter}
where $\avariablesept$ is a program variable that does not appear in $\set{\avariable,\avariablebis,\avariableter,\avariablefour,\avariablefifth,\avariablesix} \cup \chars{\asetmeetvar}$.
\end{itemize}
In order to define $\remgeq{\asetpath}{\inbound}$, we need first to identify the
pairs $\pair{\aterm_1}{\aterm_2} \in \asetpath$ such that $\sees{\aterm_1}{\aterm_2}{\emptyset}$ holds.
So, the first idea to express $\remgeq{\asetpath}{\inbound}$ is to identify the maximal subset $\asetpath' \subseteq \asetpath$
such that all the pairs $\pair{\aterm_1}{\aterm_2}$ in $\asetpath'$ satisfies $\sees{\aterm_1}{\aterm_2}{\emptyset}$
and to state that the heap truncated from the paths enforcing $\sees{\aterm_1}{\aterm_2}{\emptyset}$ has at least
$\inbound$ memory cells. This would work if all the terms were variables but with meet-point terms, taking a subheap may change
the existence of a location interpreting a meet-point term.
That is why, when a meet-point term $\ameetvar{\avariable}{\avariablebis}{\avariableter}$ is present in
$\asetpath'$, we first check whether it is equal to $\avariable$ or to $\avariableter$. If it is not the case,
that is $\reachplus(\avariable,\avariableter)$ holds, then we can use a guarded first-order quantification
of the form $\inpath{\avariable}{\avariableter}{\avariablesept}$ to capture the value
$\ameetvar{\avariable}{\avariablebis}{\avariableter}$ in the current heap, and then this value can be referred to
in any subheap thanks to the variable $\avariablesept$. Hence, in the definition of the extension of core formula
 $\remgeq{\asetpath}{\inbound}$ below, we perform a disjunction on the potential subsets
$\asetpath' \subseteq \asetpath$ and on whether if $\ameetvar{\avariable}{\avariablebis}{\avariableter}
\in \meets{\asetpath'}$, then $\avariable = \avariableter$ or not.
The formula $\remgeq{\asetpath}{\inbound}$ is equal to
\begin{nscenter}
$
\begin{aligned}[t]
\bigvee_{\mathclap{\substack{\asetpath' \subseteq \asetpath\\
  \meets{\asetpath'} = \{\ameetvar{\avariable_i}{\avariablebis_i}{\avariableter_i} \mid i \in \interval{1}{n}\}\\
  K \subseteq \interval{1}{n}
  }}}
  \Big(
  {\textstyle\bigwedge_{\pair{\aterm_1}{\aterm_2} \in \asetpath'}} \sees{\aterm_1}{\aterm_2}{\emptyset} \land
    \bigwedge_{\mathclap{\pair{\aterm_1}{\aterm_2} \in \asetpath \setminus \asetpath'}} \lnot \sees{\aterm_1}{\aterm_2}{\emptyset}
     \land
     \bigwedge_{\mathclap{i \in K}} \avariable_i \neq \avariableter_i
     \land
     \bigwedge_{\mathclap{i \in \interval{1}{n}\setminus K}} \avariable_i = \avariableter_i
     \land
     \\
\inpathindex{\avariable_i}{\avariableter_i}{\avariablesept_i}{i \in K}
        \big(\bigwedge_{\mathclap{i \in K}}
          \avariablesept_i = \ameetvar{\avariable_i}{\avariablebis_i}{\avariableter_i}
          \land
(\strict{
            \bigwedge_{
            \mathclap{\substack{
            \asetpath'' = \asetpath'[\ameetvar{\avariable_i}{\avariablebis_i}{\avariableter_i} \gets \avariablesept_i \mid i \in K][\ameetvar{\avariable_i}{\avariablebis_i}{\avariableter_i} \gets \avariable_i \mid i \in \interval{1}{n}\setminus K]\\
            \pair{\avariable}{\avariablebis} \in \asetpath''
            }}} \sees{\avariable}{\avariablebis}{\emptyset}
          } \separate \size \geq \inbound)
        \big)
     \Big),
\end{aligned}$
\end{nscenter}
where $\inpathindex{\avariable_i}{\avariableter_i}{\avariablesept_i}{i \in K}$ is a shortcut for a sequence of
$\card{K}$ applications of $\inpath{\avariable_i}{\avariableter_i}{\avariablesept_i}$ and every $\avariablesept_i$ are program variables not appearing in $\asetpath$.

Let us introduce one more definition.
Given a memory state $\pair{\astore}{\aheap}$, a finite set of terms $\asetmeetvar \subseteq_{\fin} \atermset{\PVAR}$,
we write $\pathset{\alocation}{\astore,\aheap}{\asetmeetvar}$ to denote
the set of locations reachable from $\alocation$ without going through locations
(different from $\alocation$) corresponding to terms in $\asetmeetvar$.
Formally:
\begin{itemize}
\itemsep 0 cm
\item
$\pathset{\alocation}{\astore,\aheap}{\asetmeetvar} \egdef \{ \alocation' \in \domain{\aheap} \mid \exists \alength \geq 0\ \aheap^\alength(\alocation) = \alocation' \text{ and } \aheap^{\alength'}(\alocation)
\not\in\semantics{\asetmeetvar}_{\astore,\aheap} \text{ for every } 0 < \alength' \leq \alength \}$
where $\semantics{\asetmeetvar}_{\astore,\aheap}$ is equal to
$\set{\semantics{\aterm}_{\astore,\aheap} \mid \aterm \in \asetmeetvar}$.
\end{itemize}
One can show that $\pair{\astore}{\aheap} \models \seesgeq{\aterm_1}{\aterm_2}{\asetmeetvar}{\inbound}$ iff  the conditions
below hold:
\begin{enumerate}
\item $\card{\minpath{\semantics{\aterm_1}_{\astore,\aheap}}{\semantics{\aterm_2}_{\astore,\aheap}}{\aheap}} \geq \inbound$
      (existence of a path of length at least $\inbound$),
\item $\minpath{\semantics{\aterm_1}_{\aheap}}{\semantics{\aterm_2}_{\astore,\aheap}}{\aheap} \subseteq
      \pathset{\semantics{\aterm_1}_{\astore,\aheap}}{\astore,\aheap}{\asetmeetvar}$ (no location corresponding to the interpretation
      of a term in $\asetmeetvar$ is on the path from $\semantics{\aterm_1}_{\astore,\aheap}$ to $\semantics{\aterm_2}_{\astore,\aheap}$).
\end{enumerate}

\lemmaintcoreexpress*

\begin{proof}
More specifically, from the definition above, we need to prove that every core formula $\aformulabis$ is equivalent to its extension $\extension{\aformulabis}$.
In the proof, we select several core formulae for which we show that they are equivalent to their extensions
in \intervalSL.

($\star$) First, let us show that $\avariable = \ameetvar{\avariablebis}{\avariableter}{\avariablefour}$ is logically equivalent
to the formula
$$
\reach(\avariable,\avariablefour) \land
(\reach(\avariablebis,\avariable)\separate \reach(\avariableter,\avariable)) \land
(\reachplus(\avariable,\avariable) \implies (\reach(\avariablebis,\avariable) \separate \reachplus(\avariable,\avariable))).
$$
Let us assume that $\pair{\astore}{\aheap} \models
\avariable = \ameetvar{\avariablebis}{\avariableter}{\avariablefour}$. This implies that
$\semantics{\ameetvar{\avariablebis}{\avariableter}{\avariablefour}}_{\astore,\aheap}$ is defined and equal to $\astore(\avariable)$.
By definition of $\semantics{\ameetvar{\avariablebis}{\avariableter}{\avariablefour}}_{\astore,\aheap}$ it therefore holds that there is $\alength\geq0$ such that $\aheap^\alength(\astore(\avariable)) = \astore{\avariablefour}$. Hence, $\pair{\astore}{\aheap} \models \reach(\avariable,\avariablefour)$.
Similarly, from the definition of $\semantics{\ameetvar{\avariablebis}{\avariableter}{\avariablefour}}_{\astore,\aheap}$, it also holds that
$\pair{\astore}{\aheap} \models \reach(\avariablebis,\avariable)$ and $\pair{\astore}{\aheap} \models \reach(\avariableter,\avariable)$.
Moreover, it is easy to see from its definition that the reachability predicate $\reach$ is transitive, i.e.\ $\reach(\aterm_1,\aterm_2) \land \reach(\aterm_2,\aterm_3) \implies \reach(\aterm_1,\aterm_3)$ is a tautology.
Therefore we also have $\pair{\astore}{\aheap} \models \reach(\avariablebis,\avariablefour) \land \reach(\avariableter,\avariablefour)$, fact that is again also deducible from the definition of $\semantics{\ameetvar{\avariablebis}{\avariableter}{\avariablefour}}_{\astore,\aheap}$.
We reproduce below the three possible situations for satisfying
$\avariable = \ameetvar{\avariablebis}{\avariableter}{\avariablefour}$.
\begin{center}
 \scalebox{0.85}{
     \begin{tikzpicture}[baseline]
       \node[dot,label=above:$\avariablebis$] (i) at (0,0) {};
       \node[dot,label=left:{$\avariable$, $\ameetvar{\avariablebis}{\avariableter}{\avariablefour}$}] (m) [below right = 1.5cm and 0.5cm of i] {};
       \node[dot,label=above:$\avariableter$] (j) [above right=1.5cm and 0.5cm of m] {};
       \node[dot,label=below:{$\avariablefour$\\$\avariablefour$ not inside a loop}] (k) [below of=m] {};

       \draw[reach] (i) -- (m);
       \draw[reach] (j) -- (m);
       \draw[reach] (m) -- (k);
     \end{tikzpicture}
     \quad
     \begin{tikzpicture}[baseline]
       \node[dot,label=above:$\avariablebis$] (i) at (0,0) {};
       \node[dot,label=left:{$\avariable$, $\ameetvar{\avariablebis}{\avariableter}{\avariablefour}$}] (m) [below right = 1.5cm and 0.5cm of i] {};
       \node[dot,label=above:$\avariableter$] (j) [above right=1.5cm and 0.5cm of m] {};
       \node[dot] (mid) [below=0.8cm of m] {};
       \node[dot,label=below:{$\avariablefour$}] (k) [below=1.65cm of m] {};

       \draw[reach] (i) -- (m);
       \draw[reach] (j) -- (m);
       \draw[reach] (m) -- (mid);
       \draw[reach] (mid) to [out=-35,in=35] (k);
       \draw[pto] (k) to [out=155,in=-155] node [left] {$+$} (mid);
     \end{tikzpicture}
     \qquad
     \begin{tikzpicture}[baseline]
       \node[dot,label=above:$\avariablebis$] (i) at (0,0) {};
       \node[dot,label=left:{$\avariable$,$\ameetvar{\avariablebis}{\avariableter}{\avariablefour}$}]
       (m1) [below right = 1.5cm and 0.4cm of i] {};
       \node[dot,label=right:{}] (m2) [below right = 1.7cm and 0.4cm of m1] {};
       \node[dot,label=above:$\avariableter$] (j) [above right=1.5cm and 0.5cm of m2] {};
       \node[dot,label=left:{$\avariablefour$}] (k) [below right= 2.7cm and 0.1 of i] {};

       \draw[reach] (i) -- (m1);
       \draw[pto] (m1) to node [above right] {$+$} (m2);
       \draw[reach] (j) -- (m2);
       \draw[reach] (m2) to [out=180,in=-75] (k);
       \draw[pto] (k) to [bend left=30] node [left] {$+$} (m1);

     \end{tikzpicture}
 }
\end{center}
For the three cases, it is  easy to check that
$(\reach(\avariablebis,\avariable)\separate \reach(\avariableter,\avariable))$ holds true.
Concerning the satisfaction of the formula
$(\reachplus(\avariable,\avariable) \implies (\reach(\avariablebis,\avariable) \separate \reachplus(\avariable,\avariable)))$
(only meaningful in the third case), the way to separate the heap into two disjoint subheaps
for satisfying $\reach(\avariablebis,\avariable)$ and $\reachplus(\avariable,\avariable)$ respectively
is easy.

Now, let us suppose that $\pair{\astore}{\aheap}$ satisfies
$\extension{\avariable = \ameetvar{\avariablebis}{\avariableter}{\avariablefour}}$, which again is the formula
$$
\reach(\avariable,\avariablefour) \land
(\reach(\avariablebis,\avariable)\separate \reach(\avariableter,\avariable)) \land
(\reachplus(\avariable,\avariable) \implies (\reach(\avariablebis,\avariable) \separate \reachplus(\avariable,\avariable))).
$$
Consequently,
$
\pair{\astore}{\aheap} \models \reach(\avariable,\avariablefour) \land
(\reach(\avariablebis,\avariable)\separate \reach(\avariableter,\avariable)).
$
Now, $\pair{\astore}{\aheap} \models
(\reach(\avariablebis,\avariable)\separate \reach(\avariableter,\avariable))$ clearly implies $\pair{\astore}{\aheap} \models
\reach(\avariablebis,\avariable) \land \reach(\avariableter,\avariable)$.
Indeed, $(\reach(\avariablebis,\avariable)\separate \reach(\avariableter,\avariable))$ states that there are $\aheap_1$ and $\aheap_2$ such that $\aheap = \aheap_1 + \aheap_2$ and there are $\alength_1,\alength_2$ such that $\aheap_1^{\alength_1}(\astore(\avariablebis)) = \astore(\avariable)$ and
$\aheap_2^{\alength_2}(\astore(\avariableter)) = \astore(\avariable)$. As $\aheap_1 \subheap \aheap$ and $\aheap_2 \subheap \aheap$, it must hold that
$\aheap^{\alength_1}(\astore(\avariablebis)) = \astore(\avariable)$ and
$\aheap^{\alength_2}(\astore(\avariableter) = \astore(\avariable)$ or, equivalently, $\pair{\astore}{\aheap} \models
\reach(\avariablebis,\avariable) \land \reach(\avariableter,\avariable)$.
By definition, $\pair{\astore}{\aheap} \models
\reach(\avariablebis,\avariable) \land \reach(\avariableter,\avariable) \land \reach(\avariable,\avariablefour)$ implies that $\semantics{\ameetvar{\avariablebis}{\avariableter}{\avariablefour}}_{\astore,\aheap}$
is defined. Let us consider the three possibilities.
\begin{center}
 \scalebox{0.85}{
     \begin{tikzpicture}[baseline]
       \node[dot,label=above:$\avariablebis$] (i) at (0,0) {};
       \node[dot,label=left:{$\ameetvar{\avariablebis}{\avariableter}{\avariablefour}$}] (m) [below right = 1.5cm and 0.5cm of i] {};
       \node[dot,label=above:$\avariableter$] (j) [above right=1.5cm and 0.5cm of m] {};
       \node[dot,label=below:{$\avariablefour$\\$\avariablefour$ not inside a loop}] (k) [below of=m] {};

       \draw[reach] (i) -- (m);
       \draw[reach] (j) -- (m);
       \draw[reach] (m) -- (k);
     \end{tikzpicture}
     \quad
     \begin{tikzpicture}[baseline]
       \node[dot,label=above:$\avariablebis$] (i) at (0,0) {};
       \node[dot,label=left:{$\ameetvar{\avariablebis}{\avariableter}{\avariablefour}$}] (m) [below right = 1.5cm and 0.5cm of i] {};
       \node[dot,label=above:$\avariableter$] (j) [above right=1.5cm and 0.5cm of m] {};
       \node[dot] (mid) [below=0.8cm of m] {};
       \node[dot,label=below:{$\avariablefour$}] (k) [below=1.65cm of m] {};

       \draw[reach] (i) -- (m);
       \draw[reach] (j) -- (m);
       \draw[reach] (m) -- (mid);
       \draw[reach] (mid) to [out=-35,in=35] (k);
       \draw[pto] (k) to [out=155,in=-155] node [left] {$+$} (mid);
     \end{tikzpicture}
     \qquad
     \begin{tikzpicture}[baseline]
       \node[dot,label=above:$\avariablebis$] (i) at (0,0) {};
       \node[dot,label=left:{$\ameetvar{\avariablebis}{\avariableter}{\avariablefour}$}]
       (m1) [below right = 1.5cm and 0.4cm of i] {};
       \node[dot,label=right:{$\alocation$}] (m2) [below right = 1.7cm and 0.4cm of m1] {};
       \node[dot,label=above:$\avariableter$] (j) [above right=1.5cm and 0.5cm of m2] {};
       \node[dot,label=left:{$\avariablefour$}] (k) [below right= 2.7cm and 0.1 of i] {};

       \draw[reach] (i) -- (m1);
       \draw[pto] (m1) to node [above right] {$+$} (m2);
       \draw[reach] (j) -- (m2);
       \draw[reach] (m2) to [out=180,in=-75] (k);
       \draw[pto] (k) to [bend left=30] node [left] {$+$} (m1);

     \end{tikzpicture}
 }
\end{center}
In the first and second cases, the only way to satisfy
$(\reach(\avariablebis,\avariable)\separate \reach(\avariableter,\avariable))$
is to have $\avariable = \ameetvar{\avariablebis}{\avariableter}{\avariablefour}$ (otherwise some sharing
is needed to reach $\avariable$ in two ways).
In the third case, as
$\pair{\astore}{\aheap} \models  \reach(\avariablebis,\avariable)
\land \reach(\avariableter,\avariable)$, necessarily we have
$\pair{\astore}{\aheap} \models \reachplus(\avariable,\avariable)$ and therefore
$\pair{\astore}{\aheap} \models (\reach(\avariablebis,\avariable) \separate \reachplus(\avariable,\avariable))$.
However, for any value $\alocation'$ distinct from
$\semantics{\ameetvar{\avariablebis}{\avariableter}{\avariablefour}}_{\astore,\aheap}$
in the loop containing $\astore(\avariable)$,
$\pair{\astore[\avariable \leftarrow \alocation']}{\aheap}
\not \models (\reach(\avariablebis,\avariable) \separate \reachplus(\avariable,\avariable))$.
So, we have $\astore(\avariable) = \semantics{\ameetvar{\avariablebis}{\avariableter}{\avariablefour}}_{\astore,\aheap}$.

($\star$) Now, let us show that the core formula $\seesgeq{\avariable}{\avariablebis}{\asetmeetvar \cup \{\avariableter\}}{\inbound}$ is logically
equivalent to
 $$\seesgeq{\avariable}{\avariablebis}{\asetmeetvar}{\inbound} \land
\big(\avariableter = \avariable \lor \avariableter = \avariablebis \lor (\true \separate (\reachplus(\avariable,\avariablebis) \land \lnot \reachplus(\avariable,\avariableter)))\big),
$$
assuming that $\seesgeq{\avariable}{\avariablebis}{\asetmeetvar}{\inbound}$ is already shown logically equivalent to its
extension (which can be seen as an induction hypothesis).
First, let us assume that $\pair{\astore}{\aheap} \models \seesgeq{\avariable}{\avariablebis}{\asetmeetvar \cup \{\avariableter\}}{\inbound}$.
By definition of $\models$ on core formulae, we have
\begin{enumerate}
\item $\card{\minpath{\semantics{\avariable}_{\astore,\aheap}}{\semantics{\avariablebis}_{\astore,\aheap}}{\aheap}} \geq \inbound$,
\item $\minpath{\semantics{\avariable}_{\aheap}}{\semantics{\avariablebis}_{\astore,\aheap}}{\aheap} \subseteq
      \pathset{\semantics{\avariable}_{\astore,\aheap}}{\astore,\aheap}{\asetmeetvar \cup \{\avariableter\}}$.
\end{enumerate}
As $\pathset{\semantics{\avariable}_{\astore,\aheap}}{\astore,\aheap}{\asetmeetvar \cup \{\avariableter\}} \subseteq
   \pathset{\semantics{\avariable}_{\astore,\aheap}}{\astore,\aheap}{\asetmeetvar}$, we get
$$\minpath{\semantics{\avariable}_{\aheap}}{\semantics{\aterm_2}_{\astore,\aheap}}{\aheap} \subseteq
      \pathset{\semantics{\avariable}_{\astore,\aheap}}{\astore,\aheap}{\asetmeetvar},$$ and
by induction hypothesis, $\pair{\astore}{\aheap} \models \extension{\seesgeq{\avariable}{\avariablebis}{\asetmeetvar}{\inbound}}$,
which is logically equivalent to $\pair{\astore}{\aheap} \models \seesgeq{\avariable}{\avariablebis}{\asetmeetvar}{\inbound}$.
Let $\alength$ be the minimal value greater than one such that $\aheap^{\alength}(\semantics{\avariable}_{\astore,\aheap}) =
\semantics{\avariablebis}_{\astore,\aheap}$ ($\alength \geq \inbound$).
As  $\pair{\astore}{\aheap} \models \seesgeq{\avariable}{\avariablebis}{\asetmeetvar \cup \{\avariableter\}}{\inbound}$, by definition
of $\card{\minpath{\semantics{\avariable}_{\astore,\aheap}}{\semantics{\avariablebis}_{\astore,\aheap}}{\aheap}}$ and
$ \pathset{\semantics{\avariable}_{\astore,\aheap}}{\astore,\aheap}{\asetmeetvar \cup \{\avariableter\}}$, we get one of the conditions
below holds:
\begin{itemize}
\item $\semantics{\avariable}_{\astore,\aheap} \in \semantics{\asetmeetvar \cup \{\avariableter\}}_{\astore,\aheap}$,
\item $\semantics{\avariablebis}_{\astore,\aheap} \in \semantics{\asetmeetvar \cup \{\avariableter\}}_{\astore,\aheap}$,
\item for all $\alength' \in \interval{0}{\alength}$, $\aheap^{\alength'}(\semantics{\avariable}_{\astore,\aheap}) \not \in
\semantics{\asetmeetvar \cup \{\avariableter\}}_{\astore,\aheap}$.
\end{itemize}
So, in the case $\semantics{\avariable}_{\astore,\aheap} \neq \semantics{\avariableter}_{\astore,\aheap}$
and  $\semantics{\avariablebis}_{\astore,\aheap} \neq  \semantics{\avariableter}_{\astore,\aheap}$, we have
for all $\alength' \in \interval{0}{\alength}$, $\aheap^{\alength'}(\semantics{\avariable}_{\astore,\aheap}) \neq
\semantics{\avariableter}_{\astore,\aheap}$, which implies that the shortest path from
$\semantics{\avariable}_{\astore,\aheap}$ to $\semantics{\avariablebis}_{\astore,\aheap}$ (of length at least one)
does not visit $\semantics{\avariableter}_{\astore,\aheap}$. Hence,
$$
\pair{\astore}{\aheap} \models
\neg (\avariableter = \avariable \lor \avariableter = \avariablebis)
\Rightarrow
(\true \separate (\reachplus(\avariable,\avariablebis) \land \lnot \reachplus(\avariable,\avariableter))).
$$
Now, suppose that $\pair{\astore}{\aheap} \models
\extension{\seesgeq{\avariable}{\avariablebis}{\asetmeetvar \cup \{\avariableter\}}{\inbound}}$.
As $\pair{\astore}{\aheap} \models \seesgeq{\avariable}{\avariablebis}{\asetmeetvar}{\inbound}$,
there is a path from $\semantics{\avariable}_{\astore,\aheap}$ to $\semantics{\avariablebis}_{\astore,\aheap}$
and its minimal length $\alength$ is greater than $\inbound$. Moreover, for all
$\alength' \in \interval{1}{\alength-1}$, we have $\aheap^{\alength'}(\semantics{\avariable}_{\astore,\aheap}) \not
\in \semantics{\asetmeetvar}_{\astore,\aheap}$.
As  $\pair{\astore}{\aheap} \models \avariableter = \avariable \lor \avariableter = \avariablebis \lor (\true \separate (\reachplus(\avariable,\avariablebis) \land \lnot \reachplus(\avariable,\avariableter)))$, let us perform a case analysis.
\begin{itemize}
\item Suppose that  $\pair{\astore}{\aheap} \models \avariableter = \avariable$. As $\alength$ is the minimal
length from $\semantics{\avariable}_{\astore,\aheap}$ to $\semantics{\avariablebis}_{\astore,\aheap}$, we have that
for all
$\alength' \in \interval{1}{\alength-1}$,  $\aheap^{\alength'}(\semantics{\avariable}_{\astore,\aheap}) \not
\in \semantics{\asetmeetvar \cup \set{\avariableter}}_{\astore,\aheap}$ and therefore
$\pair{\astore}{\aheap} \models
\seesgeq{\avariable}{\avariablebis}{\asetmeetvar \cup \{\avariableter\}}{\inbound}$.
\item Supposing that $\pair{\astore}{\aheap} \models \avariableter = \avariablebis$, leads to the same conclusion by the same
reasoning.
\item Now, suppose that $\pair{\astore}{\aheap} \models
(\true \separate (\reachplus(\avariable,\avariablebis) \land \lnot \reachplus(\avariable,\avariableter))$
and  $\pair{\astore}{\aheap} \not \models \avariableter = \avariable \lor \avariableter = \avariablebis$.
So, there is a subheap $\aheap'$ of $\aheap$ such that
 $\pair{\astore}{\aheap'} \models \reachplus(\avariable,\avariablebis) \land \lnot \reachplus(\avariable,\avariableter)$
and therefore for all
$\alength' \in \interval{1}{\alength-1}$, we have $(\aheap')^{\alength'}(\semantics{\avariable}_{\astore,\aheap'})
\neq \semantics{\avariableter}_{\astore,\aheap'}$, which is equivalent to
for all
$\alength' \in \interval{1}{\alength-1}$, we have $\aheap^{\alength'}(\semantics{\avariable}_{\astore,\aheap})
\neq \semantics{\avariableter}_{\astore,\aheap}$. So,
for all
$\alength' \in \interval{1}{\alength-1}$,  $\aheap^{\alength'}(\semantics{\avariable}_{\astore,\aheap}) \not
\in \semantics{\asetmeetvar \cup \set{\avariableter}}_{\astore,\aheap}$ and therefore
$\pair{\astore}{\aheap} \models
\seesgeq{\avariable}{\avariablebis}{\asetmeetvar \cup \{\avariableter\}}{\inbound}$.
\end{itemize}

($\star$) Now, let us show that the core formula
 $\seesgeq{\avariable}{\ameetvar{\avariablebis}{\avariableter}{\avariablefour}}{\asetmeetvar}{\inbound}$
 is logically
equivalent to
\begin{nscenter}
$(
\avariablebis = \ameetvar{\avariablebis}{\avariableter}{\avariablefour} \land \seesgeq{\avariable}{\avariablebis}{\asetmeetvar}{\inbound}) \lor
 \inpath{\avariablebis}{\avariablefour}{\avariablesept} (\avariablesept = \ameetvar{\avariablebis}{\avariableter}{\avariablefour} \land \seesgeq{\avariable}{\avariablesept}{\asetmeetvar}{\inbound}),
$
\end{nscenter}
 where $\avariablesept \not \in \set{\avariable,\avariablebis,\avariableter,\avariablefour} \cup \chars{\asetmeetvar}$
and
assuming that $\seesgeq{\avariable}{\avariablesept}{\asetmeetvar}{\inbound}$
 is already shown logically equivalent to its
extension (which can be seen as an induction hypothesis, and this has been proved just previously).

First, let us assume that $\pair{\astore}{\aheap} \models
\seesgeq{\avariable}{\ameetvar{\avariablebis}{\avariableter}{\avariablefour}}{\asetmeetvar}{\inbound}$.
So, there is a path from $\semantics{\avariable}_{\astore,\aheap}$ to
$\semantics{\ameetvar{\avariablebis}{\avariableter}{\avariablefour}}_{\astore,\aheap}$
and its minimal length $\alength$ is greater than $\inbound$.
If $\semantics{\ameetvar{\avariablebis}{\avariableter}{\avariablefour}}_{\astore,\aheap} = \astore(\avariablebis)$ then there is a path from $\semantics{\avariable}_{\astore,\aheap}$ to $\astore(\avariablebis)$ of minimal length at least $\inbound$ and trivially
$\pair{\astore}{\aheap} \models \avariablebis = \ameetvar{\avariablebis}{\avariableter}{\avariablefour} \land \seesgeq{\avariable}{\avariablebis}{\asetmeetvar}{\inbound})$.
Suppose instead that $\semantics{\ameetvar{\avariablebis}{\avariableter}{\avariablefour}}_{\astore,\aheap} \neq \astore(\avariablebis)$.
Then from the definition of meet-points, there is a path from $\astore(\avariablebis)$ to $\semantics{\ameetvar{\avariablebis}{\avariableter}{\avariablefour}}_{\astore,\aheap}$ and a path from $\semantics{\ameetvar{\avariablebis}{\avariableter}{\avariablefour}}_{\astore,\aheap}$ to $\astore(\avariablefour)$.
As $\semantics{\ameetvar{\avariablebis}{\avariableter}{\avariablefour}}_{\astore,\aheap} \neq \astore(\avariablebis)$, then
$\minpath{\semantics{\avariablebis}_{\astore,\aheap}}{\semantics{\avariablefour}_{\astore,\aheap}}{\aheap}$ is not empty.
By Lemma~\ref{lemma:meetinsideminpath} $\semantics{\ameetvar{\avariablebis}{\avariableter}{\avariablefour}}_{\astore,\aheap} \in
\minpath{\semantics{\avariablebis}_{\aheap}}{\semantics{\avariablefour}_{\astore,\aheap}}{\aheap} \cup \{\astore(\avariablefour)\}$.
Then there is $\alocation$ such that
$\pair{\astore [\avariablesept \gets \alocation]}{\aheap} \models
\avariablesept = \ameetvar{\avariablebis}{\avariableter}{\avariablefour}
\land \seesgeq{\avariable}{\avariablesept}{\asetmeetvar}{\inbound}$.
Namely, $\alocation = \semantics{\ameetvar{\avariablebis}{\avariableter}{\avariablefour}}_{\astore,\aheap}$
and by definition of $\models$ on core formulae, we get
$\pair{\astore}{\aheap} \models
\inpath{\avariable}{\avariablefour}{\avariablesept} (\avariablesept = \ameetvar{\avariablebis}{\avariableter}{\avariablefour} \land \seesgeq{\avariable}{\avariablesept}{\asetmeetvar}{\inbound})$.

Now, suppose that $\pair{\astore}{\aheap} \models
\extension{\seesgeq{\avariable}{\ameetvar{\avariablebis}{\avariableter}{\avariablefour}}{\asetmeetvar}{\inbound}}$.
Since the disjunction has two disjuncts, we perform a simple case analysis.
First, we assume that $\pair{\astore}{\aheap} \models \avariablebis = \ameetvar{\avariablebis}{\avariableter}{\avariablefour} \land \seesgeq{\avariable}{\avariablebis}{\asetmeetvar}{\inbound}$.
Then easily $\pair{\astore}{\aheap} \models \seesgeq{\avariable}{\ameetvar{\avariablebis}{\avariableter}{\avariablefour}}{\asetmeetvar}{\inbound}$
as $\astore(\avariablebis) = \semantics{\ameetvar{\avariablebis}{\avariableter}{\avariablefour}}_{\astore,\aheap}$.
For the second disjunct, suppose
$\pair{\astore}{\aheap} \models \inpath{\avariablebis}{\avariablefour}{\avariablesept} (\avariablesept = \ameetvar{\avariablebis}{\avariableter}{\avariablefour} \land \seesgeq{\avariable}{\avariablesept}{\asetmeetvar}{\inbound})$. By definition of $\models$ on core formulae,
there is $\alocation \in \minpath{\astore(\avariablebis)}{\astore(\avariablefour)}{\aheap}\cup\{\astore(\avariablefour)\}$ such that
$\pair{\astore[\avariablesept \gets \alocation]}{\aheap} \models
(\avariablesept = \ameetvar{\avariablebis}{\avariableter}{\avariablefour} \land \seesgeq{\avariable}{\avariablesept}{\asetmeetvar}{\inbound})$.
Obviously, this implies that $\pair{\astore}{\aheap} \models \seesgeq{\avariable}{\ameetvar{\avariablebis}{\avariableter}{\avariablefour}}{\asetmeetvar}{\inbound}$.

($\star$) In order to conclude the proof, let us show that the core formula
$\remgeq{\asetpath}{\inbound}$
 is logically
equivalent to
$$\bigvee_{\mathclap{\substack{\asetpath' \subseteq \asetpath\\
  \meets{\asetpath'} = \{\ameetvar{\avariable_i}{\avariablebis_i}{\avariableter_i} \mid i \in \interval{1}{n}\}\\
  K \subseteq \interval{1}{n}
  }}}
  \Big(
  \bigwedge_{\pair{\aterm_1}{\aterm_2} \in \asetpath'} \sees{\aterm_1}{\aterm_2}{\emptyset} \land
    \bigwedge_{\mathclap{\pair{\aterm_1}{\aterm_2} \in \asetpath \setminus \asetpath'}} \lnot \sees{\aterm_1}{\aterm_2}{\emptyset}
     \land
     \bigwedge_{\mathclap{i \in K}} \avariable_i \neq \avariableter_i
     \land
     \bigwedge_{\mathclap{i \in \interval{1}{n}\setminus K}} \avariable_i = \avariableter_i
     \land
     $$
$$ \inpathindex{\avariable_i}{\avariableter_i}{\avariablesept_i}{i \in K}
        \big(\bigwedge_{\mathclap{i \in K}}
          \avariablesept_i = \ameetvar{\avariable_i}{\avariablebis_i}{\avariableter_i}
          \land
(\strict{
            \bigwedge_{
            \mathclap{\substack{
            \asetpath'' = \asetpath'[\ameetvar{\avariable_i}{\avariablebis_i}{\avariableter_i} \gets \avariablesept_i \mid i \in K][\ameetvar{\avariable_i}{\avariablebis_i}{\avariableter_i} \gets \avariable_i \mid i \in \interval{1}{n}\setminus K]\\
            \pair{\avariable}{\avariablebis} \in \asetpath''
            }}} \sees{\avariable}{\avariablebis}{\emptyset}
          } \separate \size \geq \inbound)
        \big)
     \Big),$$

where $\inpathindex{\avariable_i}{\avariableter_i}{\avariablesept_i}{i \in K}$ is a shortcut for a sequence of
$\card{K}$ applications of $\inpath{\avariable_i}{\avariableter_i}{\avariablesept_i}$.

First, let us assume that $\pair{\astore}{\aheap} \models \remgeq{\asetpath}{\inbound}$.
By definition of $\models$, assuming that
$\remset{\astore,\aheap}{\asetpath}$ is equal to
$\domain{\aheap} \setminus \big(\bigcup_{\pair{\aterm_1}{\aterm_2}\in\asetpath} \minpath{\semantics{\aterm_1}_{\astore,\aheap}}{\semantics{\aterm_2}_{\astore,\aheap}}{\aheap}\big)$,
$\pair{\astore}{\aheap} \models \remgeq{\asetpath}{\inbound}$
is equivalent to $\card{\remset{\astore,\aheap}{\asetpath}} \geq \inbound$.
Note that $\remset{\astore,\aheap}{\asetpath}$ is also equal to
$$
\domain{\aheap} \setminus \big(\bigcup_{\pair{\aterm_1}{\aterm_2}\in\asetpath \ \& \  \pair{\astore}{\aheap} \models \sees{\aterm_1}{\aterm_2}{\emptyset}}
\minpath{\semantics{\aterm_1}_{\astore,\aheap}}{\semantics{\aterm_2}_{\astore,\aheap}}{\aheap}\big).
$$
Let $\asetpath'$ be the subset of $\asetpath$ defined as
$$
\asetpath' \egdef \set{\pair{\aterm_1}{\aterm_2} \in \asetpath \ \mid \ \pair{\astore}{\aheap} \models \sees{\aterm_1}{\aterm_2}{\emptyset}}.
$$
Obviously, $\pair{\astore}{\aheap} \models \bigwedge_{\pair{\aterm_1}{\aterm_2} \in \asetpath'} \sees{\aterm_1}{\aterm_2}{\emptyset} \land \ \ \ \ \ \
    \bigwedge_{\mathclap{\pair{\aterm_1}{\aterm_2} \in \asetpath \setminus \asetpath'}} \ \ \ \ \ \ \ \ \lnot \sees{\aterm_1}{\aterm_2}{\emptyset}$.
Assuming that $\meets{\asetpath'} = \set{\ameetvar{\avariable_i}{\avariablebis_i}{\avariableter_i} \mid i \in \interval{1}{n}}$,
let $K \subseteq \interval{1}{n}$ be such that
$$
K \egdef \set{i \in \interval{1}{n} \ \mid \ \pair{\astore}{\aheap} \models \avariable_i \neq \avariableter_i
}.
$$
Without loss of generality, let us assume that $K = \interval{1}{k}$ and $k \geq 1$ (otherwise when $K = \emptyset$
we can easily handle this degenerate case).
Obviously, $\pair{\astore}{\aheap} \models \bigwedge_{i \in K}  \avariable_i \neq \avariableter_i
     \land
     \bigwedge_{i \in \interval{1}{n}\setminus K} \avariable_i = \avariableter_i$.
So, whenever, $i \not \in K$,  $\pair{\astore}{\aheap} \models \avariable_i = \avariableter_i =
\ameetvar{\avariable_i}{\avariablebis_i}{\avariableter_i}$ and therefore $\ameetvar{\avariable_i}{\avariablebis_i}{\avariableter_i}$
can be replaced by $\avariable_i$.
For each $i \in K$, let $\alocation_i = \semantics{\ameetvar{\avariable_i}{\avariablebis_i}{\avariableter_i}}_{\astore,\aheap}$.
Let $\avariablesept_1, \ldots, \avariablesept_k$ be a set of fresh variables and
$\asetpath'' = \asetpath'[\ameetvar{\avariable_i}{\avariablebis_i}{\avariableter_i} \gets \avariablesept_i \mid i
\in K][\ameetvar{\avariable_i}{\avariablebis_i}{\avariableter_i} \gets \avariable_i \mid i \in \interval{1}{n}\setminus K]$.

By definition of $\models$ on $\remset{\astore,\aheap}{\asetpath}$, we have
$$
\pair{\astore[\avariablesept_i \gets \alocation_i, i \in K]}{\aheap}
\models
\strict{\bigwedge_{\pair{\avariable}{\avariablebis} \in \asetpath''} \sees{\avariable}{\avariablebis}{\emptyset}}
\separate \size \geq \inbound,
$$
which entails that
$$
\pair{\astore}{\aheap} \models
\inpathindex{\avariable_i}{\avariableter_i}{\avariablesept_i}{i \in K}
        \big(\bigwedge_{\mathclap{i \in K}}
          \avariablesept_i = \ameetvar{\avariable_i}{\avariablebis_i}{\avariableter_i}
          \land
(
\strict{\bigwedge_{\pair{\avariable}{\avariablebis} \in \asetpath''} \sees{\avariable}{\avariablebis}{\emptyset}}
\separate \size \geq \inbound
).
$$
So, $\pair{\astore}{\aheap} \models \extension{\remgeq{\asetpath}{\inbound}}$ as one of the disjuncts of
$\extension{\remgeq{\asetpath}{\inbound}}$ holds true.

We omit the proof in the other direction as when assuming $\pair{\astore}{\aheap} \models \extension{\remgeq{\asetpath}{\inbound}}$,
one of the disjuncts of $\extension{\remgeq{\asetpath}{\inbound}}$ holds and we can establish that
$$
\card{\domain{\aheap} \setminus \big(\bigcup_{\pair{\aterm_1}{\aterm_2}\in\asetpath} \minpath{\semantics{\aterm_1}_{\astore,\aheap}}{\semantics{\aterm_2}_{\astore,\aheap}}{\aheap}\big)} \geq \inbound.
$$
Indeed, most of the steps in the proof for the other direction, work
in both directions.
\end{proof}
