# Supplementary material for: A Complete Axiomatisation for Quantifier-Free Separation Logic
Source: arXiv:2006.05156 source file (2021-08-09)
Supplement: Supplementary file 17 [file proof-pspace.tex]

\theorempspace*

\begin{proof}
Correctness of
the symbolic approach and therefore of Algorithm~\ref{algo:symb-model-checking} below rely on the following properties
($\asms = \symbms{\astore}{\aheap}{\asetvar}{\bound}$,  for some memory state $\pair{\astore}{\aheap}$):
\begin{enumerate}
\itemsep 0 cm
\item Assume that $\bound = \bound_1 + \bound_2$ with $\bound_1, \bound_2 \geq 1$.
      \begin{enumerate}
      \itemsep 0 cm
      \item If $\symbunion{\asms_1}{\asms_2}{\asms}$
      with $\asms_i$ over $\pair{\asetvar}{\bound_i}$, then there are $\aheap_1$ and $\aheap_2$ such that
      $\aheap = \aheap_1 + \aheap_2$ and $\asms_i = \symbms{\astore}{\aheap_i}{\asetvar}{\bound_i}$ ($i \in \set{1,2}$).
      \item If $\aheap = \aheap_1 + \aheap_2$, then
            $\symbunion{\symbms{\astore}{\aheap_1}{\asetvar}{\bound_1}}{\symbms{\astore}{\aheap_2}{\asetvar}{\bound_2}}{\asms}$.
      \end{enumerate}
      The symbolic composition of symbolic memory states is defined formally in Appendix~\ref{appendix:CompositionMemoryState}.
      The two above properties are mere consequences of~\ref{compositionproperty} (see also Appendix~\ref{appendix:CompositionMemoryState}).
\item Assume that $\lfloor \frac{\bound}{2} \rfloor = \bound_1$.
      \begin{enumerate}
      \itemsep 0 cm
      \item If $\asymbexists{\avariable}{\avariablebis}{\avariableter}(\asms_1,\asms)$, then
            there is $\alocation \in \minpath{\astore(\avariable)}{\astore(\avariablebis)}{\aheap} \cup \set{\astore(\avariablebis)}$
            such that $\asms_1 = \symbms{\astore [\avariableter \gets \alocation]}{\aheap}{\asetvar \cup \set{\avariableter}}{\bound_1}$.
      \item If  $\alocation \in \minpath{\astore(\avariable)}{\astore(\avariablebis)}{\aheap} \cup \set{\astore(\avariablebis)}$,
            then $\asymbexists{\avariable}{\avariablebis}{\avariableter}(\symbms{\astore [\avariableter \gets \alocation]}{\aheap}{\asetvar \cup \set{\avariableter}}{\bound_1},\asms)$.
      \end{enumerate}
      The symbolic quantifier $\asymbexists{\avariable}{\avariablebis}{\avariableter}$ is introduced in Appendix~\ref{appendix-eliminate-exists}.
      These two properties are mere consequences of Lemma~\ref{lemma:quantificationisok}.
\end{enumerate}

Algorithm~\ref{algo:symb-model-checking} below defines the function  \textsc{MC}($\asms, \aformula$)
that takes as  arguments a satisfiable symbolic memory state $\asms$ over $\pair{\asetvar}{\bound}$
and a formula $\aformula$ with $\chars{\aformula} \subseteq \asetvar$ and $\msize{\aformula} \leq \bound$.
We write ``\Return $\mathtt{true}$ iff $\mathcal{B}$'' where $\mathcal{B}$ is a Boolean expression as a shortcut
for ``if $\mathcal{B}$ then \Return $\mathtt{true}$ else \Return $\mathtt{false}$''.
Note also that $\asms$ is understood as satisfiable when $\charsymbform{\triple{\symbterms}{\amap}{\symbrem}}$ itself is  satisfiable
in \intervalSL. By the proof of Lemma~\ref{lemma:axiomstwoRCchars}, this can be checked in polynomial-time in
$\card{\asetvar}+\bound$ (a semantical proof would be also possible).

\begin{algorithm}[!ht]
\footnotesize
\caption{Symbolic model checking \label{algo:symb-model-checking}}
\begin{algorithmic}[1]
   \Require{Satisfiable symbolic memory state $\asms = \triple{\symbterms}{\amap}{\symbrem}$ over $\pair{\asetvar}{\bound}$, a formula $\aformula$
   with $\chars{\aformula} \subseteq \asetvar$ and $\msize{\aformula} \leq \bound$.}
   \Ensure{Return $\mathtt{true}$ iff $\pair{\astore}{\aheap} \models \aformula$ whenever  $\symbms{\astore}{\aheap}{\asetvar}{\bound}=\asms$.}
   \Function{\textsc{MC}}{$\asms, \aformula$}
    \Cases{$\aformula$}
    \Case{$\emp$} \Return $\mathtt{true}$ iff ($\amap$ is never defined and $\symbrem = 0$)
    \Case{$\avariable = \avariablebis$}  $\mathtt{true}$ iff there is $\asymbterm \in \symbterms$ such that $\set{\avariable,\avariablebis} \subseteq \asymbterm$
    \Case{$\avariable \Ipto \avariablebis$} \Return $\mathtt{true}$ iff there are $\asymbterm,\asymbterm' \in \symbterms$ such that
     $\avariable \in \asymbterm$, $\avariablebis \in \asymbterm'$ and $\amap(\asymbterm) = \pair{\asymbterm'}{1}$ \Comment{$\bound \geq 2$}
     \Case{$\neg \aformulabis$} \Return (not \textsc{MC}($\asms, \aformulabis$))
     \Case{$\aformulabis_1 \wedge \aformulabis_2$} \Return (\textsc{MC}($\asms, \aformulabis_1$) and \textsc{MC}($\asms, \aformulabis_2$))
     \Case{$\aformulabis_1 \separate \aformulabis_2$} \Comment{$\bound \geq \msize{\aformulabis_1} + \msize{\aformulabis_2}$}
     \State{\Return $\mathtt{true}$ iff there are $\bound_1, \bound_2$ such that $\bound = \bound_1 + \bound_2$, $\msize{\aformulabis_1} \leq \bound_1$,
      $\msize{\aformulabis_2} \leq \bound_2$}
     \State{and there are satisfiable $\asms_1$, $\asms_2$ (resp. over  $\pair{\asetvar}{\bound_1}$ and $\pair{\asetvar}{\bound_2}$) satisfying }
     \State{($\symbunion{\asms_1}{\asms_2}{\asms}$ and \textsc{MC}($\asms_1, \aformulabis_1$) and \textsc{MC}($\asms_2, \aformulabis_2$))}
     \Case{$\inpath{\avariable}{\avariablebis}{\avariableter} \aformulabis$} \Comment{$\bound \geq 2 \times \msize{\aformulabis}$}
     \State{$\bound' := \lfloor \frac{\bound}{2} \rfloor$}
     \State{\Return $\mathtt{true}$ iff there is satisfiable $\asms'$ over $\pair{\asetvar}{\bound'}$
      such that ($\asymbexists{\avariable}{\avariablebis}{\avariableter}(\asms',\asms)$ and \textsc{MC}($\asms', \aformulabis$))}
     \EndCases
    \EndFunction
  \end{algorithmic}
\end{algorithm}

The algorithm runs in polynomial space in $\card{\asetvar}+log(\bound)+\length{\aformula}$ based on the following observations:
\begin{itemize}
\itemsep 0 cm
\item The recursion depth is linear in the size of $\aformula$.
\item Assuming $\bound = \bound_1 + \bound_2$,  $\asms_1$ over $\pair{\asetvar}{\bound_1}$,  $\asms_2$ over $\pair{\asetvar}{\bound_2}$ and  $\asms$ over $\pair{\asetvar}{\bound}$,
      checking whether $\symbunion{\asms_1}{\asms_2}{\asms}$ holds can be checked in \np. Actually, the conditions for defining $\asymbunion$ except \ref{C-wasgarbage}(b) requires
      polynomial-time only. The condition \ref{C-wasgarbage}(b) is the only one requiring \np, as one needs to guess partial functions $\amapbis_1, \amapbis_2: \domain{\amap} \rightarrow \interval{0}{\bound}$.
\item Assuming $\bound' := \lfloor \frac{\bound}{2} \rfloor$,  $\asms'$ over $\pair{\asetvar}{\bound'}$, and  $\asms$ over $\pair{\asetvar}{\bound}$,
      checking whether $\asymbexists{\avariable}{\avariablebis}{\avariableter}(\asms',\asms)$ holds can be checked in polynomial time.
\item Symbolic memory states over $\pair{\asetvar}{\bound}$ are encoded in polynomial size in $\card{\asetvar}+log(\bound)$.
\end{itemize}

The  property ($\dag$) below establishes that the algorithm is correct, explaining why we needed
the satisfaction of the properties 1(a), 1(b), 2(a) and 2(b) introduced in this proof (see its beginning).

($\dag$) For all satisfiable symbolic memory states $\asms$ over $\pair{\asetvar}{\bound}$,
for all memory states $\pair{\astore}{\aheap}$ such that $\symbms{\astore}{\aheap}{\asetvar}{\bound}=\asms$
and for all formulae $\aformula$ such that $\chars{\aformula} \subseteq \asetvar$ and
$\msize{\aformula} \leq \bound$,  we have MC($\asms$,$\aformula$) returns $\mathtt{true}$ iff  $\pair{\astore}{\aheap} \models \aformula$.

Consequently, $\aformula$ is satisfiable iff there is a satisfiable symbolic memory state $\asms$ over $\pair{\chars{\aformula}}{\msize{\aformula}}$
such that MC($\asms$,$\aformula$) returns $\mathtt{true}$, which can be checked in \pspace by Savitch's Theorem. Now, let us prove ($\dag$).
As expected, the proof is by structural induction.

\begin{description}
\itemsep 0 cm
\item[Base case: $\aformula$ equal to $\emp$.] First, suppose that $\pair{\astore}{\aheap} \models \emp$. Hence $\domain{\aheap} = \emptyset$, and if $\symbms{\astore}{\aheap}{\asetvar}{\bound} =
\triple{\symbterms}{\amap}{\symbrem} = \asms$, then $\symbrem = 0$ and $\amap$ is never defined, by definition of
$\symbms{\astore}{\aheap}{\asetvar}{\bound}$. Consequently, by line 3 in Algorithm~\ref{algo:symb-model-checking},
\textsc{MC}($\asms, \aformula$) $=$ $\mathtt{true}$. Now, suppose that \textsc{MC}($\asms, \aformula$) $=$ $\mathtt{true}$. So, by line 3
in Algorithm~\ref{algo:symb-model-checking}, $\symbrem = 0$ and $\amap$ is never defined, which implies that
whenever $\symbms{\astore}{\aheap}{\asetvar}{\bound}  = \asms$, we have $\domain{\aheap} = \emptyset$, whence $\pair{\astore}{\aheap} \models \emp$.

\item[Base case: $\aformula$ equal to $\avariable = \avariablebis$.] First, suppose that $\pair{\astore}{\aheap} \models \avariable = \avariablebis$.
Hence $\astore(\avariable) = \astore(\avariablebis)$, and if $\symbms{\astore}{\aheap}{\asetvar}{\bound} =
\triple{\symbterms}{\amap}{\symbrem} = \asms$, then there is $\asymbterm \in \symbterms$ such that $\set{\avariable,\avariablebis} \subseteq \asymbterm$, by definition of
$\symbms{\astore}{\aheap}{\asetvar}{\bound}$. Consequently, by line 4 in Algorithm~\ref{algo:symb-model-checking},
\textsc{MC}($\asms, \aformula$) $=$ $\mathtt{true}$. If we suppose that \textsc{MC}($\asms, \aformula$) $=$ $\mathtt{true}$, the proof follows the one
for the base case  $\aformula$ equal to $\emp$.

\item[Base case: $\aformula$ equal to $\avariable \Ipto \avariablebis$.] First, suppose that $\pair{\astore}{\aheap} \models \avariable \Ipto \avariablebis$.
Hence $\aheap(\astore(\avariable)) = \astore(\avariablebis)$, and if $\symbms{\astore}{\aheap}{\asetvar}{\bound} =
\triple{\symbterms}{\amap}{\symbrem} = \asms$, then
there are $\asymbterm,\asymbterm' \in \symbterms$ such that
     $\avariable \in \asymbterm$, $\avariablebis \in \asymbterm'$ and $\amap(\asymbterm) = \pair{\asymbterm'}{1}$, by definition of
$\symbms{\astore}{\aheap}{\asetvar}{\bound}$. Consequently, by line 5 in Algorithm~\ref{algo:symb-model-checking},
\textsc{MC}($\asms, \aformula$) $=$ $\mathtt{true}$.  If we suppose that \textsc{MC}($\asms, \aformula$) $=$ $\mathtt{true}$, the proof follows the one
for the base case  $\aformula$ equal to $\emp$.

\end{description}

In the induction step, the cases for Boolean connectives are by an easy verification. Let us treat the two other cases.

\begin{description}
\itemsep 0 cm

\item[Induction step: $\aformula = \aformulabis_1 \separate \aformulabis_2$.]
First, suppose that  $\pair{\astore}{\aheap} \models \aformula$.
By definition of the satisfaction relation $\models$, there are $\aheap_1$ and $\aheap_2$ such that $\aheap = \aheap_1 + \aheap_2$,
$\pair{\astore}{\aheap_1} \models \aformulabis_1$ and $\pair{\astore}{\aheap_2} \models \aformulabis_2$.
Let $\bound_1, \bound_2$ be such that $\bound = \bound_1 + \bound_2$, $\msize{\aformulabis_1} \leq \bound_1$ and $\msize{\aformulabis_2} \leq \bound_2$.
By the property 1(b), we have $\symbunion{\symbms{\astore}{\aheap_1}{\asetvar}{\bound_1}}{\symbms{\astore}{\aheap_2}{\asetvar}{\bound_2}}{\symbms{\astore}{\aheap}{\asetvar}{\bound}}$.
Obviously $\symbms{\astore}{\aheap_1}{\asetvar}{\bound_1}$ and $\symbms{\astore}{\aheap_2}{\asetvar}{\bound_2}$ are satisfiable.
By the induction hypothesis, we have \textsc{MC}($\symbms{\astore}{\aheap_1}{\asetvar}{\bound_1}, \aformulabis_1$) $=$ $\mathtt{true}$
and \textsc{MC}($\symbms{\astore}{\aheap_2}{\asetvar}{\bound_2}, \aformulabis_2$) $=$ $\mathtt{true}$.
By lines 8--11 in Algorithm~\ref{algo:symb-model-checking}, \textsc{MC}($\symbms{\astore}{\aheap}{\asetvar}{\bound}, \aformula$) $=$ $\mathtt{true}$.

Conversely, suppose that \textsc{MC}($\asms, \aformula$) $=$ $\mathtt{true}$. By lines 8--11 in Algorithm~\ref{algo:symb-model-checking},
there are $\bound_1, \bound_2$  such that $\bound = \bound_1 + \bound_2$, $\msize{\aformulabis_1} \leq \bound_1$ and $\msize{\aformulabis_2} \leq \bound_2$
and there are satisfiable $\asms_1$, $\asms_2$ (resp. over  $\pair{\asetvar}{\bound_1}$ and $\pair{\asetvar}{\bound_2}$)
such that ($\symbunion{\asms_1}{\asms_2}{\asms}$ and \textsc{MC}($\asms_1, \aformulabis_1$) and \textsc{MC}($\asms_2, \aformulabis_2$)).
As $\pair{\astore}{\aheap}$ is such that $\symbms{\astore}{\aheap}{\asetvar}{\bound} = \asms$,
by 1(a), there are  $\aheap_1$ and $\aheap_2$ such that $\aheap = \aheap_1 + \aheap_2$,
$\asms_1 = \symbms{\astore}{\aheap_1}{\asetvar}{\bound_1}$ and $\asms_2 = \symbms{\astore}{\aheap_2}{\asetvar}{\bound_2}$.
By the induction hypothesis, we have $\pair{\astore}{\aheap_1} \models \aformulabis_1$ and $\pair{\astore}{\aheap_2} \models \aformulabis_2$.
So, $\pair{\astore}{\aheap} \models \aformula$ and $\aformula$ is satisfiable.

\item[Induction step:$\aformula = \inpath{\avariable}{\avariablebis}{\avariableter} \aformulabis$]
First, suppose that  $\pair{\astore}{\aheap} \models \aformula$.
By definition of the satisfaction relation $\models$,
there is $\alocation \in \minpath{\astore(\avariable)}{\astore(\avariablebis)}{\aheap} \cup \set{\astore(\avariablebis)}$
such that $\pair{\astore[\avariableter \gets \alocation]}{\aheap} \models \aformulabis$. By 2(b), we have
$\asymbexists{\avariable}{\avariablebis}{\avariableter}(\symbms{\astore [\avariableter \gets \alocation]}{\aheap}{\asetvar \cup \set{\avariableter}}{\lfloor \frac{\bound}{2} \rfloor},
\asms)$.
By the induction hypothesis, we have  \textsc{MC}($\symbms{\astore[\avariableter \gets \alocation]}{\aheap}{\asetvar}{\lfloor \frac{\bound}{2} \rfloor}, \aformulabis$) $=$ $\mathtt{true}$.
By lines 12--14, in Algorithm~\ref{algo:symb-model-checking}, \textsc{MC}($\symbms{\astore}{\aheap}{\asetvar}{\bound}, \aformula$) $=$ $\mathtt{true}$.

Conversely, suppose that \textsc{MC}($\asms, \aformula$) $=$ $\mathtt{true}$. By lines 12--14 in Algorithm~\ref{algo:symb-model-checking},
there is a satisfiable symbolic memory state $\asms'$ over $\pair{\asetvar}{\lfloor \frac{\bound}{2} \rfloor}$
      such that ($\asymbexists{\avariable}{\avariablebis}{\avariableter}(\asms',\asms)$ and \textsc{MC}($\asms', \aformulabis$)).
As $\pair{\astore}{\aheap}$ is such that $\symbms{\astore}{\aheap}{\asetvar}{\bound} = \asms$,
by 2(a), there is $\alocation \in \minpath{\astore(\avariable)}{\astore(\avariablebis)}{\aheap} \cup \set{\astore(\avariablebis)}$
            such that $\asms' = \symbms{\astore [\avariableter \gets \alocation]}{\aheap}{\asetvar \cup \set{\avariableter}}{\lfloor \frac{\bound}{2} \rfloor}$.
By the induction hypothesis, we have $\pair{\astore[\avariableter \gets \alocation]}{\aheap} \models \aformulabis$.
Hence, by definition of $\models$, we conclude that $\pair{\astore}{\aheap} \models \aformula$.
\end{description}

\end{proof}
