# Supplementary material for: A Complete Axiomatisation for Quantifier-Free Separation Logic
Source: arXiv:2006.05156 source file (2021-08-09)
Supplement: Supplementary file 18 [file proofs-composition-sms.tex]

The following lemma guarantees that the definition for symbolic composition is indeed what we need.
\begin{restatable}{lemma}{lemmacompositionisok}\label{lemma:compositionisok}
$\asymbunion$ satisfies {\normalfont\ref{compositionproperty}}.
\end{restatable}

\begin{proof} (sketch) The proof follows a structure similar to the proof of Lemma~\ref{lemma:quantificationisok}, except that
the notion of symbolic composition is much more involved. Below, we provide the main ideas, some of them are similar to those used
for the proof of~\cite[Lemma 4.8]{Demri&Lozes&Mansutti18bis}.

For the first direction, let $\pair{\astore}{\aheap}$ be a memory state with $\aheap = \aheap_1 + \aheap_2$.
We aim at showing that
$
\symbunion{\symbms{\astore}{\aheap_1}{\asetvar}{\bound_1}}{\symbms{\astore}{\aheap_2}{\asetvar}{\bound_2}}{\symbms{\astore}{\aheap}{\asetvar}{\bound_1+\bound_2}}
$.
We should verify that  $\symbms{\astore}{\aheap_1}{\asetvar}{\bound_1}$, $\symbms{\astore}{\aheap_2}{\asetvar}{\bound_2}$ and
$\symbms{\astore}{\aheap}{\asetvar}{\bound_1+\bound_2}$ are satisfiable (obvious) and to verify the satisfaction of the conditions
\ref{C-functionality}--\ref{C-wasgarbage}. As in the first part of the proof of Lemma~\ref{lemma:quantificationisok}, checking
the satisfaction of the conditions is tedious but is not conceptually difficult as the conditions \ref{C-functionality}--\ref{C-wasgarbage}
have been precisely designed to mimick symbolically disjoint union between heaps. As in the proof of Lemma~\ref{lemma:quantificationisok},
we take also advantage of the definition of the map $\symbms{\astore}{\cdot}{\asetvar}{\cdot}$.
In short, Condition~\ref{C-functionality} holds because $\aheap_1$ and $\aheap_2$ have disjoint domains.
Condition~\ref{C-meet-points} is satisfied because when a location $\alocation$ is interpreted by a
meet-point $\ameetvar{\avariable}{\avariablebis}{\avariableter}$ in $\pair{\astore}{\aheap_i}$, taking
an extension $\aheap$ of $\aheap_i$, i.e. $\aheap_i \sqsubseteq \aheap$, entails that $\alocation$ corresponds to the interpretation
of either $\ameetvar{\avariable}{\avariablebis}{\avariableter}$ or $\ameetvar{\avariablebis}{\avariable}{\avariableter}$
in $\pair{\astore}{\aheap}$. As far as the satisfaction of~\ref{C-homomorphism} is concerned, when there is a path
between $\semantics{\aterm}_{\astore,\aheap_i}$ and  $\semantics{\aterm'}_{\astore,\aheap_i}$ in $\pair{\astore}{\aheap_i}$
without visiting other locations interpreted by terms from $\atermset{\asetvar}$, in the extended
memory state  $\pair{\astore}{\aheap}$, some of the locations of the path may correspond to
locations interpreted by terms from $\atermset{\asetvar}$ because the composition of the garbage has created
new such locations. Finally, the satisfaction of the condition~\ref{C-wasgarbage} takes care of the quantitative aspects,
for instance if the respective size of the garbage is less than that bounds $\bound_1$ and $\bound_2$ respectively,
the composition provides precise constraints. The main difficulty here rests on the fact that
the typology of locations involved in the definition of the sets $\symbsources{\asms_1}{\asms_2}{\asms}$, $\symbtargets{\asms_1}{\asms}$
and $\symbinternal{\asms_1}{\asms_2}{\asms}$ is crucial to specify how the two garbage are composed.

%% Before providing a sketch for the property~\ref{C-homomorphism}, 
Hence, the first direction has the flavour of soundness and the explanations provided in
Appendix~\ref{appendix-definition-symbolic-composition} contain the key arguments. By way of example, we show the property~\ref{C-homomorphism}.
Let $\asms_1 = \triple{\symbterms_1}{\amap_1}{\symbrem_1}$, $\asms_2 = \triple{\symbterms_2}{\amap_2}{\symbrem_2}$ and $\asms = \triple{\symbterms}{\amap}{\symbrem}$ be the three symbolic memory states
such that $\asms_1 = \symbms{\astore}{\aheap_1}{\asetvar}{\bound_1}$, $\asms_2 = \symbms{\astore}{\aheap_2}{\asetvar}{\bound_2}$ and
$\asms = \symbms{\astore}{\aheap}{\asetvar}{\bound}$
(respectively over $\pair{\asetvar}{\bound_1}$, $\pair{\asetvar}{\bound_2}$ and $\pair{\asetvar}{\bound}$).  

Each injective map $\ainj_i$ is defined such that for all $\asymbterm \in \symbterms_i$, 
we have $\semantics{\asymbterm}_{\astore,\aheap_i} = \semantics{\ainj_i(\asymbterm)}_{\astore,\aheap}$. It is possible to define $\ainj_1$ and $\ainj_2$ 
in such a way, as any location interpreted by a term in $\atermset{\asetvar}$ within $\pair{\astore}{\aheap_i}$ is also interpreted by a term in $\atermset{\asetvar}$ within $\pair{\astore}{\aheap}$
(possibly not by the same term when asymmetric meet-point terms are involved). 
Moreover, as sketched above, $\charsymbform(\asms_1)$, $\charsymbform(\asms_2)$ and $\charsymbform(\asms)$ are obviously satisfiable because the symbolic memory states
are generated from memory states  with the map $\symbms{\astore}{\cdot}{\asetvar}{\cdot}$ and Lemma~\ref{lemma:msmodelsabs} holds true. 
Let us come back now to a sketch of the proof for the satisfaction of the property~\ref{C-homomorphism}. 
First, we define the following sets of locations.
\begin{enumerate}
\item  Let $S$ be the set of locations $\alocation$ in $\semantics{\asetvar}_{\astore,\aheap}$ such that 
       within $\pair{\astore}{\aheap_1}$ and $\pair{\astore}{\aheap_2}$, the location $\alocation$ does not reach a location interpreted
by a term in $\atermset{\asetvar}$ in at least one step. One can check that $S$ is precisely equal to 
$\set{\semantics{\asymbterm}_{\astore,\aheap} \ \mid \ \asymbterm \in \symbsources{\asms_1}{\asms_2}{\asms}}$. 
\item Let $T_i$ be the set of locations $\alocation$ either in $\semantics{\asetvar}_{\astore,\aheap_i}$  or 
there are locations $\alocation_1,\alocation_2 \in \semantics{\atermset{\asetvar}}_{\astore, \aheap_i}$  such that
\begin{itemize}[nosep]
\item there is a path from $\alocation_1$ to $\alocation_2$ in $\pair{\astore}{\aheap_i}$ of length at least one and no other location in 
$\semantics{\atermset{\asetvar}}_{\astore, \aheap_i}$ occurs in the path,
\item the location $\alocation$ is on the minimal path  from $\alocation_1$ to $\alocation_2$ within $\pair{\astore}{\aheap}$ and $\alocation \in 
\semantics{\atermset{\asetvar}}_{\astore, \aheap}$.
\end{itemize}
One can check that $T_i$ is precisely equal to 
$\set{\semantics{\asymbterm}_{\astore,\aheap} \ \mid \ \asymbterm \in \symbtargets{\asms_i}{\asms}}$. 
\item Let $N$ be the set of locations $\alocation$ in $\semantics{\atermset{\asetvar}}_{\astore,\aheap}$ such that
      \begin{itemize}
      \item there is a location $\alocation'$ in $\semantics{\atermset{\asetvar}}_{\astore, \aheap}$ such that 
            there is a path from $\alocation$ to $\alocation'$ in $\pair{\astore}{\aheap}$ of length at least one and no other location in 
            $\semantics{\atermset{\asetvar}}_{\astore, \aheap}$ occurs in the path,
      \item $\alocation \not \in (T_1 \cup T_2) \setminus S$. 
      \end{itemize}
     One can check that $N$ is precisely equal to 
$\set{\semantics{\asymbterm}_{\astore,\aheap} \ \mid \ \asymbterm \in \symbinternal{\asms_1}{\asms_2}{\asms}}$. 
\end{enumerate}

Let $\aterm_1,\aterm_2 \in \atermset{\asetvar}$  and $i \in \set{1,2}$ be such that $\amap_i(\equivclass{\aterm_1}{\symbterms_i}) = (\equivclass{\aterm_2}{\symbterms_i},\inbound)$.
Let us treat the case $\inbound < \bound_i$ (the case $\inbound = \bound_i$ is similar). The minimal path from $\semantics{\aterm_1}_{\astore, \aheap_i}$ to $\semantics{\aterm_2}_{\astore, \aheap_i}$ is of the form
below:
$$
\semantics{\aterm_1}_{\astore, \aheap_i} = \alocation_0 \mapsto \alocation_1 \mapsto \cdots \mapsto \alocation_{\inbound} = \semantics{\aterm_2}_{\astore, \aheap_i}.
$$
By construction of $\amap_i$, $\set{\alocation_1, \ldots. \alocation_{\inbound-1}} \cap \semantics{\atermset{\asetvar}}_{\astore,\aheap_i} = \emptyset$. 
Let $\alocation_{u_0}, \ldots, \alocation_{u_{n+1}}$ be the maximal amount of locations from  $\alocation_0,\alocation_1, \cdots,\alocation_{\inbound}$
such that $\set{\alocation_{u_0}, \ldots, \alocation_{u_{n+1}}} \subseteq \semantics{\atermset{\asetvar}}_{\astore,\aheap}$ and $u_0 < \cdots < u_{n+1}$. 
Obviously, $u_0 = 0$, $u_{n+1} = \inbound$ and $\set{\alocation_{u_1}, \ldots, \alocation_{u_{n}}} \subseteq T_i$. 

Let $\asymbterm_{0}, \cdots, \asymbterm_{n+1}$ be in $\symbterms$ such that for all $j \in \interval{0}{n+1}$, we have
$\semantics{\asymbterm_j}_{\astore,\aheap} = \alocation_{u_j}$. 
\begin{enumerate}
\item By definition of $\ainj_i$, we have $\aterm_1 \in \ainj_i^{-1}(\asymbterm_0)$, whence $\asymbterm_0 = \equivclass{\aterm_1}{\symbterms_i}$.
      Similarly, one can show that $\asymbterm_{n+1} {=} \ainj_i(\equivclass{\aterm_2}{\symbterms_i})$, which corresponds to the satisfaction of the condition~\ref{C-homomorphism}(a).  
\item Let $j \in \interval{1}{n}$. As $\set{\alocation_j} = \semantics{\asymbterm_j}_{\astore,\aheap}$ and $\alocation_j \not \in \semantics{\atermset{\asetvar}}_{\astore,\aheap_i}$,
by definition of $\ainj_i$, we can conclude that  $\asymbterm_j \not \in \ainj_i(\symbterms_i)$. Consequently, $\asymbterm_j \not \in \range{\ainj_1} \cup \range{\ainj_2}$.
This corresponds to the satisfaction of the condition~\ref{C-homomorphism}(b).
\item Let $j \in \interval{0}{n}$. By maximality of the sequence $\alocation_{u_0}, \ldots, \alocation_{u_{n+1}}$, $\amap(\asymbterm_j) = \pair{\asymbterm_{j+1}}{\inbound_j}$
for some $\inbound_j < \inbound$ (as $\inbound < \bound$). This corresponds to the satisfaction of the condition~\ref{C-homomorphism}(c).
\item Finally, as $\inbound < \bound_i$ and $\inbound_j < \bound_i$ for each $j \in \interval{0}{n}$, we necessarily have $\inbound_0 + \cdots + \inbound_n = \inbound$,
with corresponds to the satisfaction of the condition~\ref{C-homomorphism}(d).
\end{enumerate}
The satisfaction of the other conditions is shown following a similar pattern.

For the other direction, we assume that $\symbunion{\asms_1}{\asms_2}{\symbms{\astore}{\aheap}{\asetvar}{\bound_1+\bound_2}}$ with
$\asms_1$ and $\asms_2$,
respectively over $\pair{\asetvar}{\bound_1}$ and $\pair{\asetvar}{\bound_2}$. One can show that there are
subheaps $\aheap_1$ and $\aheap_2$ such that  $\aheap = \aheap_1 + \aheap_2$,
$\asms_1 = \symbms{\astore}{\aheap_1}{\asetvar}{\bound_1}$ and $\asms_2 = \symbms{\astore}{\aheap_2}{\asetvar}{\bound_2}$.
This direction has the flavour of completeness. 
As in the proof of~\cite[Lemma 4.8]{Demri&Lozes&Mansutti18bis}, we need to construct $\aheap_1$ and $\aheap_2$ from
$\aheap$ by identifying the paths from $\aheap$ that are given to $\aheap_i$, and those that are
defined as composition of the memory cells from $\aheap_1$ and from $\aheap_2$. This is the place where
the maps $\amapbis_1,\amapbis_2: \symbinternal{\asms_1}{\asms_2}{\asms} \to \interval{1}{\bound_1 + \bound_2}$ in the condition~\ref{C-wasgarbage}
are helpful. 
%% SD 04/07/2019
%% This part will remain commented until we have to decent version
\cut{
\newpage
Suggestion for a new condition:
If ($\symbrem_1 < \bound_1$ or $\symbrem_2 < \bound_2$) and $\symbrem < \bound_1 + \bound_2$, then 
there exist $\symbrem_1', \symbrem'_2$ such that 
\begin{enumerate}
\item  $\symbrem = \symbrem_1' +\symbrem'_2$,
\item for $i \in \set{1,2}$, we have
$
\min(\symbrem'_i + \sum_{\asymbterm \in \symbinternal{\asms_1}{\asms_2}{\asms}} \amapbis_i(\asymbterm), \bound_i)
= 
\min(\symbrem_i, \bound_i)
$.
\end{enumerate}
}
By way of example, let us provide below a sketch on how to build the heaps $\aheap_1$ and $\aheap_2$. 
Let $\asms_1$, $\asms_2$ and $\asms$ be  three symbolic memory states
such that  $\asms = \triple{\symbterms}{\amap}{\symbrem}$ and $\symbunion{\asms_1}{\asms_2}{\symbms{\astore}{\aheap}{\asetvar}{\bound_1+\bound_2}}$.
We write $\asms_1 = \triple{\symbterms_1}{\amap_1}{\symbrem_1}$, 
$\asms_2 = \triple{\symbterms_2}{\amap_2}{\symbrem_2}$ and $\asms = \triple{\symbterms}{\amap}{\symbrem}$
(respectively over $\pair{\asetvar}{\bound_1}$, $\pair{\asetvar}{\bound_2}$ and $\pair{\asetvar}{\bound}$). 
The construction is rather long and can be roughly described as follows. The heaps $\aheap_1$ and $\aheap_2$ are constructed incrementally by adding memory cells
to it (starting by two heaps with empty domain). 
\begin{enumerate}
\item For each $i \in \set{1,2}$, and for all $\asymbterm \in \domain{\amap_i}$ with $\amap_i(\asymbterm) = \pair{\asymbterm'}{\inbound}$, 
      all the memory cells for the path from $\alocation$ with $\set{\alocation} = \semantics{\ainj_i(\asymbterm)}_{\astore,\aheap}$
      to  $\alocation'$ with $\set{\alocation'} = \semantics{\ainj_i(\asymbterm')}_{\astore,\aheap}$ are added to $\aheap_i$. 
      This is the easy case to distribute the memory cells, as the whole path from $\alocation$ to $\alocation'$ has to be preserved in $\aheap_i$. 
\item Let $\asymbterm$ be in $\symbinternal{\asms_1}{\asms_2}{\asms}$. As $\asymbterm$ belongs to
$\domain{\amap}$, let us say that $\amap(\asymbterm) = \pair{\asymbterm'}{\inbound}$. 
      \begin{description}
      \item[Case 1:] $\amapbis_1(\asymbterm) < \bound_1$. \\
      Pick $\amapbis_1(\asymbterm)$ memory cells contributing to the minimal path from $\alocation$ to $\alocation'$
      and assign them to $\aheap_1$. Pick the remaining memory cells
      contributing to the minimal path from $\alocation$ to $\alocation'$, and assign them to $\aheap_2$.
      \item[Case 2:] Otherwise, $\amapbis_2(\asymbterm) < \bound_2$. \\
      Pick $\amapbis_2(\asymbterm)$ memory cells contributing to the minimal path from $\alocation$ to $\alocation'$
      and assign them to $\aheap_2$. Pick the remaining memory cells
      contributing to the minimal path from $\alocation$ to $\alocation'$, and assign them to $\aheap_1$.
      \item[Case 3:] Otherwise ($\amapbis_1(\asymbterm) =  \bound_1$ and $\amapbis_2(\asymbterm) = \bound_2$). \\
      Pick $\bound_1$ memory cells contributing to the minimal path from $\alocation$ to $\alocation'$
      and assign them to $\aheap_1$. Pick the remaining memory cells
      contributing to the minimal path from $\alocation$ to $\alocation'$, and assign them to $\aheap_2$.
      \end{description}
      The condition~\ref{C-wasgarbage}(a) contributes to the correctness of the appropriateness of the heaps $\aheap_1$ and $\aheap_2$. 

      %% SD 05/07/19 GARBAGE
      \cut{
      \begin{description}
      \item[Case 1:] $\inbound < \bound_1 + \bound_2$. \\
      By definition of  $\symbms{\astore}{\cdot}{\asetvar}{\cdot}$, there are locations $\alocation$ and $\alocation'$
      such that $\semantics{\asymbterm}_{\astore, \aheap} = \set{\alocation}$, 
      $\semantics{\asymbterm'}_{\astore, \aheap} = \set{\alocation'}$, and there is a minimal 
      path from $\alocation$ to $\alocation'$
      in $\pair{\astore}{\aheap}$ of length $\inbound$. 
      By the condition~\ref{C-wasgarbage}(b), $\inbound = \amapbis_1(\asymbterm) +  \amapbis_2(\asymbterm)$. 
      Pick $\amapbis_1(\asymbterm)$ memory cells contributing to the minimal path from $\alocation$ to $\alocation'$
      and assign them to $\aheap_1$. Similarly, pick the remaining $\amapbis_2(\asymbterm)$ memory cells
      contributing to the minimal path from $\alocation$ to $\alocation'$, and assign them to $\aheap_2$.
      \item[Case 2:] $\inbound = \bound_1 + \bound_2$.\\
      Again,  there are locations $\alocation$ and $\alocation'$
      such that $\semantics{\asymbterm}_{\astore, \aheap} = \set{\alocation}$, 
      $\semantics{\asymbterm'}_{\astore, \aheap} = \set{\alocation'}$, and there is a minimal 
      path from $\alocation$ to $\alocation'$
      in $\pair{\astore}{\aheap}$ of length at least $\bound_1 + \bound_2$.
      \begin{description}
      \item[Case 2.1:] $\amapbis_1(\asymbterm) < \bound_1$. \\
      Pick $\amapbis_1(\asymbterm)$ memory cells contributing to the minimal path from $\alocation$ to $\alocation'$
      and assign them to $\aheap_1$. Pick the remaining memory cells
      contributing to the minimal path from $\alocation$ to $\alocation'$, and assign them to $\aheap_2$.
      \item[Case 2.1:] Otherwise, $\amapbis_2(\asymbterm) < \bound_2$. \\
      Pick $\amapbis_2(\asymbterm)$ memory cells contributing to the minimal path from $\alocation$ to $\alocation'$
      and assign them to $\aheap_2$. Pick the remaining memory cells
      contributing to the minimal path from $\alocation$ to $\alocation'$, and assign them to $\aheap_1$.
      \item[Case 2.2:] Otherwise ($\amapbis_1(\asymbterm) =  \bound_1$ and $\amapbis_2(\asymbterm) = \bound_2$). \\
      Pick $\bound_1$ memory cells contributing to the minimal path from $\alocation$ to $\alocation'$
      and assign them to $\aheap_1$. Pick the remaining memory cells
      contributing to the minimal path from $\alocation$ to $\alocation'$, and assign them to $\aheap_2$.
      \end{description}
      \end{description}
      }
\item Now, let us explain how to complete the garbage for $\aheap_1$ and $\aheap_2$. 
      By the condition~\ref{C-wasgarbage}, there are $\symbrem_1', \symbrem_2'$ such that
      $\symbrem = \symbrem_1' + \symbrem_2'$  and the conditions~\ref{C-wasgarbage}(a)--\ref{C-wasgarbage}(c) hold. 
      We perform a case analysis as above.
      \begin{description}
      \item[Case 1:] $\symbrem_1' < \bound_1$. \\
      Pick $\symbrem'_1$ memory cells with address in 
      $\remset{\astore,\aheap}{\atermset{\asetvar} \times \atermset{\asetvar}}$ 
      (whose cardinality is at least $\min(\symbrem'_1 + \symbrem'_2, \bound_1 + \bound_2)$ by the condition~\ref{C-wasgarbage})
      and assign them to $\aheap_1$. 
      Pick the remaining memory cells with address in 
      $\remset{\astore,\aheap}{\atermset{\asetvar} \times \atermset{\asetvar}}$ and assign them to $\aheap_2$.
      \item[Case 2:] Otherwise, $\symbrem_2' < \bound_2$. \\
      Pick $\symbrem'_2$ memory cells with address in 
      $\remset{\astore,\aheap}{\atermset{\asetvar} \times \atermset{\asetvar}}$ 
      (whose cardinality is at least $\min(\symbrem'_1 + \symbrem'_2, \bound_1 + \bound_2)$) and assign them to $\aheap_2$. 
      Pick the remaining memory cells with address in 
      $\remset{\astore,\aheap}{\atermset{\asetvar} \times \atermset{\asetvar}}$ and assign them to $\aheap_1$.
      \item[Case 3:] $\symbrem_1' = \bound_1$ and $\symbrem_2' = \bound_2$. \\
      Pick $\bound_1$ memory cells with address in 
      $\remset{\astore,\aheap}{\atermset{\asetvar} \times \atermset{\asetvar}}$ 
      (whose cardinality is at least $\bound_1 + \bound_2$) and assign them to $\aheap_1$. 
      Pick the remaining memory cells with address in 
      $\remset{\astore,\aheap}{\atermset{\asetvar} \times \atermset{\asetvar}}$ and assign them to $\aheap_2$.
      \end{description}
      The satisfaction of the condition~\ref{C-wasgarbage}(b) guarantees that 
      $$
      \min(\card{\remset{\astore,\aheap_1}{\atermset{\asetvar} \times \atermset{\asetvar}}}, \bound_1) = 
      \min(\symbrem_1, \bound_1)   \ \ \ \ \ 
      \min(\card{\remset{\astore,\aheap_2}{\atermset{\asetvar} \times \atermset{\asetvar}}}, \bound_2) = 
      \min(\symbrem_2, \bound_2).
      $$
      %% SD 05/07/2019
      %% GARBAGE Again
      \cut{
      First of all, let us consider the addition of the following condition:
      \begin{description}
      \item[\lemmalab{new}{C-new}.] If 
      %% ($\symbrem_1 < \bound_1$ or $\symbrem_2 < \bound_2$) and  
      $\symbrem < \bound_1 + \bound_2$, then  
      there exist $\symbrem_1', \symbrem'_2$ such that 
      \begin{enumerate}
      \item  $\symbrem = \symbrem_1' +\symbrem'_2$,
      \item for $i \in \set{1,2}$, we have
      $
      \min(\symbrem'_i + \sum_{\asymbterm \in \symbinternal{\asms_1}{\asms_2}{\asms}} \amapbis_i(\asymbterm), \bound_i)
      = 
      \min(\symbrem_i, \bound_i)$.
      \end{enumerate}
      \cut{
      %% Note that this also implies that $\symbrem < \bound_1 + \bound_2$ whenever 
      %% ($\symbrem_1 < \bound_1$ and $\symbrem_2 < \bound_2$). 
      So, assuming  that $\symbrem_i < \bound_i$, this means that 
      $\symbrem'_i + \sum_{\asymbterm \in \symbinternal{\asms_1}{\asms_2}{\asms}} \amapbis_i(\asymbterm) = \symbrem_i$, whence
      $ \sum_{\asymbterm \in \symbinternal{\asms_1}{\asms_2}{\asms}} \amapbis_i(\asymbterm) \leq \symbrem_i$ and 
      condition~\ref{C-wasgarbage}(a) holds. 
      Similarly, if $\symbrem_1 < \bound_1$ and $\symbrem_2 < \bound_2$,  then
      $$
      (\symbrem'_1 + \sum_{\asymbterm \in \symbinternal{\asms_1}{\asms_2}{\asms}} \amapbis_1(\asymbterm)) +
      (\symbrem'_2 + \sum_{\asymbterm \in \symbinternal{\asms_1}{\asms_2}{\asms}} \amapbis_2(\asymbterm))
      $$
      $$
      = \symbrem + \sum_{\asymbterm \in \symbinternal{\asms_1}{\asms_2}{\asms}} (\amapbis_1(\asymbterm)) +  \amapbis_2(\asymbterm))),
      $$
      which corresponds to the condition~\ref{C-stillgarbage} by using condition~\ref{C-wasgarbage}(b).
      }
      \end{description}
Now, let us explain how to complete the garbage for $\aheap_1$ and $\aheap_2$, respectively, assuming the condition~\ref{C-new}. 
\begin{description}
\item[Case 1:] ($\symbrem_1 < \bound_1$ and $\symbrem_2 < \bound_2$). \\ 
By the condition~\ref{C-stillgarbage}, $\symbrem \leq \symbrem_1 + \symbrem_2$ and 
therefore  $\symbrem < \bound_1 + \bound_2$.
By the condition~\ref{C-new}, there are $\symbrem_1', \symbrem'_2$ such that 
$\symbrem = \symbrem_1' +\symbrem'_2$ and 
for all $i \in \set{1,2}$, 
      $
      \min(\symbrem'_i + \sum_{\asymbterm \in \symbinternal{\asms_1}{\asms_2}{\asms}} \amapbis_i(\asymbterm), \bound_i)
      = 
      \min(\symbrem_i, \bound_i)$.
So, pick $\symbrem'_1$ memory cells with address in 
$\remset{\astore,\aheap}{\atermset{\asetvar} \times \atermset{\asetvar}}$ 
(whose cardinality is
$\symbrem$) and assign them to $\aheap_1$.
Pick the remaining $\symbrem'_2$ memory cells with address in 
$\remset{\astore,\aheap}{\atermset{\asetvar} \times \atermset{\asetvar}}$ and assign them to $\aheap_2$.
\item[Case 2:] Otherwise ($\symbrem_1 = \bound_1$ or $\symbrem_2 = \bound_2$).
\begin{description}
\item[Case 2.1:] $\symbrem = \bound_1 + \bound_2$ \\
If $\symbrem_1 < \bound_1$ (and therefore $\symbrem_2 = \bound_2$) then, by the condition~\ref{C-wasgarbage}(a), 
$\sum_{\asymbterm \in \symbinternal{\asms_1}{\asms_2}{\asms}} \amapbis_1(\asymbterm)$ does not exceed $\symbrem_1$.
So, pick $\symbrem_1 - \sum_{\asymbterm \in \symbinternal{\asms_1}{\asms_2}{\asms}} \amapbis_1(\asymbterm)$
memory cells with address in 
$\remset{\astore,\aheap}{\atermset{\asetvar} \times \atermset{\asetvar}}$  (whose cardinality is at least
$\bound_1 + \bound_2$)
and assign them to $\aheap_1$.
Pick the remaining memory cells with address in 
$\remset{\astore,\aheap}{\atermset{\asetvar} \times \atermset{\asetvar}}$ and assign them to $\aheap_2$.

If $\symbrem_2 < \bound_2$ (and therefore $\symbrem_1 = \bound_1$), then we perform a similar reasoning.

In the remaining case $\symbrem_1 = \bound_1$ and $\symbrem_2 = \bound_2$, 
pick $\bound_1$
memory cells with address in 
$\remset{\astore,\aheap}{\atermset{\asetvar} \times \atermset{\asetvar}}$ 
(whose cardinality is again at least
$\bound_1 + \bound_2$)
and assign them to $\aheap_1$.
Pick the remaining memory cells with address in 
$\remset{\astore,\aheap}{\atermset{\asetvar} \times \atermset{\asetvar}}$ and assign them to $\aheap_2$.

\item[Case 2.2:] $\symbrem < \bound_1 + \bound_2$ \\
By the condition~\ref{C-new}, there are $\symbrem_1', \symbrem'_2$ such that 
$\symbrem = \symbrem_1' +\symbrem'_2$ and 
for all $i \in \set{1,2}$, 
      $
      \min(\symbrem'_i + \sum_{\asymbterm \in \symbinternal{\asms_1}{\asms_2}{\asms}} \amapbis_i(\asymbterm), \bound_i)
      = 
      \min(\symbrem_i, \bound_i)$.
So, pick $\symbrem'_1$ memory cells with address in 
$\remset{\astore,\aheap}{\atermset{\asetvar} \times \atermset{\asetvar}}$ and assign them to $\aheap_1$.
Pick the remaining $\symbrem'_2$ memory cells with address in 
$\remset{\astore,\aheap}{\atermset{\asetvar} \times \atermset{\asetvar}}$ and assign them to $\aheap_2$.
\end{description}
\end{description}
}
\end{enumerate}

\end{proof}

We now show that, thanks to the property above, $\asymbunion$ correctly behaves with respect to the $\separate$ operator, as stated at the beginning of this section.

\begin{lemma}\label{lemma:CompositionVsStar}
Let $\asms_1$, $\asms_2$ and $\asms$
symbolic memory states respectively over $\pair{\asetvar}{\bound_1}$, $\pair{\asetvar}{\bound_2}$ and $\pair{\asetvar}{\bound}$ and such that $\charsymbform(\asms)$ is satisfiable.
Then,
\begin{nscenter}
$\symbunion{\asms_1}{\asms_2}{\asms}$ iff
$\models \charsymbform(\asms) \implies \charsymbform(\asms_1) \separate \charsymbform(\asms_2)$.
\end{nscenter}
\end{lemma}

\begin{proof}
For the left to right direction, suppose
$\symbunion{\asms_1}{\asms_2}{\asms}$ and $\charsymbform(\asms)$ satisfiable.
Then, let $\pair{\astore}{\aheap}$ such that $\pair{\astore}{\aheap} \models \charsymbform(\asms)$.
We prove that then $\pair{\astore}{\aheap} \models \charsymbform(\asms_1) \separate \charsymbform(\asms_2)$.
By Lemma~\ref{lemma:msmodelsabs}, $\charsymbform(\asms) = \symbms{\astore}{\aheap}{\asetvar}{\bound_1+\bound_2}$.
Then, by Lemma~\ref{lemma:compositionisok} there must exists $\aheap_1$ and $\aheap_2$ such that
\begin{itemize}
\item $\aheap = \aheap_1 + \aheap_2$;
\item $\symbms{\astore}{\aheap_1}{\asetvar}{\bound_1} = \asms_1$;
\item $\symbms{\astore}{\aheap_2}{\asetvar}{\bound_2} = \asms_2$.
\end{itemize}
Again by Lemma~\ref{lemma:msmodelsabs} we then obtain that
\begin{itemize}
\item $\pair{\astore}{\aheap_1} \models \charsymbform(\asms_1)$;
\item $\pair{\astore}{\aheap_2} \models \charsymbform(\asms_2)$.
\end{itemize}
Then, together with $\aheap = \aheap_1 + \aheap_2$, by definition of the $\separate$, we conclude
$\pair{\astore}{\aheap} \models \charsymbform(\asms_1) \separate \charsymbform(\asms_2)$.

For the right to left direction, suppose
$\models \charsymbform(\asms) \implies \charsymbform(\asms_1)\separate \charsymbform(\asms_2)$.
As $\charsymbform(\asms)$ is satisfiable by hypothesis, there is a memory state
$\pair{\astore}{\aheap} \models \charsymbform(\asms)$.
Hence, from the formula above, there are $\aheap_1$ and $\aheap_2$ such that
\begin{itemize}
\item $\aheap = \aheap_1 + \aheap_2$;
\item $\pair{\astore}{\aheap_1} \models \charsymbform(\asms_1)$;
\item $\pair{\astore}{\aheap_2} \models \charsymbform(\asms_2)$.
\end{itemize}
By Lemma~\ref{lemma:msmodelsabs} we obtain
\begin{itemize}
\item $\symbms{\astore}{\aheap}{\asetvar}{\bound_1+\bound_2} = \asms$;
\item $\symbms{\astore}{\aheap_1}{\asetvar}{\bound_1} = \asms_1$;
\item $\symbms{\astore}{\aheap_2}{\asetvar}{\bound_2} = \asms_2$.
\end{itemize}
As moreover $\aheap = \aheap_1+\aheap_2$,
by Lemma~\ref{lemma:compositionisok} we conclude: $\symbunion{\asms_1}{\asms_2}{\asms}$.
\end{proof}
