# Supplementary material for: A Complete Axiomatisation for Quantifier-Free Separation Logic
Source: arXiv:2006.05156 source file (2021-08-09)
Supplement: Supplementary file 20 [file lemma-PSLvalid.tex]

Recall that intermediate axioms, such as \ref{coreAx:AllocSize}, do not need to be proved semantically as they are provable tautologies in $\coresys(\separate,\magicwand)$.
The axioms~\ref{coreAx:EqRef},
%\ref{coreAx:EqSymm},
\ref{coreAx:PointAlloc} and \ref{coreAx:PointInj} were already discussed in the body of the paper and their validity should be straightforward.
Moreover, the validity of the axioms~\ref{starAx:Commute},~\ref{starAx:Assoc} and~\ref{starAx:False}
and the three rules (\ref{rule:starinference},~\ref{rule:staradj} and~\ref{rule:magicwandadj}) is inherited from Boolean BI 
(see~\cite{Brotherston&Villard14} and~\cite[Section 2]{Galmiche&Larchey06}).

\begin{itemize}
\item The proof of every instantiation of \ref{starAx:MonoCore} is similar (and quite easy), therefore we show just the case of $\avariable \Ipto \avariablebis \separate \true \implies \avariable \Ipto \avariablebis$.
Suppose $\pair{\astore}{\aheap} \models \avariable \Ipto \avariablebis \separate \true$. Then there is a subheap $\aheap_1 \sqsubseteq \aheap$ such that $\pair{\astore}{\aheap_1} \models \avariable \Ipto \avariablebis$.
Hence, $\aheap_1(\astore(\avariable)) = \astore(\avariablebis)$.
As $\aheap_1 \sqsubseteq \aheap$, we obtain  $\aheap(\astore(\avariable)) = \astore(\avariablebis)$ which by definition implies $\pair{\astore}{\aheap} \models \avariable \Ipto \avariablebis$.
\item \ref{starAx:AllocNeg}.
Suppose $\pair{\astore}{\aheap} \models \lnot \alloc{\avariable} \separate \lnot \alloc{\avariable}$. Then there are
two disjoint heaps $\aheap_1,\aheap_2$ such that $\aheap = \aheap_1 + \aheap_2$, $\pair{\astore}{\aheap_1} \models \lnot \alloc{\avariable}$ and $\pair{\astore}{\aheap_2} \models \lnot \alloc{\avariable}$.
Then $\astore(\avariable) \not \in \domain{\aheap_1}$ and $\astore(\avariable) \not \in \domain{\aheap_2}$.
Since $\aheap = \aheap_1 + \aheap_2$, $\domain{\aheap} = \domain{\aheap_1}\cup\domain{\aheap_2}$ and therefore
$\astore(\avariable) \not \in \domain{\aheap}$.
We conclude that $\pair{\astore}{\aheap} \models \lnot \alloc{\avariable}$.
\item \ref{starAx:PointsNeg}.
Suppose $\pair{\astore}{\aheap} \models (\alloc{\avariable} \land \lnot \avariable \Ipto \avariablebis) \separate \true$.
Then there is a subheap $\aheap_1 \sqsubseteq \aheap$ such that $\pair{\astore}{\aheap_1} \models \alloc{\avariable} \land \lnot \avariable \Ipto \avariablebis$.
Hence, $\astore(\avariable) \in \domain{\aheap_1}$ and $\aheap_1(\astore(\avariable)) \neq \astore(\avariablebis)$.
As $\aheap_1 \sqsubseteq \aheap$, we obtain  $\astore(\avariable) \in \domain{\aheap}$ and $\aheap(\astore(\avariable)) \neq \astore(\avariablebis)$ which by definition implies $\pair{\astore}{\aheap} \models \lnot \avariable \Ipto \avariablebis$.
\item \ref{starAx:AllocSizeOne}. Suppose $\pair{\astore}{\aheap} \models \alloc{\avariable}$.
Then $\astore(\avariable) \in \domain{\aheap}$. Let $\aheap_1 \egdef \{\astore(\avariable)\pto\aheap(\astore(\avariable))\}$. Trivially, $\aheap_1 \sqsubseteq \aheap$ and
$\pair{\astore}{\aheap_1} \models \alloc{\avariable} \land \size = 1$.
We define $\aheap_2$ as the heap such that $\aheap_2 + \aheap_1 = \aheap$.
Trivially, $\pair{\astore}{\aheap_2} \models \true$.
Hence, $\pair{\astore}{\aheap} \models (\alloc{\avariable} \land \size = 1) \separate \true$.

The proof of validity of \ref{starAx:SizeOne} is similar.
\item \ref{starAx:SizeNeg}.
We suppose that $\inbound_1,\inbound_2\geq 1$, as the formula $\lnot \size \geq 0$ is by definition $\lnot \true$ and therefore is unsatisfiable.
Hence, the axiom~\ref{starAx:SizeNeg} is trivially valid by the axiom~\ref{starAx:False} for $\inbound_1$ and $\inbound_2$ equal to $0$.
Suppose $\pair{\astore}{\aheap} \models \lnot \size \geq \inbound_1 \separate \lnot \size \geq \inbound_2$.
Then there are two disjoint heaps $\aheap_1,\aheap_2$ such that $\aheap_1 + \aheap_2 = \aheap$, $\pair{\astore}{\aheap_1} \models \lnot \size \geq \inbound_1$ and $\pair{\astore}{\aheap_2} \models \lnot \size \geq \inbound_2$.
Then, by definition of $\size$, $\card{\domain{\aheap_1}} \leq \inbound_1-1$ and $\card{\domain{\aheap_2}} \leq \inbound_2-1$.
Then, as $\domain{\aheap} = \domain{\aheap_1}\cup\domain{\aheap_2}$, we obtain $\card{\domain{\aheap}} \leq \inbound_1+\inbound_2-2$, which implies
$\pair{\astore}{\aheap} \models \lnot \size \geq \inbound_1+\inbound_2 \dotminus 1$.
\item \ref{starAx:SizeTwo}. Suppose $\pair{\astore}{\aheap} \models \alloc{\avariable} \land \alloc{\avariablebis} \land \avariable \neq \avariablebis$. Then 
by definition,
$\astore(\avariable) \neq \astore(\avariablebis)$ and both $\astore(\avariable)$ and $\astore(\avariablebis)$ are in $\domain{\aheap}$. Hence $\card{\domain{\aheap}} \geq 2$, which implies $\pair{\astore}{\aheap} \models \size \geq 2$.
%%
%% SD 17/02/19
%% The axioms do not seem to be there anymore.
%% 
\cut{
\item \ref{wandAx:Emp}. Suppose $\pair{\astore}{\aheap} \models \emp \magicwand \aformula$.
Then for every $\aheap'\perp\aheap$ such that $\domain{\aheap'} = \emptyset$, $\pair{\astore}{\aheap+\aheap'} \models \aformula$.
However $\aheap + \aheap' = \aheap$ as $\aheap'$ is empty and therefore $\pair{\astore}{\aheap} \models \aformula$.
\item \ref{wandAx:GroundAlloc}.
Suppose $\pair{\astore}{\aheap} \models (\alloc{\avariable} \magicwand \bottom)$. Then for every $\aheap_1\perp\aheap$ such that $\astore(\avariable) \in \domain{\aheap_1}$, $\pair{\astore}{\aheap+\aheap'} \models \bottom$.
$\bottom$ is unsatisfiable, we then deduce that the set of heaps that is dijoint from $\aheap$ and have $\astore(\avariable)$ in their domain must be empty. We then conclude that $\astore(\avariable) \in \domain{\aheap}$ and therefore $\pair{\astore}{\aheap} \models \alloc{\avariable}$.
}
\item \ref{wandAx:Size}. Let $\asetvar\subseteq_\fin\PVAR$ and  $\pair{\astore}{\aheap}$ be a memory state.
Let $\aheap_1$ be a heap of size one such that $\aheap_1(\alocation) = \alocation$ for some $\alocation \not \in \domain{\aheap}\cup\astore(\asetvar)$.
Trivially $\pair{\astore}{\aheap_1}\models \size = 1 \land \bigwedge_{\avariable \in \asetvar} \lnot \alloc{\avariable}$.
Moreover $\aheap_1\perp\aheap$ holds, hence $\aheap_1+\aheap_2$ is defined and $\pair{\astore}{\aheap+\aheap_1} \models \true$.
Then, $\pair{\astore}{\aheap} \models (\size = 1 \land \bigwedge_{\avariable \in \asetvar} \lnot \alloc{\avariable}) \septraction \true$.
\item \ref{wandAx:PointsTo}. Suppose $\pair{\astore}{\aheap} \models \lnot \alloc{\avariable}$.
Let $\aheap_1$ be the heap of size one such that $\aheap_1(\astore(\avariable)) = \astore(\avariablebis)$.
Trivially, $\pair{\astore}{\aheap} \models \avariable \Ipto \avariablebis \land \size = 1$. Moreover, as $\astore(\avariable) \not\in\domain{\aheap}$, $\aheap_1\perp\aheap$ holds, hence $\aheap_1+\aheap_2$ is defined and $\pair{\astore}{\aheap+\aheap_1} \models \true$.
Then, $\pair{\astore}{\aheap} \models (\avariable \Ipto \avariablebis \land \size=1) \septraction \true$.
\item \ref{wandAx:Alloc}. Let $\asetvar \subseteq_\fin \PVAR$ and
suppose $\pair{\astore}{\aheap} \models \lnot \alloc{\avariable}$.
Let $\aheap_1$ be the heap of size one such that $\aheap_1(\astore(\avariable)) = \alocation$ where $\alocation \not \in \astore(\asetvar)$.
Trivially, $\pair{\astore}{\aheap_1} \models \alloc{\avariable} \land \size = 1 \land \bigwedge_{\avariablebis \in \asetvar} \lnot \avariable \Ipto \avariablebis$.
Moreover, as $\astore(\avariable) \not\in\domain{\aheap}$, $\aheap_1\perp\aheap$ holds, hence $\aheap+\aheap_1$ is defined and $\pair{\astore}{\aheap+\aheap_1} \models \true$.
Then, $\pair{\astore}{\aheap} \models (\alloc{\avariable} \land \size = 1 \land \bigwedge_{\avariablebis \in \asetvar} \lnot \avariable \Ipto \avariablebis) \septraction \true$.\qedhere
\end{itemize}
