# Supplementary material for: A Complete Axiomatisation for Quantifier-Free Separation Logic
Source: arXiv:2006.05156 source file (2021-08-09)
Supplement: Supplementary file 21 [file lemma-magicwandPSLelim.tex]

\begin{proof}(of Lemma~\ref{lemma:magicwandPSLelim})

SD: This proof needs to be significantly polished and completed to be able to be followed
smoothly (existence of Lemma~\ref{lemma:septractionadmissiblebis}  could contribute to this).

If either $\aformula$ or $\aformulabis$ is unsatisfiable, then $\prove_{\magicwandsys}
\aformula\septraction\aformulabis \implies \bot$ by using Lemma~\ref{lemma:corePSLtwo}
and the admissible axioms~\ref{mwAx:ImpL} and~\ref{mwAx:ImpR} from Lemma~\ref{lemma:septractionadmissible}.
So, in that case, it is enough  to take $\aformulater$ equal to $\lnot \avariable = \avariable$. Otherwise,
let $\aformulater$ be the formula introduced in Lemma~\ref{lemma:coreformulaseptraction}.
  \begin{itemize}
  \item Let us first show that $\prove_{\magicwandsys} \aformula\septraction\aformulabis\implies\aformulater$.
   $$
   \begin{array}{l|ll}
   1 & \neg \aformulater \separate \aformula \implies \neg \aformulabis 
   & \mbox{Completeness of $\starsys$} \\
   2 & \neg \aformulater \implies (\aformula \magicwand \neg \aformulabis)
   & \mbox{\ref{rule:staradj}, 1} \\
   3 & \neg (\aformula \magicwand \neg \aformulabis) \implies \aformulater
   & \mbox{Prop. reasoning, 2} \\
   4 & (\aformula \septraction \aformulabis) \implies \aformulater
   & \mbox{Def. $\septraction$, 3} 
   \end{array}
   $$
%% SD 06/05/20 -- previous version
\cut{
    By definition of $\septraction$, 
    the formula $\aformula\septraction\aformulabis\implies\aformulater$
    is propositionnally equivalent to $\neg\aformulater\implies\aformula\magicwand\neg\aformulabis$. By the rule~\ref{rule:staradj},
    this
    formula derives from $\aformula*\neg\aformulater\implies\neg\aformulabis$,
    which is valid by Lemma~\ref{lemma:coreformulaseptraction}. 
    So $\prove_{\starsys}\aformula*\neg\aformulater\implies\neg\aformulabis$
    by Theorem~\ref{theo:starCompleteness}. Finally, by Lemma~\ref{lemma:admissible-axioms-2}, 
    $\prove_{\magicwandsys}\aformula \separate \neg\aformulater\implies\neg\aformulabis$.
}
  \item Let us now show that $\prove_{\magicwandsys} \aformulater\implies \aformula\septraction\aformulabis$.
    First, let us  note that, since $\aformulater \separate \aformula \implies \aformulabis$
    is valid (Lemma~\ref{lemma:coreformulaseptraction}),
    it is derivable in $\starsys{}$ (due to its completeness), and therefore, by the rule~\ref{rule:staradj},
    $\prove_{\magicwandsys}\aformulater\implies\aformula\magicwand\aformulabis$. From that, it follows that it is enough to show that
    $\aformulater\implies\aformula\septraction\top$ is derivable in $\magicwandsys$. Indeed,
    from $\aformulater\implies \aformula\septraction\top$ and $\aformulater\implies\aformula\magicwand\aformulabis$, we get by \ref{mwAx:Mix}
    that $\aformulater\implies\aformula\septraction\aformulabis$ is derivable too.

    Let us therefore prove that $\aformulater\implies\aformula\septraction\top$ is derivable.
    Without loss of generality, we assume that $\aformulater$ is satisfiable (otherwise, by completeness of $\starsys$, 
    $\aformulater\implies \aformula\septraction\top$ is derivable).
    This implies that $\aformula$, $\aformulabis$ and $\aformulater$ have exactly the same equalities and
    inequalities. 
    We reason by induction on the number of positive literals of the form $\alloc{\avariable}$
    occurring in $\aformula$.
    \begin{itemize}

    \item
      Assume no $\alloc{\avariable}$ occurs positively in $\aformula$. 
      The satisfiable formula $\aformula$ can be decomposed as follows
      $
      \aformula = \mathsf{UNALLOC}(\asetvar) \wedge \aformula_{\size} \wedge \aformula_{eq} \wedge \aformula_{\Ipto}
      $, 
      where
      \begin{itemize}
      \item $\mathsf{UNALLOC}(\asetvar) \egdef \bigwedge\{\neg\alloc{\avariable}\mid\avariable\in\asetvar\}$.
      \item $\aformula_{\size}$ is a satisfiable conjunction of size literals and therefore by 
       Lemma~\ref{lemma:septractionadmissiblebis}, 
        $$
        \prove_{\magicwandsys} (\mathsf{UNALLOC}(\asetvar) \land \aformula_{\size}) \septraction \true
        $$
       \item $\aformula_{eq}$ is a (satisfiable) conjunction of equalities and inequalities that occurs also
       in $\aformulabis$ and $\aformulater$. Since $\prove_{\magicwandsys} \aformulater \implies \aformula_{eq}$,
       using the admissible axioms~\ref{mwAx:SeptEq} and~\ref{mwAx:SeptIneq} as many times as 
       the number of literals in  $\aformula_{eq}$ (as well as the admissible rule~\ref{rule:imptr}), 
       we can conclude that
       $$
       \prove_{\magicwandsys} \aformulater \implies  (\mathsf{UNALLOC}(\asetvar) \land \aformula_{\size} \land \aformula_{eq}) 
       \septraction \true.
       $$
       It is worth noting that in the remaining cases below, we shall use this type of argument to deal with
       equalities and inequalities. 
       \item  $\aformula_{\Ipto}$ is a conjunction of negated literals of the form
              $\neg (\avariable \Ipto \avariable')$ with $\avariable, \avariable' \in \asetvar$. 
              By using the axiom~\ref{coreAx:PointAlloc} and propositional reasoning, we obtain
              $$
              \prove_{\magicwandsys} \mathsf{UNALLOC}(\asetvar) \implies \aformula_{\Ipto}.
              $$ 
              Using the admissible rule~\ref{mwAx:ImpL} with the above implication, we can conclude that 
       $$
       \prove_{\magicwandsys} \aformulater \implies  (\mathsf{UNALLOC}(\asetvar) \land \aformula_{\size} \land \aformula_{eq} \land
        \aformula_{\Ipto}) \septraction \true.
       $$
      \end{itemize}
%% SD 07/05/20 -- previous version. Part of the reasoning is now to be done in the proof
%% of Lemma~\label{lemma:septractionadmissiblebis}. 
\cut{
      Then, since $\aformula$ is satisfiable,
      $\aformula$ is either equivalent to $\mathsf{UNALLOC}(\asetvar)\wedge \size\geq\inbound_1$ or
      equivalent to $\mathsf{UNALLOC}(\asetvar)\wedge \size=\inbound_2$
      where $\mathsf{UNALLOC}(\asetvar) \egdef \bigwedge\{\neg\alloc{\avariable}\mid\avariable\in\asetvar\}$.
      Let $\inbound$ be either $\inbound_1+1$ or $\inbound_2$.
      Applying \ref{wandAx:Size} $\inbound$ times in conjunction with \ref{mwAx:ImpR},
      we get
      $$
      \underbrace{(\mathsf{UNALLOC}(\asetvar)\wedge\size=1) \septraction (\mathsf{UNALLOC}(\asetvar)\wedge\size=1) \septraction\ldots\septraction}_{\inbound\mbox{ times}}  \top.
      $$
      Applying~\ref{mwAx:Curry}, \ref{mwAx:ImpL} and reasoning in $\starsys{}$, we get
      $\prove_{\magicwandsys} (\mathsf{UNALLOC}(\asetvar)\wedge\size=\inbound)\septraction\top$, and finally 
      by~\ref{mwAx:ImpL} we get $\prove_{\magicwandsys} \aformula\septraction\top$.
}
      
    \item
      Assume $\alloc{\avariable}$ occurs positively in $\aformula$ together with $\avariable\Ipto\avariablebis$.
      Then, there is $\aformula'$ in $\coretype{\asetvar}{\bound}$ such that $\aformula\iff(\avariable\Ipto\avariablebis\wedge\size=1) \separate \aformula'$
      is valid (and therefore derivable in $\starsys$) and $\aformula'$ has at least one less 
      positive occurrences of literals of the form $\alloc{\avariableter}$.
      {\bf SD: If $\aformula$ contains $\size \geq \bound$, then how to guarantee that
      $\aformula'$ is a core type, as it may contain either $\size \geq \bound$ or $\size \geq \bound-1$?}
      Since $\aformulater\implies\aformula\septraction\top$ is valid ({\bf SD: why?}), so is 
      $\aformulater \separate (\avariable\Ipto\avariablebis\wedge\size=1)\implies\aformula'\septraction\top$.
      By the induction hypothesis ({\bf SD: What does it mean here? I stop updating the rest of the proof before solving 
      this.}), 
      $\aformulater \separate (\avariable\Ipto\avariablebis\wedge\size=1)\implies\aformula'\septraction\top$ is derivable.
      By definition of $\aformulater$, $\neg\alloc{\avariable}$ occurs in $\aformulater$.
      By using the axiom~\ref{wandAx:PointsTo}, we conclude
      $\prove_{\magicwandsys} \aformulater\implies(\avariable \Ipto \avariablebis \land \size = 1) \septraction \true$.
      On the other hand,
      $\aformulater\implies (\avariable \Ipto \avariablebis \land \size = 1) \magicwand \big((\avariable \Ipto \avariablebis \land \size = 1) * \aformulater\big)$
      is derivable by adjunction rule, so by \ref{mwAx:Mix},
      $$
      \aformulater\implies(\avariable \Ipto \avariablebis \land \size = 1) \septraction \big((\avariable \Ipto \avariablebis \land \size = 1) * \aformulater\big)
      $$
      is derivable. From this and $\prove_{\magicwandsys} 
      \aformulater \separate (\avariable\Ipto\avariablebis\wedge\size=1)\implies\aformula'\septraction\top$, we get by using the
      intermediate axiom~\ref{mwAx:ImpR}
      $$
      \prove_{\magicwandsys}  \aformulater\implies(\avariable \Ipto \avariablebis \land \size = 1) \septraction (\aformula'\septraction\top).
      $$
       Then, by~\ref{mwAx:Curry} and~\ref{mwAx:ImpL},  $\prove_{\magicwandsys} \aformulater\implies\aformula\septraction\top$.

    \item
      (SD: to present this derivation in the Hilberty-style)
      Assume $\alloc{\avariable}$ occurs positively in $\aformula$ but without any literal of the form $\avariable\Ipto\avariablebis$.
      Then there is $\aformula'$ in $\coretype{\asetvar}{\bound}$ such that $\aformula\iff(\alloc{\avariable}\wedge\mathsf{UNDEF}\wedge\size=1) \separate \aformula'$ is valid
      (and therefore derivable in $\starsys$),
      where $\mathsf{UNDEF}$ is $\bigwedge\{\neg\avariable\Ipto\avariablebis\mid\avariablebis\in \asetvar\}$
      and $\aformula'$ has at least one less positive occurrence of literals of the form $\alloc{\avariableter}$.
      Since $\aformulater\implies\aformula\septraction\top$ is valid ({\bf SD: why?}), so is
      $\aformulater*(\alloc{\avariable}\wedge\mathsf{UNDEF} \wedge\size=1)\implies\aformula'\septraction\top$.
      By induction hypothesis ({\bf SD: see above}), $\aformulater*(\alloc{\avariable}\wedge\mathsf{UNDEF}\wedge\size=1)\implies\aformula'\septraction\top$ is derivable.
      By definition of $\aformulater$, $\neg\alloc{\avariable}$ occurs in $\aformulater$.
      By using the axiom~\ref{wandAx:Alloc}, $\prove_{\magicwandsys} 
      \aformulater\implies(\alloc{\avariable}\wedge\mathsf{UNDEF}\land \size = 1) \septraction \true$.
      With the same reasoning as in previous item, we get
      $$
      \prove_{\magicwandsys}  \aformulater\implies(\alloc{\avariable}\wedge\mathsf{UNDEF} \land \size = 1) \septraction (\aformula'\septraction\top)
      $$
      Finally, by using the intermediate axioms~\ref{mwAx:Curry} and~\ref{mwAx:ImpL} $\prove_{\magicwandsys} 
      \aformulater\implies\aformula\septraction\top$. \qedhere
    \end{itemize}
  \end{itemize}
\end{proof}
