# Supplementary material for: A Complete Axiomatisation for Quantifier-Free Separation Logic
Source: arXiv:2006.05156 source file (2021-08-09)
Supplement: Supplementary file 22 [file lemma-starPSLelim.tex]

Let $\aformula$ and $\aformulabis$ in $\coretype{\asetvar}{\bound}$. 
Let us first treat the case where one of the two formulas is unsatisfiable.
Assume for instance that
$\aformula$ is not satisfiable. Then $\prove_{\coresys} \aformula\implies \bot$ by completeness of $\coresys$ (Lemma~\ref{prop:corePSLtwo}). By 
the rule~\ref{rule:starinference} and by the axiom~\ref{starAx:False}, we get  $\prove_{\starsys}\aformula*\aformulabis\implies\bot$.

Let us now assume that both $\aformula$ and $\aformulabis$ are satisfiable. Let $\aformulater$
be defined as
  $$
  \begin{array}{llll}
  &\bigwedge \formulasubset{\avariable \sim \avariablebis \inside \orliterals{\aformula}{\aformulabis}}{\bmat[\sim \in \{=,\neq\}]}
  & \land &
  \bigwedge \aformulasubset{\alloc{\avariable}\inside \orliterals{\aformula}{\aformulabis}}
  \\ \land &
  \bigwedge \aformulasubset{\lnot\alloc{\avariable} \inside\andliterals{\aformula}{\aformulabis}}
  & \land &
  \bigwedge \formulasubset{\lnot \avariable \Ipto \avariablebis}{\bmat[\alloc{\avariable}\land\lnot\avariable\Ipto\avariablebis\inside \orliterals{\aformula}{\aformulabis}]}
  \\ \land &
  \bigwedge \formulasubset{\avariable \neq \avariable}{\bmat[\alloc{\avariable}\inside\andliterals{\aformula}{\aformulabis}]}
  & \land & \bigwedge \formulasubset{\size\geq\inbound_1{+}\inbound_2}{\bmat[\size\geq\inbound_1\inside\aformula\\\size\geq\inbound_2\inside\aformulabis]}
  \\ \land &
  \bigwedge \aformulasubset{\avariable \Ipto \avariablebis \inside \orliterals{\aformula}{\aformulabis}}
  &\land &
  \bigwedge \formulasubset{\lnot\size\geq\inbound_1{+}\inbound_2{\dotminus}1}{\bmat[\lnot\size\geq\inbound_1\inside\aformula\\\lnot\size\geq\inbound_2\inside\aformulabis]}
  \end{array}
  $$

and let us show that $\prove_{\starsys}\aformula \separate \aformulabis\iff\aformulater$.
\begin{itemize}
\item Let us first show that $\prove_{\starsys}\aformula \separate \aformulabis\implies\aformulater$.
  We show that for any literal $\aliteral$ of $\aformulater$, $\prove_{\starsys}\aformula \separate \aformulabis\implies \aliteral$. We reason by a case analysis on $\aliteral$.

  \begin{itemize}
  \item
    All equalities and inequalities that occur in $\aformula$ or $\aformulabis$,
    and all literals of the
  form $\avariable\Ipto\avariablebis$ that occur in $\aformulater$ follow from the
rule~\ref{rule:starinference} and
  the axiom~\ref{starAx:MonoCore}.
   \item Assume there is a literal $\avariable\neq\avariable$ that occurs in $\aformulater$.
     This is necessarily due to $\alloc{\avariable}$ occurring both in $\aformula$ and
     $\aformulabis$. Then $\bot$ follows from the rule~\ref{rule:starinference}
     and the axiom~\ref{starAx:DoubleAlloc}.
  \item
  All literals of the form $\alloc{\avariable}$ follow from
  the rule~\ref{rule:starinference} and the axiom~\ref{starAx:StarAlloc}.
  \item
  All literals of the form $\neg\alloc{\avariable}$ 
  follow from the rule~\ref{rule:starinference} and the axiom~\ref{starAx:AllocNeg}.
  \item
    Let $\neg\avariable\Ipto\avariablebis$ be a literal occurring in $\aformulater$
    be fixed. Then $\alloc{\avariable}\wedge\neg\avariable\Ipto\avariablebis$ occurs either in
    $\aformula$ or $\aformulabis$. By the rule~\ref{rule:starinference} (and possibly by $\separate$-commutativity, see the axiom~\ref{starAx:Commute}), we get
    $
    \prove_{\starsys} \aformula \separate \aformulabis\implies (\alloc{\avariable}\wedge\neg\avariable\Ipto\avariablebis) \separate \top
    $
    and by the axiom~\ref{starAx:PointsNeg} and classical reasoning we finally get
    $
    \prove_{\starsys} \aformula \separate \aformulabis\implies \neg\avariable\Ipto\avariablebis
    $.
  \item
    Let a literal of the form $\size\geq \inbound_1+\inbound_2$
    occurring in $\aformulater$
    be fixed. Then $\size\geq\inbound_1'$ occurs in $\aformula$ and
    $\size\geq\inbound_2'$ occurs in $\aformulabis$ with $\inbound_1+\inbound_2 = \inbound_1'+\inbound_2'$. 
     By the rule~\ref{rule:starinference}
    $
    \prove_{\starsys} \aformula * \aformulabis\implies \size\geq \inbound_1' \separate \size\geq\inbound_2' 
    $;
    but then, by definition of
    $\size\geq \inbound$, we get 
    $
    \prove_{\starsys} \aformula*\aformulabis\implies \size\geq \inbound_1+\inbound_2    
    $
    
  \item
    Let a literal of the form $\neg (\size\geq \inbound_1+\inbound_2 \dotminus 1)$
    occurring in $\aformulater$
    be fixed. Then
    $\neg(\size\geq\inbound_1')$ occurs in $\aformula$ and
    $\neg(\size\geq\inbound_2')$ occurs in $\aformulabis$ with $\inbound_1+\inbound_2 = \inbound_1'+\inbound_2'$.
    By rule~\ref{rule:starinference},
    $
    \prove_{\starsys} \aformula*\aformulabis\implies \big(\neg (\size\geq \inbound_1')\big)*\big(\neg(\size\geq\inbound_2')\big)    
    $ ;
    but then by the axiom~\ref{starAx:SizeNeg}, 
    $
    \prove_{\starsys} \aformula*\aformulabis\implies \neg (\size\geq \inbound_1+\inbound_2 \dotminus 1).    
    $
    \end{itemize}
  
\item
   Let us now show that $\prove_{\starsys}\aformulater\implies\aformula*\aformulabis$.
   If there is an equality literal $\avariable=\avariablebis$
   that occurs positively in $\aformula$ and negatively in $\aformulabis$, then both
   occur in $\aformulater$, therefore $\prove_{\starsys}\aformulater\implies\bot$
   and $\prove_{\starsys}\aformulater\implies\aformula*\aformulabis$ by classical reasoning.
   Let us therefore assume that $\aformula$ and $\aformulabis$ contain exactly
   the same (in)equalities. Since $\aformula$ is satisfiable, these equalities
   define an equivalence relation.
   Let $\avariable_1,\ldots\avariable_n,\avariablebis_1,\ldots\avariablebis_m$ be an enumeration of representatives of the
   equivalence classes (one per equivalence class) such that $\alloc{\avariable_i}$ occurs in $\aformulater$.
   Applying the same reasoning as in the proof of Proposition~\ref{prop:admissible-axioms-1},
   we deduce from $\aformulater$
   $$
   \big(\alloc{\avariable_1}\wedge\size=1\big)*\cdots *
   \big(\alloc{\avariable_n}\wedge\size=1\big)*\top
   $$
   The rest of the proof is split in three big steps : (1) isolating allocated cells and garbage, (2) splitting them according to the goal $\aformula*\aformulabis$,
   (3) adding missing literals.
   \begin{enumerate}

   \item
   Let $\mathsf{ALLOC} = \big(\alloc{\avariable_1}\wedge\size=1\big) \separate \cdots \separate \big(\alloc{\avariable_n}\wedge\size=1\big)$
   and let $\mathsf{GARB} = \bigwedge\{\size\geq \inbound -n\mid\size\geq\inbound\in\literals{\aformulater}\}\wedge\bigwedge\{\neg (\size\geq \inbound -n)\mid\neg(\size\geq\inbound)\in\literals{\aformulater}\}$.
   We want to show that $\prove_{\starsys}\aformulater\implies\mathsf{ALLOC} * \mathsf{GARB}$.
   We proceed by showing that 
   $$
   \prove_{\starsys}\big(\aformulater \wedge (\mathsf{ALLOC}*\aformula_{g})\big)\implies \big(\mathsf{ALLOC}*(\aformula_{g}\wedge\aliteral)\big)
   $$
   where
   $\aliteral$ is any literal of $\mathsf{GARB}$, and $\aformula_{g}$ is any formula. Applying this reasoning
   iteratively on all $\aliteral$ of $\mathsf{GARB}$, we will reach our goal.
   There are two cases:
   \begin{itemize}
   \item $\aliteral$ is a literal $\size\geq \inbound-n$.
   From $\mathsf{ALLOC}*\aformula_{g}$, the rule~\ref{rule:starinference} and the axiom~\ref{starAx:DistrOr} we get
   $\big(\mathsf{ALLOC}*(\aformula_{g}\wedge \aliteral)\big)\vee\big(\mathsf{ALLOC}*(\aformula_{g}\wedge \neg\aliteral)\big)$. So by classical reasoning
   we resume to show that 
   $\mathsf{ALLOC} * \neg (\size\geq \inbound - n)$ implies $\bot$. By $*$ introduction and \ref{starAx:SizeNeg}
   we get $\neg \size\geq \inbound$. By definition of $\mathsf{GARB}$, $\size\geq\inbound$ occurs in $\aformulater$, so
   we get a contradiction.
   \item
   $\aliteral$ is a literal $\neg \size\geq \inbound-n$. Similarly,
   let us derive a contradiction from $\mathsf{ALLOC} \separate \size\geq \inbound - n$. By $*$ introduction and by definition of $\size\geq \inbound$,
   we get $\size\geq \inbound$, which contradicts $\neg \size\geq\inbound$ occurring in $\aformulater$.
   \end{itemize}

   \item Therefore, we  proved that $\prove_{\starsys}\aformulater\implies\mathsf{ALLOC} * \mathsf{GARB}$.
   If there is a formula $\alloc{\avariable_i}$ ocurring both in $\aformula$ and $\aformulabis$, then
   $\avariable_i\neq\avariable_i$ occurs in $\aformulater$ by definition of $\aformulater$, therefore $\aformulater\implies\aformula*\aformulabis$.
   We can thus assume that the set of variables $\avariable_1,\dots,\avariable_n$ can be split into two subsets, the one ``allocated''
   in $\aformula$, and the others in $\aformulabis$. Let $n_\aformula$ denote the number
   of equivalence classes allocated in $\aformula$, and let
   $$
   \begin{array}{lcl}
    \mathsf{ALLOC}(\aformula) & = &\circledast\{\alloc{\avariable_i}\wedge\size=1\mid\alloc{\avariable_i}\in\literals{\aformula}\}\\
    \mathsf{GARB}(\aformula) & = & \bigwedge\{\size\geq \inbound -n_\aformula\mid\size\geq\inbound\in\literals{\aformula}\}\\ & \wedge & \bigwedge\{\neg (\size\geq \inbound -n_\aformula)\mid\neg(\size\geq\inbound)\in\literals{\aformula}\}
    \end{array}               
    $$
    and let  $\mathsf{ALLOC}(\aformulabis)$ and $\mathsf{GARB}(\aformulabis)$ be defined accordingly.
   By definition of $\aformulater$, $\mathsf{GARB}\implies\mathsf{GARB}(\aformula) * \mathsf{GARB}(\aformulabis)$, and therefore
   $$
   \prove_{\starsys}\aformulater\implies \mathsf{ALLOC}(\aformula) *\mathsf{ALLOC}(\aformulabis) * \mathsf{GARB}(\aformula) * \mathsf{GARB}(\aformulabis)
   $$
   Let 
    $$
    \aformula^{(1)} =   \bigwedge_{\alloc{\avariable_i}\in\literals{\aformula}} \alloc{\avariable_i}\wedge
   \bigwedge_{\size\geq \inbound\in\literals{\aformula}}\size\geq\inbound\wedge
   \bigwedge_{\neg\size\geq \inbound\in\literals{\aformula}}\neg\size\geq\inbound
   $$
    and let $\aformulabis^{(1)}$ be defined accordingly.

   By the axioms~\ref{starAx:StarAlloc},~\ref{starAx:MonoCore},~\ref{starAx:SizeOne},~\ref{starAx:SizeNeg},~\ref{starAx:SizeTwo}, and the 
   rule~\ref{rule:starinference},
   we get
   $$
   \prove_{\starsys} \aformulater\implies\aformula^{(1)}*\aformulabis^{(1)}.
   $$

   \item We now need to add to the conjunct $\aformula^{(1)}$ all missing literals from $\aformula$, and similarly for
   $\aformulabis^{(1)}$. We add these literals iteratively, changing progressively $\aformula^{(1)}$ into $\aformula$.
   So at the $n$th step of the completion, we proved that $\prove_{\starsys}\aformulater \implies\aformula^{(n)}*\aformulabis^{(n)}$
   where $\aformula^{(n)}$ is of the form $\aformula^{(1)}\wedge\aliteral_1\wedge\ldots\wedge\aliteral_{s_n}$ and similarly for $\aformulabis^{(n)}$.
   Let $\aliteral$ be literal of $\aformula$ that does not occur yet in $\aformula^{(n)}$. We reason by a case analysis on $\aliteral$
   \begin{itemize}

   \item $\aliteral$ is an (in)equality : assuming by absurd $(\aformula^{(n)}\wedge\neg\aliteral)*\aformulabis^{(n)}$ we get by the axiom~\ref{starAx:MonoCore}
   and the rule~\ref{rule:starinference},  $\neg \aliteral$; by definition of $\aformulater$, $\aliteral$ occurs in $\aformulater$, whence the contradiction.

   \item $\aliteral$ is of the form $\alloc{\avariable}$ : then by construction of $\aformula^{(1)}$
   there is a variable $\avariable_i$ such that $\alloc{\avariable_i}$ occurs
   in $\aformula^{(n)}$ and $\avariable=\avariable_i$ occurs in $\aformulater$. We can therefore apply the axiom~\ref{coreAx:EqSub}.

   \item $\aliteral$ is of the form $\neg\alloc{\avariable}$. There are two subcases :
       \begin{itemize}
       \item
       $\alloc{\avariable}$ is a literal of $\aformulabis$. Then we derive a contradiction from
       $(\aformula^{(n)}\wedge\alloc{\avariable}) \separate \aformulabis$ by the axiom~\ref{starAx:DoubleAlloc}.
       \item
       $\neg \alloc{\avariable}$ is a literal of $\aformulabis$. Then by definition of $\aformulater$,
       $\neg \alloc{\avariable}$ is a literal of $\aformulater$.  We derive a contradiction from
       $(\aformula^{(n)}\wedge\alloc{\avariable}) \separate \aformulabis$ by the axiom~\ref{starAx:MonoCore}.
       \end{itemize}
   \item $\aliteral$ is of the form $\avariable\Ipto\avariablebis$.
   Then $\avariable\Ipto\avariablebis$ is a literal of
   $\aformulater$. Since $\aformula$ is satisfiable, $\alloc{\avariable}$ is a literal of $\aformula$.
   By construction of $\aformula^{(1)}$, there is $\avariable_i$ such that $\alloc{\avariable_i}$ occurs in $\aformula^{(1)}$ and
   $\avariable=\avariable_i$ is a literal of $\aformulater$. So $\aformulater\implies(\aformula^{(n)}\wedge\alloc{\avariable})*\aformulabis^{(n)}$.
   Assuming by absurd $\aformula^{(n)}\wedge\alloc{\avariable}\wedge\neg\avariable\Ipto\avariablebis)*\aformulabis^{(n)}$, we get
   by the axiom~\ref{starAx:PointsNeg} $\neg\avariable\Ipto\avariablebis$, and a contradiction with $\avariable\Ipto\avariablebis$ occuring in $\aformulater$.

   \item $\aliteral$ is of the form $\neg \avariable\Ipto\avariablebis$. There are three subcases:
         \begin{itemize}
         \item $\neg\alloc{\avariable}$ occurs in $\aformula$. Following the same argument as above, we can assume that $\neg\alloc{\avariable}$ occurs
         in $\aformula^{(n)}$. Assuming by absurd $(\aformula^{(n)}\wedge\avariable\Ipto\avariablebis)*\aformulabis^{(n)}$, we get a contradiction 
         by
         the axioms~\ref{coreAx:PointAlloc} and~\ref{starAx:False}.
         \item $\alloc{\avariable}$ occurs both in $\aformula$ and $\aformulabis$. Then $\avariable\neq\avariable$ occurs in $\aformulater$, so
         $\aformulater\implies\aformula*\aformulabis$
         \item $\alloc{\avariable}$ occurs in $\aformula$ but not in $\aformulabis$. Since $\aformulabis$ is satisfiable, $\neg\avariable\Ipto\avariablebis$
         occurs in $\aformulabis$, therefore $\neg\avariable\Ipto\avariablebis$ is a literal of $\aformulater$.
         Assuming by absurd $(\aformula^{(n)}\wedge\avariable\Ipto\avariablebis)*\aformulabis^{(n)}$, we get $\avariable\Ipto\avariablebis$ 
         by
         the axiom~\ref{starAx:MonoCore}, and the contradiction with $\aformulater$.
         \end{itemize}        
   \end{itemize}
\end{enumerate}       
\end{itemize}
