# Supplementary material for: A Complete Axiomatisation for Quantifier-Free Separation Logic
Source: arXiv:2006.05156 source file (2021-08-09)
Supplement: Supplementary file 23 [file proof-corePSLtwo.tex]

\propcorePSLtwo*

\begin{proof}
We show that $\aformula$ is unsatisfiable if and only if $\vdash_{\coresys}\aformula\implies\bot$.
The ``only if'' part follows from the soundness of $\coresys$, so we just sketch the proof of the ``if'' part.
Let $\aformula\in \coretype{\asetvar}{\bound}$ be fixed such that $\not\vdash_{\coresys}\aformula\Rightarrow \bot$, and let us prove that
$\aformula$ is satisfiable.
By the axioms~\ref{coreAx:EqRef}
%,$\ref{coreAx:EqSymm}$,
and~\ref{coreAx:EqSub},
there is an equivalence relation $\approx$ on $\asetvar$ such that
$\avariable\approx\avariablebis$ iff $\avariable=\avariablebis$ occurs positively
in $\aformula$. We write $[\avariable]$ to denote the equivalence class of $\avariable$
with respect to $\approx$.
By the axioms $\ref{coreAx:EqSub}$, $\ref{coreAx:PointInj}$,
there is a partial map $f: (\asetvar/\approx)\to(\asetvar/\approx)$ on equivalence classes such
that $\avariable\Ipto \avariablebis$ occurs positively iff $f([x])$ is defined and $f([x])=[y]$.
Let $D=\{[\avariable]\mid \alloc{\avariable}\mbox{ occurs positively in }\aformula\}$.
By the axiom $\ref{coreAx:PointAlloc}$, $\mathsf{dom}(f)\subseteq D$.
Let $n$ be the greatest $\beta$ such that $\size\geq\beta$ occurs positively in $\aformula$.
By the axiom~\ref{coreAx:AllocSize}, $n\geq \card{D}$.
Let $\alocation_0,\alocation_1,\dots,\alocation_n\in\LOC$ be $n+1$ distinct locations, and let
us fix an enumeration $C_1,\dots,C_{\card{D}}$ on the equivalence classes of $\approx$.
Let $(\astore,\aheap)$ be defined by
\begin{itemize}
\item $\astore(\avariable)=\alocation_i$ if $[x]$ is the $i$th equivalence class,
\item $\aheap(\alocation_i)=\alocation_j$ if $0<i\leq \card{D}$ and the $i$th equivalence class is mapped to the $j$th
one by $f$,
\item $\aheap(\alocation_i)=\alocation_0$ if either $0<i\leq \card{D}$ and the $i$th equivalence class is not in the domain of $f$, or $i> \card{D}$.
\end{itemize}
Then, by construction, $\pair{\astore}{\aheap}$ satisfies all positive literals of the form $\avariable=\avariablebis$ or $\avariable\Ipto\avariablebis$ or $\alloc{\avariable}$
that occur positively in $\aformula$, and all negative literals of the same form that occur negatively in $\aformula$. It also
satisfies $\size\geq n$, falsifies $\size\geq n+1$ (assuming $n+1 \leq \bound$), and by thr axiom~\ref{coreAx:Size}, it satisfies all size literals
in $\aformula$.
\end{proof}
