# Supplementary material for: A Complete Axiomatisation for Quantifier-Free Separation Logic
Source: arXiv:2006.05156 source file (2021-08-09)
Supplement: Supplementary file 24 [file proof-lemma-quantificationisok.tex]

\begin{proof} 
First, assume that $\minpath{\astore(\avariable)}{\astore(\avariablebis)}{\aheap} \neq \emptyset$ and
there is $\alocation \in \minpath{\astore(\avariable)}{\astore(\avariablebis)}{\aheap}\cup\{\astore(\avariablebis)\}$ such that 
$\symbms{\astore[\avariableter \gets \alocation]}{\aheap}{\asetvar\cup\{\avariableter\}}{\bound} = \triple{\symbterms}{\amap}{\symbrem}$.
Let us show that $\symbexists{\triple{\symbterms}{\amap}{\symbrem}}{\symbms{\astore}{\aheap}{\asetvar}{2\bound+b}}{\avariable}{\avariablebis}{\avariableter}$.
Let us verify the satisfaction of the conditions \ref{E-satisfiability}--\ref{E-new-location}.

Before checking the satisfaction of \ref{E-satisfiability}--\ref{E-new-location}, let us recall what are
$\triple{\symbterms}{\amap}{\symbrem}$ and $\triple{\symbterms'}{\amap'}{\symbrem'} = \symbms{\astore}{\aheap}{\asetvar}{2\bound+b}$.
Let us start by the definition of  $\triple{\symbterms'}{\amap'}{\symbrem'}$.
\begin{itemize}
\item $\symbterms' = \{ \{ \aterm_1 \in \atermset{\asetvar} \mid \pair{\astore}{\aheap} \models \aterm_1 = \aterm_2 \} \mid \aterm_2 \in \atermset{\asetvar} \}$;
\item $\amap'(\asymbterm) = (\asymbterm',\inbound)$ $\equivdef$ there are $\aterm_1 {\in} \asymbterm$ and $\aterm_2 {\in} \asymbterm'$ such that $\pair{\astore}{\aheap} \models \seesgeq{\aterm_1}{\aterm_2}{\atermset{\asetvar}}{\inbound}$ and if $\inbound < 2\bound+b$ then
$\pair{\astore}{\aheap} \models \lnot \seesgeq{\aterm_1}{\aterm_2}{\atermset{\asetvar}}{\inbound{+}1}$;
\item $\symbrem' = \inbound$ $\equivdef$ $\pair{\astore}{\aheap} \models \remgeq{\atermset{\asetvar}\times\atermset{\asetvar}}{\inbound}$ and 
if $\inbound < 2\bound +b$ then
$\pair{\astore}{\aheap} \models \lnot\remgeq{\atermset{\asetvar}\times\atermset{\asetvar}}{\inbound{+}1}$.
\end{itemize}
Here is the definition for $\triple{\symbterms}{\amap}{\symbrem}$:
\begin{itemize}
\item $\symbterms \egdef \{ \{ \aterm_1 \in \atermset{\asetvar \cup\{\avariableter\}} \mid \pair{\astore[\avariableter \gets \alocation]}{\aheap} \models 
\aterm_1 = \aterm_2 \} \mid \aterm_2 \in \atermset{\asetvar \cup\{\avariableter\}} \}$;
\item $\amap(\asymbterm) = (\asymbterm',\inbound)$ $\equivdef$ there are $\aterm_1 {\in} \asymbterm$ and $\aterm_2 {\in} \asymbterm'$ such that 
$\pair{\astore[\avariableter \gets \alocation]}{\aheap} \models \seesgeq{\aterm_1}{\aterm_2}{\atermset{\asetvar\cup\set{\avariableter}}}{\inbound}$ and 
if $\inbound < \bound$ then
$\pair{\astore[\avariableter \gets \alocation]}{\aheap} \models \lnot \seesgeq{\aterm_1}{\aterm_2}{\atermset{\asetvar\cup\set{\avariableter}}}{\inbound{+}1}$;
\item $\symbrem = \inbound$ $\equivdef$ $\pair{\astore[\avariableter \gets \alocation]}{\aheap} \models 
\remgeq{\atermset{\asetvar \cup\set{\avariableter}}\times\atermset{\asetvar\cup\set{\avariableter}}}{\inbound}$ and if $\inbound < \bound$ then
$\pair{\astore[\avariableter \gets \alocation]}{\aheap} \models 
\lnot \remgeq{\atermset{\asetvar\cup\set{\avariableter}}\times\atermset{\asetvar\cup\set{\avariableter}}}{\inbound{+}1}$.
\end{itemize}
The satisfaction of \ref{E-satisfiability} is obvious whereas the satisfaction of~\ref{E-garbage}
follows from the fact that 
$$
\remset{\astore[\avariableter \gets \alocation],\aheap}{\atermset{\asetvar\cup\set{\avariableter}}\times\atermset{\asetvar\cup\set{\avariableter}}} = \remset{\astore,\aheap}{\atermset{\asetvar}\times\atermset{\asetvar}}.
$$
Indeed, as  $\minpath{\astore(\avariable)}{\astore(\avariablebis)}{\aheap} \neq \emptyset$
and $\alocation \in \minpath{\astore(\avariable)}{\astore(\avariablebis)}{\aheap}\cup\{\astore(\avariablebis)\}$, 
the new value of $\avariableter$ in $\pair{\astore[\avariableter \gets \alocation]}{\aheap}$ does not change the memory cells
in the garbage with respect to 
$\atermset{\asetvar\cup\set{\avariableter}}\times\atermset{\asetvar\cup\set{\avariableter}} \ni \pair{\avariable}{\avariablebis}$.
Let us check the remaining conditions.

\begin{description}
\itemsep 0 cm 
\item[\ref{E-placement}] As $\alocation \in \minpath{\astore(\avariable)}{\astore(\avariablebis)}{\aheap}\cup\{\astore(\avariablebis)\}$, there is a minimal
path of length at least one in $\pair{\astore[\avariableter \gets \alocation]}{\aheap}$ of the form below:
$$
\semantics{\avariable}_{\astore,\aheap} = \semantics{\avariable}_{\astore[\avariableter \gets \alocation],\aheap} = \alocation_0 \mapsto
\alocation_1 \mapsto \cdots \mapsto \alocation_N = \semantics{\avariablebis}_{\astore,\aheap} = \semantics{\avariablebis}_{\astore[\avariableter \gets \alocation],\aheap}
$$
such that:
\begin{enumerate}
\item There are $0 = n_1 < \cdots < n_{\gamma} = N$ ($\gamma \geq 2$) such that $\alocation_{n_1}, \ldots, \alocation_{n_{\gamma}}$
are the only locations in $\set{\alocation_0, \ldots, \alocation_N}$ belonging to 
$\semantics{\atermset{\asetvar\cup\set{\avariableter}}}_{\astore[\avariableter \gets \alocation],\aheap}$.
\item There is some $\gamma' \in \interval{1}{\gamma}$ such that $\alocation_{n_{\gamma'}} = \alocation$ (indeed $\avariableter \in \atermset{\asetvar\cup\set{\avariableter}}$). 
Consequently, 
$$\set{\semantics{\avariable}_{\astore[\avariableter \gets \alocation],\aheap}, \semantics{\avariablebis}_{\astore[\avariableter \gets \alocation],\aheap},
\semantics{\avariableter}_{\astore[\avariableter \gets \alocation],\aheap}} \subseteq \set{\alocation_0, \ldots, \alocation_N}.
$$
\end{enumerate}
For every $i \in \interval{1}{\gamma}$, let $\asymbterm_i = \set{\aterm \in \atermset{\asetvar\cup\set{\avariableter}} \mid 
\semantics{\aterm}_{\astore[\avariableter \gets \alocation],\aheap} = \alocation_{n_i}}$. By definition of $n_i$, $\asymbterm_i$ is non-empty. Therefore,
by definition of $\triple{\symbterms}{\amap}{\symbrem}$ above, 
the following conditions hold:
\begin{enumerate}
\item for every $j \in \interval{1}{\gamma-1}$, $(\pi_1 \circ \amap)(\asymbterm_j) = \asymbterm_{j+1}$;
\item $\avariableter \in  \bigcup_{j \in \interval{1}{\gamma}}\asymbterm_j$, and $\avariablebis \not \in \bigcup_{j \in \interval{1}{\gamma-1}}\asymbterm_j$.
\end{enumerate} 
This concludes the verification for the condition~\ref{E-placement}. 
\item[\ref{E-no-new-location}] Assume that there is $\aterm \in \equivclass{\avariableter}{\symbterms}$
such that $\avariableter \not \in \chars{\aterm}$. Hence $\aterm \in \atermset{\asetvar}$ and therefore
for every $\asymbterm' \in \symbterms'$, there is  some $\asymbterm \in \symbterms$ such that
$\semantics{\asymbterm'}_{\astore,\aheap} = \semantics{\asymbterm}_{\astore[\avariableter \gets \alocation],\aheap}$
(note that $\semantics{\asymbterm'}_{\astore,\aheap}$ is  a singleton set).
Typically, no new location in the memory state $\pair{\astore[\avariableter \gets \alocation]}{\aheap}$ is interpreted
by a term from $\atermset{\asetvar \cup \set{\avariableter}}  \setminus \atermset{\asetvar}$.
Similarly, for every $\asymbterm \in \symbterms$, there is $\asymbterm' \in \symbterms'$ such that
$\semantics{\asymbterm'}_{\astore,\aheap} = \semantics{\asymbterm}_{\astore[\avariableter \gets \alocation],\aheap}$.
Actually, $\asymbterm'$ can be simply defined as $\asymbterm \cap \atermset{\asetvar}$ 
and therefore $\asymbterm' \subseteq \asymbterm$.  Let $\amapbis: \symbterms \to \symbterms'$ be the map
such that $\amapbis(\asymbterm) \egdef \asymbterm \cap \atermset{\asetvar}$. From the above observations, we can make the following conclusions.
\begin{itemize}
\item $\amapbis$ is a bijection.
\item For every $\asymbterm \in \symbterms$, $\amapbis(\asymbterm) \subseteq \asymbterm$.
\item Suppose that $\amap(\asymbterm_1) = \pair{\asymbterm_2}{\inbound}$.
      As no new location in the memory state $\pair{\astore[\avariableter \gets \alocation]}{\aheap}$ is interpreted
by a term from $\atermset{\asetvar} \cup \set{\avariableter} \setminus \atermset{\asetvar}$,
      we have $\amap'(\amapbis(\asymbterm_1)) = \pair{\amapbis(\asymbterm_2)}{\inbound'}$ for some $\inbound' \in \interval{1}{2 \bound + b}$.
      When $\inbound' < \bound$, again, as there is no new location  interpreted
by a term from $\atermset{\asetvar \cup \set{\avariableter}}  \setminus \atermset{\asetvar}$,
      we can conclude that $\inbound = \inbound'$. 
\item Finally, suppose that $\amap'(\amapbis(\asymbterm_1)) = \pair{\amapbis(\asymbterm_2)}{\inbound'}$
      and $\inbound = \inbound'$ if $\inbound' < \bound$, otherwise $\inbound = \bound$. As above, 
      no new location in the memory state $\pair{\astore[\avariableter \gets \alocation]}{\aheap}$ is interpreted
by a term from $\atermset{\asetvar} \cup \set{\avariableter} \setminus \atermset{\asetvar}$ and therefore we have 
$\amap(\asymbterm_1) = \pair{\asymbterm_2}{\inbound}$.
\end{itemize}
\item[\ref{E-new-location}] Contrary to the previous condition, assume that there is no 
 $\aterm \in \equivclass{\avariableter}{\symbterms}$
such that $\avariableter \not \in \chars{\aterm}$. Consequently, $\asymbterm_{\gamma'-1} \cap \atermset{\asetvar} \neq \emptyset$,
$\asymbterm_{\gamma'+1} \cap \atermset{\asetvar} \neq \emptyset$ and $\avariableter \in \asymbterm_{\gamma'} = \equivclass{\avariableter}{\symbterms}$. 
Let $\amapbis: (\symbterms \setminus \set{\equivclass{\avariableter}{\symbterms}}) \rightarrow \symbterms'$ be the map
such that $\amapbis(\asymbterm) \egdef \asymbterm \cap \atermset{\asetvar}$. Observe that by assumption, $\equivclass{\avariableter}{\symbterms} \cap
\atermset{\asetvar} = \emptyset$. Hence, the only new location in $\pair{\astore[\avariableter \gets \alocation]}{\aheap}$  interpreted
by a term from $\atermset{\asetvar \cup \set{\avariableter}}  \setminus \atermset{\asetvar}$ is precisely $\alocation$.
From the above observations, we can make the following conclusions.
\begin{enumerate}
\item $\amapbis$ is a bijection and for every $\asymbterm \in \symbterms$, $\amapbis(\asymbterm) \subseteq \asymbterm$.
\item Suppose that $\amap(\asymbterm_1) = \pair{\asymbterm_2}{\inbound}$ with $\asymbterm_1, \asymbterm_2 \in 
\symbterms \setminus \set{\equivclass{\avariableter}{\symbterms}}$. As $\alocation$ is the only location
in $\semantics{\atermset{\asetvar} \cup \set{\avariableter}}_{\astore[\avariableter \gets \alocation],\aheap} \setminus 
\semantics{\atermset{\asetvar}}_{\astore,\aheap}$, 
 we have $\amap'(\amapbis(\asymbterm_1)) = \pair{\amapbis(\asymbterm_2)}{\inbound'}$ for some $\inbound' \in \interval{1}{2 \bound+b}$.
      When $\inbound' < \bound$, again, as there is no new location  interpreted
by a term from $\atermset{\asetvar \cup \set{\avariableter}} \setminus \atermset{\asetvar}$,
      we can conclude that $\inbound = \inbound'$. 
\item Suppose that $\amap(\asymbterm_1) = \pair{\equivclass{\avariableter}{\symbterms}}{\inbound_1}$ and
$\amap(\equivclass{\avariableter}{\symbterms}) = \pair{\asymbterm_2}{\inbound_2}$. Necessarily, $\asymbterm_1 = \asymbterm_{\gamma'-1}$
and $\asymbterm_2 = \asymbterm_{\gamma'+1}$. Again, as $\alocation$ is the only location in 
 $\semantics{\atermset{\asetvar \cup \set{\avariableter}} }_{\astore[\avariableter \gets \alocation],\aheap} \setminus 
\semantics{\atermset{\asetvar}}_{\astore,\aheap}$, we have $\amap'(\amapbis(\asymbterm_1)) = \pair{\amapbis(\asymbterm_2)}{\inbound'}$
for some $\inbound'$. By a simple analysis on the way $\inbound$ and $\inbound'$ are computed (by truncation up to $\bound$ and $2 \bound+b$ respectively),
we can conclude that 
$\inbound' = \inbound_1+\inbound_2$ if $\inbound_1 < \bound$ and $\inbound_2 < \bound$, otherwise $\inbound' \in 
\interval{\inbound_1+\inbound_2}{2 \bound+b}$. 
\item Using similar arguments, one can show that for all $\asymbterm_1',\asymbterm_2'\in \symbterms'$, if 
      $(\pi_1 \circ \amap')(\asymbterm_1') = \asymbterm_2'$ then either
      $(\pi_1 \circ \amap)(\amapbis^{-1}(\asymbterm_1')) = \amapbis^{-1}(\asymbterm_2')$ or we have
     $(\pi_1 \circ \amap)(\amapbis^{-1}(\asymbterm_1')) = \equivclass{\avariableter}{\symbterms}$ and 
     $(\pi_1 \circ \amap)(\equivclass{\avariableter}{\symbterms}) = \amapbis^{-1}(\asymbterm_2')$.
\end{enumerate}

\end{description}

For the proof of the other direction, let us assume that $\triple{\symbterms}{\amap}{\symbrem}$ is a symbolic memory state
over $\pair{\asetvar\cup\{\avariableter\}}{\bound}$ such that 
$\symbexists{\triple{\symbterms}{\amap}{\symbrem}}{\symbms{\astore}{\aheap}{\asetvar}{2\bound+b}}{\avariable}{\avariablebis}{\avariableter}$.
As previously, we write $\triple{\symbterms'}{\amap'}{\symbrem'}$ to denote $\symbms{\astore}{\aheap}{\asetvar}{2\bound+b}$. 
Let us show that 
$\minpath{\astore(\avariable)}{\astore(\avariablebis)}{\aheap} \neq \emptyset$ and
there is $\alocation \in \minpath{\astore(\avariable)}{\astore(\avariablebis)}{\aheap}\cup\{\astore(\avariablebis)\}$ such that 
$\symbms{\astore[\avariableter \gets \alocation]}{\aheap}{\asetvar\cup\{\avariableter\}}{\bound} = \triple{\symbterms}{\amap}{\symbrem}$.
Note that the condition~\ref{E-placement} combined with either the condition~\ref{E-no-new-location} or the condition~\ref{E-new-location}
leads to get  $\minpath{\astore(\avariable)}{\astore(\avariablebis)}{\aheap} \neq \emptyset$.
Let us start by defining $\alocation$.
\begin{enumerate}
\item In the case there is $\aterm \in \equivclass{\avariableter}{\symbterms}$ such that $\avariableter \not \in \chars{\aterm}$,
let $\alocation = \semantics{\aterm}_{\astore,\aheap}$. 
\item Otherwise, let $I$ be such that $\avariableter \in \asymbterm_{I}$ from the condition~\ref{E-placement}.
As $\amap(\asymbterm_{I-1}) = \pair{\equivclass{\avariableter}{\symbterms}}{\inbound_1}$ and
$\amap(\equivclass{\avariableter}{\symbterms}) = \pair{\asymbterm_{I+1}}{\inbound_2}$, by the condition~\ref{E-new-location}, 
 we have $\amap'(\amapbis(\asymbterm_{I-1})) = \pair{\amapbis(\asymbterm_{I+1})}{\inbound'}$
for some $\inbound'$. Moreover, $\inbound' = \inbound_1+\inbound_2$ if $\inbound_1 < \bound$ and $\inbound_2 < \bound$, otherwise 
$\inbound' \in \interval{\inbound_1 + \inbound_2}{2 \bound+b}$.
By definition of $\amap'$,  in $\pair{\astore}{\aheap}$, there is a path from the unique location in $\semantics{\amapbis(\asymbterm_{I-1})}_{\astore,\aheap}$ and
the unique location in $\semantics{\amapbis(\asymbterm_{I+1})}_{\astore,\aheap}$ of the form $\alocation_0 \mapsto \alocation_1 \mapsto \cdots \mapsto \alocation_N$
with $\inbound' = \min(N,2 \bound+b)$. If $\inbound_1 < \bound$, then $\alocation = \alocation_{\inbound_1}$ otherwise
$\alocation = \alocation_{N - \inbound_2}$.
\end{enumerate}
It remains to check that $\symbms{\astore[\avariableter \gets \alocation]}{\aheap}{\asetvar\cup\{\avariableter\}}{\bound} = \triple{\symbterms}{\amap}{\symbrem}$,
which follows essentially from the satisfaction of the conditions~\ref{E-satisfiability}--\ref{E-new-location}.
For instance, the value $\symbrem$ matches thanks to the condition~\ref{E-garbage} and the value $\amap$ matches by the 
conditions~\ref{E-no-new-location} and~\ref{E-new-location}. The condition~\ref{E-satisfiability} is helpful for having the right set $\symbterms$. 
\end{proof}
