# Supplementary material for: A Complete Axiomatisation for Quantifier-Free Separation Logic
Source: arXiv:2006.05156 source file (2021-08-09)
Supplement: Supplementary file 25 [file proof-theo-core2PSLcompl.tex]

\begin{proof} 
Let $\aformula$ be a Boolean combination of core formulae.
As $\coresys$ is sound, we have $\prove_{\coresys} \aformula$ implies that $\aformula$ is
valid.
Now, let us assume that $\aformula$ is valid, and let us prove that $\prove_{\coresys}\aformula$.
Similarly to the proof of Lemma~\ref{prop:corePSLone}, one can show there is a disjunction $\aformulabis=\aformula_1\vee\ldots\vee\aformula_n$ of core types
such that $\prove_{\coresys}(\neg \aformula)\Leftrightarrow\aformulabis$.
Since $\aformula$ is valid, the formulae
$\neg\aformula$, $\aformulabis$ and $\aformulabis_i$ are unsatisfiable (for all $i$).
By Lemma~\ref{lemma:axiomtwoRCct}, $\prove_{\coresys}\aformulabis_i\Rightarrow\bot$ (for all $i$).
Therefore, by classical reasoning, $\prove_{\coresys}\neg\aformula\Rightarrow\bot$ and therefore $\prove_{\coresys}\aformula$.
\end{proof}
