# Supplementary material for: A Complete Axiomatisation for Quantifier-Free Separation Logic
Source: arXiv:2006.05156 source file (2021-08-09)
Supplement: Supplementary file 26 [file proof-theorem-corePSLcompl.tex]

\theocorePSLcompl*

In order to prove Theorem~\ref{theo:corePSLcompl}, let us first establish the following lemma.

\begin{restatable}{lemma}{propcorePSLone}
\stmtdesc{Core Types Lemma}
\label{prop:corePSLone}
Let $\aformula \in \boolcomb{\coreformulae{\asetvar}{\bound}}$. There is a disjunction
$\aformulabis=\aformulabis_1\vee\ldots\vee\aformulabis_n$ with
$\aformulabis_i\in\coretype{\asetvar}{\bound}$ for all $i$
such that $\prove_{\coresys} \aformula \iff \aformulabis$.
\end{restatable}

\begin{proof}
Let $\aformulabis_1\vee\ldots\vee\aformulabis_n$ be a formula in disjunctive normal form equivalent to $\aformula$. If $\aformulabis_i$ is not a core type, there is a core formula $\aformulater\in\coreformulae{\asetvar}{\bound}$ that occurs neither positively nor negatively in $\aformula_i$.
Replacing $\aformula_i$ with $(\aformula_i\wedge\aformulater)\vee(\aformula_i\wedge\neg\aformulater)$, and repeating this for all missing core types and for all $i$, we obtain a
disjunction of core types of the expected form. Since all equivalences follow from reasoning in classical logic, the equivalence between $\aformula$ and the obtained formula can be proved
in $\coresys$.
\end{proof}

\begin{proof} (Theorem~\ref{theo:corePSLcompl})
Let $\aformula$ be a Boolean combination of core formulae.
As all the axioms are valid (the proof can be found in Appendix~\ref{appendix:PSLSoundness}), $\prove_{\coresys} \aformula$ implies that $\aformula$ is
valid.
Now, let us assume that $\aformula$ is valid, and let us prove that $\prove_{\coresys}\aformula$.
By Lemma~\ref{prop:corePSLone}, there is a disjunction $\aformulabis=\aformula_1\vee\ldots\vee\aformula_n$ of core types
such that $\prove_{\coresys}(\neg \aformula)\Leftrightarrow\aformulabis$.
Since $\aformula$ is valid, the formulae
$\neg\aformula$, $\aformulabis$ and all the $\aformulabis_i$'s are unsatisfiable.
By Lemma~\ref{prop:corePSLtwo}, $\prove_{\coresys}\aformulabis_i\Rightarrow\bot$, for all $i$.
Therefore, by classical reasoning, $\prove_{\coresys}\neg\aformula\Rightarrow\bot$.
\end{proof}
