# Supplementary material for: A Complete Axiomatisation for Quantifier-Free Separation Logic
Source: arXiv:2006.05156 source file (2021-08-09)
Supplement: Supplementary file 28 [file two-lemmata-core-types.tex]

\begin{lemma}\label{lemma:deterministicexistentialcompletion}
Let $\bound \in \Nat^+$ and let $\asetvar \subseteq_\fin \PVAR$ such that $\avariableter \not \in \asetvar$.
Let $\aformula \in \coretype{\asetvar \cup \{\avariableter\}}{\bound}$ be a satisfiable formula such that
for two terms
$\aterm_1,\aterm_2 \in \atermset{\asetvar}$ we have
  \begin{itemize}
    \item $\sees{\aterm_1}{\aterm_2}{\atermset{\asetvar}} \inside \aformula$;
    \item $\threeorliterals{\aterm_1 = \avariableter}{\aterm_2 = \avariableter}{\lnot \sees{\aterm_1}{\aterm_2}{\{\avariableter\}}} \inside \aformula$.
  \end{itemize}
Let $\aformula' = \bigwedge\{ \aformulater \inside \aformula \mid \aformulater \in \coreformulae{\asetvar}{\bound}\}$.
It holds that,
\begin{enumerate}
\item if there is $\aterm \in \{\aterm_1,\aterm_2\}$ such that $\aterm = \avariableter \inside \aformula$ then
$\prove_{\coresys} (\aterm = \avariableter \land \aformula') \iff \aformula$;
\item otherwise, there are $\inbound_1,\inbound_2 \in \interval{1}{\bound}$ such that
\begin{itemize}
\item $\seesgeq{\aterm_1}{\avariableter}{\atermset{\asetvar}}{\inbound_1} \land \seesgeq{\avariableter}{\aterm_2}{\atermset{\asetvar}}{\inbound_2} \inside \aformula$;
\item $\seesgeq{\aterm_1}{\avariableter}{\atermset{\asetvar}}{\inbound_1+1} \not\inside \aformula$ and $\seesgeq{\avariableter}{\aterm_2}{\atermset{\asetvar}}{\inbound_2+1} \not\inside \aformula$.
\end{itemize}
Let $\sim_1,\sim_2\in\{\geq,=\}$ such that for every $i \in \{1,2\}$, $\sim_i$ is $=$ iff $\inbound_i < \bound$.
Then
\begin{nscenter}
$\prove_{\coresys} (\sees{\aterm_1}{\avariableter}{\atermset{\asetvar}}{\sim_1}{\inbound_1} \land \sees{\avariableter}{\aterm_2}{\atermset{\asetvar}}{\sim_2}{\inbound_2}  \land \avariableter \not\in\{\aterm_1,\aterm_2\} \land \aformula') \iff \aformula$.
\end{nscenter}
\end{enumerate}
\end{lemma}

Let us informally explain this lemma. As hypothesis, we consider a core type  $\aformula \in \coretype{\asetvar \cup \{\avariableter\}}{\bound}$ where the variable $\avariableter$ is in the path starting from the location corresponding to $\aterm_1$ and ending in the location corresponding to $\aterm_2$, for some $\aterm_1$ and $\aterm_2$ in $\atermset{\asetvar}$ such that $\sees{\aterm_1}{\aterm_2}{\atermset{\asetvar}} \inside \aformula$.
Then, the lemma states that given a literal $\aformulabis \inside \aformula$ such that $\aformulabis \in \coreformulae{\asetvar\cup\{\avariableter\}}{\inbound}$ and $\avariableter \in \chars{\aformulabis}$,
the formula obtained from $\aformula$ by eliminating $\aformulabis$ is equivalent to the original one, with
the following exceptions of formulae that must be kept:
\begin{itemize}
\item if $\avariableter = \aterm_1$ or $\avariableter = \aterm_2$ occurs positively in $\aformula$, then one of these two formulae must be kept.
\item otherwise
(notice that then we are in the case that ${\lnot \sees{\aterm_1}{\aterm_2}{\{\avariableter\}}} \inside \aformula$) it is sufficient to keep
 $\sees{\aterm_1}{\avariableter}{\atermset{\asetvar}}{\sim_1}{\inbound_1} \land \sees{\avariableter}{\aterm_2}{\atermset{\asetvar}}{\sim_2}{\inbound_2}  \land \avariableter \not\in\{\aterm_1,\aterm_2\}$
where $\sees{\aterm_1}{\avariableter}{\atermset{\asetvar}}{\sim_1}{\inbound_1} \land \sees{\avariableter}{\aterm_2}{\atermset{\asetvar}}{\sim_2}{\inbound_2}$ has the ``maximal amount of information'' among all the $\sees{\aterm_1}{\avariableter}{\atermset{\asetvar}}$ and $\sees{\avariableter}{\aterm_2}{\atermset{\asetvar}}$
formulae.
Informally (the formal definition is in the statement of the lemma)
$\sees{\aterm_1}{\avariableter}{\atermset{\asetvar}}{\sim_1}{\inbound_1} \land \sees{\avariableter}{\aterm_2}{\atermset{\asetvar}}{\sim_2}{\inbound_2}$ has the ``maximal amount of information'' if it is not a consequence of a formula of the same shape (conjunctions of sees formulae).
For example, if $\sees{\aterm_1}{\avariableter}{\atermset{\asetvar}}{\geq}{3}$, $\sees{\aterm_1}{\avariableter}{\atermset{\asetvar}}{\geq}{4}$, $\lnot\sees{\aterm_1}{\avariableter}{\atermset{\asetvar}}{\geq}{5}$ and
$\lnot\sees{\aterm_1}{\avariableter}{\atermset{\asetvar}}{\geq}{6}$ all occurs in $\literals{\aformula}$, it is sufficient to keep
$\sees{\aterm_1}{\avariableter}{\atermset{\asetvar}}{\geq}{4}$ and $\lnot\sees{\aterm_1}{\avariableter}{\atermset{\asetvar}}{\geq}{5}$,
as the two other literals can clearly be deduced from these two (see the axiom~\ref{core2Ax:SeesMono1}).
\end{itemize}

\begin{proof}(sketch)
Let us start the proof by reasoning independently on the two cases dividing the lemma, and define
$\aformulater$ to be $\aterm = \avariableter$ if we are in the first case, and otherwise, if we are in the second case, let $\aformulater$ to be
\begin{nscenter}
$\sees{\aterm_1}{\avariableter}{\atermset{\asetvar}}{\sim_1}{\inbound_1} \land \sees{\avariableter}{\aterm_2}{\atermset{\asetvar}}{\sim_2}{\inbound_2}  \land \avariableter \not\in\{\aterm_1,\aterm_2\}$
\end{nscenter}
w.r.t. $\sim_1$, $\sim_2$, $\inbound_1$ and $\inbound_2$ as in the statement (the existence of $\aformulater$ in this case is easy to prove, as all its conjuncts are in $\literals{\aformula}$).
We want to prove that $\prove_{\coresys} \aformulater \land \aformula' \iff \aformula$, where
$\aformula' = \bigwedge\{ \aformulater \inside \aformula \mid \aformulater \in \coreformulae{\asetvar}{\bound}\}$.
Notice that, since $\coresys$ is a sound and complete axiomatisation for Boolean combination of core formulae, we can reason semantically in order to deduce that the above double implication is provable in the system.
Hence we show that $\models \aformulater \land \aformula' \iff \aformula$.
The right-to-let direction
$\models \aformulater \land \aformula' \Leftarrow \aformula$ trivially holds from $\aformulater \land \aformula' \inside \aformula$. From the satisfiability of $\aformula$, we then conclude that $\aformulater \land \aformula'$ is satisfiable.

In order to show that $\models \aformulater \land \aformula' \Rightarrow \aformula$, we consider two memory states
$\pair{\astore}{\aheap}$ and $\pair{\astore'}{\aheap'}$ satisfying $\aformulater \land \aformula'$.
We then prove that $\charsymbform(\symbms{\astore}{\aheap}{\asetvar \cup \{\avariableter\}}{\bound}) \iff \charsymbform(\symbms{\astore'}{\aheap'}{\asetvar \cup \{\avariableter\}}{\bound})$.
This is enough to prove the left-to-right direction.
Indeed, by Lemma~\ref{lemma:coretypecharsms} we know that every characteristic formula $\charsymbform(\asms)$ of a symbolic memory state $\asms$  w.r.t. $\pair{\asetvar \cup \{\avariableter\}}{\bound}$ is equivalent to exactly one core type of $\coretype{\asetvar \cup \{\avariableter\}}{\bound}$.
Moreover, since $\aformulater$ and $\aformula'$ are formulae in $\coreformulae{\asetvar \cup \{\avariableter\}}{\bound}$, by standard arguments we then conclude that $\aformulater \land \aformula'$ is equivalent to the infinite disjunction
$\bigvee_{(\astore'',\aheap'') \models \aformulater \land \aformula'} \charsymbform(\symbms{\astore''}{\aheap''}{\asetvar \cup \{\avariableter\}}{\bound}$.
Then, by proving that for every two $\pair{\astore}{\aheap}$ and $\pair{\astore'}{\aheap'}$ satisfying $\aformulater \land \aformula'$ are such that
$\charsymbform(\symbms{\astore}{\aheap}{\asetvar \cup \{\avariableter\}}{\bound}) \iff \charsymbform(\symbms{\astore'}{\aheap'}{\asetvar \cup \{\avariableter\}}{\bound})$, we directly conclude that there is a symbolic memory state
$\asms \in \symbdomain{\asetvar \cup \{\avariableter\}}{\bound}$
such that $\aformulater \land \aformula' \iff \charsymbform(\asms)$.
Thus, again by Lemma~\ref{lemma:coretypecharsms}, there is exactly one core type $\aformulabis$ in $\coretype{\asetvar \cup \{\avariableter\}}{\bound}$ such that
$\charsymbform(\asms) \iff \aformulabis$.
From the left-to-right direction of this lemma (i.e. $\aformula \implies \aformula' \land \aformulater$) together with $\aformula' \land \aformulater \implies \charsymbform(\asms)$, by propositional calculus we then conclude that
$\aformula \implies \aformula \land \aformulabis$. As $\aformula$ is  satisfiable by hypothesis, 
by definition of core types this implies that $\aformula \iff \aformulabis$, ending the proof.

Therefore, we show that given two memory states
$\pair{\astore}{\aheap}$ and $\pair{\astore'}{\aheap'}$ satisfying $\aformulater \land \aformula'$,
it holds that
$\charsymbform(\symbms{\astore}{\aheap}{\asetvar \cup \{\avariableter\}}{\bound}) \iff \charsymbform(\symbms{\astore'}{\aheap'}{\asetvar \cup \{\avariableter\}}{\bound})$.
To do so, we reason on the structure of the symbolic memory state and prove the equivalent statement
$\symbms{\astore}{\aheap}{\asetvar \cup \{\avariableter\}}{\bound} = \symbms{\astore'}{\aheap'}{\asetvar \cup \{\avariableter\}}{\bound}$.
First of, notice that directly by definition of core types, the fact that $\aformula \in \coretype{\asetvar \cup \{\avariableter\}}{\bound}$ and $\aformula' \inside \aformula$, we conclude that $\aformula'$ is a core type of $\coretype{\asetvar}{\bound}$.
Hence from $\pair{\astore}{\aheap} \models \aformula'$ and $\pair{\astore'}{\aheap'} \models \aformula'$ we already conclude by Lemma~\ref{lemma:msmodelsabs} that
$\symbms{\astore}{\aheap}{\asetvar}{\bound} = \symbms{\astore'}{\aheap'}{\asetvar}{\bound}$.
We say that a location is $\atermset{\asetvar}$\emph{-labelled} if it corresponds to a term of $\atermset{\asetvar}$.
We now consider the formula $\aformulater$, and essentially prove the following two properties:
\begin{enumerate}
\item Let $\asetbis$ be the set of $\atermset{\asetvar}$-labelled locations of $\pair{\astore}{\aheap}$, and let $\asetbis'$ be the set of its $\atermset{\asetvar \cup \{\avariableter\}}$-labelled locations. Then $\asetbis' = \asetbis$ (when $\aformulater$ corresponds to the first case of the statement) or $\asetbis' = \asetbis \cup \{\astore(\avariableter)\}$ (when $\aformulater$ corresponds to the second case of the statement).
\item Given a $\atermset{\asetvar}$-labelled location $\alocation$ of $\pair{\astore}{\aheap}$, given $\aformulater$ we can deterministically compute the set of terms $\aterm \in \atermset{\asetvar \cup \{\avariableter\}}$ such that $\semantics{\aterm}_{\astore,\aheap} = \alocation$.
\end{enumerate}
The same two properties also hold for $\pair{\astore'}{\aheap'}$. By definition of $\aformulater$, from these two properties we will conclude that
$\symbms{\astore}{\aheap}{\asetvar \cup \{\avariableter\}}{\bound}) = \symbms{\astore'}{\aheap'}{\asetvar \cup \{\avariableter\}}{\bound}$.
Moreover, notice that we can prove (2) from the proof of (1) as soon as for a given term $\ameetvar{\avariable'}{\avariablebis'}{\avariablesix'}$ where at least one variable between
$\avariable'$, $\avariablebis'$ and $\avariablesix'$ equals $\avariableter$, we can deterministically conclude that $\semantics{\ameetvar{\avariable'}{\avariablebis'}{\avariablesix'}}_{\astore,\aheap} = \astore(\avariableter)$ or find a term $\ameetvar{\avariable''}{\avariablebis''}{\avariablesix''} \in \atermset{\asetvar}$ such that
$\semantics{\ameetvar{\avariable'}{\avariablebis'}{\avariablesix'}}_{\astore,\aheap} = \semantics{\ameetvar{\avariable''}{\avariablebis''}{\avariablesix''}}_{\astore,\aheap}$.
This is exactly what we do. Hence, we focus on the proof of (1), which is by cases depending on $\aformulater$.
\begin{description}
  \item[a. $\aformulater$ is $\aterm {=} \avariableter$ for some $\aterm \in \{\aterm_1,\aterm_2\}$.] W.l.o.g. let $\aterm$ be syntactically equal to $\ameetvar{\avariable}{\avariablebis}{\avariablesix}$
  (indeed, if $\aterm$ is $\avariable \in \asetvar$, then by axiom~\ref{core2Ax:Self} we can consider $\ameetvar{\avariable}{\avariable}{\avariable}$ instead).
  Let us prove that the set $\asetbis$ of $\atermset{\asetvar}$-labelled locations of $\pair{\astore}{\aheap}$, equals the set $\asetbis'$ of $\atermset{\asetvar \cup \{\avariableter\}}$-labelled locations of $\pair{\astore}{\aheap}$.
  By definition every $\atermset{\asetvar}$-labelled locations is also a $\atermset{\asetvar \cup \{\avariableter\}}$-labelled locations, so we simply need to prove that $\asetbis' \subseteq \asetbis$.
  Let $\alocation$ be a $\atermset{\asetvar \cup \{\avariableter\}}$-labelled locations corresponding to a term $\overline{\aterm}$. If $\avariableter$ does not appear (syntactically) in $\overline{\aterm}$, then trivially $\alocation$ is also a
  $\atermset{\asetvar}$-labelled location. Otherwise, w.l.o.g. (again, see the axiom~\ref{core2Ax:Self}), let $\ameetvar{\avariable'}{\avariablebis'}{\avariablesix'}$ be a term such that
  $\semantics{\ameetvar{\avariable'}{\avariablebis'}{\avariablesix'}}_{\astore,\aheap} = \alocation$ and
  at least one variable between
  $\avariable'$, $\avariablebis'$ and $\avariablesix'$ equals $\avariableter$.
  By definition of meet-point, $\alocation$ is the first location reachable from $\astore(\avariable')$ that reaches $\astore(\avariablesix')$ and is also reached by $\astore(\avariablebis')$.
  We show that then there is a term in $\widehat{\aterm} \in \atermset{\asetvar}$ such that $\semantics{\ameetvar{\avariable'}{\avariablebis'}{\avariablesix'}}_{\astore,\aheap} = \semantics{\widehat{\aterm}}_{\astore,\aheap}$.
  We proceed by cases:
  \begin{itemize}
  \item if (syntactically) $\avariablesix' = \avariableter$, then $\alocation$ is also the first location reachable from $\astore(\avariable')$ that reaches $\astore(\avariablesix)$ and is also reached by $\astore(\avariablebis')$.
  Hence $\semantics{\ameetvar{\avariable'}{\avariablebis'}{\avariablesix'}}_{\astore,\aheap} = \semantics{\ameetvar{\avariable'}{\avariablebis'}{\avariablesix}}_{\astore,\aheap}$.
  \item if (syntactically) $\avariable' = \avariableter$, then $\alocation$ is also the first location reachable from $\astore(\avariable)$ that reaches $\astore(\avariablesix')$ and is also reached by $\astore(\avariablebis')$.
  Hence $\semantics{\ameetvar{\avariable'}{\avariablebis'}{\avariablesix'}}_{\astore,\aheap} = \semantics{\ameetvar{\avariable}{\avariablebis'}{\avariablesix'}}_{\astore,\aheap}$.
  \item if (syntactically) $\avariablebis' = \avariableter$, then $\alocation$ is also the first location reachable from $\astore(\avariable')$ that reaches $\astore(\avariablesix')$ and is also reached by $\astore(\avariable)$.
  Hence $\semantics{\ameetvar{\avariable'}{\avariablebis'}{\avariablesix'}}_{\astore,\aheap} = \semantics{\ameetvar{\avariable'}{\avariable}{\avariablesix'}}_{\astore,\aheap}$.
  \end{itemize}
  Thus, it is easy to see that by iterating the three steps just above, given $\ameetvar{\avariable'}{\avariablebis'}{\avariablesix'}$ it is always possible to (deterministically, since $=$ is an equivalence relation) replace every occurrence of $\avariableter$ in order to find a term $\widehat{\aterm} \in \atermset{\asetvar}$ such that $\semantics{\widehat{\aterm}}_{\astore,\aheap} = \alocation$.
  Hence $\asetbis' = \asetbis$.
  \item[b. $\aformulater$ is $\sees{\aterm_1}{\avariableter}{\atermset{\asetvar}}{\sim_1}{\inbound_1} \land \sees{\avariableter}{\aterm_2}{\atermset{\asetvar}}{\sim_2}{\inbound_2}  \land \avariableter \not\in\{\aterm_1,\aterm_2\}$.]

  W.r.t. the sets $\asetbis$ and $\asetbis'$ in the statement of (1), we prove that $\asetbis' = \asetbis \cup \{\astore(\avariableter)\}$. As in the previous case, it is sufficient to show $\asetbis' \subseteq \asetbis \cup \{\astore(\avariableter)\}$.
  W.l.o.g. (see the axiom~\ref{core2Ax:Self})
  suppose
  $\aterm_1 = \ameetvar{\avariable}{\avariablebis}{\avariablesix}$ and
  $\aterm_2 = \ameetvar{\avariable'}{\avariablebis'}{\avariablesix'}$, syntactically.
  From $\aformulater$, we conclude that every location in the path from $\semantics{\aterm_1}_{\astore,\aheap}$ to $\semantics{\aterm_2}_{\astore,\aheap}$, both ends excluded, is not a $\atermset{\asetvar}$-labelled location.
  However, one of these locations corresponds to $\astore(\avariableter)$, hence $\astore(\avariableter) \in \asetbis'$ and moreover $\aheap$ must present exactly one of the following three patterns:
  \begin{center}
  \vspace{-0.7cm}
   \scalebox{0.85}{
       \begin{tikzpicture}[baseline]
         \node (i) at (0,0) {};
         \node[dot,label=below:{$\ameetvar{\avariable}{\avariablebis}{\avariablesix}$}] (m) [below = 1.5cm of i] {};
         \node[dot,label=above:{$\avariableter$}] (z) [right = 1cm of m] {};
         \node[dot,label=right:$\ameetvar{\avariable'}{\avariablebis'}{\avariablesix'}$] (j) [right= 1cm of z] {};
         \node[label=below:{does not loop}] (k) [below of=j] {};
         \node (kk) [above = 1.5cm of j] {};

         \draw[reach] (i) -- (m);
         \draw[pto] (m) to node [above] {$+$} (z);
         \draw[pto] (z) to node [above] {$+$} (j);
         \draw[reach] (kk) -- (j);
         \draw[reach] (j) -- (k);
       \end{tikzpicture}
       \quad
       \begin{tikzpicture}[baseline]
         \node (i) at (0,0) {};
         \node[dot,label=below:{$\ameetvar{\avariable}{\avariablebis}{\avariablesix}$}] (m) [below = 1.5cm of i] {};
         \node[dot,label=above:{$\avariableter$}] (z) [right = 1cm of m] {};
         \node[dot,label=right:$\ameetvar{\avariable'}{\avariablebis'}{\avariablesix'}$] (j) [right= 1cm of z] {};
         \node[dot,label=above right:{$\overline{\alocation}$}] (k) [below of=j] {};
         \node (kk) [above = 1.5cm of j] {};

         \draw[reach] (i) -- (m);
         \draw[pto] (m) to node [above] {$+$} (z);
         \draw[pto] (z) to node [above] {$+$} (j);
         \draw[reach] (j) -- (k);
         \draw[reach] (kk) -- (j);
         \draw[reach] (k) to [out=-20, in=-160
                , looseness=0.8, loop
                , distance=2cm, reach] node {} (k);
       \end{tikzpicture}
       \quad
       \begin{tikzpicture}[baseline]
         \node (i) at (0,0) {};
         \node[dot,label=left:{$\ameetvar{\avariable}{\avariablebis}{\avariablesix}$}] (m) [below = 1.5cm of i] {};
         \node[dot,label=above:{$\avariableter$}] (z) [right = 1cm of m] {};
         \node[dot,label=right:$\ameetvar{\avariable'}{\avariablebis'}{\avariablesix'}$] (j) [right= 1cm of z] {};
         \node (kk) [above = 1.5cm of j] {};

         \draw[reach] (i) -- (m);
         \draw[pto] (m) to node [above] {$+$} (z);
         \draw[pto] (z) to node [above] {$+$} (j);
         \draw[reach] (kk) -- (j);
         \draw[reach] (j) to [out=-90, in=-90
                , looseness=0.8, loop
                , distance=2cm, reach] node {} (m);
       \end{tikzpicture}
   }
  \end{center}
  Let $\alocation$ be a $\atermset{\asetvar \cup \{\avariableter\}}$-labelled locations corresponding to a term $\overline{\aterm}$. If $\avariableter$ does not appear (syntactically) in $\overline{\aterm}$, or $\alocation = \astore(\avariableter)$, then $\alocation \in \asetbis \cup \{\astore(\avariableter)\}$.
   Otherwise, w.l.o.g. (again, see the axiom~\ref{core2Ax:Self}), let us consider $\ameetvar{\widehat{\avariable}}{\widehat{\avariablebis}}{\widehat{\avariablesix}}$ be a term such that $\astore(\avariableter) \neq \alocation$,
  $\semantics{\ameetvar{\widehat{\avariable}}{\widehat{\avariablebis}}{\widehat{\avariablesix}}}_{\astore,\aheap} = \alocation$ and
  at least one variable between
  $\avariable'$, $\avariablebis'$ and $\avariablesix'$ equals $\avariableter$.
  By definition of meet-point, $\alocation$ is the first location reachable from $\astore(\avariable')$ that reaches $\astore(\avariablesix')$ and is also reached by $\astore(\avariablebis')$.
  We show that then there is a term in $\widehat{\aterm} \in \atermset{\asetvar}$ such that $\semantics{\ameetvar{\widehat{\avariable}}{\widehat{\avariablebis}}{\widehat{\avariablesix}}}_{\astore,\aheap} = \semantics{\widehat{\aterm}}_{\astore,\aheap}$.
  We proceed by cases:
  \begin{itemize}
  \item if (syntactically) $\widehat{\avariablesix} = \avariableter$, then $\alocation$ is also the first location reachable from $\astore(\widehat{\avariablebis})$ that reaches $\astore(\avariablesix')$ and is also reached by $\astore(\widehat{\avariablebis})$.
  Hence $\semantics{\ameetvar{\widehat{\avariable}}{\widehat{\avariablebis}}{\widehat{\avariablesix}}}_{\astore,\aheap} = \semantics{\ameetvar{\widehat{\avariable}}{\widehat{\avariablebis}}{\avariablesix'}}_{\astore,\aheap}$.
  \item Suppose (syntactically) $\widehat{\avariable} = \avariableter$.
  Then, the third pattern cannot occur in $\aheap$.
  Indeed, Suppose (ad absurdum) that the third pattern occurs in $\aheap$ and therefore that
   $\astore(\avariableter)$ belongs to a cycle.
   It is then easy to see that $\ameetvar{\avariableter}{\widehat{\avariablebis}}{\widehat{\avariablesix}}$ then corresponds to the location $\astore(\avariableter)$.
  Informally, this holds as by definition $\semantics{\ameetvar{\avariableter}{\widehat{\avariablebis}}{\widehat{\avariablesix}}}_{\astore,\aheap}$ must be the \emph{first location} that is reached by $\astore(\avariableter)$, reaches $\widehat{\avariablebis}$ and is reached by $\astore(\avariablesix)$.
  Since $\astore(\avariable)$ belongs to a cycle, the constraint of being the ``first location'' holds for $\astore(\avariableter)$.
  A more formal proof of this can be found inside Lemma~\ref{lemma:axiomstwoRCchars} (point 2, see also \ref{axiom2:auxlemma7}).
  Then, the third pattern leads to a contradiction with $\alocation \neq \astore(\avariableter)$.

  Therefore, the first or second pattern holds in $\aheap$. In each of these two cases, since $\alocation \neq \astore(\avariableter)$, we can easily prove that $\alocation$ is also the first location reachable from $\astore(\avariable)$ that reaches $\astore(\widehat{\avariablesix})$ and is reached by $\astore(\widehat{\avariablebis})$.
  Hence,
  $\ameetvar{\widehat{\avariable}}{\widehat{\avariablebis}}{\widehat{\avariablesix}} = \ameetvar{\avariable}{\widehat{\avariablebis}}{\widehat{\avariablesix}}$.
  \item Suppose (syntactically) $\widehat{\avariablebis} = \avariableter$.
  We then split the proof, depending on whether or not the third pattern occurs in $\aheap$.
  \begin{itemize}
  \item Similarly to the last point of the proof, if the first or second pattern occur in $\aheap$, then in both cases  $\alocation$ is also the first location reachable from $\astore(\avariable)$ that reaches $\astore(\widehat{\avariablesix})$ and is reached by $\astore(\widehat{\avariablebis})$.
  Hence,
  $\ameetvar{\widehat{\avariable}}{\widehat{\avariablebis}}{\widehat{\avariablesix}} = \ameetvar{\avariable}{\widehat{\avariablebis}}{\widehat{\avariablesix}}$.
  \item If instead we have that the third pattern occur in $\aheap$,
  then $\alocation$ that belongs to the same cycle as $\astore(\avariableter)$ (recall that $\alocation \neq \astore(\avariableter)$).
  Trivially, if $\semantics{\ameetvar{\widehat{\avariable}}{\widehat{\avariablebis}}{\widehat{\avariablesix}}}_{\astore,\aheap} = \semantics{\ameetvar{\avariable}{\avariablebis}{\avariablesix}}_{\astore,\aheap}$, we
  the term $\ameetvar{\avariable}{\avariablebis}{\avariablesix}$ is a solution for the term $\widehat{\aterm}$ we are searching.
  Otherwise, we have $\alocation = \semantics{\ameetvar{\widehat{\avariable}}{\widehat{\avariablebis}}{\widehat{\avariablesix}}}_{\astore,\aheap} \not \in \{ \astore(\avariableter), \semantics{\ameetvar{\avariable}{\avariablebis}{\avariablesix}}_{\astore,\aheap}\}$.
  Then, as shown in Lemma~\ref{lemma:axiomstwoRCchars} (points 5 and 6), from the fact that $\alocation$, $\astore(\avariableter)$ and $\semantics{\ameetvar{\avariable}{\avariablebis}{\avariablesix}}_{\astore,\aheap}$ are dfferent and belongs to the same loop, we conclude that
  $\semantics{\ameetvar{\widehat{\avariable}}{\widehat{\avariablebis}}{\widehat{\avariablesix}}}_{\astore,\aheap} = \semantics{\ameetvar{\widehat{\avariable}}{\avariableter}{\widehat{\avariablesix}}}_{\astore,\aheap}$.
  \end{itemize}
  \end{itemize}
  Again, it is easy to see that we can iterate these three steps and, given $\ameetvar{\widehat{\avariable}}{\widehat{\avariablebis}}{\widehat{\avariablesix}}$, always (deterministically) find a term $\widehat{\aterm} \in \atermset{\asetvar}$ such that $\semantics{\widehat{\aterm}}_{\astore,\aheap} = \alocation$.
  This concludes the proof of $\asetbis' = \asetbis \cup \{\astore(\avariableter)\}$.
\end{description}
This ends the proofs of (1) and (2).

We are now ready to show that $\symbms{\astore}{\aheap}{\asetvar \cup \{\avariableter\}}{\bound} = \symbms{\astore'}{\aheap'}{\asetvar \cup \{\avariableter\}}{\bound}$. We consider the following four objects:
\begin{itemize}
\item $\symbms{\astore}{\aheap}{\asetvar}{\bound} = \triple{\symbterms_{\asetvar}}{\amap_{\asetvar}}{\symbrem_{\asetvar}}$ and $\symbms{\astore}{\aheap}{\asetvar \cup \{\avariableter\}}{\bound} =
\triple{\symbterms_{\asetvar \cup \{\avariableter\}}}{\amap_{\asetvar \cup \{\avariableter\}}}{\symbrem_{\asetvar \cup \{\avariableter\}}}$;
\item $\symbms{\astore'}{\aheap'}{\asetvar}{\bound} = \triple{\symbterms_{\asetvar}'}{\amap_{\asetvar}'}{\symbrem_{\asetvar}'}$
and $\symbms{\astore'}{\aheap'}{\asetvar \cup \{\avariableter\}}{\bound} = \triple{\symbterms_{\asetvar \cup \{\avariableter\}}'}{\amap_{\asetvar \cup \{\avariableter\}}'}{\symbrem_{\asetvar \cup \{\avariableter\}}'}$.
\end{itemize}
Recall that $\symbms{\astore}{\aheap}{\asetvar}{\bound} = \symbms{\astore'}{\aheap'}{\asetvar}{\bound}$.
From this, together $\pair{\astore}{\aheap} \models \aformulater$, $\pair{\astore'}{\aheap'} \models \aformulater$ and
$\symbms{\astore}{\aheap}{\asetvar}{\bound}) = \symbms{\astore'}{\aheap'}{\asetvar}{\bound}$, by (1) and (2) we already conclude that $\symbterms_{\asetvar \cup \{\avariableter\}} = \symbterms_{\asetvar \cup \{\avariableter\}}'$.
Let us how show that $\symbrem_{\asetvar \cup \{\avariableter\}} = \symbrem_{\asetvar \cup \{\avariableter\}}'$.
First, by definition of symbolic memory state, given a memory state $\pair{\astore''}{\aheap''}$ and  $\symbms{\astore''}{\aheap''}{\asetvar}{\bound} = \triple{\symbterms}{\amap}{\symbrem}$ the natural number $\symbrem$ encoding the number of memory cells (up to $\bound$)
not in paths between terms of $\atermset{\asetvar}$. Formally, for $\inbound \in \interval{0}{\bound}$
\begin{nscenter}
$\symbrem = \inbound$ $\equivdef$ $\pair{\astore''}{\aheap''} \models \remgeq{\atermset{\asetvar}\times\atermset{\asetvar}}{\inbound}$ and if $\inbound < \bound$ then
$\pair{\astore''}{\aheap''} \models \lnot\remgeq{\atermset{\asetvar}\times\atermset{\asetvar}}{\inbound{+}1}$.
\end{nscenter}
Let us consider $\pair{\astore}{\aheap}$ (the same reasoning can be done for $\pair{\astore'}{\aheap'}$).
Since $\pair{\astore}{\aheap} \models \aformulater$, it is easy to see that the location $\astore(\avariableter)$ belongs to a (possibly empty) path between two terms in $\atermset{\asetvar}$. Hence, $\symbrem_{\asetvar \cup \{\avariableter\}} = \symbrem_{\asetvar}$.
Then, from $\symbms{\astore}{\aheap}{\asetvar}{\bound} = \symbms{\astore'}{\aheap'}{\asetvar}{\bound}$ (more precisely from $\symbrem_{\asetvar} = \symbrem_{\asetvar}'$), we conclude that
$\symbrem_{\asetvar \cup \{\avariableter\}} = \symbrem_{\asetvar \cup \{\avariableter\}}'$.
Lastly, let us show that $\amap_{\asetvar \cup \{\avariableter\}} = \amap_{\asetvar \cup \{\avariableter\}}'$.
We divide the proof into two cases, depending on whether $\aformulater$ corresponds to the first or second case in the statement of the lemma.
\begin{description}
\item[a. $\aformulater$ is $\aterm {=} \avariableter$ for some $\aterm \in \{\aterm_1,\aterm_2\}$.]
Then, from (1) and (2) we have that there is a bijection $\amapbis: \symbterms_{\asetvar \cup \{\avariableter\}} \to  \symbterms_{\asetvar}$ such that for every $\asetmeetvar \in \symbterms_{\asetvar \cup \{\avariableter\}}$,
$\amapbis(\asetmeetvar) \subseteq \asetmeetvar$.
Hence, by definition of symbolic memory state, for every $\aterm \in \atermset{\asetvar \cup \{\avariableter\}}$,
$\amap_{\asetvar \cup \{\avariable\}}(\equivclass{\aterm'}{\symbterms_{\asetvar\cup\{ \avariableter \}}}) = \amap_{\asetvar}(\equivclass{\aterm'}{\symbterms_{\asetvar}})$
where $\aterm' \in \amapbis(\equivclass{\aterm}{\symbterms_{\asetvar\cup\{ \avariableter \}}})$.
As $\symbterms_{\asetvar} = \symbterms_{\asetvar}'$ and $\symbterms_{\asetvar \cup \{\avariableter\}} = \symbterms_{\asetvar \cup \{\avariableter\}}'$, we can use the same $\amapbis$
and conclude a similar statement for $\pair{\astore'}{\aheap'}$, i.e. for every $\aterm \in \atermset{\asetvar \cup \{\avariableter\}}$,
$\amap_{\asetvar \cup \{\avariable\}}'(\equivclass{\aterm'}{\symbterms_{\asetvar\cup\{ \avariableter \}}'}) = \amap_{\asetvar}'(\equivclass{\aterm'}{\symbterms_{\asetvar}'})$
where $\aterm' \in \amapbis(\equivclass{\aterm}{\symbterms_{\asetvar\cup\{ \avariableter \}}})$.
Thus, from $\amap_{\asetvar} = \amap_{\asetvar}'$, we conclude that
$\amap_{\asetvar\cup\{ \avariableter \}} = \amap_{\asetvar\cup\{ \avariableter \}}'$.
\item[b. $\aformulater$ is $\sees{\aterm_1}{\avariableter}{\atermset{\asetvar}}{\sim_1}{\inbound_1} \land \sees{\avariableter}{\aterm_2}{\atermset{\asetvar}}{\sim_2}{\inbound_2}  \land \avariableter \not\in\{\aterm_1,\aterm_2\}$.]
Let us consider $\pair{\astore}{\aheap}$ (the same reasoning can be done for $\pair{\astore'}{\aheap'}$)
First, from (1) and (2) it holds that for every term $\aterm \in \atermset{\asetvar \cup \{\avariableter\}}$,
$\pair{\astore}{\aheap} \models \aterm = \avariableter$ or there is $\aterm' \in \atermset{\asetvar}$ such that
$\pair{\astore}{\aheap} \models \aterm = \aterm'$.
Hence, by axioms~\ref{core2Ax:SeesTermEq} and~\ref{core2Ax:SeesRef}
from $\pair{\astore}{\aheap} \models \aformulater$ we conclude that
\begin{nscenter}
$\pair{\astore}{\aheap} \models \sees{\aterm_1}{\avariableter}{\atermset{\asetvar \cup \{\avariableter\}}}{\sim_1}{\inbound_1} \land \sees{\avariableter}{\aterm_2}{\atermset{\asetvar \cup \{\avariableter\}}}{\sim_2}{\inbound_2}
\land \avariableter \not\in\{\aterm_1,\aterm_2\}$.
\end{nscenter}
Moreover, again from (1) and (2)
there is a bijection $\amapbis: \symbterms_{\asetvar \cup \{\avariableter\}} \setminus \{\equivclass{\avariableter}{\symbterms_{\asetvar \cup \{\avariableter\}}} \to  \symbterms_{\asetvar}$
such that for every $\asetmeetvar \in \symbterms_{\asetvar \cup \{\avariableter\}} \setminus \{\equivclass{\avariableter}{\symbterms_{\asetvar \cup \{\avariableter\}}}$,
$\amapbis(\asetmeetvar) \subseteq \asetmeetvar$.
Then, by definition of symbolic memory state, we can show that for every term $\aterm \in \atermset{\asetvar \cup \{\avariableter\}}$,
\begin{itemize}
\item if $\equivclass{\aterm}{\symbterms_{\asetvar \cup \{\avariableter\}}} \neq \equivclass{\aterm_1}{\symbterms_{\asetvar \cup \{\avariableter\}}}$ and
$\equivclass{\aterm}{\symbterms_{\asetvar \cup \{\avariableter\}}} \neq \equivclass{\avariableter}{\symbterms_{\asetvar \cup \{\avariableter\}}}$, then
$\amap_{\asetvar \cup \{\avariable\}}(\equivclass{\aterm'}{\symbterms_{\asetvar\cup\{ \avariableter \}}}) = \amap_{\asetvar}(\equivclass{\aterm'}{\symbterms_{\asetvar}})$
where $\aterm' \in \amapbis(\equivclass{\aterm}{\symbterms_{\asetvar\cup\{ \avariableter \}}})$;
\item if $\equivclass{\aterm}{\symbterms_{\asetvar \cup \{\avariableter\}}} = \equivclass{\aterm_1}{\symbterms_{\asetvar \cup \{\avariableter\}}}$ then
$\amap_{\asetvar \cup \{\avariable\}}(\equivclass{\aterm}{\symbterms_{\asetvar\cup\{ \avariableter \}}}) = \pair{\equivclass{\avariableter}{\symbterms_{\asetvar \cup \{\avariableter\}}}}{\inbound_1}$;
\item if $\equivclass{\aterm}{\symbterms_{\asetvar \cup \{\avariableter\}}} = \equivclass{\avariableter}{\symbterms_{\asetvar \cup \{\avariableter\}}}$,
$\amap_{\asetvar \cup \{\avariable\}}(\equivclass{\aterm}{\symbterms_{\asetvar\cup\{ \avariableter \}}}) = \pair{\equivclass{\aterm_2}{\symbterms_{\asetvar \cup \{\avariableter\}}}}{\inbound_2}$.
\end{itemize}
As $\symbterms_{\asetvar} = \symbterms_{\asetvar}'$ and $\symbterms_{\asetvar \cup \{\avariableter\}} = \symbterms_{\asetvar \cup \{\avariableter\}}'$, we can use the same $\amapbis$
and conclude a similar statement for $\pair{\astore'}{\aheap'}$.
Again from $\amap_{\asetvar} = \amap_{\asetvar}'$, we conclude that
$\amap_{\asetvar\cup\{ \avariableter \}} = \amap_{\asetvar\cup\{ \avariableter \}}'$. \qedhere
\end{description}
\end{proof}
