# Supplementary material for: A Complete Axiomatisation for Quantifier-Free Separation Logic
Source: arXiv:2006.05156 source file (2021-08-09)
Supplement: Supplementary file 29 [file unused-tautologies.tex]

% for natural deduction. A proof
% \[
%   \begin{nd}
%   \hypo {1} {\aformula_1}
%   \hypo [\vdots] {2} {\vdots}
%   \hypo [n] {3} {\aformula_n}
%   \have [n+1] {4} {\aformulabis_1}
%   \have [\vdots] {5} {\vdots}
%   \have [j] {6} {\aformulater} \by{A, $i_{1}$, \dots, $i_{k}$}{}
%   \have [\vdots] {7} {\vdots}
%   \have [n+m] {8} {\aformulabis_m}
%   \end{nd}
% \]
% where $\aformula_1,\dots,\aformula_n$ are the premises whereas $\aformulabis_1,\dots,\aformulabis_m$ are derivations, can be seen as the formula $\bigwedge_{i \in \interval{1}{n}} \aformula_{i} \implies \bigwedge_{i \in \interval{1}{m}} \aformulabis_i$.
% In the proof below, we are only interested in the last derivation, so that we obtain a proof of $\bigwedge_{i \in \interval{1}{n}} \aformula_{i} \implies \aformulabis_m$.
% With the notation
% \begin{nscenter}
% $
%   \begin{nd}
%   \have [j] {6} {\aformulater} \by{A, $i_{1}$, \dots, $i_{k}$}{}
%   \end{nd}
% $
% \end{nscenter}
% we denote that $\aformulater$ is derivable from the hypothesis and derivations labeled in the proof with the indices $i_{1}$, \dots, $i_{k}$ (that are bound to be less than $j$) by applying the axiom or rule $A$.
%
% Some trivial steps, as the use of the symmetry axiom~\ref{core2Ax:EqSymm} and proofs that are exclusively from propositional calculus (e.g. the proof of $(\aformula \lxor \aformulabis) \land \aformula \Rightarrow \lnot \aformulabis$) are omitted to shorten the presentation.
% It should be kept in mind that these are not natural deduction proofs, as our system uses axioms to express logical reasoning, whereas natural deduction focus on inference rules. In the proofs, by $\land\text{E}$ we denote the tautology $\aformula_1 \land \aformula_2 \land \dots \land \aformula_n \implies \aformulabis_1 \land \aformulabis_2 \land \dots \land \aformulabis_m$ for any $\{\aformulabis_1,\dots,\aformulabis_n\}\subseteq\{\aformula_1,\dots,\aformula_m\}$.
% By $\lor\text{E}$ we instead denote the tautology
% \begin{nscenter}
% $(\Gamma \Rightarrow ((\aformula \lor \aformulabis) \land (\aformula \Rightarrow \aformulater)\land(\aformulabis \Rightarrow \aformulater))) \implies (\Gamma \Rightarrow \aformulater)$
% \end{nscenter}
% that corresponds to a proof by cases started with hypothesis $\Gamma$.
% Similarly, by $\lnot\text{I}$ we instead denote the tautology
% \begin{nscenter}
% $(\Gamma \Rightarrow (\aformula \Rightarrow \bottom)) \implies (\Gamma \Rightarrow \lnot \aformula)$
% \end{nscenter}
% that corresponds to a proof by contradiction started with hypothesis $\Gamma$.

% \item\label{axiom2:oldbeforeaxiom}
% $\boxed{
% \symmetric{\ameetvar{\avariable}{\avariablebis}{\avariableter}} \land
% \defined{\ameetvar{\avariable}{\avariablefour}{\avariableter}} \land
% \ameetvar{\avariable}{\avariablebis}{\avariableter} \neq \ameetvar{\avariable}{\avariablefour}{\avariableter}
%  \Rightarrow (\ameetvar{\avariable}{\avariablebis}{\avariableter} = \ameetvar{\avariablebis}{\avariablefour}{\avariableter}
%  \lxor
%  \ameetvar{\avariable}{\avariablefour}{\avariableter} = \ameetvar{\avariablebis}{\avariablefour}{\avariableter})}
%  $
% In this formula, $\lxor$ is the xor-connective, so that $\aformula \lxor \aformulabis$ is equivalent to $\aformula \iff \lnot \aformulabis$.
% This tautology provides a slight generalisation of axiom \ref{core2Ax:Before}, recalled below, that better reflects the definition of $\before{\aterm}{\aterm'}$, making some proofs lighter.
% \[
% \ref{core2Ax:Before}:\ \symmetric{\ameetvar{\avariable}{\avariablebis}{\avariableter}} \land \defined{\ameetvar{\avariable}{\avariablefour}{\avariableter}} \land
% \ameetvar{\avariable}{\avariablefour}{\avariableter} \neq \ameetvar{\avariablebis}{\avariablefour}{\avariableter}
%  \Rightarrow (
%  \ameetvar{\avariable}{\avariablebis}{\avariableter} = \ameetvar{\avariable}{\avariablefour}{\avariableter}
%  \lor
%  \ameetvar{\avariable}{\avariablebis}{\avariableter} = \ameetvar{\avariablebis}{\avariablefour}{\avariableter}
%  )
%  \]
%  Notice that, by propositional calculus, \ref{core2Ax:Before} can be rewriten as
%  \[\symmetric{\ameetvar{\avariable}{\avariablebis}{\avariableter}} \land \defined{\ameetvar{\avariable}{\avariablefour}{\avariableter}} \land
% \ameetvar{\avariable}{\avariablefour}{\avariableter} \neq \ameetvar{\avariablebis}{\avariablefour}{\avariableter}
% \land
%  \ameetvar{\avariable}{\avariablebis}{\avariableter} \neq \ameetvar{\avariable}{\avariablefour}{\avariableter}
%   \Rightarrow
%   \ameetvar{\avariable}{\avariablebis}{\avariableter} = \ameetvar{\avariablebis}{\avariablefour}{\avariableter}
%   \]
% Hence, to prove in the calculus the tautology
% \[
% \symmetric{\ameetvar{\avariable}{\avariablebis}{\avariableter}} \land
% \defined{\ameetvar{\avariable}{\avariablefour}{\avariableter}} \land
% \ameetvar{\avariable}{\avariablebis}{\avariableter} \neq \ameetvar{\avariable}{\avariablefour}{\avariableter}
%  \Rightarrow (\ameetvar{\avariable}{\avariablebis}{\avariableter} = \ameetvar{\avariablebis}{\avariablefour}{\avariableter}
%  \lxor
%  \ameetvar{\avariable}{\avariablefour}{\avariableter} = \ameetvar{\avariablebis}{\avariablefour}{\avariableter})
% \]
% It is sufficient to show that the following implication is derivable
% \[
% \symmetric{\ameetvar{\avariable}{\avariablebis}{\avariableter}} \land
% \defined{\ameetvar{\avariable}{\avariablefour}{\avariableter}} \land
% \ameetvar{\avariable}{\avariablebis}{\avariableter} \neq \ameetvar{\avariable}{\avariablefour}{\avariableter}
% \land
% \ameetvar{\avariable}{\avariablebis}{\avariableter} = \ameetvar{\avariablebis}{\avariablefour}{\avariableter}
%  \Rightarrow
%  \ameetvar{\avariable}{\avariablefour}{\avariableter} \neq \ameetvar{\avariablebis}{\avariablefour}{\avariableter}
% \]
% which is trivially provable as $\ameetvar{\avariable}{\avariablebis}{\avariableter} \neq \ameetvar{\avariable}{\avariablefour}{\avariableter}
% \land
% \ameetvar{\avariable}{\avariablebis}{\avariableter} = \ameetvar{\avariablebis}{\avariablefour}{\avariableter}$
% implies $ \ameetvar{\avariable}{\avariablefour}{\avariableter} \neq \ameetvar{\avariablebis}{\avariablefour}{\avariableter}$ by axiom~\ref{core2Ax:Substitute}.


% \item\label{axiom2:auxlemmaunused}
% $
% \boxed{\defined{\ameetvar{\avariable}{\avariablebis}{\avariableter}} \land \defined{\ameetvar{\avariable}{\avariablefour}{\avariablefifth}} \land \lnot \defined{\ameetvar{\avariable}{\avariablebis}{\avariablefifth}}
% \implies \before{\ameetvar{\avariable}{\avariablefour}{\avariablefifth}}{\ameetvar{\avariable}{\avariablebis}{\avariableter}}
% }
% $
% \[
% \begin{nd}
% \hypo {1} {\defined{\ameetvar{\avariable}{\avariablebis}{\avariableter}}}
% \hypo {2} {\defined{\ameetvar{\avariable}{\avariablefour}{\avariablefifth}}}
% \hypo {3} {\lnot \defined{\ameetvar{\avariable}{\avariablebis}{\avariablefifth}}}
% \have {4} {\defined{\ameetvar{\avariableter}{\avariableter}{\avariablefifth}} \lor \defined{\ameetvar{\avariablefifth}{\avariablefifth}{\avariableter}}} \by{\ref{core2Ax:PedLinear}}{1,2}
% \open
% \hypo {5} {\defined{\ameetvar{\avariableter}{\avariableter}{\avariablefifth}}}
% \have {6} {\defined{\ameetvar{\avariable}{\avariablebis}{\avariablefifth}}} \by{\ref{core2Ax:Pedix}}{1,5}
% \have {7} {\bottom} \by{\landcontr}{3,6}
% \close
% \have {8} {\lnot \defined{\ameetvar{\avariableter}{\avariableter}{\avariablefifth}}} \ni{5-7}
% \have {9} {\defined{\ameetvar{\avariablefifth}{\avariablefifth}{\avariableter}}} \by{\modusponens}{4,8}
% \have {10} {\defined{\ameetvar{\avariable}{\avariablefour}{\avariableter}}} \by{\ref{core2Ax:Pedix}}{2,9}
% \open
% \hypo {11} {\ameetvar{\avariable}{\avariablefour}{\avariablefifth} = \ameetvar{\avariable}{\avariablebis}{\avariableter}}
% \have {12} {\defined{\ameetvar{\avariable}{\avariablebis}{\avariablefifth}}} \by{\ref{core2Ax:PedInv}}{11}
% \have {13} {\bottom} \by{\landcontr}{3,12}
% \close
% \have {14}  {\ameetvar{\avariable}{\avariablefour}{\avariablefifth} \neq \ameetvar{\avariable}{\avariablebis}{\avariableter}} \ni{11-13}
% \open
% \hypo {15} {\ameetvar{\avariable}{\avariablefour}{\avariablefifth} = \ameetvar{\avariablefour}{\avariablebis}{\avariableter}}
% \have {16} {\defined{\ameetvar{\avariablefour}{\avariablebis}{\avariablefifth}}} \by{\ref{core2Ax:PedInv}}{15}
% \have {17} {\defined{\ameetvar{\avariablebis}{\avariablefour}{\avariablefifth}}} \by{\ref{core2Ax:Bothdef}}{16}
% \have {18} {\defined{\ameetvar{\avariable}{\avariablebis}{\avariablefifth}}} \by{\ref{core2Ax:PedDefines}}{2,17}
% \have {19} {\bottom} \by{\landcontr}{3,18}
% \close
% \have {20} {\ameetvar{\avariable}{\avariablefour}{\avariablefifth} \neq \ameetvar{\avariablefour}{\avariablebis}{\avariableter}} \ni{15-19}
% \open
% \hypo {21} {\asymmetric{\ameetvar{\avariable}{\avariablefour}{\avariablefifth}}}
% \have {22} {\before{\ameetvar{\avariable}{\avariablebis}{\avariableter}}{\ameetvar{\avariable}{\avariablefour}{\avariablefifth}}} \by{\ref{axiom2:auxlemma7}}{1,14,21}
% \have {23} {\defined{\ameetvar{\avariable}{\avariablebis}{\avariablefifth}}} \ae{22}
% \have {24} {\bottom} \by{\landcontr}{3,23}
% \close
% \have {25} {\lnot \asymmetric{\ameetvar{\avariable}{\avariablefour}{\avariablefifth}}} \ni{21-24}
% \have {26} {\symmetric{\ameetvar{\avariable}{\avariablefour}{\avariablefifth}}} \by{$\lnot (\aformula \land \lnot \aformulabis) \land \aformula \implies \aformulabis$}{2,25}
% \have {27} {\before{\ameetvar{\avariable}{\avariablefour}{\avariablefifth}}{\ameetvar{\avariable}{\avariablebis}{\avariableter}}}
% \by{\defofbefore}{1,10,14,20,26}
% \end{nd}
% \]

\subsubsection{\ref{axiom2:firstbefore}}
\begin{enumerate}[align=left]
\item[\lemmalab{MeetFirstBefore}{axiom2:firstbefore}]
$
\boxed{
\begin{aligned}[t]
&(\before{\avariable}{\ameetvar{\avariablefour}{\avariablefifth}{\avariableter}}
\land \before{\avariablebis}{\ameetvar{\avariablefour}{\avariablefifth}{\avariableter}}
\land\\
&\ameetvar{\avariable}{\avariablebis}{\avariableter} \neq \ameetvar{\avariablefour}{\avariablefifth}{\avariableter})
\implies \before{\ameetvar{\avariable}{\avariablebis}{\avariableter}}{\ameetvar{\avariablefour}{\avariablefifth}{\avariableter}}
\end{aligned}
}
$
\[
\begin{nd}
\hypo {1} {\before{\avariable}{\ameetvar{\avariablefour}{\avariablefifth}{\avariableter}}}
\hypo {2} {\before{\avariablebis}{\ameetvar{\avariablefour}{\avariablefifth}{\avariableter}}}
\hypo {3} {\ameetvar{\avariable}{\avariablebis}{\avariableter} \neq \ameetvar{\avariablefour}{\avariablefifth}{\avariableter}}
\have {4} {\bigvee_{a \in \{\avariablefour,\avariablefifth\}} \big(
\before{\ameetvar{\avariable}{\avariable}{\avariable}}{\ameetvar{\avariable}{a}{\avariableter}} \land\\ \ameetvar{\avariable}{a}{\avariableter} = \ameetvar{\avariablefour}{\avariablefifth}{\avariableter}
\big)}
\by{\defofbefore}{1}
\open
\hypo {5} {\before{\ameetvar{\avariable}{\avariable}{\avariable}}{\ameetvar{\avariable}{a}{\avariableter}}} \by{where $a$ is $\avariablefour$ or $\avariablefifth$}{}
\hypo {6} {\ameetvar{\avariable}{a}{\avariableter} = \ameetvar{\avariablefour}{\avariablefifth}{\avariableter}}
\have {7} {\bigvee_{b \in \{a\}\cup(\{\avariablefour,\avariablefifth\}\setminus\{a\})}\\ \big(
\before{\ameetvar{\avariablebis}{\avariablebis}{\avariablebis}}{\ameetvar{\avariablebis}{b}{\avariableter}} \land\\ \ameetvar{\avariablebis}{b}{\avariableter} = \ameetvar{\avariablefour}{\avariablefifth}{\avariableter} \big)}
\by{\defofbefore}{2}
\open
\hypo {8} {\before{\ameetvar{\avariablebis}{\avariablebis}{\avariablebis}}{\ameetvar{\avariablebis}{b}{\avariableter}}} \by{where $b = a$ (syntactically)}{}
\hypo {9} {\ameetvar{\avariablebis}{b}{\avariableter} = \ameetvar{\avariablefour}{\avariablefifth}{\avariableter}}
\have {10} {\ameetvar{\avariable}{a}{\avariableter} = \ameetvar{\avariablebis}{a}{\avariableter}} \by{\ref{core2Ax:Substitute}, renaming $b$ in $a$}{6,9}
\have {11} {\symmetric{\ameetvar{\avariable}{\avariablebis}{\avariableter}}} \by{\ref{core2Ax:Symmetric}}{10}
\have {12} {\defined{\ameetvar{\avariable}{a}{\avariableter}}} \by{\ref{axiom2:auxlemma1}}{10}
\have {13} {\ameetvar{\avariable}{\avariablebis}{\avariableter} \neq \ameetvar{\avariable}{a}{\avariableter}} \by{\ref{core2Ax:Substitute}}{3,6}
\have {14} {\ameetvar{\avariable}{\avariablebis}{\avariableter} \neq \ameetvar{\avariablebis}{a}{\avariableter}} \by{\ref{core2Ax:Substitute}}{3,9}
\have {15} {\before{\ameetvar{\avariable}{\avariablebis}{\avariableter}}{\ameetvar{\avariable}{a}{\avariableter}}}
\by{\defofbefore}{11,12,13,14}
\have {16} {\before{\ameetvar{\avariable}{\avariablebis}{\avariableter}}{\ameetvar{\avariablefour}{\avariablefifth}{\avariableter}}}
\by{\ref{axiom2:beforelemma0two}}{6,15}
\close
\open
\hypo {17} {\before{\ameetvar{\avariablebis}{\avariablebis}{\avariablebis}}{\ameetvar{\avariablebis}{b}{\avariableter}}} \by{where $b \neq a$ (syntactically)}{}
\hypo {18} {\ameetvar{\avariablebis}{b}{\avariableter} = \ameetvar{\avariablefour}{\avariablefifth}{\avariableter}}
\have {19} {\ameetvar{\avariable}{a}{\avariableter} = \ameetvar{\avariablebis}{b}{\avariableter}} \by{\ref{core2Ax:Substitute}}{6,18}
\have {20} {\ameetvar{\avariable}{a}{\avariableter} = \ameetvar{\avariable}{\avariablebis}{\avariableter} \lor\\ \ameetvar{\avariable}{a}{\avariableter}=\ameetvar{\avariable}{b}{\avariableter}} \by{\ref{core2Ax:Symmetric}}{19}
\open
\hypo {21} {\ameetvar{\avariable}{a}{\avariableter} = \ameetvar{\avariable}{\avariablebis}{\avariableter}}
\have {22} {\ameetvar{\avariablefour}{\avariablefifth}{\avariableter} = \ameetvar{\avariable}{\avariablebis}{\avariableter}} \by{\ref{core2Ax:Substitute}}{6,21}
\have {23} {\bottom} \by{\landcontr}{3,22}
\close
\have {24} {\ameetvar{\avariable}{a}{\avariableter} \neq \ameetvar{\avariable}{\avariablebis}{\avariableter}} \ni{21-23}
\have {25} {\ameetvar{\avariable}{a}{\avariableter}=\ameetvar{\avariable}{b}{\avariableter}} \by{\modusponens}{}
\have {25b}  {\ameetvar{\avariable}{b}{\avariableter} = \ameetvar{\avariablefour}{\avariablefifth}{\avariableter}} \by{\ref{core2Ax:Substitute}}{6,25}
\have {26} {\ameetvar{\avariable}{b}{\avariableter} = \ameetvar{\avariablebis}{b}{\avariableter}}
 \by{\ref{core2Ax:Substitute}}{19,25}
\have {27} {\symmetric{\ameetvar{\avariable}{\avariablebis}{\avariableter}}} \by{\ref{core2Ax:Symmetric}}{26}
\have {28} {\defined{\ameetvar{\avariable}{b}{\avariableter}}} \by{\ref{axiom2:auxlemma1}}{26}
\have {29} {\ameetvar{\avariable}{\avariablebis}{\avariableter} \neq \ameetvar{\avariable}{b}{\avariableter}} \by{\ref{core2Ax:Substitute}}{3,25b}
\have {30} {\ameetvar{\avariable}{\avariablebis}{\avariableter} \neq \ameetvar{\avariablebis}{b}{\avariableter}} \by{\ref{core2Ax:Substitute}}{3,9}
\have {31} {\before{\ameetvar{\avariable}{\avariablebis}{\avariableter}}{\ameetvar{\avariable}{b}{\avariableter}}}
\by{\defofbefore}{27,28,29,30}
\end{nd}
\]
\[
\begin{ndresume}
\have {32} {\before{\ameetvar{\avariable}{\avariablebis}{\avariableter}}{\ameetvar{\avariablefour}{\avariablefifth}{\avariableter}}}
\by{\ref{axiom2:beforelemma0two}}{25b,31}
\close
\have {33} {\before{\ameetvar{\avariable}{\avariablebis}{\avariableter}}{\ameetvar{\avariablefour}{\avariablefifth}{\avariableter}}}
\oe{7,8-16,17-32}
\close
\have {34} {\before{\ameetvar{\avariable}{\avariablebis}{\avariableter}}{\ameetvar{\avariablefour}{\avariablefifth}{\avariableter}}}
\oe{4,5-33}
\end{ndresume}
\]
\end{enumerate}

\subsubsection{\ref{axiom2:samelooplemma0three}}
\begin{enumerate}[align=left]
\item[\lemmalab{AsymSubscript}{axiom2:samelooplemma0three}]
$
\boxed{\asymmetric{\ameetvar{\avariable}{\avariablebis}{\avariableter}} \land \avariableter \neq \ameetvar{\avariable}{\avariablebis}{\avariableter}\implies \sameloop{\ameetvar{\avariable}{\avariablebis}{\avariableter}}{\avariableter}}
$\\
\[
\begin{nd}
\hypo {1} {\asymmetric{\ameetvar{\avariable}{\avariablebis}{\avariableter}}}
\hypo {2} {\avariableter \neq \ameetvar{\avariable}{\avariablebis}{\avariableter}}
\have {3} {\defined{\ameetvar{\avariable}{\avariablebis}{\avariableter}}} \ae{1}
\have {4} {\defined{\ameetvar{\avariableter}{\avariable}{\avariableter}}} \by{\ref{axiom2:auxlemmaPedDef}}{3}
\have {5} {\defined{\ameetvar{\avariable}{\avariableter}{\avariableter}}} \by{\ref{core2Ax:Bothdef}}{4}
\open
\hypo {6} {\symmetric{\ameetvar{\avariable}{\avariableter}{\avariableter}}}
\have {7} {\ameetvar{\avariableter}{\avariablebis}{\avariableter} = \ameetvar{\avariable}{\avariablebis}{\avariableter}}
\by{\ref{core2Ax:OneAsym}}{1,6}
\have {8} {\defined{\ameetvar{\avariableter}{\avariablebis}{\avariableter}}} \by{\ref{axiom2:auxlemma1}}{7}
\have {9} {\avariableter = \ameetvar{\avariableter}{\avariablebis}{\avariableter}} \by{\ref{core2Ax:Self2}}{8}
\have {10} {\avariableter = \ameetvar{\avariable}{\avariablebis}{\avariableter}} \by{\ref{core2Ax:Substitute}}{7,9}
\have {11} {\bottom} \by{\landcontr}{2,10}
\close
\have {12} {\lnot \symmetric{\ameetvar{\avariable}{\avariableter}{\avariableter}}} \ni{6-11}
\have {13} {\asymmetric{\ameetvar{\avariable}{\avariableter}{\avariableter}}} \by{\ndref{5} $\land$ \ndref{12}}{}
\have {14}
{\ameetvar{\avariable}{\avariablebis}{\avariableter} = \ameetvar{\avariable}{\avariableter}{\avariableter}}
\by{\ref{core2Ax:BothAsym}}{1,13}
\have {15} {\avariableter = \ameetvar{\avariableter}{\avariable}{\avariableter}} \by{\ref{core2Ax:Self2}}{4}
\have {16} {\avariableter = \ameetvar{\avariableter}{\avariableter}{\avariableter}} \by{\ref{core2Ax:Self}}{}
\have {17}
{\ameetvar{\avariableter}{\avariableter}{\avariableter} = \ameetvar{\avariableter}{\avariable}{\avariableter}}
\by{\ref{core2Ax:Substitute}}{15,16}
\have {18} {\sameloop{\ameetvar{\avariable}{\avariablebis}{\avariableter}}{\avariableter}}
\by{\defofsameloop}{13,14,17}
\end{nd}
\]
\end{enumerate}

% \item
% $
% \boxed{ \before{\aterm_1}{\aterm_2} \land \aterm_1 = \aterm_3 \implies \before{\aterm_3}{\aterm_2}}
% $
%
% This is a generalisation of \ref{axiom2:auxlemma9} and \ref{axiom2:auxlemma10}.
% It is sufficient to prove the result for $\aterm_1$, $\aterm_2$ and $\aterm_3$ meet-point expressions,
% as $\avariable = \ameetvar{\avariable}{\avariable}{\avariable}$ by axiom~\ref{core2Ax:Self} and
% by definition $\before{\avariable}{\aterm} = \before{\ameetvar{\avariable}{\avariable}{\avariable}}{\aterm}$ and $\before{\aterm}{\avariable} = \before{\aterm}{\ameetvar{\avariable}{\avariable}{\avariable}}$.
% \[
% \begin{nd}
% \hypo {1} {\before{\ameetvar{\avariable}{\avariablebis}{\avariableter}}{\ameetvar{\avariablefour}{\avariablefifth}{\avariablesix}}}
% \hypo {2} {\ameetvar{\avariable}{\avariablebis}{\avariableter} = \ameetvar{\avariablesept}{\avariableoct}{\avariablenine}}
% \have {3} {\defined{\ameetvar{\avariablesept}{\avariableoct}{\avariablenine}}} \by{\ref{axiom2:auxlemma1}}{2}
% \have {3b} {\defined{\ameetvar{\avariableoct}{\avariablesept}{\avariablenine}}} \by{\ref{core2Ax:Bothdef}}{3}
% \have {4} {\defined{\ameetvar{\avariablesept}{\avariableoct}{\avariableter}}} \by{\ref{core2Ax:PedInv}}{2}
% \have {5} {\ameetvar{\avariablesept}{\avariableoct}{\avariablenine} = \ameetvar{\avariablesept}{\avariableoct}{\avariableter}} \by{\ref{core2Ax:EqDef}}{3,4}
% \have {6} {\ameetvar{\avariable}{\avariablebis}{\avariableter} = \ameetvar{\avariablesept}{\avariableoct}{\avariableter}} \by{\ref{core2Ax:Substitute}}{2,5}
% \have {7} {\ameetvar{\avariablesept}{\avariableoct}{\avariableter} = \ameetvar{\avariable}{\avariablebis}{\avariableter}} \by{\ref{core2Ax:EqSymm}}{6}
% \have {8} {\ameetvar{\avariablesept}{\avariableoct}{\avariableter} = \ameetvar{\avariablesept}{\avariable}{\avariableter} \lor \ameetvar{\avariablesept}{\avariableoct}{\avariableter} = \ameetvar{\avariableoct}{\avariable}{\avariableter}} \by{\ref{core2Ax:Symmetric}}{7}
% \open
% \hypo {A1} {\ameetvar{\avariablesept}{\avariableoct}{\avariableter} = \ameetvar{\avariablesept}{\avariable}{\avariableter}}
% \have {A1b} {\ameetvar{\avariable}{\avariablebis}{\avariableter} = \ameetvar{\avariablesept}{\avariable}{\avariableter}} \by{\ref{core2Ax:Substitute}}{7,A1}
% \have {A2} {\symmetric{\ameetvar{\avariable}{\avariablesept}{\avariableter}}} \by{\ref{core2Ax:Symmetric}}{A1b}
% \have {AA} {\ameetvar{\avariable}{\avariablebis}{\avariableter} = \ameetvar{\avariable}{\avariablesept}{\avariableter}} \by{\ref{core2Ax:Substitute}}{A1,A2}
% \have {A3} {\bigvee_{a \in \{\avariablefour,\avariablefifth\}} \before{\ameetvar{\avariable}{\avariablebis}{\avariableter}}{\ameetvar{\avariable}{a}{\avariablesix}}
% \land \ameetvar{\avariable}{a}{\avariablesix} = \ameetvar{\avariablefour}{\avariablefifth}{\avariablesix}
% }
% \by{\defofbefore}{1}
% \end{nd}
% \]
% \[
% \begin{ndresume}
% %1 of 4
% \open
% \hypo {A4a} {\before{\ameetvar{\avariable}{\avariablebis}{\avariableter}}{\ameetvar{\avariable}{\avariablefour}{\avariablesix}}}
% \hypo {A4b} {\ameetvar{\avariable}{\avariablefour}{\avariablesix} = \ameetvar{\avariablefour}{\avariablefifth}{\avariablesix}}
% \have {A6} {\before{\ameetvar{\avariable}{\avariablesept}{\avariableter}}{\ameetvar{\avariable}{\avariablefour}{\avariablesix}}} \by{\ref{axiom2:auxlemma10}}{AA,A4a}
% \have {A7} {\before{\ameetvar{\avariablesept}{\avariable}{\avariableter}}{\ameetvar{\avariablesept}{\avariablefour}{\avariablesix}} \land \ameetvar{\avariablesept}{\avariablefour}{\avariablesix} = \ameetvar{\avariable}{\avariablefour}{\avariablesix}} \by{\ref{axiom2:auxlemma5}}{A6}
% \have {A8} {\before{\ameetvar{\avariablesept}{\avariable}{\avariableter}}{\ameetvar{\avariablesept}{\avariablefour}{\avariablesix}}} \ae{A7}
% \have {A9} {\ameetvar{\avariablesept}{\avariablefour}{\avariablesix} = \ameetvar{\avariable}{\avariablefour}{\avariablesix}} \ae{A7}
% \have {A10} {\before{\ameetvar{\avariablesept}{\avariableoct}{\avariableter}}{\ameetvar{\avariablesept}{\avariablefour}{\avariablesix}}} \by{\ref{axiom2:auxlemma10}}{A1,A8}
% \have {A11} {\before{\ameetvar{\avariablesept}{\avariableoct}{\avariablenine}}{\ameetvar{\avariablesept}{\avariablefour}{\avariablesix}}} \by{\ref{axiom2:auxlemma9}}{3,A10}
% \have {A12} {\ameetvar{\avariablesept}{\avariablefour}{\avariablesix} = \ameetvar{\avariablefour}{\avariablefifth}{\avariablesix}} \by{\ref{core2Ax:Substitute}}{A4b,A9}
% \have {A13} {\before{\ameetvar{\avariablesept}{\avariableoct}{\avariablenine}}{\ameetvar{\avariablesept}{\avariablefour}{\avariablesix}} \land \ameetvar{\avariablesept}{\avariablefour}{\avariablesix} = \ameetvar{\avariablefour}{\avariablefifth}{\avariablesix}} \by{\ndref{A11} $\land$ \ndref{A12}}{}
% \have {A14}
% {\bigvee_{a \in \{\avariablefour,\avariablefifth\}} \before{\ameetvar{\avariablesept}{\avariableoct}{\avariablenine}}{\ameetvar{\avariablesept}{a}{\avariablesix}}
% \land \ameetvar{\avariablesept}{a}{\avariablesix} = \ameetvar{\avariablefour}{\avariablefifth}{\avariablesix}
% }
% \by{$\aformula \Rightarrow \aformula \lor \aformulabis$}{A13}
% \have {A15}
% {\before{\ameetvar{\avariablesept}{\avariableoct}{\avariablenine}}{\ameetvar{\avariablefour}{\avariablefifth}{\avariablesix}}} \by{\defofbefore}{A14}
% \close
% %2 of 4
% \open
% \hypo {B1} {\before{\ameetvar{\avariable}{\avariablebis}{\avariableter}}{\ameetvar{\avariable}{\avariablefifth}{\avariablesix}}}
% \hypo {B2} {\ameetvar{\avariable}{\avariablefifth}{\avariablesix} = \ameetvar{\avariablefour}{\avariablefifth}{\avariablesix}}
% \have {B3} {\before{\ameetvar{\avariable}{\avariablesept}{\avariableter}}{\ameetvar{\avariable}{\avariablefifth}{\avariablesix}}} \by{\ref{axiom2:auxlemma10}}{AA,B1}
% \have {B4} {\before{\ameetvar{\avariablesept}{\avariable}{\avariableter}}{\ameetvar{\avariablesept}{\avariablefifth}{\avariablesix}} \land \ameetvar{\avariablesept}{\avariablefifth}{\avariablesix} = \ameetvar{\avariable}{\avariablefifth}{\avariablesix}} \by{\ref{axiom2:auxlemma5}}{B3}
% \have {B5} {\before{\ameetvar{\avariablesept}{\avariable}{\avariableter}}{\ameetvar{\avariablesept}{\avariablefifth}{\avariablesix}}} \ae{B4}
% \have {B6} {\ameetvar{\avariablesept}{\avariablefifth}{\avariablesix} = \ameetvar{\avariable}{\avariablefifth}{\avariablesix}} \ae{B4}
% \have {B7} {\before{\ameetvar{\avariablesept}{\avariableoct}{\avariableter}}{\ameetvar{\avariablesept}{\avariablefifth}{\avariablesix}}} \by{\ref{axiom2:auxlemma10}}{A1,B5}
% \have {B8} {\before{\ameetvar{\avariablesept}{\avariableoct}{\avariablenine}}{\ameetvar{\avariablesept}{\avariablefifth}{\avariablesix}}} \by{\ref{axiom2:auxlemma9}}{3,B7}
% \have {B9} {\ameetvar{\avariablesept}{\avariablefifth}{\avariablesix} = \ameetvar{\avariablefour}{\avariablefifth}{\avariablesix}} \by{\ref{core2Ax:Substitute}}{B2,B6}
% \have {B10} {\before{\ameetvar{\avariablesept}{\avariableoct}{\avariablenine}}{\ameetvar{\avariablesept}{\avariablefifth}{\avariablesix}} \land \ameetvar{\avariablesept}{\avariablefifth}{\avariablesix} = \ameetvar{\avariablefour}{\avariablefifth}{\avariablesix}} \by{\ndref{B8} $\land$ \ndref{B9}}{}
% \have {B11}
% {\bigvee_{a \in \{\avariablefour,\avariablefifth\}} \before{\ameetvar{\avariablesept}{\avariableoct}{\avariablenine}}{\ameetvar{\avariablesept}{a}{\avariablesix}}
% \land \ameetvar{\avariablesept}{a}{\avariablesix} = \ameetvar{\avariablefour}{\avariablefifth}{\avariablesix}
% }
% \by{$\aformula \Rightarrow \aformula \lor \aformulabis$}{B10}
% \have {B12}
% {\before{\ameetvar{\avariablesept}{\avariableoct}{\avariablenine}}{\ameetvar{\avariablefour}{\avariablefifth}{\avariablesix}}} \by{\defofbefore}{B11}
% \close
% \have {twoOfFour}
% {\before{\ameetvar{\avariablesept}{\avariableoct}{\avariablenine}}{\ameetvar{\avariablefour}{\avariablefifth}{\avariablesix}}} \oe{A3,A4a-A15,B1-B12}
% \close
% \open
% \hypo {C1} {\ameetvar{\avariablesept}{\avariableoct}{\avariableter} = \ameetvar{\avariableoct}{\avariable}{\avariableter}}
% \have {C1a} {\symmetric{\ameetvar{\avariablesept}{\avariableoct}{\avariableter}}} \by{\ref{core2Ax:Symmetric}}{C1}
% \have {C1aa} {\ameetvar{\avariableoct}{\avariablesept}{\avariableter} = \ameetvar{\avariableoct}{\avariable}{\avariableter}} \by{\ref{core2Ax:Substitute}}{C1,C1a}
% \have {C2} {\ameetvar{\avariable}{\avariablebis}{\avariableter} = \ameetvar{\avariableoct}{\avariable}{\avariableter}}
% \by{\ref{core2Ax:Substitute}}{6,C1}
% \have {C3} {\symmetric{\ameetvar{\avariable}{\avariableoct}{\avariableter}}}
% \have {C4} {\ameetvar{\avariable}{\avariablebis}{\avariableter} = \ameetvar{\avariable}{\avariableoct}{\avariableter}} \by{\ref{core2Ax:Substitute}}{C2,C3}
% \have {C5} {\bigvee_{a \in \{\avariablefour,\avariablefifth\}} \before{\ameetvar{\avariable}{\avariablebis}{\avariableter}}{\ameetvar{\avariable}{a}{\avariablesix}}
% \land \ameetvar{\avariable}{a}{\avariablesix} = \ameetvar{\avariablefour}{\avariablefifth}{\avariablesix}
% }
% \by{\defofbefore}{1}
% \end{ndresume}
% \]
% \[
% \begin{ndresume}
% %3 of 4
% \open
% \hypo {D1} {\before{\ameetvar{\avariable}{\avariablebis}{\avariableter}}{\ameetvar{\avariable}{\avariablefour}{\avariablesix}}}
% \hypo {D2} {\ameetvar{\avariable}{\avariablefour}{\avariablesix} = \ameetvar{\avariablefour}{\avariablefifth}{\avariablesix}}
% \have {D3} {\before{\ameetvar{\avariable}{\avariableoct}{\avariableter}}{\ameetvar{\avariable}{\avariablefour}{\avariablesix}}} \by{\ref{axiom2:auxlemma10}}{C4,D1}
% \have {D4} {\before{\ameetvar{\avariableoct}{\avariable}{\avariableter}}{\ameetvar{\avariableoct}{\avariablefour}{\avariablesix}} \land \ameetvar{\avariableoct}{\avariablefour}{\avariablesix} = \ameetvar{\avariable}{\avariablefour}{\avariablesix}} \by{\ref{axiom2:auxlemma5}}{D3}
% \have {D5} {\before{\ameetvar{\avariableoct}{\avariable}{\avariableter}}{\ameetvar{\avariableoct}{\avariablefour}{\avariablesix}}} \ae{D4}
% \have {D6} {\ameetvar{\avariableoct}{\avariablefour}{\avariablesix} = \ameetvar{\avariable}{\avariablefour}{\avariablesix}} \ae{D4}
% \have {D7} {\before{\ameetvar{\avariableoct}{\avariablesept}{\avariableter}}{\ameetvar{\avariableoct}{\avariablefour}{\avariablesix}}} \by{\ref{axiom2:auxlemma10}}{C1aa,D5}
% \have {D7a}
% {\before{\ameetvar{\avariableoct}{\avariablesept}{\avariablenine}}{\ameetvar{\avariableoct}{\avariablefour}{\avariablesix}}} \by{\ref{axiom2:auxlemma9}}{3b,D7}
% \have {D8} {\before{\ameetvar{\avariablesept}{\avariableoct}{\avariablenine}}{\ameetvar{\avariablesept}{\avariablefour}{\avariablesix}} \land \ameetvar{\avariablesept}{\avariablefour}{\avariablesix} = \ameetvar{\avariableoct}{\avariablefour}{\avariablesix}} \by{\ref{axiom2:auxlemma5}}{D7a}
% \have {D9} {\before{\ameetvar{\avariablesept}{\avariableoct}{\avariablenine}}{\ameetvar{\avariablesept}{\avariablefour}{\avariablesix}}}
% \ae{D8}
% \have {D10} {\ameetvar{\avariablesept}{\avariablefour}{\avariablesix} = \ameetvar{\avariableoct}{\avariablefour}{\avariablesix}}
% \ae{D8}
% \have {D11} {\ameetvar{\avariablesept}{\avariablefour}{\avariablesix} = \ameetvar{\avariable}{\avariablefour}{\avariablesix}} \by{\ref{core2Ax:Substitute}}{D6,D10}
% \have {D12} {\ameetvar{\avariablesept}{\avariablefour}{\avariablesix} = \ameetvar{\avariablefour}{\avariablefifth}{\avariablesix}} \by{\ref{core2Ax:Substitute}}{D2,D11}
% \have {D13} {\before{\ameetvar{\avariablesept}{\avariableoct}{\avariablenine}}{\ameetvar{\avariablesept}{\avariablefour}{\avariablesix}} \land \ameetvar{\avariablesept}{\avariablefour}{\avariablesix} = \ameetvar{\avariablefour}{\avariablefifth}{\avariablesix}} \by{\ndref{D9} $\land$ \ndref{D12}}{}
% \have {D14}
% {\bigvee_{a \in \{\avariablefour,\avariablefifth\}} \before{\ameetvar{\avariablesept}{\avariableoct}{\avariablenine}}{\ameetvar{\avariablesept}{a}{\avariablesix}}
% \land \ameetvar{\avariablesept}{a}{\avariablesix} = \ameetvar{\avariablefour}{\avariablefifth}{\avariablesix}
% }
% \by{$\aformula \Rightarrow \aformula \lor \aformulabis$}{D13}
% \have {D15}
% {\before{\ameetvar{\avariablesept}{\avariableoct}{\avariablenine}}{\ameetvar{\avariablefour}{\avariablefifth}{\avariablesix}}} \by{\defofbefore}{D14}
% \close
% %4 of 4
% \open
% \hypo {E1} {\before{\ameetvar{\avariable}{\avariablebis}{\avariableter}}{\ameetvar{\avariable}{\avariablefour}{\avariablesix}}}
% \hypo {E2} {\ameetvar{\avariable}{\avariablefifth}{\avariablesix} = \ameetvar{\avariablefour}{\avariablefifth}{\avariablesix}}
% \have {E3} {\before{\ameetvar{\avariable}{\avariableoct}{\avariableter}}{\ameetvar{\avariable}{\avariablefifth}{\avariablesix}}} \by{\ref{axiom2:auxlemma10}}{C4,E1}
% \have {E4} {\before{\ameetvar{\avariableoct}{\avariable}{\avariableter}}{\ameetvar{\avariableoct}{\avariablefifth}{\avariablesix}} \land \ameetvar{\avariableoct}{\avariablefifth}{\avariablesix} = \ameetvar{\avariable}{\avariablefifth}{\avariablesix}} \by{\ref{axiom2:auxlemma5}}{E3}
% \have {E5} {\before{\ameetvar{\avariableoct}{\avariable}{\avariableter}}{\ameetvar{\avariableoct}{\avariablefifth}{\avariablesix}}} \ae{E4}
% \have {E6} {\ameetvar{\avariableoct}{\avariablefifth}{\avariablesix} = \ameetvar{\avariable}{\avariablefifth}{\avariablesix}} \ae{E4}
% \have {E7} {\before{\ameetvar{\avariableoct}{\avariablesept}{\avariableter}}{\ameetvar{\avariableoct}{\avariablefifth}{\avariablesix}}} \by{\ref{axiom2:auxlemma10}}{C1aa,E5}
% \have {E7a}
% {\before{\ameetvar{\avariableoct}{\avariablesept}{\avariablenine}}{\ameetvar{\avariableoct}{\avariablefifth}{\avariablesix}}} \by{\ref{axiom2:auxlemma9}}{3b,E7}
% \have {E8} {\before{\ameetvar{\avariablesept}{\avariableoct}{\avariablenine}}{\ameetvar{\avariablesept}{\avariablefifth}{\avariablesix}} \land \ameetvar{\avariablesept}{\avariablefifth}{\avariablesix} = \ameetvar{\avariableoct}{\avariablefifth}{\avariablesix}} \by{\ref{axiom2:auxlemma5}}{E7a}
% \have {E9} {\before{\ameetvar{\avariablesept}{\avariableoct}{\avariablenine}}{\ameetvar{\avariablesept}{\avariablefifth}{\avariablesix}}}
% \ae{E8}
% \have {E10} {\ameetvar{\avariablesept}{\avariablefifth}{\avariablesix} = \ameetvar{\avariableoct}{\avariablefifth}{\avariablesix}}
% \ae{E8}
% \have {E11} {\ameetvar{\avariablesept}{\avariablefifth}{\avariablesix} = \ameetvar{\avariable}{\avariablefifth}{\avariablesix}} \by{\ref{core2Ax:Substitute}}{E6,E10}
% \have {E12} {\ameetvar{\avariablesept}{\avariablefifth}{\avariablesix} = \ameetvar{\avariablefour}{\avariablefifth}{\avariablesix}} \by{\ref{core2Ax:Substitute}}{E2,E11}
% \have {E13} {\before{\ameetvar{\avariablesept}{\avariableoct}{\avariablenine}}{\ameetvar{\avariablesept}{\avariablefifth}{\avariablesix}} \land \ameetvar{\avariablesept}{\avariablefifth}{\avariablesix} = \ameetvar{\avariablefour}{\avariablefifth}{\avariablesix}} \by{\ndref{E9} $\land$ \ndref{E12}}{}
% \have {E14}
% {\bigvee_{a \in \{\avariablefour,\avariablefifth\}} \before{\ameetvar{\avariablesept}{\avariableoct}{\avariablenine}}{\ameetvar{\avariablesept}{a}{\avariablesix}}
% \land \ameetvar{\avariablesept}{a}{\avariablesix} = \ameetvar{\avariablefour}{\avariablefifth}{\avariablesix}
% }
% \by{$\aformula \Rightarrow \aformula \lor \aformulabis$}{E13}
% \have {E15}
% {\before{\ameetvar{\avariablesept}{\avariableoct}{\avariablenine}}{\ameetvar{\avariablefour}{\avariablefifth}{\avariablesix}}} \by{\defofbefore}{E14}
% \close
% \have {fourOfFour}
% {\before{\ameetvar{\avariablesept}{\avariableoct}{\avariablenine}}{\ameetvar{\avariablefour}{\avariablefifth}{\avariablesix}}} \oe{C5,D1-D15,E1-E15}
% \close
% \have {done}
% {\before{\ameetvar{\avariablesept}{\avariableoct}{\avariablenine}}{\ameetvar{\avariablefour}{\avariablefifth}{\avariablesix}}} \oe{8,A1-twoOfFour,C1-fourOfFour}
% \end{ndresume}
% \]

\begin{enumerate}[align=left]
\item[\lemmalab{Eq>Sees}{axiom2:eqpreservesees}]
$
\boxed{\aterm_3 = \aterm_4 \implies (\seesgeq{\aterm_1}{\aterm_2}{\asetmeetvar\cup \{\aterm_3\}}{\inbound} \iff \seesgeq{\aterm_1}{\aterm_2}{\asetmeetvar \cup \{\aterm_3,\aterm_4\}}{\inbound})}
$\\
The left to right direction of the double implication is by \ref{core2Ax:SeesTermEq}
wereas the right to left direction is axiom~\ref{core2Ax:SeesMono1}.

\item[\lemmalab{$\lnot$Def>Sees}{axiom2:seesnotdef}]
$
\boxed{\lnot \defined{\aterm_3} \implies (\seesgeq{\aterm_1}{\aterm_2}{\asetmeetvar}{\inbound} \iff \seesgeq{\aterm_1}{\aterm_2}{\asetmeetvar \cup \{\aterm_3\}}{\inbound})}
$\\
We only show the left to right direction of the double implication as the right to left direction is axiom~\ref{core2Ax:SeesMono1}.
\[
\begin{nd}
\hypo {2} {\lnot \defined{\aterm_3}}
\hypo {1} {\seesgeq{\aterm_1}{\aterm_2}{\asetmeetvar}{\inbound}}
\have {3} {\sees{\aterm_1}{\aterm_2}{\asetmeetvar}} \by{repeated applications of \ref{core2Ax:SeesMono2}}{1}
\open
\hypo {4} {\lnot \sees{\aterm_1}{\aterm_2}{\{\aterm_3\}}}
\have {5} {\sees{\aterm_1}{\aterm_3}{\asetmeetvar} \land \sees{\aterm_3}{\aterm_2}{\asetmeetvar}} \by{\ref{core2Ax:SeesNegSum}}{4}
\have {6} {\defined{\aterm_3}} \by{\ref{core2Ax:SeesDef}}{5}
\have {7} {\bottom} \by{\landcontr}{2,6}
\close
\have {8} {\sees{\aterm_1}{\aterm_2}{\{\aterm_3\}}} \ni{4-7}
\have {9} {\seesgeq{\aterm_1}{\aterm_2}{\asetmeetvar\cup \{\aterm_3\}}{\inbound }} \by{\ref{core2Ax:SeesMax}}{1,8}
\end{nd}
\]
\end{enumerate}

\subsubsection{\ref{axiom2:seeslengthpreserved2}}
\begin{enumerate}[align=left]
\item[\lemmalab{SeesLengthPreserved}{axiom2:seeslengthpreserved2}]
$
\boxed{
\begin{aligned}[t]
&
\aterm \in \asetmeetvar \implies\\
&(\sees{\aterm_1}{\aterm_2}{\asetmeetvar\cup\{\aterm\}}{=}{\inbound} \iff \sees{\aterm_1}{\aterm_2}{\asetmeetvar}{=}{\inbound})
\end{aligned}}
$\\
Left to right direction of the double implication is a weaker version of \ref{axiom2:seeslengthpreserved}. For the right to left direction:
\[
\begin{nd}
\hypo {1} {\seesgeq{\aterm_1}{\aterm_2}{\asetmeetvar}{\inbound}}
\hypo {2} {\lnot \seesgeq{\aterm_1}{\aterm_2}{\asetmeetvar}{\inbound{+}1}}
\hypo {2b} {\aterm_3 \in \asetmeetvar}
\have {3} {\seesgeq{\aterm_1}{\aterm_2}{\asetmeetvar\cup \{\aterm_3\}}{\inbound}} \by{\ref{core2Ax:SeesTermEq}}{1}
\open
\hypo {4}{\seesgeq{\aterm_1}{\aterm_2}{\asetmeetvar \cup \{\aterm_3\}}{\inbound{+}1}}
\have {5} {\seesgeq{\aterm_1}{\aterm_2}{\asetmeetvar}{\inbound{+}1}} \by{\ref{core2Ax:SeesMono1}}{1,4}
\have {6} {\bottom} \by{\landcontr}{2,5}
\close
\have {7} {\lnot \seesgeq{\aterm_1}{\aterm_2}{\asetmeetvar \cup \{\aterm_3\}}{\inbound{+}1}} \ni{4-6}
\have {8} {\sees{\aterm_1}{\aterm_2}{\asetmeetvar\cup \{\aterm_3\}}{=}{\inbound}} \by{\ndref{3} $\land$ \ndref{7}}{}
\end{nd}
\]
\end{enumerate}

\subsubsection{\ref{axiom2:strictsees}}
\begin{enumerate}[align=left]
\item[\lemmalab{StrictSees}{axiom2:strictsees}]
$
\boxed{\sees{\aterm_1}{\aterm_2}{\asetmeetvar} \implies \bigwedge_{\aterm_3 \in \asetmeetvar} \lnot (\before{\aterm_1}{\aterm_3} \land \before{\aterm_3}{\aterm_2})}
$\\
By absurd, we prove that if there is $\aterm_3 \in \asetmeetvar$ such that $\before{\aterm_1}{\aterm_3} \land \before{\aterm_3}{\aterm_2}$, then from
$\sees{\aterm_1}{\aterm_2}{\asetmeetvar}$ we reach a contradiction.
\[
\begin{nd}
\hypo {1} {\sees{\aterm_1}{\aterm_2}{\asetmeetvar}}
\hypo {2} {\before{\aterm_1}{\aterm_3} \land \before{\aterm_3}{\aterm_2}} \by{for some $\aterm_3 \in \asetmeetvar$}{}
\have {3} {\lnot \sees{\aterm_1}{\aterm_2}{\{\aterm_3\}}} \by{\ref{axiom2:beforesees}}{2}
\have {4} {\sees{\aterm_1}{\aterm_2}{\{\aterm_3\}}} \by{repeated application of \ref{core2Ax:SeesMono1}}{1}
\have {5} {\bottom} \by{\landcontr}{3,4}
\end{nd}
\]
\end{enumerate}

\subsection{Intermediate tautologies about $\mathtt{rem}$}
\label{subsection-intermediate-tautologies-rem}
\input{appendixproofs/apdxsection-int-taut-rem}

\begin{enumerate}[align=left]
\item[\lemmalab{Eq>RemL}{axiom2:eqpreserveremL}]
$\boxed{\aterm_1 = \aterm_2 \implies  (\remgeq{\{\pair{\aterm_1}{\aterm_3}\} \cup \asetpath}{\inbound} \iff \remgeq{\{\pair{\aterm_1}{\aterm_3},\pair{\aterm_2}{\aterm_3}\} \cup \asetpath}{\inbound})}$\\
The left to right direction of the double implication is by \ref{core2Ax:RemTEq1}
wereas the right to left direction is axiom~\ref{core2Ax:RemMono2}.

\item[\lemmalab{Eq>RemR}{axiom2:eqpreserveremR}]
$\boxed{\aterm_1 = \aterm_2 \implies (\remgeq{\{\pair{\aterm_3}{\aterm_1}\} \cup \asetpath}{\inbound} \iff \remgeq{\{\pair{\aterm_3}{\aterm_1},\pair{\aterm_3}{\aterm_2}\} \cup \asetpath}{\inbound})}$\\
The left to right direction of the double implication is by \ref{core2Ax:RemTEq2}
wereas the right to left direction is axiom~\ref{core2Ax:RemMono2}.

\item[\lemmalab{$\lnot$Def>RemL}{axiom2:remnotdefL}]
$
\boxed{\lnot \defined{\aterm_1} \implies (\remgeq{\asetpath}{\inbound} \iff \remgeq{\asetpath \cup \{(\aterm_1,\aterm_2)\}}{\inbound})}
$\\
We only show the left to right direction of the double implication as the right to left direction is axiom~\ref{core2Ax:RemMono2}.
\[
\begin{nd}
\hypo {1} {\remgeq{\asetpath}{\inbound}}
\hypo {2} {\lnot \defined{\aterm_1}}
\open
\hypo {4} {\sees{\aterm_1}{\aterm_2}{\emptyset}}
\have {6} {\defined{\aterm_1}} \by{\ref{core2Ax:SeesDef}}{4}
\have {7} {\bottom} \by{\landcontr}{2,6}
\close
\have {8} {\lnot\sees{\aterm_1}{\aterm_2}{\emptyset}} \ni{4-7}
\have {9} {\remgeq{\asetpath \cup \{(\aterm_1,\aterm_2)\}}{\inbound}} \by{\ref{core2Ax:RemNotSees}}{1,8}
\end{nd}
\]

\item[\lemmalab{$\lnot$Def>RemR}{axiom2:remnotdefR}]
$
\boxed{\lnot \defined{\aterm_1} \implies (\remgeq{\asetpath}{\inbound} \iff \remgeq{\asetpath \cup \{(\aterm_2,\aterm_1)\}}{\inbound})}
$\\
We only show the left to right direction of the double implication as the right to left direction is axiom~\ref{core2Ax:RemMono2}.
\[
\begin{nd}
\hypo {2} {\lnot \defined{\aterm_1}}
\hypo {1} {\remgeq{\asetpath}{\inbound}}
\open
\hypo {4} {\sees{\aterm_2}{\aterm_1}{\emptyset}}
\have {6} {\defined{\aterm_1}} \by{\ref{core2Ax:SeesDef}}{4}
\have {7} {\bottom} \by{\landcontr}{2,6}
\close
\have {8} {\lnot\sees{\aterm_2}{\aterm_1}{\emptyset}} \ni{4-7}
\have {9} {\remgeq{\asetpath \cup \{(\aterm_2,\aterm_1)\}}{\inbound}} \by{\ref{core2Ax:RemNotSees}}{1,8}
\end{nd}
\]
\end{enumerate}

\subsubsection{\ref{axiom2:remeqpreserved}}
\begin{enumerate}[align=left]
\item[\lemmalab{RemEqPreserved}{axiom2:remeqpreserved}]
$
\boxed{
\begin{aligned}[t]
&(\textstyle\bigvee_{\pair{\aterm_3}{\aterm_4} \in \asetpath} (\aterm_3 = \aterm_1 \land \aterm_2 = \aterm_4)) \implies\\
&(\rem{\{\pair{\aterm_1}{\aterm_2}\}\cup\asetpath}{=}{\inbound} \iff  \rem{\asetpath}{=}{\inbound})
\end{aligned}}
$\\
We show one direction of the double implication. The other direction is analogous.
\[
\begin{nd}
\hypo {1} {\remgeq{\{\pair{\aterm_1}{\aterm_2}\}\cup\asetpath}{\inbound}}
\hypo {2} {\lnot\remgeq{\{\pair{\aterm_1}{\aterm_2}\}\cup\asetpath}{\inbound{+}1}}
\hypo {3} {\bigvee_{\pair{\aterm_3}{\aterm_4} \in \asetpath} (\aterm_3 = \aterm_1 \land \aterm_2 = \aterm_4)}
\have {4} {\remgeq{\asetpath}{\inbound}} \by{\ref{core2Ax:RemMono2}}{1}
\open
\hypo {5} {\remgeq{\asetpath}{\inbound{+}1}}
\have {6} {\remgeq{\asetpath\cup\{\pair{\aterm_1}{\aterm_4}\}}{\inbound{+}1}} \by{\ref{core2Ax:RemTEq1}}{3,5}
\have {7} {\remgeq{\asetpath\cup\{\pair{\aterm_1}{\aterm_4},\pair{\aterm_1}{\aterm_2}\}}{\inbound{+}1}} \by{\ref{core2Ax:RemTEq2}}{3,6}
\have {8} {\remgeq{\asetpath\cup\{\pair{\aterm_1}{\aterm_2}\}}{\inbound{+}1}} \by{\ref{core2Ax:RemMono2}}{7}
 \have {9} {\bottom} \by{\landcontr}{2,8}
\close
 \have {10} {\lnot\remgeq{\asetpath}{\inbound{+}1}} \ni{5-9}
 \have {11} {\rem{\asetpath}{=}{\inbound}} \by{\ndref{4} $\land$ \ndref{10}}{}
\end{nd}
\]
\end{enumerate}
